# Supplementary material for: Towards Effective Planning Strategies for Dynamic Opinion Networks
Source: arXiv:2410.14091 source file (2024-11-03)
Supplement: Supplementary file 1 [file appendix.tex]

\section{Appendix}

\subsection{Experimental Methods}

% In our study, we investigate the problem of containing misinformation spread through two different approaches: Reinforcement Learning (RL) and Supervised Learning (SL). 

% For our study, we consider a graph as a network of interconnected agents (undirected graphs) where each node of the graph represents an agent and an edge is considered as a connection between the agents. Every agent holds an opinion value on a topic [-1,1], while the weight on the edge is considered as the mutual trust level between the connected agents [0,1]. 

In our study, we investigate the problem of containing misinformation spread through two different approaches: Reinforcement Learning (RL) and Supervised Learning (SL). Our objective is to assess and compare the effectiveness of these methodologies in controlling the dissemination of false information across a network of interconnected agents.

\paragraph{Network Model and Assumptions}

For our study, the underlying structure of the social network is conceptualized as a graph, representing a network of interconnected agents. This is further detailed as follows:

\begin{itemize}
    \item The graph is undirected, indicating that relationships between agents are bi-directional.
    \item Each node within the graph represents an individual agent. These agents are the fundamental units within our network, each holding specific opinions on a given topic.
    \item An edge between any two nodes signifies a direct connection or relationship between those agents, facilitating the flow and exchange of opinions.
    \item Opinion values held by agents are quantified within the range \([-1, 1]\).
    \item The weight assigned to an edge quantifies the mutual trust level between the connected agents, scaled within the interval \([0, 1]\).
\end{itemize}

Within this framework, we explore three distinct cases based on the type of opinion values, and trust. The opinion dynamic models considered for each case are detailed in the further sections of the appendix.

\begin{itemize}
    \item \textbf{Case-1:} Binary Opinion Values with Binary Trust Values.
    \item \textbf{Case-2:} Floating-Point Opinion Values with Binary Trust Values.
    \item \textbf{Case-3:} Floating-Point Opinion Values with Floating-Point Trust Values.
\end{itemize}

\subsubsection{Setup for RL}
All the networks that were generated while training the RL policies are modeled using the \texttt{Watts-Strogatz small-world} graph to simulate the interconnections of agents in a social network. This model captures the essence of real-world social structures with its characteristic short path lengths and high clustering coefficient. 

\paragraph{Network Configuration and Parameters}

The experiments are structured around three distinct cases, each examining different combinations of opinion values and trust levels within the network. The parameters varied across experiments include:

\begin{itemize}
    \item \textbf{Network Length:} The size of the network, measured by the number of nodes, is varied among 10, 25, and 50 nodes to understand the scale's effect on opinion dynamics.
    \item \textbf{Initial Infected Nodes:} The initial number of nodes with the 'infected' opinion. This parameter is varied as 1, 2, or 3 to assess the impact of initial opinion spread.
    \item \textbf{Action Budget:} The number of actions available for influencing network opinions, tested with 1, 2, and 3 actions to evaluate the effectiveness of intervention strategies.
    \item \textbf{Source Trust:} The level of trust in the source of information is given a fixed value of 1.
\end{itemize}

\subsubsection{Setup for SL}

In the supervised learning setup, we conducted experiments with three distinct graph structures: Watts-Strogatz small-world, Erdos-Renyi, and Tree graphs. Each graph type facilitated the training of unique models to evaluate the respective dynamics and structural influences on the performance of the models.

\paragraph{Network Configuration and Parameters} The configuration of our network for the supervised learning experiments involved the use of a Graph Convolutional Network (GCN) model. This setup bore both similarities and differences compared to the Residual Network (ResNet) model used in the reinforcement learning experiments. While using the  parameters such as network length, initial infected nodes, action budget, and source trust configurations were retained, the feature set evaluated was expanded as described below:

\begin{itemize}
    \item \textbf{Network Length:} Consistent with the reinforcement learning configuration, the networks used for training and testing in the supervised learning model comprised 10, 25, and 50 nodes.
    
    \item \textbf{Initial Infected Nodes:} We initialized the graphs with 1, 2, or 3 'infected' nodes to simulate varying levels of initial misinformation spread.

    \item \textbf{Action Budget:} The model was allowed 1, 2, or 3 actions per iteration, enabling us to assess the impact of different levels of intervention capabilities on the misinformation spread within the network.

    \item \textbf{Features:} The model incorporated three distinct features for each node within the graph:
    \begin{enumerate}
        \item \textbf{Opinion Value:} Each node possessed an opinion value within the range \([-1, 1]\). A value below \(-0.95\) indicated a highly misinformed node, prone to disseminating misinformation to adjacent nodes.
        
        \item \textbf{Degree of a Node:} This feature quantified the number of connections (or edges) a node had with others, focusing only on those connections that could potentially participate in further misinformation spread (excluding already blocked or misinformed nodes).
        
        \item \textbf{Minimal Distance from a Source Node:} Reflecting the dynamic changes in node opinions, this feature measured the shortest path from any given node to the nearest infected source node. Nodes unreachable from any infected source were assigned a distance of infinity. 
    \end{enumerate}

\end{itemize}

\begin{table}[h]
\centering
\caption{Comprehensive breakdown of experimental configurations for RL setup detailing the parameters for each of the four case scenarios investigated in the study. The table enumerates the variations in the number of nodes within the network, the range of initially 'infected' nodes, and the action count available for intervention, across different network sizes.}
\label{tab:exp-table}
\begin{tabular}{|c|c|lccccccccc|c|}
\toprule
\multicolumn{1}{|l|}{Case No.} & \multicolumn{1}{l|}{\# nodes} & \multicolumn{10}{l|}{Parameters for \# infected and \# action count}                                                                                                                                                                         & \multicolumn{1}{l|}{Source Trust} \\ \toprule
\multirow{6}{*}{Case 1}        & \multirow{2}{*}{10}           & \multicolumn{1}{l|}{\# Infected} & \multicolumn{3}{c|}{1}                                                   & \multicolumn{3}{c|}{2}                                                   & \multicolumn{3}{c|}{3}                              & \multirow{2}{*}{1.0}              \\ \cline{3-12}
                               &                               & \multicolumn{1}{l|}{\# Actions}  & \multicolumn{1}{c|}{1} & \multicolumn{1}{c|}{2} & \multicolumn{1}{c|}{3} & \multicolumn{1}{c|}{1} & \multicolumn{1}{c|}{2} & \multicolumn{1}{c|}{3} & \multicolumn{1}{c|}{1} & \multicolumn{1}{c|}{2} & 3 &                                   \\ \cline{2-13} 
                               & \multirow{2}{*}{25}           & \multicolumn{1}{l|}{\# Infected} & \multicolumn{3}{c|}{1}                                                   & \multicolumn{3}{c|}{2}                                                   & \multicolumn{3}{c|}{3}                              & \multirow{2}{*}{1.0}              \\ \cline{3-12}
                               &                               & \multicolumn{1}{l|}{\# Actions}  & \multicolumn{1}{c|}{1} & \multicolumn{1}{c|}{2} & \multicolumn{1}{c|}{3} & \multicolumn{1}{c|}{1} & \multicolumn{1}{c|}{2} & \multicolumn{1}{c|}{3} & \multicolumn{1}{c|}{1} & \multicolumn{1}{c|}{2} & 3 &                                   \\ \cline{2-13} 
                               & \multirow{2}{*}{50}           & \multicolumn{1}{l|}{\# Infected} & \multicolumn{3}{c|}{1}                                                   & \multicolumn{3}{c|}{2}                                                   & \multicolumn{3}{c|}{3}                              & \multirow{2}{*}{1.0}              \\ \cline{3-12}
                               &                               & \multicolumn{1}{l|}{\# Actions}  & \multicolumn{1}{c|}{1} & \multicolumn{1}{c|}{2} & \multicolumn{1}{c|}{3} & \multicolumn{1}{c|}{1} & \multicolumn{1}{c|}{2} & \multicolumn{1}{c|}{3} & \multicolumn{1}{c|}{1} & \multicolumn{1}{c|}{2} & 3 &                                   \\ 
                               \midrule
                               \midrule
\multirow{6}{*}{Case 2}        & \multirow{2}{*}{10}           & \multicolumn{1}{l|}{\# Infected} & \multicolumn{3}{c|}{1}                                                   & \multicolumn{3}{c|}{2}                                                   & \multicolumn{3}{c|}{3}                              & \multirow{2}{*}{1.0}              \\ \cline{3-12}
                               &                               & \multicolumn{1}{l|}{\# Actions}  & \multicolumn{1}{c|}{1} & \multicolumn{1}{c|}{2} & \multicolumn{1}{c|}{3} & \multicolumn{1}{c|}{1} & \multicolumn{1}{c|}{2} & \multicolumn{1}{c|}{3} & \multicolumn{1}{c|}{1} & \multicolumn{1}{c|}{2} & 3 &                                   \\ \cline{2-13} 
                               & \multirow{2}{*}{25}           & \multicolumn{1}{l|}{\# Infected} & \multicolumn{3}{c|}{1}                                                   & \multicolumn{3}{c|}{2}                                                   & \multicolumn{3}{c|}{3}                              & \multirow{2}{*}{1.0}              \\ \cline{3-12}
                               &                               & \multicolumn{1}{l|}{\# Actions}  & \multicolumn{1}{c|}{1} & \multicolumn{1}{c|}{2} & \multicolumn{1}{c|}{3} & \multicolumn{1}{c|}{1} & \multicolumn{1}{c|}{2} & \multicolumn{1}{c|}{3} & \multicolumn{1}{c|}{1} & \multicolumn{1}{c|}{2} & 3 &                                   \\ \cline{2-13} 
                               & \multirow{2}{*}{50}           & \multicolumn{1}{l|}{\# Infected} & \multicolumn{3}{c|}{1}                                                   & \multicolumn{3}{c|}{2}                                                   & \multicolumn{3}{c|}{3}                              & \multirow{2}{*}{1.0}              \\ \cline{3-12}
                               &                               & \multicolumn{1}{l|}{\# Actions}  & \multicolumn{1}{c|}{1} & \multicolumn{1}{c|}{2} & \multicolumn{1}{c|}{3} & \multicolumn{1}{c|}{1} & \multicolumn{1}{c|}{2} & \multicolumn{1}{c|}{3} & \multicolumn{1}{c|}{1} & \multicolumn{1}{c|}{2} & 3 &                                   \\ 

                               \midrule
                               \midrule

\multirow{6}{*}{Case 3 v1}        & \multirow{2}{*}{10}           & \multicolumn{1}{l|}{\# Infected} & \multicolumn{3}{c|}{1}                                                   & \multicolumn{3}{c|}{2}                                                   & \multicolumn{3}{c|}{3}                              & \multirow{2}{*}{1.0}              \\ \cline{3-12}
                               &                               & \multicolumn{1}{l|}{\# Actions}  & \multicolumn{1}{c|}{1} & \multicolumn{1}{c|}{2} & \multicolumn{1}{c|}{3} & \multicolumn{1}{c|}{1} & \multicolumn{1}{c|}{2} & \multicolumn{1}{c|}{3} & \multicolumn{1}{c|}{1} & \multicolumn{1}{c|}{2} & 3 &                                   \\ \cline{2-13} 
                               & \multirow{2}{*}{25}           & \multicolumn{1}{l|}{\# Infected} & \multicolumn{3}{c|}{1}                                                   & \multicolumn{3}{c|}{2}                                                   & \multicolumn{3}{c|}{3}                              & \multirow{2}{*}{1.0}              \\ \cline{3-12}
                               &                               & \multicolumn{1}{l|}{\# Actions}  & \multicolumn{1}{c|}{1} & \multicolumn{1}{c|}{2} & \multicolumn{1}{c|}{3} & \multicolumn{1}{c|}{1} & \multicolumn{1}{c|}{2} & \multicolumn{1}{c|}{3} & \multicolumn{1}{c|}{1} & \multicolumn{1}{c|}{2} & 3 &                                   \\ \cline{2-13} 
                               & \multirow{2}{*}{50}           & \multicolumn{1}{l|}{\# Infected} & \multicolumn{3}{c|}{1}                                                   & \multicolumn{3}{c|}{2}                                                   & \multicolumn{3}{c|}{3}                              & \multirow{2}{*}{1.0}              \\ \cline{3-12}
                               &                               & \multicolumn{1}{l|}{\# Actions}  & \multicolumn{1}{c|}{1} & \multicolumn{1}{c|}{2} & \multicolumn{1}{c|}{3} & \multicolumn{1}{c|}{1} & \multicolumn{1}{c|}{2} & \multicolumn{1}{c|}{3} & \multicolumn{1}{c|}{1} & \multicolumn{1}{c|}{2} & 3 &                                   \\ 
                               \midrule
                               \midrule
\multirow{6}{*}{Case 3 v2}        & \multirow{2}{*}{10}           & \multicolumn{1}{l|}{\# Infected} & \multicolumn{3}{c|}{1}                                                   & \multicolumn{3}{c|}{2}                                                   & \multicolumn{3}{c|}{3}                              & \multirow{2}{*}{1.0}              \\ \cline{3-12}
                               &                               & \multicolumn{1}{l|}{\# Actions}  & \multicolumn{1}{c|}{1} & \multicolumn{1}{c|}{2} & \multicolumn{1}{c|}{3} & \multicolumn{1}{c|}{1} & \multicolumn{1}{c|}{2} & \multicolumn{1}{c|}{3} & \multicolumn{1}{c|}{1} & \multicolumn{1}{c|}{2} & 3 &                                   \\ \cline{2-13} 
                               & \multirow{2}{*}{25}           & \multicolumn{1}{l|}{\# Infected} & \multicolumn{3}{c|}{1}                                                   & \multicolumn{3}{c|}{2}                                                   & \multicolumn{3}{c|}{3}                              & \multirow{2}{*}{1.0}              \\ \cline{3-12}
                               &                               & \multicolumn{1}{l|}{\# Actions}  & \multicolumn{1}{c|}{1} & \multicolumn{1}{c|}{2} & \multicolumn{1}{c|}{3} & \multicolumn{1}{c|}{1} & \multicolumn{1}{c|}{2} & \multicolumn{1}{c|}{3} & \multicolumn{1}{c|}{1} & \multicolumn{1}{c|}{2} & 3 &                                   \\ \cline{2-13} 
                               & \multirow{2}{*}{50}           & \multicolumn{1}{l|}{\# Infected} & \multicolumn{3}{c|}{1}                                                   & \multicolumn{3}{c|}{2}                                                   & \multicolumn{3}{c|}{3}                              & \multirow{2}{*}{1.0}              \\ \cline{3-12}
                               &                               & \multicolumn{1}{l|}{\# Actions}  & \multicolumn{1}{c|}{1} & \multicolumn{1}{c|}{2} & \multicolumn{1}{c|}{3} & \multicolumn{1}{c|}{1} & \multicolumn{1}{c|}{2} & \multicolumn{1}{c|}{3} & \multicolumn{1}{c|}{1} & \multicolumn{1}{c|}{2} & 3 &                                   \\ 
                               \bottomrule
\end{tabular}
\end{table}

%%%%%% Status Table %%%%%%%%%

\begin{table}[h!]
\centering
\caption{Status table for experiments}
\label{tab:model_comparison}
\begin{tabular}{|c|c|c|}
\hline
\textbf{Model} & \textbf{Reinforcement Learning} & \textbf{Supervised Learning} \\ \hline
\multirow{4}{*}{ResNet}  & \cellcolor{highlight}Case1    & \multirow{4}{*}{-} \\ \cline{2-2}
        & \cellcolor{highlight}Case2    &  \\ \cline{2-2}
        & \cellcolor{highlight}Case3 v1 &  \\ \cline{2-2}
        & Case3 v2 &  \\ \hline
\multirow{4}{*}{GCN}     & \cellcolor{lightorange}Case1    &  \cellcolor{highlight}Case1 \\ \cline{2-2}
        & \cellcolor{lightorange}Case2    &  \cellcolor{highlight}Case2 \\ \cline{2-2}
        & Case3 v1                      &  Case3 v1 \\ \cline{2-2}
        & Case3 v2                      &  Case3 v2 \\ \hline
\end{tabular}
\end{table}

%%%%%%%%%%%%%%%%%%%%%%%%%%%%%%%%%%%%%%%%%%%%%%%%%%%

\subsection{Data}

\subsubsection{Training Data Generation}

\paragraph{Reinforcement Learning (RL)}
The dataset for training the reinforcement learning (RL) policy was synthetically generated with a controlled set of parameters as outlined in the above section. Specifically, the networks utilized for RL training were constructed based on the \texttt{Watts-Strogatz model}, maintaining a consistent configuration with the number of nearest neighbors \(k=3\) and the rewiring probability \(p=0.4\) across all the instances. For each training episode, we generated 200 random states to ensure a diverse range of scenarios for the RL algorithm to learn from.

\paragraph{Supervised Learning (SL)} There are not many readily available dataset for this problem. But to tackle supervised learning we need to generate labeled data. To solve this challenge, we synthesize graph-based synthetic datasets the model is trained on. Concretely, for each training epoch, a graph $G$ is selected. For each node $n_i$ within $G$, we compute a node's infection propagation metric (infection rate) upon removal to identify the node whose elimination minimally impacts the infection spread throughout $G$. Denote this optimal node as $x$. The training target, $T \in \mathbb{N}^{N \times 1}$, where $N$ is the number of nodes in $G$, is constructed such that $T_i = 1$ if $i = x$, and $T_i = 0$ otherwise. This binary vector is the ground truth in training the Graph Convolutional Network (GCN) model.

The GCN's output, $O \in \mathbb{R}^{N \times 1}$, is juxtaposed against $T$, and the difference between $O$ and $T$ is assessed via the Binary Cross-Entropy (BCE) loss function, $\mathcal{L}_{BCE}(O, T)$. After the loss computation, gradient backpropagation updates the model parameters.

\subsection{Test Data Generation}

To evaluate the efficacy of our intervention strategies and the dynamics of opinion spread within networks, we generated two distinct synthetic datasets using the Watts-Strogatz model. This model was chosen for its ability to produce networks with small-world properties, such as higher clustering coefficients and short average path lengths, which are typical of social networks. The generation process utilized the NetworkX library, with specific parameters set to emulate various network complexities and initial conditions of misinformation spread.

The model parameters were set as follows for all datasets:
\begin{itemize}
\item Number of nearest neighbors (k): 3.
\item Rewiring probability (p): 0.4, indicating the probability of each edge being rewired to a new node to introduce randomness and simulate long-range connections.
\end{itemize}

\paragraph{Dataset v1}

In Dataset v1, we aimed to explore the impact of network size and the initial count of infected nodes on the spread of misinformation. The dataset specifications were as follows:
\begin{itemize}
\item Network sizes of 10, 25, and 50 nodes were selected to represent small, medium, and relatively larger networks.
\item For each network size, simulations were run with 1 (\(d1\)), 2 (\(d2\)), and 3 (\(d3\)) initially infected nodes, leading to the creation of 9 distinct datasets.
\item Each configuration was used to generate 1000 states, with the opinion values of non-infected nodes drawn from a uniform distribution ranging from -0.5 to 0.6.
\end{itemize}

\paragraph{Dataset v2}

Dataset v2 was designed to investigate the influence of the initial degree of infected nodes on misinformation spread. The degree of a node is defined as the number of unique neighbors to which it is connected. This dataset includes:
\begin{itemize}
\item Networks of 10, 25, and 50 nodes, similar to Dataset v1, to maintain consistency in comparing the effects of network size.
\item Initial infected node counts of 1, 2, and 3 for each network size, further diversified by considering initial degrees of 1, 2, 3, and 4 for the infected nodes.
\item A total of 36 datasets were generated, with 12 datasets for each network size, each comprising 1000 states.
\end{itemize}

%%%%%%%%%%%%%%%%%%%%%%%%%%%%%%%%%%%%%%%%%%%%%%%%%%

\subsection{Opinion Dynamics}
The dynamics of opinion formation and evolution within the network are governed by distinct models, delineating how agents update their opinions over time. These models are essential for understanding the mechanisms through which opinions propagate and change, influenced by the inter-agent interactions and the underlying trust framework. We detail the transition functions employed for the different cases studied:

\begin{itemize}
    \item \textbf{Case-1: Discrete Switching.} This simplistic model embodies a binary shift in opinions.

    \item \textbf{Case-2: Linear Adjustment.} The opinion of an agent $i$ at time $t+1$, denoted as $x_i(t+1)$, is updated based on its previous state $x_i(t)$ and the influence of a connected agent $k$. The adjustment is moderated by a factor $\mu_{ik}$, representing the strength of influence or trust between agents $i$ and $k$. The updated opinion is given by:
    \[x_i(t+1) = x_i(t) + \mu_{ik}(x_k(t) - x_i(t))\]
    This model encapsulates a gradual, linear adjustment of opinions over time.

    \item \textbf{Case-3:}
    \begin{enumerate}
        \item \textbf{v1: Linear Adjustment (Repeated).} Identical to Case-2, this variation also utilizes the linear adjustment model for opinion updates.
        \item \textbf{v2: DeGroot’s Propagation Model.} This model introduces a collective influence mechanism, where the opinion of agent $i$ at time $t+1$, $x_i(t+1)$, is the aggregate of the opinions of all connected agents $k$ at time $t$, weighted by $\mu_{ik}$. The model is formalized as:
        \[x_i(t+1) = \sum_{k} \mu_{ik} x_k(t)\]
        DeGroot’s model emphasizes the cumulative impact of a network’s opinion landscape on an individual’s stance, showcasing the significance of network structure and trust weights in shaping opinion dynamics.
    \end{enumerate}
\end{itemize}

Each of these models serves to elucidate the varied mechanisms by which opinions can evolve within a network, from binary switches to more nuanced, continuous updates influenced by direct interactions and collective surroundings.

At each time step:
\begin{itemize}
    \item Nodes identified as sources of misinformation (\texttt{`infected nodes'}) transmit the misinformation to their immediate neighbors following the previously detailed propagation models.
    \item  Concurrently, our intervention strategy involves selecting a subset of these neighbors (\texttt{`candidate nodes'})—constrained by an action budget—to receive credible information from a trusted source. This trusted source is characterized by a trust parameter set to 1 and an opinion value also set to 1, indicating maximum reliability and positive influence.
\end{itemize}

\paragraph{Evolution and Termination Conditions}

\begin{itemize}
    \item A node that exceeds a positive information threshold of 0.95 is considered `blocked', ceasing to interact with the misinformation spread or further disseminate positive influence. 
    \item Conversely, a node reaching an opinion level of -1 transforms into an `infected node', beginning to propagate misinformation.
    \item The simulation concludes when there are no viable `candidate nodes' for misinformation spread.
\end{itemize}

Our primary objective is to devise a learning mechanism that efficiently identifies and selects key nodes within the network. Through strategic selection, these nodes will receive positive information, aiming to counteract and contain the spread of misinformation. The effectiveness of this approach hinges on the ability to limit the dissemination of misinformation to as few nodes as possible, thereby mitigating its overall impact on the network’s opinion dynamics.
\subsection{Model}

\subsubsection{Supervised Learning}

\textbf{Graph Neural Networks (GNNs)} are advanced deep learning models tailored for handling data with a graph structure. Such models are particularly adept at processing information within complex networks by learning to synthesize node representations. These representations are derived through the aggregation and transformation of information from neighboring nodes. Specifically, the representation of a node $v_i$ in a graph $G$ is iteratively updated by integrating information from its immediate neighbors, denoted as $N(v_i)$. This process employs a propagation function $f$, parameterized by neural network weights $W$ and an activation function $\sigma$. The updated representation of a node in a multi-layered Graph Convolutional Network (GCN), as proposed in the literature, can be mathematically expressed as:

\begin{equation}
    H^{(l+1)} = \sigma\left(\tilde{D}^{-\frac{1}{2}}\tilde{A}\tilde{D}^{-\frac{1}{2}}H^{(l)}W^{(l)}\right)
\end{equation}

Here, $\tilde{A} = A + I_N$ represents the augmented adjacency matrix of the graph $G$, incorporating self-connections by adding the identity matrix $I_N$. The diagonal matrix $\tilde{D}_{ii} = \sum_j\tilde{A}_{ij}$ facilitates the normalization of $\tilde{A}$. The term $W^{(l)}$ denotes the weight matrix at layer $l$, and $\sigma(\cdot)$ is the activation function. The matrix $H^{(l)} \in \mathbb{R}^{N \times D}$ encapsulates the node features at layer $l$.

We engage with a graph comprising $N$ nodes in the application discussed. Our GCN outputs a vector $O \in \mathbb{R}^{N \times 1}$, representing the likelihood of each node $v_i \in V$ being pivotal for propagation through the network. This mechanism enables the model to figure out  significance of each node in mitigating information spread within the graph structure.

\paragraph{GCN Architecture Overview}

Our model is structured as follows: It comprises three graph convolutional layers followed by a linear layer. The architecture is designed to progressively transform the input node features into a space where the final classification (e.g., determining the likelihood of a node being pivotal in propagation minimization). 

\begin{itemize}
\item \textbf{Initial Graph Convolution:} The model begins with a graph convolutional layer (\texttt{GCNConv}), taking \texttt{input\_size} features and transforming them into a hidden representation of size \texttt{hidden\_size}. This layer is followed by a ReLU activation function.
\item \textbf{Hidden Graph Convolutional Layers:} After the initial layer, the architecture includes four  \texttt{GCNConv} layers, all utilizing \texttt{hidden\_size} units. These layers are designed to iteratively process and refine the features extracted from the graph's structure. Each of these layers is followed by a ReLU activation to introduce non-linearity.
\begin{itemize}
\item The model employs repeated application of the \texttt{GCNConv} layer with \texttt{hidden\_size} units, demonstrating the capacity to deepen the network's understanding of the graph's topology through successive transformations.
\end{itemize}
\item \textbf{Output Graph Convolution:} A final \texttt{GCNConv} layer reduces the hidden representation to the desired \texttt{num\_classes}, preparing the features for the prediction task.
\item \textbf{Linear Layer and Sigmoid Activation:} The architecture concludes with a linear transformation (\texttt{nn.Linear}) directly mapping the output of the last \texttt{GCNConv} layer to \texttt{num\_classes}. A sigmoid activation function is applied to this output, producing probabilities for each class in a binary classification scenario.
\end{itemize}

In this specific implementation, the \texttt{input\_size} is set to 3, indicative of the initial feature dimensionality per node. The \texttt{hidden\_size} is configured at 128, providing a substantial feature space for intermediate representations. Lastly, the \texttt{num\_classes} is established at 1, signifying only one numerical output for each nodes.

% For the section of your paper that discusses the implementation of supervised learning models, especially those involving graph convolutional networks, you could structure the information about the used Python packages in a similar way to your ResNet model description. Here's a suggestion on how to present it:

\paragraph{Packages Used} The development of our supervised learning models, particularly those utilizing graph convolutional networks, leveraged several Python packages instrumental in defining, training, and evaluating our models. Below is a list of these packages and a brief description of their roles in our implementation:

\begin{itemize}
\item \texttt{torch}: Serves as the foundational framework for constructing and training various neural network models, including those for graph-based data.
\item \texttt{torch\_geometric}: An extension of PyTorch tailored for graph neural networks. It provides efficient data structures for graphs and a collection of methods for graph convolutional operations, making it essential for implementing graph convolutional neural networks (GCNs).
\item \texttt{networkx}: Utilized for generating and manipulating complex networks. In our project, \texttt{networkx} is primarily used for creating synthetic graph data and for preprocessing tasks that require graph analysis and manipulations before feeding the data into the neural network models.
\end{itemize}

\subsubsection{Reinforcement Learning}
\paragraph{ResNet Architecture}
The Residual Network (ResNet) model implemented in our study is a variant of the conventional ResNet architecture. The core component of our ResNet model is the \textbf{ResidualBlock}, which allows for the training of deeper networks by addressing the vanishing gradient problem through skip connections. Each \textbf{ResidualBlock} consists of two sequences of convolutional layers (\texttt{Conv2d}), batch normalization (\texttt{BatchNorm2d}), and sigmoid activations. A distinctive feature is the adaptation of the skip connection to include a convolutional layer and batch normalization if there is a discrepancy in the input and output channels or the stride is not equal to one.

\paragraph{ResNet Architecture Overview}
\begin{itemize}
    \item \textbf{Initial Convolution:} Begins with a convolutional layer applying 64 filters of size 3x3, followed by batch normalization and sigmoid activation.
    \item \textbf{Residual Blocks:} Three main layers (\texttt{layer1}, \texttt{layer2}, \texttt{layer3}) constructed with the \texttt{\_make\_layer} method. Each layer contains a sequence of \textbf{ResidualBlocks}, with channel sizes of 32, 64, and 128, respectively. The number of blocks per layer is determined by the \texttt{num\_blocks} parameter.
        \begin{itemize}
            \item Each \textbf{ResidualBlock} implements two sequences of convolutional operations, batch normalization, and sigmoid activation, with an optional convolution in the shortcut connection for channel or stride adjustments.
        \end{itemize}
    \item \textbf{Adaptive Input Reshaping:} Inputs are dynamically reshaped to a square form based on the square root of the second dimension, ensuring compatibility with different input sizes.
    \item \textbf{Pooling and Output Layer:} Concludes with an average pooling layer to reduce spatial dimensions, followed by a fully connected layer mapping 128 features to a single output, thus producing the final prediction.
\end{itemize}

\paragraph{Training Details}
Our model is trained using the PyTorch library, leveraging its comprehensive suite of neural network tools and functions. The optimizer of choice is the Adam optimizer (\texttt{torch.optim.Adam}), selected for its adaptive learning rate properties, which helps in converging faster. The learning rate was set to $0.0005$, balancing the trade-off between training speed and the risk of overshooting minimal loss values. The training process involved the iterative adjustment of weights through backpropagation, minimizing the loss calculated at the output layer. This procedure was executed repeatedly over batches of training data, with the model parameters updated in each iteration to reduce the prediction error.

\paragraph{Packages Used}
The implementation of our ResNet model and the training process was facilitated by the following Python packages:
\begin{itemize}
    \item \texttt{torch}: Provides the core framework for defining and training neural networks.
    \item \texttt{torch.nn}: A submodule of PyTorch that contains classes and methods specifically designed for building neural networks.
    \item \texttt{torch.nn.functional}: Offers functional interfaces for operations used in building neural networks, like activations and pooling functions.
    \item \texttt{torch.optim}: Contains optimizers such as Adam, which are used for updating model parameters during training.
\end{itemize}

% ----------------------

% Definitions of ResNet and GCN (with details about layers, size, Input and Output) Architecture

% Training details - like Packages used (optimizer etc)

% Mention the packages used for these specifications - be detailed

\subsection{Metrics}

\paragraph{Training Loss}
\begin{itemize}
    \item \textbf{RL}: The training loss for our model is computed using the Mean Squared Error (MSE) metric. In each episode, the loss is calculated across a batch of samples drawn from the replay buffer. Specifically, it measures the squared difference between the predicted value function of the current state from the policy network and the Bellman target — the observed reward plus the value of the subsequent state as estimated by the target network. Executing this calculation over batches of experiences allows the policy network to learn from a diverse set of state transitions, thereby refining its predictions to better approximate the true expected rewards through temporal difference learning.
    
    \item \textbf{SL}: In the Supervised Learning (SL) framework, for our study, we employed the Binary Cross Entropy (BCE) loss to train the Graph Convolutional Network (GCN) model. Here, we delineate the iterative process used during the training phase under this setting. The model is fed with a new graph state at the beginning of each iteration. The GCN produces an output vector $O \in [0,1]^{N \times 1}$, where $N$ is the number of nodes in the graph. Each component of O, denoted as $O_i$, represents the probability that node $i$ should be blocked to minimize the propagation rate in the network. A greedy algorithm is employed to ascertain the optimal node to block. For each node $i$, temporarily set the node as blocked. We compute the propagation rate of the network with node $i$ blocked. Then, we revert the blockage of node $i$ and proceed to evaluate the next node. We select the node that, when blocked, results in the lowest propagation rate across the network. Upon determining the node $j$, which yields the minimum propagation rate when blocked, a target vector $T \in {0,1}^{N \times 1}$ is constructed such that $T_j = 1$ (indicating the target node to block), and $T_i = 0$ for all $i \neq j$.

    The BCE loss between the output vector $O$ and the target vector $T$ is computed as follows:

    \begin{align*}
        \text{BCE Loss} = -\frac{1}{N} \sum_{i=1}^{N} \left[ T_i \log(O_i) + (1-T_i) \log(1-O_i) \right]
    \end{align*}

    The Binary Cross Entropy (BCE) loss is particularly useful in this context because it measures the performance of the model in terms of how effectively it can predict the binary outcome (block/no block) for each node in the graph. Unlike our reinforcement learning setup, which utilizes batch updates across multiple states or episodes, the supervised learning approach updates the model weights based on the loss calculated from a single graph state per iteration.

\end{itemize}

\paragraph{Reward Functions for RL setup}

The reward function is designed to encourage policies that effectively mitigate the spread of misinformation. It includes components that penalize the increase in misinformation spread, the number of candidate nodes considered for selection, and rewards strategies that minimize the total time to contain misinformation. Specifically, the reward functions used are:

\begin{itemize}
    \item $R_0 = -(\Delta \text{infection rate})$
    \begin{itemize}
        \item Encourages the model to reduce the rate at which the misinformation spreads by penalizing increases in infection rate.
    \end{itemize}
    \item $R_1 = -(\text{\# candidate nodes})$
    \begin{itemize}
        \item Candidate nodes are the immediate neighbors of the infected nodes which are susceptible to infection in the next timestep. By penalizing the number of these candidate nodes, the reward function incentivizes strategies that result in fewer susceptible nodes at each step, thereby indirectly encouraging the containment of misinformation to a smaller subset of the network.
    \end{itemize}
    \item $R_2 = -(\text{\# candidate nodes}) - (\Delta \text{infection rate})$
    \begin{itemize}
        \item Combines the penalties for both a high number of candidate nodes and increases in infection rate to balance efficiency with efficacy in mitigating spread.
    \end{itemize}
    \item $R_3 = 1 - (\frac{\text{\# time steps}}{\text{Total time steps}})$
    \begin{itemize}
        \item Rewards quicker resolutions by assigning higher rewards for solutions that require fewer time steps, incentivizing the model to contain misinformation rapidly.
    \end{itemize}
    \item $R_4 = -(\text{infection rate})$
    \begin{itemize}
        \item Directly penalizes the current infection rate, driving the model to favor actions that result in lower overall infection rates.
    \end{itemize}
\end{itemize}

\paragraph{Infection Rate}
The infection rate measures the proportion of the network that is infected over time and is a crucial metric for evaluating the spread of misinformation within a simulated environment. It is calculated as the ratio of infected nodes to the total number of nodes within the network at a given timestep:
\[
\text{Infection Rate} = \frac{\text{Number of Infected Nodes}}{\text{Total Number of Nodes}}
\]
This metric serves not only as a means to understand the dynamics of misinformation spread during simulations but also as a vital testing metric for evaluating model performance on test datasets. Models that effectively contain or reduce the infection rate are considered to have performed well, as they demonstrate the ability to mitigate the spread of misinformation across the network.

\subsection{Supervised Learning}

\paragraph{Training Methodology:} The supervised learning training process can be summarized as follows:

\begin{itemize}
    \item \textbf{Initialize the Graph: } Start iteration with a graph in a new state or a completely new graph. 

    \item \textbf{Generate Output: } Use the GCN model to produce an output vector where each element represents the likelihood of a node needing to be blocked to control propagation.

    \item \textbf{Select the Best Node: } 
    \begin{enumerate}
        \item Temporarily block one node at a time and calculate how this affects the spread (propagation rate) throughout the network.
        \item Unblock the node and repeat for all nodes.
        \item Identify which node, when blocked, offers the most significant reduction in propagation.
    \end{enumerate}

    \item \textbf{Create Target Vector: } We construct a target vector that identifies the optimal node to block (1 for the target node, 0 for others). 

    \item \textbf{Calculate Loss:} Then we ompute the Binary Cross Entropy (BCE) loss, which measures the difference between the GCN’s predictions and the correct targets (from the target vector).

    \item \textbf{Update the Model:} Use the calculated loss to update the model’s parameters, aiming to reduce prediction errors in future iterations.

    \item  \textbf{Repeat: } Continue this process iteratively to refine the model’s predictions, cycling through the graph states and improving the strategy for blocking nodes. For a single graph we do this process until there are nodes which can be blocked to stop propagation or we take a completely new graph to repeat the process. 
\end{itemize}

\paragraph{Comparative Models } In this section, we detail the experiments conducted to evaluate the efficacy of our supervised learning model by comparing it with three alternative models. Each model adopts a distinct node selection strategy to mitigate propagation in the network. These models were selected to highlight different strategies and their impacts on managing propagation through the network. By comparing these models, we aim to demonstrate the superiority of our GCN-based approach, particularly in terms of its strategic adaptability and learning efficacy. Here are brief descriptions of these comparative models: 

\begin{itemize}
    \item \textbf{Randomized Policy Model: } This model operates under a non-deterministic approach, where it selects nodes to block at random from the set of uninfected or unblocked nodes in each iteration. 

    \item \textbf{Max Degree Policy Model (Static):} This strategy involves blocking the node with the highest degree (i.e., the node with the most connections) that is still available for blocking. The selection is based solely on the initial graph structure, ignoring any changes to the network topology or node status in subsequent iterations. It provides a heuristic benchmark, leveraging the assumption that highly connected nodes, if blocked, can significantly impede overall propagation.

    \item \textbf{Max Degree Policy Model (Dynamic): } Similar to the static version, this model focuses on the node with the highest degree. However, it dynamically recalculates the degrees in each iteration, considering only the uninfected or unblocked nodes. This adaptation allows the model to respond to the evolving network state, potentially improving the blocking strategy as the simulation progresses.
    
\end{itemize}

Following are the different experiments we have tried with our supervised learning-based model.

\paragraph{Case-1}
\begin{itemize}
    \item \textbf{Type:} Binary Opinion and Binary Trust.
    \item \textbf{Opinion Dynamic Model:} Discrete Switching.
\end{itemize}

\paragraph{Inference on Different Types of Networks: } 

\begin{longtable}[c]{|c|ccc|}
\caption{Inference Results on Different Datasets for Case 1}
\label{tab:Case1_SL}\\
\hline
\multirow{2}{*}{\textbf{Number of Nodes Datasets}} &
  \multicolumn{3}{c|}{\textbf{Datasets}} \\ \cline{2-4} 
 & \multicolumn{1}{c|}{\textbf{Watts-Strogatz Network}} & \multicolumn{1}{c|}{\textbf{Tree}} & \textbf{\begin{tabular}[c]{@{}c@{}}Erdos-Renyi Net\\ work\end{tabular}} \\ \hline
\endfirsthead
\multicolumn{4}{c}%
{{\bfseries Table \thetable\ continued from previous page}} \\
\hline
\multirow{2}{*}{\textbf{Number of Nodes Datasets}} &
  \multicolumn{3}{c|}{\textbf{Datasets}} \\ \cline{2-4} 
 & \multicolumn{1}{c|}{\textbf{Watts-Strogatz Network}} & \multicolumn{1}{c|}{\textbf{Tree}} & \textbf{\begin{tabular}[c]{@{}c@{}}Erdos-Renyi Net\\ work\end{tabular}} \\ \hline
\endhead
10 &
  \multicolumn{1}{c|}{Figure \ref{fig:c1n10}} &
  \multicolumn{1}{c|}{Figure \ref{fig:Treec1n10}} &
  {Figure \ref{fig:ERc1n10}} \\ \hline
25 &
  \multicolumn{1}{c|}{Figure \ref{fig:c1n25}} &
  \multicolumn{1}{c|}{Figure \ref{fig:Treec1n25}} &
  {Figure \ref{fig:ERc1n25}} \\ \hline
50 &
  \multicolumn{1}{c|}{Figure \ref{fig:c1n50}} &
  \multicolumn{1}{c|}{Figure \ref{fig:Treec1n50}} &
  {Figure \ref{fig:ERc1n50}} \\ \hline
\end{longtable}

\paragraph{Case-2}

\begin{itemize}
    \item \textbf{Type:} Floating-point Opinion and Binary Trust.
    \item \textbf{Opinion Dynamic Model:} Discrete Switching.
\end{itemize}

\paragraph{Inference on Different Types of Networks: }

\begin{longtable}[c]{|c|ccc|}
\caption{Inference Results on Different Datasets for Case 2}
\label{tab:Case2_SL}\\
\hline
\multirow{2}{*}{\textbf{Number of Nodes Datasets}} &
  \multicolumn{3}{c|}{\textbf{Datasets}} \\ \cline{2-4} 
 & \multicolumn{1}{c|}{\textbf{Watts-Strogatz Network}} & \multicolumn{1}{c|}{\textbf{Tree}} & \textbf{\begin{tabular}[c]{@{}c@{}}Erdos-Renyi Net\\ work\end{tabular}} \\ \hline
\endfirsthead
\multicolumn{4}{c}%
{{\bfseries Table \thetable\ continued from previous page}} \\
\hline
\multirow{2}{*}{\textbf{Number of Nodes Datasets}} &
  \multicolumn{3}{c|}{\textbf{Datasets}} \\ \cline{2-4} 
 & \multicolumn{1}{c|}{\textbf{Watts-Strogatz Network}} & \multicolumn{1}{c|}{\textbf{Tree}} & \textbf{\begin{tabular}[c]{@{}c@{}}Erdos-Renyi Net\\ work\end{tabular}} \\ \hline
\endhead
10 &
  \multicolumn{1}{c|}{Figure \ref{fig:c2n10}} &
  \multicolumn{1}{c|}{Figure \ref{fig:Treec2n10}} &
  {Figure \ref{fig:ERc2n10}} \\ \hline
25 &
  \multicolumn{1}{c|}{Figure \ref{fig:c2n25}} &
  \multicolumn{1}{c|}{Figure \ref{fig:Treec2n25}} &
  {Figure \ref{fig:ERc2n25}} \\ \hline
50 &
  \multicolumn{1}{c|}{Figure \ref{fig:c2n50}} &
  \multicolumn{1}{c|}{Figure \ref{fig:Treec2n50}} &
  {Figure \ref{fig:ERc2n50}} \\ \hline
\end{longtable}

\paragraph{Case-3}

\begin{itemize}
    \item \textbf{Type:} Floating-point Opinion and Floating-point Trust.
    \item \textbf{Opinion Dynamic Model:} Linear Adjustment. 
\end{itemize}

\paragraph{Inference on Different Types of Networks: }

\begin{longtable}[c]{|c|ccc|}
\caption{Inference Results on Different Datasets for Case 3}
\label{tab:Case3_SL}\\
\hline
\multirow{2}{*}{\textbf{Number of Nodes Datasets}} &
  \multicolumn{3}{c|}{\textbf{Datasets}} \\ \cline{2-4} 
 & \multicolumn{1}{c|}{\textbf{Watts-Strogatz Network}} & \multicolumn{1}{c|}{\textbf{Tree}} & \textbf{\begin{tabular}[c]{@{}c@{}}Erdos-Renyi Net\\ work\end{tabular}} \\ \hline
\endfirsthead
\multicolumn{4}{c}%
{{\bfseries Table \thetable\ continued from previous page}} \\
\hline
\multirow{2}{*}{\textbf{Number of Nodes Datasets}} &
  \multicolumn{3}{c|}{\textbf{Datasets}} \\ \cline{2-4} 
 & \multicolumn{1}{c|}{\textbf{Watts-Strogatz Network}} & \multicolumn{1}{c|}{\textbf{Tree}} & \textbf{\begin{tabular}[c]{@{}c@{}}Erdos-Renyi Net\\ work\end{tabular}} \\ \hline
\endhead
10 &
  \multicolumn{1}{c|}{Figure \ref{fig:c3n10}} &
  \multicolumn{1}{c|}{Figure \ref{fig:Treec3n10}} &
  {Figure \ref{fig:ERc3n10}} \\ \hline
25 &
  \multicolumn{1}{c|}{Figure \ref{fig:c3n25}} &
  \multicolumn{1}{c|}{Figure \ref{fig:Treec3n25}} &
  {Figure \ref{fig:ERc3n25}} \\ \hline
50 &
  \multicolumn{1}{c|}{Figure \ref{fig:c3n50}} &
  \multicolumn{1}{c|}{Figure \ref{fig:Treec3n50}} &
  {Figure \ref{fig:ERc3n50}} \\ \hline
\end{longtable}

\subsection{Reinforcement Learning}
\paragraph{Training Methodology:}
The Neural Network model is trained using a variant of Q-learning, with a replay buffer approach to stabilize the learning process, aimed at learning the value function. Training commences with a fully exploratory policy (epsilon = 1) and transitions to an exploitation-focused strategy as epsilon decays over time. The learning rate is set to \(5 \times 10^{-4}\), and mean squared error (MSE) loss is utilized to measure the prediction quality.

At each episode, \texttt{200} random initial states are generated, with a selected parameter of the number of initially infected nodes, and actions are determined through an epsilon-greedy method, balancing between exploration and exploitation. The agent performs actions by selecting nodes in the network to effectively contain misinformation spread. For each action, the network's new state and corresponding reward are observed, which are then stored in the replay buffer. 

Batch updates are carried out by sampling from this buffer, ensuring that learning occurs across a diverse set of state-action-reward-next-state tuples. We have used a batch-size of \texttt{100} across the experiments. The policy network parameters are optimized using the Adam optimizer, and the target network's parameters are periodically updated to reflect the policy network, reducing the likelihood of divergence.

The training process continues for \texttt{300} number of episodes, with the epsilon parameter decaying after each timestep within an episode, encouraging the model to rely more on learned values rather than random actions as training progresses. The duration of each episode and overall training, along with average rewards and loss, are logged for post-training analysis. The model parameters yielding the best performance on the validation set are preserved for subsequent evaluation phases.
%%%%%%%%%%% ResNet - RL %%%%%%%%%%%%%%%%%%%%
\subsubsection{ResNet}

\subsubsubsection{Case-1} 

\begin{itemize}
    \item \textbf{Type:} Binary Opinion and Binary Trust.
    \item \textbf{Opinion Dynamic Model:} Discrete Switching.
\end{itemize}

\paragraph{R0}
\begin{itemize}
    \item The loss plot is presented in Figure \ref{fig:resnet_c1r0_loss}.
    \item Dataset v1 Inference Result: 10 Nodes - Figure \ref{fig:inf_resnet_c1r0_10}.
    \item Dataset v1 Inference Result: 25 Nodes - Figure \ref{fig:inf_resnet_c1r0_25}.
    \item Dataset v1 Inference Result: 50 Nodes - Figure \ref{fig:inf_resnet_c1r0_50}.
\end{itemize}

\paragraph{R1}
\begin{itemize}
    \item The loss plot is presented in Figure \ref{fig:resnet_c1r1_loss}.
    \item Dataset v1 Inference Result: 10 Nodes - Figure \ref{fig:inf_resnet_c1r1_10}.
    \item Dataset v1 Inference Result: 25 Nodes - Figure \ref{fig:inf_resnet_c1r1_25}.
    \item Dataset v1 Inference Result: 50 Nodes - Figure \ref{fig:inf_resnet_c1r1_50}.
\end{itemize}

\paragraph{R2}
\begin{itemize}
    \item The loss plot is presented in Figure \ref{fig:resnet_c1r2_loss}.
    \item Dataset v1 Inference Result: 10 Nodes - Figure \ref{fig:inf_resnet_c1r2_10}.
    \item Dataset v1 Inference Result: 25 Nodes - Figure \ref{fig:inf_resnet_c1r2_25}.
    \item Dataset v1 Inference Result: 50 Nodes - Figure \ref{fig:inf_resnet_c1r2_50}.
\end{itemize}

\paragraph{R3}
\begin{itemize}
    \item The loss plot is presented in Figure \ref{fig:resnet_c1r3_loss}.
    \item Dataset v1 Inference Result: 10 Nodes - Figure \ref{fig:inf_resnet_c1r3_10}.
    \item Dataset v1 Inference Result: 25 Nodes - Figure \ref{fig:inf_resnet_c1r3_25}.
    \item Dataset v1 Inference Result: 50 Nodes - Figure \ref{fig:inf_resnet_c1r3_50}.
\end{itemize}

\paragraph{R4}
\begin{itemize}
    \item The loss plot is presented in Figure \ref{fig:resnet_c1r4_loss}.
    \item Dataset v1 Inference Result: 10 Nodes - Figure \ref{fig:inf_resnet_c1r4_10}.
    \item Dataset v1 Inference Result: 25 Nodes - Figure \ref{fig:inf_resnet_c1r4_25}.
    \item Dataset v1 Inference Result: 50 Nodes - Figure \ref{fig:inf_resnet_c1r4_50}.
\end{itemize}

%%%%%%%%%%%%%%%%%%%%%%%%%%%%%%%%%%%%%%%%%%%%

\paragraph{Case-2}
\begin{itemize}
    \item \textbf{Type:} Floating Point Opinion and Binary Trust.
    \item \textbf{Opinion Dynamic Model:} Linear Adjustment.
\end{itemize}

\paragraph{R0}
\begin{itemize}
    \item The loss plot is presented in Figure \ref{fig:resnet_c2r0_loss}.
    \item Dataset v1 Inference Result: 10 Nodes - Figure \ref{fig:inf_resnet_c2r0_10}.
    \item Dataset v1 Inference Result: 25 Nodes - Figure \ref{fig:inf_resnet_c2r0_25}.
    \item Dataset v1 Inference Result: 50 Nodes - Figure \ref{fig:inf_resnet_c2r0_50}.
\end{itemize}

\paragraph{R1}
\begin{itemize}
    \item The loss plot is presented in Figure \ref{fig:resnet_c2r1_loss}.
    \item Dataset v1 Inference Result: 10 Nodes - Figure \ref{fig:inf_resnet_c2r1_10}.
    \item Dataset v1 Inference Result: 25 Nodes - Figure \ref{fig:inf_resnet_c2r1_25}.
    \item Dataset v1 Inference Result: 50 Nodes - Figure \ref{fig:inf_resnet_c2r1_50}.
\end{itemize}

\paragraph{R2}
\begin{itemize}
    \item The loss plot is presented in Figure \ref{fig:resnet_c2r2_loss}.
    \item Dataset v1 Inference Result: 10 Nodes - Figure \ref{fig:inf_resnet_c2r2_10}.
    \item Dataset v1 Inference Result: 25 Nodes - Figure \ref{fig:inf_resnet_c2r2_25}.
    \item Dataset v1 Inference Result: 50 Nodes - Figure \ref{fig:inf_resnet_c2r2_50}.
\end{itemize}

\paragraph{R3}
\begin{itemize}
    \item The loss plot is presented in Figure \ref{fig:resnet_c2r3_loss}.
    \item Dataset v1 Inference Result: 10 Nodes - Figure \ref{fig:inf_resnet_c2r3_10}.
    \item Dataset v1 Inference Result: 25 Nodes - Figure \ref{fig:inf_resnet_c2r3_25}.
    \item Dataset v1 Inference Result: 50 Nodes - Figure \ref{fig:inf_resnet_c2r3_50}.
\end{itemize}

\paragraph{R4}
\begin{itemize}
    \item The loss plot is presented in Figure \ref{fig:resnet_c2r4_loss}.
    \item Dataset v1 Inference Result: 10 Nodes - Figure \ref{fig:inf_resnet_c2r4_10}.
    \item Dataset v1 Inference Result: 25 Nodes - Figure \ref{fig:inf_resnet_c2r4_25}.
    \item Dataset v1 Inference Result: 50 Nodes - Figure \ref{fig:inf_resnet_c2r4_50}.
\end{itemize}

%%%%%%%%%%%%%%%%%%%%%%%%%%%%%%%%%%%%%%%%%%%%%%%%

\paragraph{Case-3}

\paragraph{v1}
    
\begin{itemize}
    \item \textbf{Type:} Floating Point Opinion and Floating Point Trust.
    \item \textbf{Opinion Dynamic Model:} Linear Adjustment.
\end{itemize}

\paragraph{R0}
\begin{itemize}
    \item The loss plot is presented in Figure \ref{fig:resnet_c3v1r0_loss}.
    \item Dataset v1 Inference Result: 10 Nodes - Figure -.
    \item Dataset v1 Inference Result: 25 Nodes - Figure \ref{fig:inf_resnet_c3v1r0_25}.
    \item Dataset v1 Inference Result: 50 Nodes - Figure \ref{fig:inf_resnet_c3v1r0_50}.
\end{itemize}

\paragraph{R1}
\begin{itemize}
    \item The loss plot is presented in Figure \ref{fig:resnet_c3v1r1_loss}.
    \item Dataset v1 Inference Result: 10 Nodes - Figure \ref{fig:inf_resnet_c3v1r1_10}.
    \item Dataset v1 Inference Result: 25 Nodes - Figure \ref{fig:inf_resnet_c3v1r1_25}.
    \item Dataset v1 Inference Result: 50 Nodes - Figure \ref{fig:inf_resnet_c3v1r1_50}.
\end{itemize}

\paragraph{R2}
\begin{itemize}
    \item The loss plot is presented in Figure \ref{fig:resnet_c3v1r2_loss}.
    \item Dataset v1 Inference Result: 10 Nodes - Figure \ref{fig:inf_resnet_c3v1r2_10}.
    \item Dataset v1 Inference Result: 25 Nodes - Figure \ref{fig:inf_resnet_c3v1r2_25}.
    \item Dataset v1 Inference Result: 50 Nodes - Figure \ref{fig:inf_resnet_c3v1r2_50}.
\end{itemize}

\paragraph{R3}
\begin{itemize}
    \item The loss plot is presented in Figure \ref{fig:resnet_c3v1r3_loss}.
    \item Dataset v1 Inference Result: 10 Nodes - Figure \ref{fig:inf_resnet_c3v1r3_10}.
    \item Dataset v1 Inference Result: 25 Nodes - Figure \ref{fig:inf_resnet_c3v1r3_25}.
    \item Dataset v1 Inference Result: 50 Nodes - Figure \ref{fig:inf_resnet_c3v1r3_50}.
\end{itemize}

\paragraph{R4}
\begin{itemize}
    \item The loss plot is presented in Figure \ref{fig:resnet_c3v1r4_loss}.
    \item Dataset v1 Inference Result: 10 Nodes - Figure \ref{fig:inf_resnet_c3v1r4_10}.
    \item Dataset v1 Inference Result: 25 Nodes - Figure \ref{fig:inf_resnet_c3v1r4_25}.
    \item Dataset v1 Inference Result: 50 Nodes - Figure \ref{fig:inf_resnet_c3v1r4_50}.
\end{itemize}

% ###################################

\paragraph{v2}
\begin{itemize}
    \item \textbf{Type:} Floating Point Opinion and Floating Point Trust.
    \item \textbf{Opinion Dynamic Model:} DeGroot's Propagation Model.
\end{itemize}

\paragraph{R0}
\paragraph{R1}
\paragraph{R2}
\paragraph{R3}
\paragraph{R4}

%%%%%%%%%%% GCN - RL %%%%%%%%%%%%%%%%%%%%
\subsubsection{GCN}
\subsubsubsection{Case-1} 

\begin{itemize}
    \item \textbf{Type:} Binary Opinion and Binary Trust.
    \item \textbf{Opinion Dynamic Model:} Discrete Switching.
\end{itemize}

\paragraph{R0}
The loss plot is presented in Figure \ref{fig:gcn_c1r0_loss}.

\paragraph{R1}
The loss plot is presented in Figure \ref{fig:gcn_c1r1_loss}.

\paragraph{R2}
The loss plot is presented in Figure \ref{fig:gcn_c1r2_loss}.

\paragraph{R3}
The loss plot is presented in Figure \ref{fig:gcn_c1r3_loss}.

\paragraph{R4}
The loss plot is presented in Figure \ref{fig:gcn_c1r4_loss}.

%%%%%%%%%%%%%%%%%%%%%%%%%%%%%%%%%%%%%%%%%%%%

\paragraph{Case-2}
\begin{itemize}
    \item \textbf{Type:} Floating Point Opinion and Binary Trust.
    \item \textbf{Opinion Dynamic Model:} Linear Adjustment.
\end{itemize}

\paragraph{R0}
The loss plot is presented in Figure \ref{fig:gcn_c2r0_loss}.

\paragraph{R1}
The loss plot is presented in Figure \ref{fig:gcn_c2r1_loss}.

\paragraph{R2}
The loss plot is presented in Figure \ref{fig:gcn_c2r2_loss}.

\paragraph{R3}
The loss plot is presented in Figure \ref{fig:gcn_c2r3_loss}.

\paragraph{R4}
The loss plot is presented in Figure \ref{fig:gcn_c2r4_loss}.

%%%%%%%%%%%%%%%%%%%%%%%%%%%%%%%%%%%%%%%%%%%%%%%%

\paragraph{Case-3}

\paragraph{v1}
    
\begin{itemize}
    \item \textbf{Type:} Floating Point Opinion and Floating Point Trust.
    \item \textbf{Opinion Dynamic Model:} Linear Adjustment.
\end{itemize}

\paragraph{R0}
\paragraph{R1}
\paragraph{R2}
\paragraph{R3}
\paragraph{R4}
% ###################################

\paragraph{v2}
\begin{itemize}
    \item \textbf{Type:} Floating Point Opinion and Floating Point Trust.
    \item \textbf{Opinion Dynamic Model:} DeGroot's Propagation Model.
\end{itemize}

\paragraph{R0}
\paragraph{R1}
\paragraph{R2}
\paragraph{R3}
\paragraph{R4}

% ##############################################################
% ######################## Figures Below #######################
% ##############################################################

% ######################################
% ################ SL ##################
% ######################################

%%%%%%%%%%%% Figures %%%%%%%%%%%%%

% ###### Case 1 ##########

\begin{figure}[!h]
    \centering
    \includegraphics[scale=0.3]{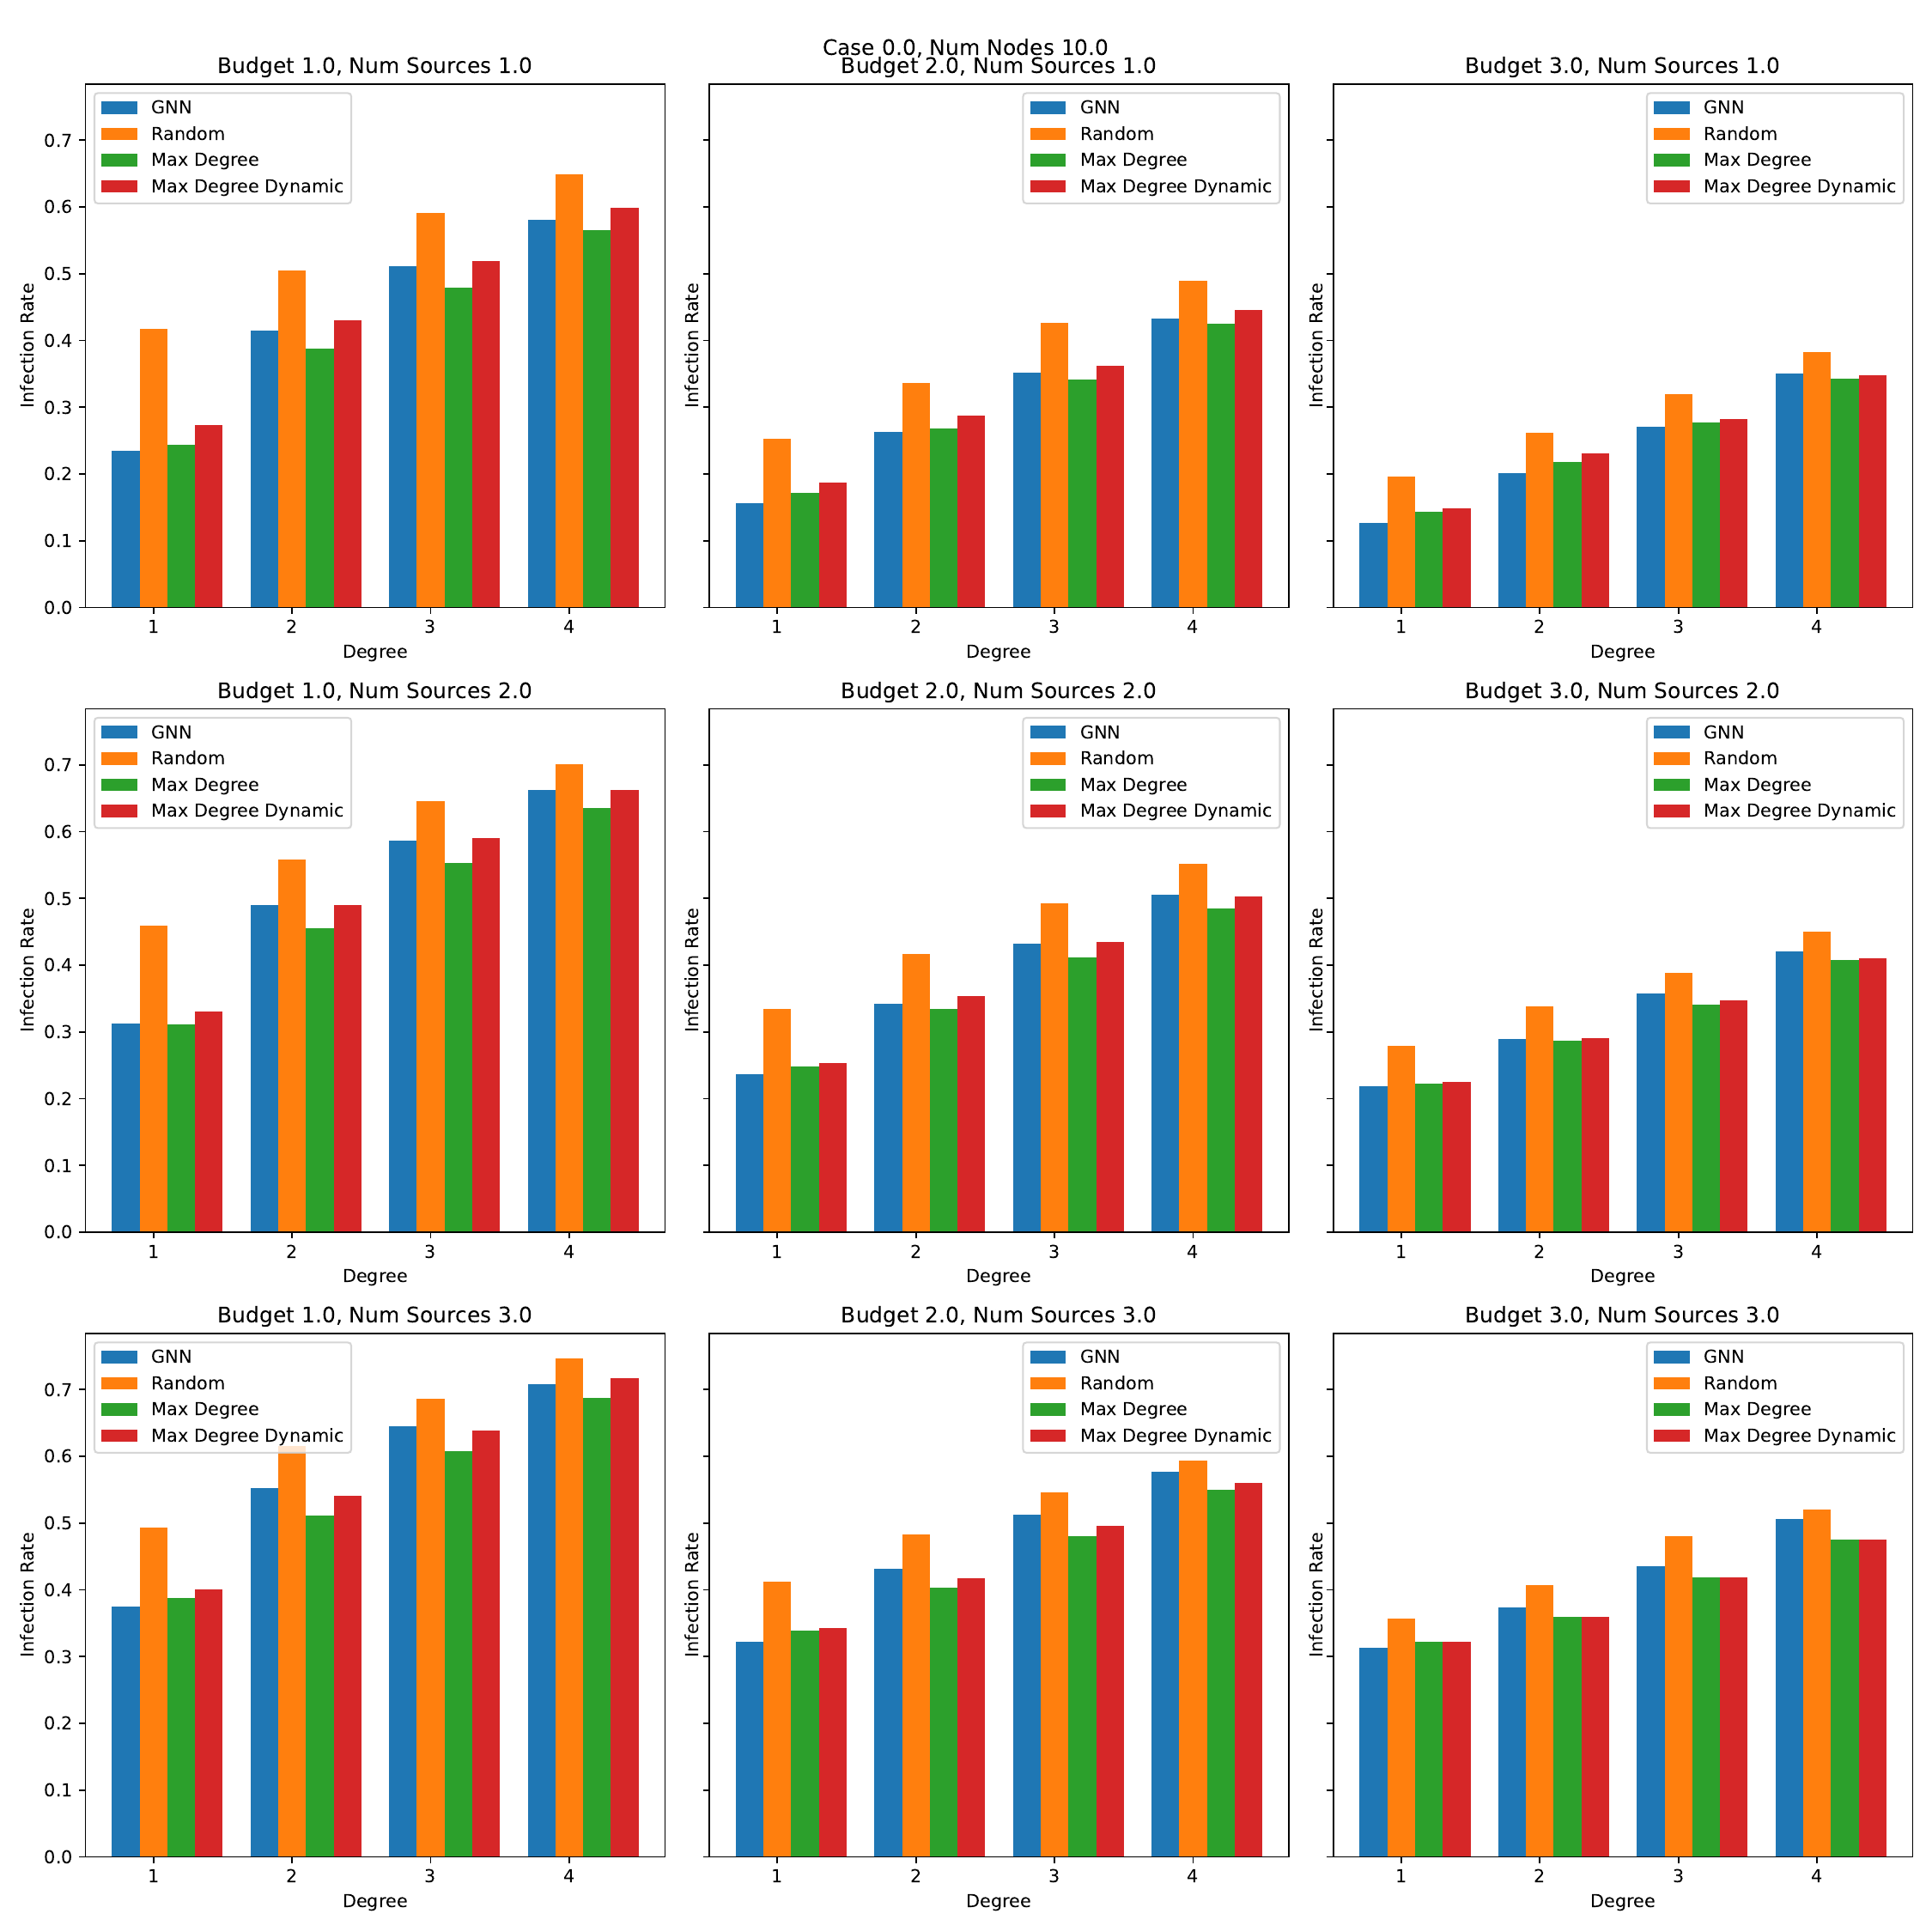}
    \caption{\footnotesize Dataset: Watts-Strogatz, Case-1 Node-10: Performance Evaluation of GCN-Based Supervised Learning Model: This series of bar plots presents a comparative analysis between our GCN-based SL model (blue), Randomized Policy model(yellow), Max Degree Policy model (Static) (green) and Max Degree Policy model (Dynamic) (red) on 10-node network environment. Progressing from left to right, the plots depict scenarios with increasing action budgets, ranging from 1 to 3 actions permitted. Vertically, the plots are ordered to show the effect of varying the initial count of infected nodes, starting with one and increasing to three. Each set of bars within the plots is categorized by the average connectivity (degree) of the infected nodes.}
    \label{fig:c1n10}
\end{figure}

\begin{figure}[!h]
    \centering
    \includegraphics[scale=0.3]{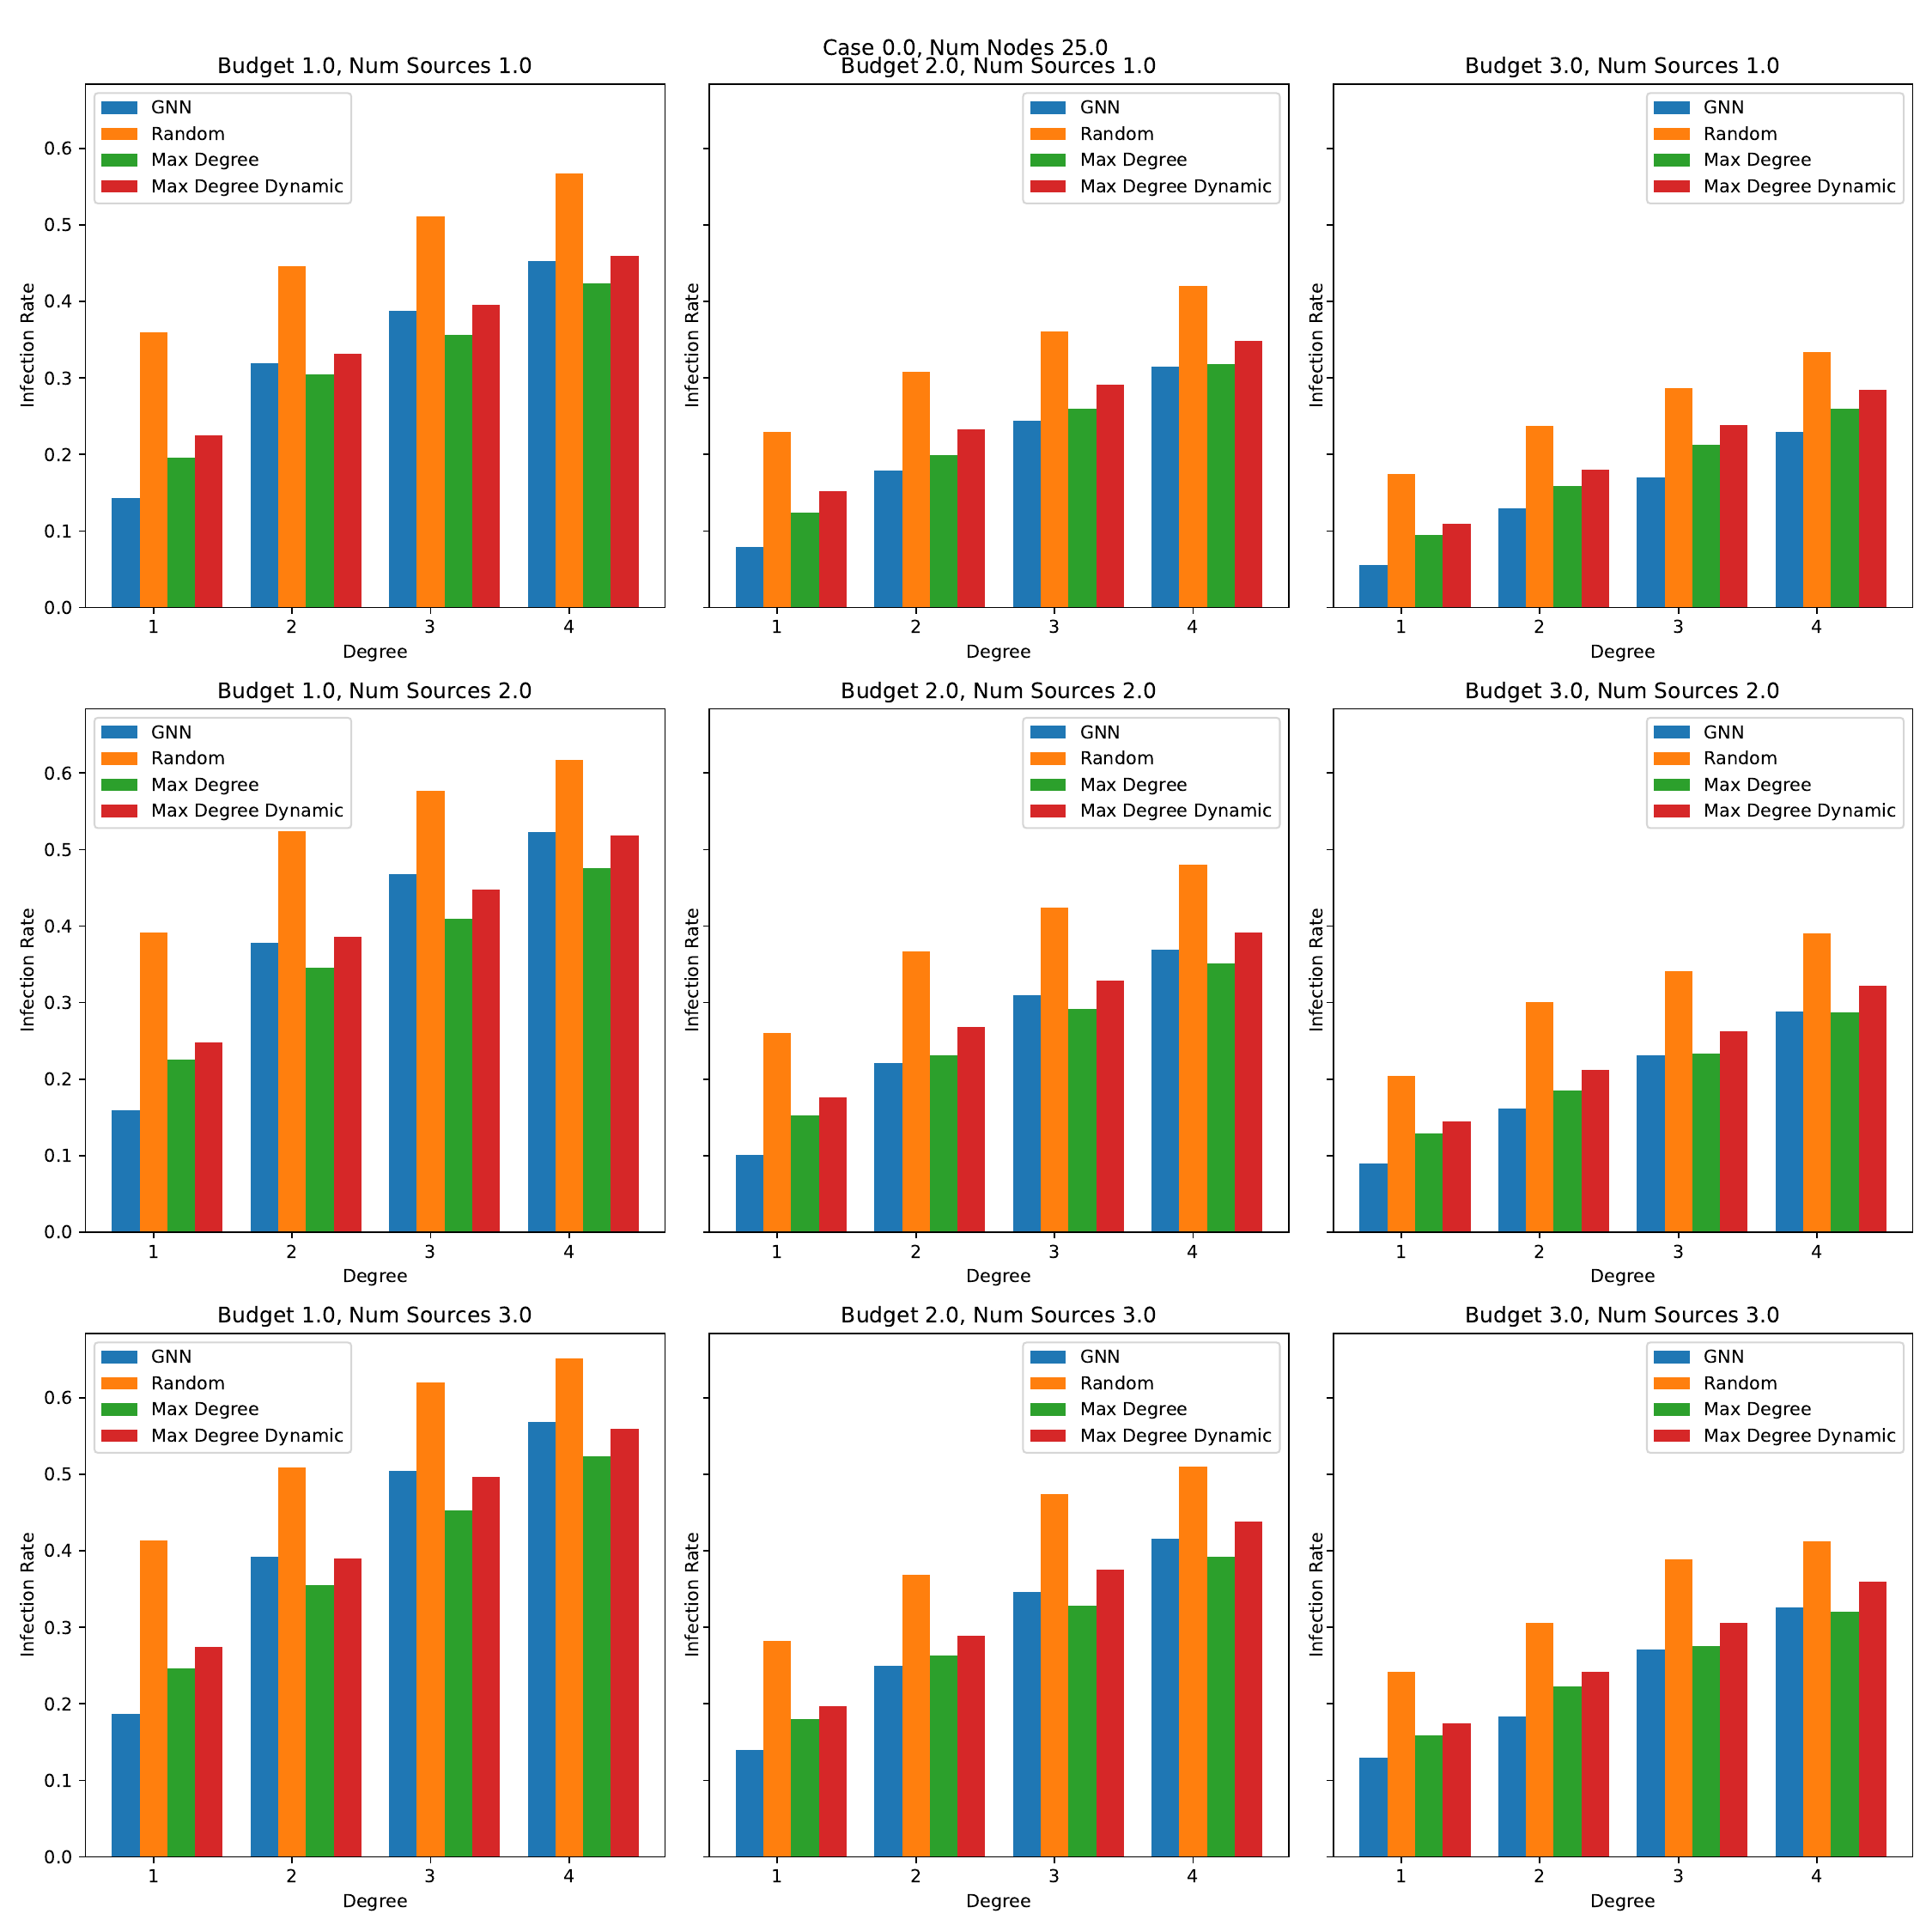}
    \caption{\footnotesize Dataset: Watts-Strogatz, Case-1 Node-25: Performance Evaluation of GCN-Based Supervised Learning Model: This series of bar plots presents a comparative analysis between our GCN-based SL model (blue), Randomized Policy model(yellow), Max Degree Policy model (Static) (green) and Max Degree Policy model (Dynamic) (red) on 25-node network environment. Progressing from left to right, the plots depict scenarios with increasing action budgets, ranging from 1 to 3 actions permitted. Vertically, the plots are ordered to show the effect of varying the initial count of infected nodes, starting with one and increasing to three. Each set of bars within the plots is categorized by the average connectivity (degree) of the infected nodes.}
    \label{fig:c1n25}
\end{figure}

\begin{figure}[!h]
    \centering
    \includegraphics[scale=0.3]{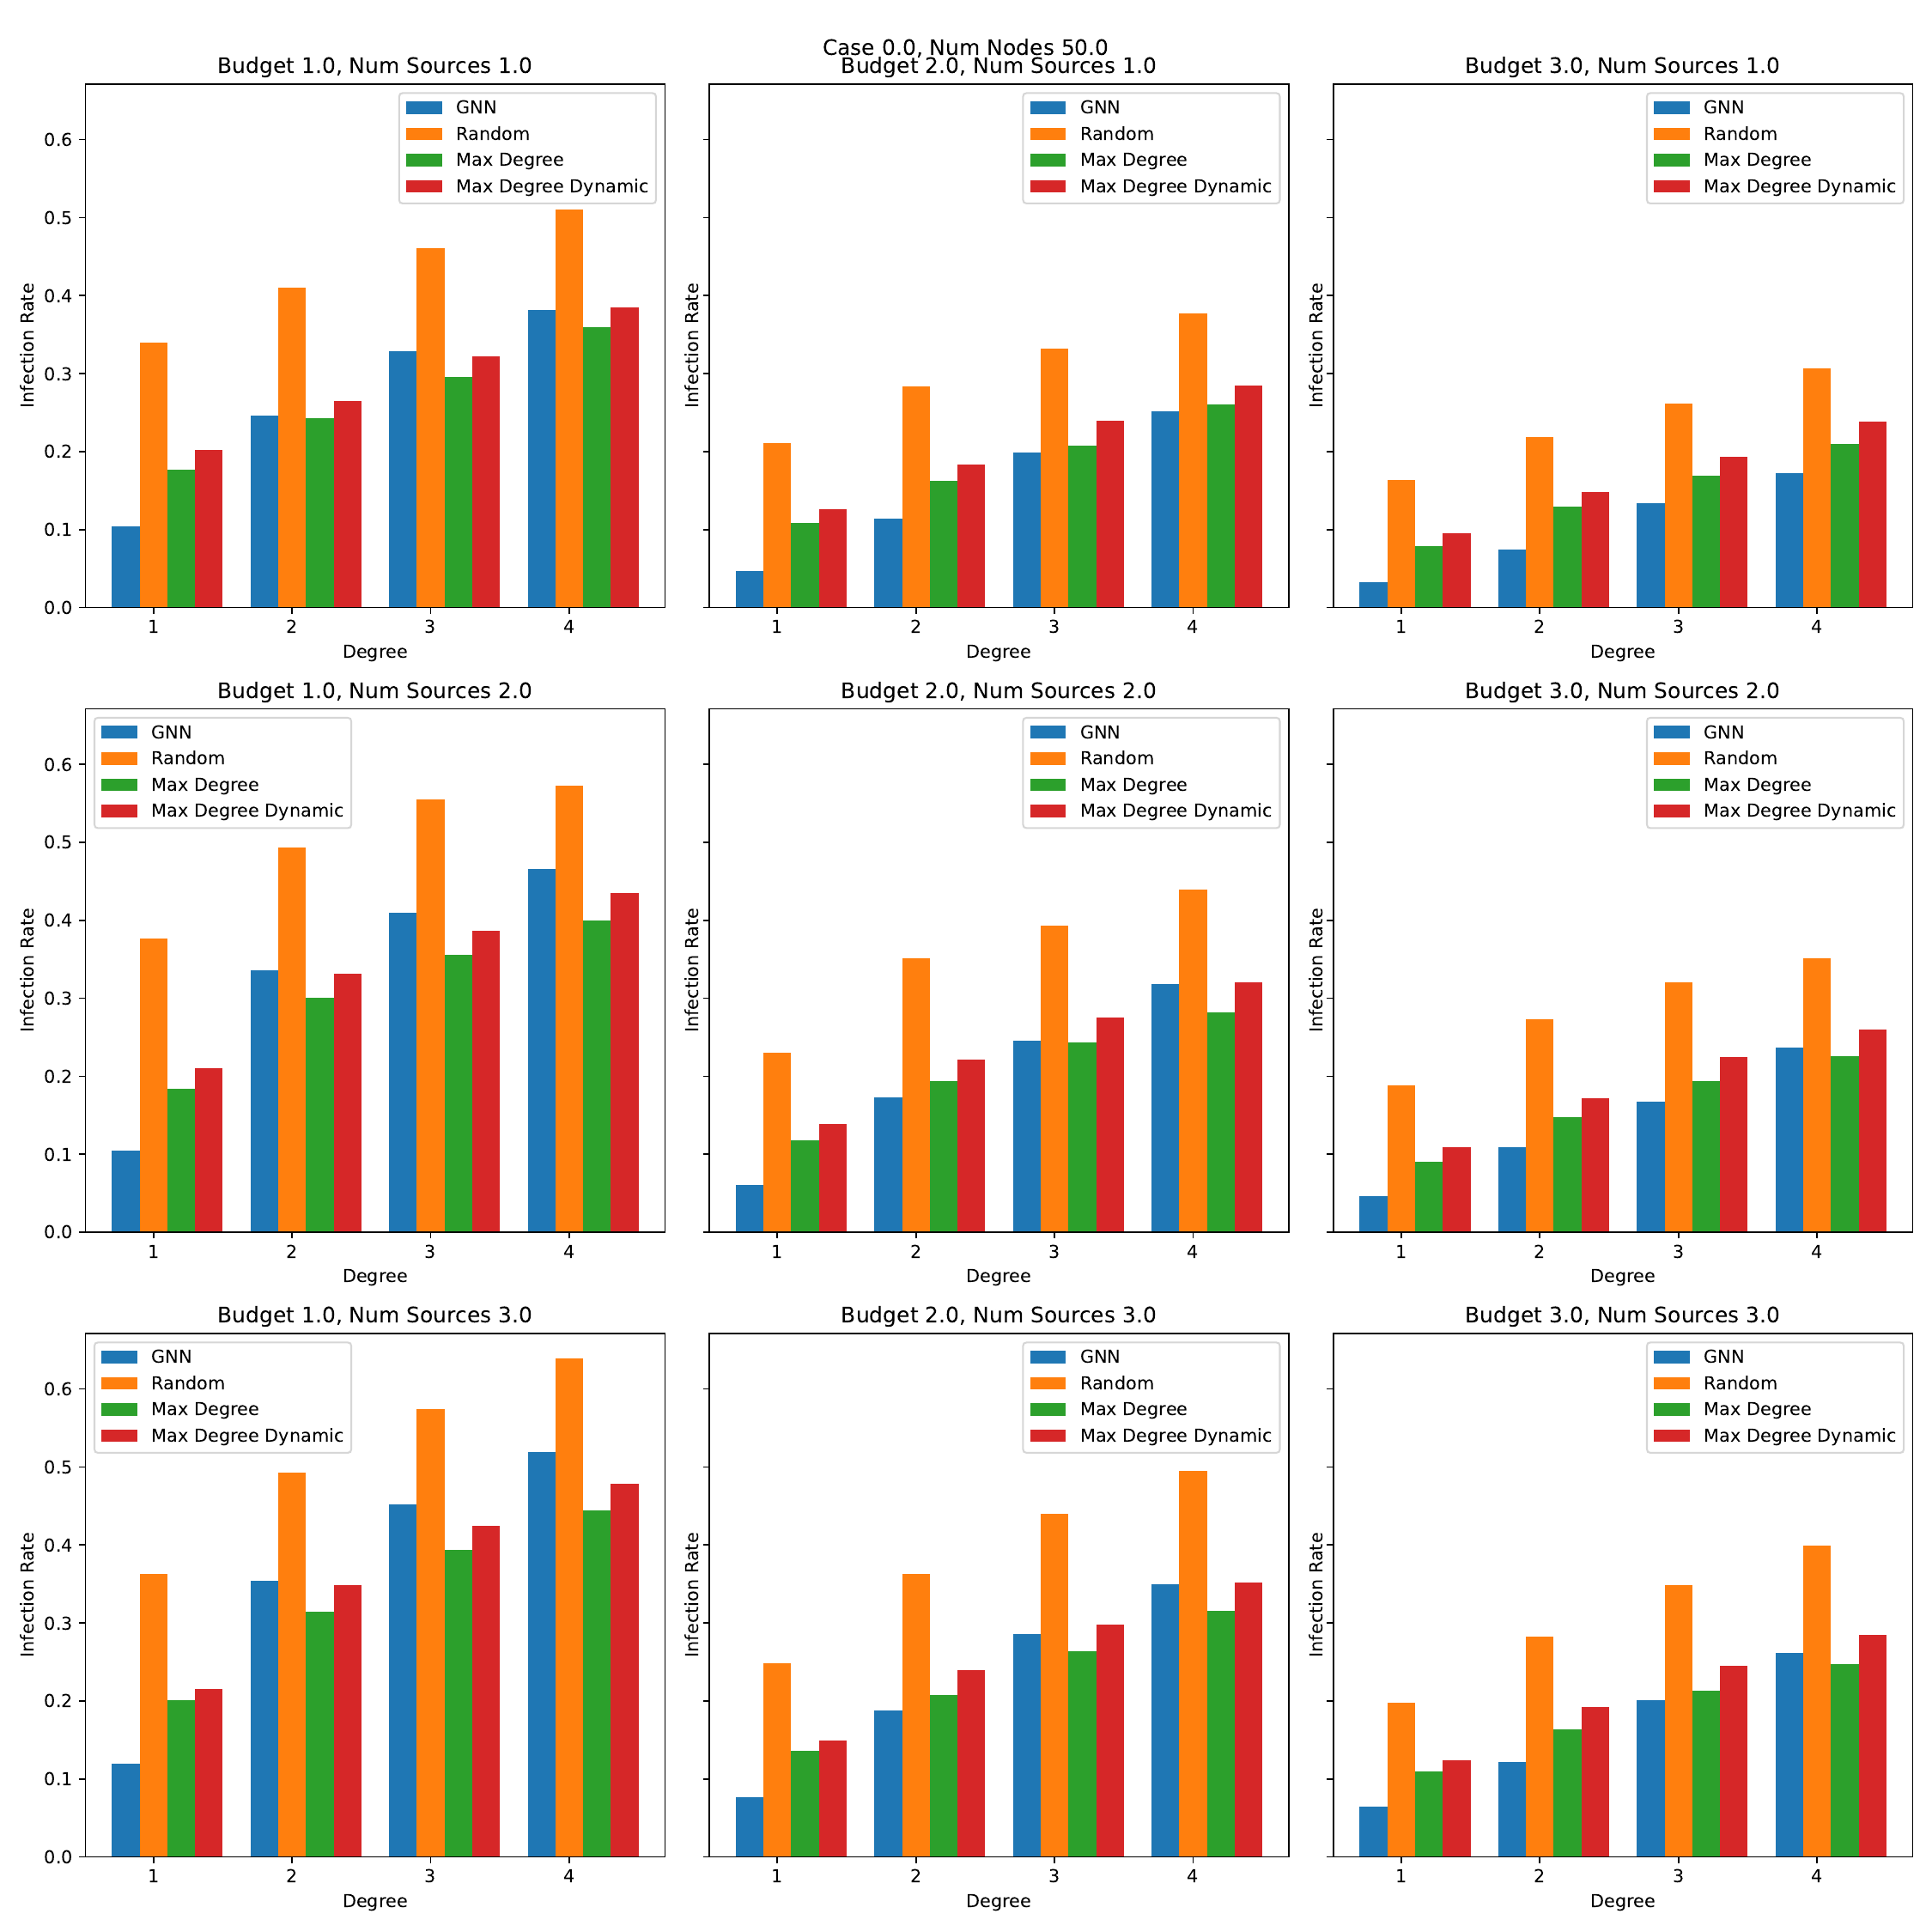}
    \caption{\footnotesize Dataset: Watts-Strogatz, Case-1 Node-50: Performance Evaluation of GCN-Based Supervised Learning Model: This series of bar plots presents a comparative analysis between our GCN-based SL model (blue), Randomized Policy model(yellow), Max Degree Policy model (Static) (green) and Max Degree Policy model (Dynamic) (red) on 50-node network environment. Progressing from left to right, the plots depict scenarios with increasing action budgets, ranging from 1 to 3 actions permitted. Vertically, the plots are ordered to show the effect of varying the initial count of infected nodes, starting with one and increasing to three. Each set of bars within the plots is categorized by the average connectivity (degree) of the infected nodes.}
    \label{fig:c1n50}
\end{figure}

\begin{figure}[!h]
    \centering
    \includegraphics[scale=0.3]{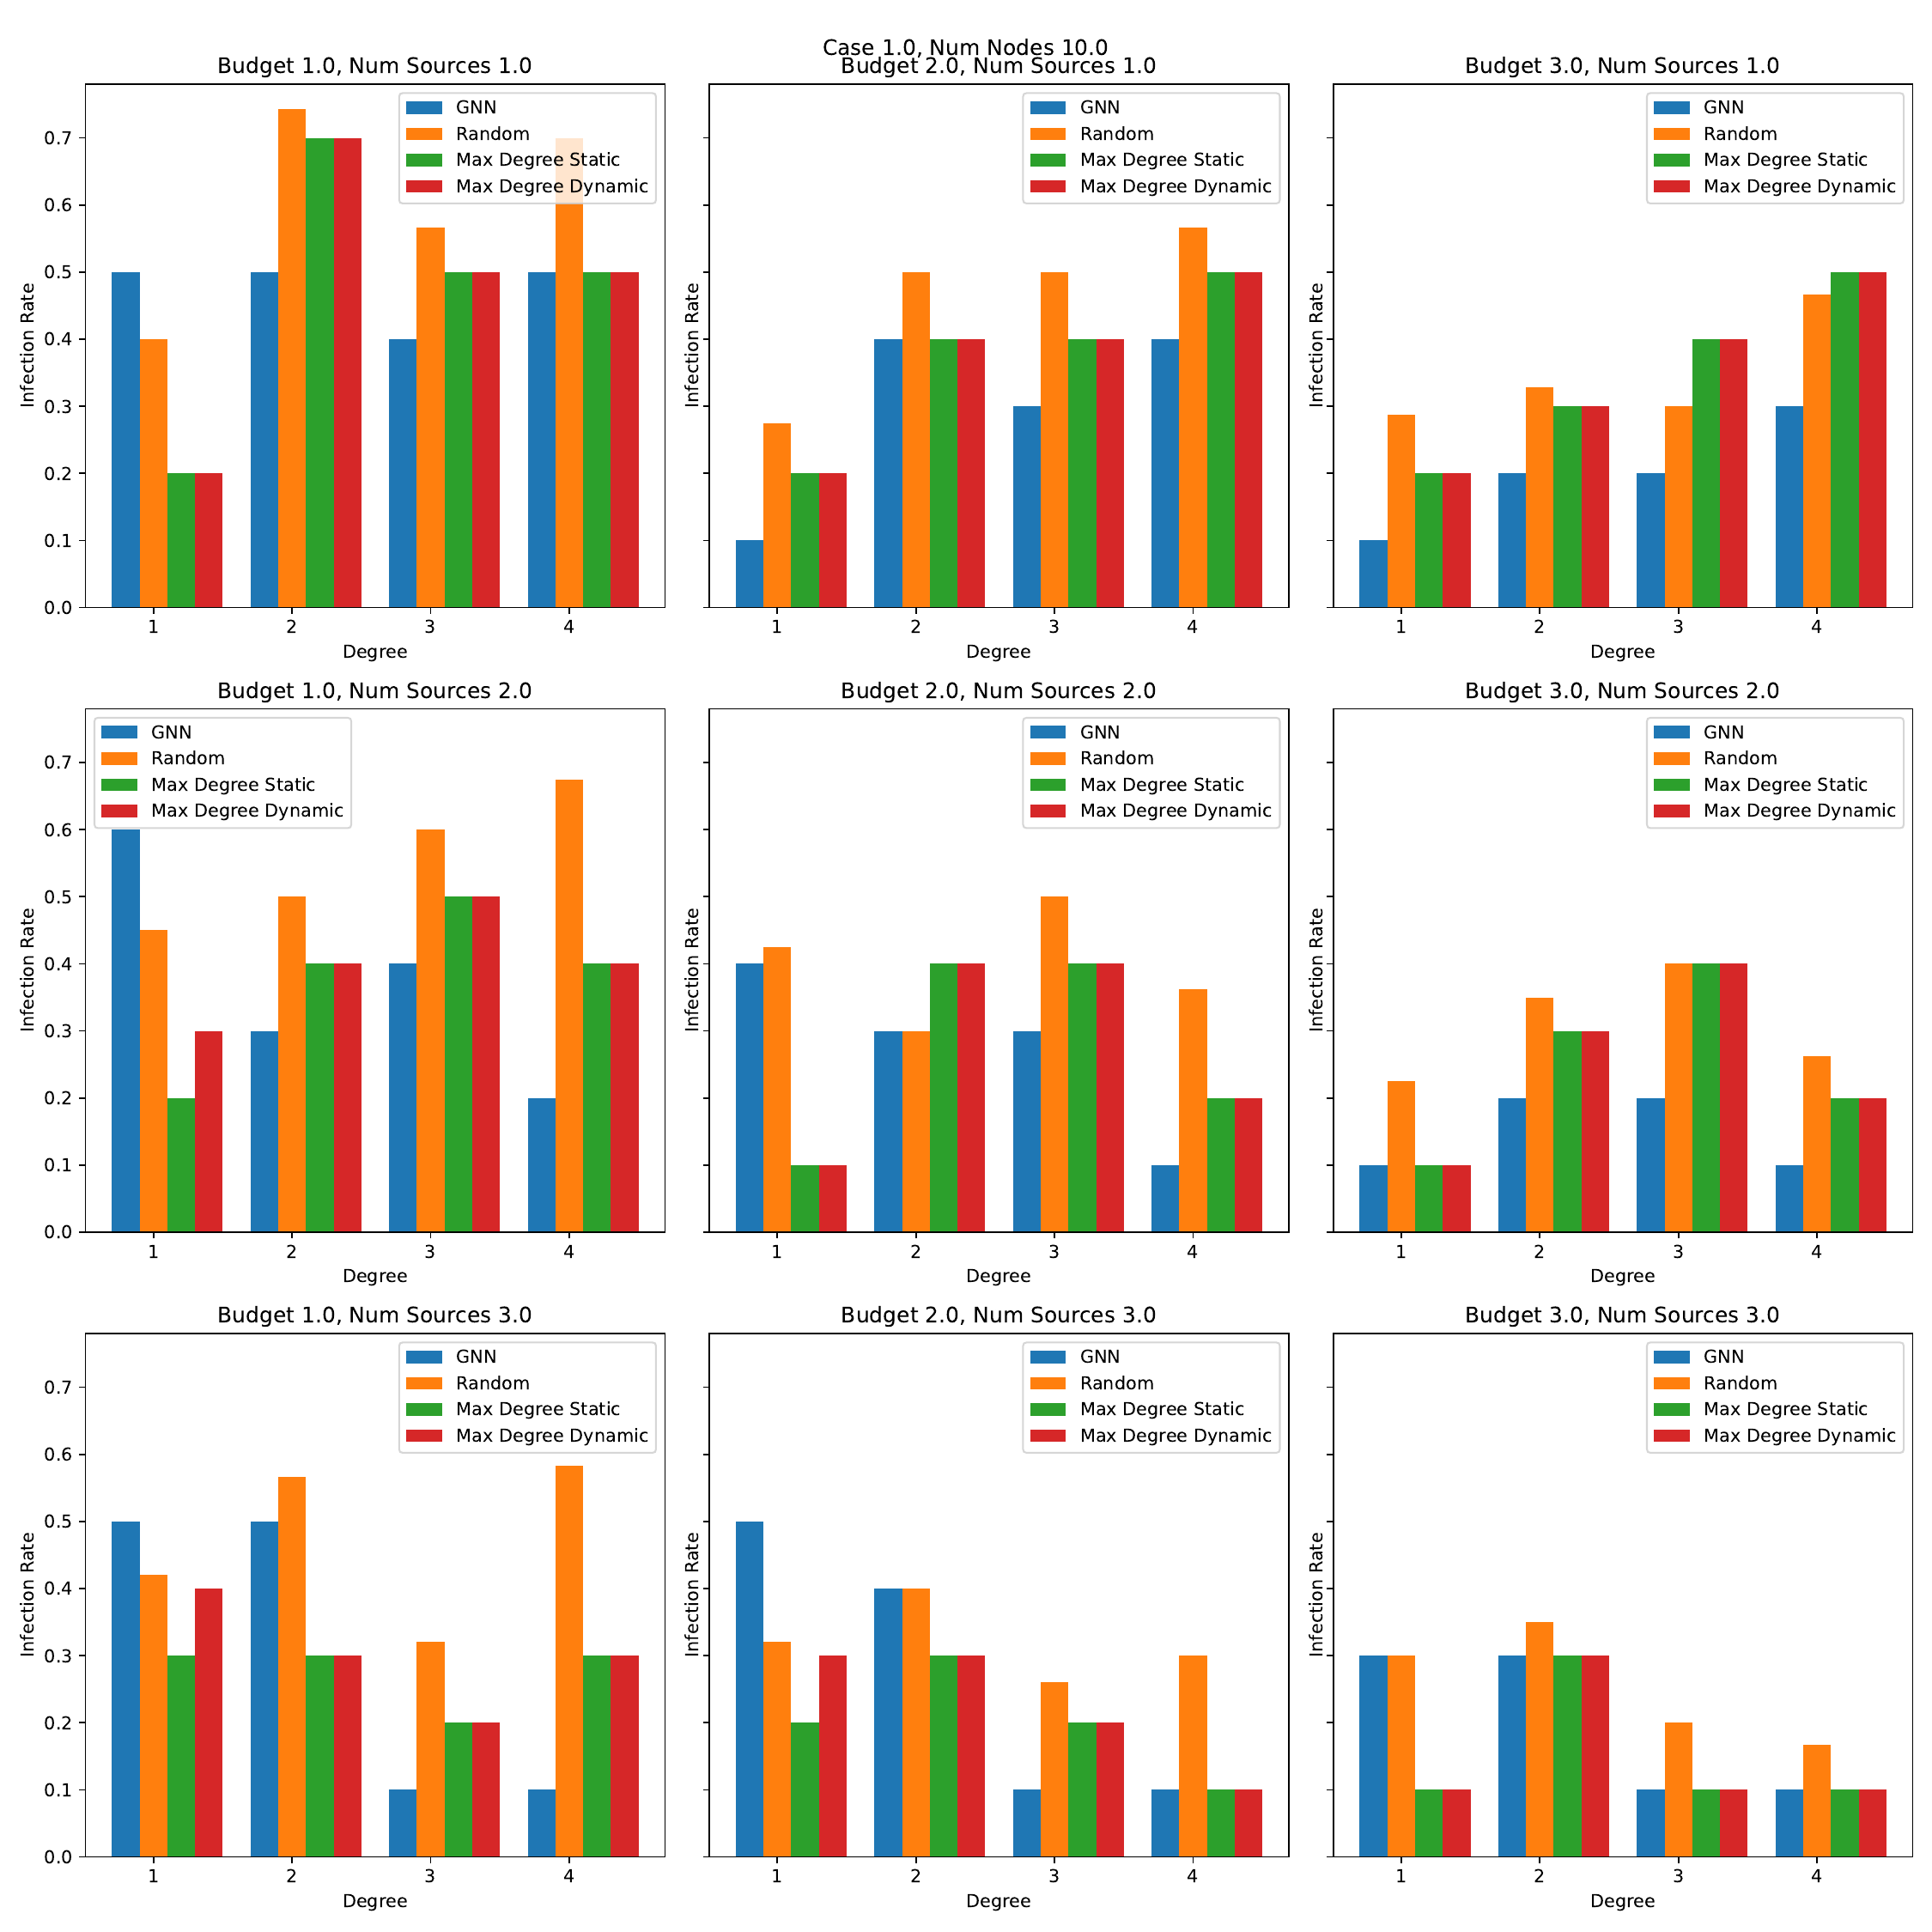}
    \caption{\footnotesize Dataset: Tree, Case-1 Node-10: Performance Evaluation of GCN-Based Supervised Learning Model: This series of bar plots presents a comparative analysis between our GCN-based SL model (blue), Randomized Policy model(yellow), Max Degree Policy model (Static) (green) and Max Degree Policy model (Dynamic) (red) on 10-node network environment. Progressing from left to right, the plots depict scenarios with increasing action budgets, ranging from 1 to 3 actions permitted. Vertically, the plots are ordered to show the effect of varying the initial count of infected nodes, starting with one and increasing to three. Each set of bars within the plots is categorized by the average connectivity (degree) of the infected nodes.}
    \label{fig:Treec1n10}
\end{figure}

\begin{figure}[!h]
    \centering
    \includegraphics[scale=0.3]{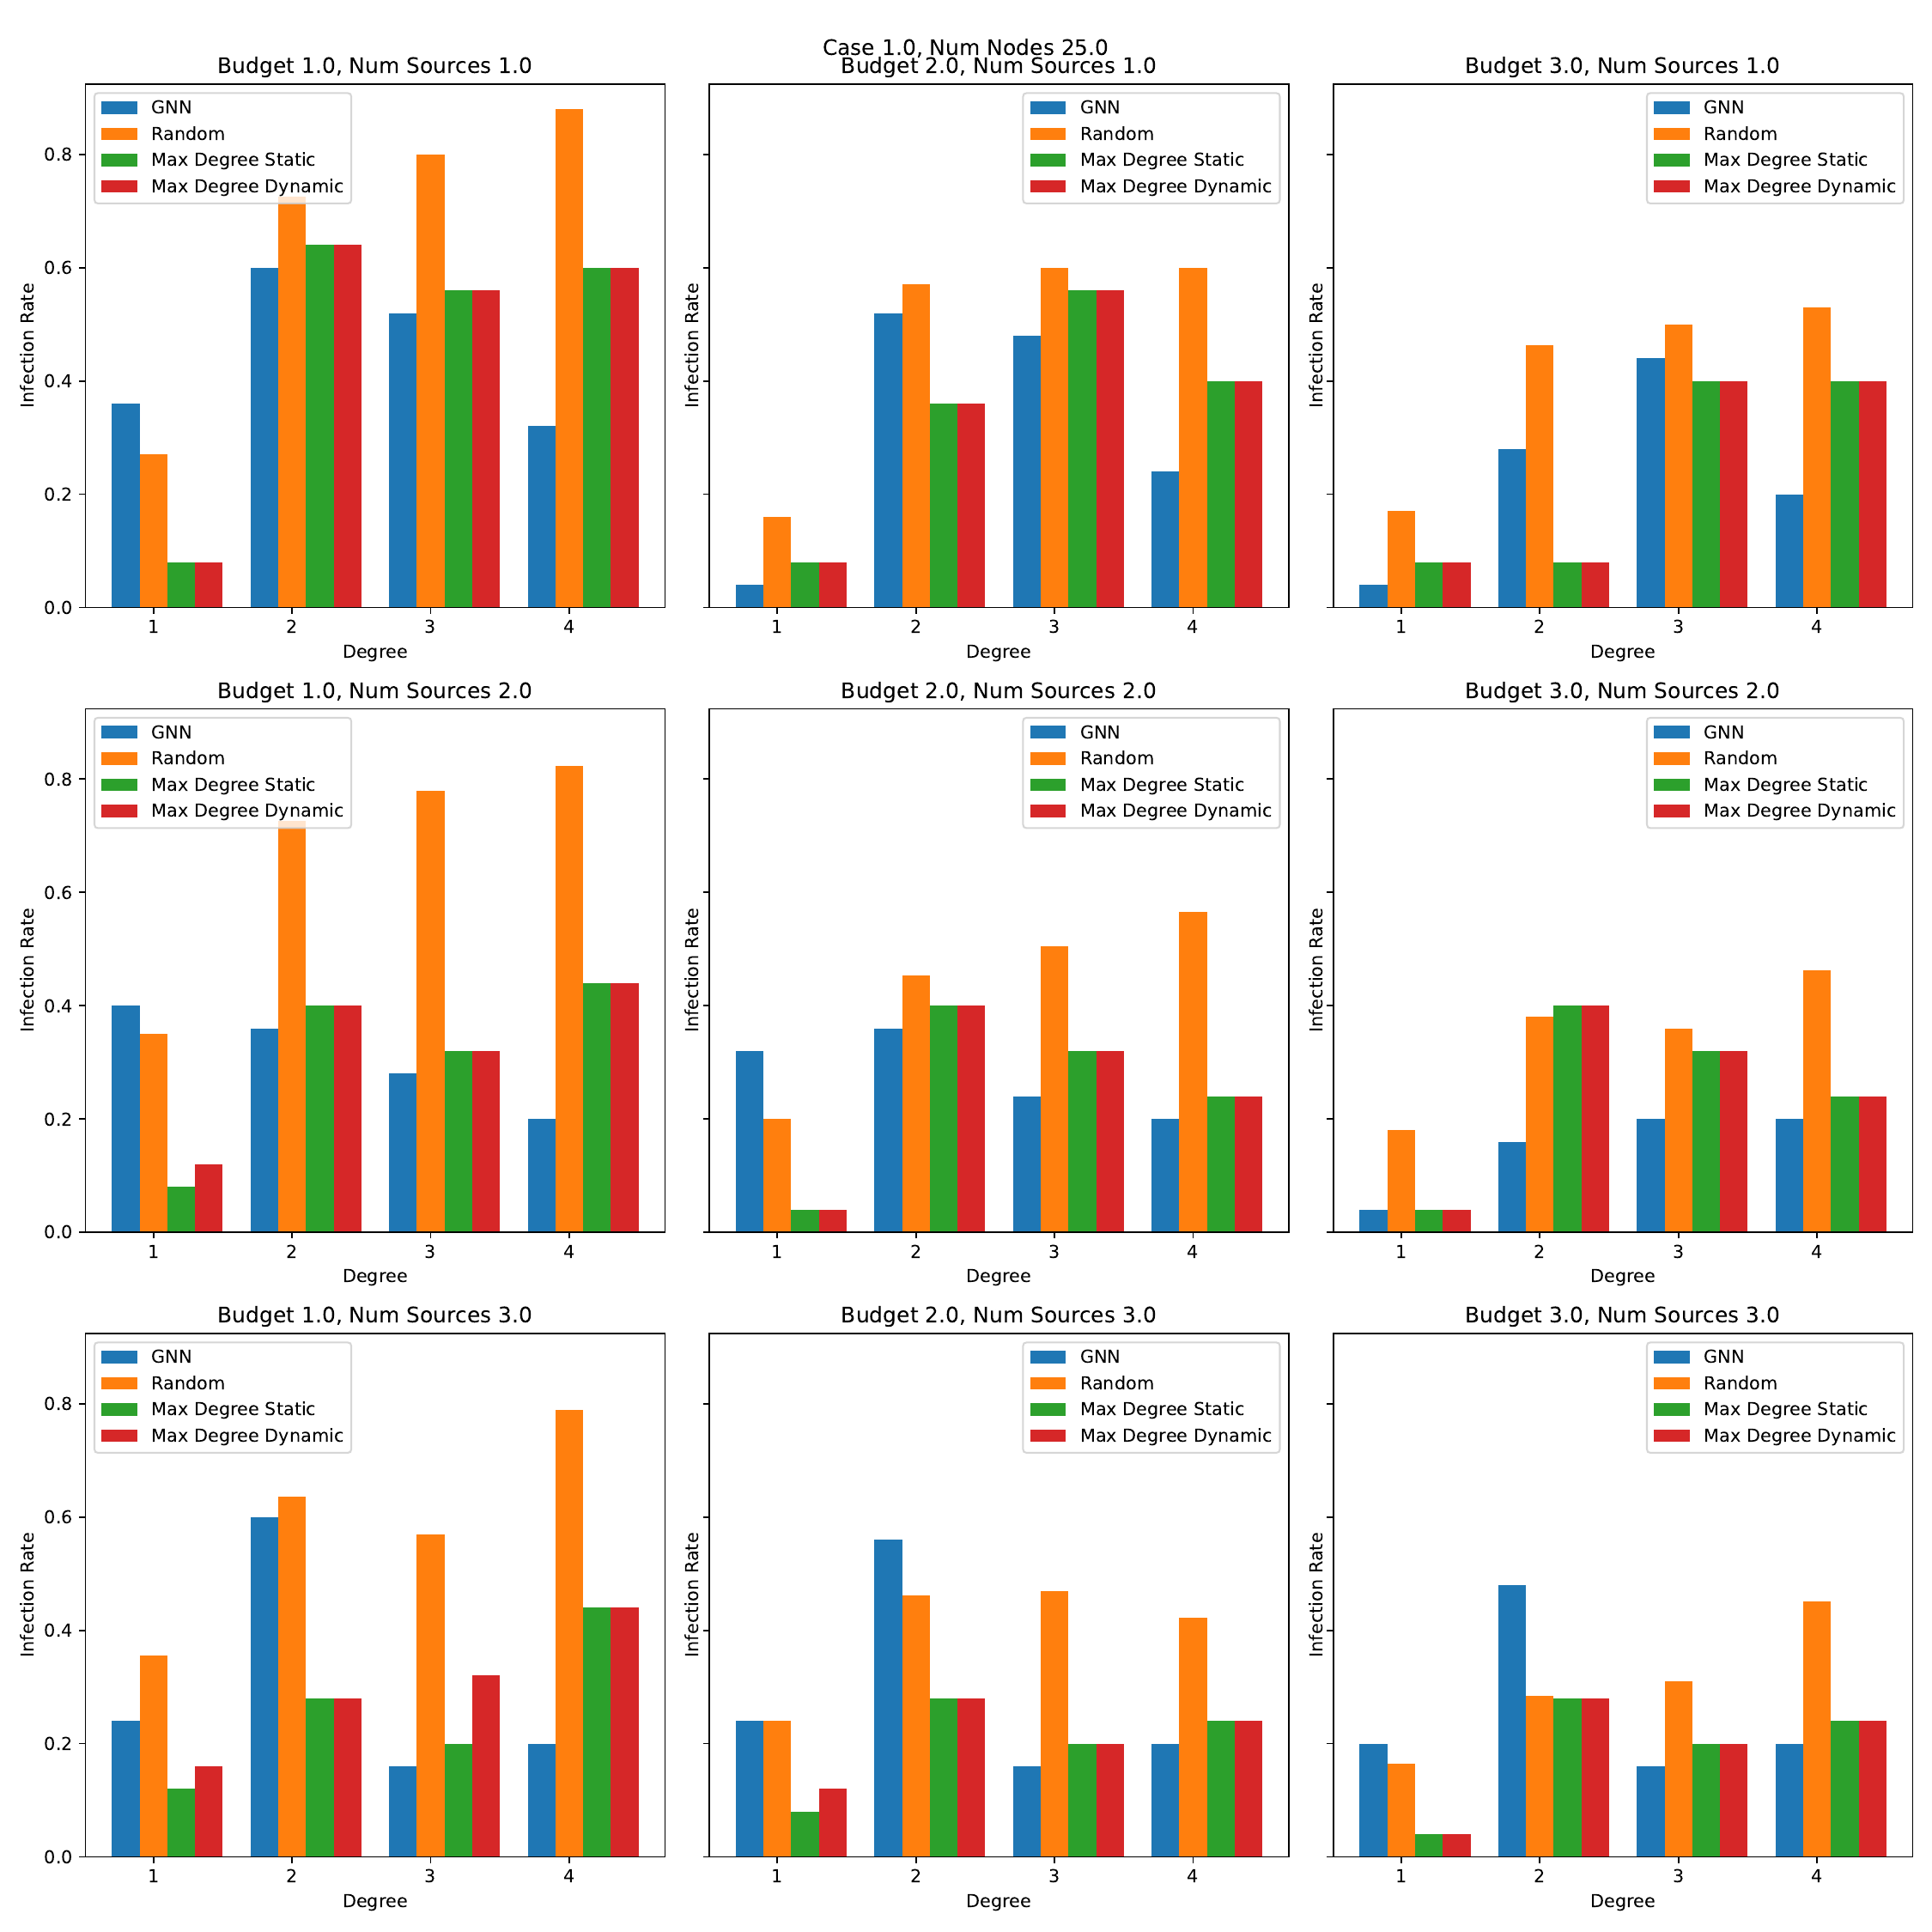}
    \caption{\footnotesize Dataset: Tree, Case-1 Node-25: Performance Evaluation of GCN-Based Supervised Learning Model: This series of bar plots presents a comparative analysis between our GCN-based SL model (blue), Randomized Policy model(yellow), Max Degree Policy model (Static) (green) and Max Degree Policy model (Dynamic) (red) on 25-node network environment. Progressing from left to right, the plots depict scenarios with increasing action budgets, ranging from 1 to 3 actions permitted. Vertically, the plots are ordered to show the effect of varying the initial count of infected nodes, starting with one and increasing to three. Each set of bars within the plots is categorized by the average connectivity (degree) of the infected nodes.}
    \label{fig:Treec1n25}
\end{figure}

\begin{figure}[!h]
    \centering
    \includegraphics[scale=0.3]{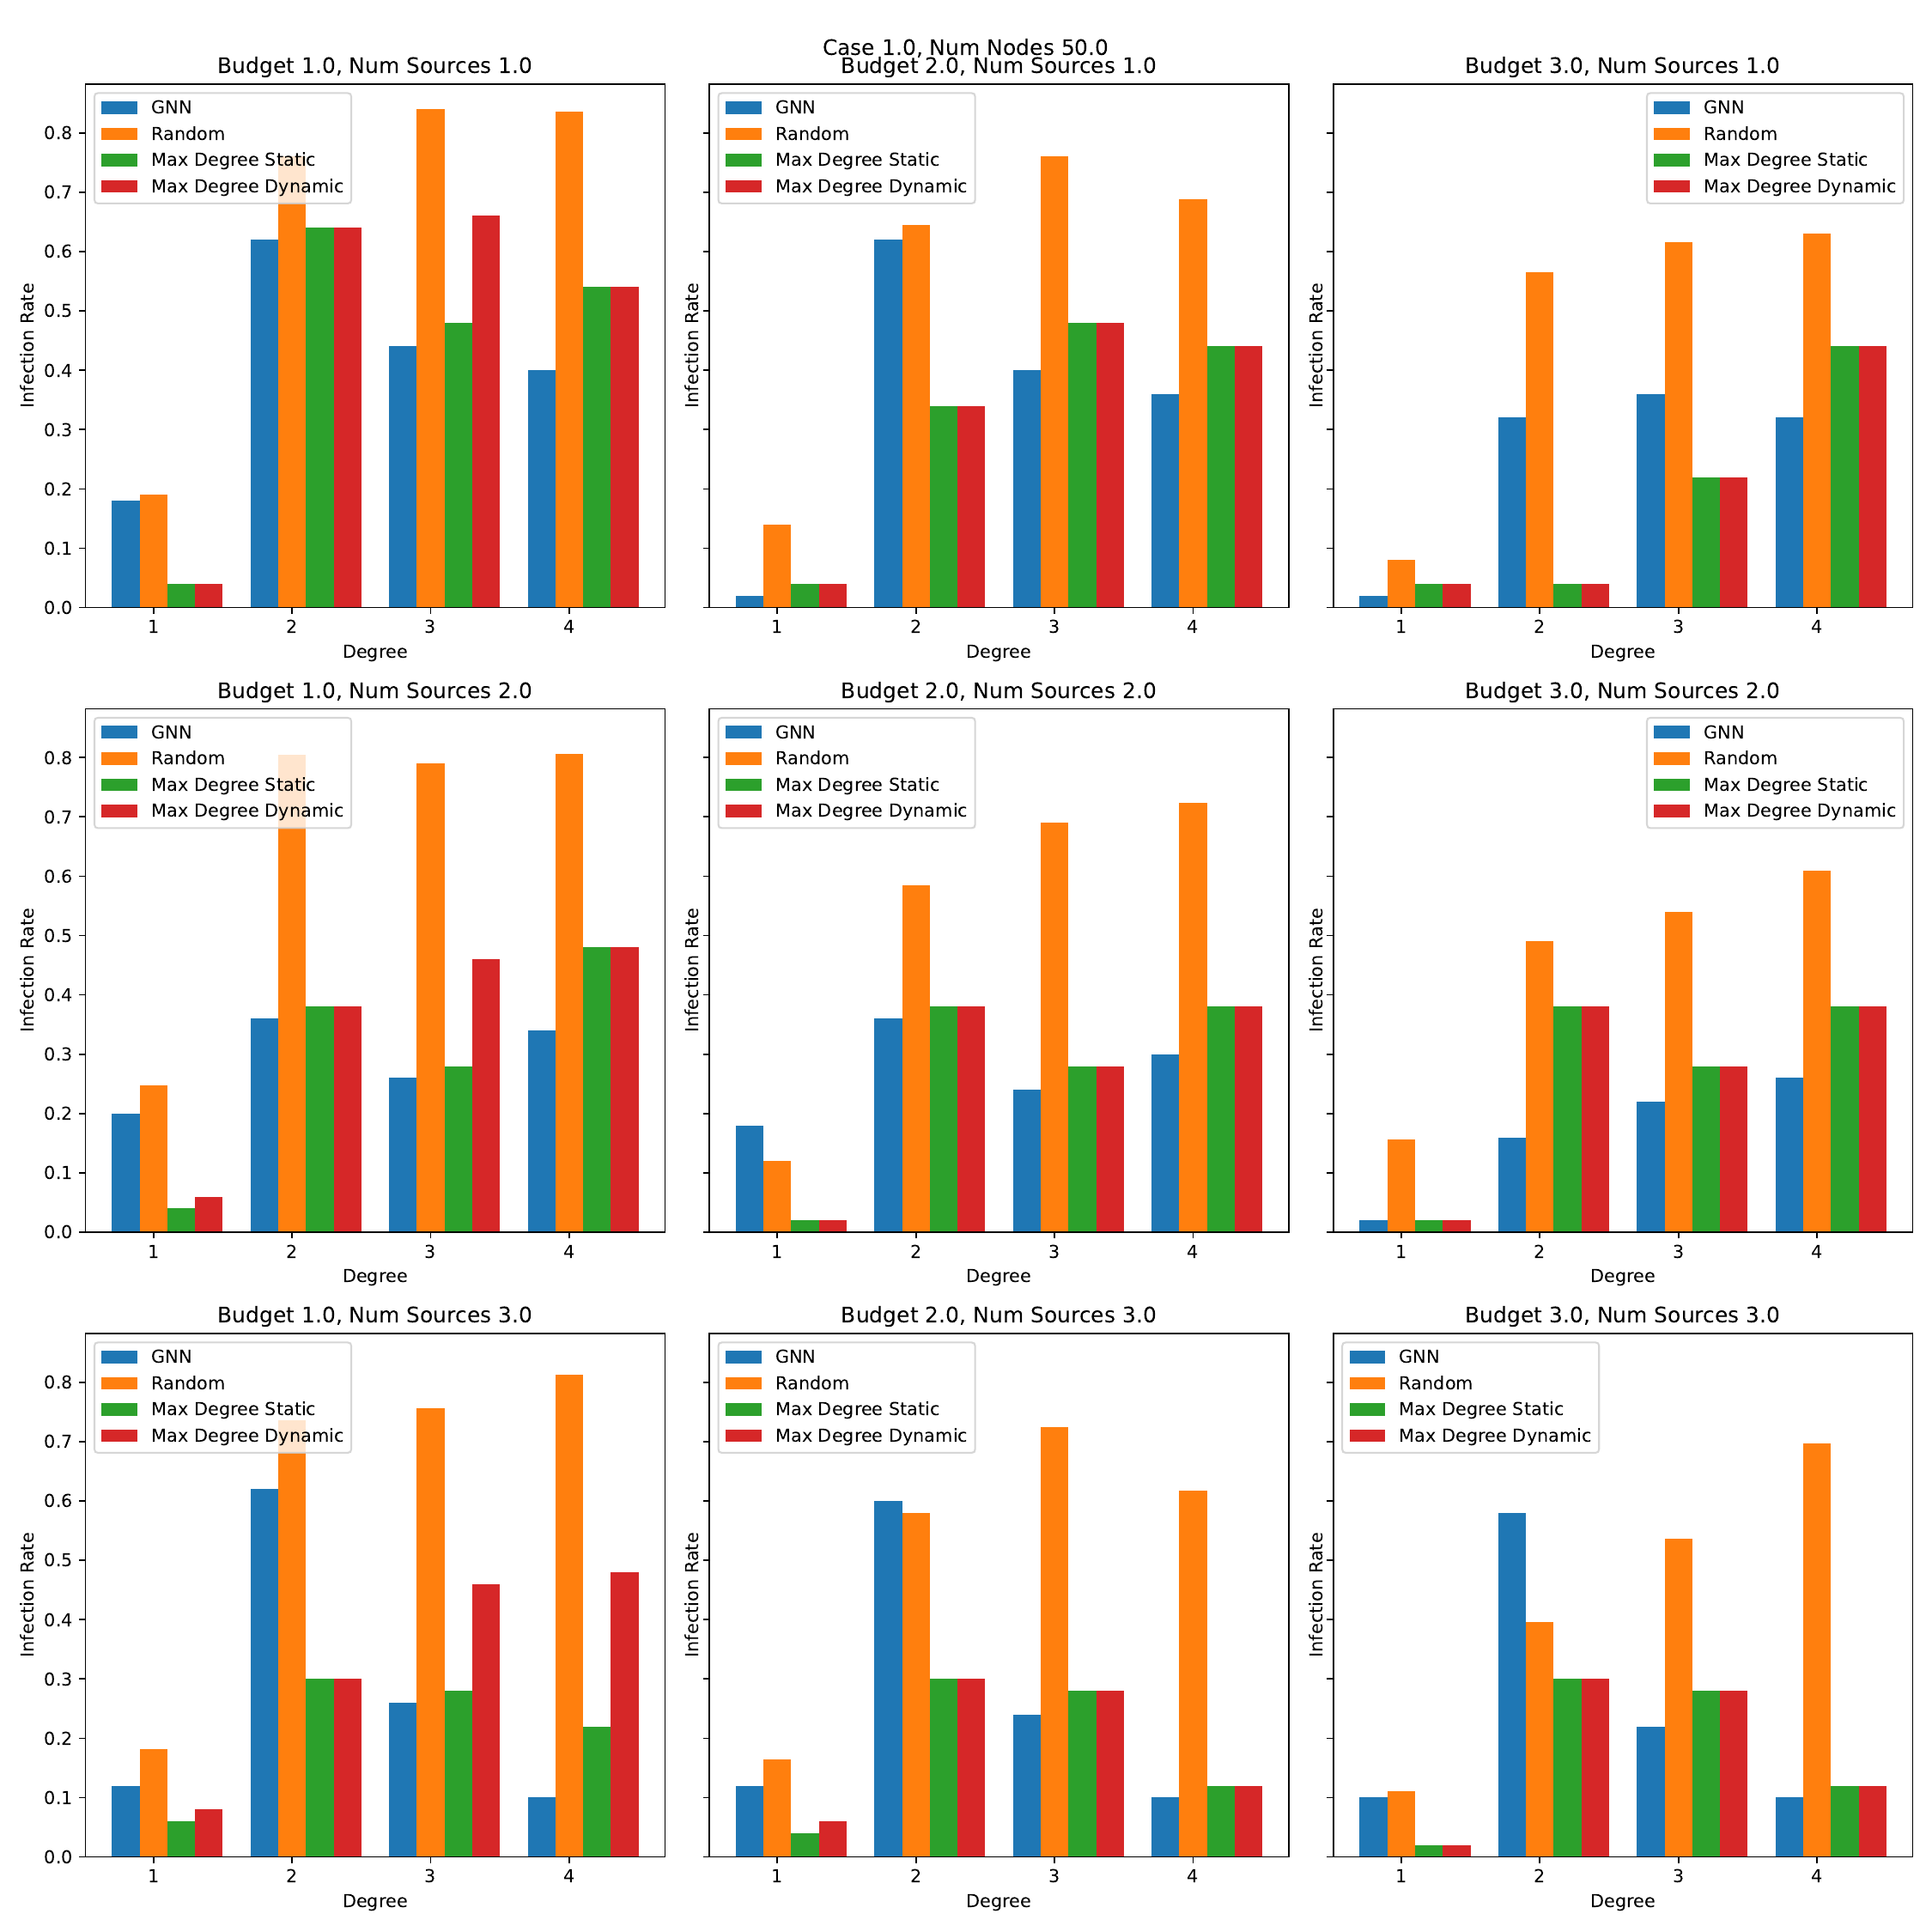}
    \caption{\footnotesize Dataset: Tree, Case-1 Node-50: Performance Evaluation of GCN-Based Supervised Learning Model: This series of bar plots presents a comparative analysis between our GCN-based SL model (blue), Randomized Policy model(yellow), Max Degree Policy model (Static) (green) and Max Degree Policy model (Dynamic) (red) on 25-node network environment. Progressing from left to right, the plots depict scenarios with increasing action budgets, ranging from 1 to 3 actions permitted. Vertically, the plots are ordered to show the effect of varying the initial count of infected nodes, starting with one and increasing to three. Each set of bars within the plots is categorized by the average connectivity (degree) of the infected nodes.}
    \label{fig:Treec1n50}
\end{figure}

\begin{figure}[!h]
    \centering
    \includegraphics[scale=0.3]{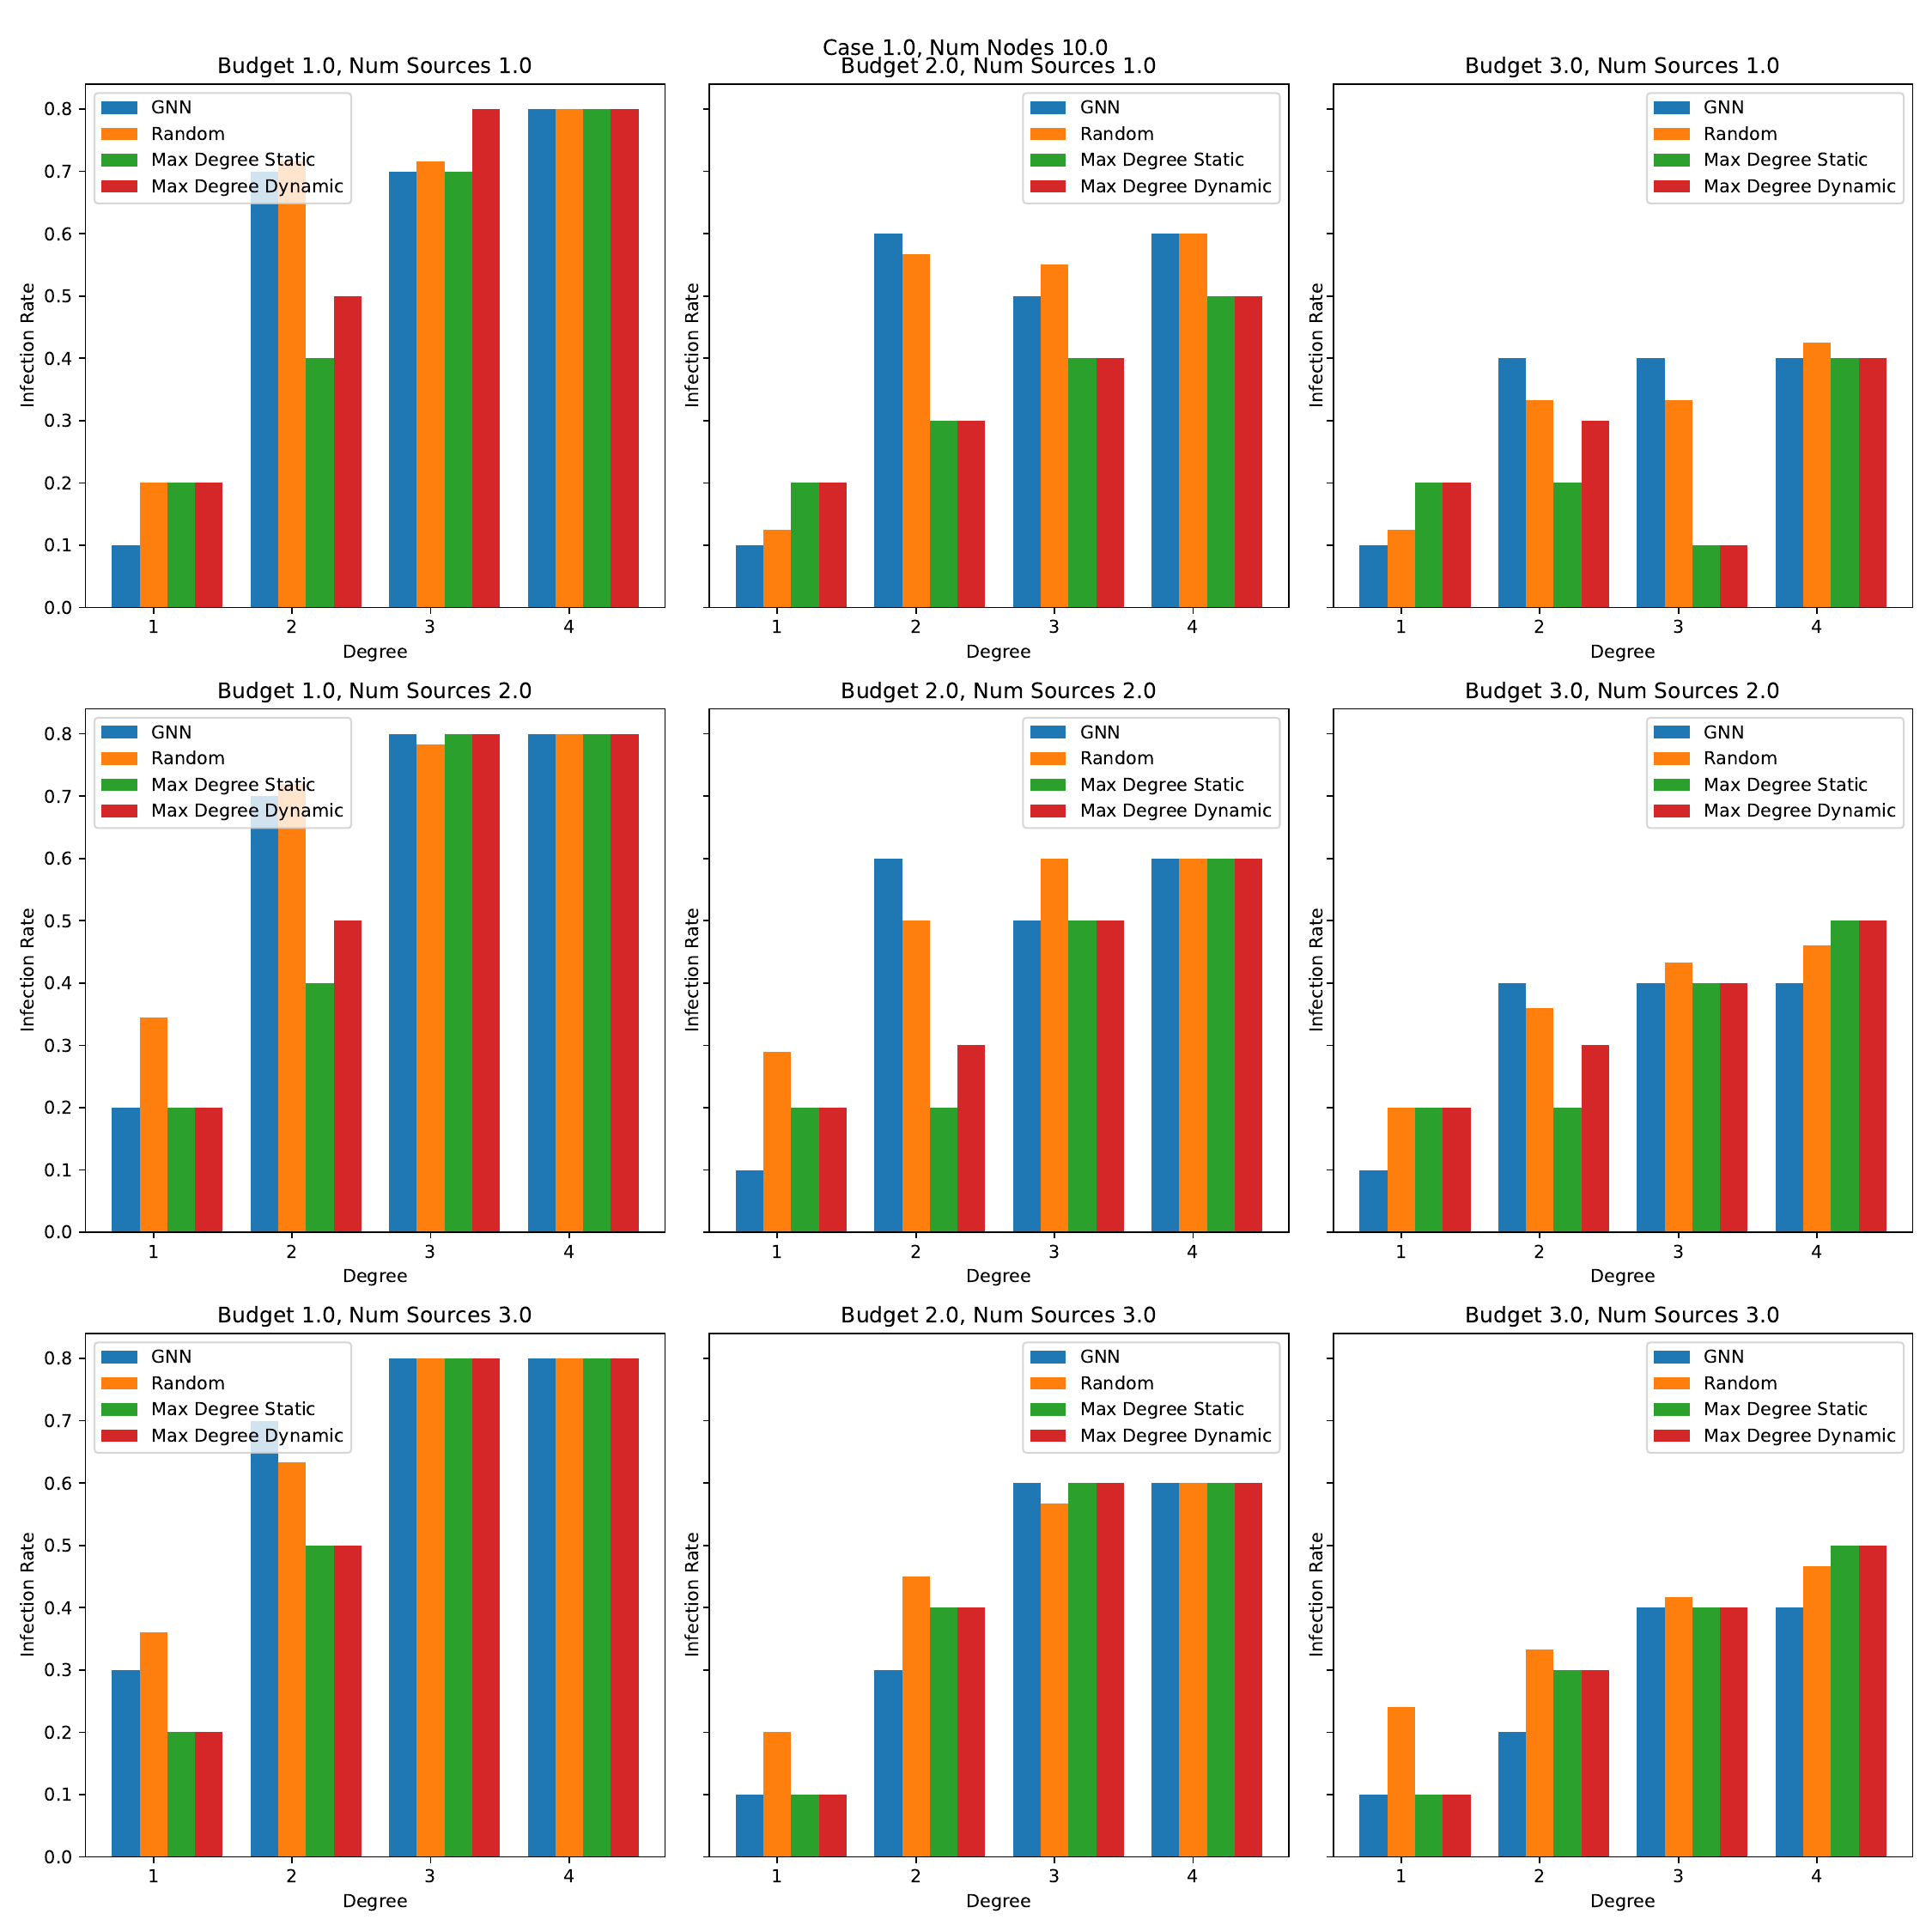}
    \caption{\footnotesize Dataset: Erdos-Renyi, Case-1 Node-10: Performance Evaluation of GCN-Based Supervised Learning Model: This series of bar plots presents a comparative analysis between our GCN-based SL model (blue), Randomized Policy model(yellow), Max Degree Policy model (Static) (green) and Max Degree Policy model (Dynamic) (red) on 10-node network environment. Progressing from left to right, the plots depict scenarios with increasing action budgets, ranging from 1 to 3 actions permitted. Vertically, the plots are ordered to show the effect of varying the initial count of infected nodes, starting with one and increasing to three. Each set of bars within the plots is categorized by the average connectivity (degree) of the infected nodes.}
    \label{fig:ERc1n10}
\end{figure}

\begin{figure}[!h]
    \centering
    \includegraphics[scale=0.3]{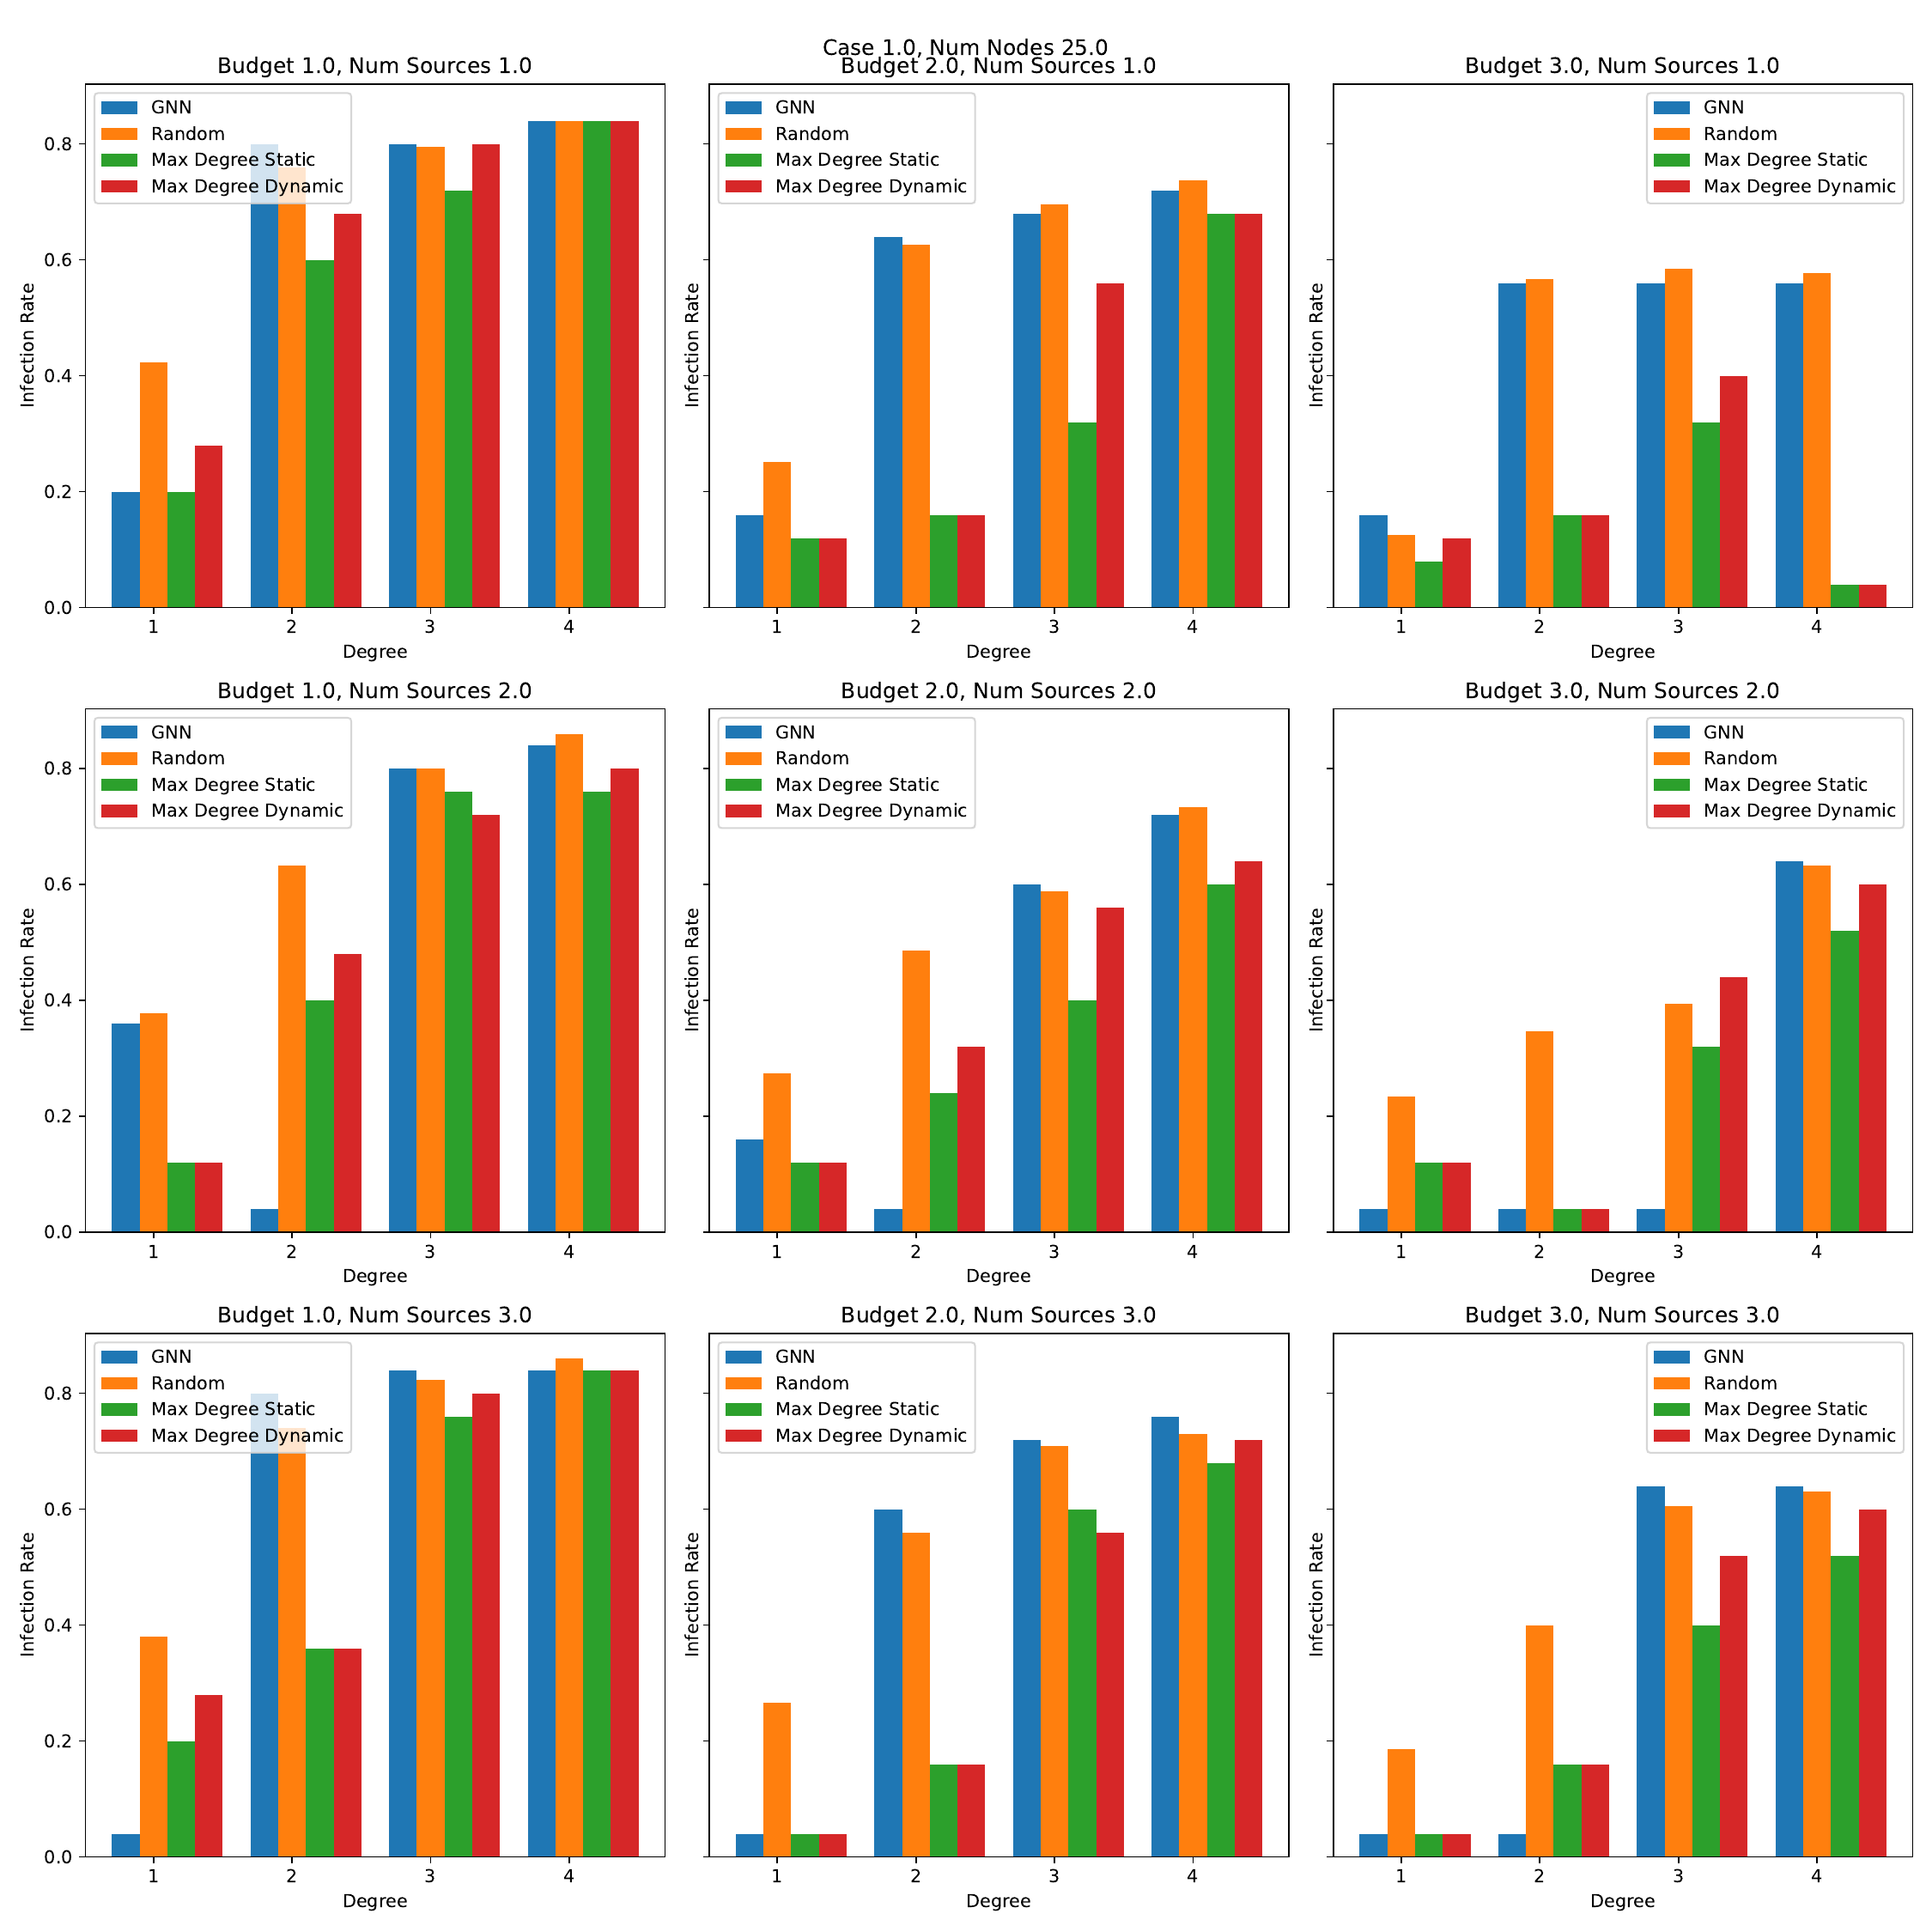}
    \caption{\footnotesize Dataset: Erdos-Renyi, Case-1 Node-25: Performance Evaluation of GCN-Based Supervised Learning Model: This series of bar plots presents a comparative analysis between our GCN-based SL model (blue), Randomized Policy model(yellow), Max Degree Policy model (Static) (green) and Max Degree Policy model (Dynamic) (red) on 25-node network environment. Progressing from left to right, the plots depict scenarios with increasing action budgets, ranging from 1 to 3 actions permitted. Vertically, the plots are ordered to show the effect of varying the initial count of infected nodes, starting with one and increasing to three. Each set of bars within the plots is categorized by the average connectivity (degree) of the infected nodes.}
    \label{fig:ERc1n25}
\end{figure}

\begin{figure}[!h]
    \centering
    \includegraphics[scale=0.3]{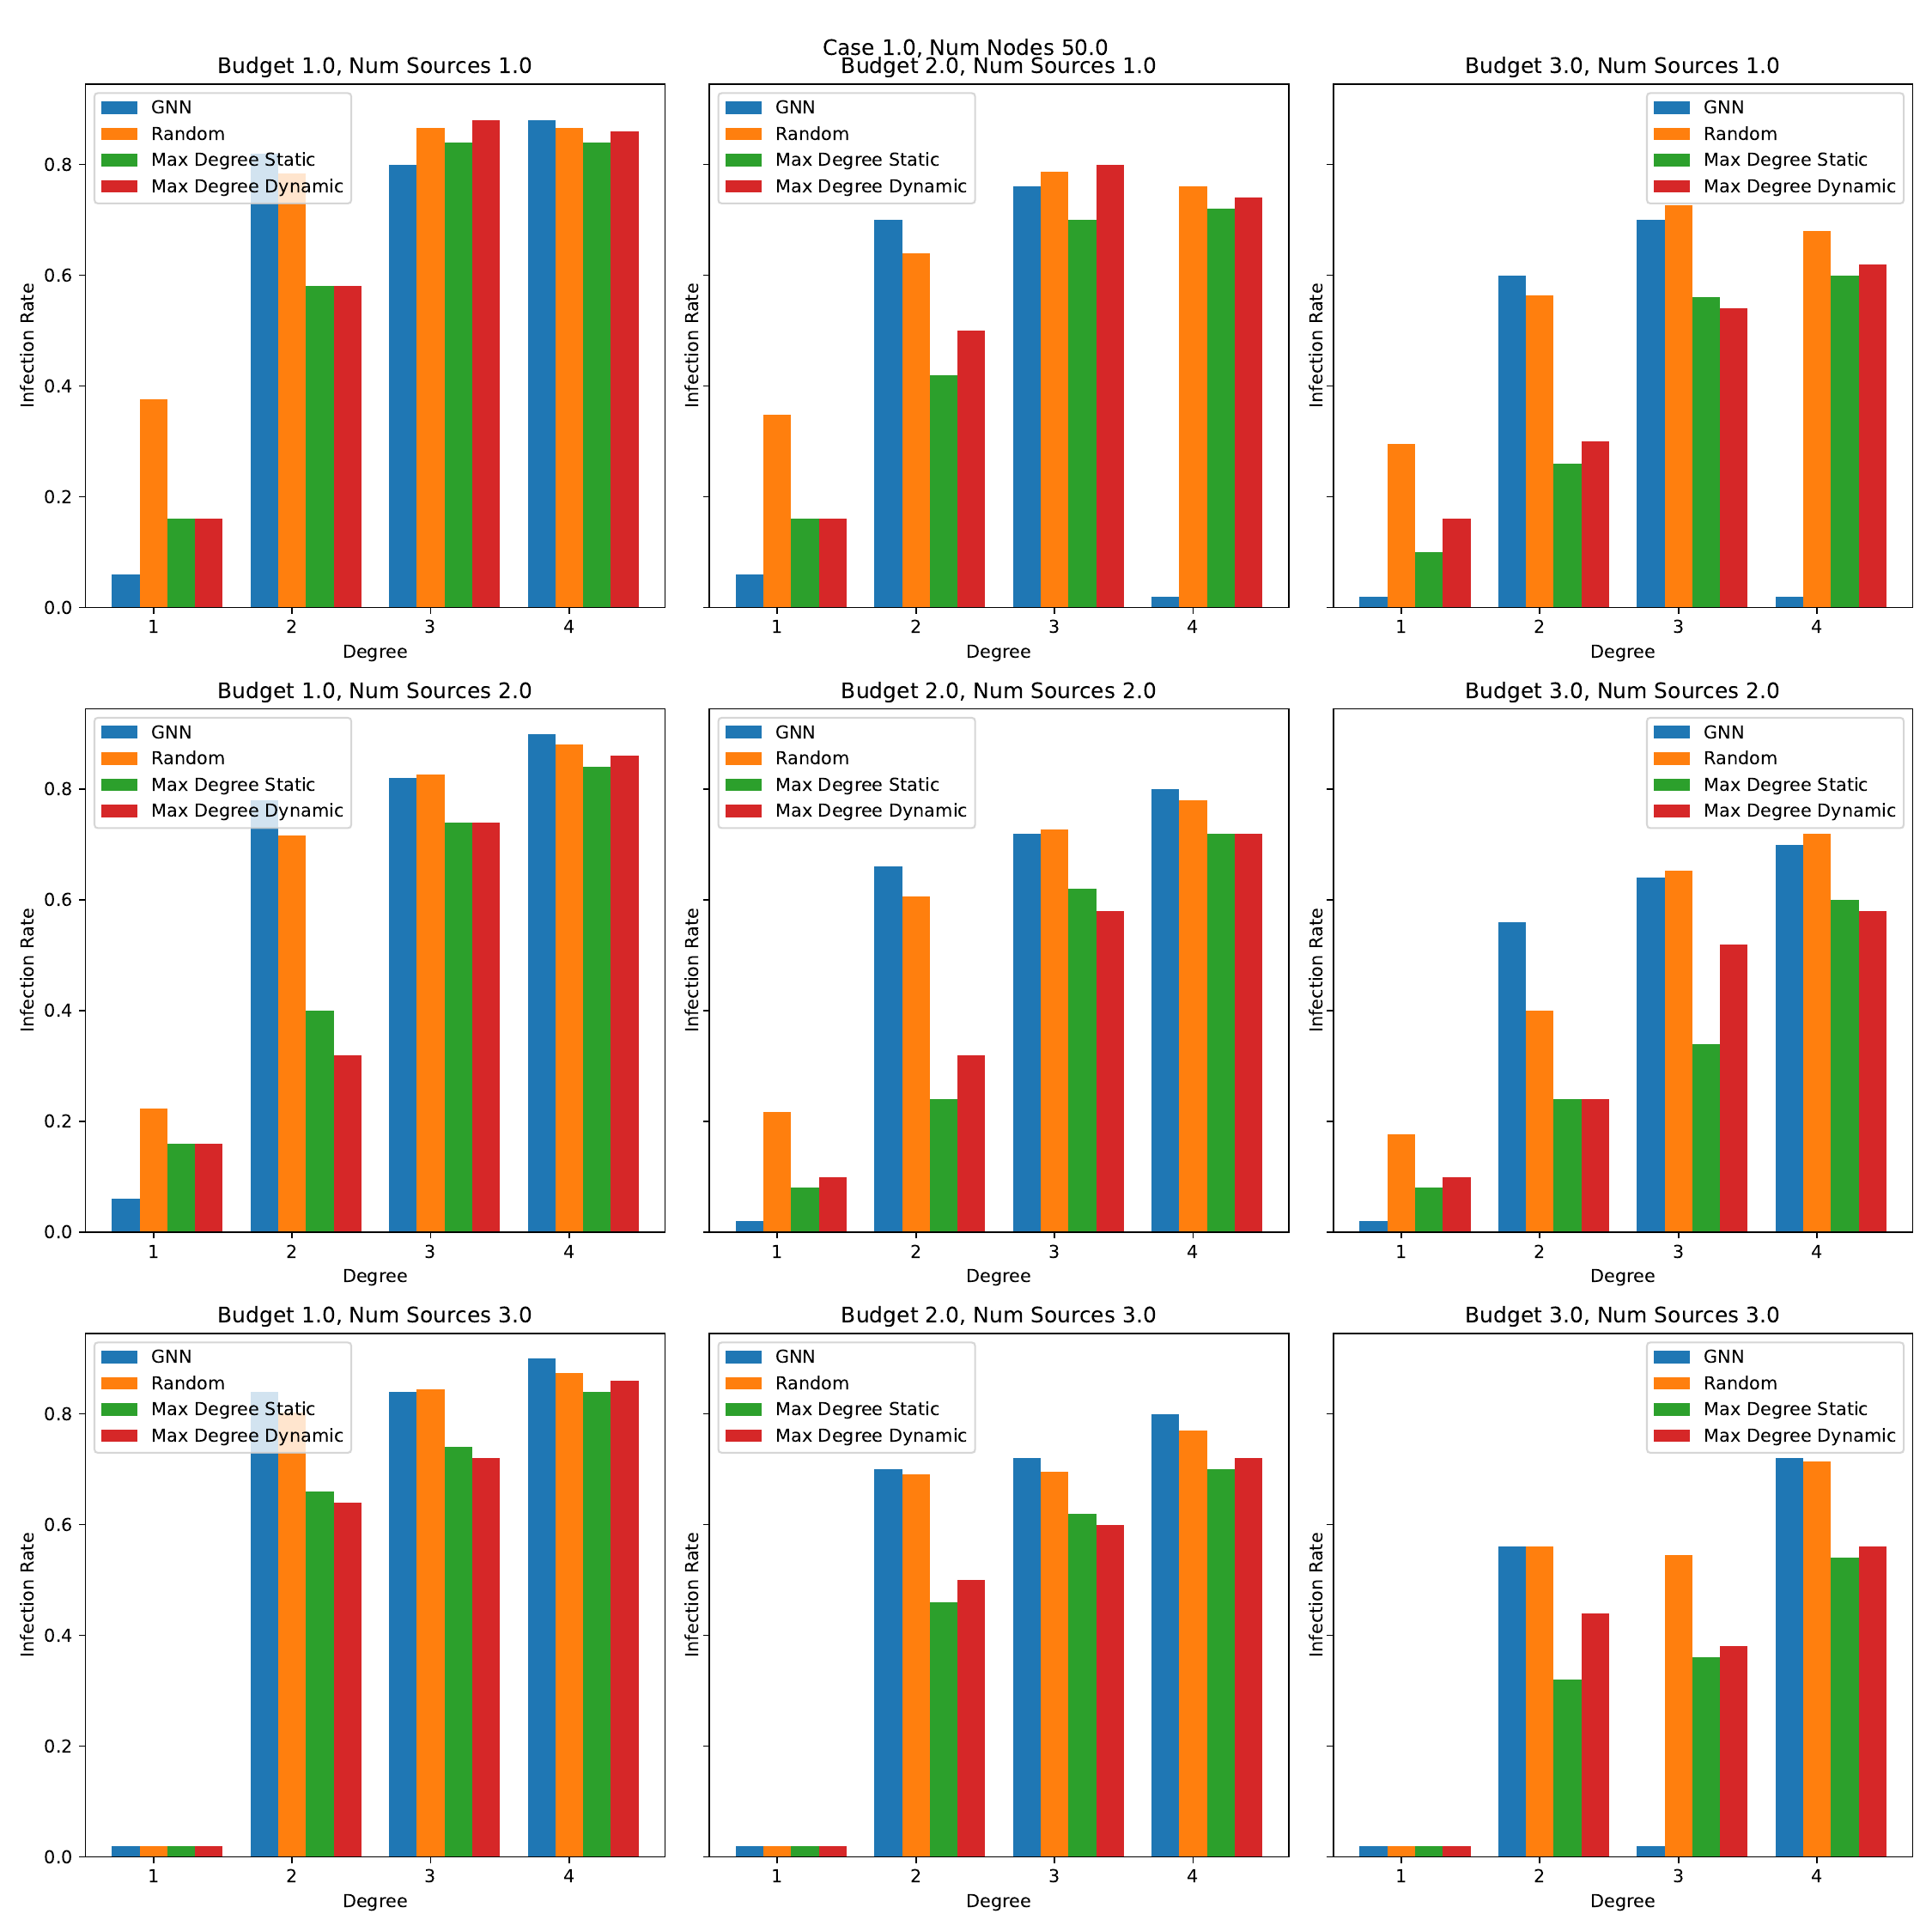}
    \caption{\footnotesize Dataset: Erdos-Renyi, Case-1 Node-50: Performance Evaluation of GCN-Based Supervised Learning Model: This series of bar plots presents a comparative analysis between our GCN-based SL model (blue), Randomized Policy model(yellow), Max Degree Policy model (Static) (green) and Max Degree Policy model (Dynamic) (red) on 25-node network environment. Progressing from left to right, the plots depict scenarios with increasing action budgets, ranging from 1 to 3 actions permitted. Vertically, the plots are ordered to show the effect of varying the initial count of infected nodes, starting with one and increasing to three. Each set of bars within the plots is categorized by the average connectivity (degree) of the infected nodes.}
    \label{fig:ERc1n50}
\end{figure}

% ######## Case 2 #########

\begin{figure}[!h]
    \centering
    \includegraphics[scale=0.3]{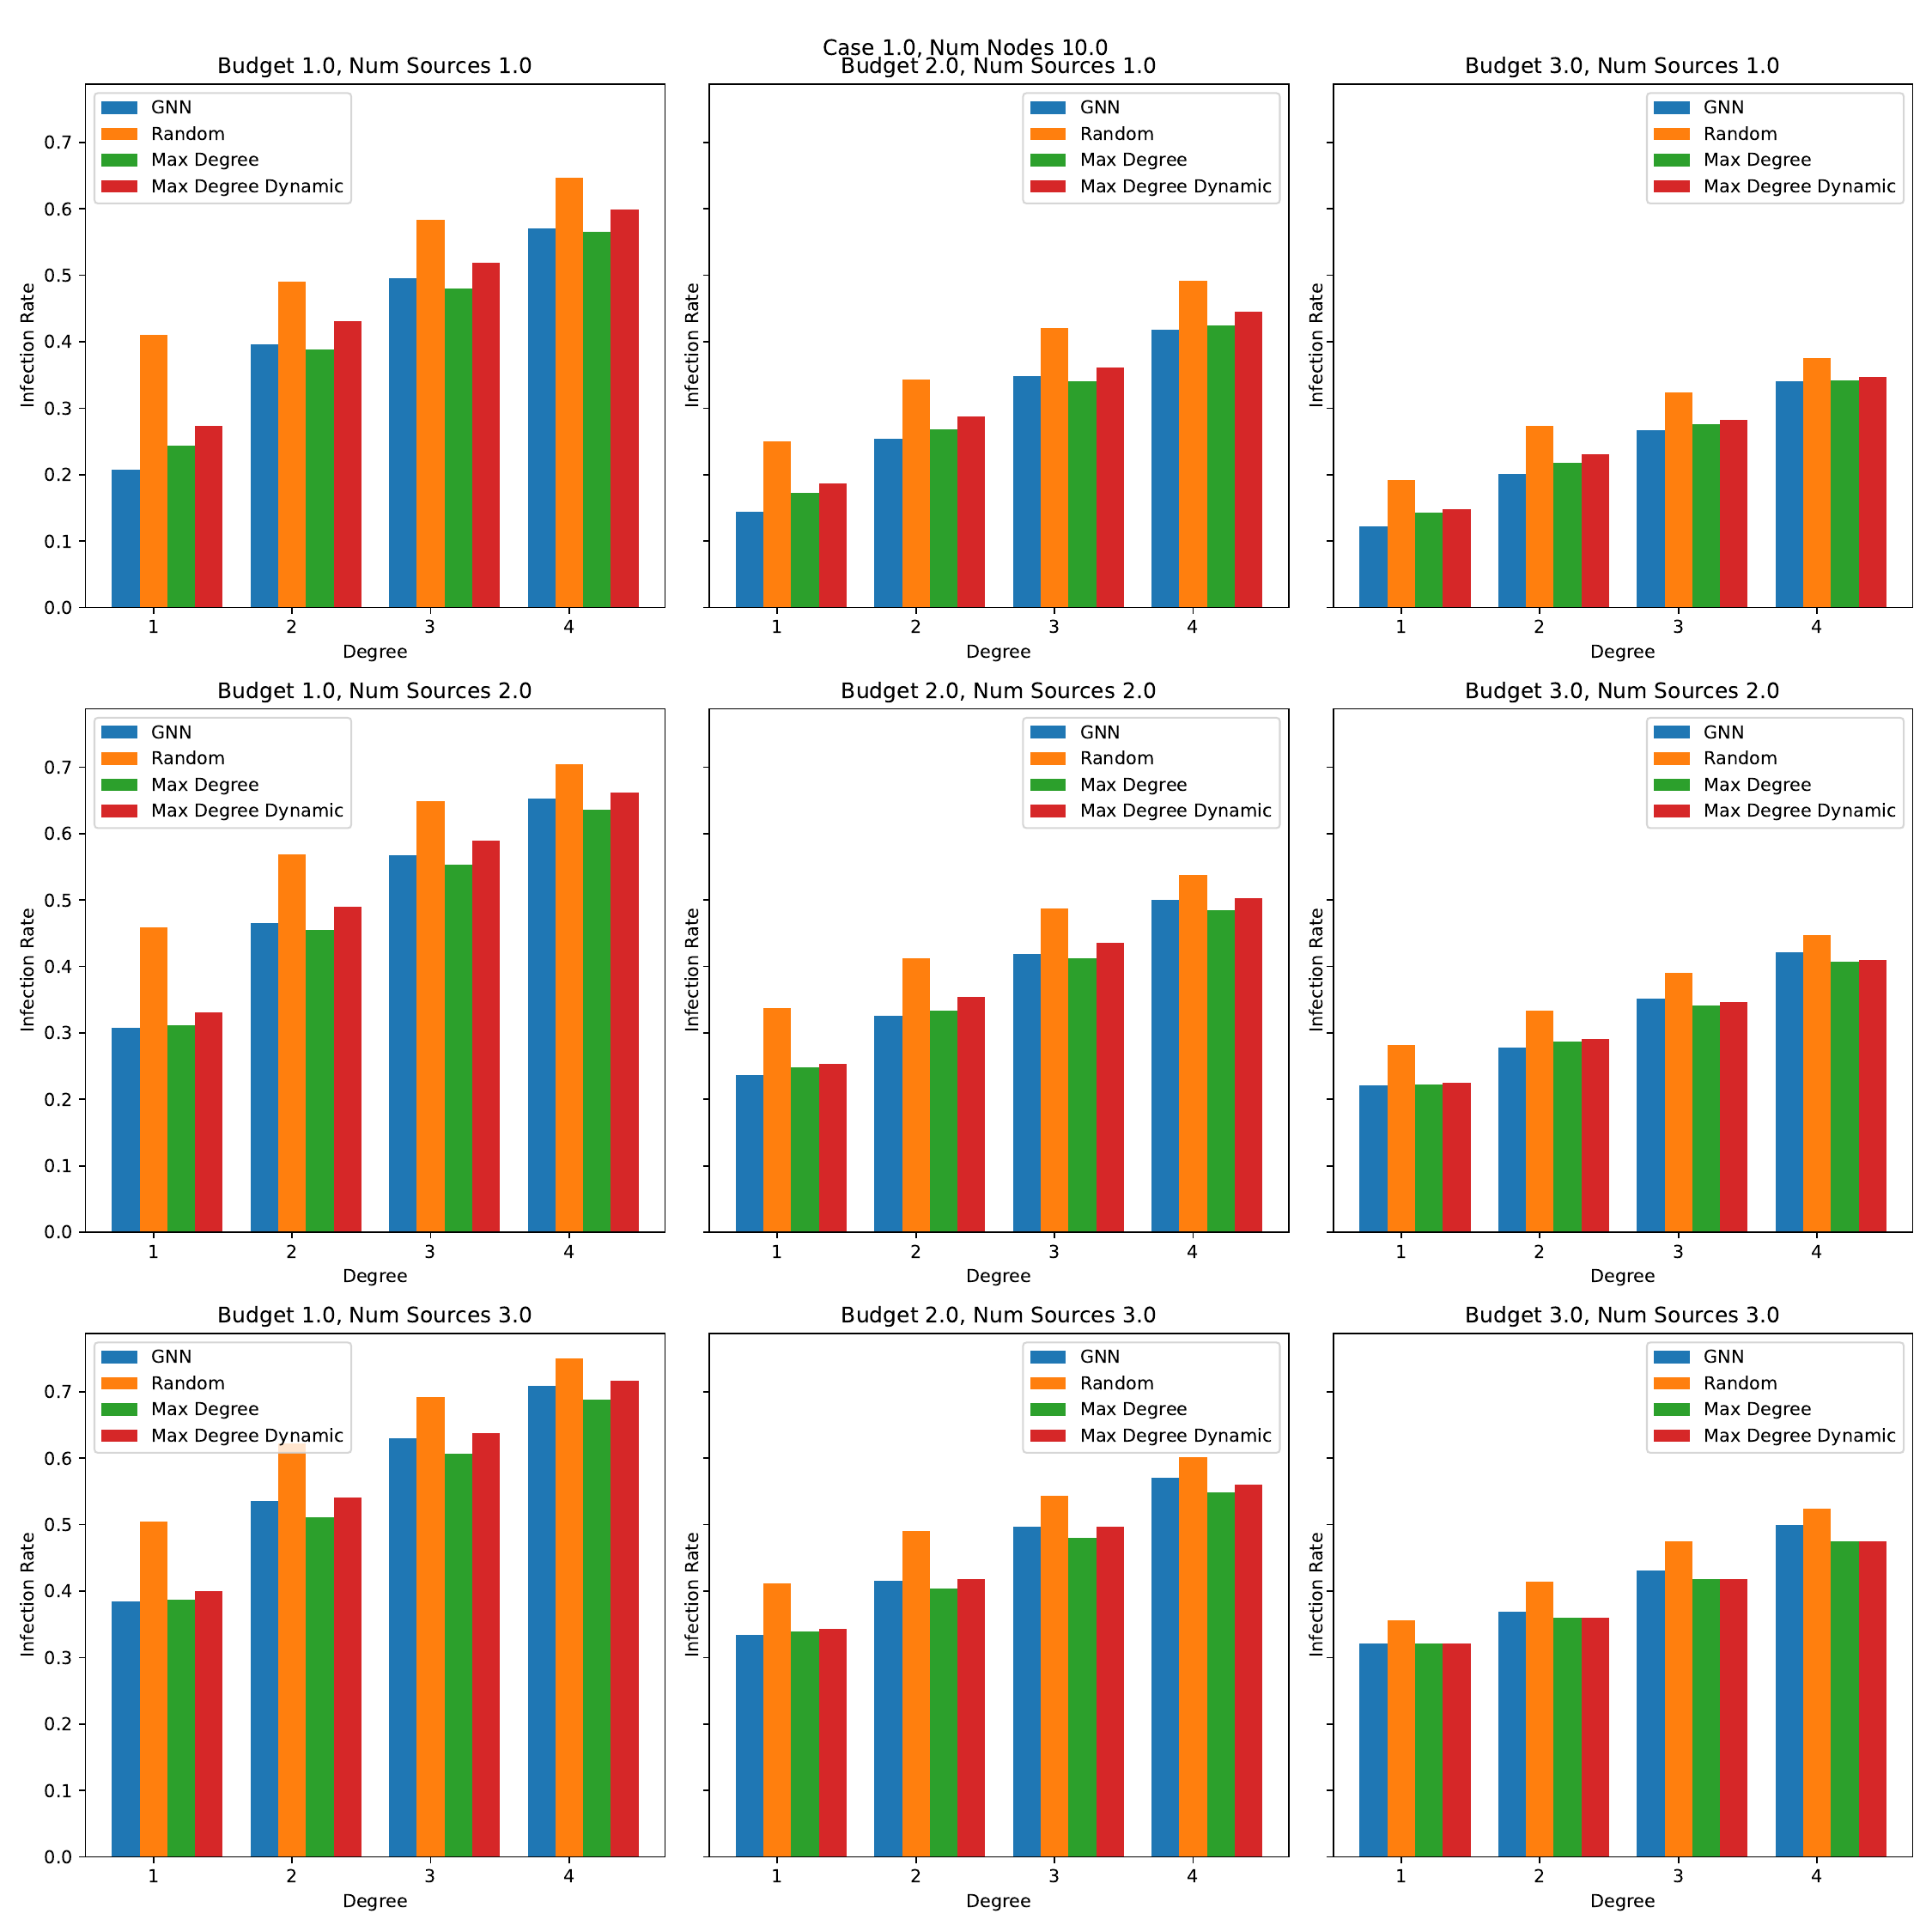}
    \caption{\footnotesize Dataset: Watts-Strogatz, Case-2 Node-10: Performance Evaluation of GCN-Based Supervised Learning Model: This series of bar plots presents a comparative analysis between our GCN-based SL model (blue), Randomized Policy model(yellow), Max Degree Policy model (Static) (green) and Max Degree Policy model (Dynamic) (red) on 10-node network environment. Progressing from left to right, the plots depict scenarios with increasing action budgets, ranging from 1 to 3 actions permitted. Vertically, the plots are ordered to show the effect of varying the initial count of infected nodes, starting with one and increasing to three. Each set of bars within the plots is categorized by the average connectivity (degree) of the infected nodes.}
    \label{fig:c2n10}
\end{figure}

\begin{figure}[!h]
    \centering
    \includegraphics[scale=0.3]{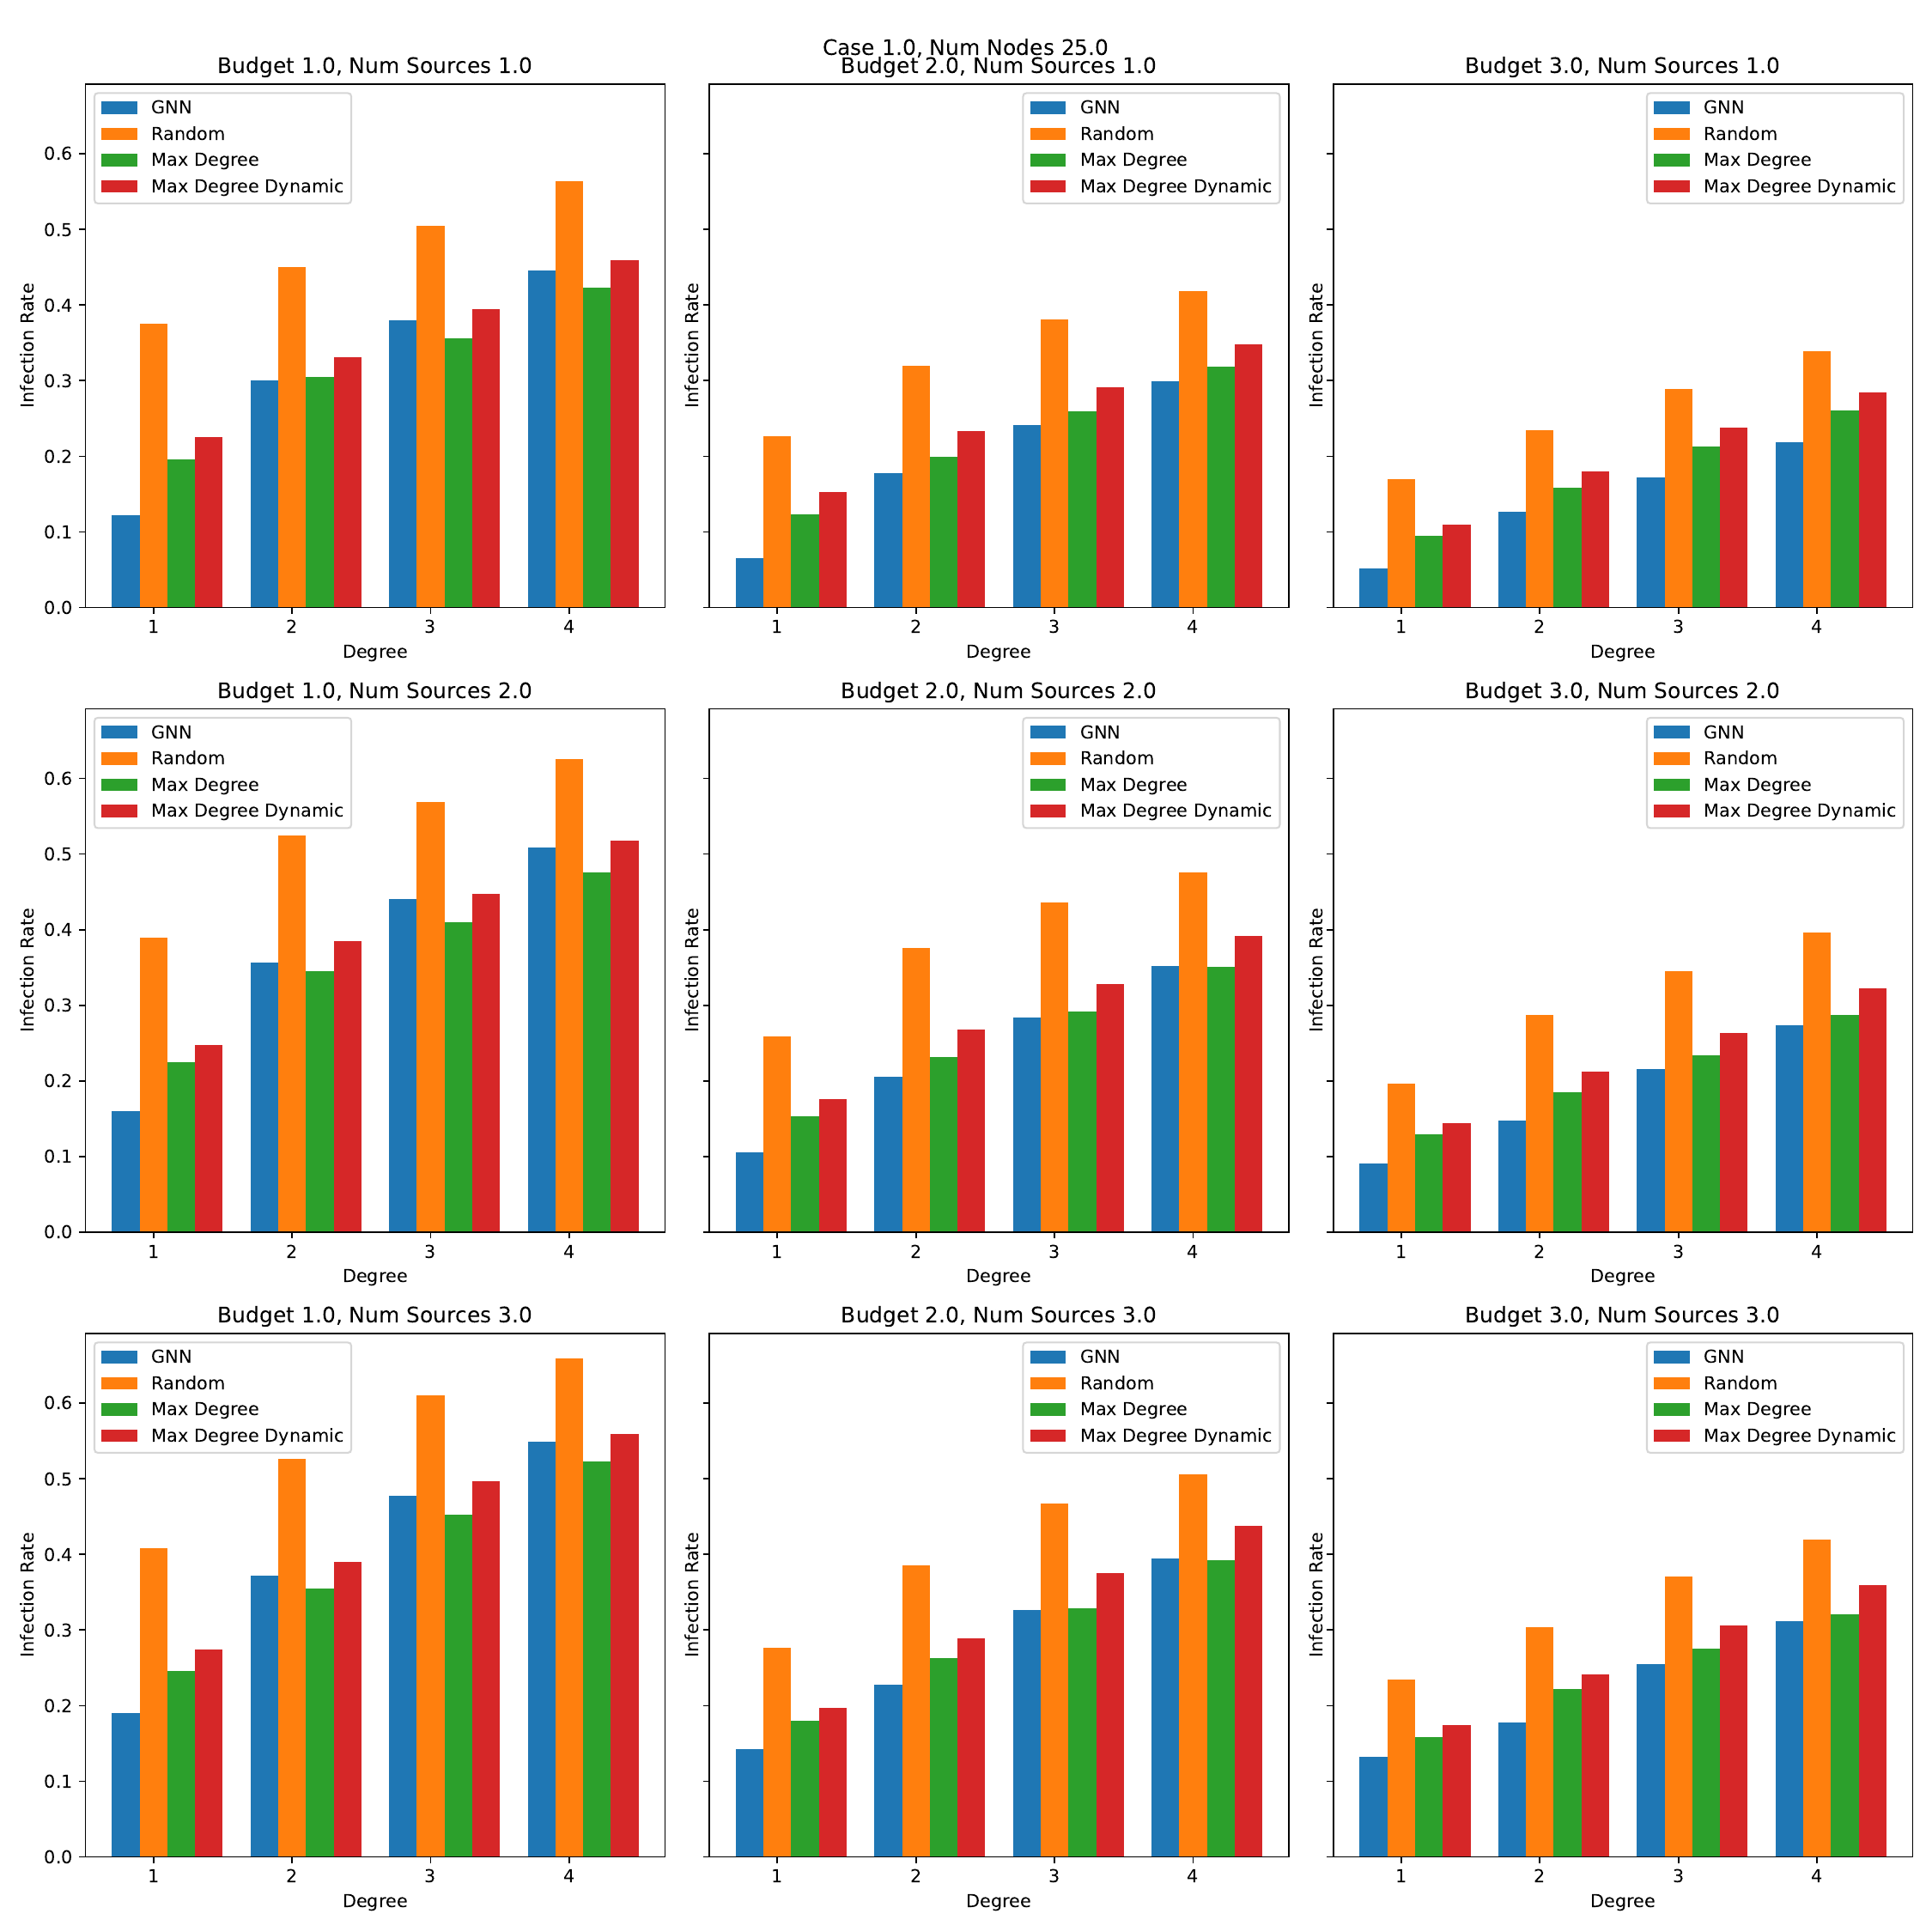}
    \caption{\footnotesize Dataset: Watts-Strogatz, Case-2 Node-25: Performance Evaluation of GCN-Based Supervised Learning Model: This series of bar plots presents a comparative analysis between our GCN-based SL model (blue), Randomized Policy model(yellow), Max Degree Policy model (Static) (green) and Max Degree Policy model (Dynamic) (red) on 25-node network environment. Progressing from left to right, the plots depict scenarios with increasing action budgets, ranging from 1 to 3 actions permitted. Vertically, the plots are ordered to show the effect of varying the initial count of infected nodes, starting with one and increasing to three. Each set of bars within the plots is categorized by the average connectivity (degree) of the infected nodes.}
    \label{fig:c2n25}
\end{figure}

\begin{figure}[!h]
    \centering
    \includegraphics[scale=0.3]{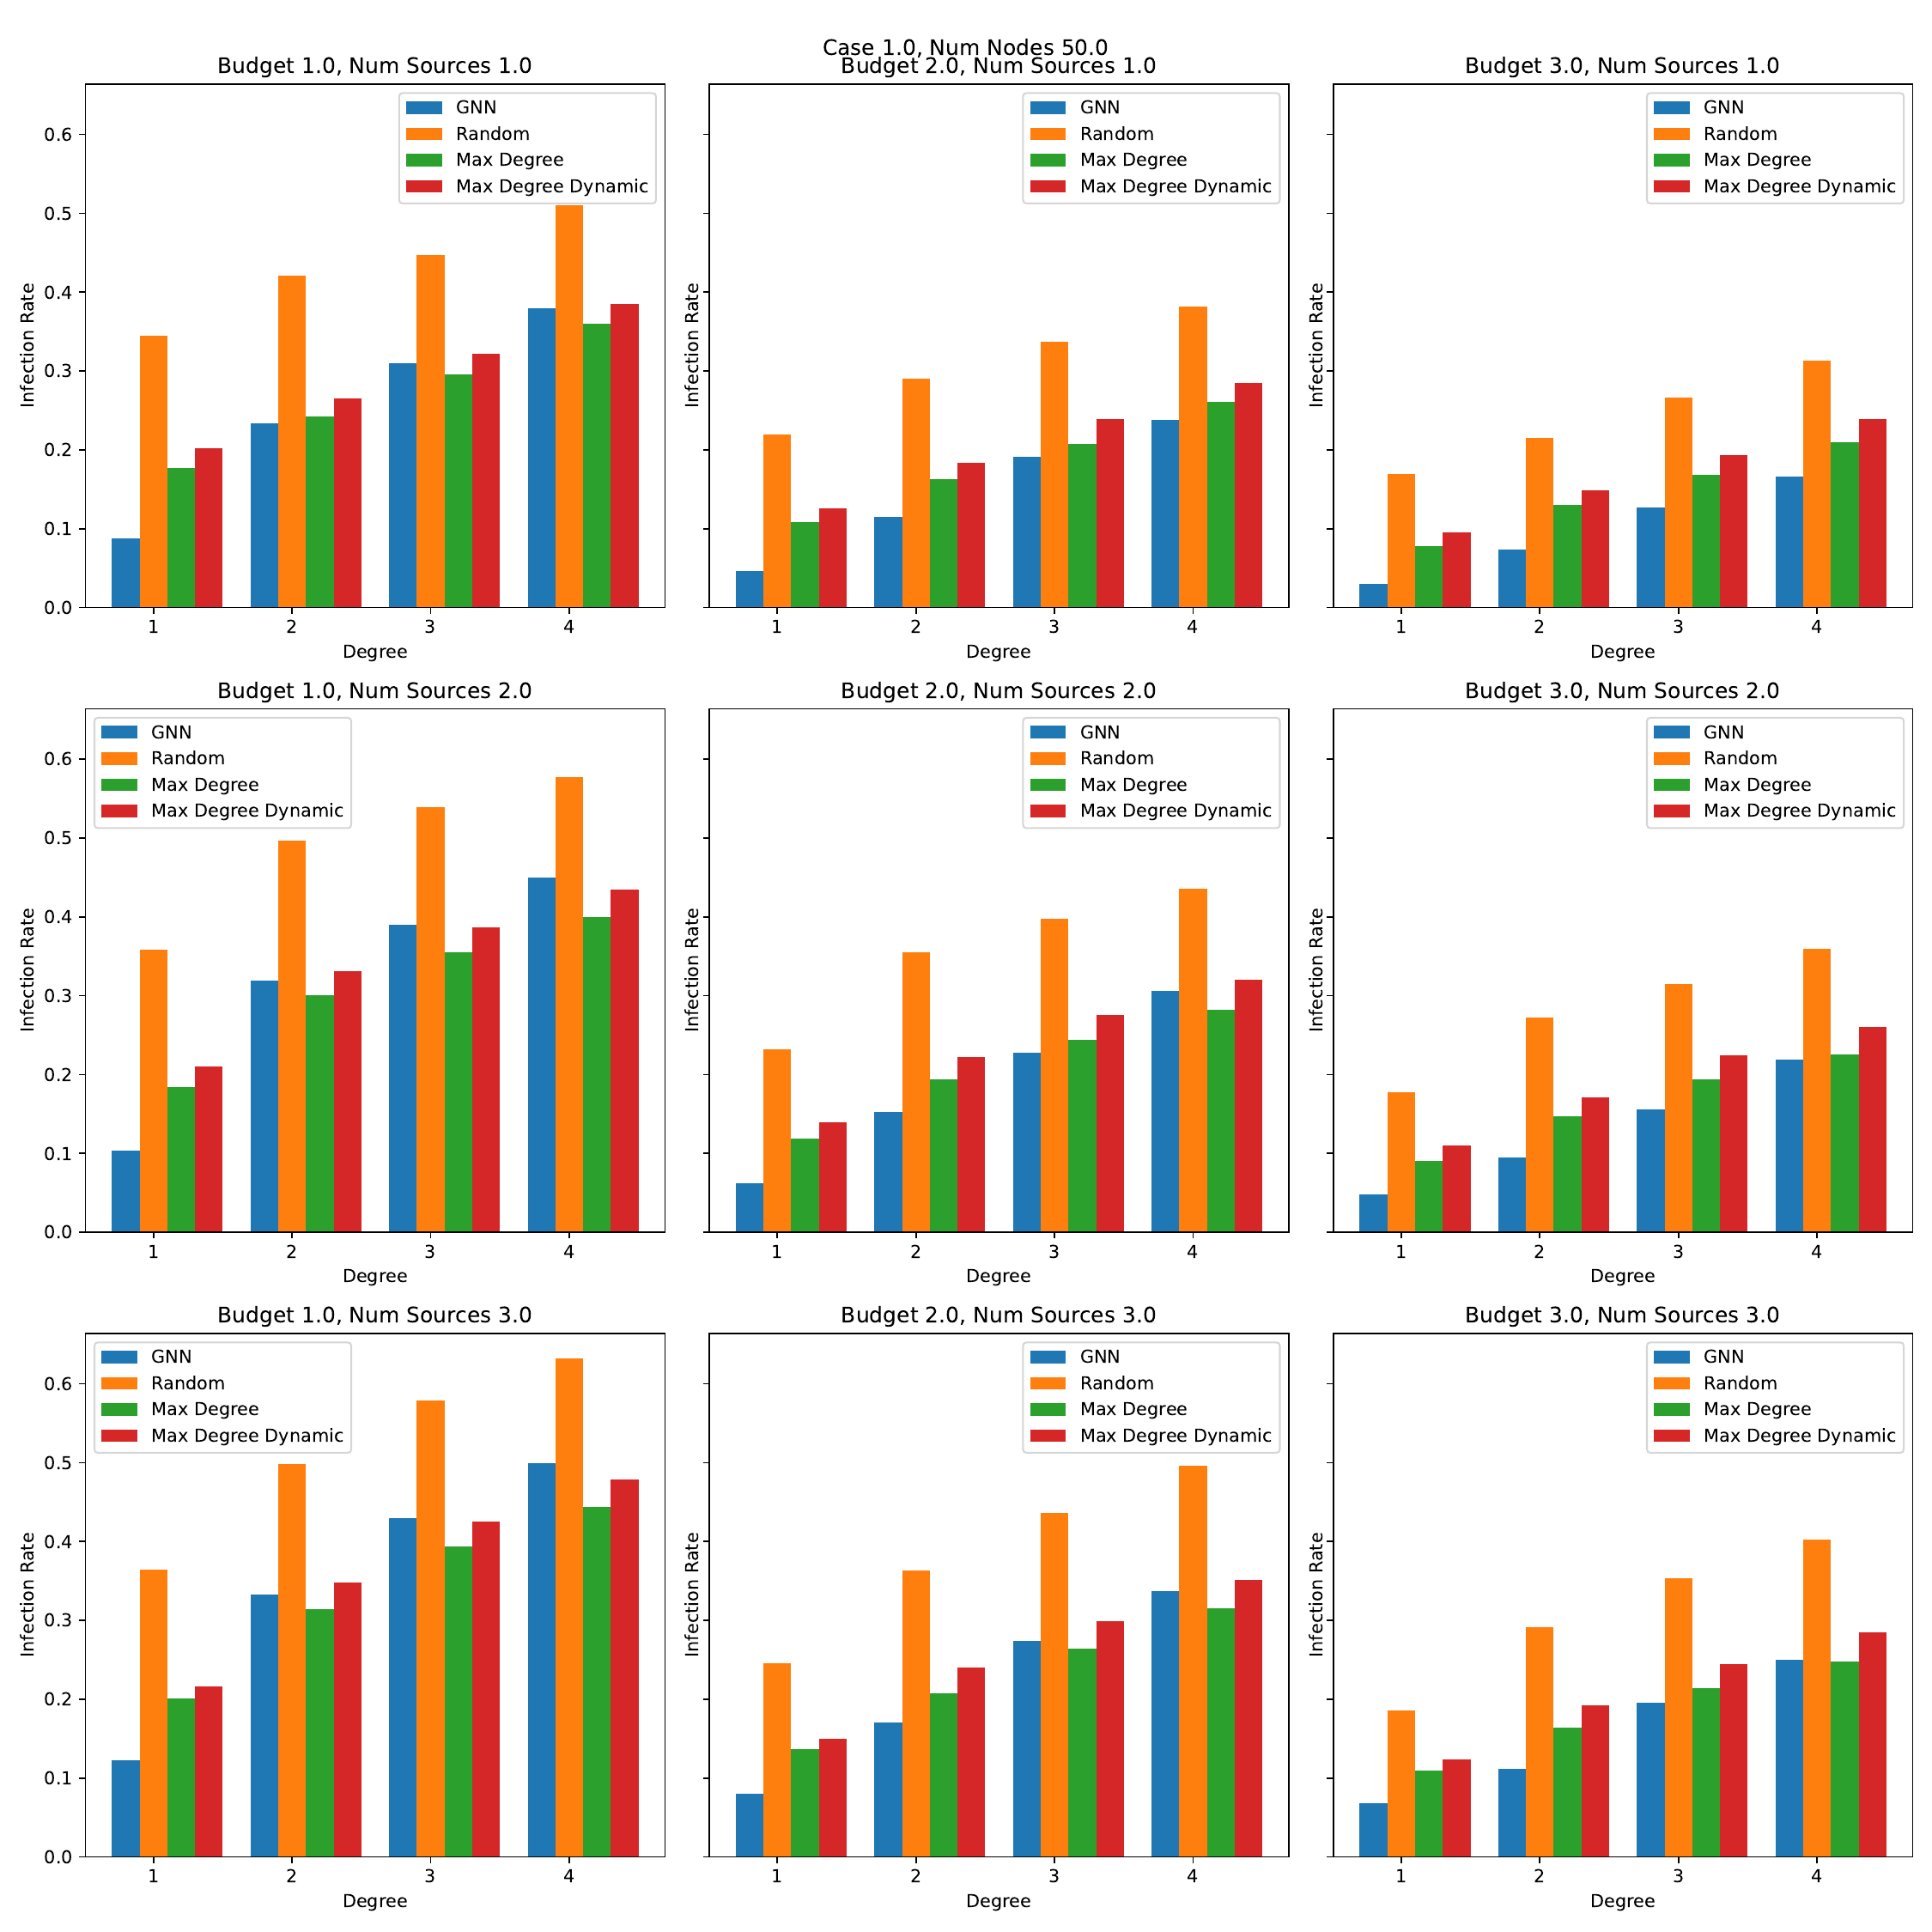}
    \caption{\footnotesize Dataset: Watts-Strogatz, Case-2 Node-50: Performance Evaluation of GCN-Based Supervised Learning Model: This series of bar plots presents a comparative analysis between our GCN-based SL model (blue), Randomized Policy model(yellow), Max Degree Policy model (Static) (green) and Max Degree Policy model (Dynamic) (red) on 50-node network environment. Progressing from left to right, the plots depict scenarios with increasing action budgets, ranging from 1 to 3 actions permitted. Vertically, the plots are ordered to show the effect of varying the initial count of infected nodes, starting with one and increasing to three. Each set of bars within the plots is categorized by the average connectivity (degree) of the infected nodes.}
    \label{fig:c2n50}
\end{figure}

\begin{figure}[!h]
    \centering
    \includegraphics[scale=0.3]{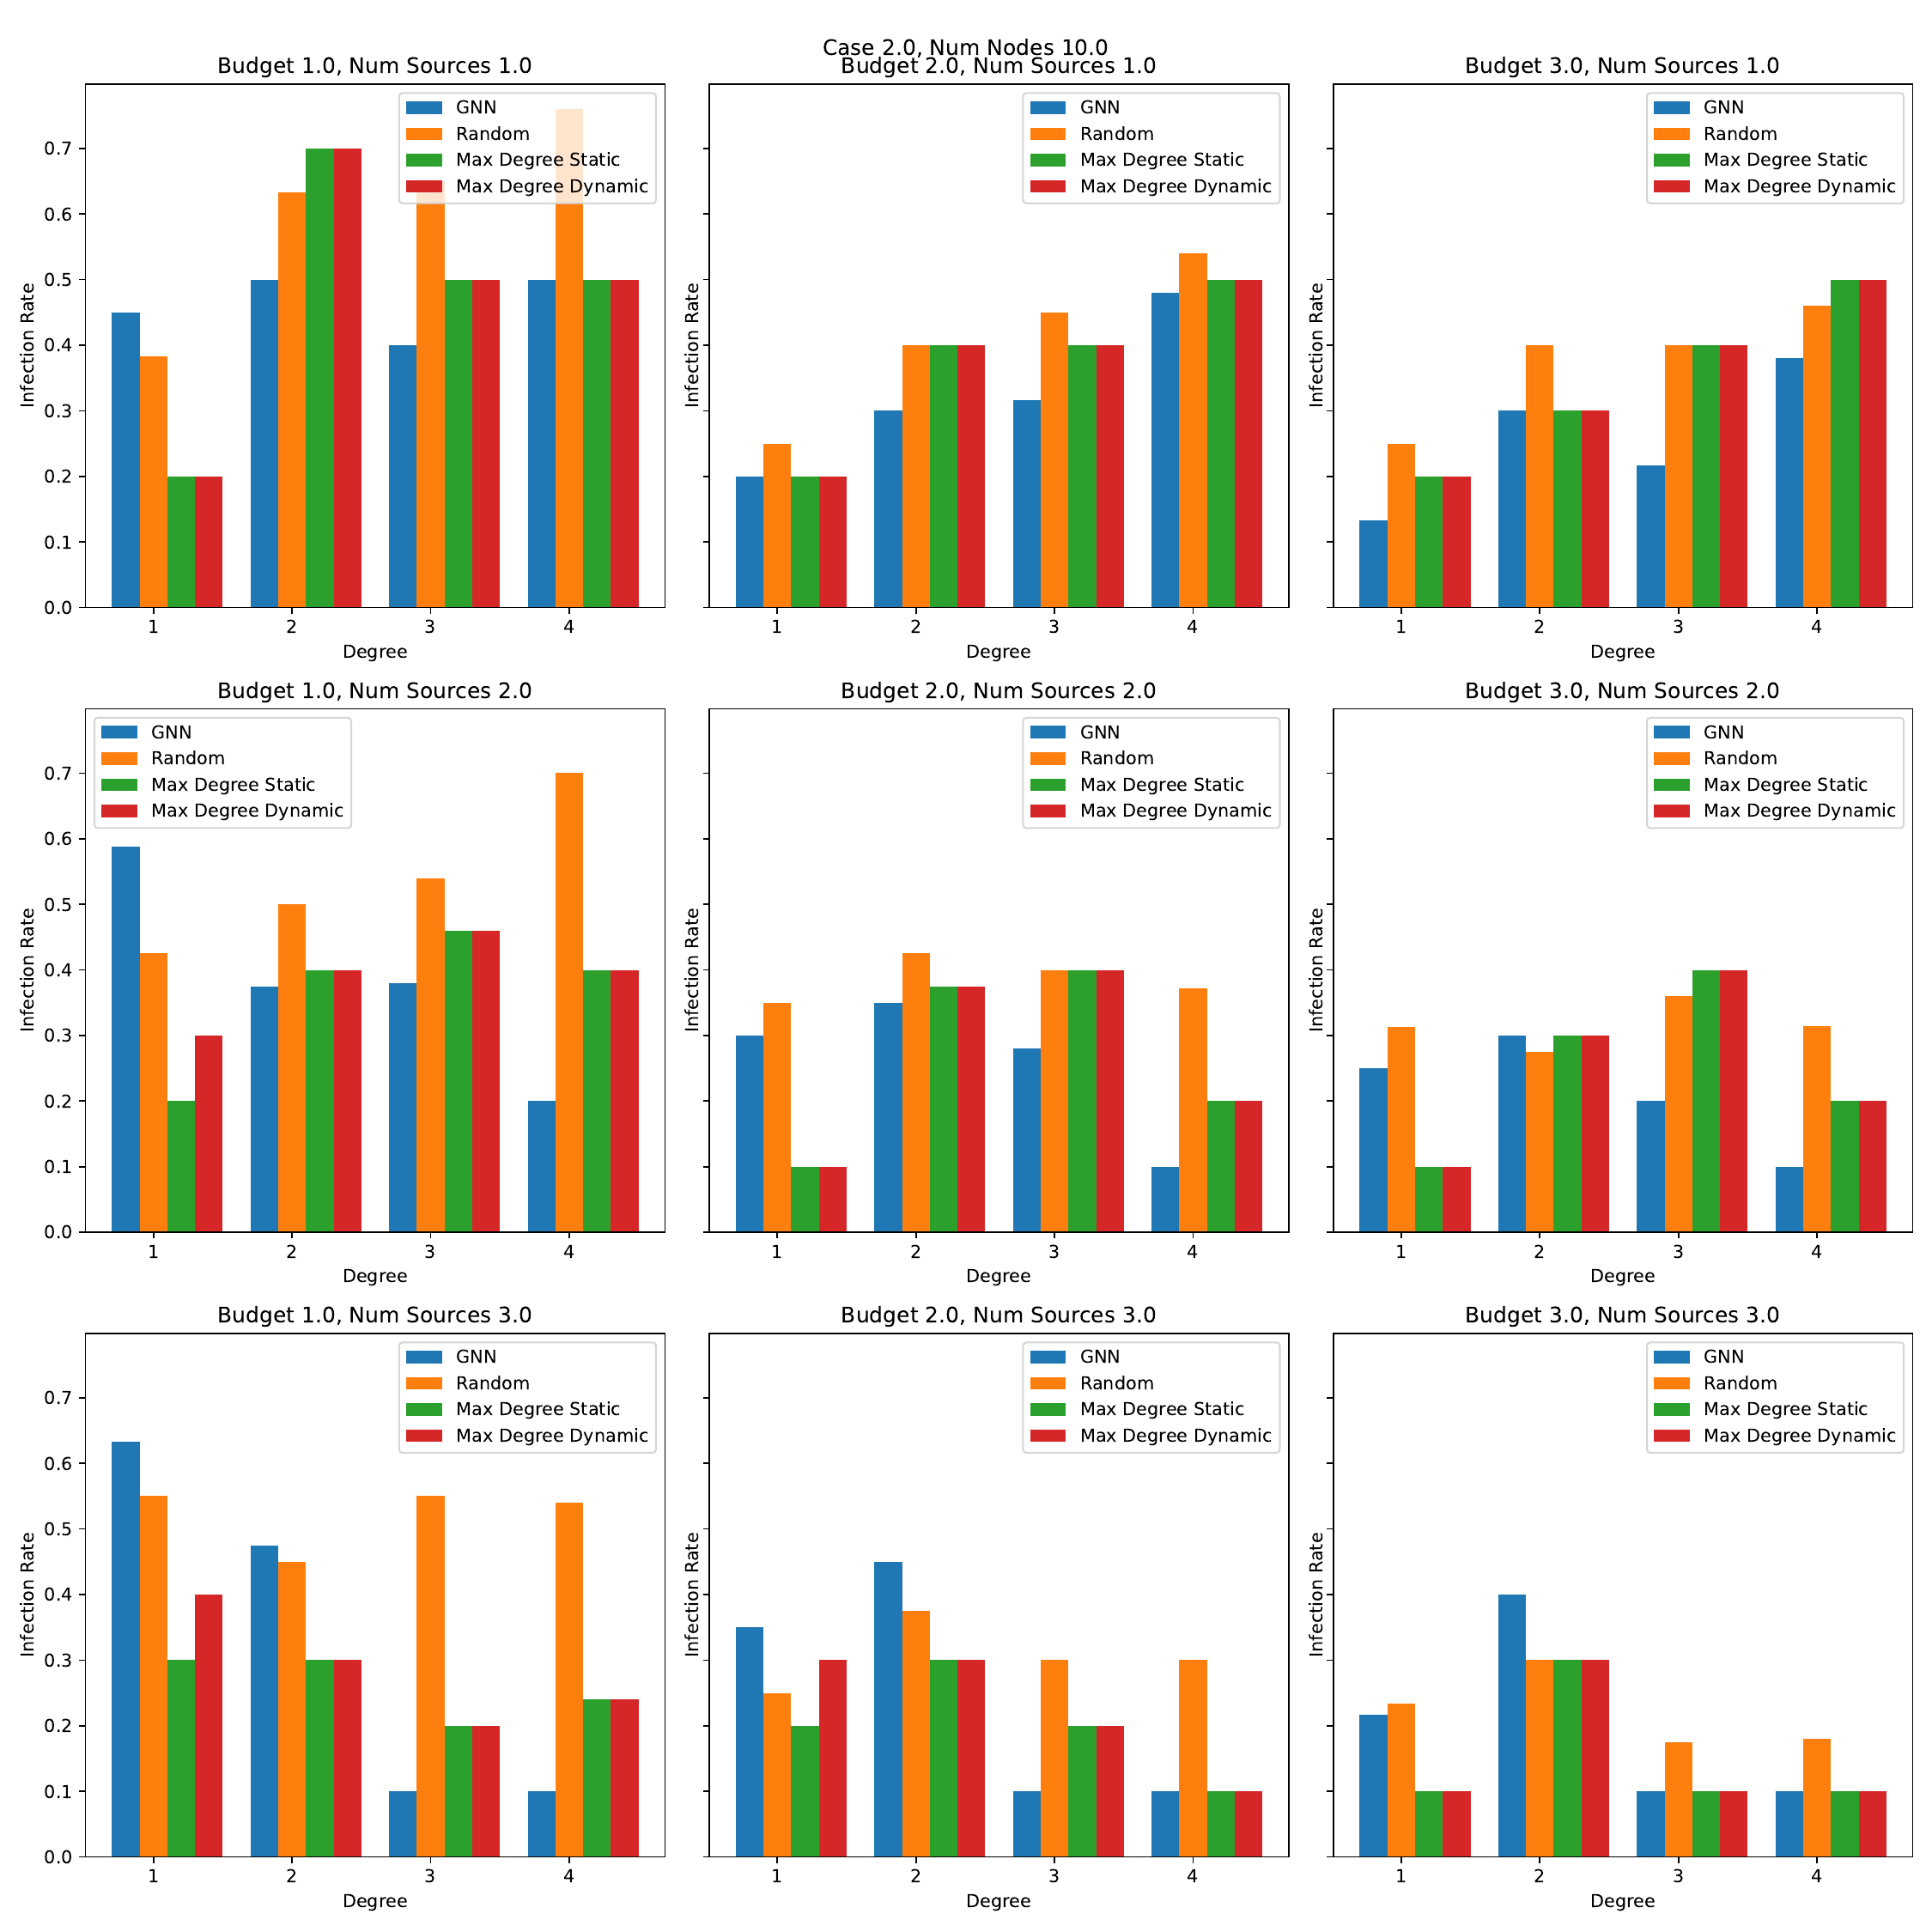}
    \caption{\footnotesize Dataset: Tree, Case-2 Node-10: Performance Evaluation of GCN-Based Supervised Learning Model: This series of bar plots presents a comparative analysis between our GCN-based SL model (blue), Randomized Policy model(yellow), Max Degree Policy model (Static) (green) and Max Degree Policy model (Dynamic) (red) on 10-node network environment. Progressing from left to right, the plots depict scenarios with increasing action budgets, ranging from 1 to 3 actions permitted. Vertically, the plots are ordered to show the effect of varying the initial count of infected nodes, starting with one and increasing to three. Each set of bars within the plots is categorized by the average connectivity (degree) of the infected nodes.}
    \label{fig:Treec2n10}
\end{figure}

\begin{figure}[!h]
    \centering
    \includegraphics[scale=0.3]{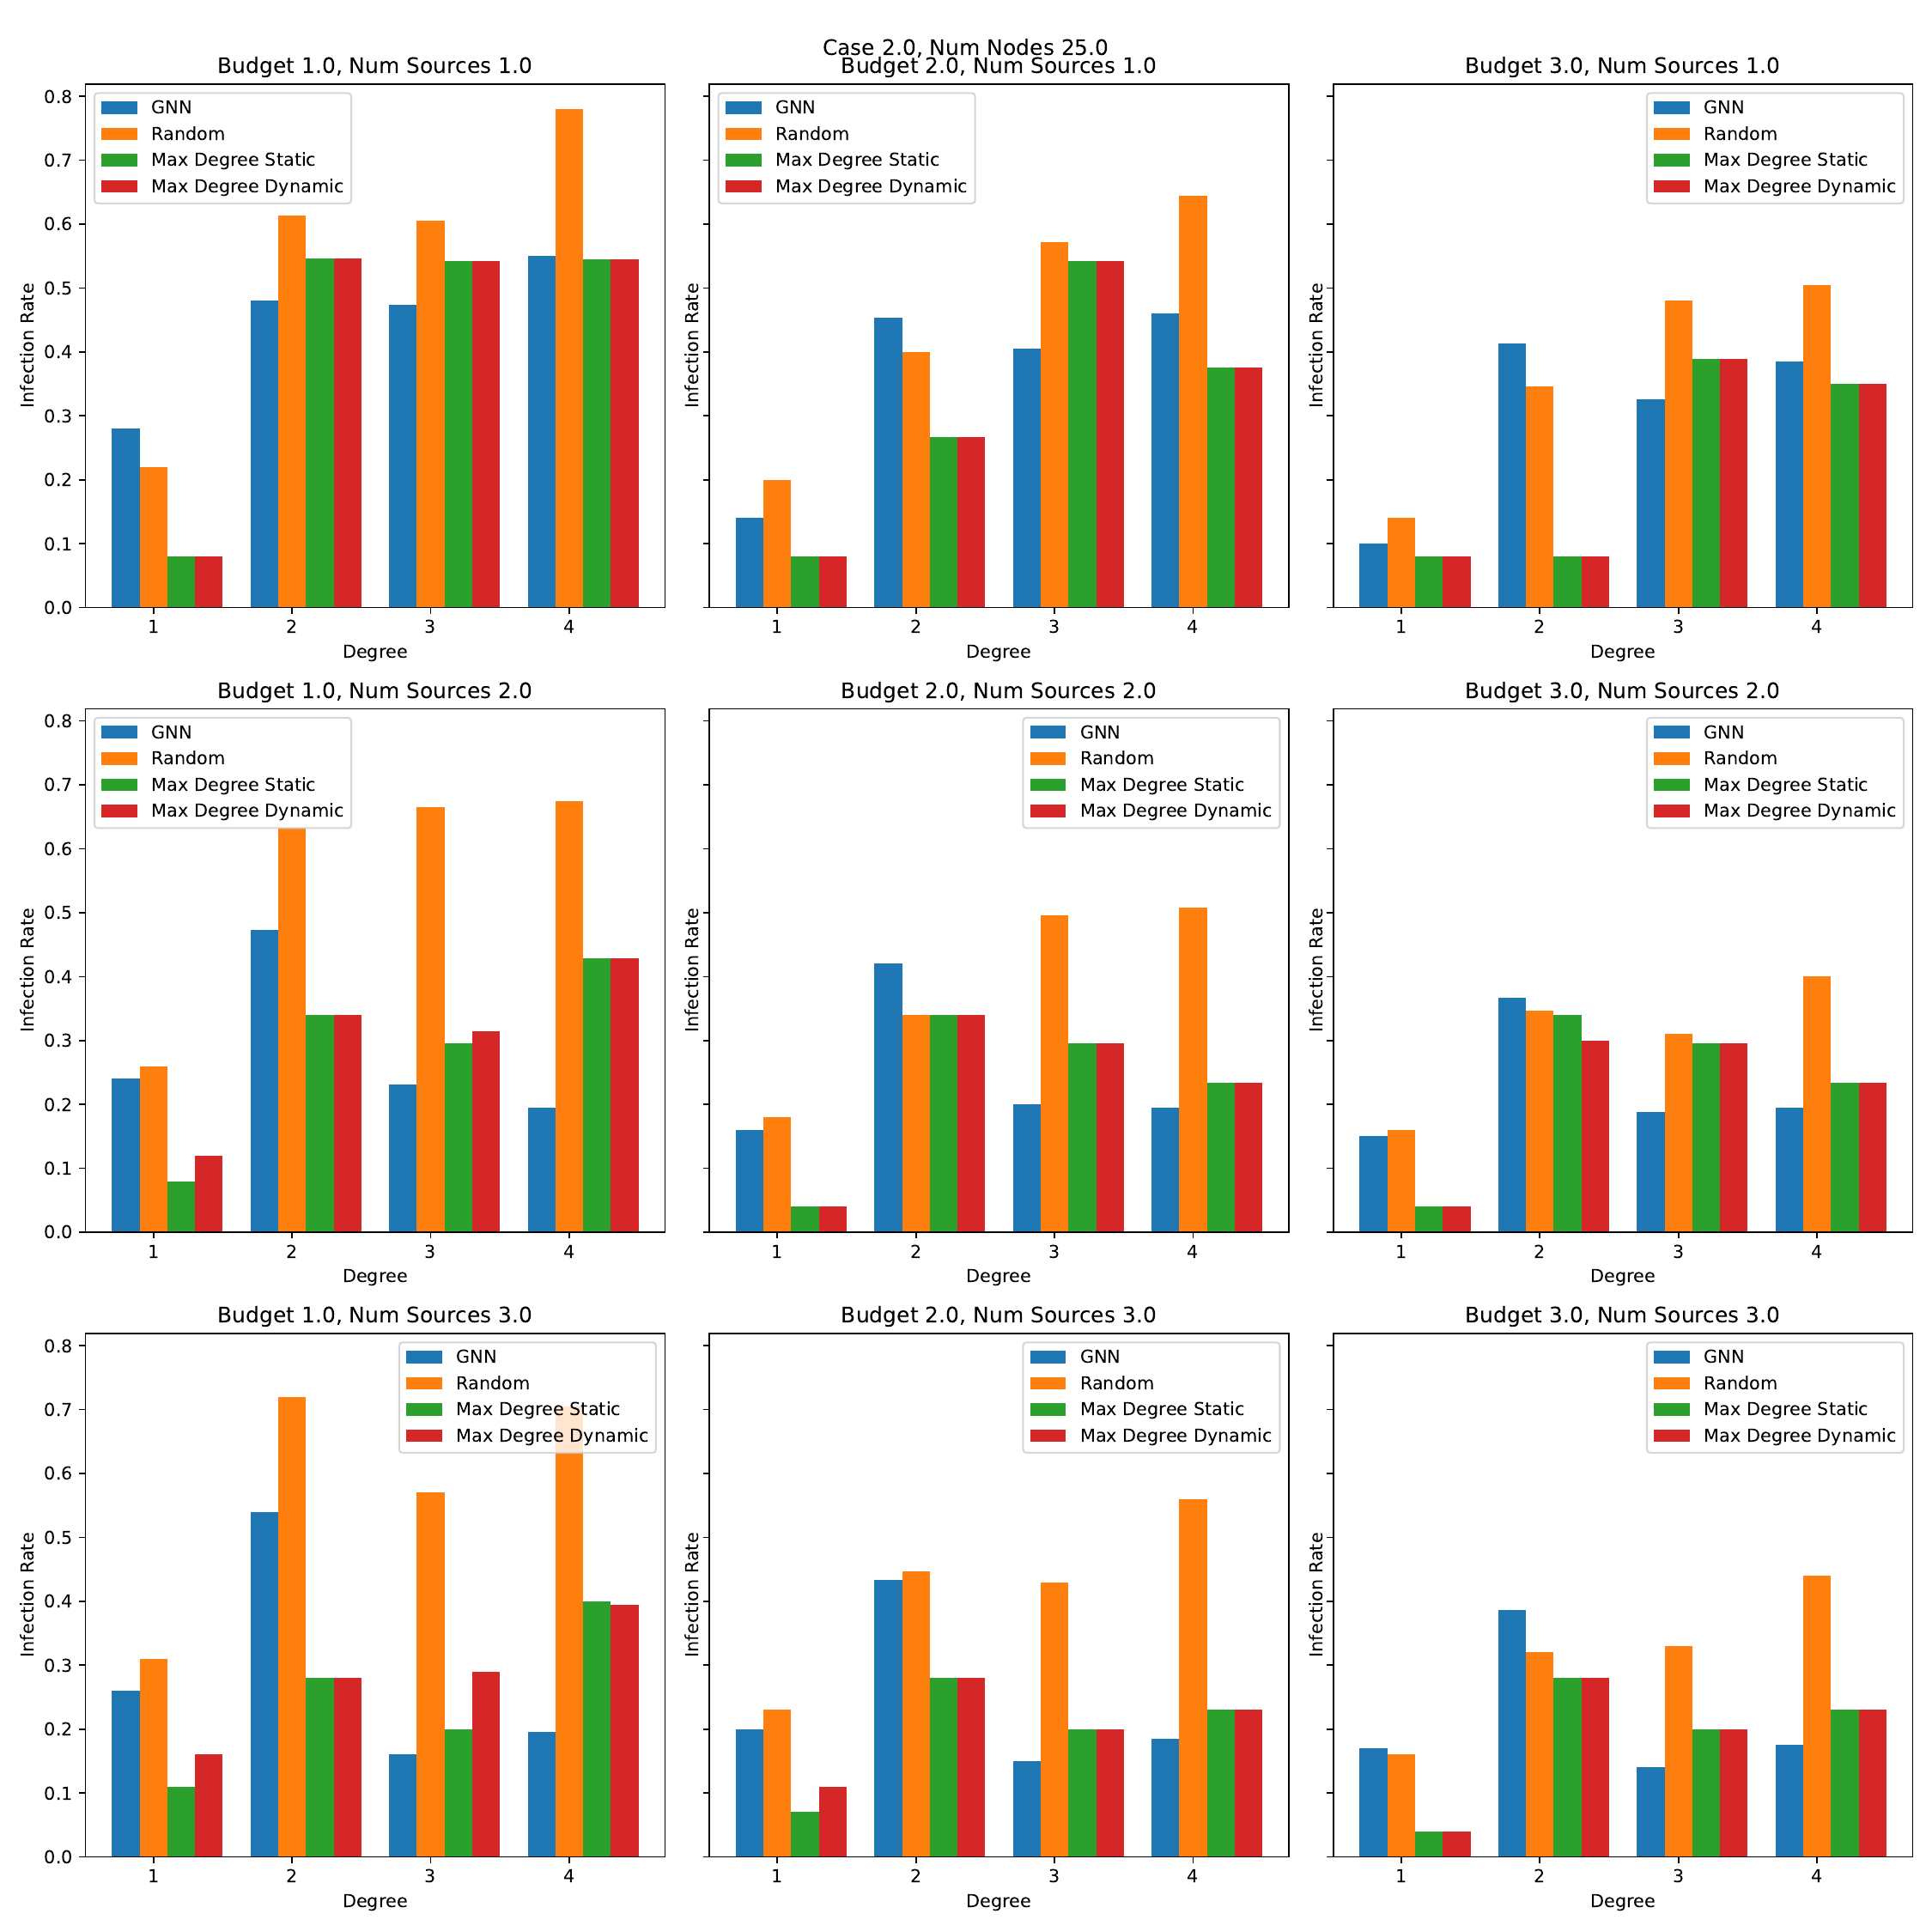}
    \caption{\footnotesize Dataset: Tree, Case-2 Node-25: Performance Evaluation of GCN-Based Supervised Learning Model: This series of bar plots presents a comparative analysis between our GCN-based SL model (blue), Randomized Policy model(yellow), Max Degree Policy model (Static) (green) and Max Degree Policy model (Dynamic) (red) on 25-node network environment. Progressing from left to right, the plots depict scenarios with increasing action budgets, ranging from 1 to 3 actions permitted. Vertically, the plots are ordered to show the effect of varying the initial count of infected nodes, starting with one and increasing to three. Each set of bars within the plots is categorized by the average connectivity (degree) of the infected nodes.}
    \label{fig:Treec2n25}
\end{figure}

\begin{figure}[!h]
    \centering
    \includegraphics[scale=0.3]{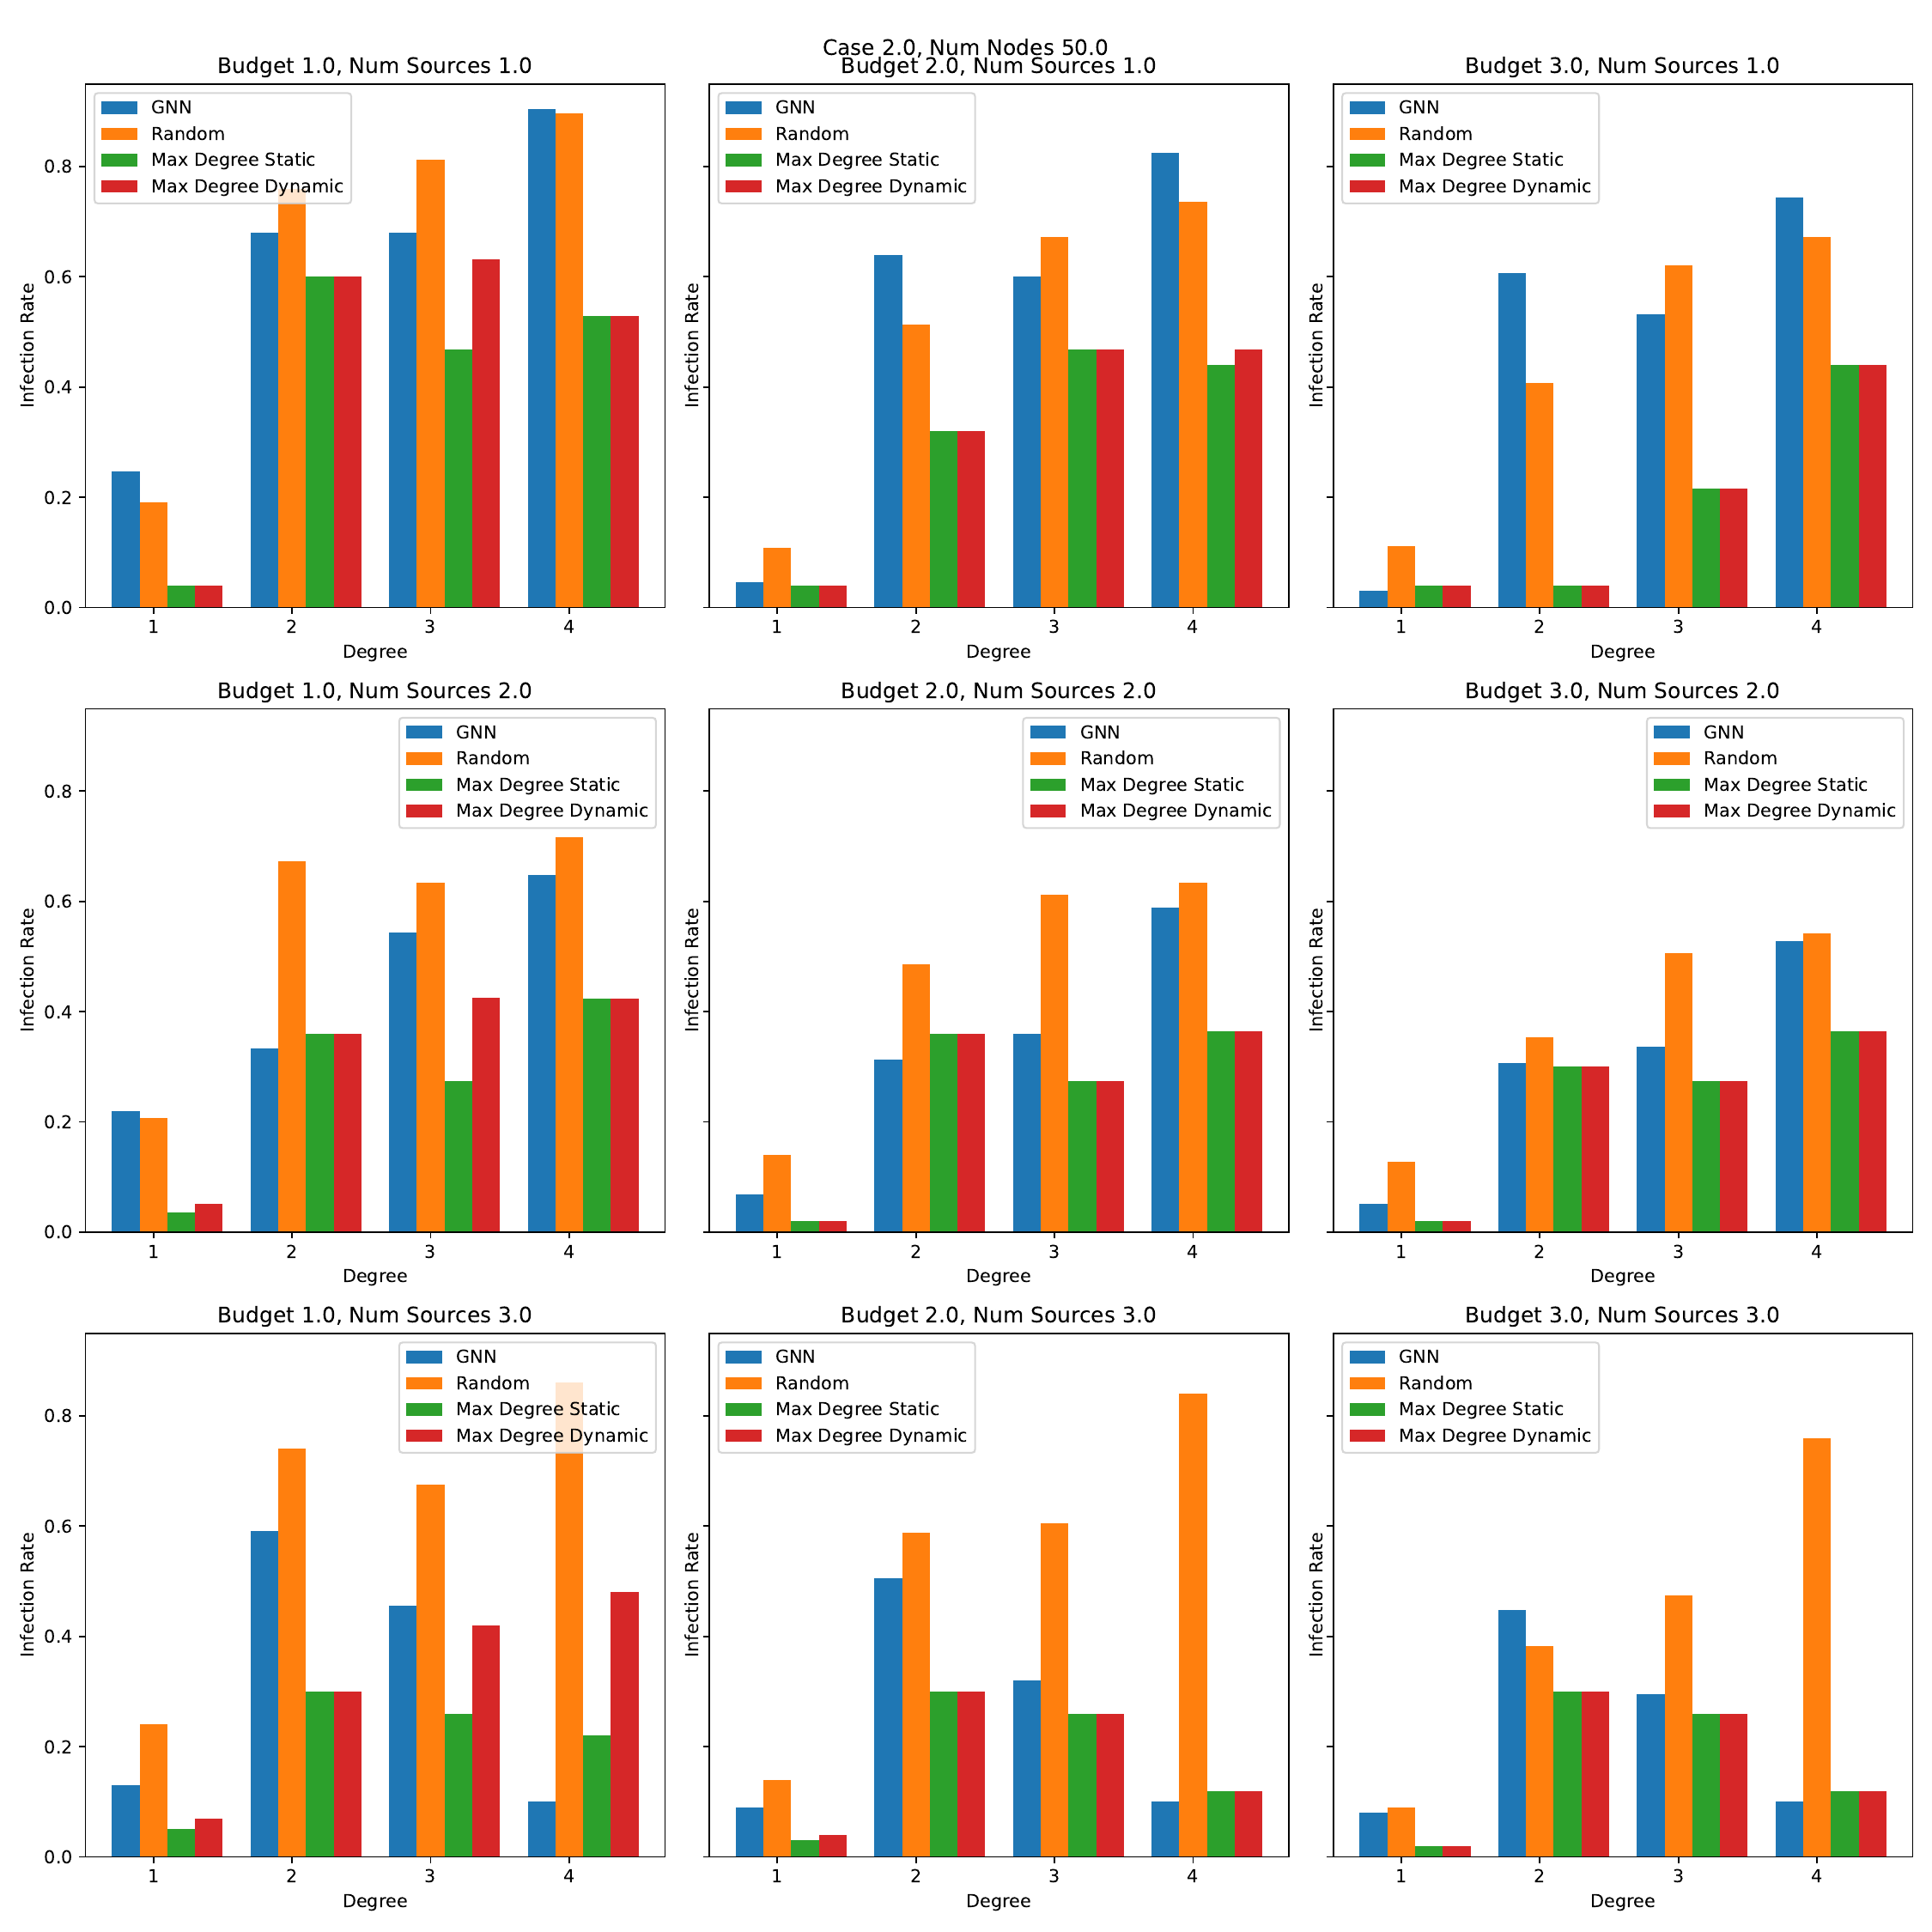}
    \caption{\footnotesize Dataset: Tree, Case-2 Node-50: Performance Evaluation of GCN-Based Supervised Learning Model: This series of bar plots presents a comparative analysis between our GCN-based SL model (blue), Randomized Policy model(yellow), Max Degree Policy model (Static) (green) and Max Degree Policy model (Dynamic) (red) on 25-node network environment. Progressing from left to right, the plots depict scenarios with increasing action budgets, ranging from 1 to 3 actions permitted. Vertically, the plots are ordered to show the effect of varying the initial count of infected nodes, starting with one and increasing to three. Each set of bars within the plots is categorized by the average connectivity (degree) of the infected nodes.}
    \label{fig:Treec2n50}
\end{figure}

\begin{figure}[!h]
    \centering
    \includegraphics[scale=0.3]{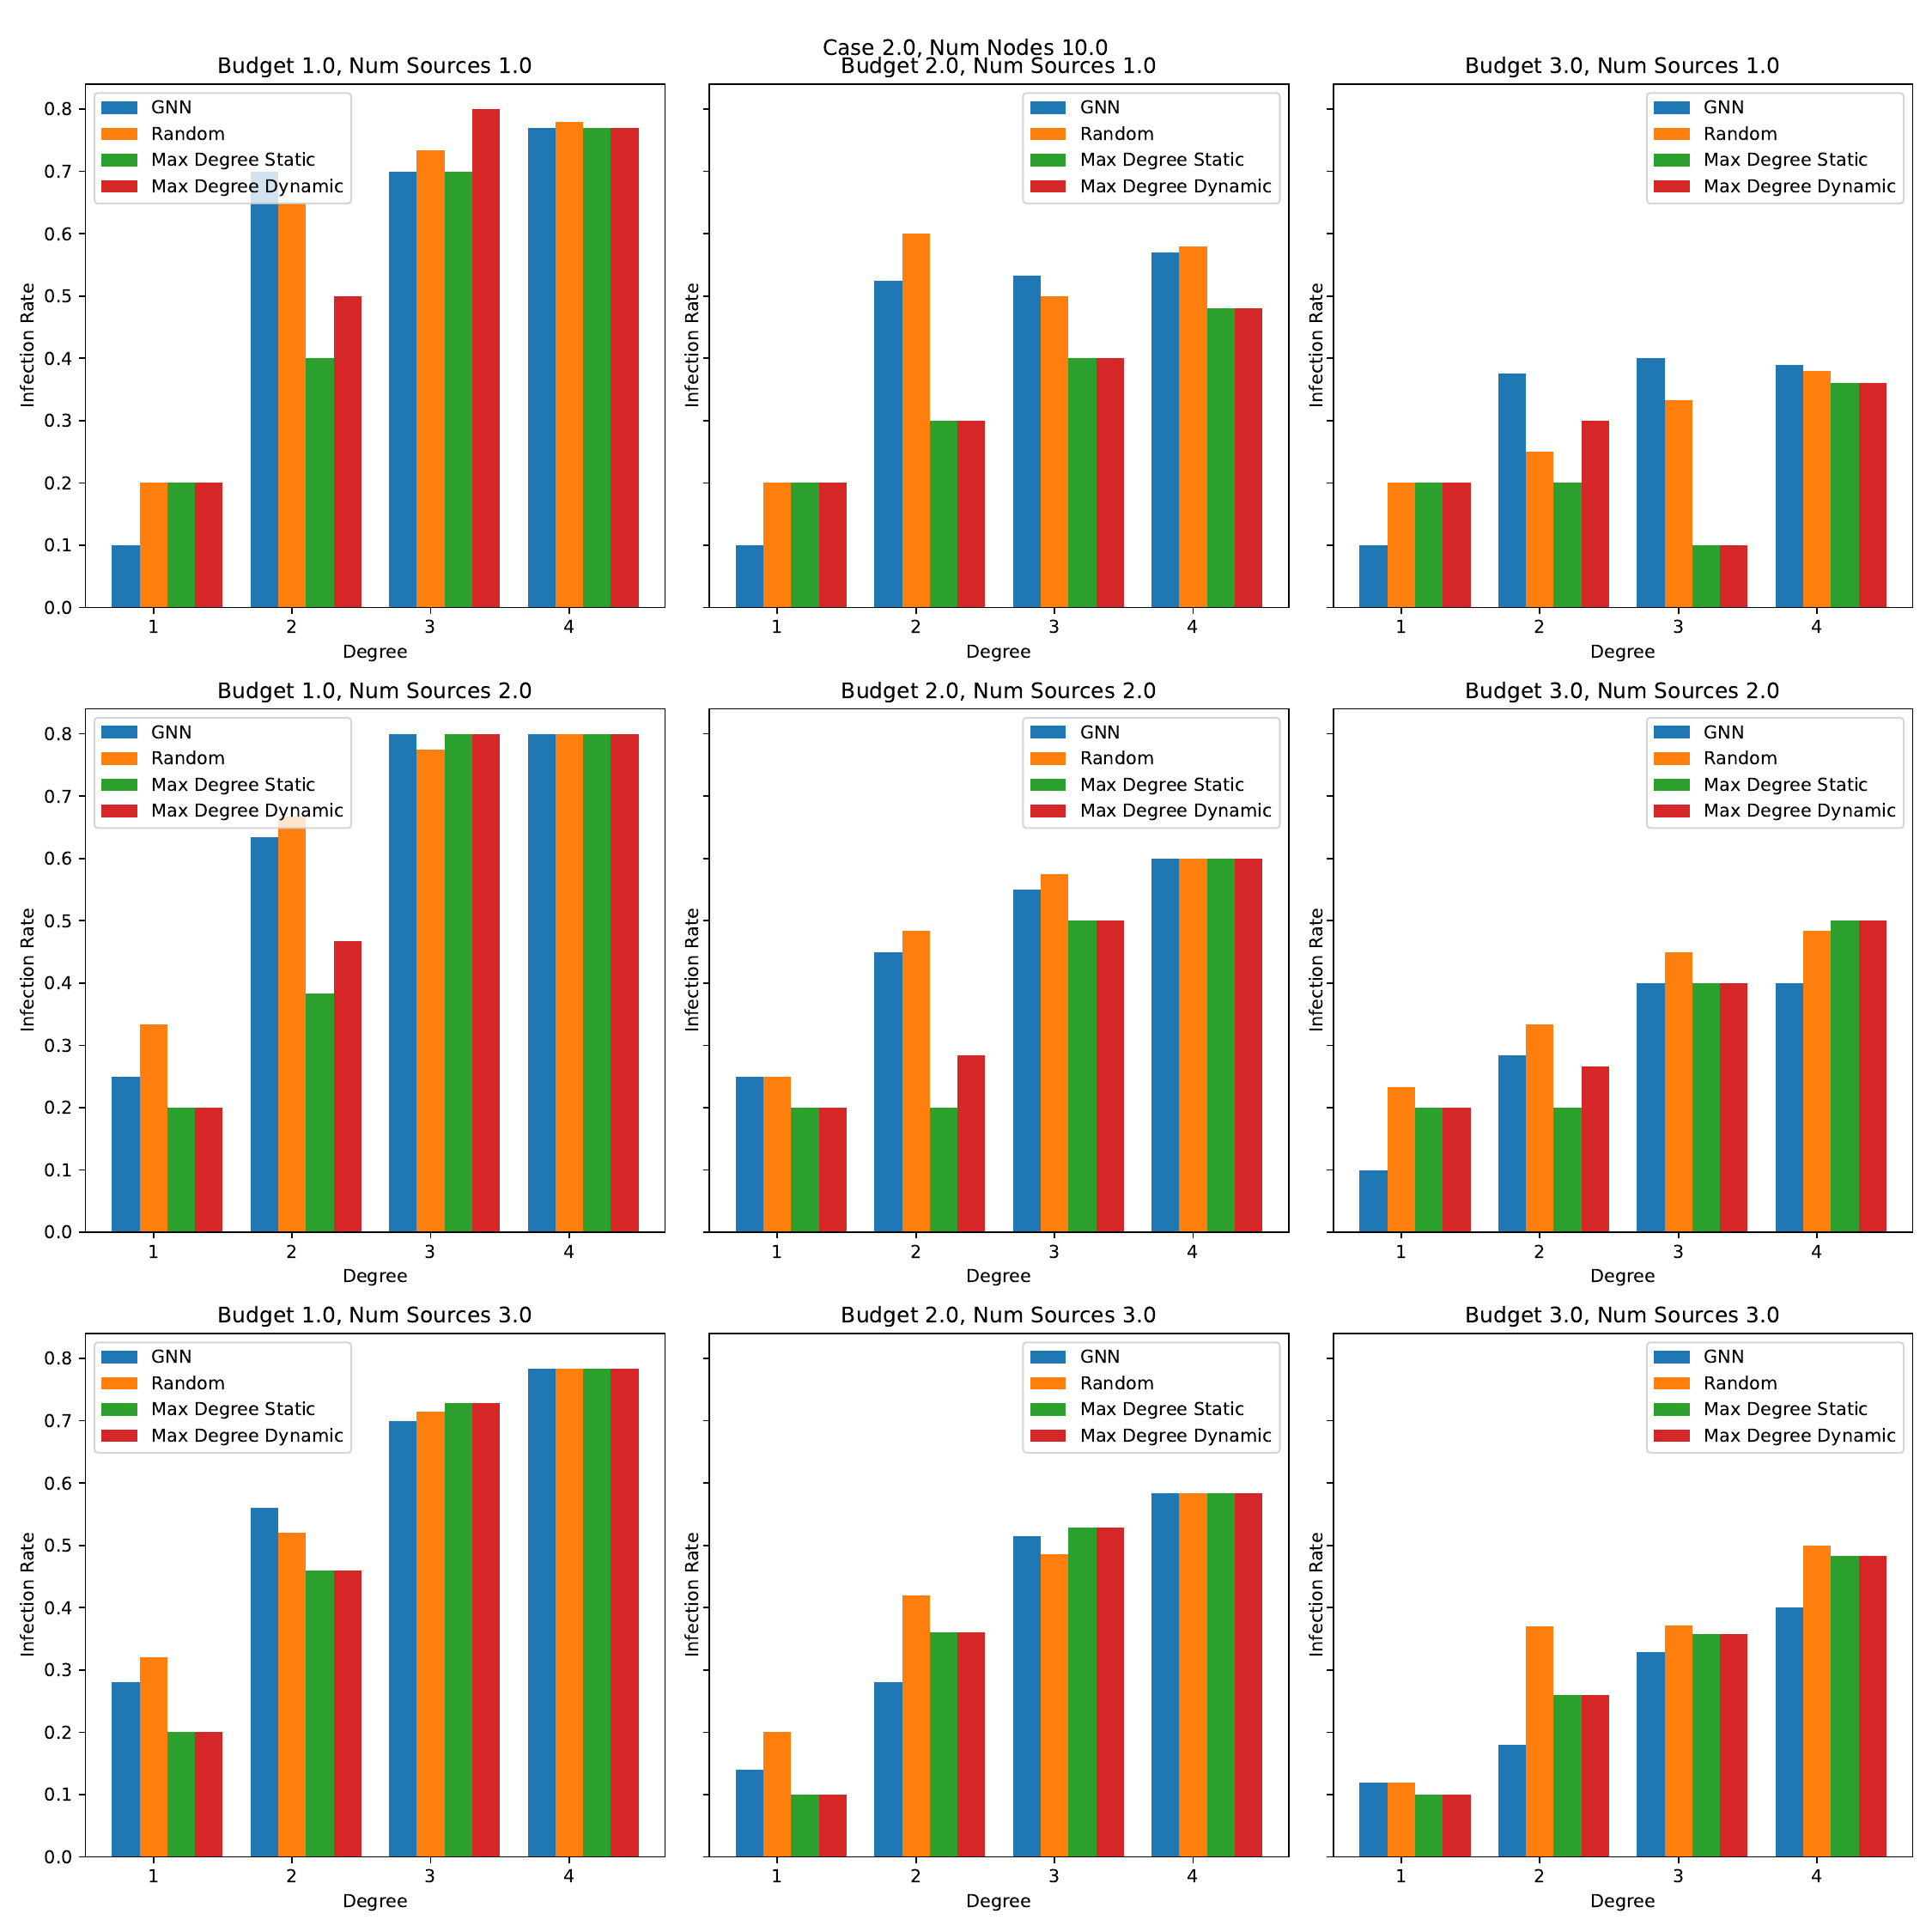}
    \caption{\footnotesize Dataset: Erdos-Renyi, Case-2 Node-10: Performance Evaluation of GCN-Based Supervised Learning Model: This series of bar plots presents a comparative analysis between our GCN-based SL model (blue), Randomized Policy model(yellow), Max Degree Policy model (Static) (green) and Max Degree Policy model (Dynamic) (red) on 10-node network environment. Progressing from left to right, the plots depict scenarios with increasing action budgets, ranging from 1 to 3 actions permitted. Vertically, the plots are ordered to show the effect of varying the initial count of infected nodes, starting with one and increasing to three. Each set of bars within the plots is categorized by the average connectivity (degree) of the infected nodes.}
    \label{fig:ERc2n10}
\end{figure}

\begin{figure}[!h]
    \centering
    \includegraphics[scale=0.3]{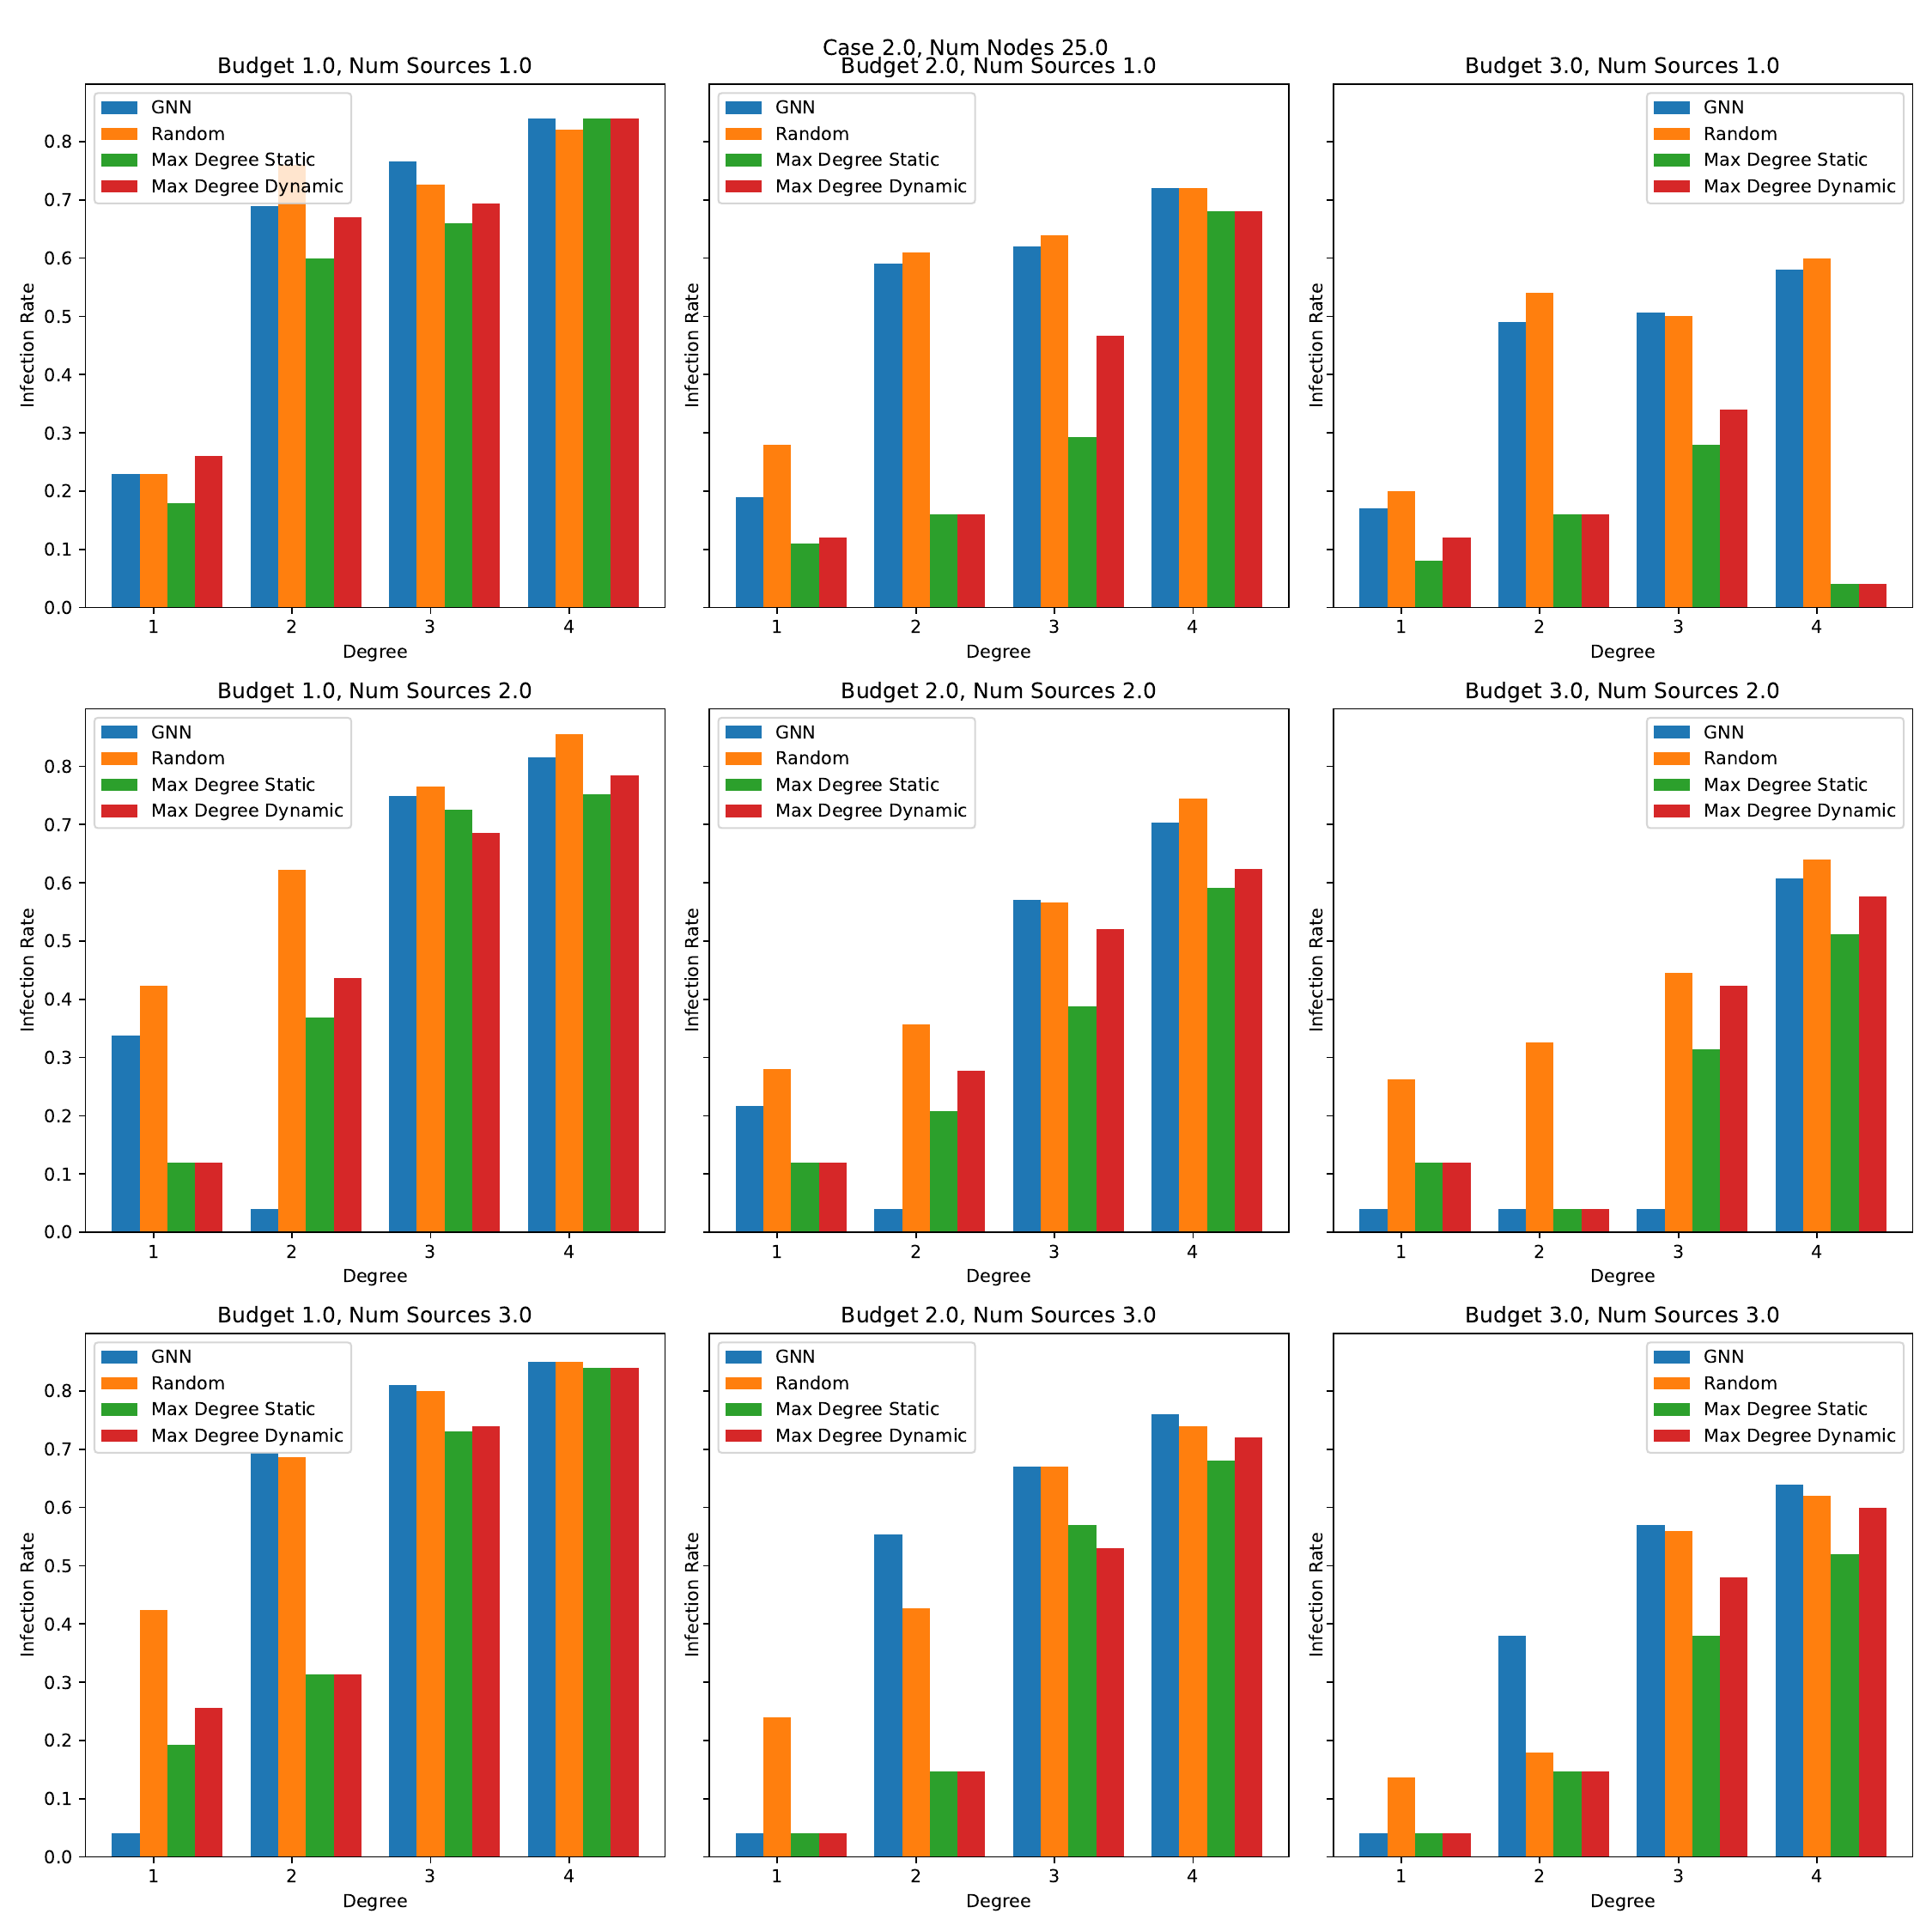}
    \caption{\footnotesize Dataset: Erdos-Renyi, Case-2 Node-25: Performance Evaluation of GCN-Based Supervised Learning Model: This series of bar plots presents a comparative analysis between our GCN-based SL model (blue), Randomized Policy model(yellow), Max Degree Policy model (Static) (green) and Max Degree Policy model (Dynamic) (red) on 10-node network environment. Progressing from left to right, the plots depict scenarios with increasing action budgets, ranging from 1 to 3 actions permitted. Vertically, the plots are ordered to show the effect of varying the initial count of infected nodes, starting with one and increasing to three. Each set of bars within the plots is categorized by the average connectivity (degree) of the infected nodes.}
    \label{fig:ERc2n25}
\end{figure}

\begin{figure}[!h]
    \centering
    \includegraphics[scale=0.3]{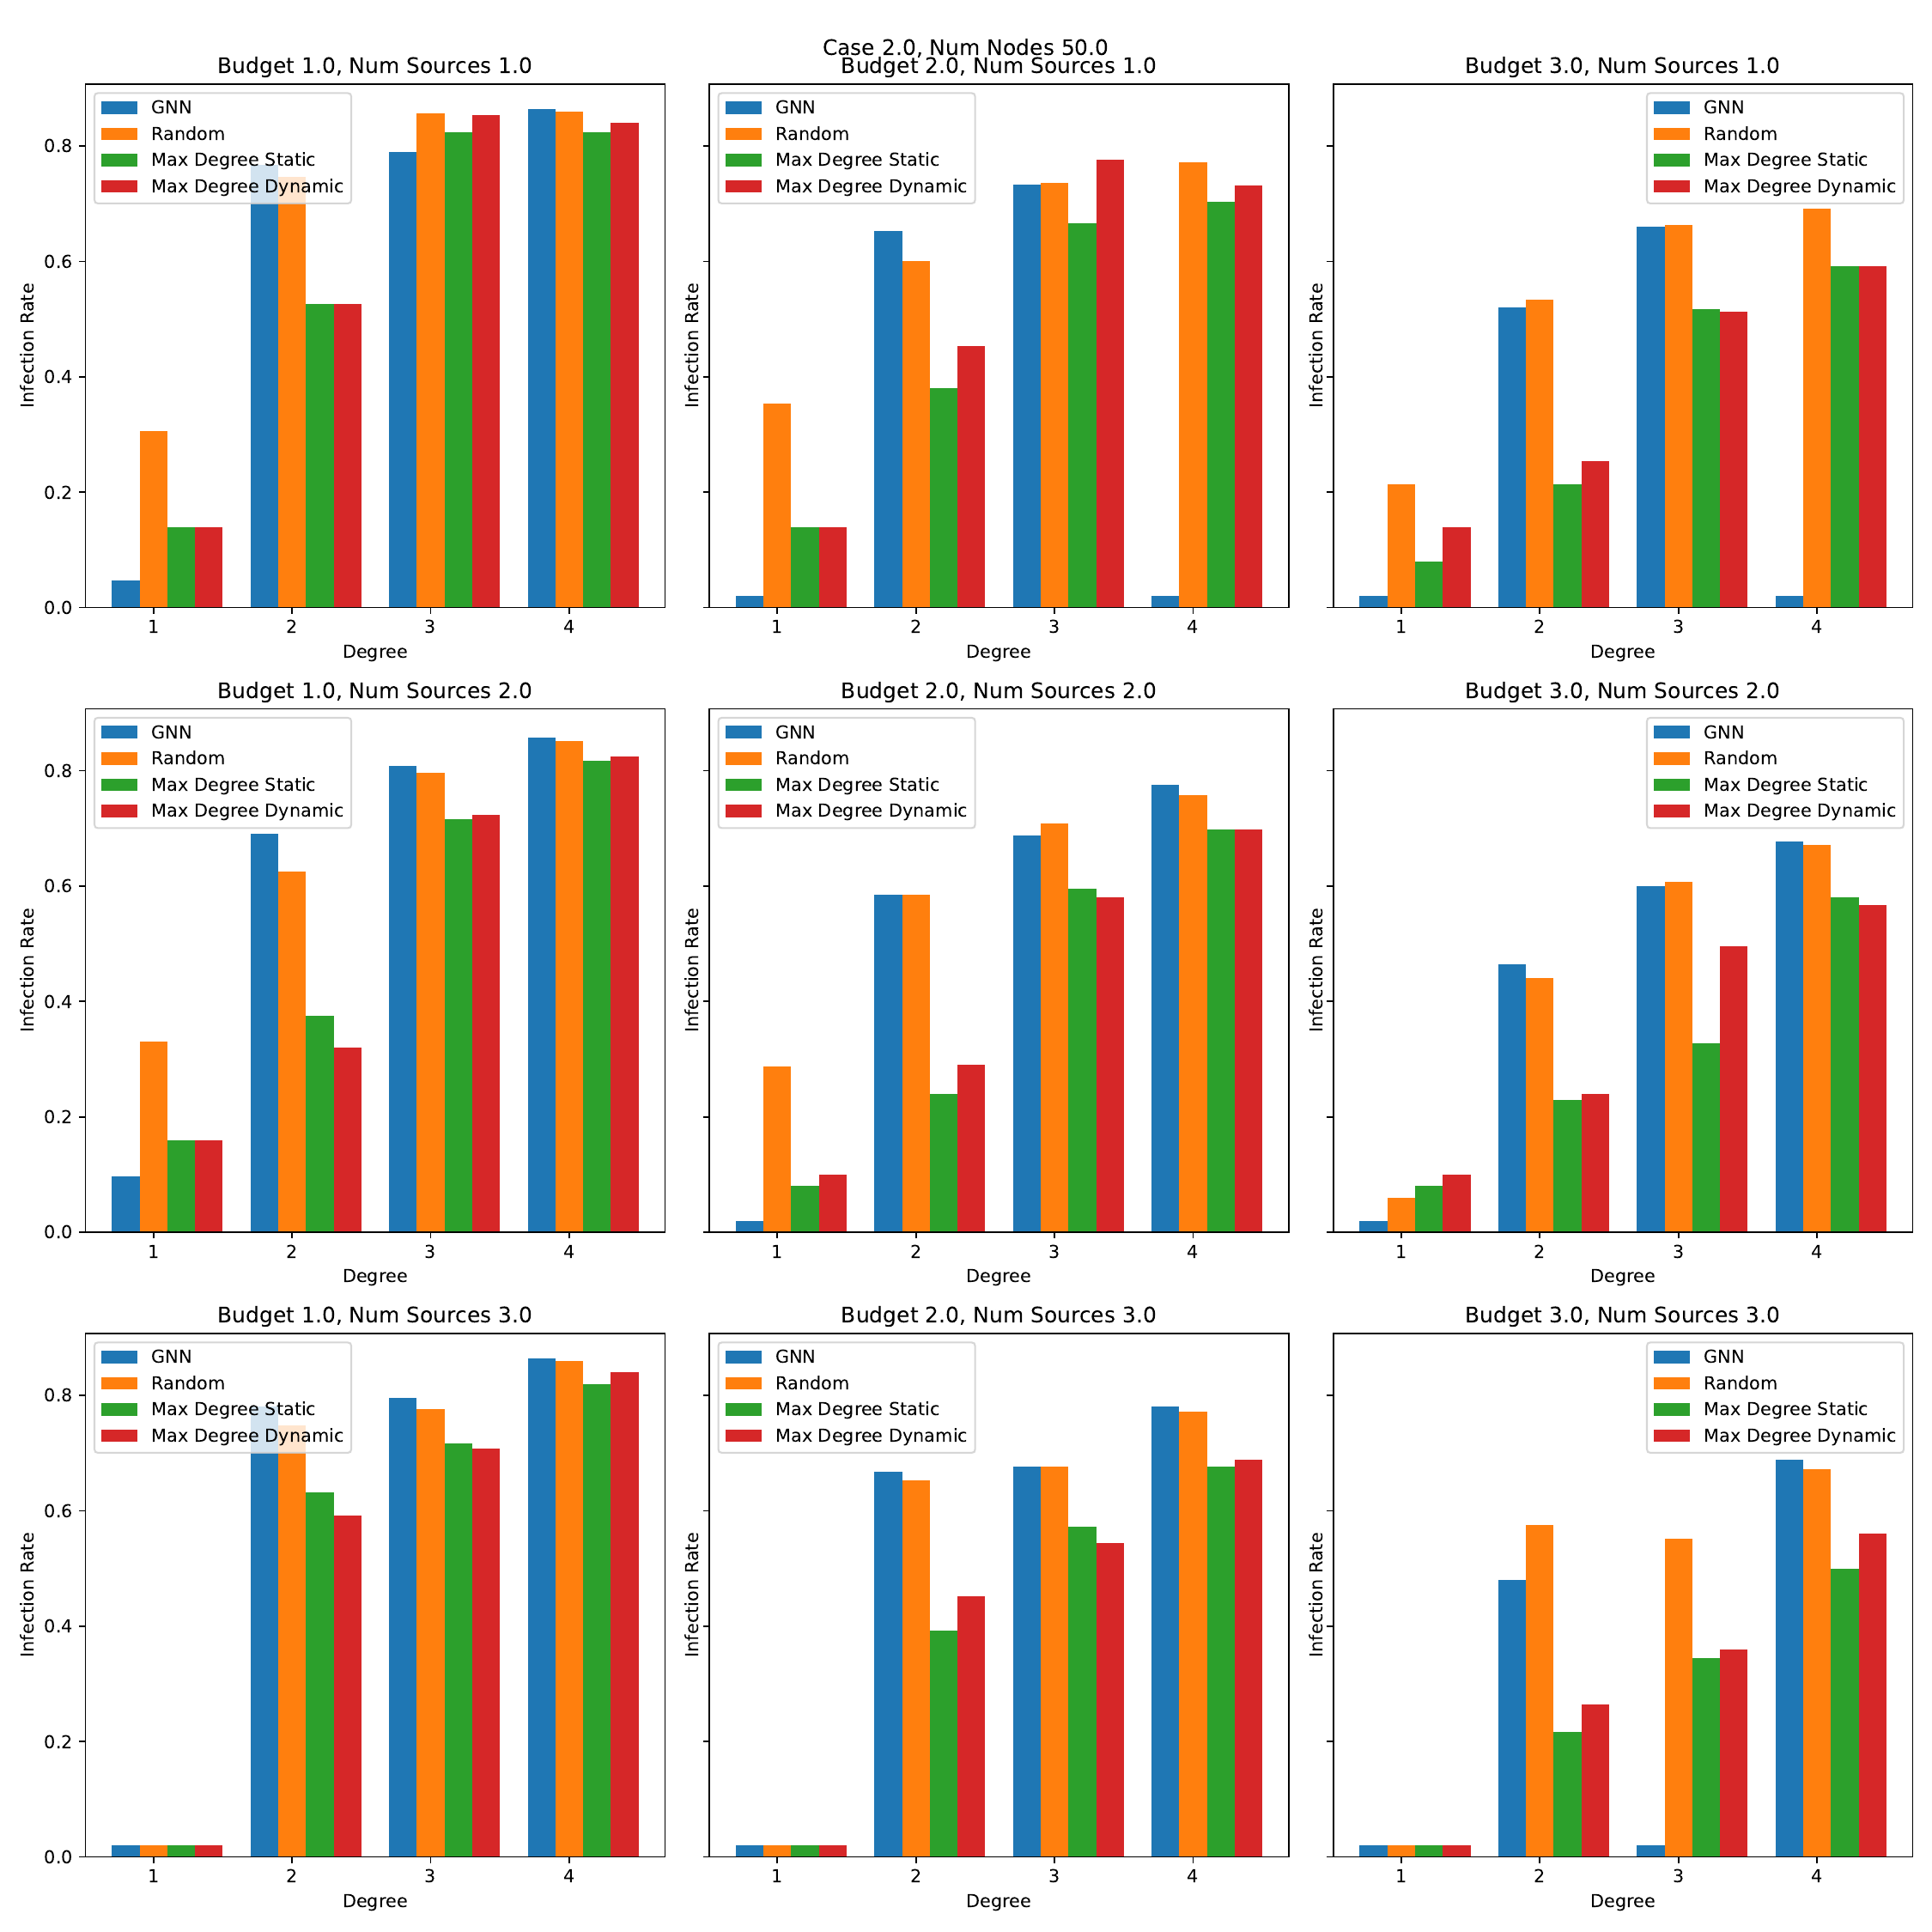}
    \caption{\footnotesize Dataset: Erdos-Renyi, Case-2 Node-50: Performance Evaluation of GCN-Based Supervised Learning Model: This series of bar plots presents a comparative analysis between our GCN-based SL model (blue), Randomized Policy model(yellow), Max Degree Policy model (Static) (green) and Max Degree Policy model (Dynamic) (red) on 10-node network environment. Progressing from left to right, the plots depict scenarios with increasing action budgets, ranging from 1 to 3 actions permitted. Vertically, the plots are ordered to show the effect of varying the initial count of infected nodes, starting with one and increasing to three. Each set of bars within the plots is categorized by the average connectivity (degree) of the infected nodes.}
    \label{fig:ERc2n50}
\end{figure}

% ######## Case 3 #########

\begin{figure}[!h]
    \centering
    \includegraphics[scale=0.3]{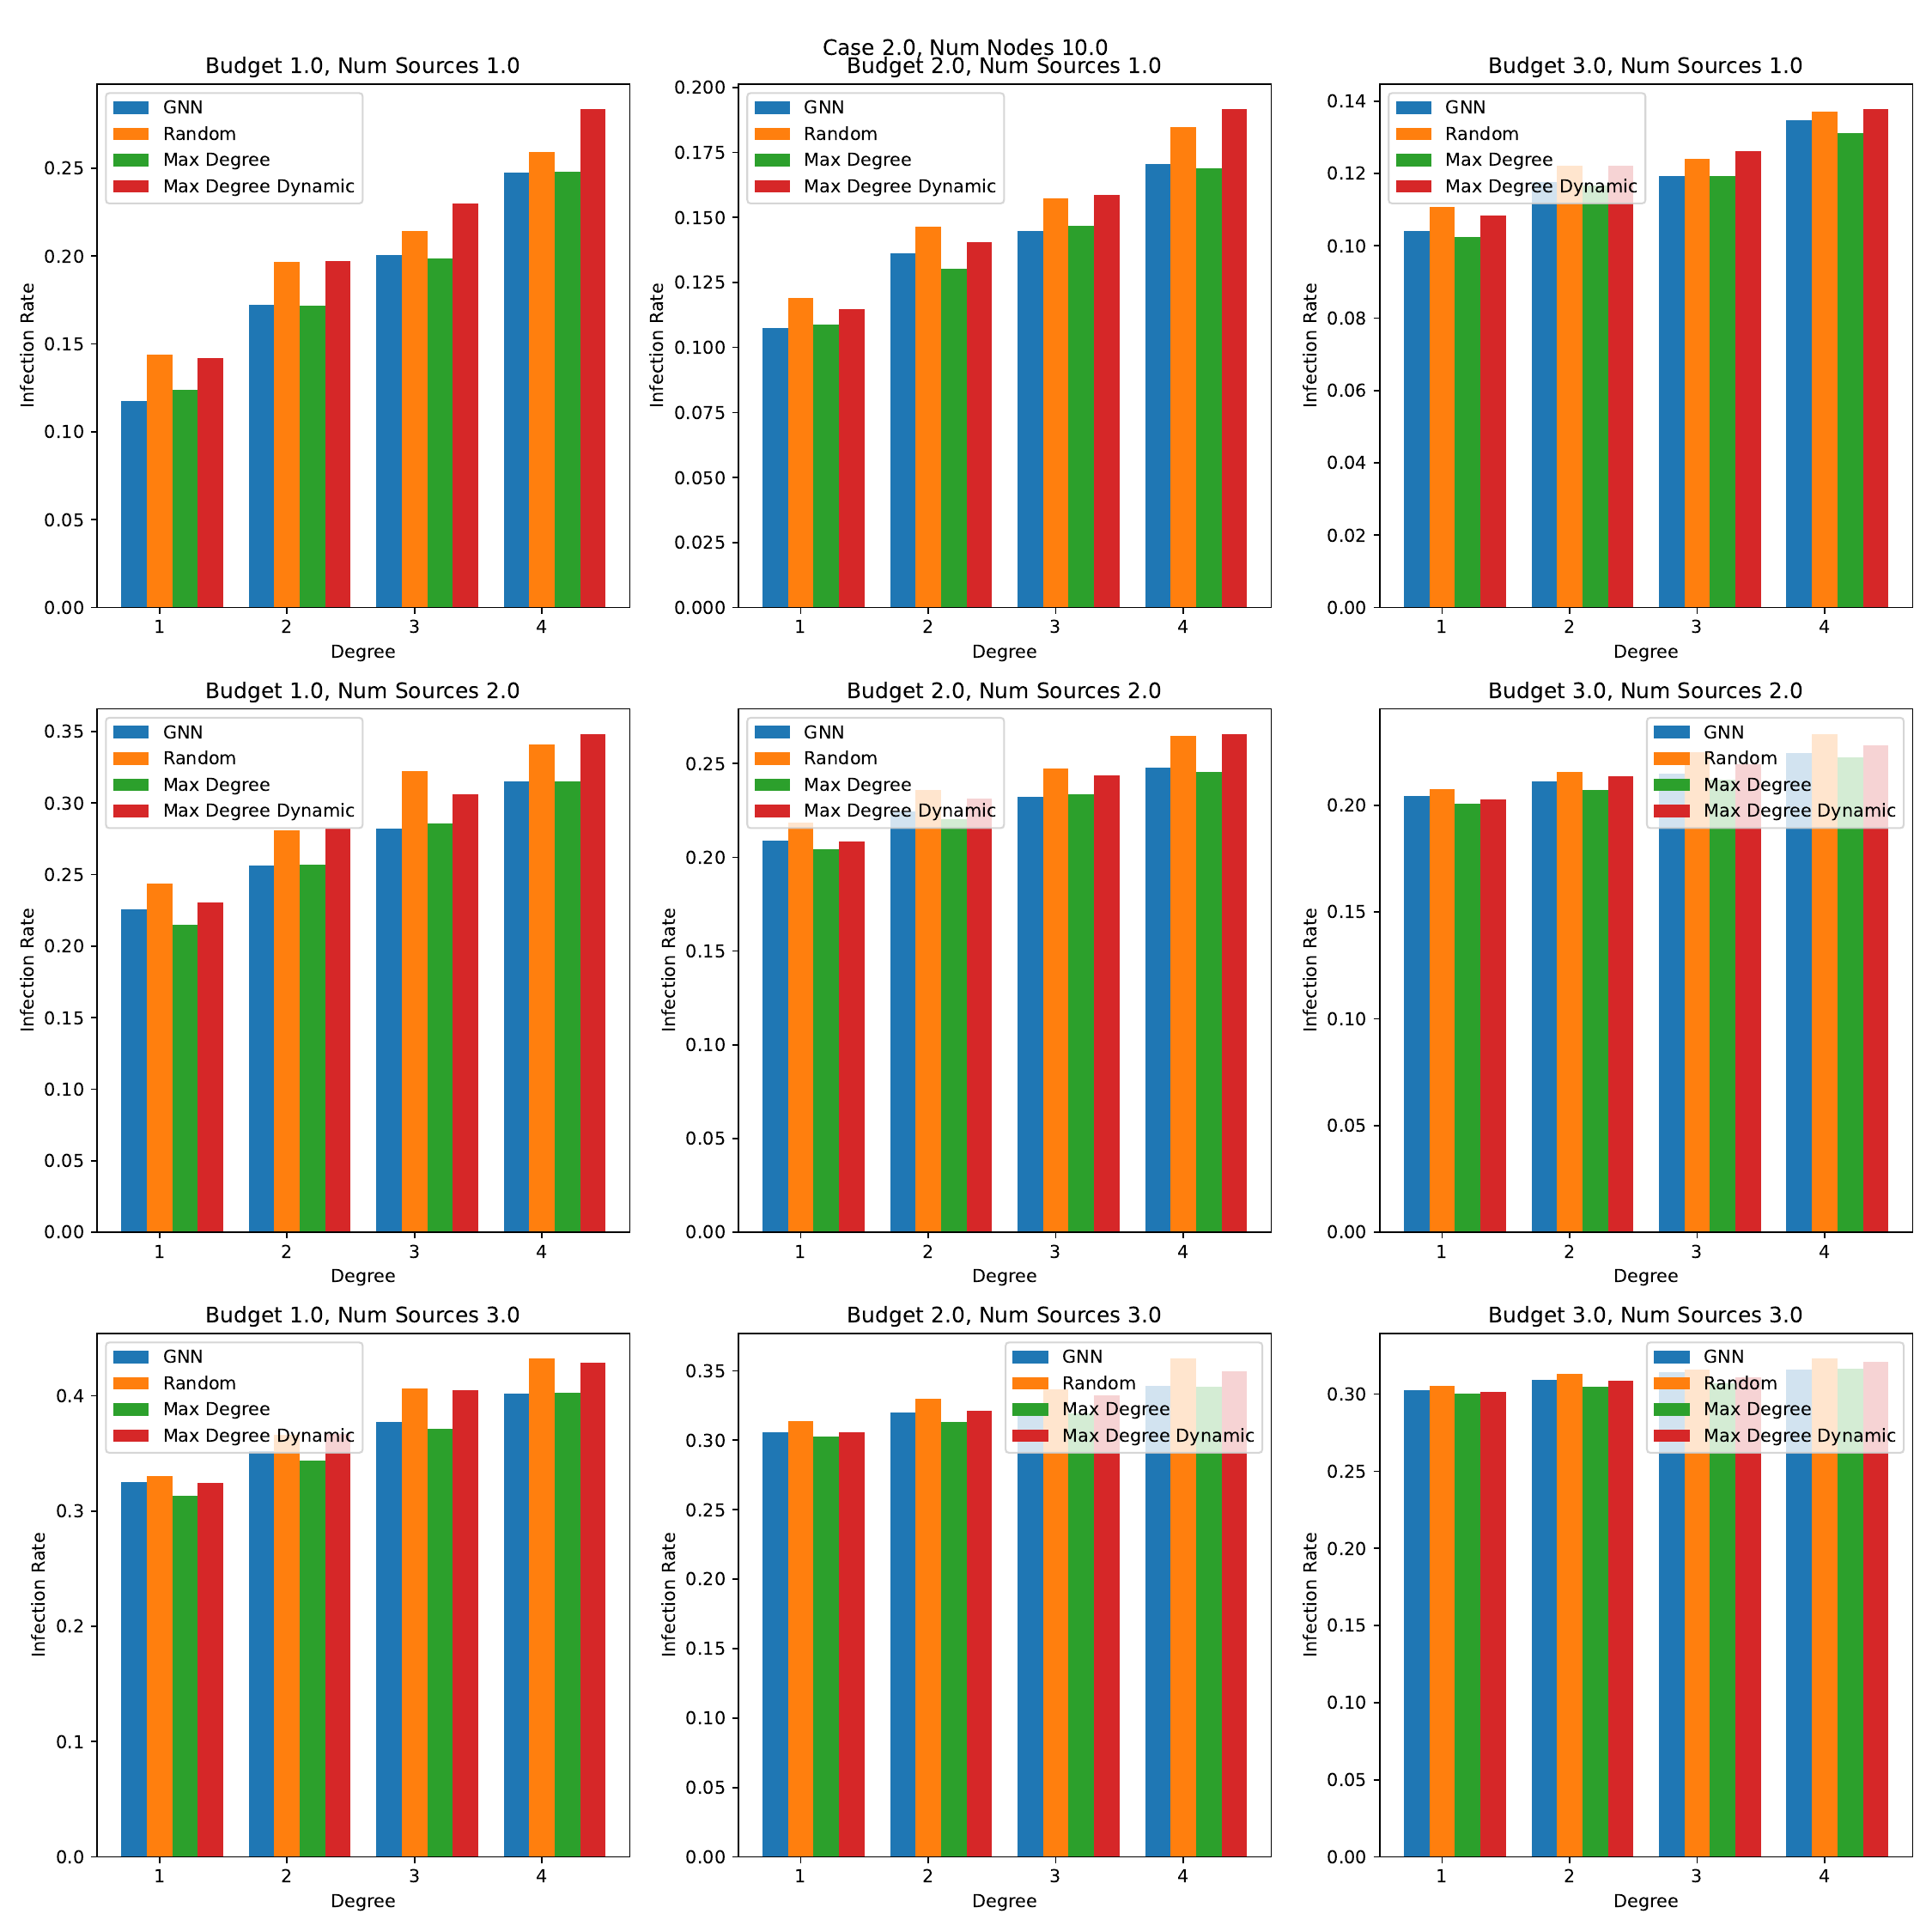}
    \caption{\footnotesize Dataset: Watts\_Strogatz, Case-3 Node-10: Performance Evaluation of GCN-Based Supervised Learning Model: This series of bar plots presents a comparative analysis between our GCN-based SL model (blue), Randomized Policy model(yellow), Max Degree Policy model (Static) (green) and Max Degree Policy model (Dynamic) (red) on 10-node network environment. Progressing from left to right, the plots depict scenarios with increasing action budgets, ranging from 1 to 3 actions permitted. Vertically, the plots are ordered to show the effect of varying the initial count of infected nodes, starting with one and increasing to three. Each set of bars within the plots is categorized by the average connectivity (degree) of the infected nodes.}
    \label{fig:c3n10}
\end{figure}

\begin{figure}[!h]
    \centering
    \includegraphics[scale=0.3]{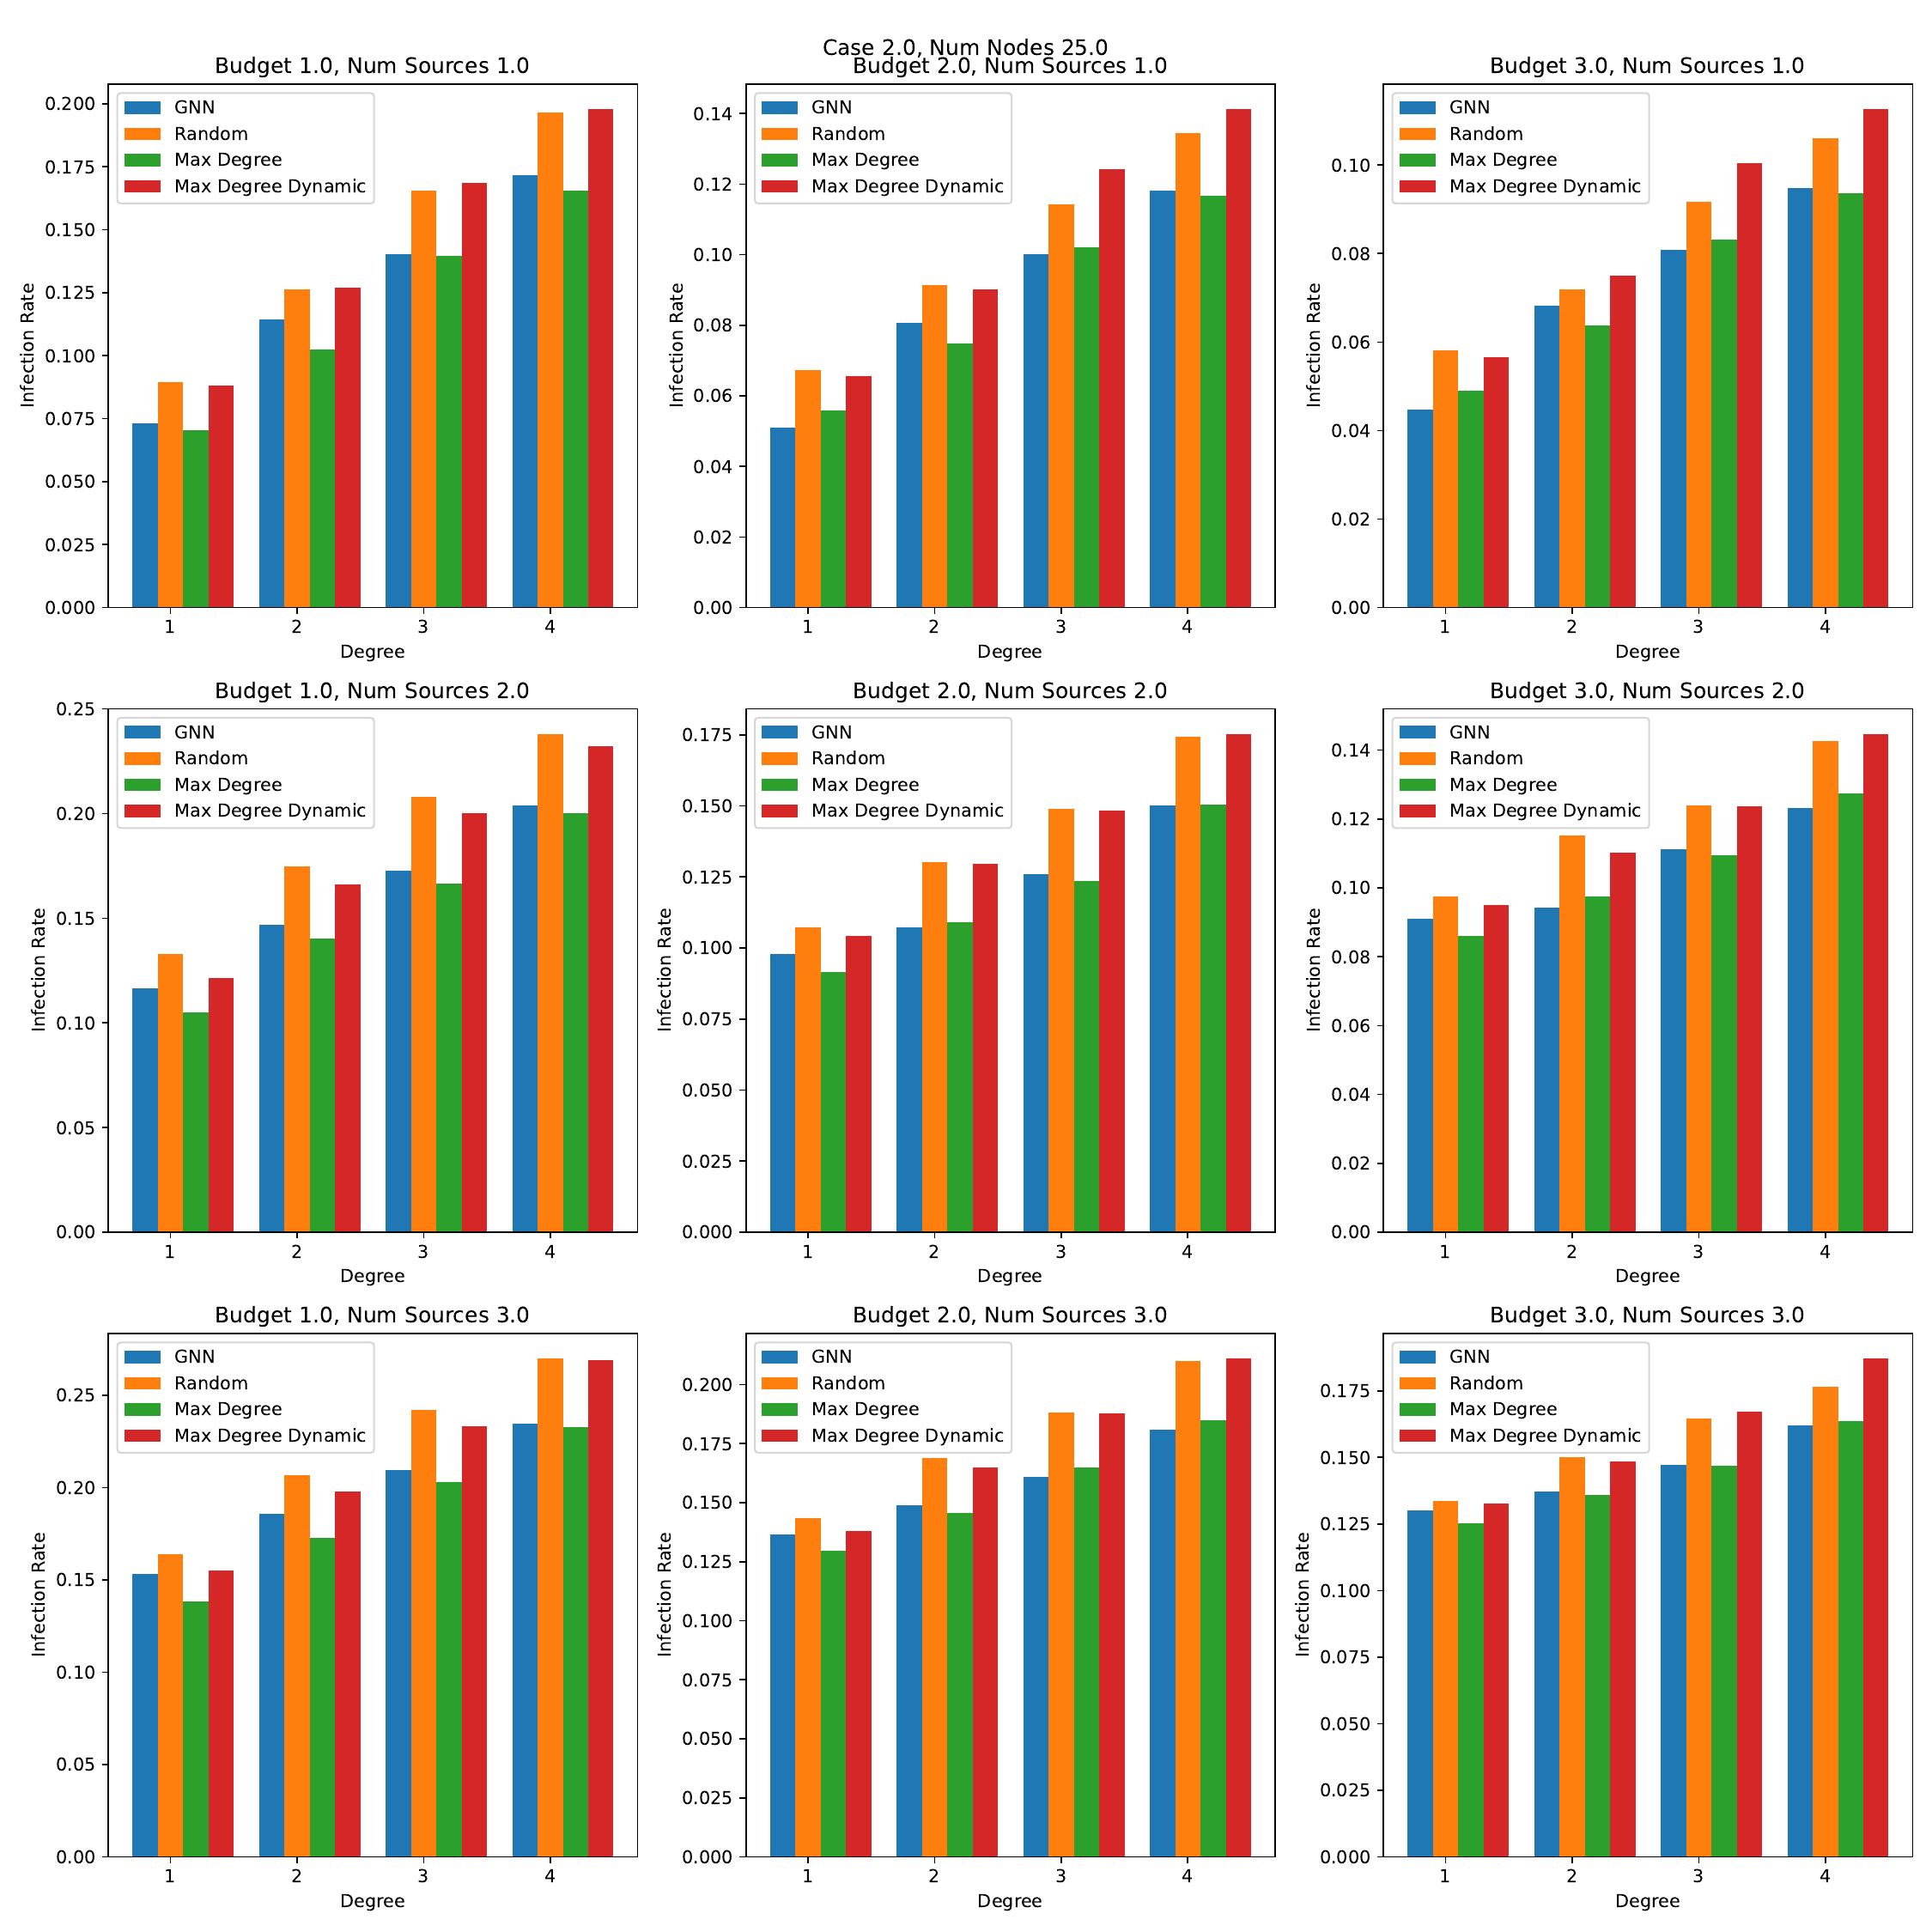}
    \caption{\footnotesize Dataset: Watts\_Strogatz, Case-3 Node-25: Performance Evaluation of GCN-Based Supervised Learning Model: This series of bar plots presents a comparative analysis between our GCN-based SL model (blue), Randomized Policy model(yellow), Max Degree Policy model (Static) (green) and Max Degree Policy model (Dynamic) (red) on 25-node network environment. Progressing from left to right, the plots depict scenarios with increasing action budgets, ranging from 1 to 3 actions permitted. Vertically, the plots are ordered to show the effect of varying the initial count of infected nodes, starting with one and increasing to three. Each set of bars within the plots is categorized by the average connectivity (degree) of the infected nodes.}
    \label{fig:c3n25}
\end{figure}

\begin{figure}[!h]
    \centering
    \includegraphics[scale=0.3]{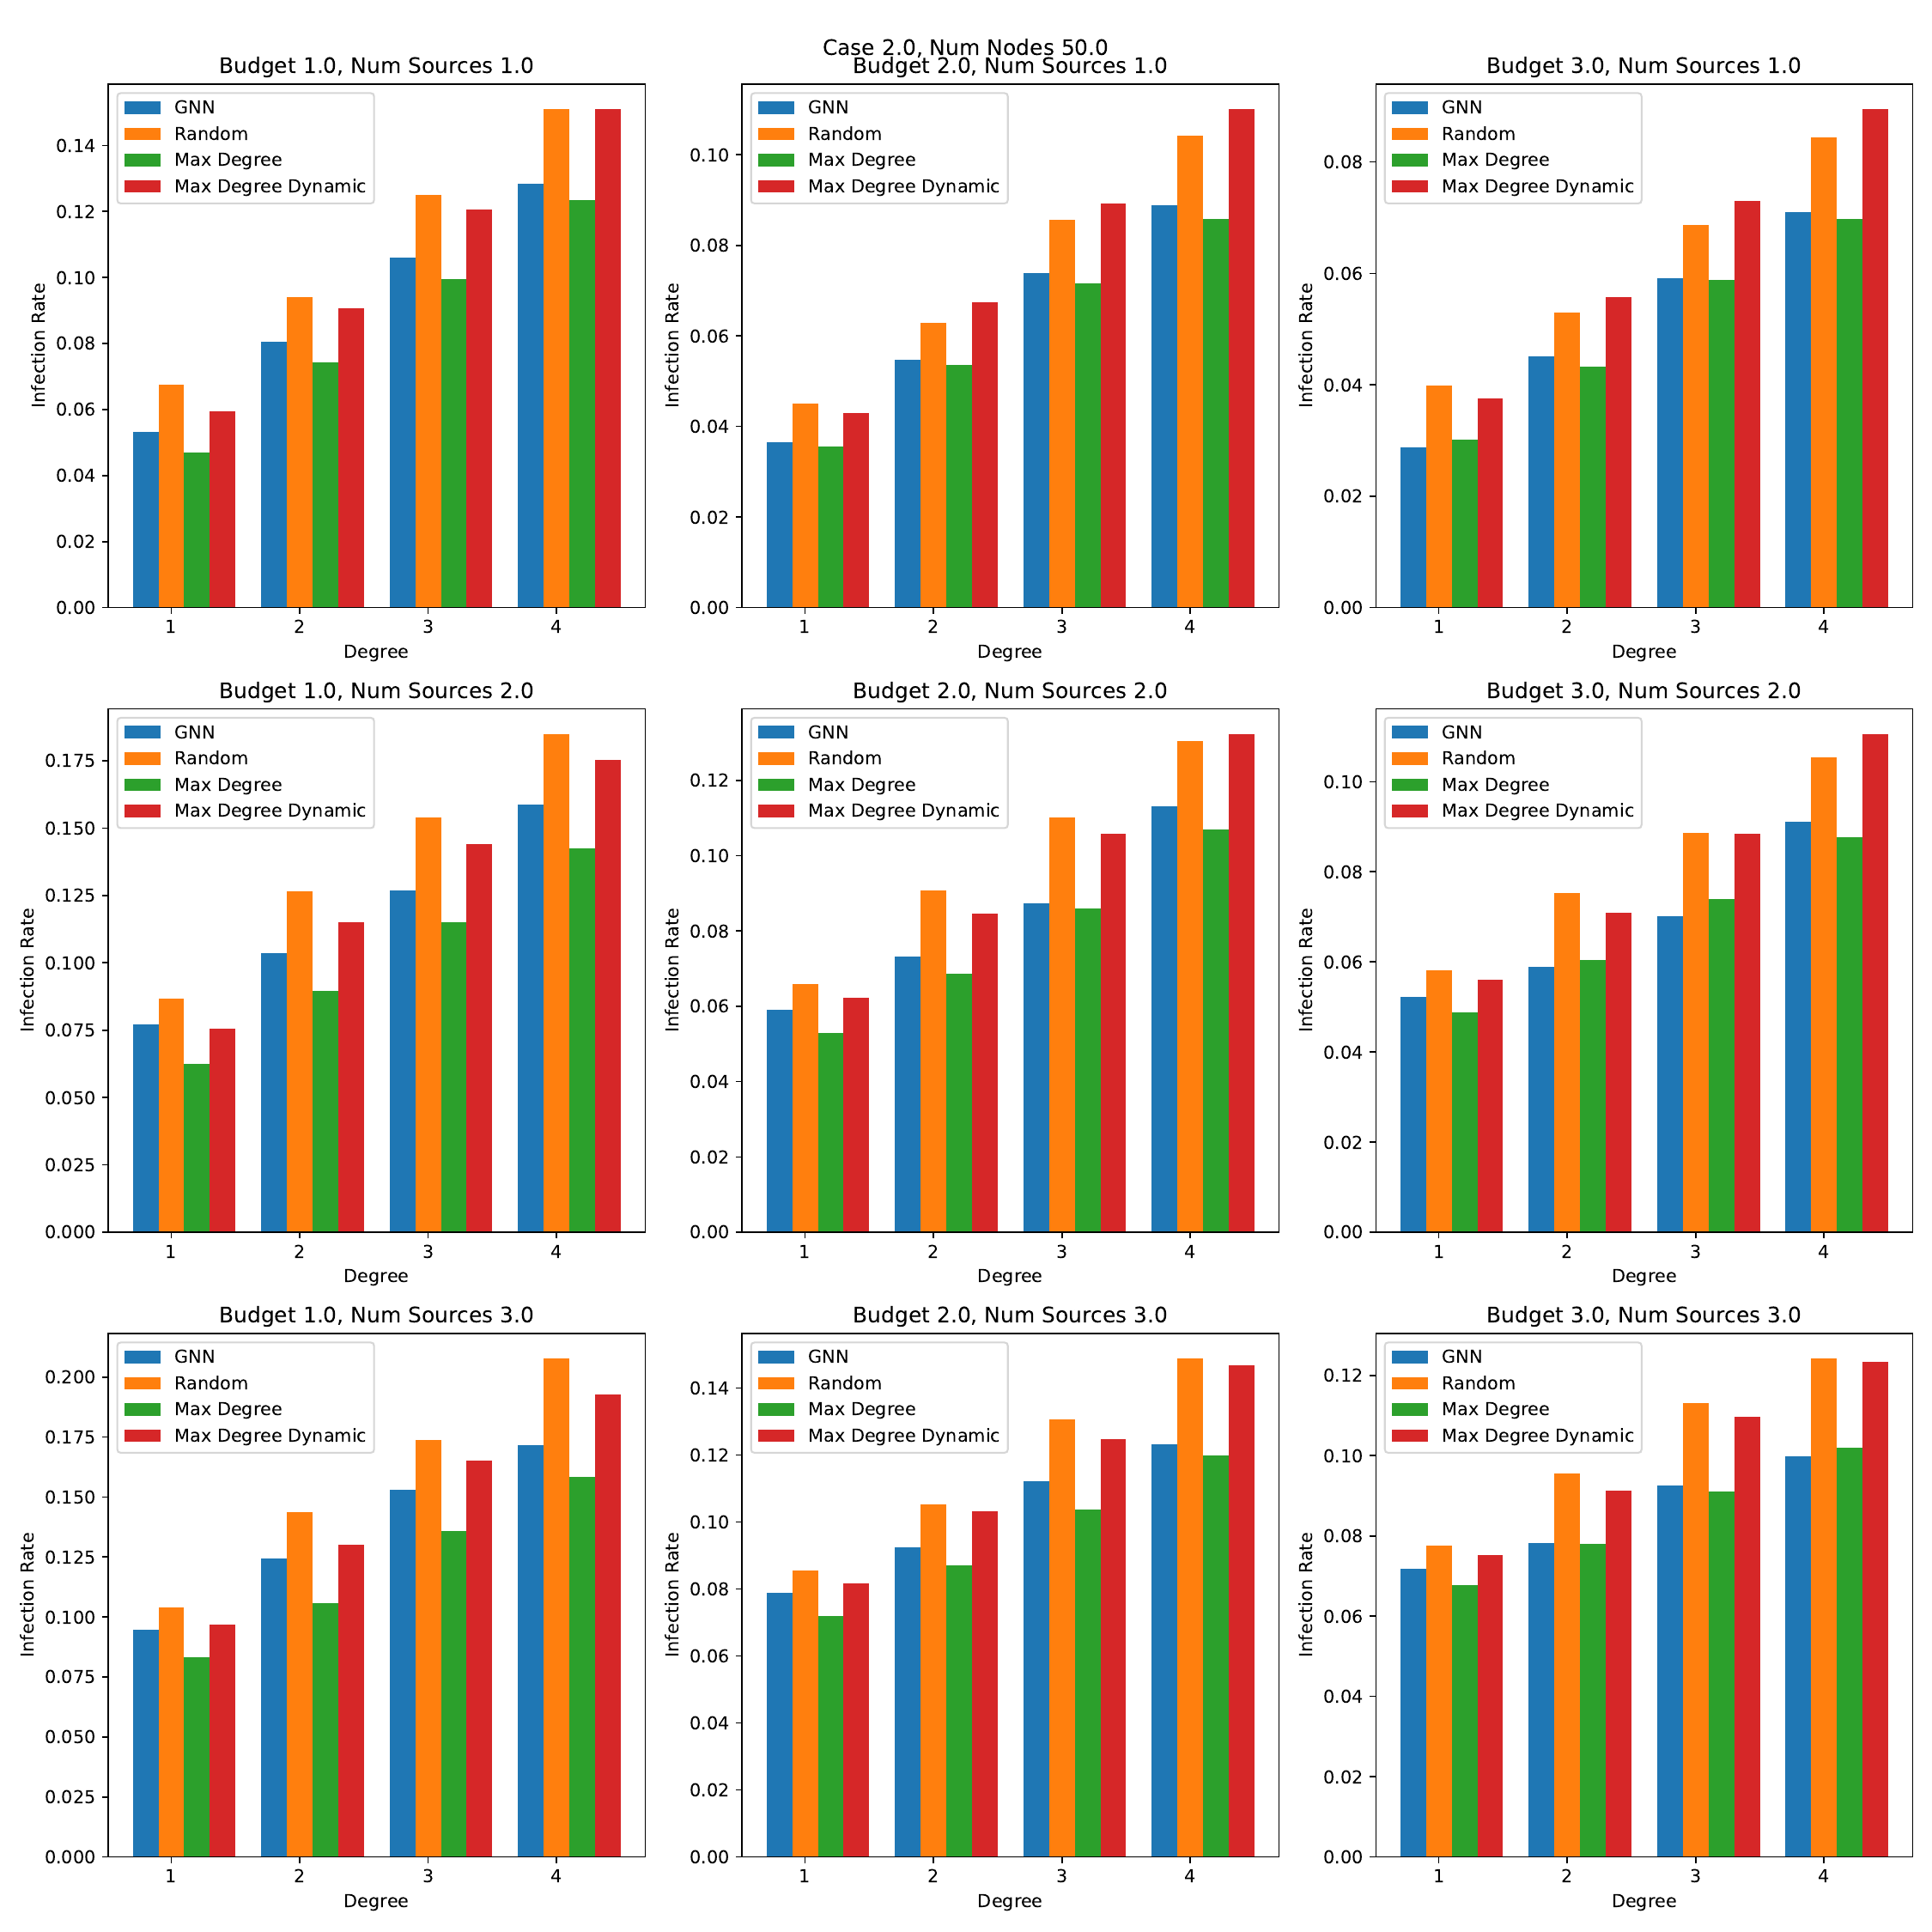}
    \caption{\footnotesize Dataset: Watts\_Strogatz, Case-3 Node-50: Performance Evaluation of GCN-Based Supervised Learning Model: This series of bar plots presents a comparative analysis between our GCN-based SL model (blue), Randomized Policy model(yellow), Max Degree Policy model (Static) (green) and Max Degree Policy model (Dynamic) (red) on 25-node network environment. Progressing from left to right, the plots depict scenarios with increasing action budgets, ranging from 1 to 3 actions permitted. Vertically, the plots are ordered to show the effect of varying the initial count of infected nodes, starting with one and increasing to three. Each set of bars within the plots is categorized by the average connectivity (degree) of the infected nodes.}
    \label{fig:c3n50}
\end{figure}

\begin{figure}[!h]
    \centering
    \includegraphics[scale=0.3]{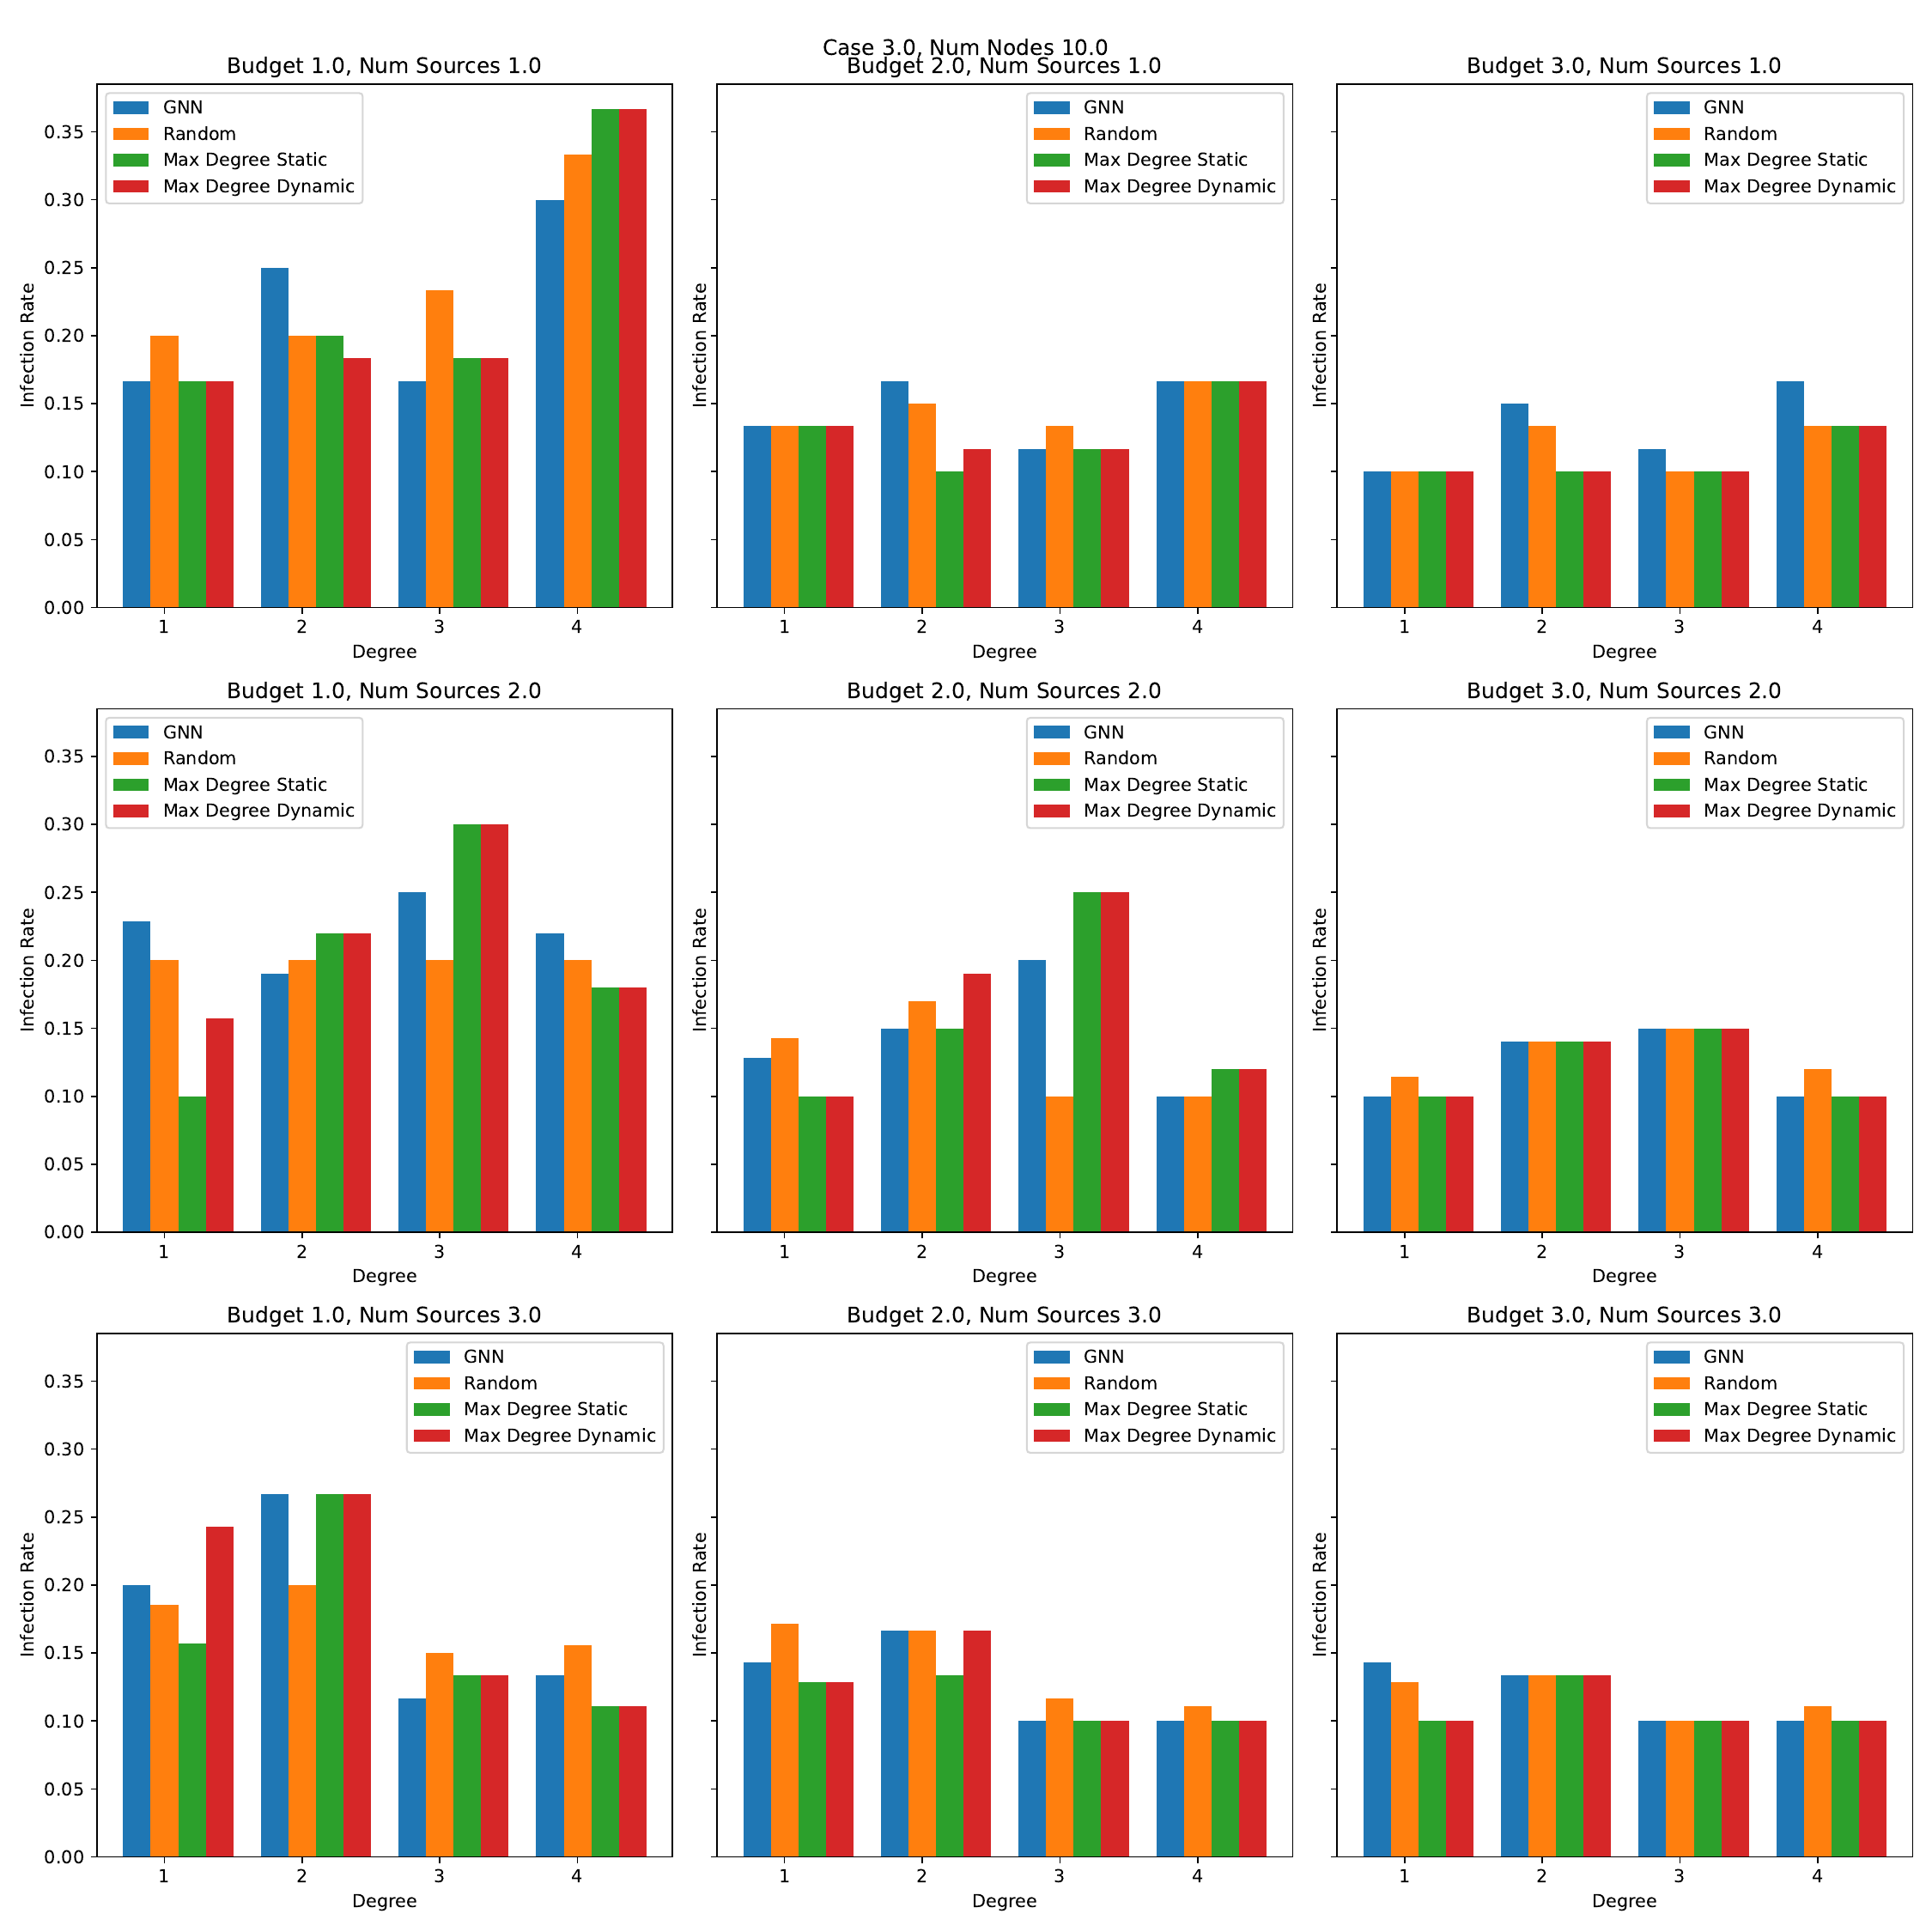}
    \caption{\footnotesize Dataset: Tree, Case-3 Node-10: Performance Evaluation of GCN-Based Supervised Learning Model: This series of bar plots presents a comparative analysis between our GCN-based SL model (blue), Randomized Policy model(yellow), Max Degree Policy model (Static) (green) and Max Degree Policy model (Dynamic) (red) on 10-node network environment. Progressing from left to right, the plots depict scenarios with increasing action budgets, ranging from 1 to 3 actions permitted. Vertically, the plots are ordered to show the effect of varying the initial count of infected nodes, starting with one and increasing to three. Each set of bars within the plots is categorized by the average connectivity (degree) of the infected nodes.}
    \label{fig:Treec3n10}
\end{figure}

\begin{figure}[!h]
    \centering
    \includegraphics[scale=0.3]{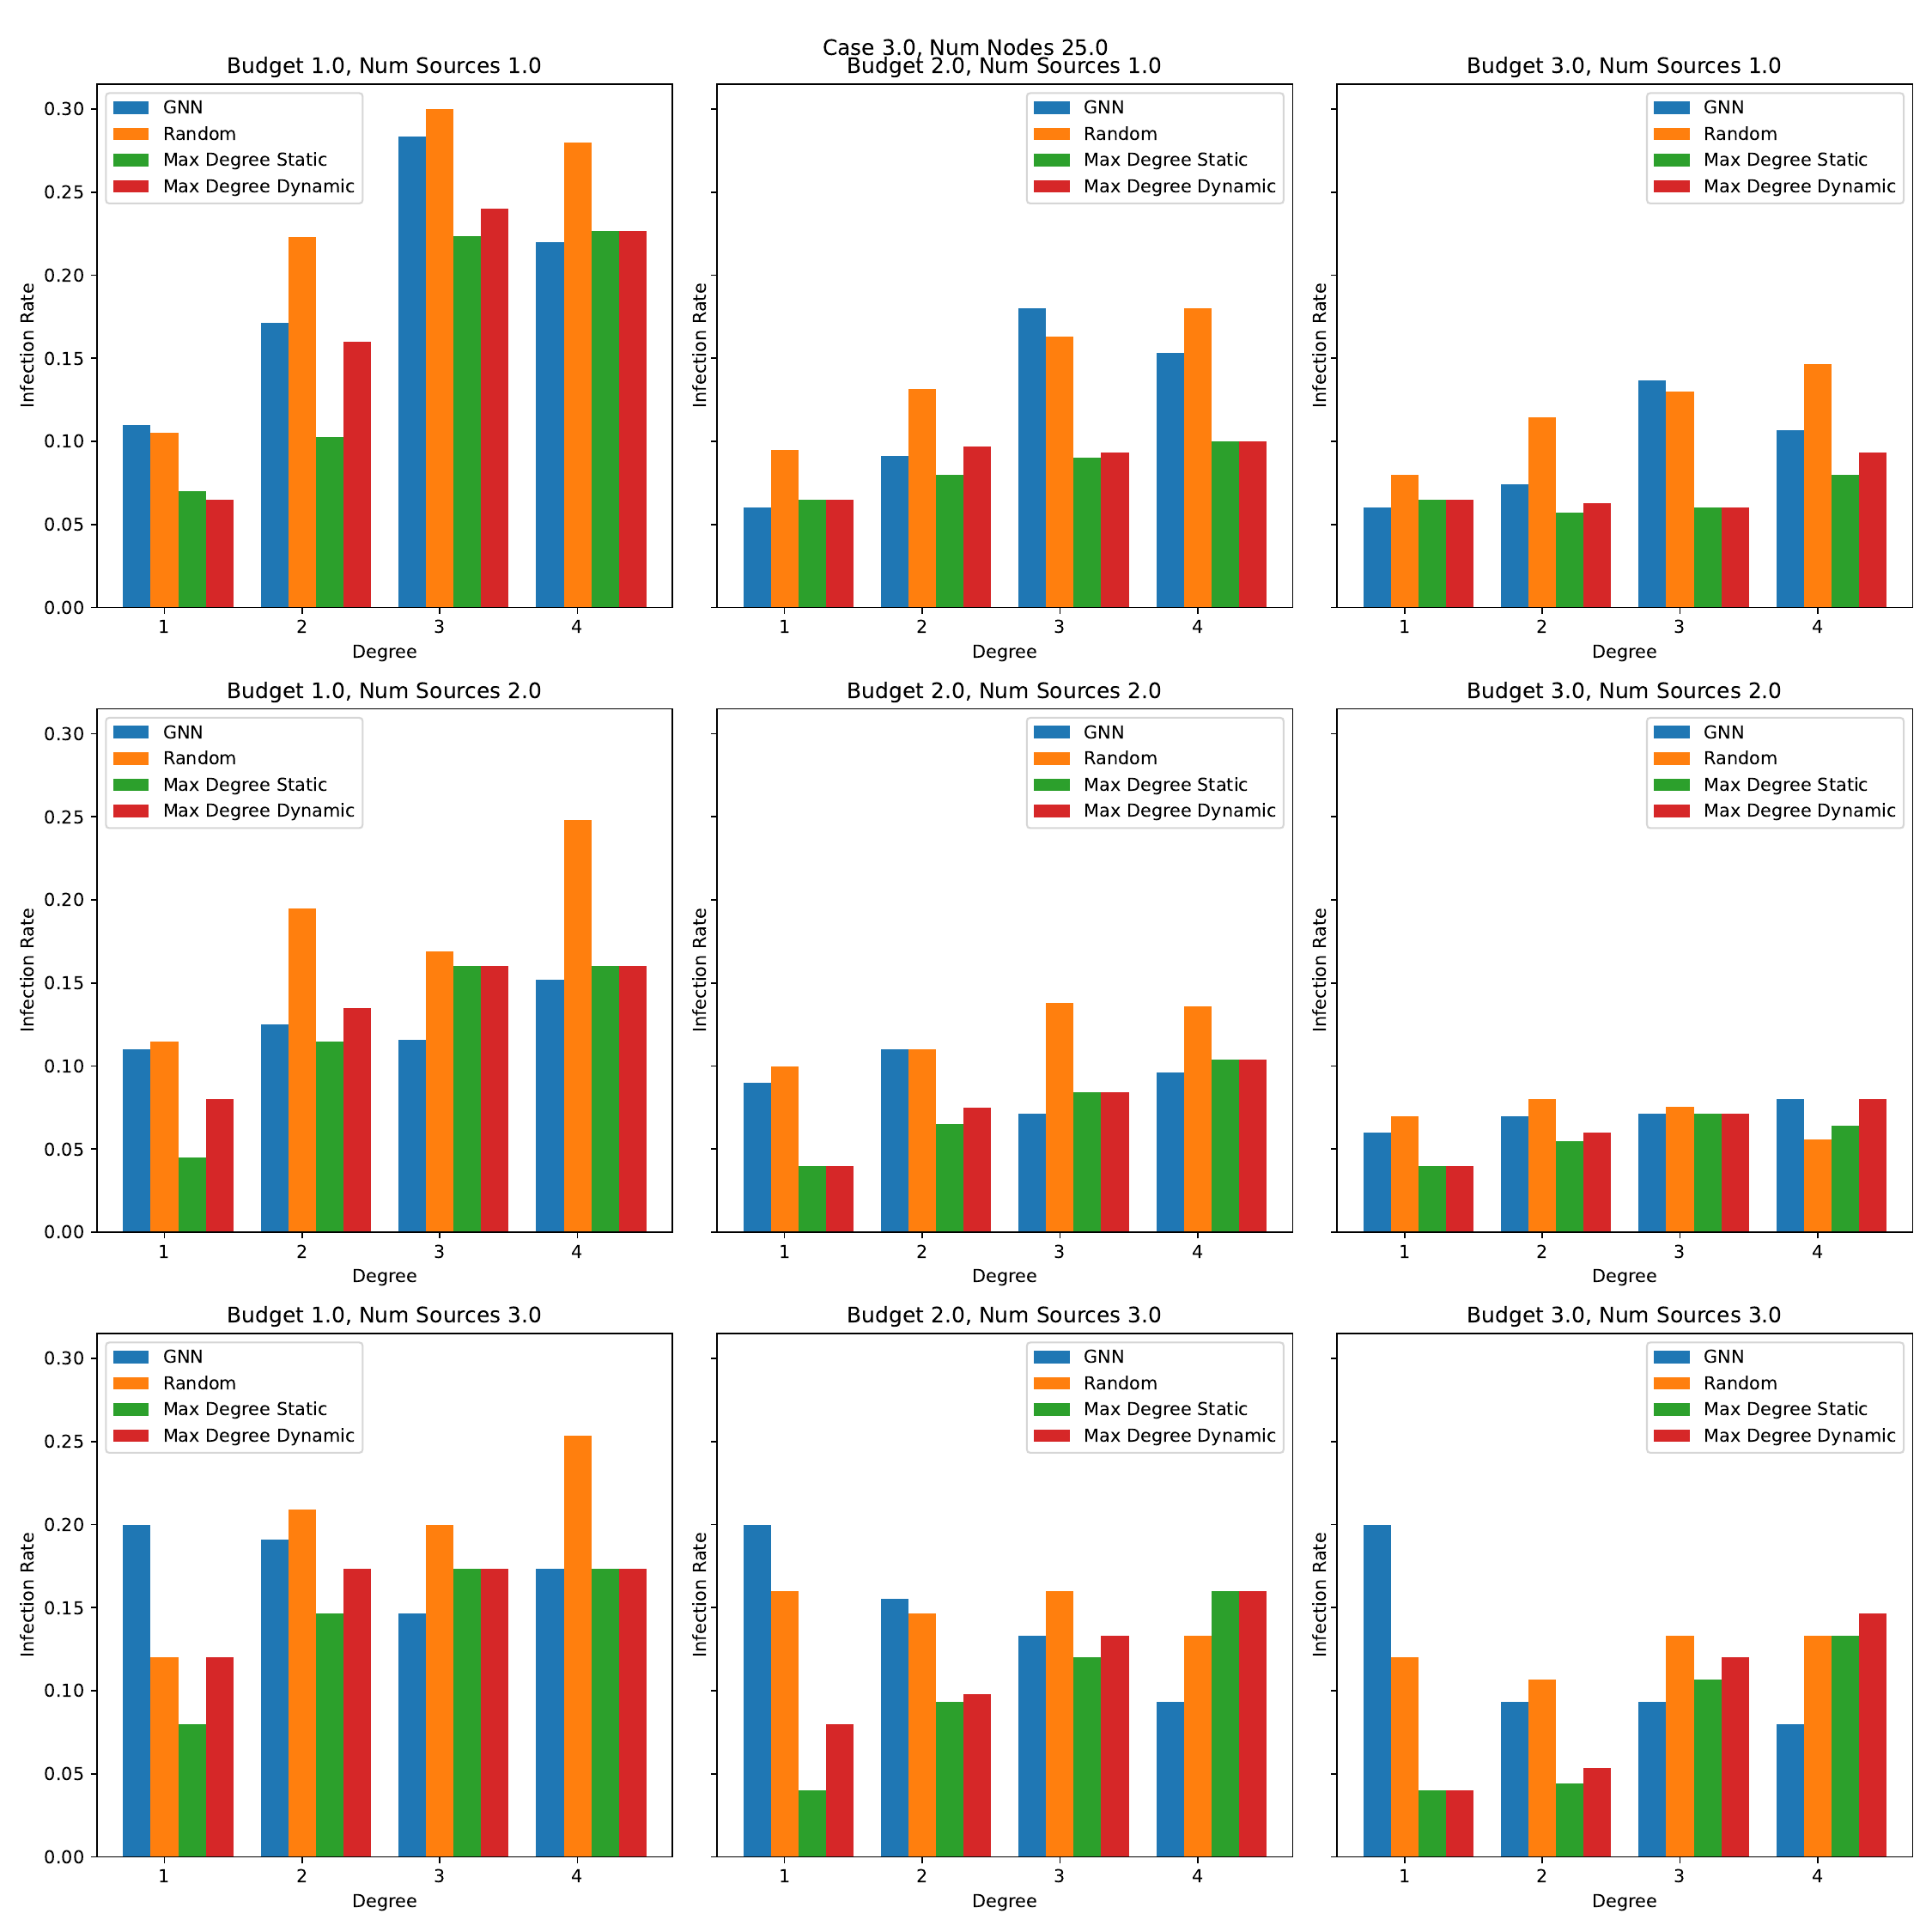}
    \caption{\footnotesize Dataset: Tree, Case-3 Node-25: Performance Evaluation of GCN-Based Supervised Learning Model: This series of bar plots presents a comparative analysis between our GCN-based SL model (blue), Randomized Policy model(yellow), Max Degree Policy model (Static) (green) and Max Degree Policy model (Dynamic) (red) on 25-node network environment. Progressing from left to right, the plots depict scenarios with increasing action budgets, ranging from 1 to 3 actions permitted. Vertically, the plots are ordered to show the effect of varying the initial count of infected nodes, starting with one and increasing to three. Each set of bars within the plots is categorized by the average connectivity (degree) of the infected nodes.}
    \label{fig:Treec3n25}
\end{figure}

\begin{figure}[!h]
    \centering
    \includegraphics[scale=0.3]{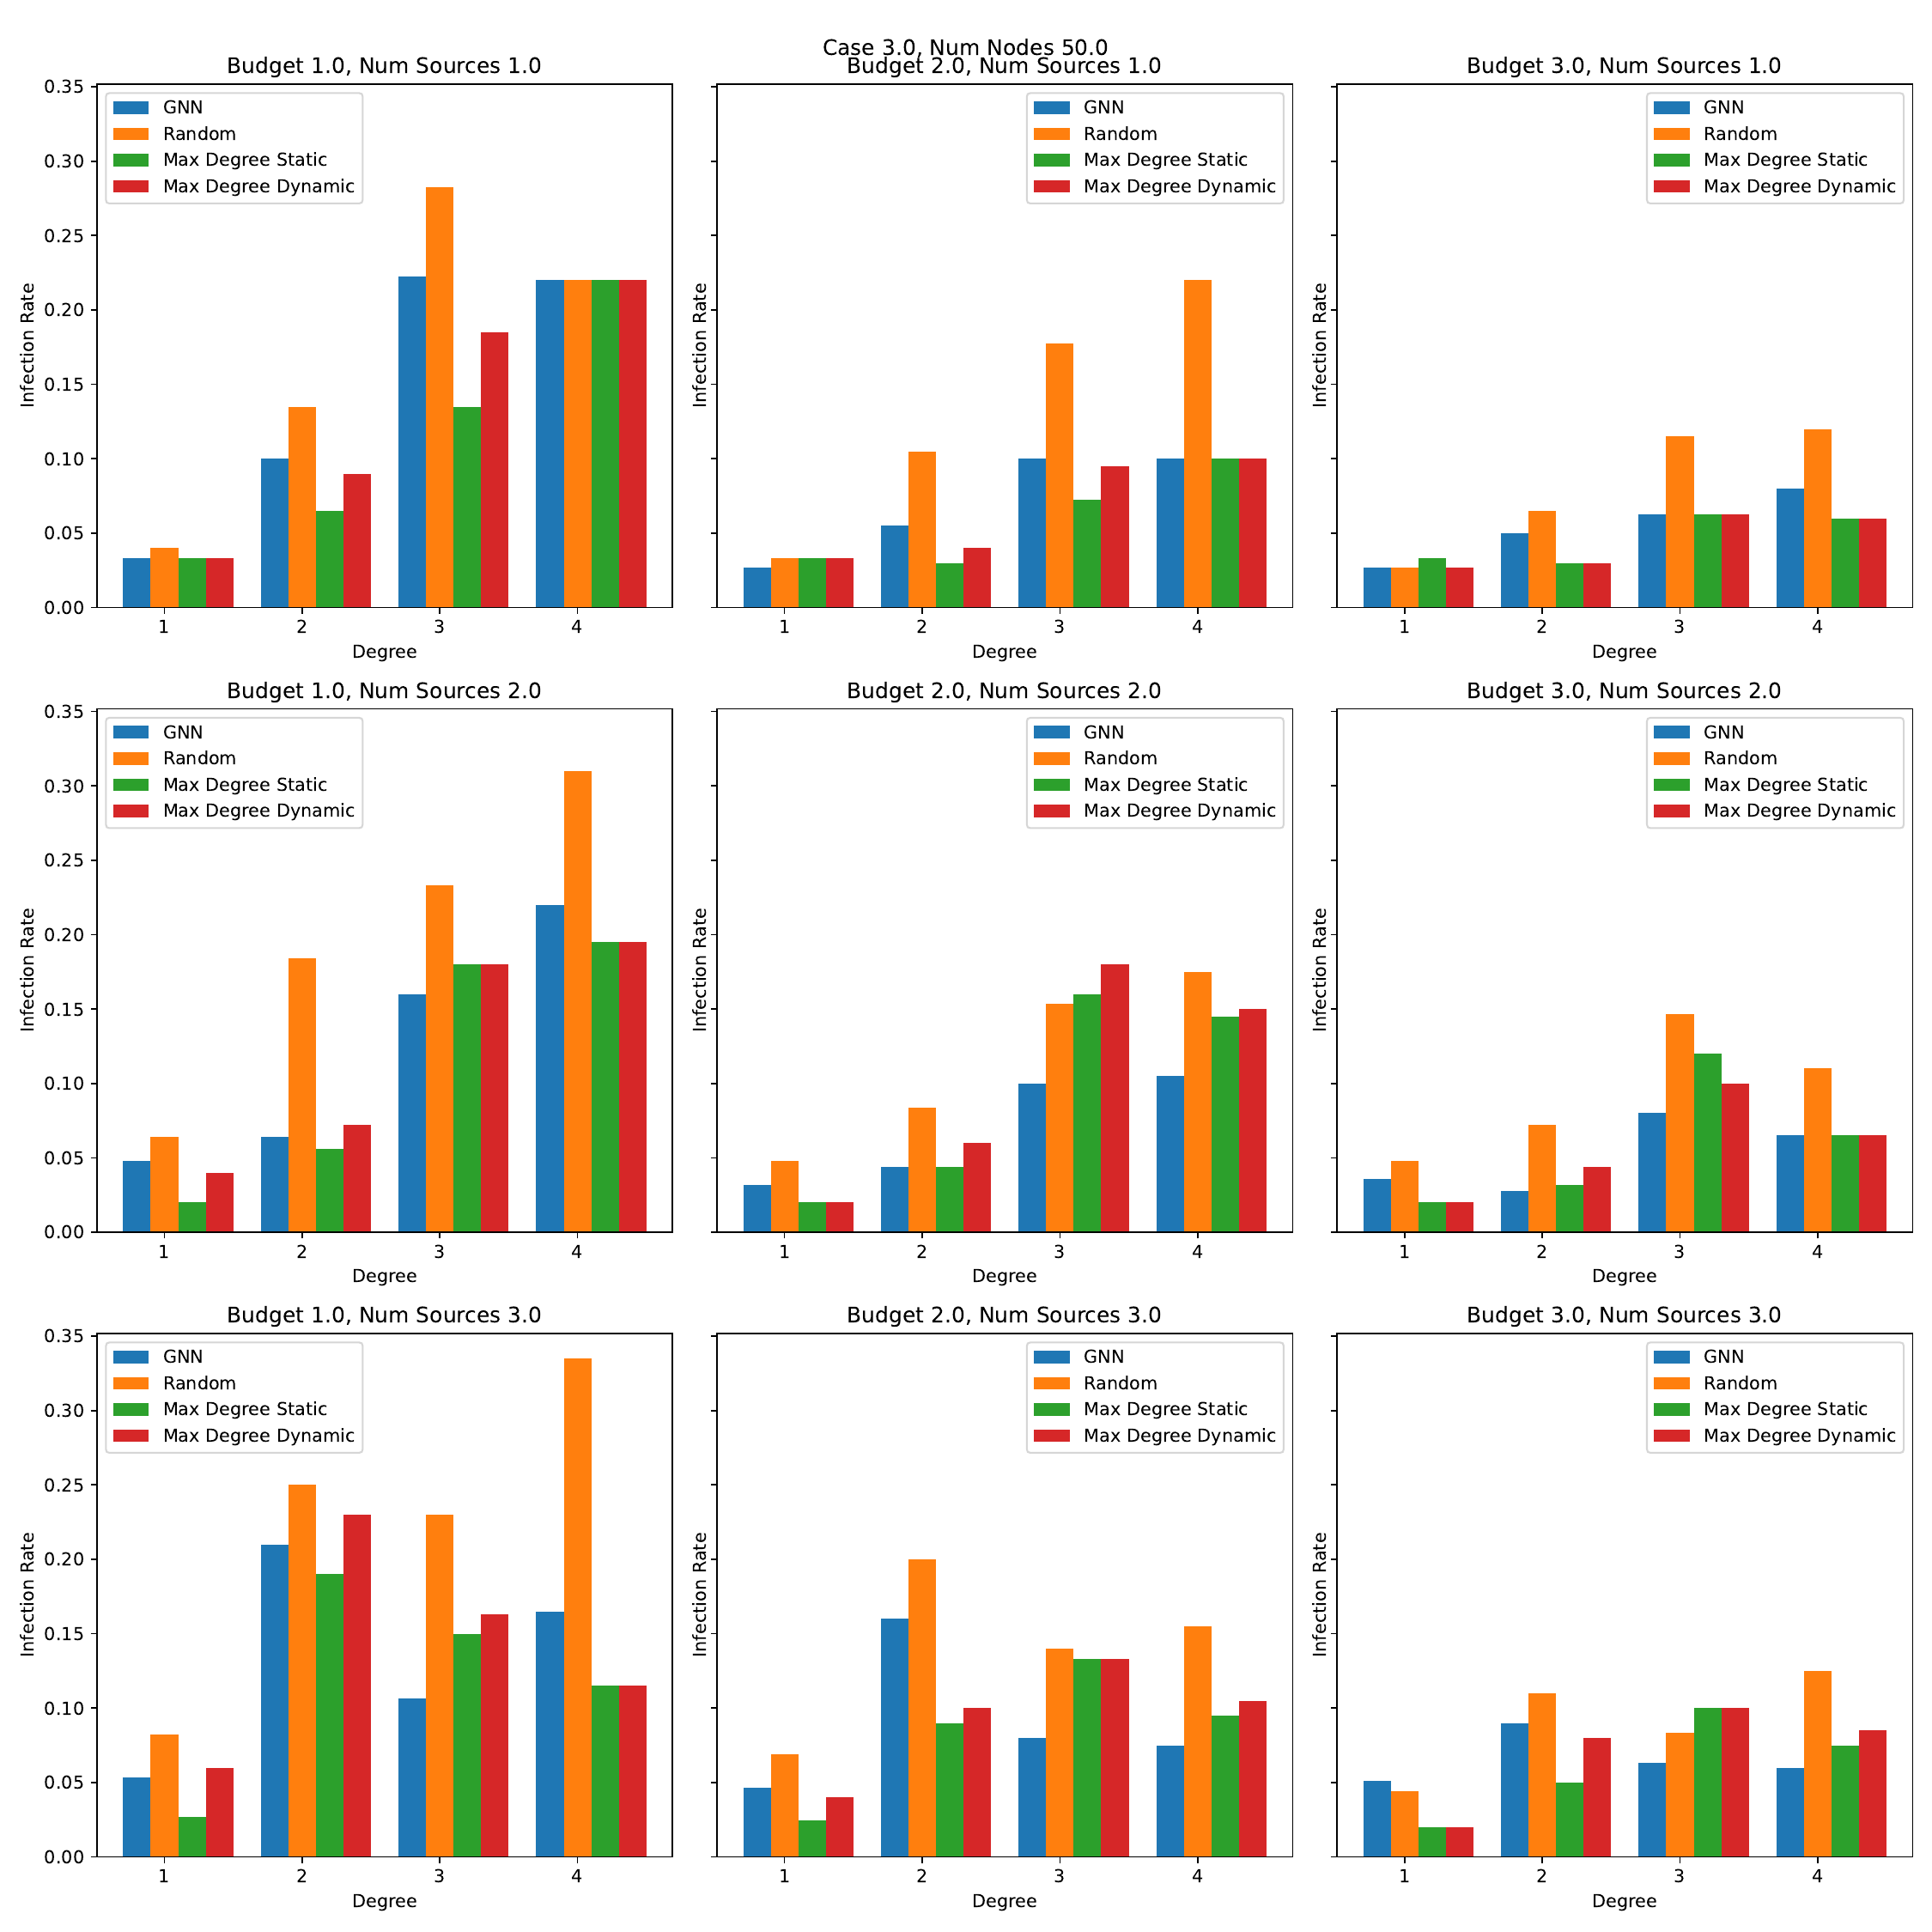}
    \caption{\footnotesize Dataset: Tree, Case-3 Node-50: Performance Evaluation of GCN-Based Supervised Learning Model: This series of bar plots presents a comparative analysis between our GCN-based SL model (blue), Randomized Policy model(yellow), Max Degree Policy model (Static) (green) and Max Degree Policy model (Dynamic) (red) on 25-node network environment. Progressing from left to right, the plots depict scenarios with increasing action budgets, ranging from 1 to 3 actions permitted. Vertically, the plots are ordered to show the effect of varying the initial count of infected nodes, starting with one and increasing to three. Each set of bars within the plots is categorized by the average connectivity (degree) of the infected nodes.}
    \label{fig:Treec3n50}
\end{figure}

\begin{figure}[!h]
    \centering
    \includegraphics[scale=0.3]{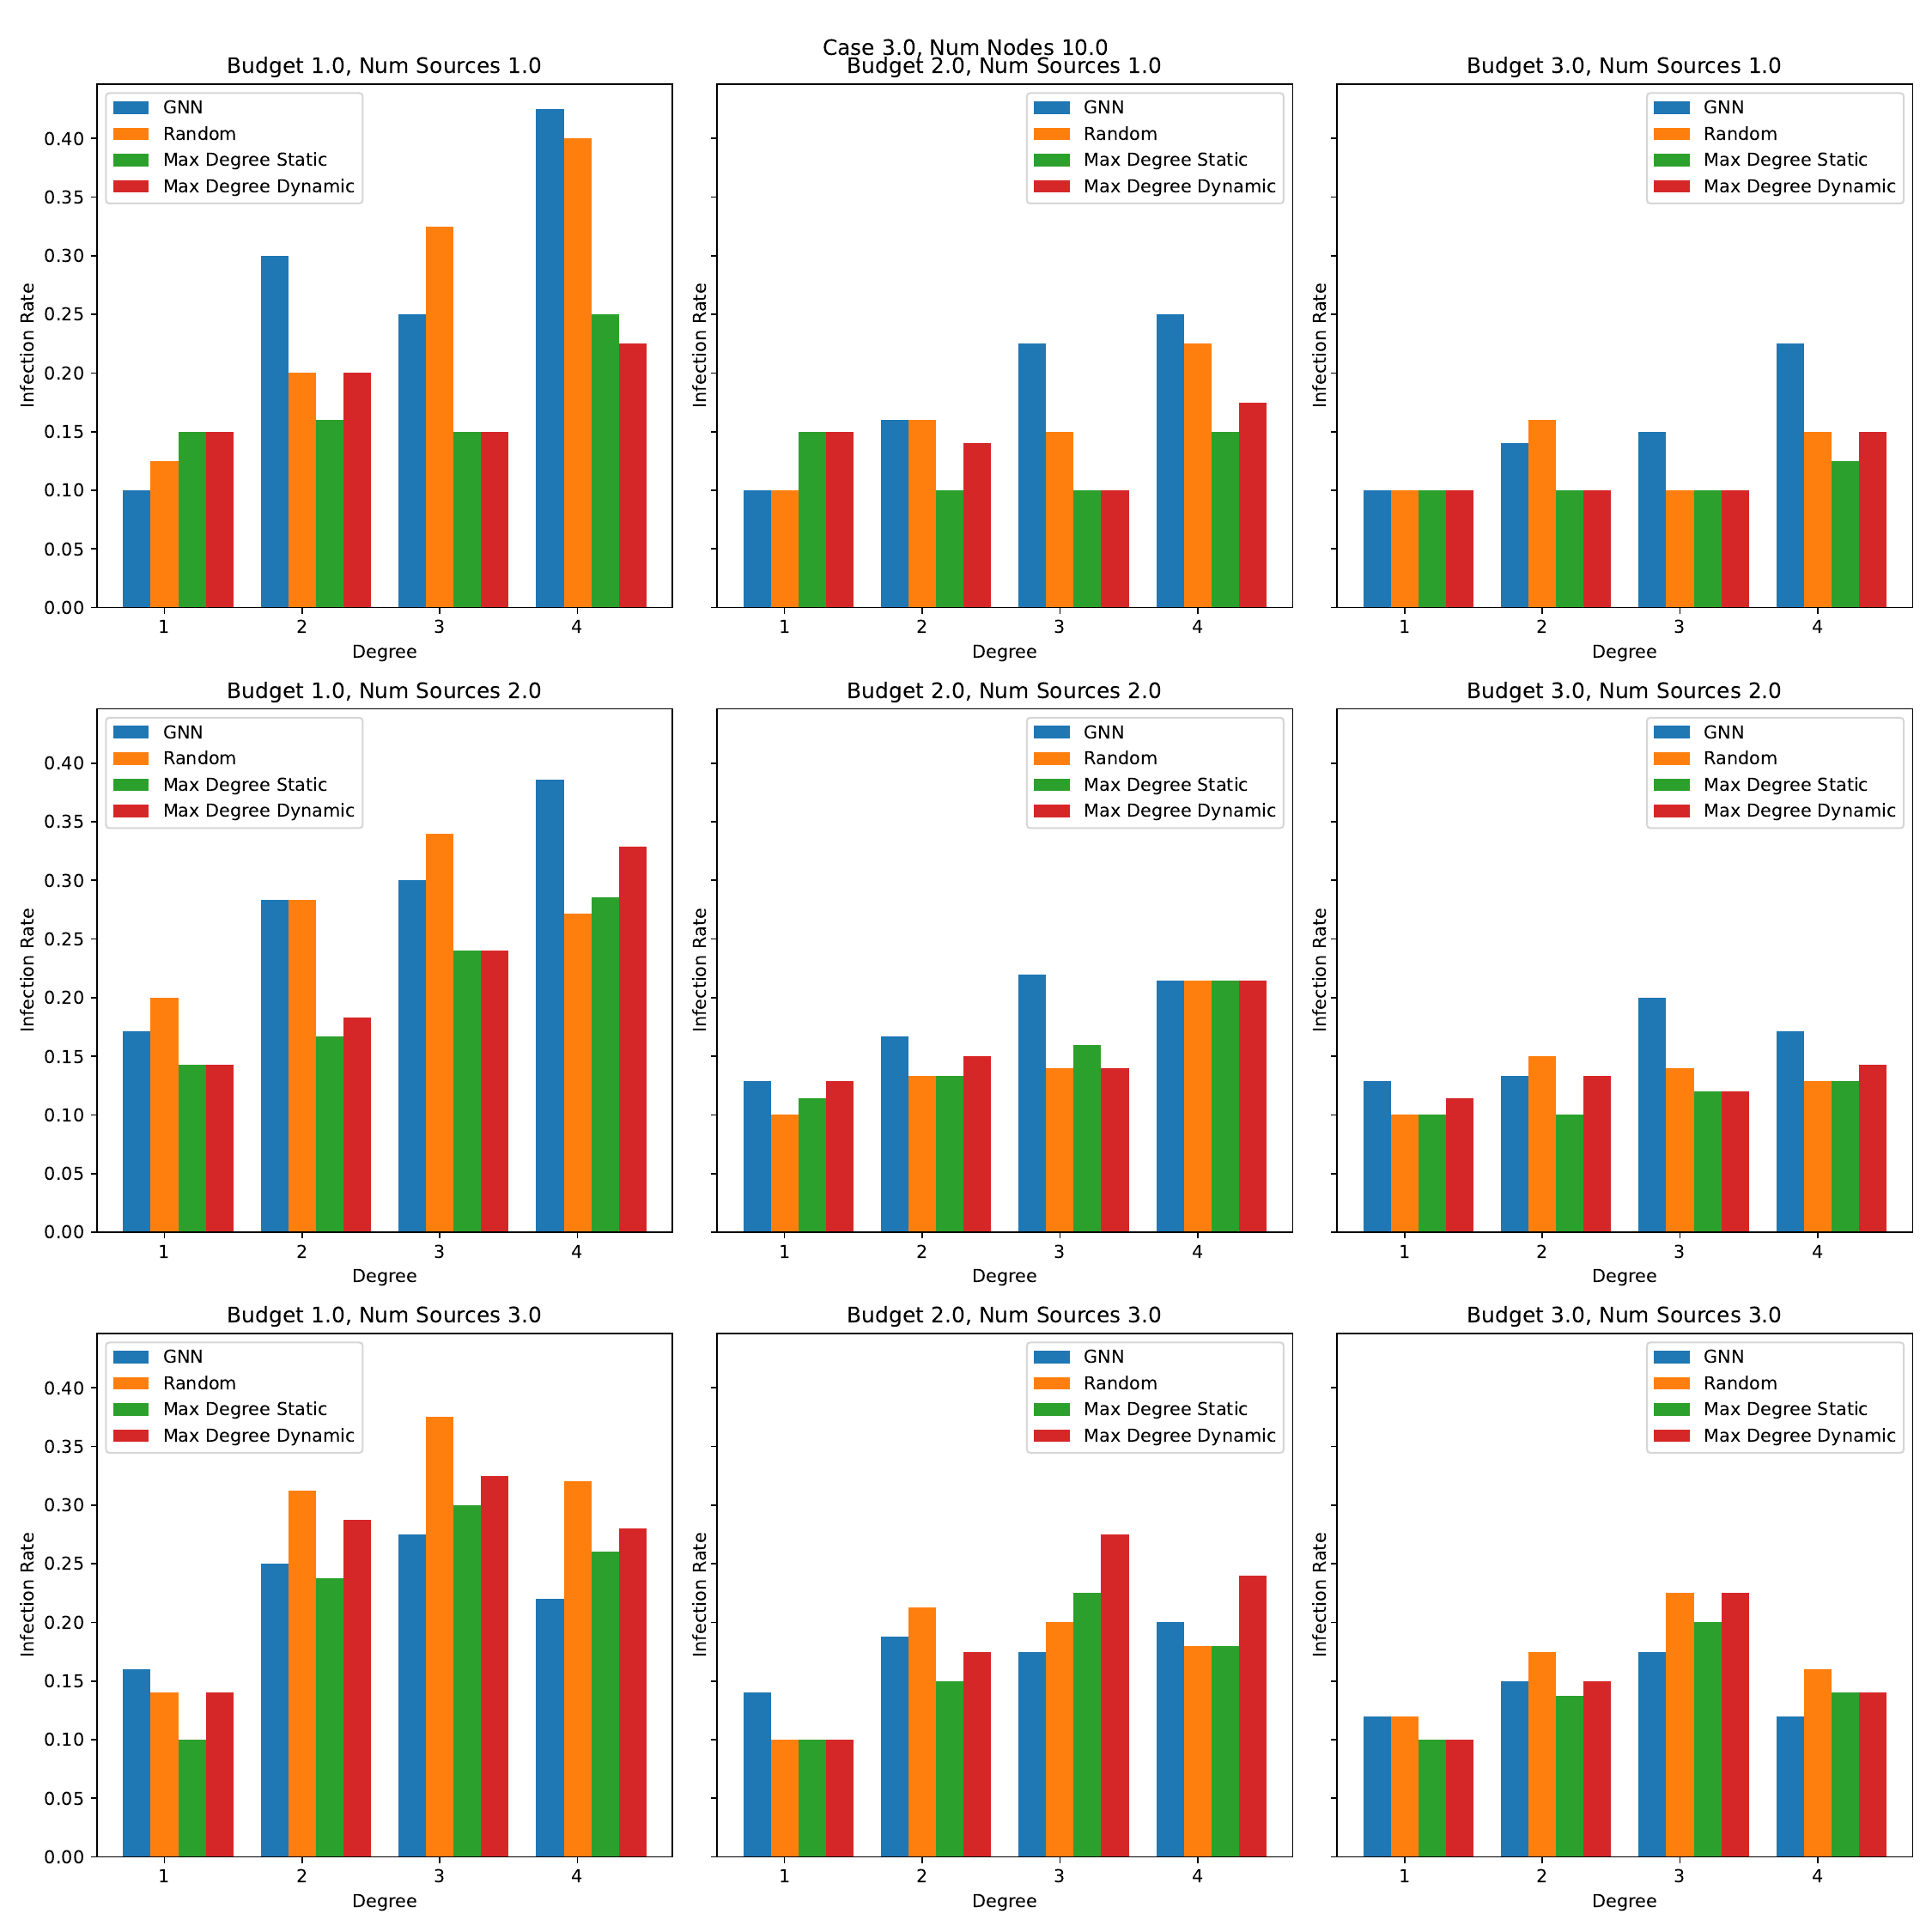}
    \caption{\footnotesize Dataset: Erdos-Renyi, Case-3 Node-10: Performance Evaluation of GCN-Based Supervised Learning Model: This series of bar plots presents a comparative analysis between our GCN-based SL model (blue), Randomized Policy model(yellow), Max Degree Policy model (Static) (green) and Max Degree Policy model (Dynamic) (red) on 25-node network environment. Progressing from left to right, the plots depict scenarios with increasing action budgets, ranging from 1 to 3 actions permitted. Vertically, the plots are ordered to show the effect of varying the initial count of infected nodes, starting with one and increasing to three. Each set of bars within the plots is categorized by the average connectivity (degree) of the infected nodes.}
    \label{fig:ERc3n10}
\end{figure}

\begin{figure}[!h]
    \centering
    \includegraphics[scale=0.3]{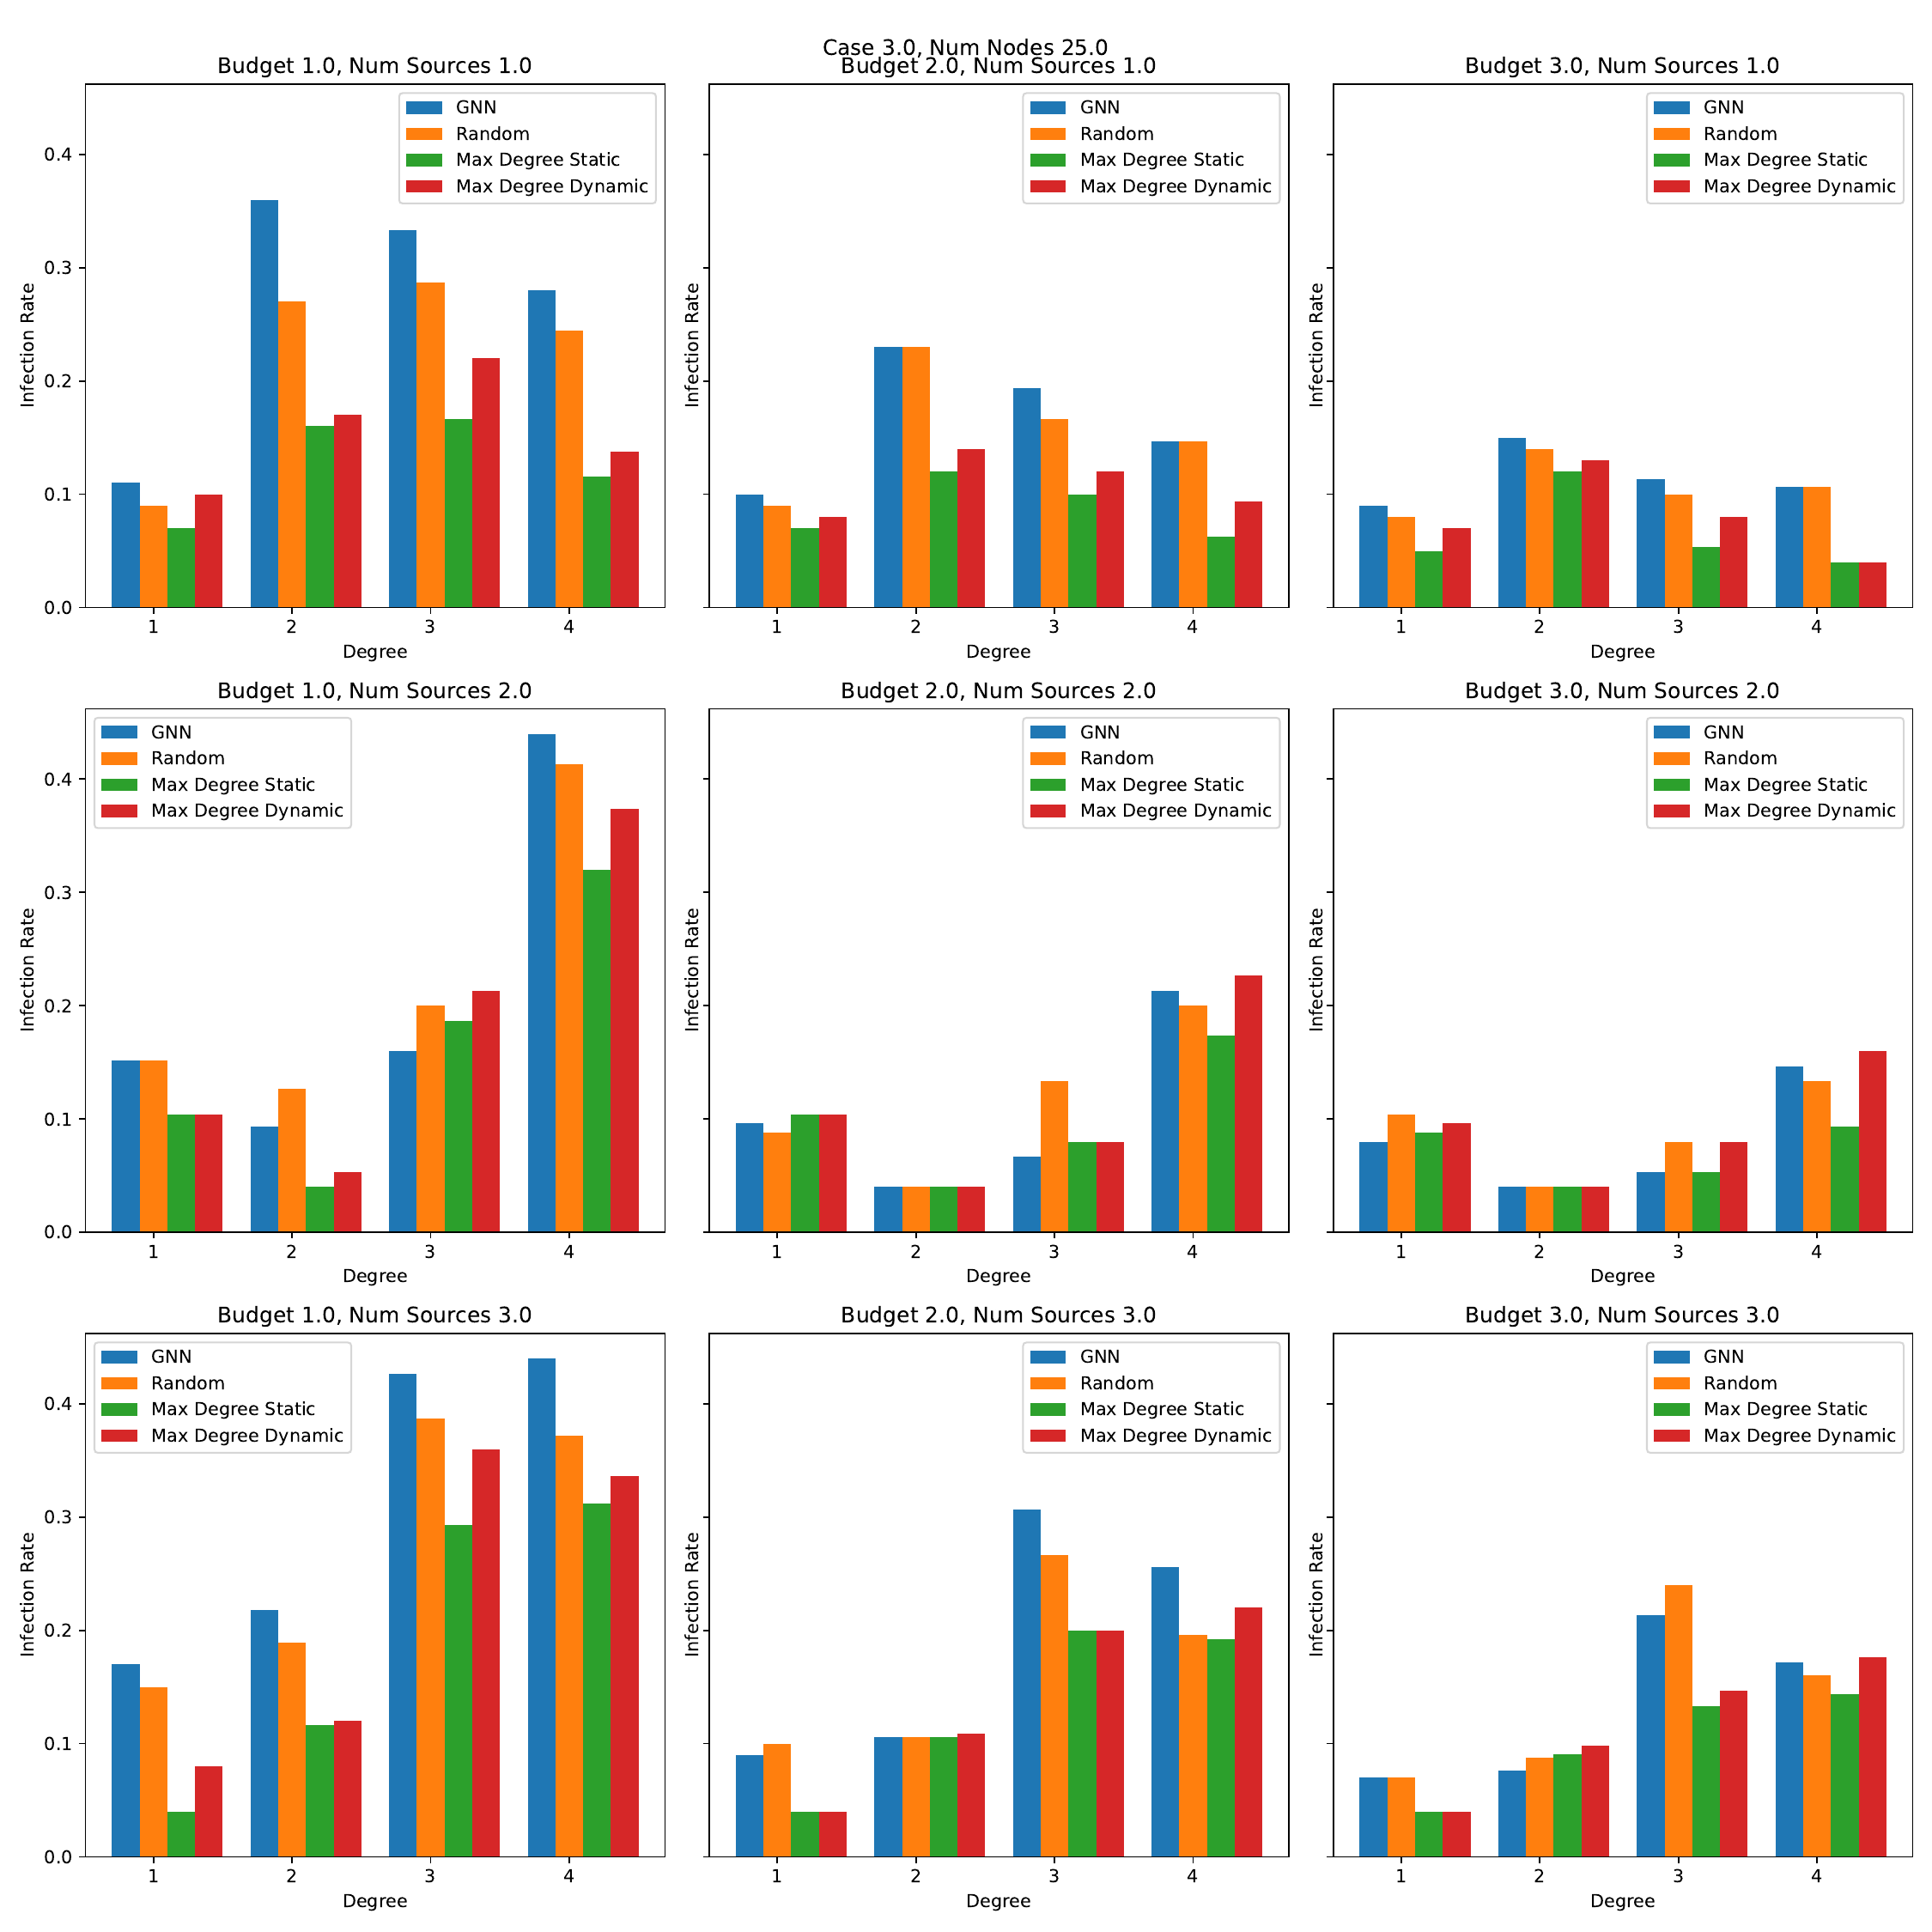}
    \caption{\footnotesize Dataset: Erdos-Renyi, Case-3 Node-25: Performance Evaluation of GCN-Based Supervised Learning Model: This series of bar plots presents a comparative analysis between our GCN-based SL model (blue), Randomized Policy model(yellow), Max Degree Policy model (Static) (green) and Max Degree Policy model (Dynamic) (red) on 25-node network environment. Progressing from left to right, the plots depict scenarios with increasing action budgets, ranging from 1 to 3 actions permitted. Vertically, the plots are ordered to show the effect of varying the initial count of infected nodes, starting with one and increasing to three. Each set of bars within the plots is categorized by the average connectivity (degree) of the infected nodes.}
    \label{fig:ERc3n25}
\end{figure}

\begin{figure}[!h]
    \centering
    \includegraphics[scale=0.3]{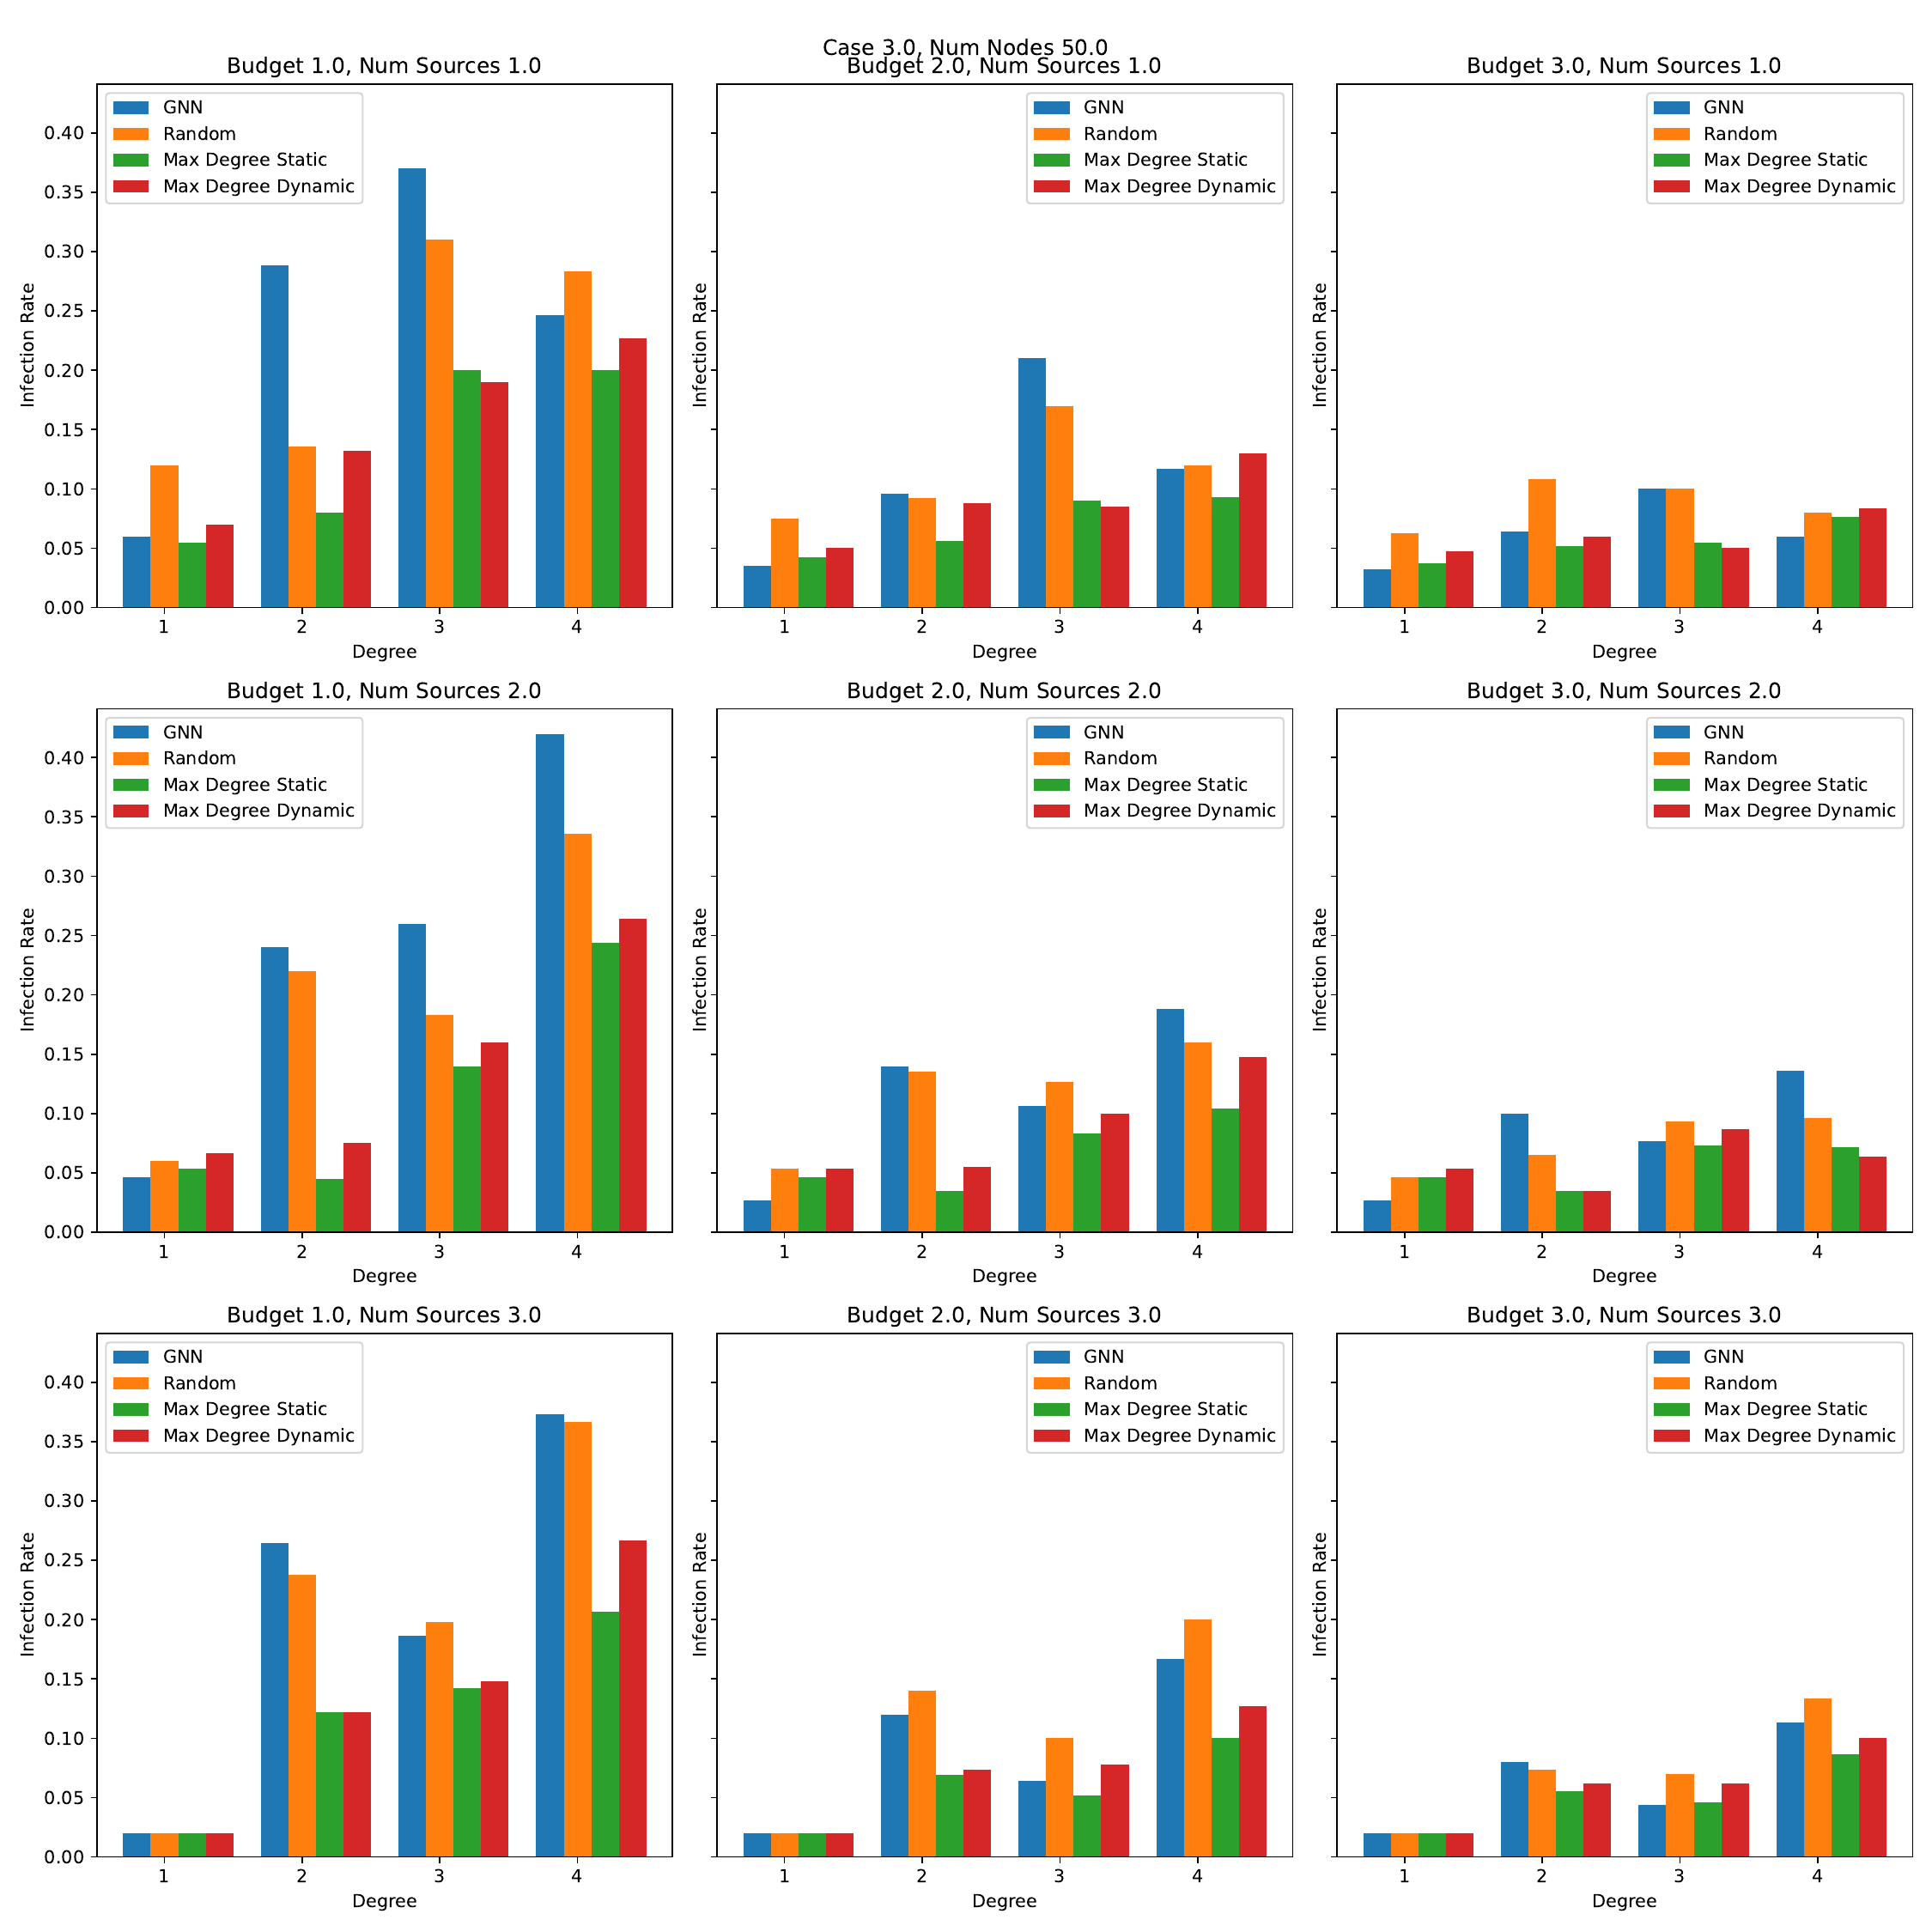}
    \caption{\footnotesize Dataset: Erdos-Renyi, Case-3 Node-50: Performance Evaluation of GCN-Based Supervised Learning Model: This series of bar plots presents a comparative analysis between our GCN-based SL model (blue), Randomized Policy model(yellow), Max Degree Policy model (Static) (green) and Max Degree Policy model (Dynamic) (red) on 25-node network environment. Progressing from left to right, the plots depict scenarios with increasing action budgets, ranging from 1 to 3 actions permitted. Vertically, the plots are ordered to show the effect of varying the initial count of infected nodes, starting with one and increasing to three. Each set of bars within the plots is categorized by the average connectivity (degree) of the infected nodes.}
    \label{fig:ERc3n50}
\end{figure}

%%%%%%%%%%%%%%%%%%%%%%%%%%%%%%%%%%

% ######################################
% ################ RL ##################
% ######################################

%###### Case 1 ResNet Figures #######

%%%%% R0 %%%%%%%%
\begin{figure}[!h]
    \centering
    \includegraphics[scale=0.34]{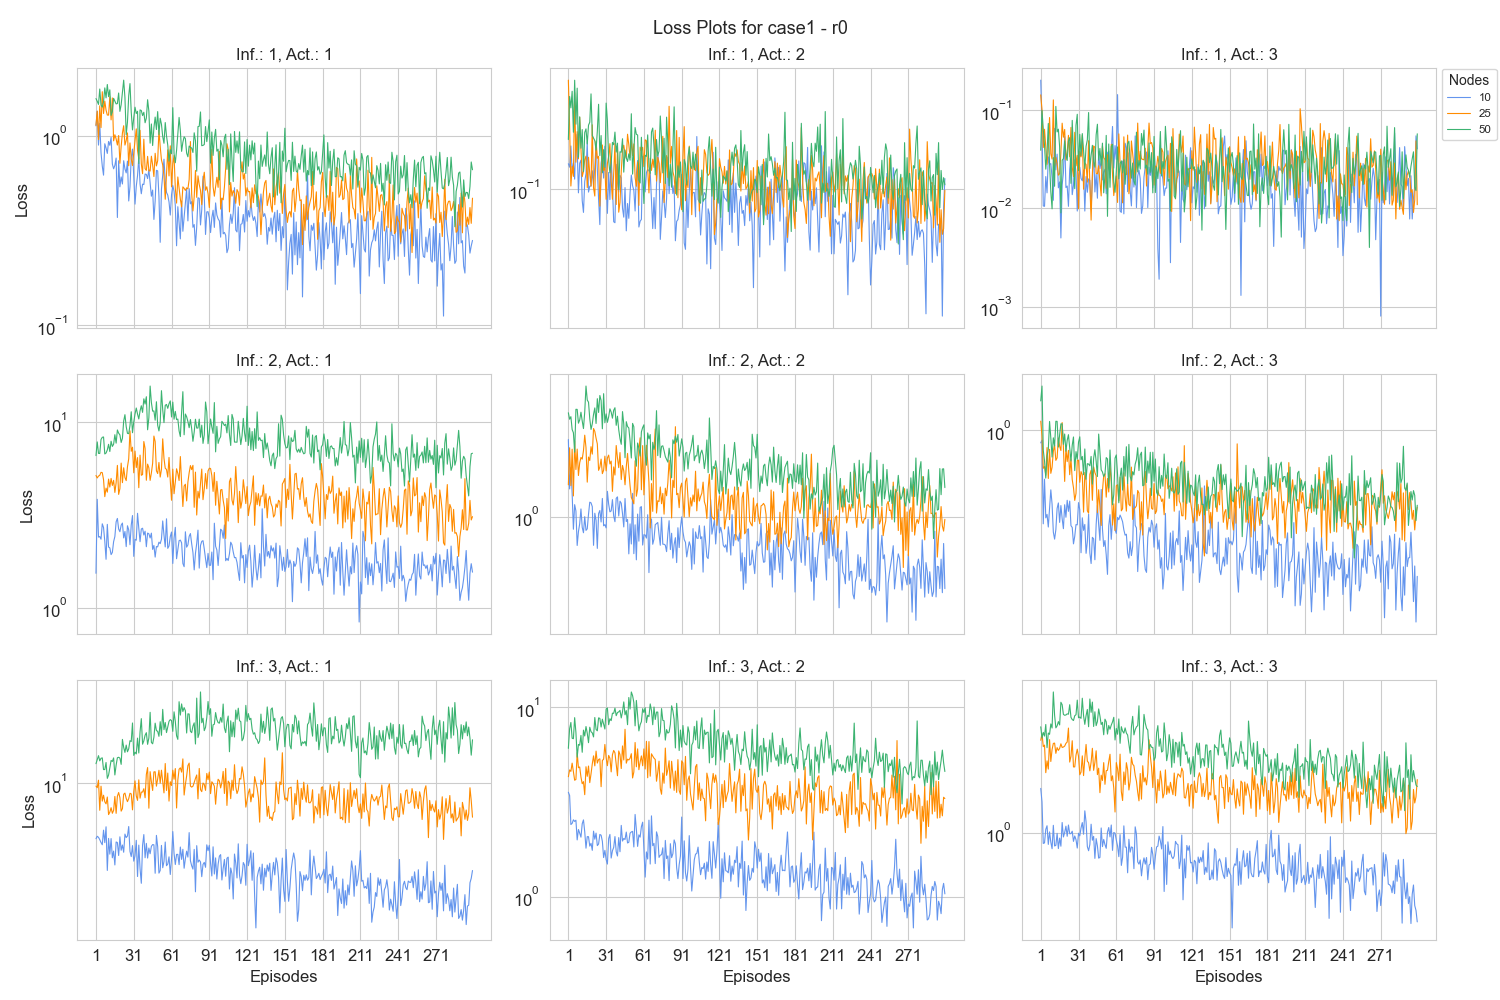}
    \caption{\footnotesize Case-1 using R0: Training MSE loss evolution for RL policy using ResNet model across networks of 10 (blue), 25 (orange), and 50 (green) nodes, for varying initial misinformation sources (Inf.) and action budgets (Act.). Plotted on a logarithmic scale, the loss decreases over episodes, indicating improved policy performance and adaptation across network sizes.}
    \label{fig:resnet_c1r0_loss}
\end{figure}

\begin{figure}
    \centering
    \includegraphics[scale=0.34]{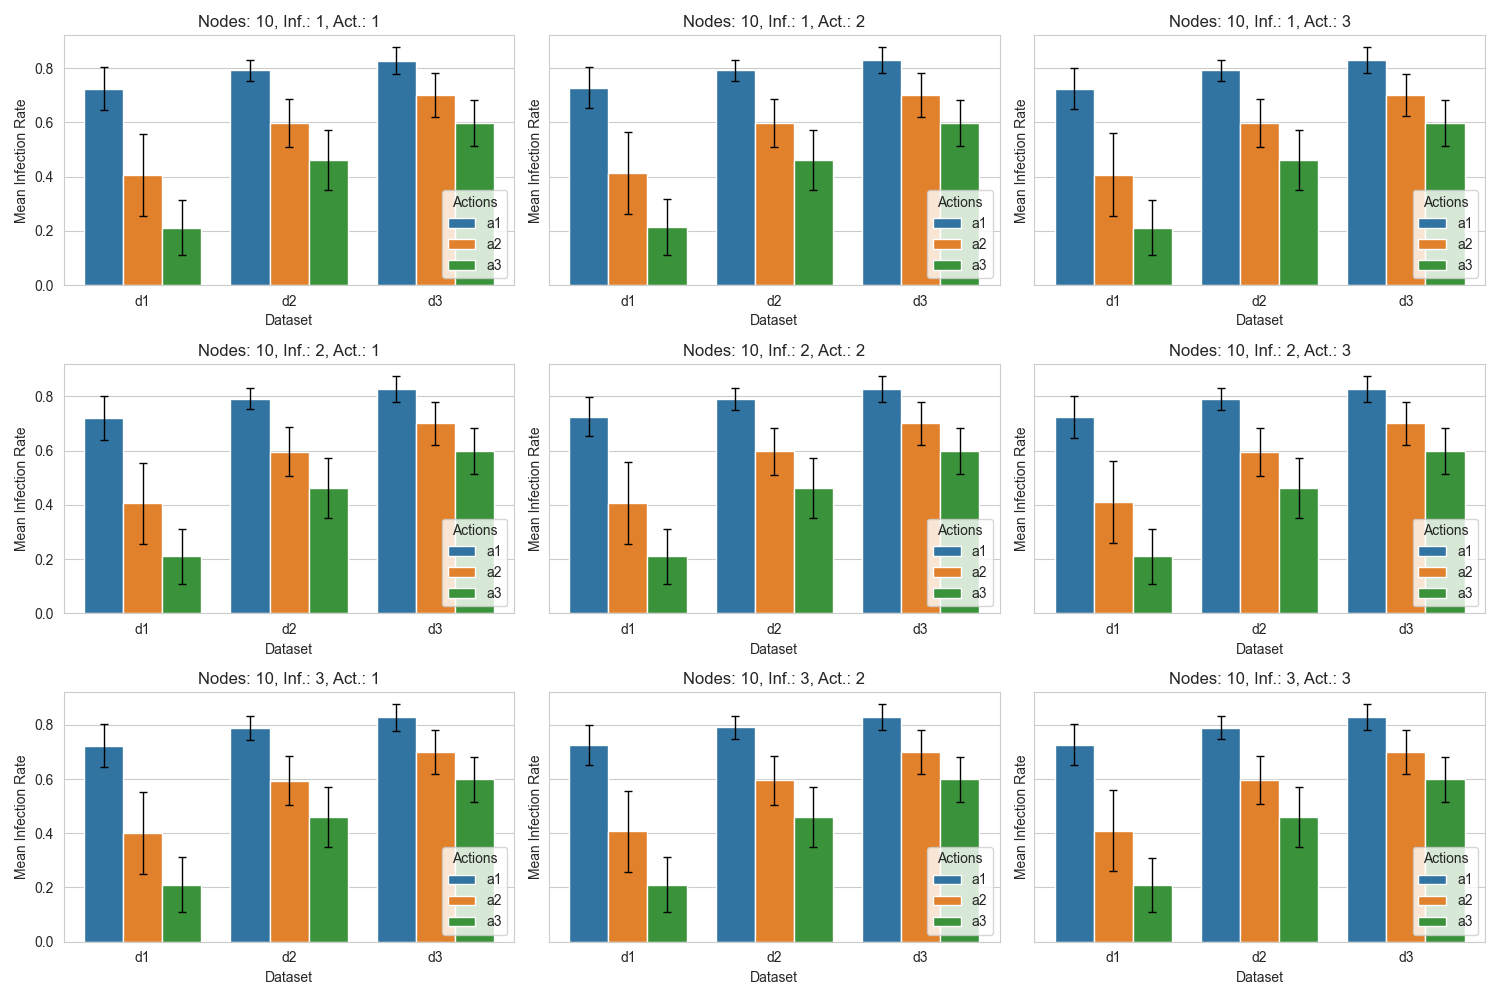}
    \caption{Case-1 using R0: Performance comparison of the RL policies trained using ResNet model for a 10-node network. The barplot displays the mean infection rate for datasets d1, d2, and d3 of Dataset v1 type, differentiated by the number of initial misinformation sources (Inf.) and action budgets (Act.: a1, a2, a3). Each subplot illustrates the performance of a policy trained with the parameters indicated in its title. Lower infection rates indicate more effective policy learning and misinformation containment.}
    \label{fig:inf_resnet_c1r0_10}
\end{figure}

\begin{figure}
    \centering
    \includegraphics[scale=0.34]{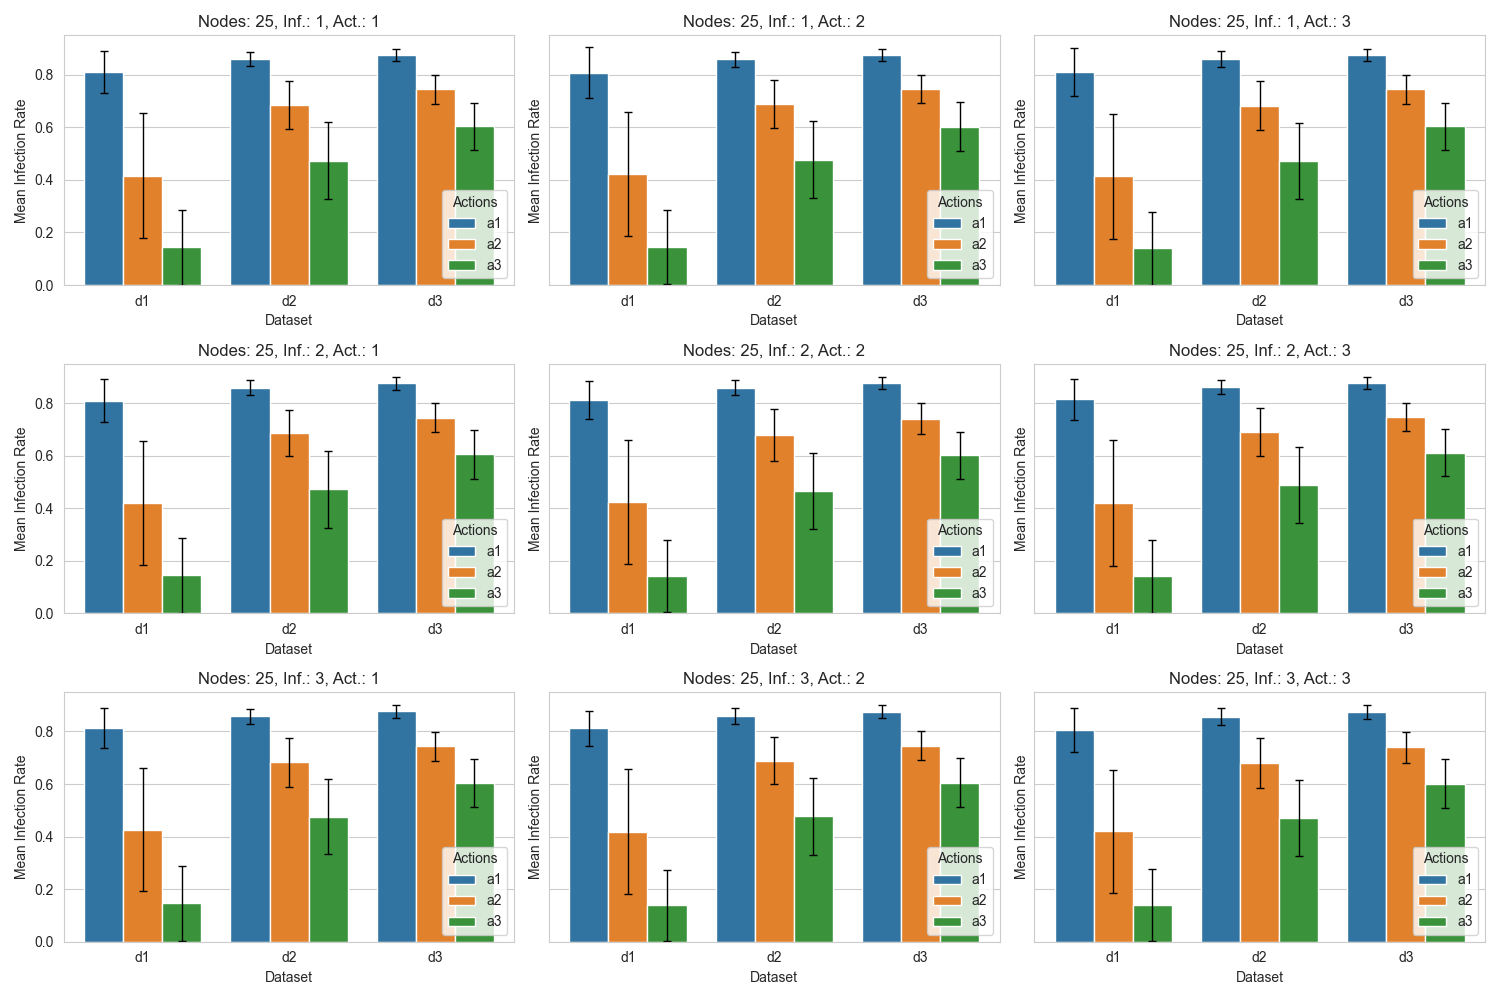}
    \caption{Case-1 using R0: Performance comparison of the RL policies trained using ResNet model for a 25-node network. The barplot displays the mean infection rate for datasets d1, d2, and d3 of Dataset v1 type, differentiated by the number of initial misinformation sources (Inf.) and action budgets (Act.: a1, a2, a3). Each subplot illustrates the performance of a policy trained with the parameters indicated in its title. Lower infection rates indicate more effective policy learning and misinformation containment.}
    \label{fig:inf_resnet_c1r0_25}
\end{figure}

\begin{figure}
    \centering
    \includegraphics[scale=0.34]{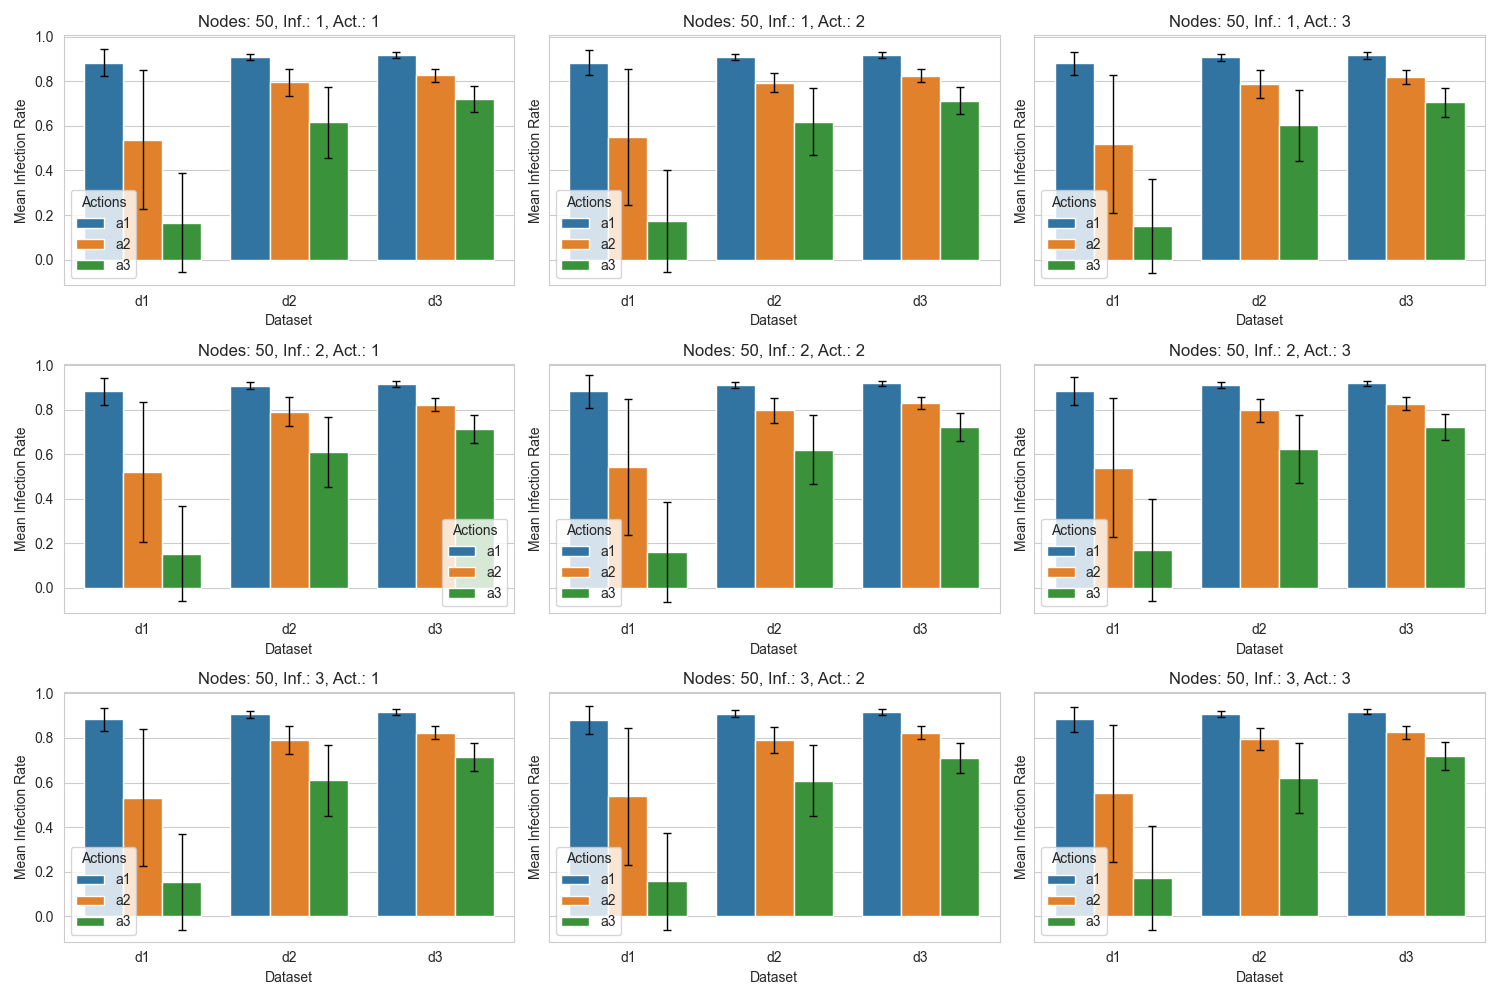}
    \caption{Case-1 using R0: Performance comparison of the RL policies trained using ResNet model for a 50-node network. The barplot displays the mean infection rate for datasets d1, d2, and d3 of Dataset v1 type, differentiated by the number of initial misinformation sources (Inf.) and action budgets (Act.: a1, a2, a3). Each subplot illustrates the performance of a policy trained with the parameters indicated in its title. Lower infection rates indicate more effective policy learning and misinformation containment.}
    \label{fig:inf_resnet_c1r0_50}
\end{figure}

%%%%%% R1 %%%%%%%%

\begin{figure}[!h]
    \centering
    \includegraphics[scale=0.34]{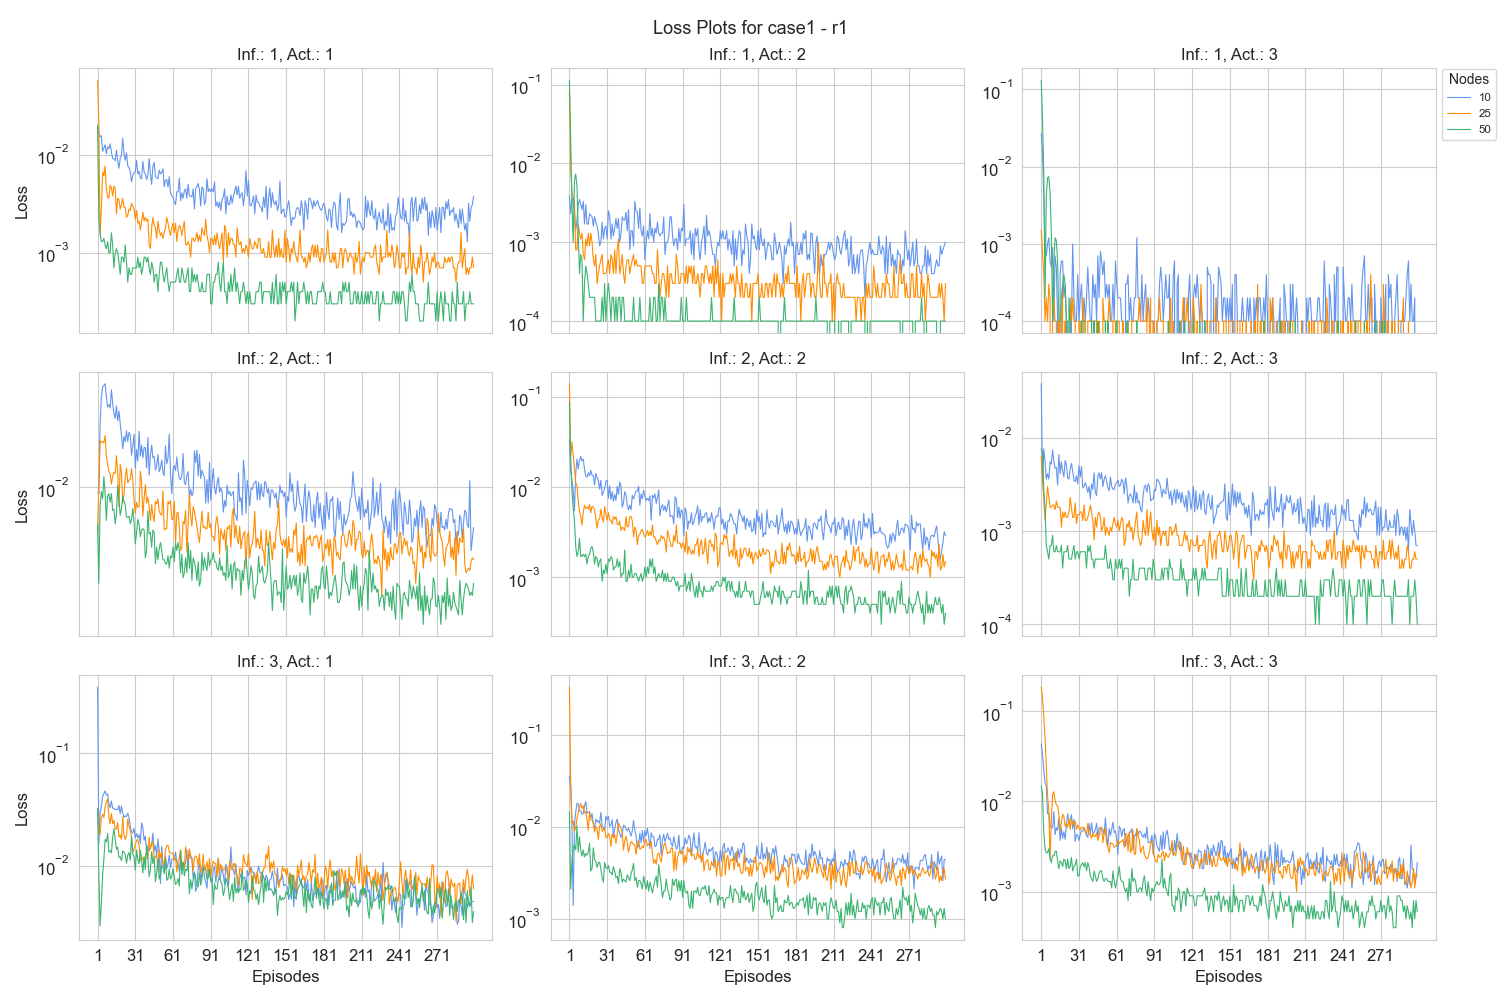}
    \caption{Case-1 using R1: Training MSE loss evolution for RL policy using ResNet model across networks of 10 (blue), 25 (orange), and 50 (green) nodes, for varying initial misinformation sources (Inf.) and action budgets (Act.). Plotted on a logarithmic scale, the loss decreases over episodes, indicating improved policy performance and adaptation across network sizes.}
    \label{fig:resnet_c1r1_loss}
\end{figure}

\begin{figure}
    \centering
    \includegraphics[scale=0.34]{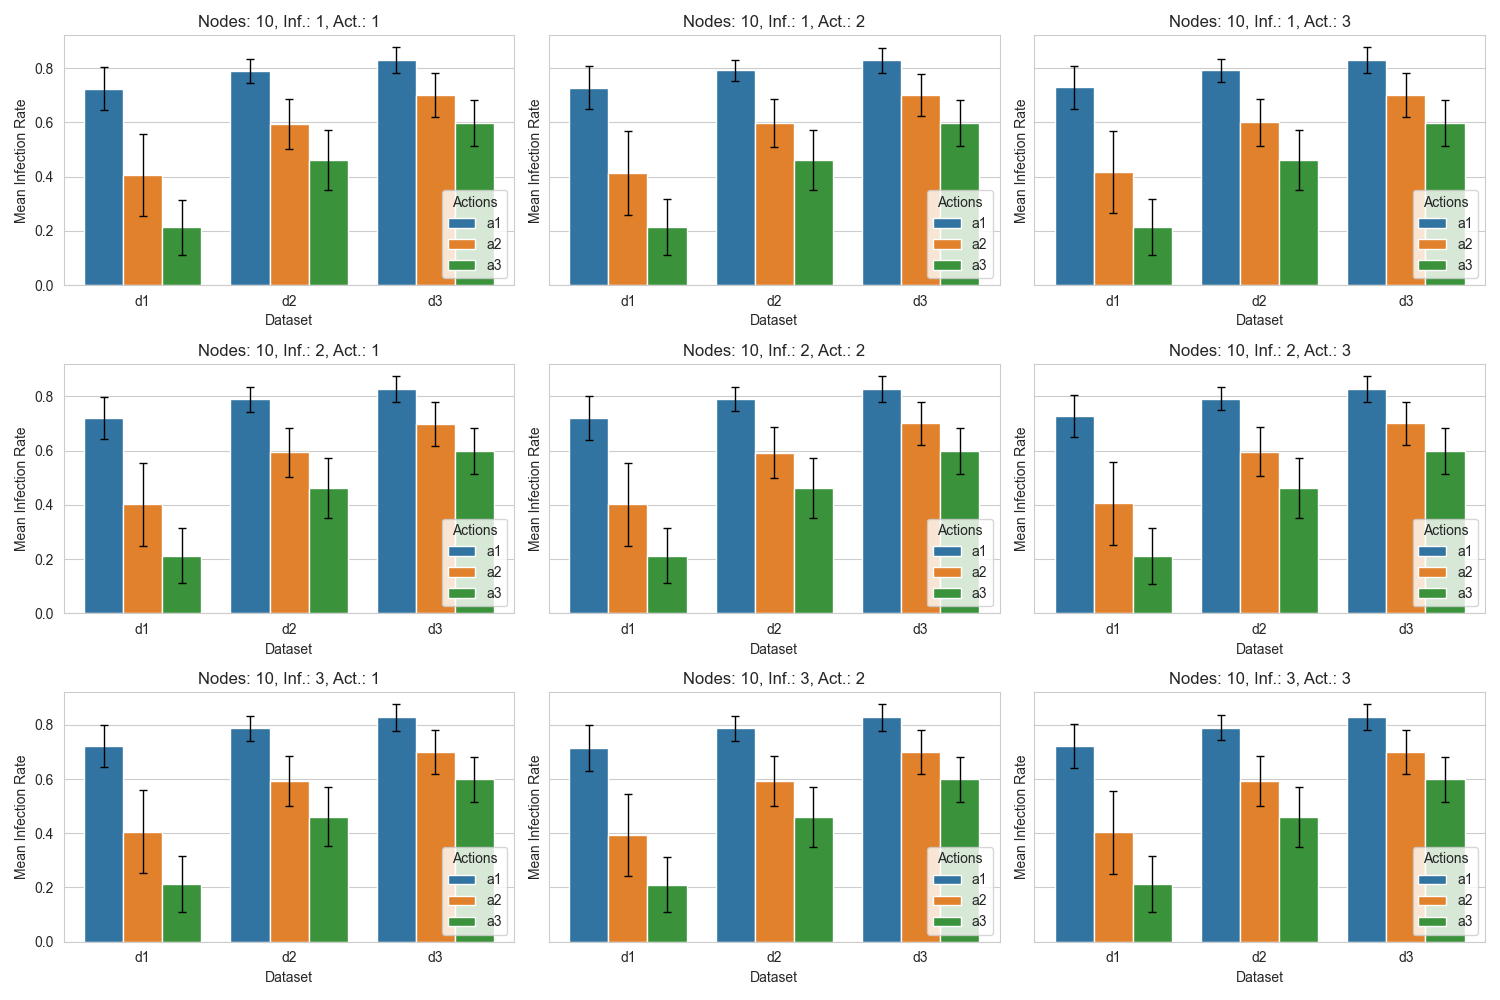}
    \caption{Case-1 using R1: Performance comparison of the RL policies trained using ResNet model for a 10-node network. The barplot displays the mean infection rate for datasets d1, d2, and d3 of Dataset v1 type, differentiated by the number of initial misinformation sources (Inf.) and action budgets (Act.: a1, a2, a3). Each subplot illustrates the performance of a policy trained with the parameters indicated in its title. Lower infection rates indicate more effective policy learning and misinformation containment.}
    \label{fig:inf_resnet_c1r1_10}
\end{figure}

\begin{figure}
    \centering
    \includegraphics[scale=0.34]{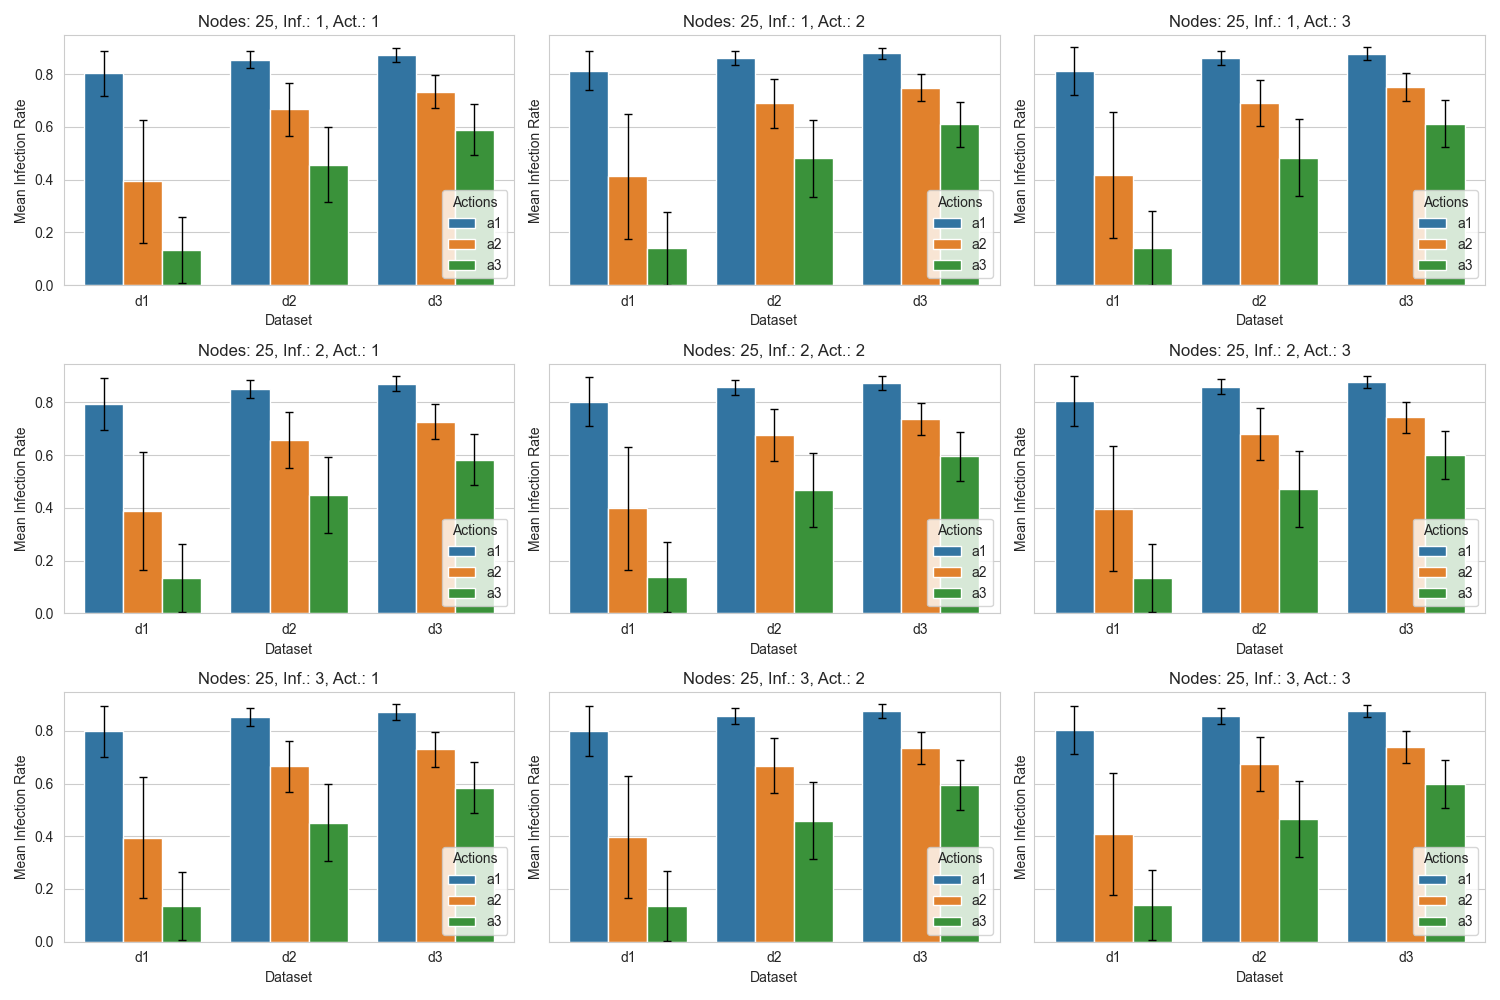}
    \caption{Case-1 using R1: Performance comparison of the RL policies trained using ResNet model for a 25-node network. The barplot displays the mean infection rate for datasets d1, d2, and d3 of Dataset v1 type, differentiated by the number of initial misinformation sources (Inf.) and action budgets (Act.: a1, a2, a3). Each subplot illustrates the performance of a policy trained with the parameters indicated in its title. Lower infection rates indicate more effective policy learning and misinformation containment.}
    \label{fig:inf_resnet_c1r1_25}
\end{figure}

\begin{figure}
    \centering
    \includegraphics[scale=0.34]{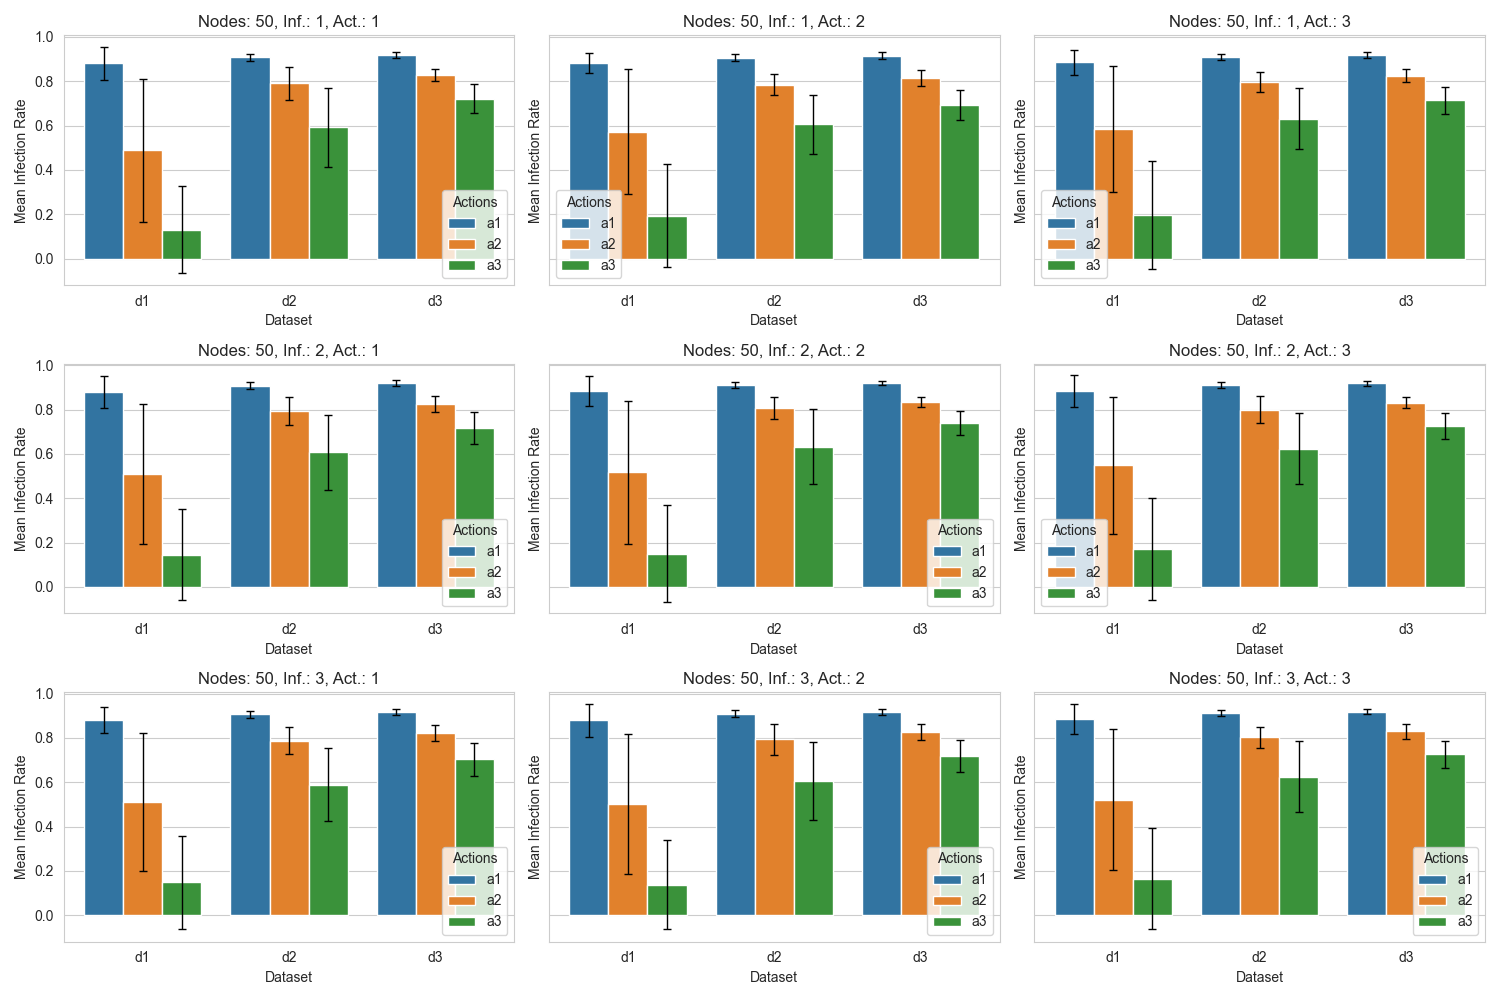}
    \caption{Case-1 using R1: Performance comparison of the RL policies trained using ResNet model for a 50-node network. The barplot displays the mean infection rate for datasets d1, d2, and d3 of Dataset v1 type, differentiated by the number of initial misinformation sources (Inf.) and action budgets (Act.: a1, a2, a3). Each subplot illustrates the performance of a policy trained with the parameters indicated in its title. Lower infection rates indicate more effective policy learning and misinformation containment.}
    \label{fig:inf_resnet_c1r1_50}
\end{figure}

%%%%%% R2 %%%%%%%%

\begin{figure}[!h]
    \centering
    \includegraphics[scale=0.34]{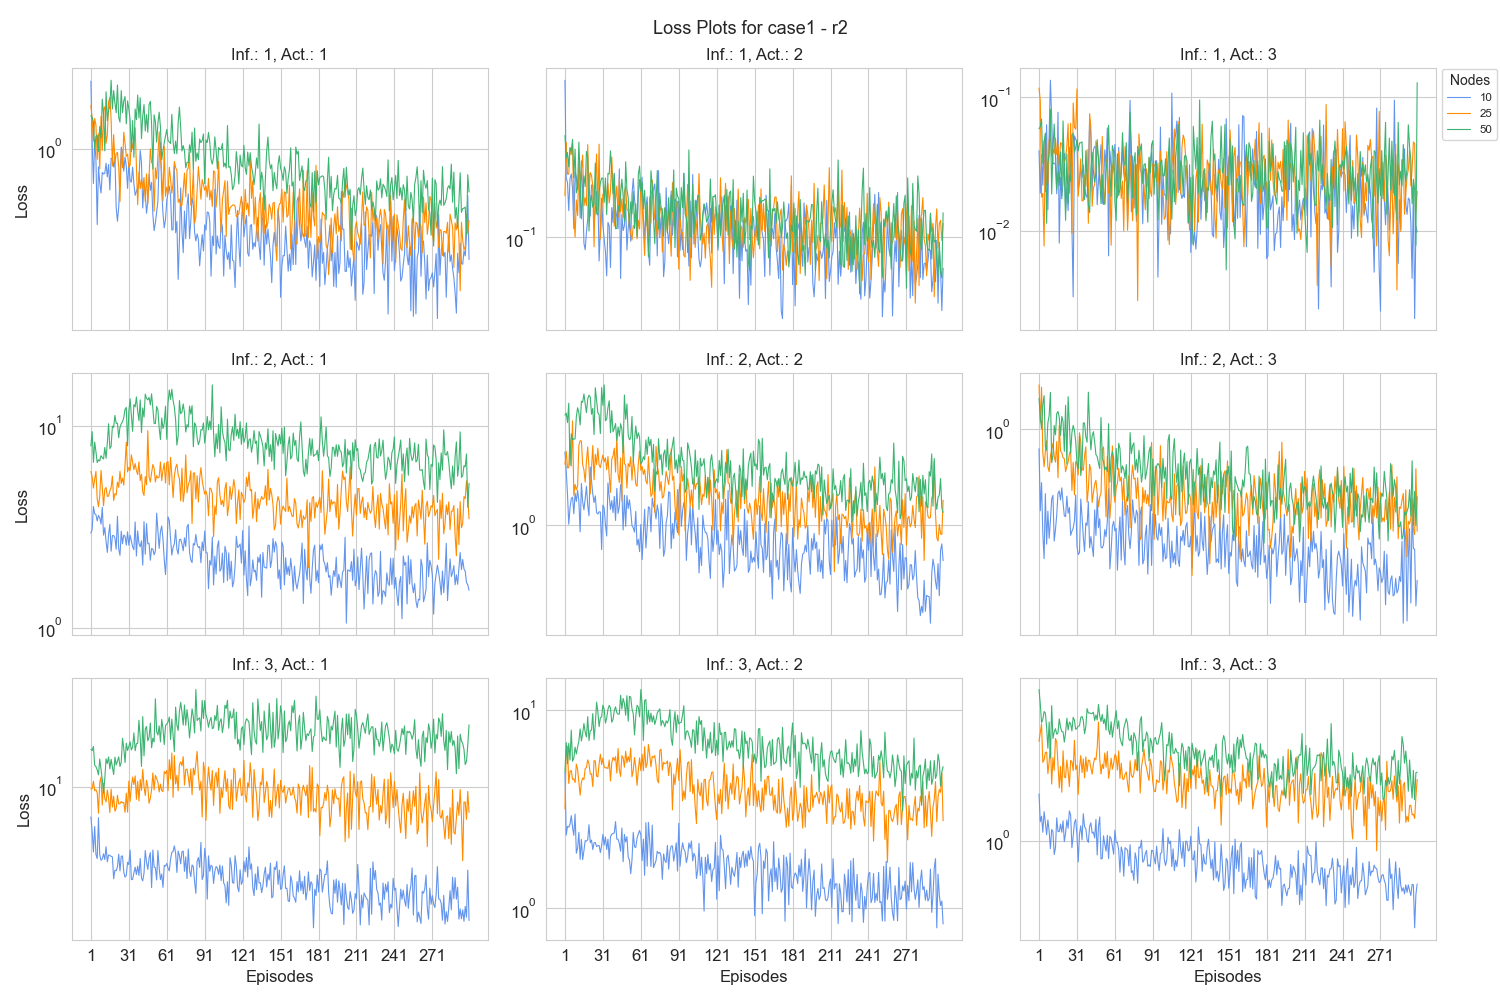}
    \caption{Case-1 using R2: Training MSE loss evolution for RL policy using ResNet model across networks of 10 (blue), 25 (orange), and 50 (green) nodes, for varying initial misinformation sources (Inf.) and action budgets (Act.). Plotted on a logarithmic scale, the loss decreases over episodes, indicating improved policy performance and adaptation across network sizes.}
    \label{fig:resnet_c1r2_loss}
\end{figure}

\begin{figure}
    \centering
    \includegraphics[scale=0.34]{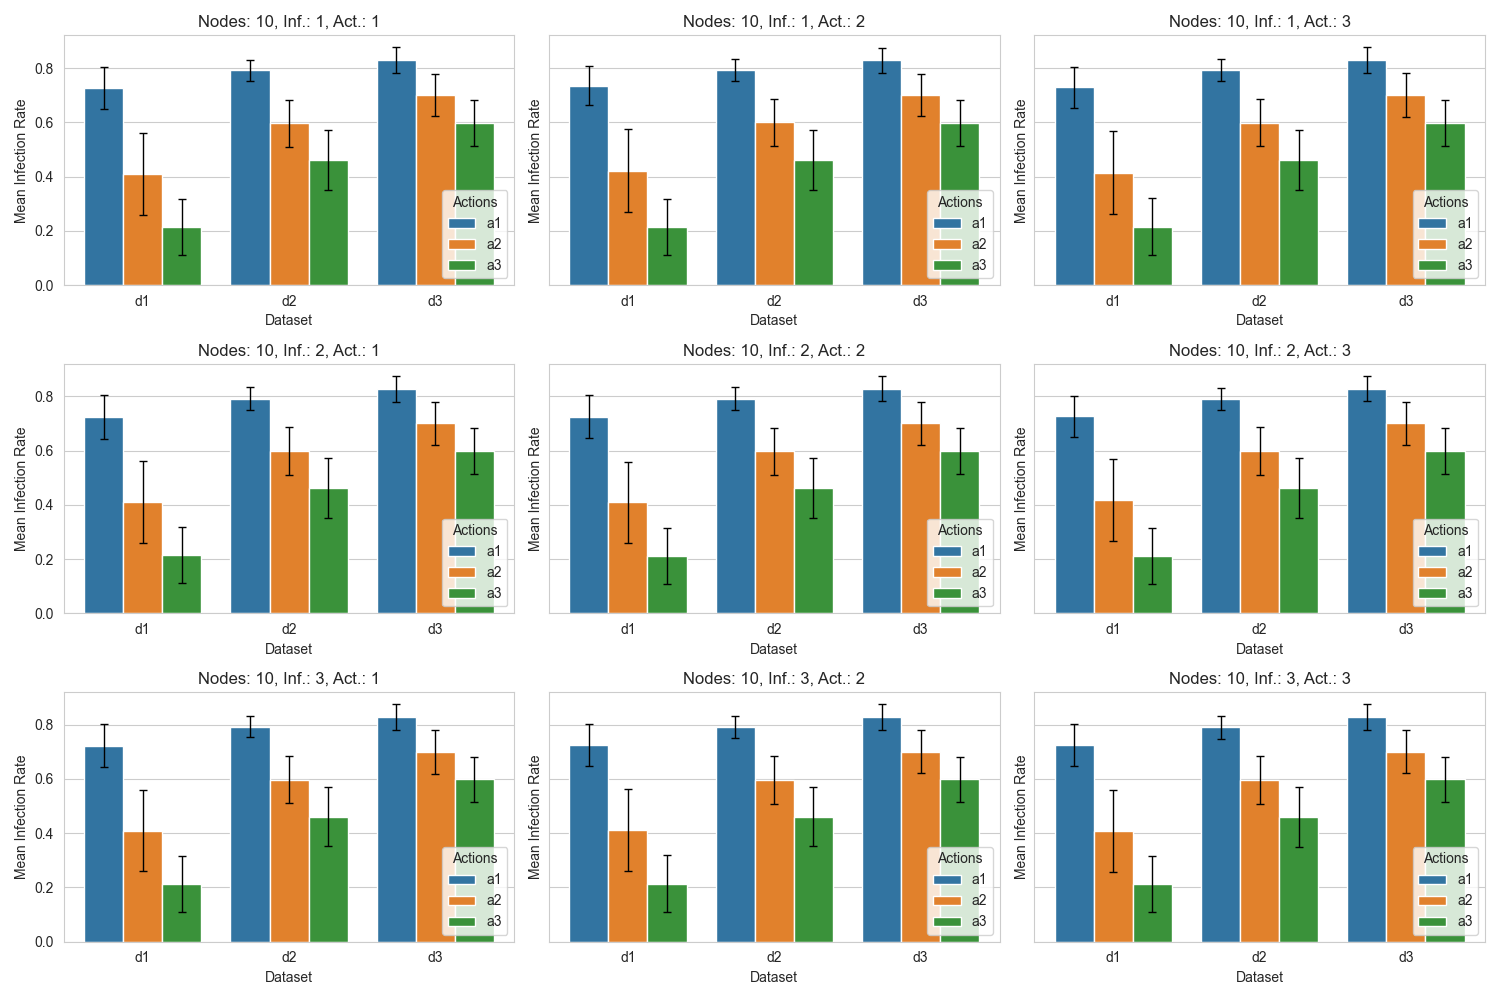}
    \caption{Case-1 using R2: Performance comparison of the RL policies trained using ResNet model for a 10-node network. The barplot displays the mean infection rate for datasets d1, d2, and d3 of Dataset v1 type, differentiated by the number of initial misinformation sources (Inf.) and action budgets (Act.: a1, a2, a3). Each subplot illustrates the performance of a policy trained with the parameters indicated in its title. Lower infection rates indicate more effective policy learning and misinformation containment.}
    \label{fig:inf_resnet_c1r2_10}
\end{figure}

\begin{figure}
    \centering
    \includegraphics[scale=0.34]{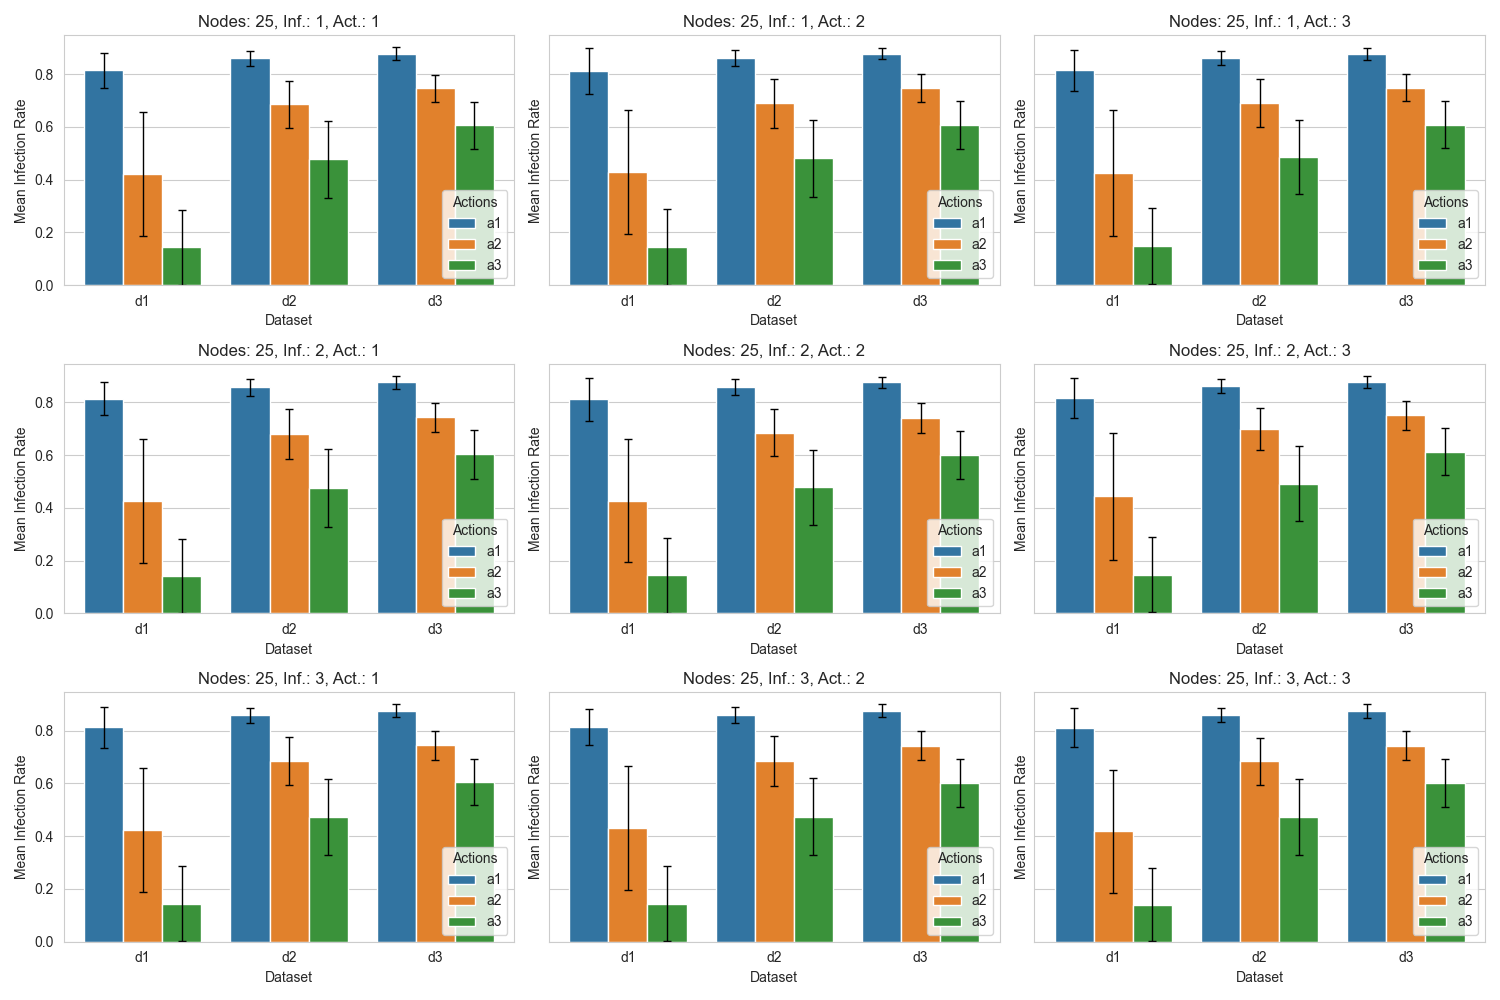}
    \caption{Case-1 using R2: Performance comparison of the RL policies trained using ResNet model for a 25-node network. The barplot displays the mean infection rate for datasets d1, d2, and d3 of Dataset v1 type, differentiated by the number of initial misinformation sources (Inf.) and action budgets (Act.: a1, a2, a3). Each subplot illustrates the performance of a policy trained with the parameters indicated in its title. Lower infection rates indicate more effective policy learning and misinformation containment.}
    \label{fig:inf_resnet_c1r2_25}
\end{figure}

\begin{figure}
    \centering
    \includegraphics[scale=0.34]{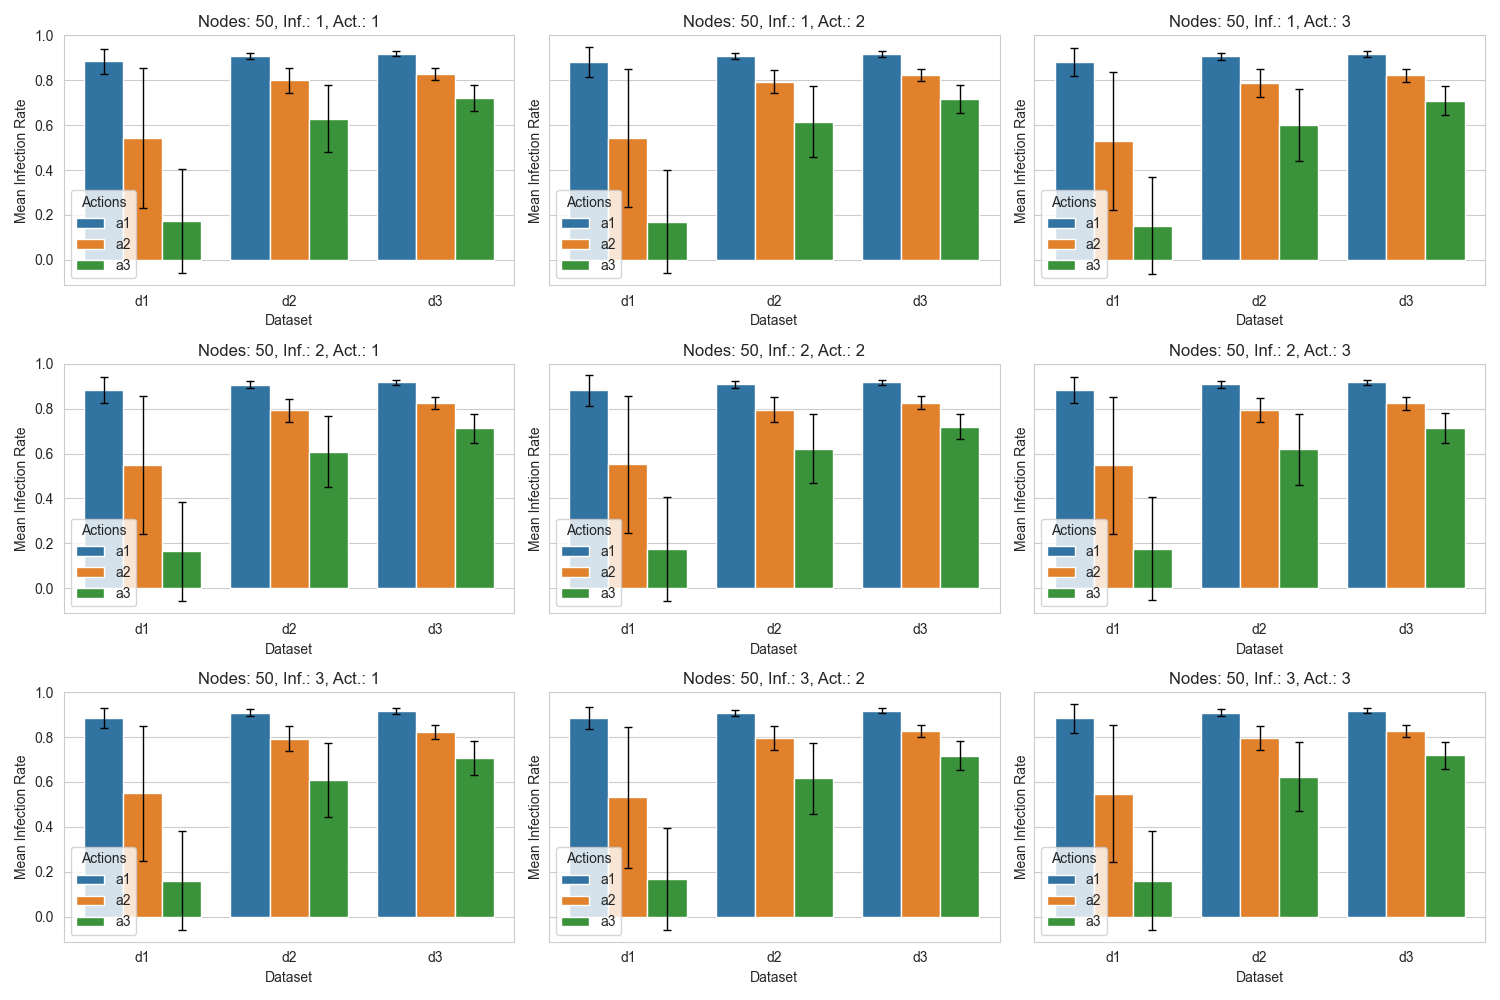}
    \caption{Case-1 using R2: Performance comparison of the RL policies trained using ResNet model for a 50-node network. The barplot displays the mean infection rate for datasets d1, d2, and d3 of Dataset v1 type, differentiated by the number of initial misinformation sources (Inf.) and action budgets (Act.: a1, a2, a3). Each subplot illustrates the performance of a policy trained with the parameters indicated in its title. Lower infection rates indicate more effective policy learning and misinformation containment.}
    \label{fig:inf_resnet_c1r2_50}
\end{figure}

%%%%%% R3 %%%%%%%%

\begin{figure}[!h]
    \centering
    \includegraphics[scale=0.34]{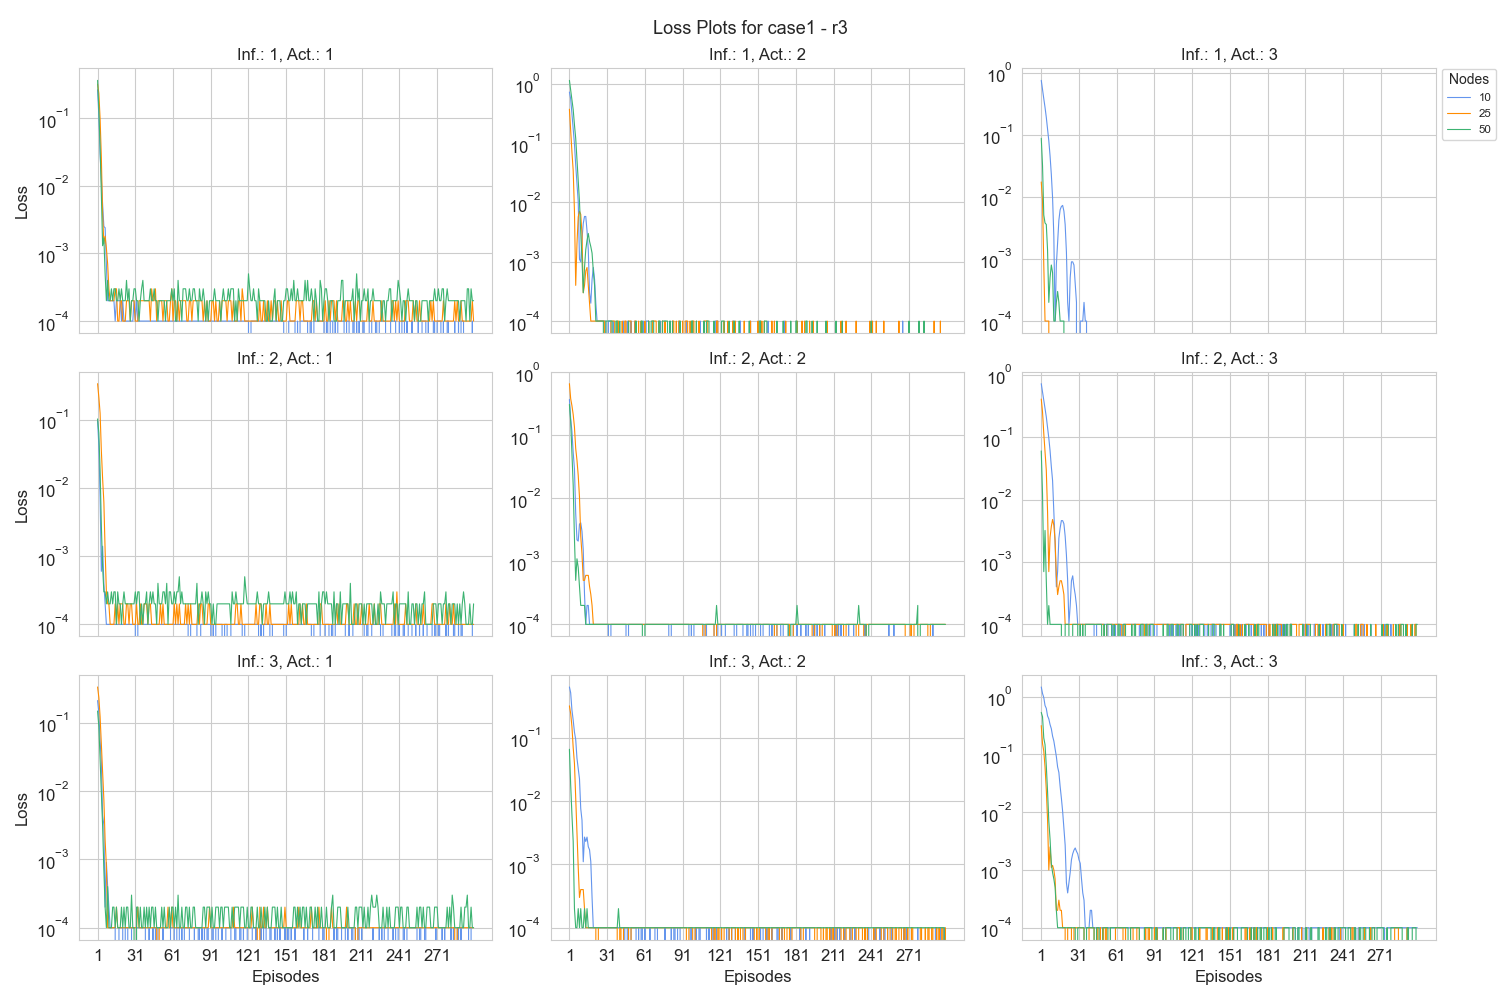}
    \caption{Case-1 using R3: Training MSE loss evolution for RL policy using ResNet model across networks of 10 (blue), 25 (orange), and 50 (green) nodes, for varying initial misinformation sources (Inf.) and action budgets (Act.). Plotted on a logarithmic scale, the loss decreases over episodes, indicating improved policy performance and adaptation across network sizes.}
    \label{fig:resnet_c1r3_loss}
\end{figure}

\begin{figure}
    \centering
    \includegraphics[scale=0.34]{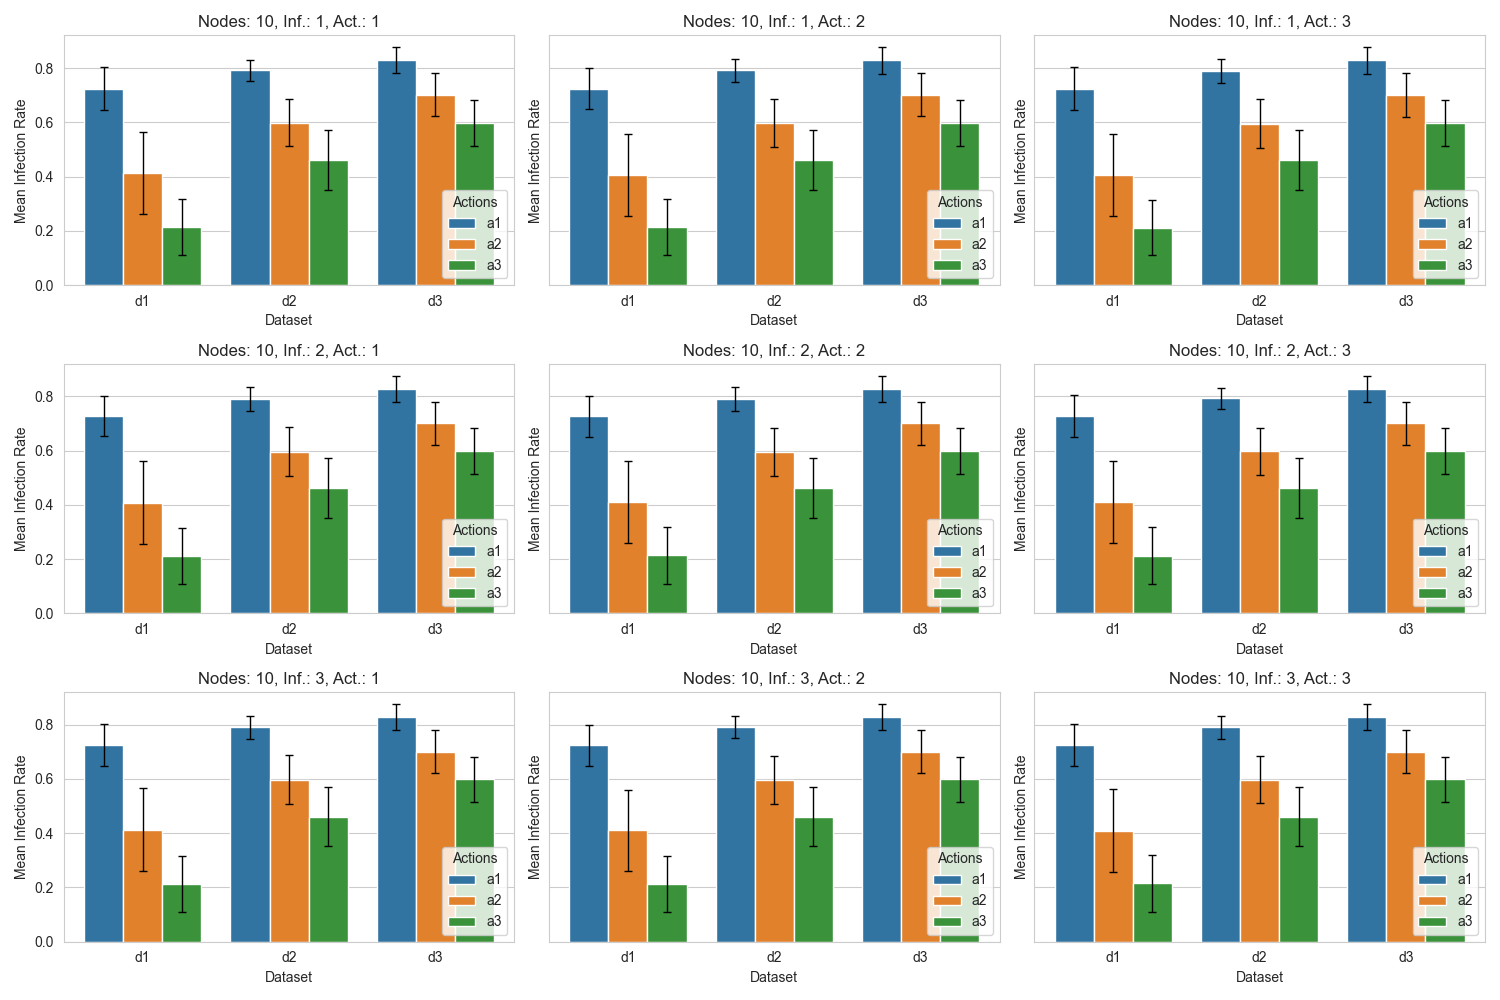}
    \caption{Case-1 using R3: Performance comparison of the RL policies trained using ResNet model for a 10-node network. The barplot displays the mean infection rate for datasets d1, d2, and d3 of Dataset v1 type, differentiated by the number of initial misinformation sources (Inf.) and action budgets (Act.: a1, a2, a3). Each subplot illustrates the performance of a policy trained with the parameters indicated in its title. Lower infection rates indicate more effective policy learning and misinformation containment.}
    \label{fig:inf_resnet_c1r3_10}
\end{figure}

\begin{figure}
    \centering
    \includegraphics[scale=0.34]{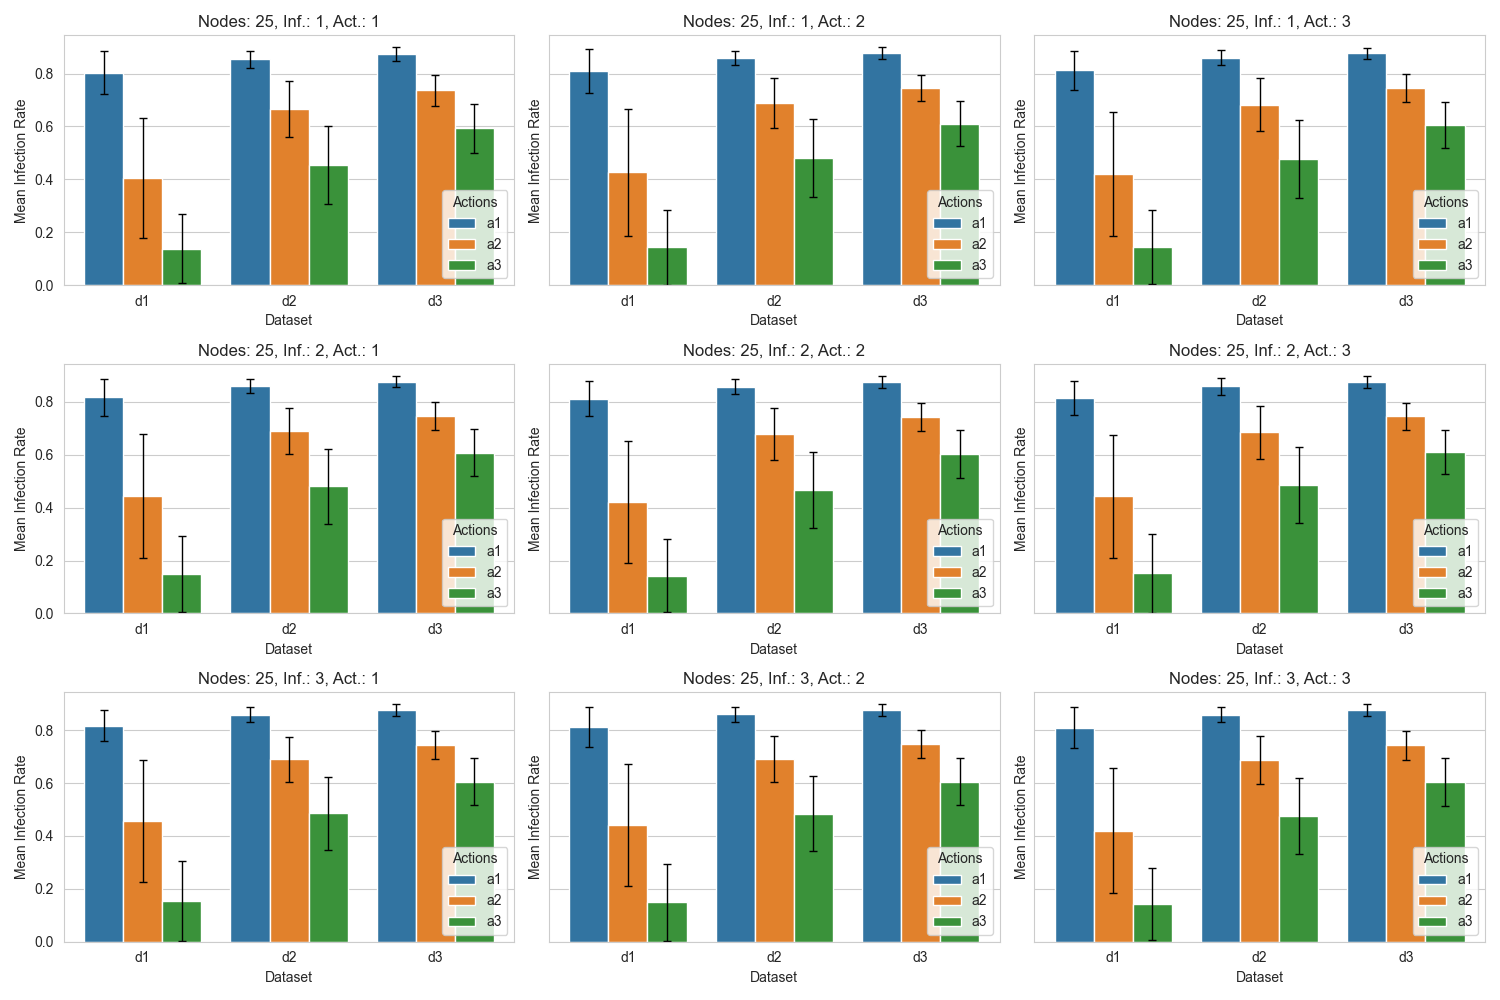}
    \caption{Case-1 using R3: Performance comparison of the RL policies trained using ResNet model for a 25-node network. The barplot displays the mean infection rate for datasets d1, d2, and d3 of Dataset v1 type, differentiated by the number of initial misinformation sources (Inf.) and action budgets (Act.: a1, a2, a3). Each subplot illustrates the performance of a policy trained with the parameters indicated in its title. Lower infection rates indicate more effective policy learning and misinformation containment.}
    \label{fig:inf_resnet_c1r3_25}
\end{figure}

\begin{figure}
    \centering
    \includegraphics[scale=0.34]{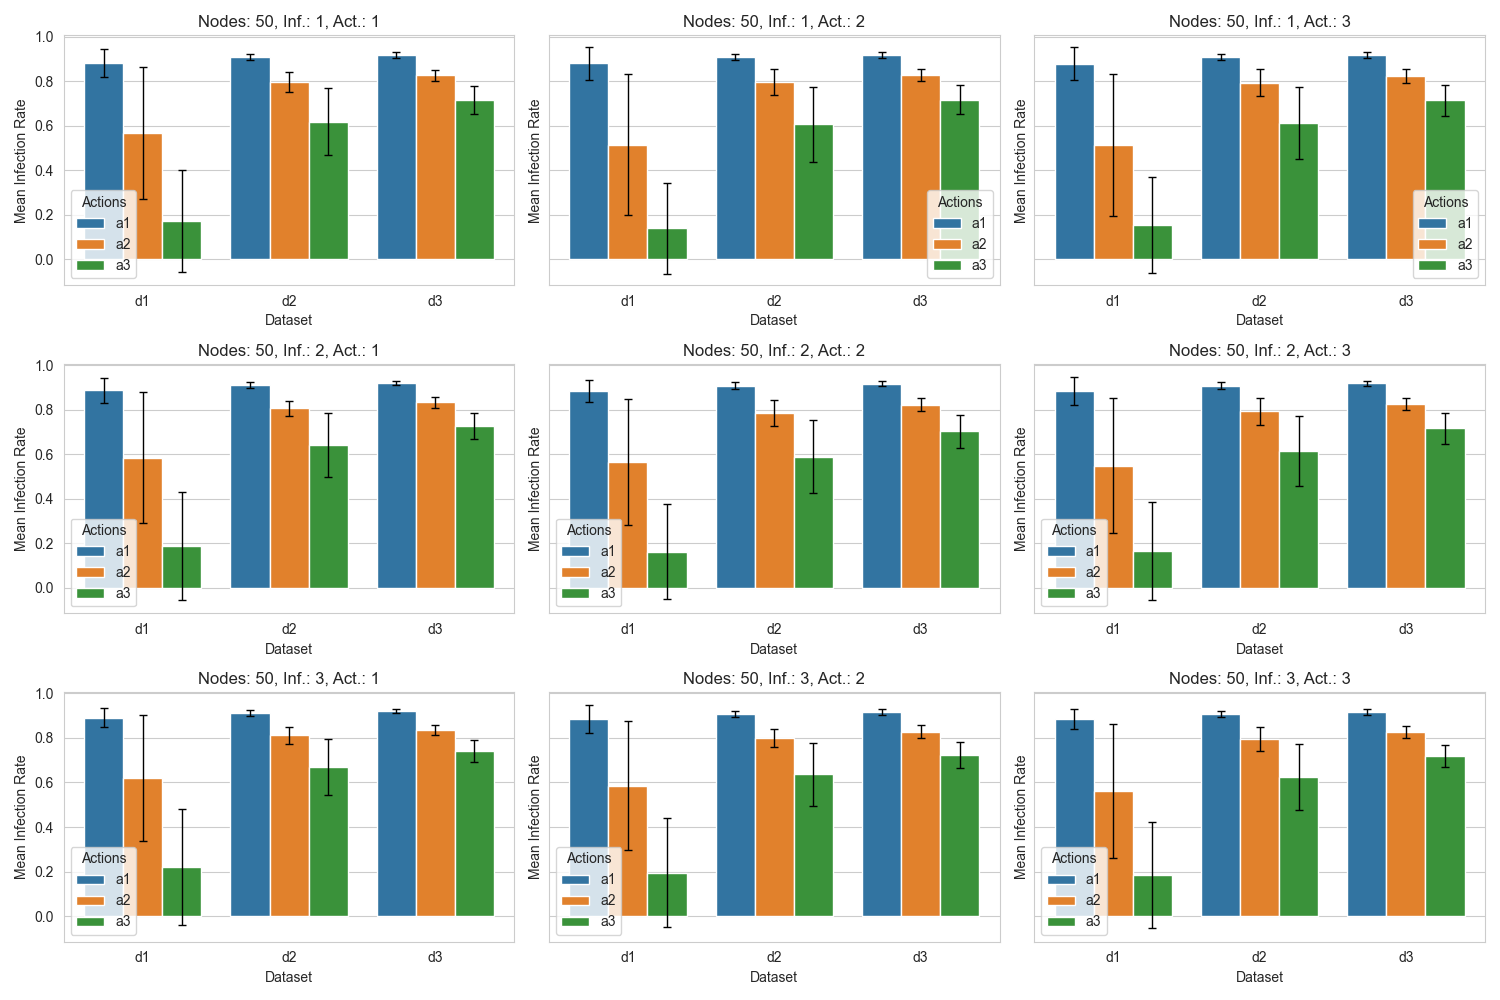}
    \caption{Case-1 using R3: Performance comparison of the RL policies trained using ResNet model for a 50-node network. The barplot displays the mean infection rate for datasets d1, d2, and d3 of Dataset v1 type, differentiated by the number of initial misinformation sources (Inf.) and action budgets (Act.: a1, a2, a3). Each subplot illustrates the performance of a policy trained with the parameters indicated in its title. Lower infection rates indicate more effective policy learning and misinformation containment.}
    \label{fig:inf_resnet_c1r3_50}
\end{figure}

%%%%%% R4 %%%%%%%%

\begin{figure}[!h]
    \centering
    \includegraphics[scale=0.34]{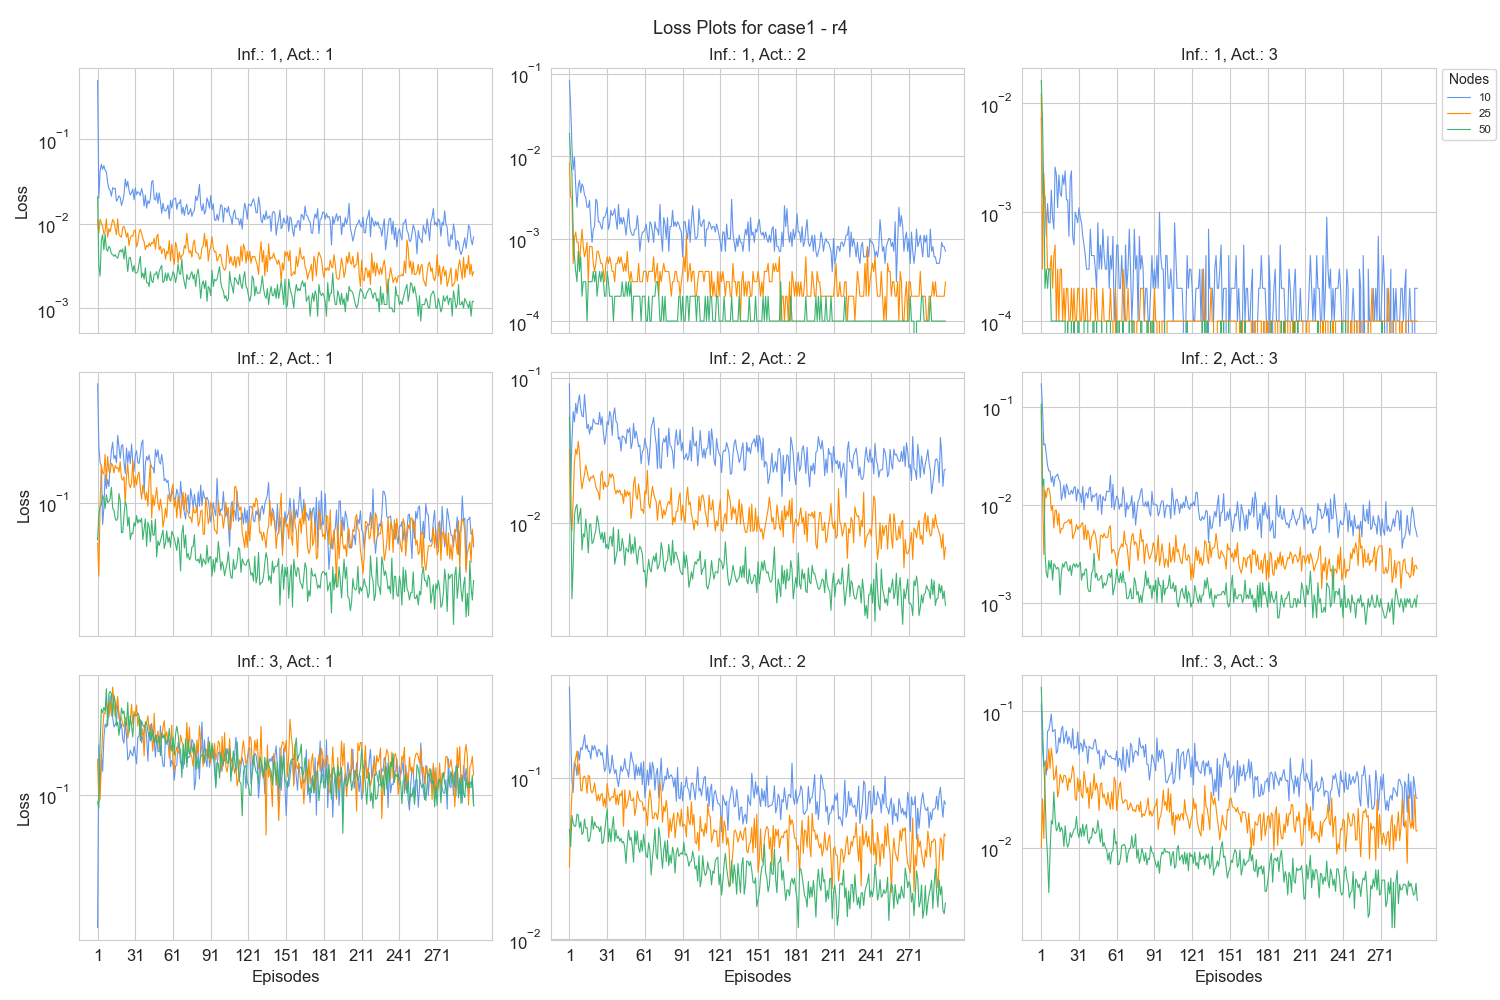}
    \caption{Case-1 using R4: Training MSE loss evolution for RL policy using ResNet model across networks of 10 (blue), 25 (orange), and 50 (green) nodes, for varying initial misinformation sources (Inf.) and action budgets (Act.). Plotted on a logarithmic scale, the loss decreases over episodes, indicating improved policy performance and adaptation across network sizes.}
    \label{fig:resnet_c1r4_loss}
\end{figure}

\begin{figure}
    \centering
    \includegraphics[scale=0.34]{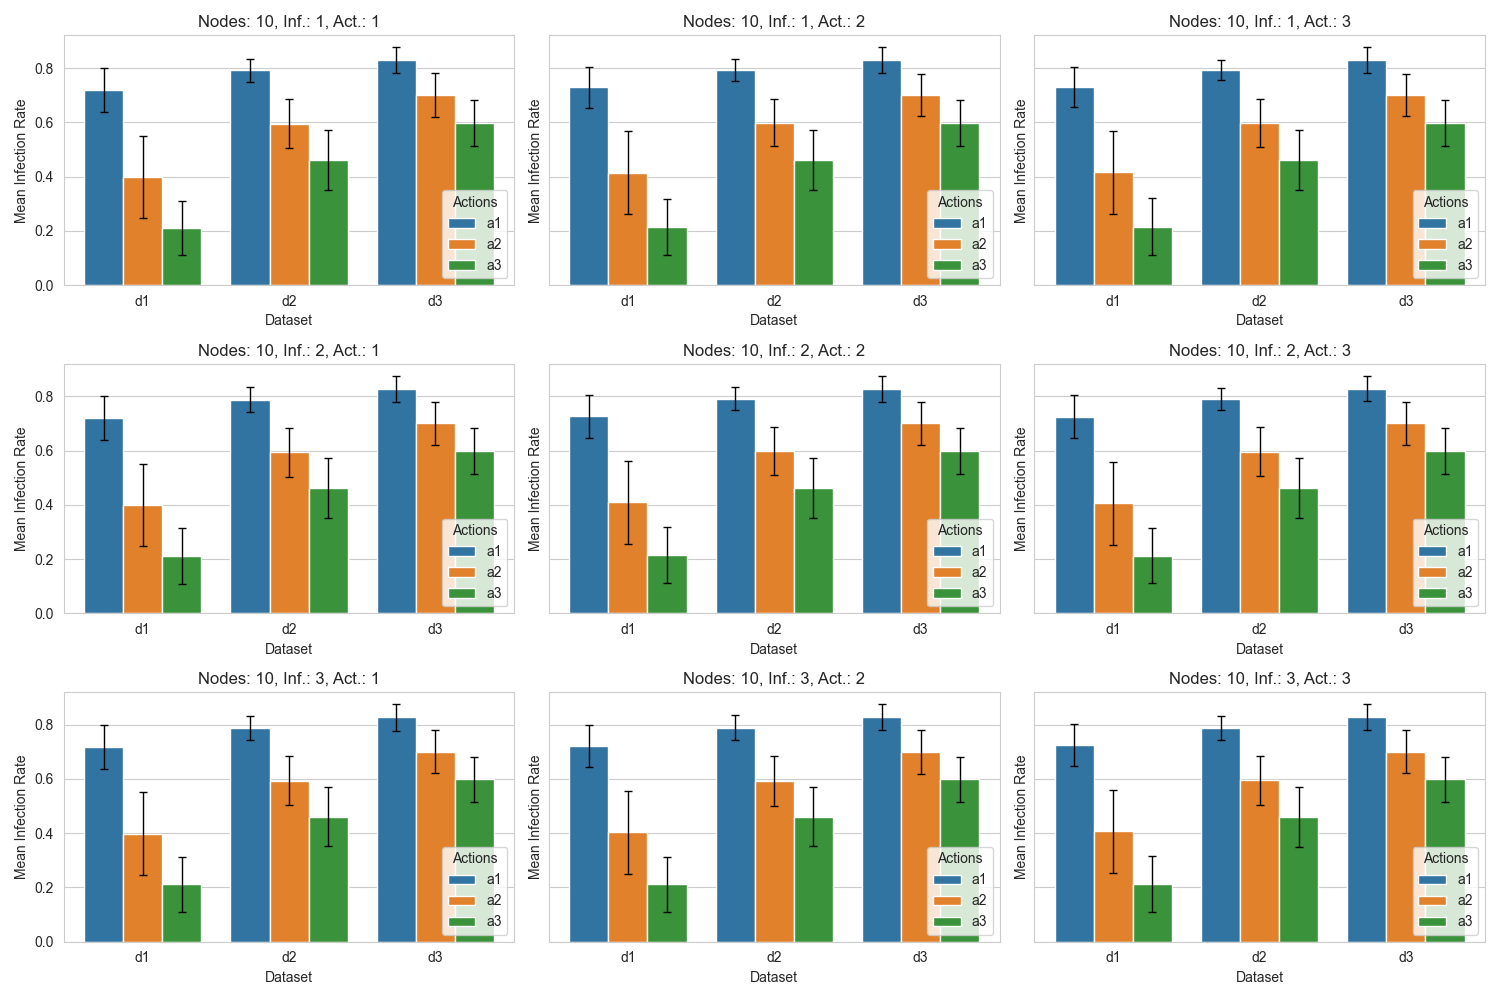}
    \caption{Case-1 using R4: Performance comparison of the RL policies trained using ResNet model for a 10-node network. The barplot displays the mean infection rate for datasets d1, d2, and d3 of Dataset v1 type, differentiated by the number of initial misinformation sources (Inf.) and action budgets (Act.: a1, a2, a3). Each subplot illustrates the performance of a policy trained with the parameters indicated in its title. Lower infection rates indicate more effective policy learning and misinformation containment.}
    \label{fig:inf_resnet_c1r4_10}
\end{figure}

\begin{figure}
    \centering
    \includegraphics[scale=0.34]{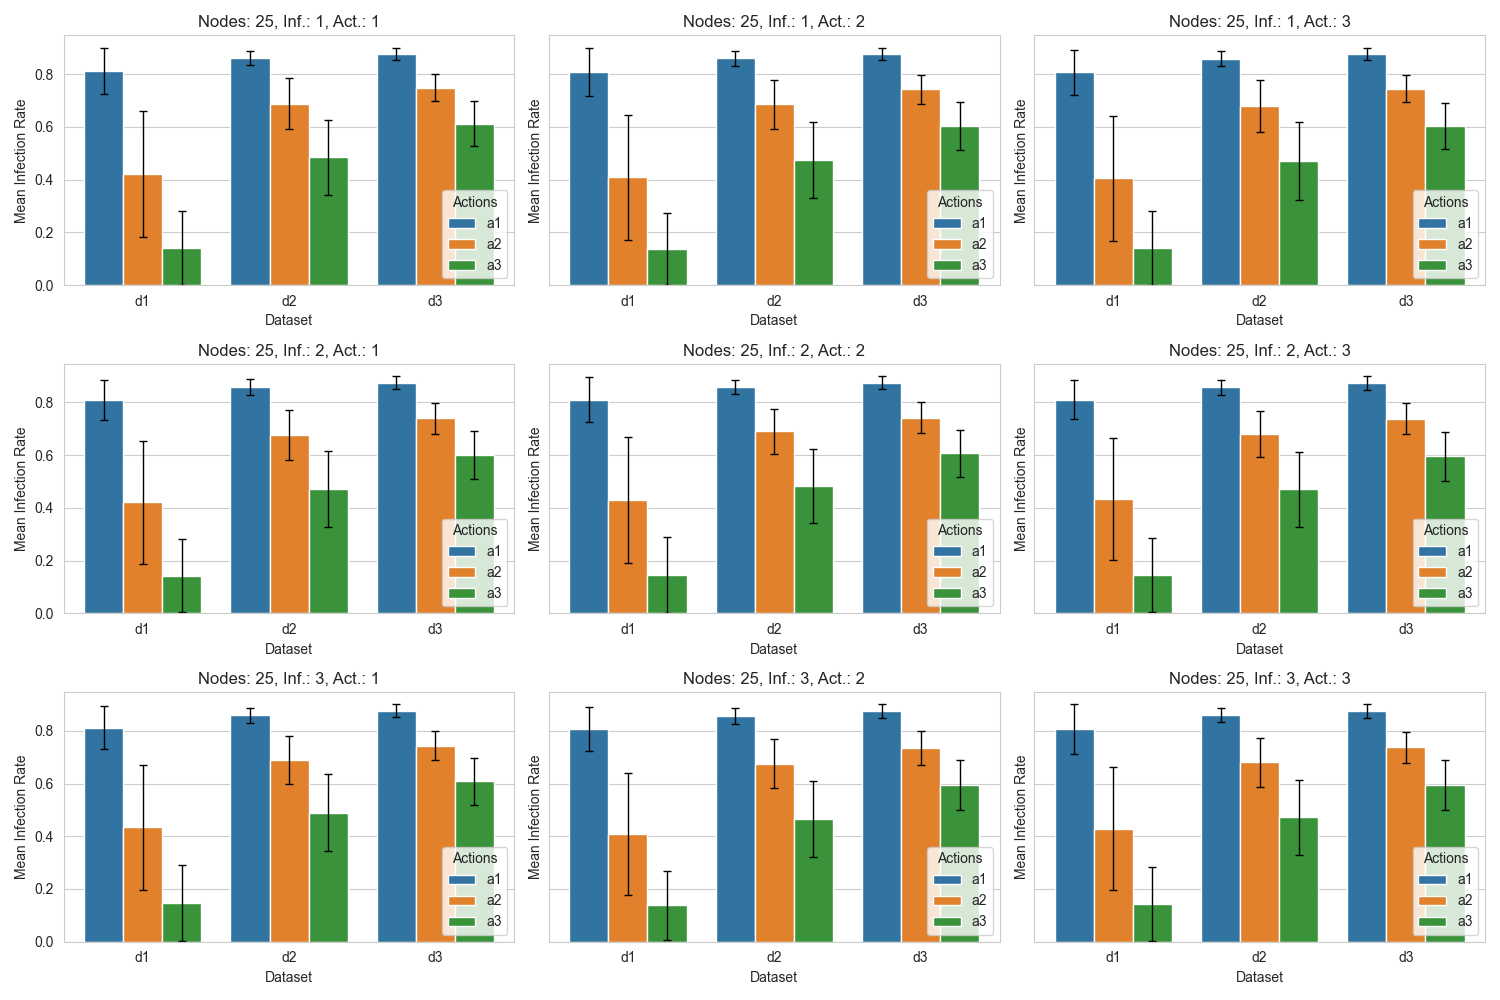}
    \caption{Case-1 using R4: Performance comparison of the RL policies trained using ResNet model for a 25-node network. The barplot displays the mean infection rate for datasets d1, d2, and d3 of Dataset v1 type, differentiated by the number of initial misinformation sources (Inf.) and action budgets (Act.: a1, a2, a3). Each subplot illustrates the performance of a policy trained with the parameters indicated in its title. Lower infection rates indicate more effective policy learning and misinformation containment.}
    \label{fig:inf_resnet_c1r4_25}
\end{figure}

\begin{figure}
    \centering
    \includegraphics[scale=0.34]{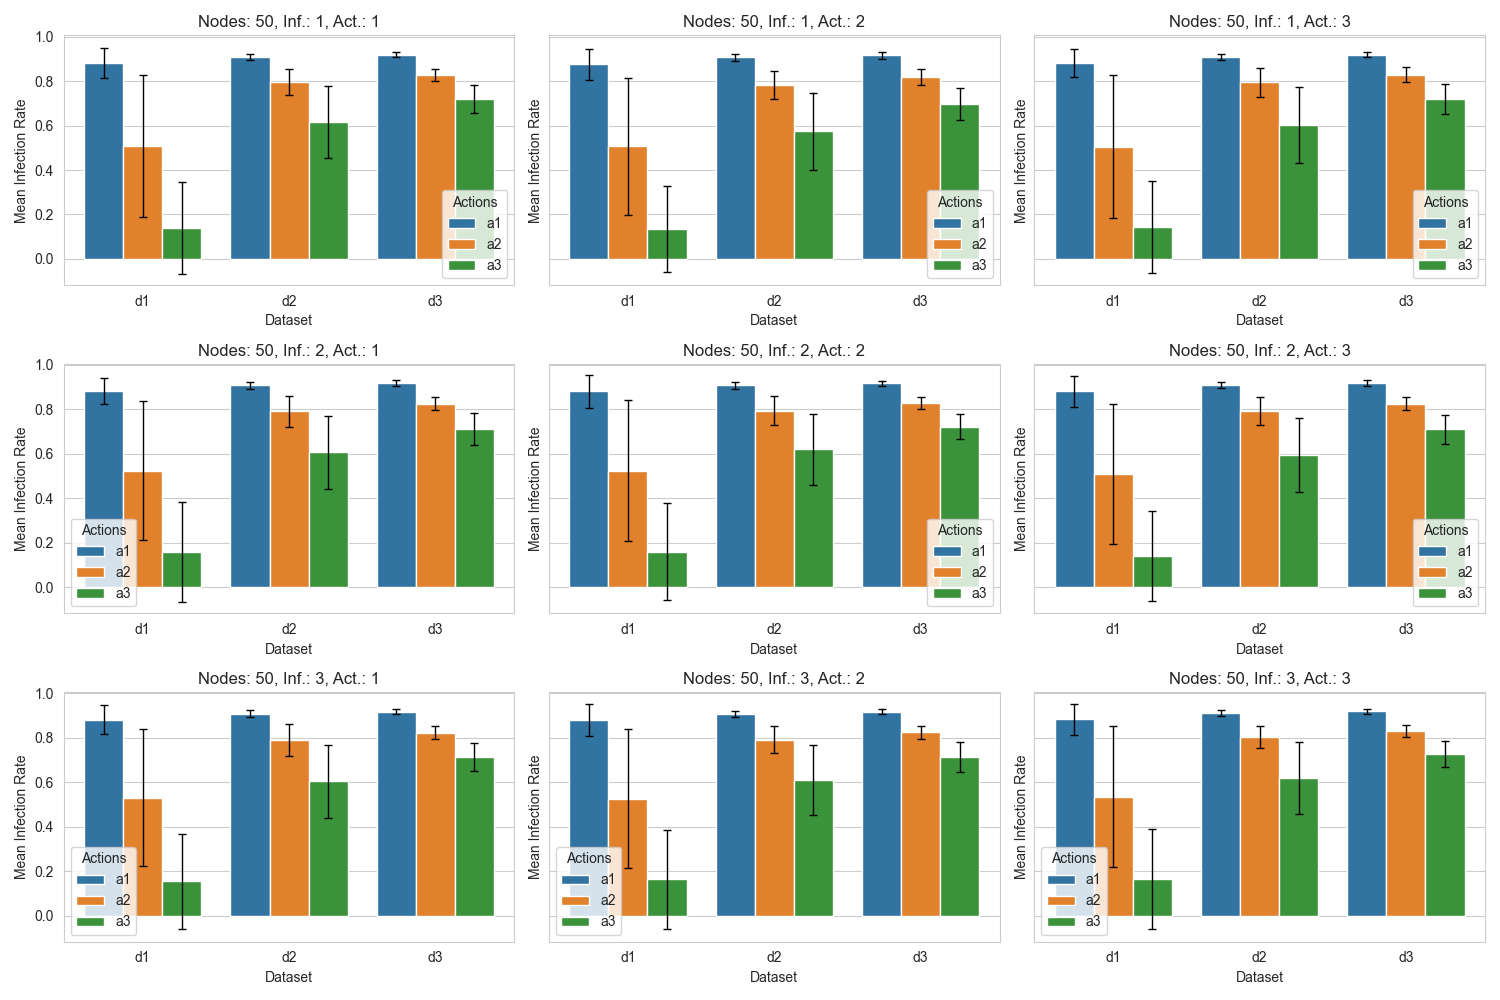}
    \caption{Case-1 using R4: Performance comparison of the RL policies trained using ResNet model for a 50-node network. The barplot displays the mean infection rate for datasets d1, d2, and d3 of Dataset v1 type, differentiated by the number of initial misinformation sources (Inf.) and action budgets (Act.: a1, a2, a3). Each subplot illustrates the performance of a policy trained with the parameters indicated in its title. Lower infection rates indicate more effective policy learning and misinformation containment.}
    \label{fig:inf_resnet_c1r4_50}
\end{figure}

% --------------------Inference------------------------

%###########################

%###### Case 2 ResNet Figures #######

%%%%%% R0 %%%%%%%%
\begin{figure}[!h]
    \centering
    \includegraphics[scale=0.34]{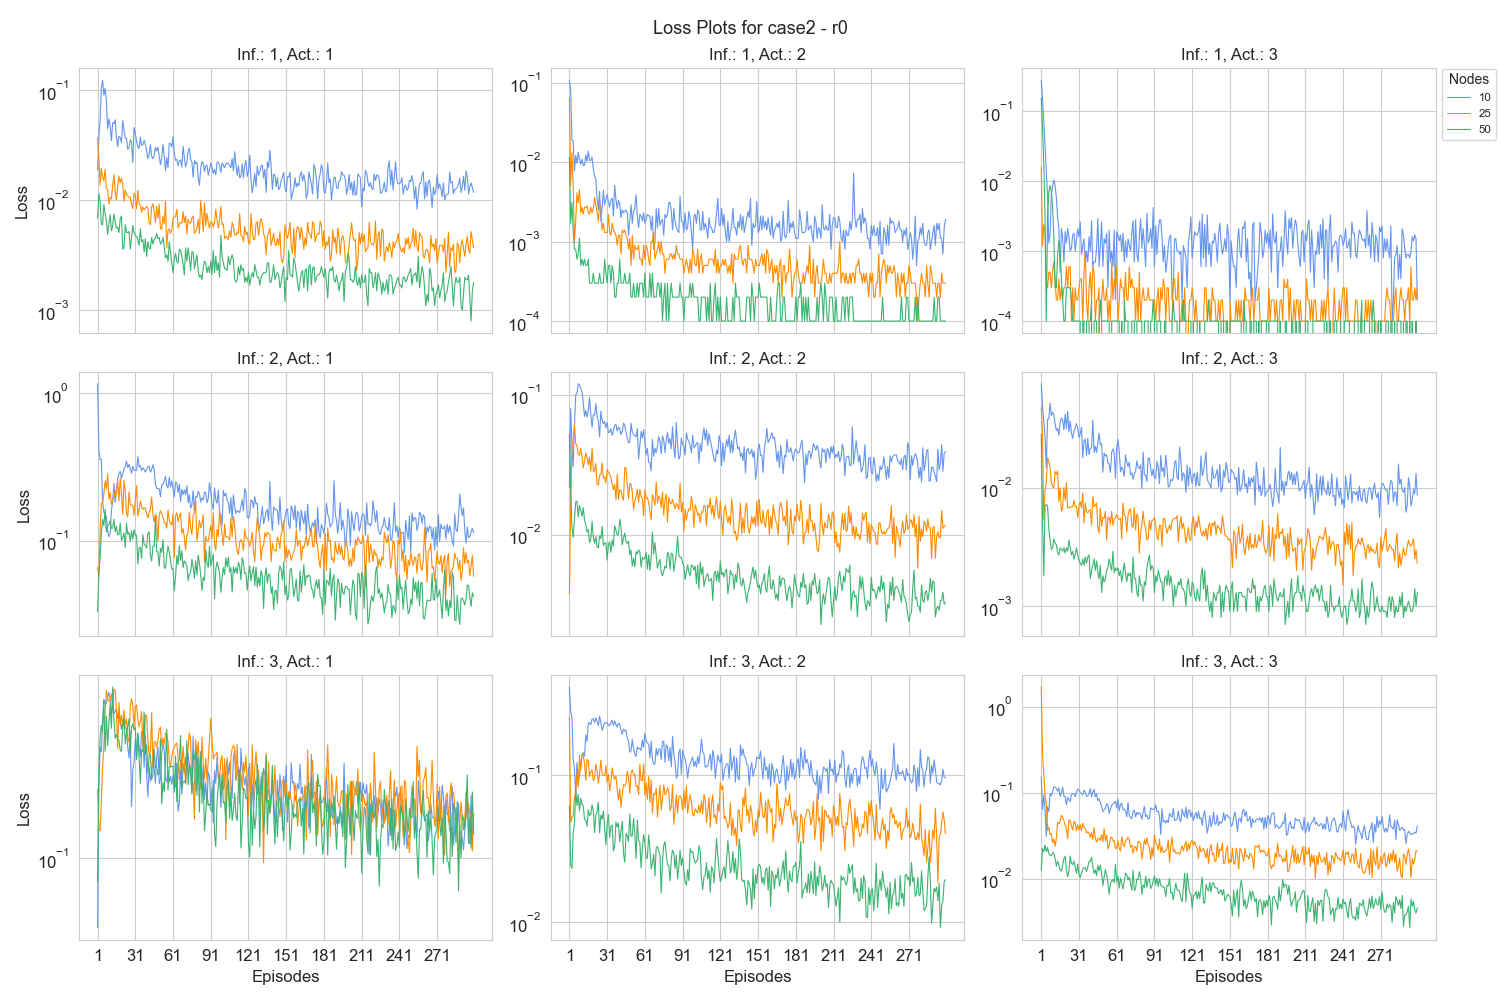}
    \caption{Case-2 using R0: Training MSE loss evolution for RL policy using ResNet model across networks of 10 (blue), 25 (orange), and 50 (green) nodes, for varying initial misinformation sources (Inf.) and action budgets (Act.). Plotted on a logarithmic scale, the loss decreases over episodes, indicating improved policy performance and adaptation across network sizes.}
    \label{fig:resnet_c2r0_loss}
\end{figure}

\begin{figure}
    \centering
    \includegraphics[scale=0.34]{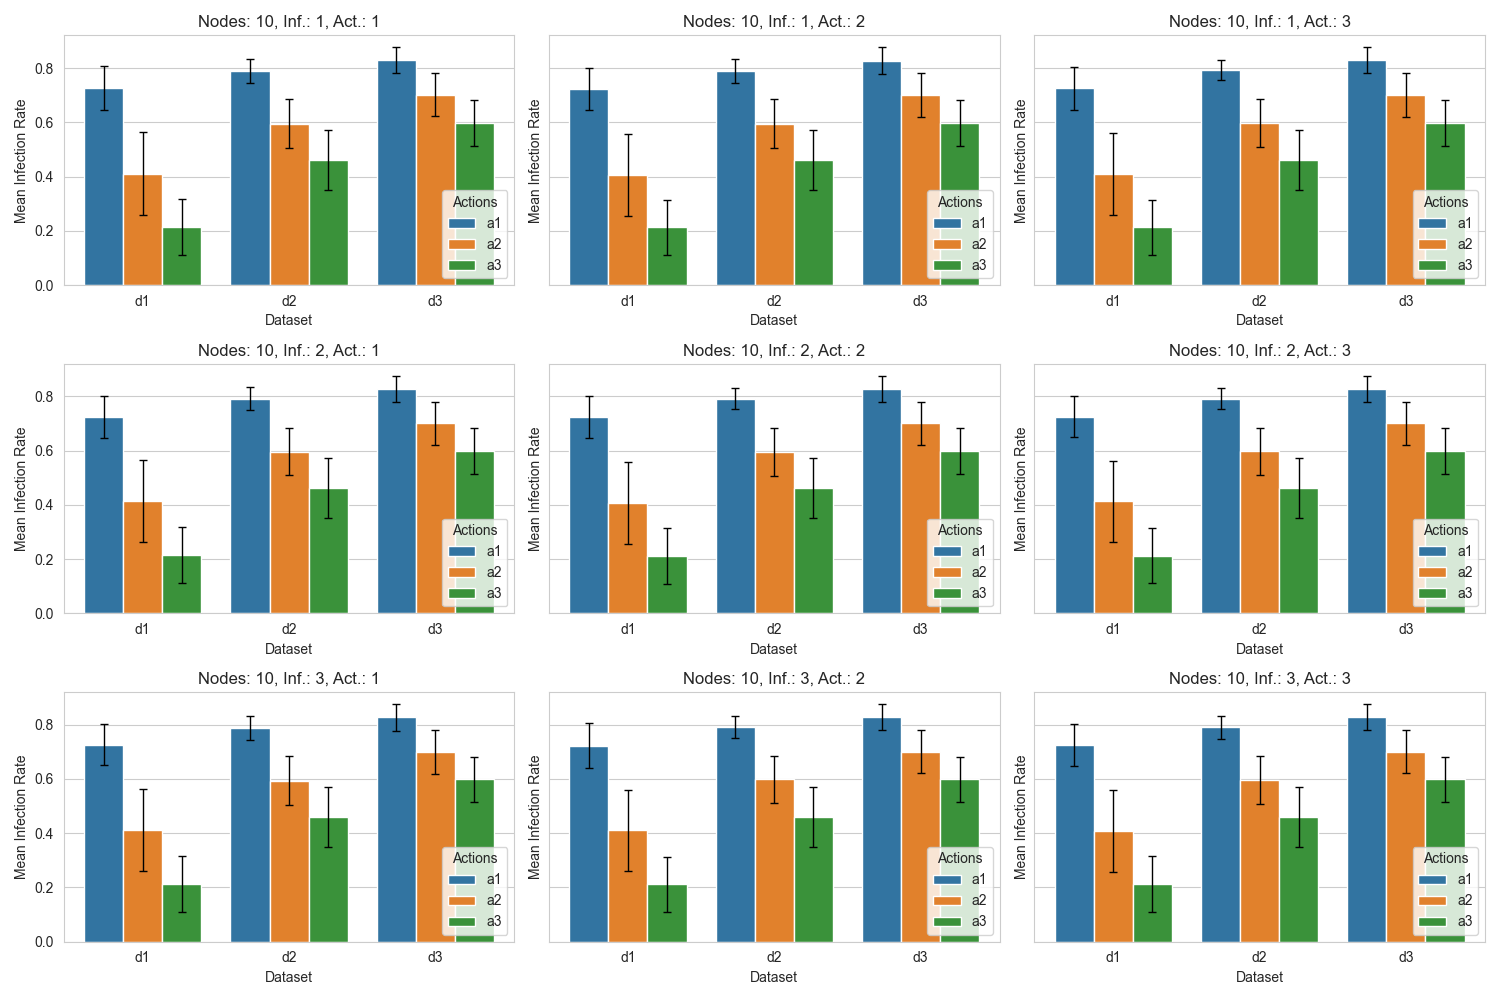}
    \caption{Case-2 using R0: Performance comparison of the RL policies trained using ResNet model for a 10-node network. The barplot displays the mean infection rate for datasets d1, d2, and d3 of Dataset v1 type, differentiated by the number of initial misinformation sources (Inf.) and action budgets (Act.: a1, a2, a3). Each subplot illustrates the performance of a policy trained with the parameters indicated in its title. Lower infection rates indicate more effective policy learning and misinformation containment.}
    \label{fig:inf_resnet_c2r0_10}
\end{figure}

\begin{figure}
    \centering
    \includegraphics[scale=0.34]{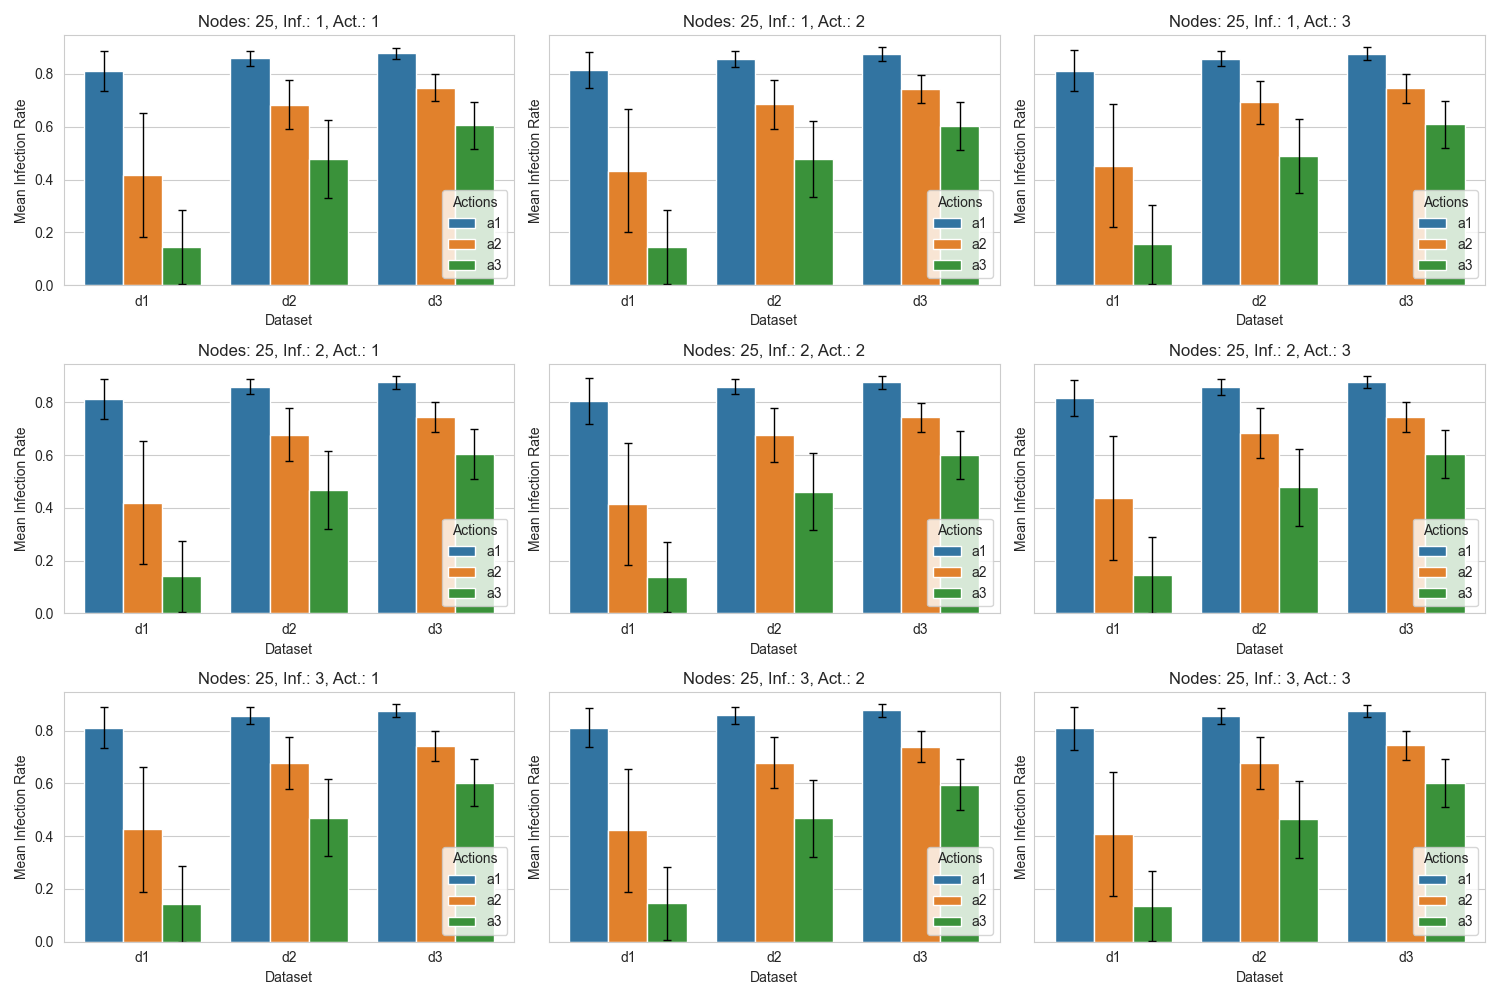}
    \caption{Case-2 using R0: Performance comparison of the RL policies trained using ResNet model for a 25-node network. The barplot displays the mean infection rate for datasets d1, d2, and d3 of Dataset v1 type, differentiated by the number of initial misinformation sources (Inf.) and action budgets (Act.: a1, a2, a3). Each subplot illustrates the performance of a policy trained with the parameters indicated in its title. Lower infection rates indicate more effective policy learning and misinformation containment.}
    \label{fig:inf_resnet_c2r0_25}
\end{figure}

\begin{figure}
    \centering
    \includegraphics[scale=0.34]{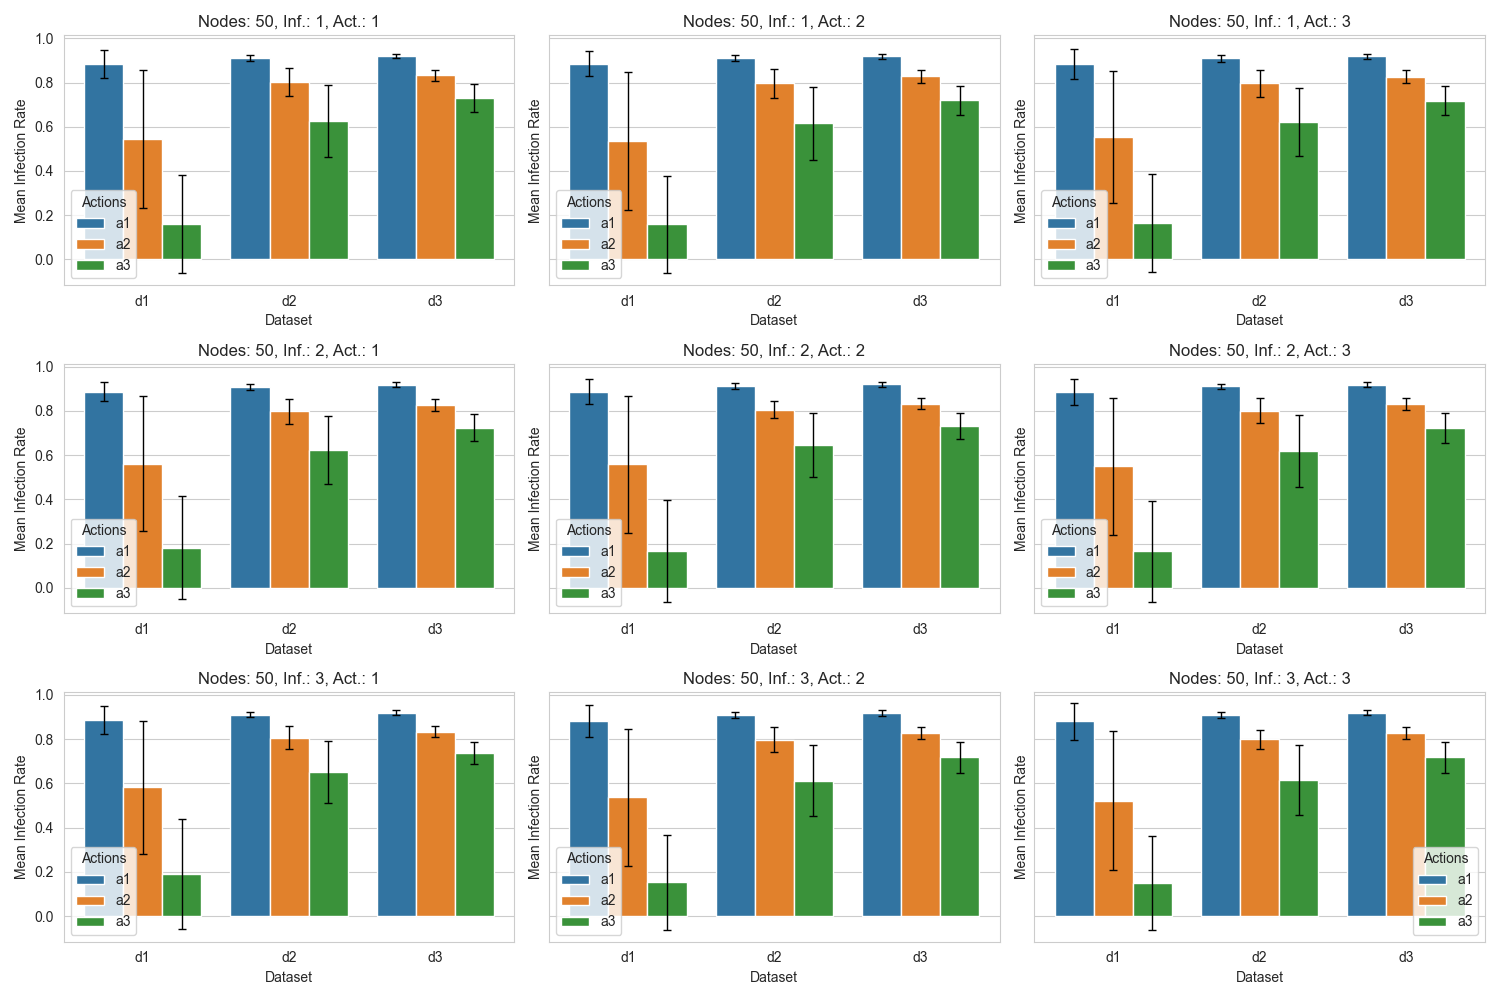}
    \caption{Case-2 using R0: Performance comparison of the RL policies trained using ResNet model for a 50-node network. The barplot displays the mean infection rate for datasets d1, d2, and d3 of Dataset v1 type, differentiated by the number of initial misinformation sources (Inf.) and action budgets (Act.: a1, a2, a3). Each subplot illustrates the performance of a policy trained with the parameters indicated in its title. Lower infection rates indicate more effective policy learning and misinformation containment.}
    \label{fig:inf_resnet_c2r0_50}
\end{figure}

%%%%%% R1 %%%%%%%%
\begin{figure}[!h]
    \centering
    \includegraphics[scale=0.34]{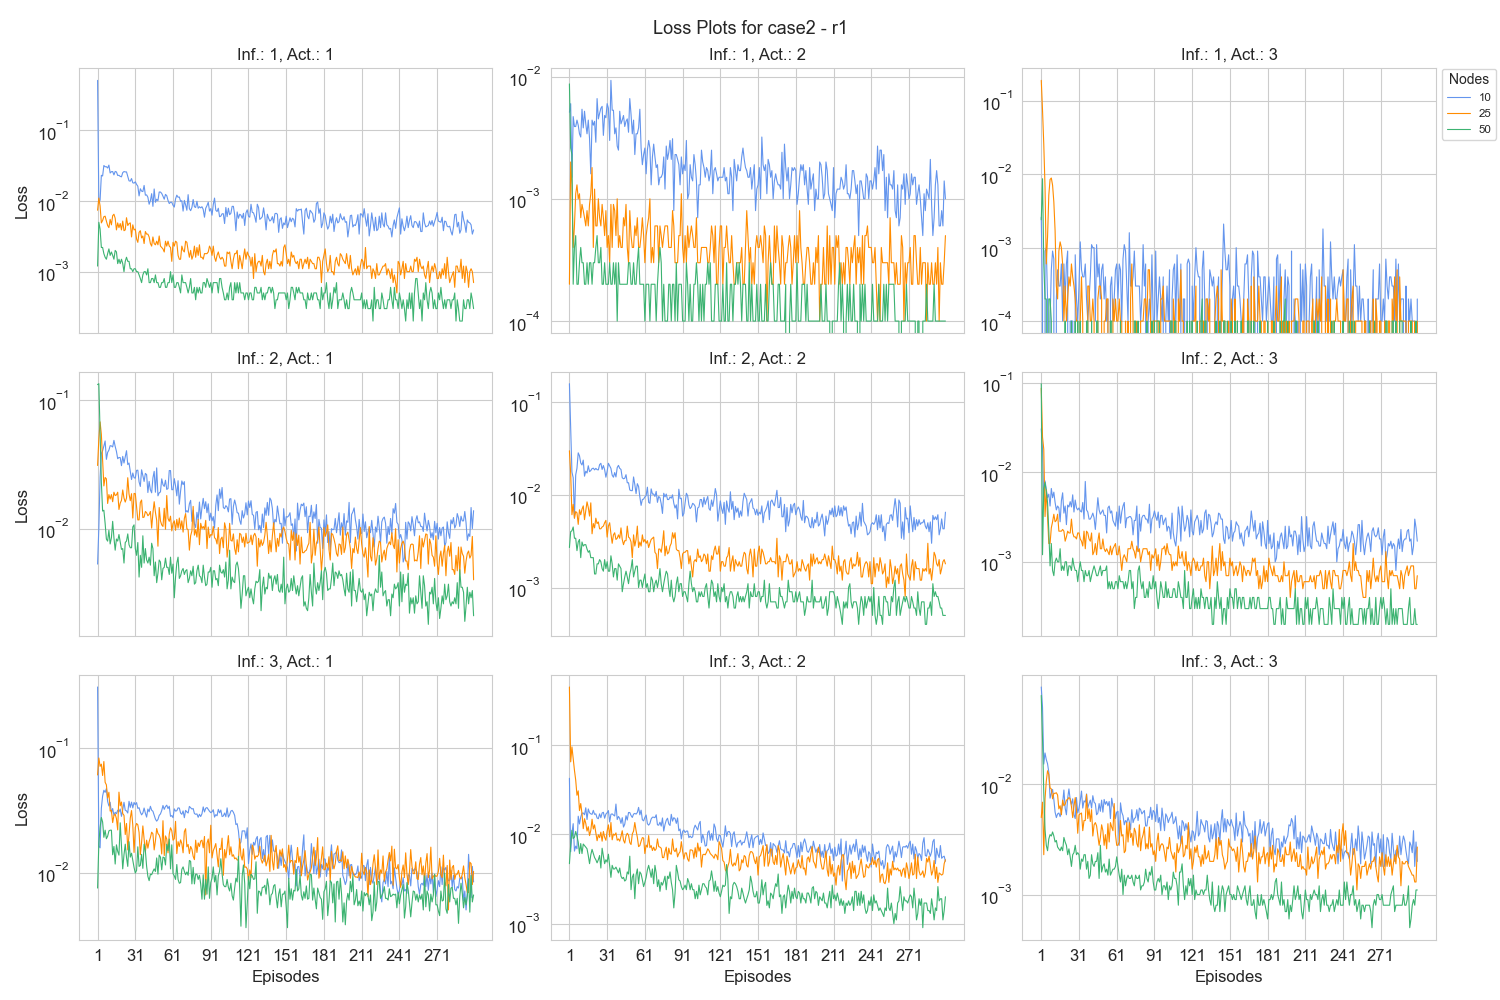}
    \caption{Case-2 using R1: Training MSE loss evolution for RL policy using ResNet model across networks of 10 (blue), 25 (orange), and 50 (green) nodes, for varying initial misinformation sources (Inf.) and action budgets (Act.). Plotted on a logarithmic scale, the loss decreases over episodes, indicating improved policy performance and adaptation across network sizes.}
    \label{fig:resnet_c2r1_loss}
\end{figure}

\begin{figure}
    \centering
    \includegraphics[scale=0.34]{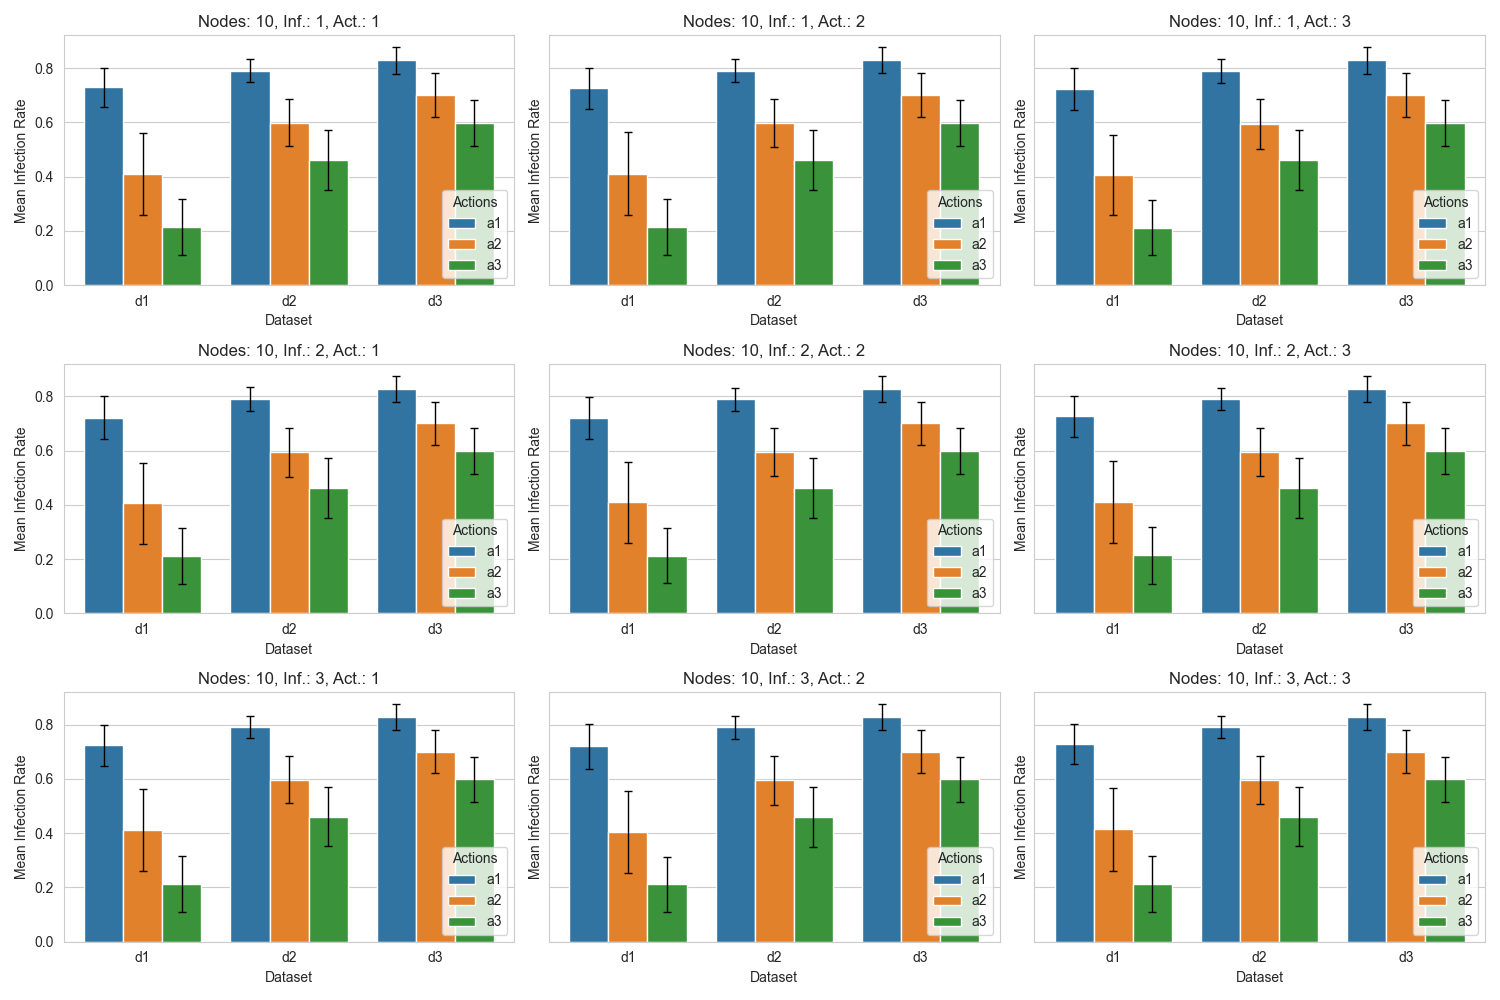}
    \caption{Case-2 using R1: Performance comparison of the RL policies trained using ResNet model for a 10-node network. The barplot displays the mean infection rate for datasets d1, d2, and d3 of Dataset v1 type, differentiated by the number of initial misinformation sources (Inf.) and action budgets (Act.: a1, a2, a3). Each subplot illustrates the performance of a policy trained with the parameters indicated in its title. Lower infection rates indicate more effective policy learning and misinformation containment.}
    \label{fig:inf_resnet_c2r1_10}
\end{figure}

\begin{figure}
    \centering
    \includegraphics[scale=0.34]{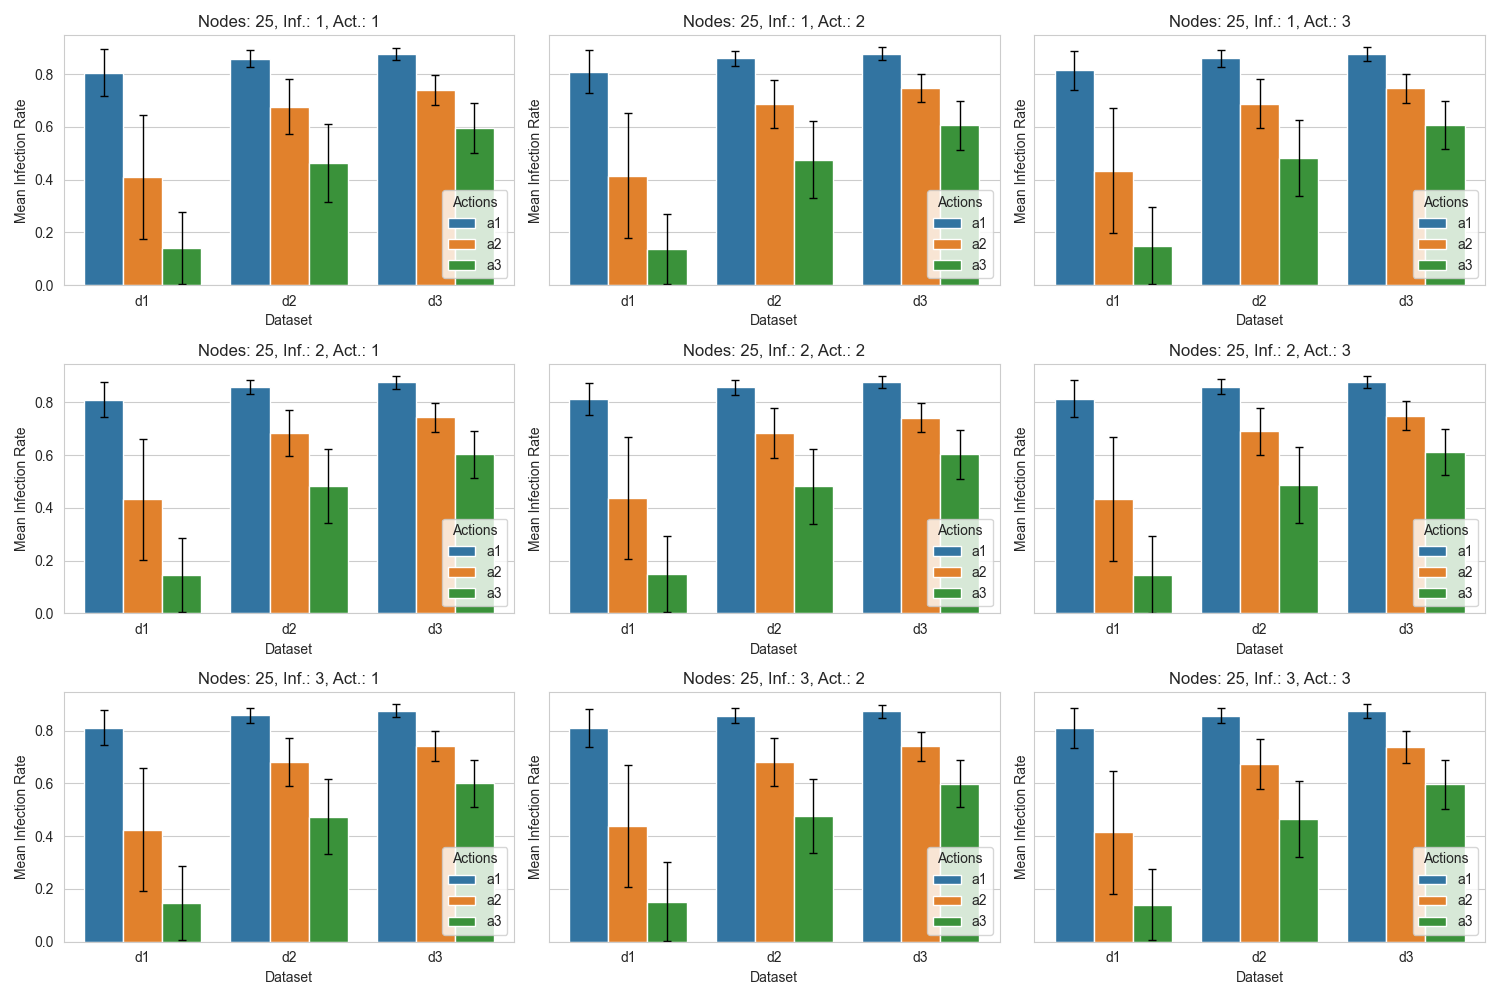}
    \caption{Case-2 using R1: Performance comparison of the RL policies trained using ResNet model for a 25-node network. The barplot displays the mean infection rate for datasets d1, d2, and d3 of Dataset v1 type, differentiated by the number of initial misinformation sources (Inf.) and action budgets (Act.: a1, a2, a3). Each subplot illustrates the performance of a policy trained with the parameters indicated in its title. Lower infection rates indicate more effective policy learning and misinformation containment.}
    \label{fig:inf_resnet_c2r1_25}
\end{figure}

\begin{figure}
    \centering
    \includegraphics[scale=0.34]{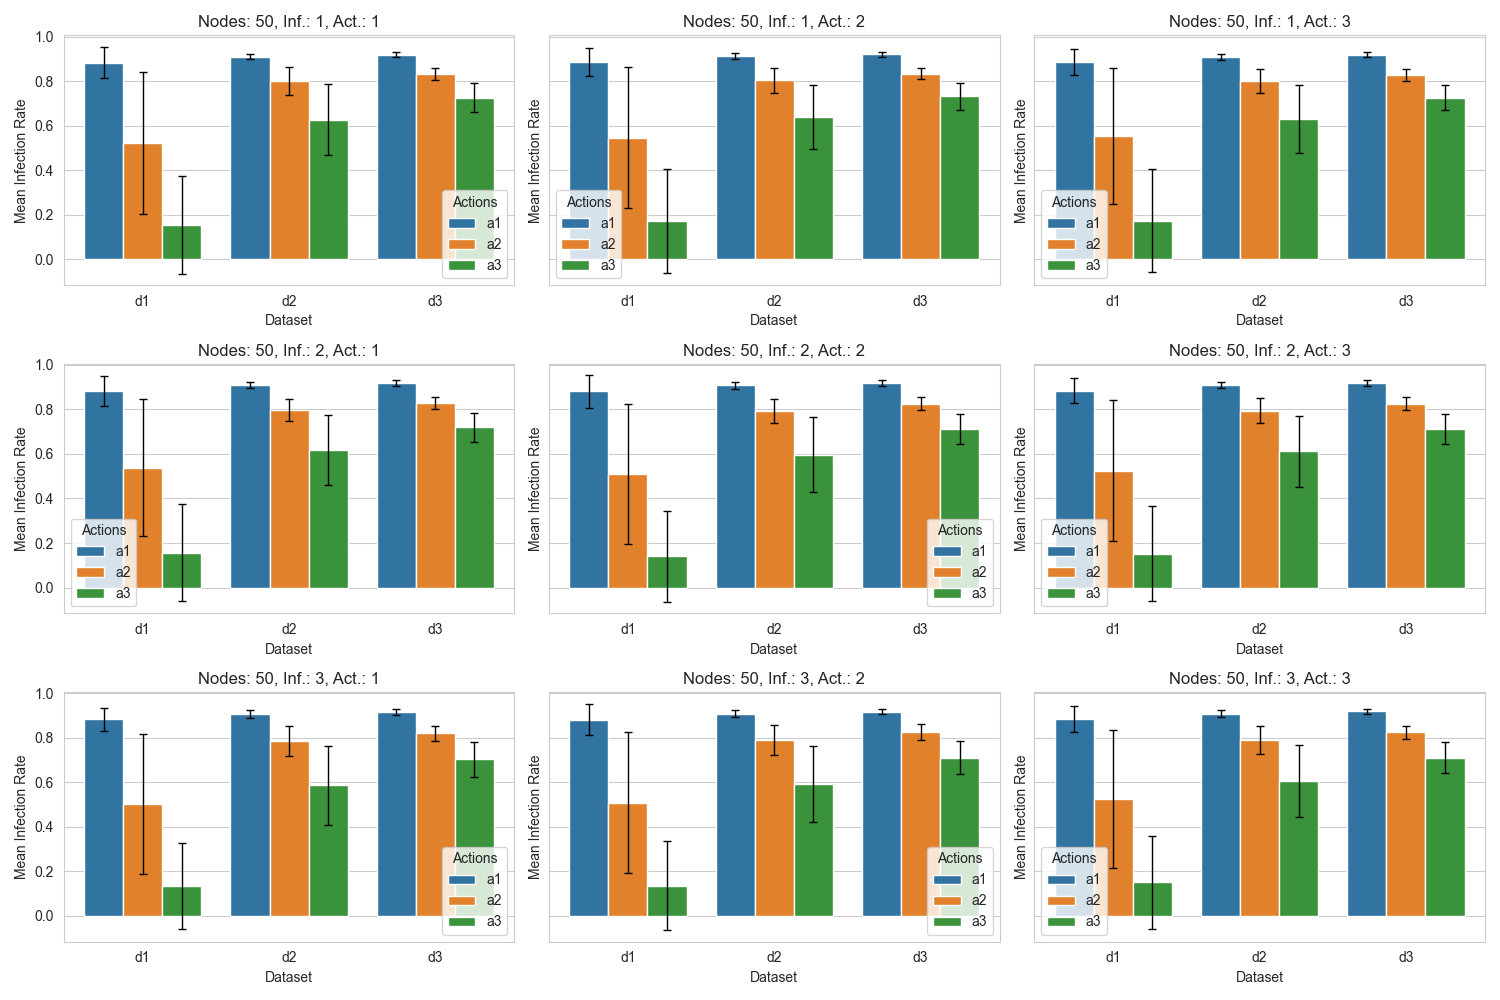}
    \caption{Case-2 using R1: Performance comparison of the RL policies trained using ResNet model for a 50-node network. The barplot displays the mean infection rate for datasets d1, d2, and d3 of Dataset v1 type, differentiated by the number of initial misinformation sources (Inf.) and action budgets (Act.: a1, a2, a3). Each subplot illustrates the performance of a policy trained with the parameters indicated in its title. Lower infection rates indicate more effective policy learning and misinformation containment.}
    \label{fig:inf_resnet_c2r1_50}
\end{figure}

%%%%%% R2 %%%%%%%%
\begin{figure}[!h]
    \centering
    \includegraphics[scale=0.34]{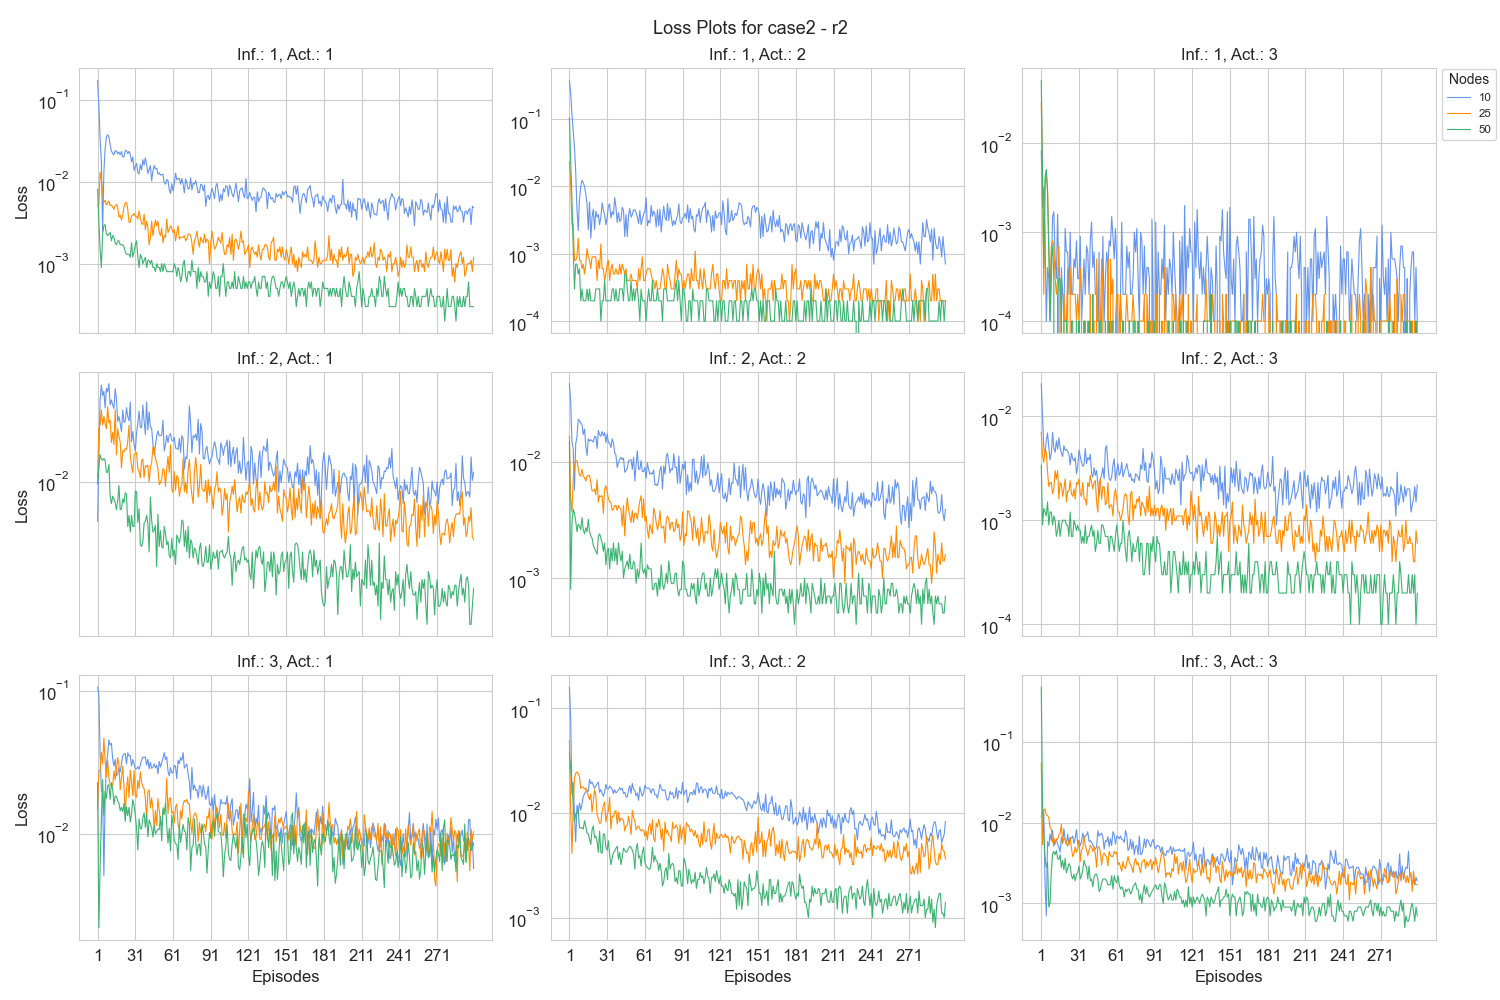}
    \caption{Case-2 using R2: Training MSE loss evolution for RL policy using ResNet model across networks of 10 (blue), 25 (orange), and 50 (green) nodes, for varying initial misinformation sources (Inf.) and action budgets (Act.). Plotted on a logarithmic scale, the loss decreases over episodes, indicating improved policy performance and adaptation across network sizes.}
    \label{fig:resnet_c2r2_loss}
\end{figure}

\begin{figure}
    \centering
    \includegraphics[scale=0.34]{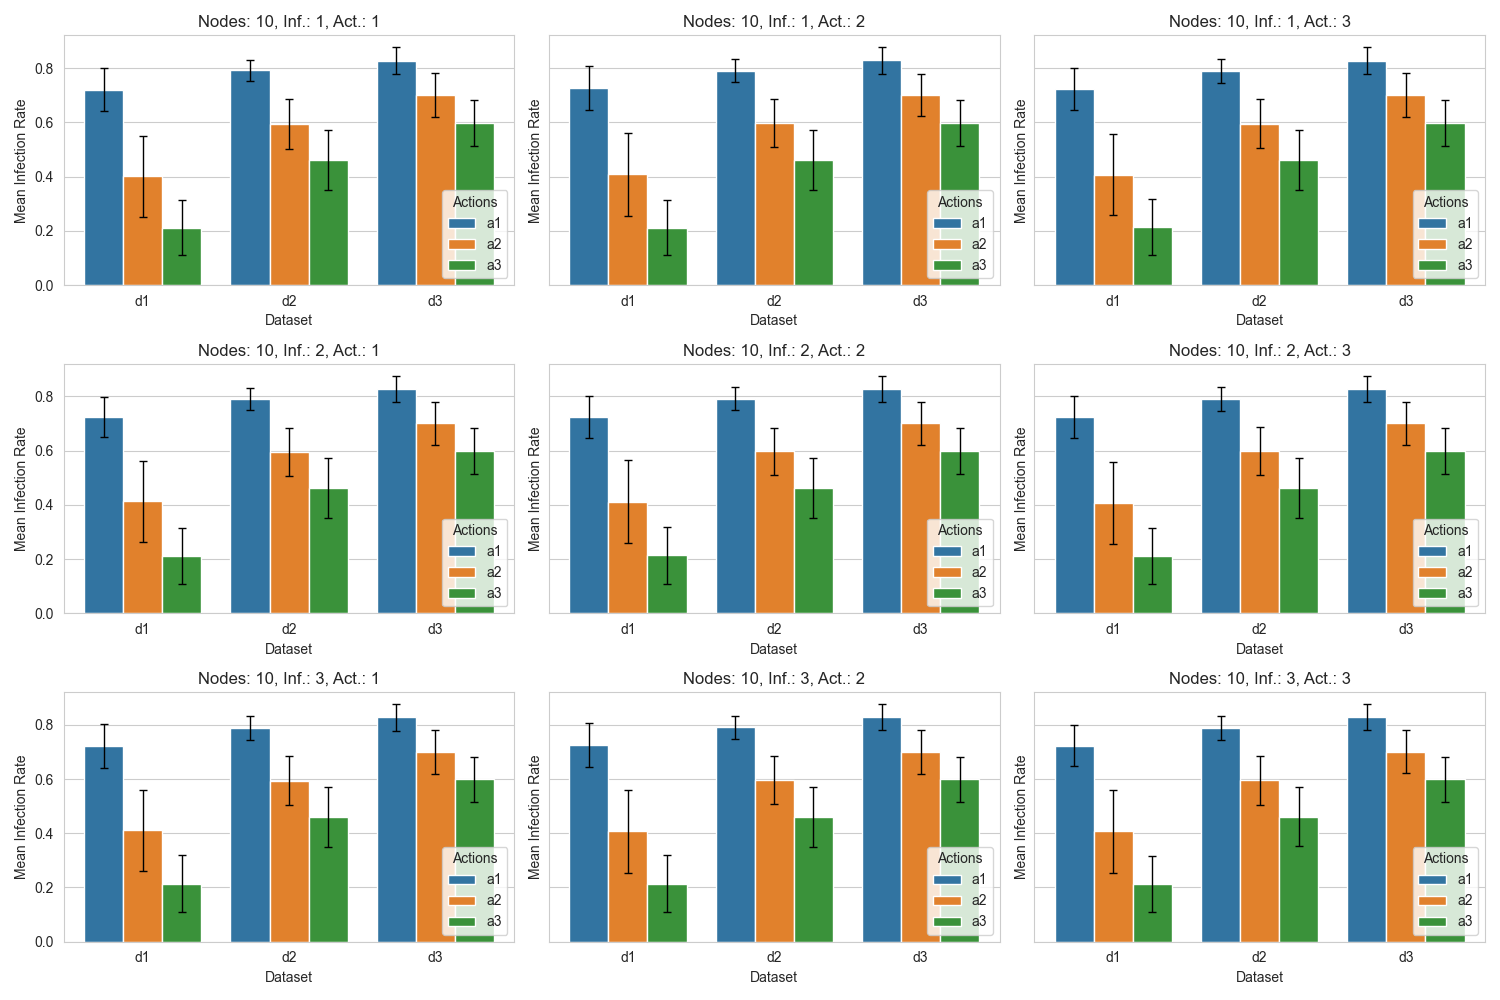}
    \caption{Case-2 using R2: Performance comparison of the RL policies trained using ResNet model for a 10-node network. The barplot displays the mean infection rate for datasets d1, d2, and d3 of Dataset v1 type, differentiated by the number of initial misinformation sources (Inf.) and action budgets (Act.: a1, a2, a3). Each subplot illustrates the performance of a policy trained with the parameters indicated in its title. Lower infection rates indicate more effective policy learning and misinformation containment.}
    \label{fig:inf_resnet_c2r2_10}
\end{figure}

\begin{figure}
    \centering
    \includegraphics[scale=0.34]{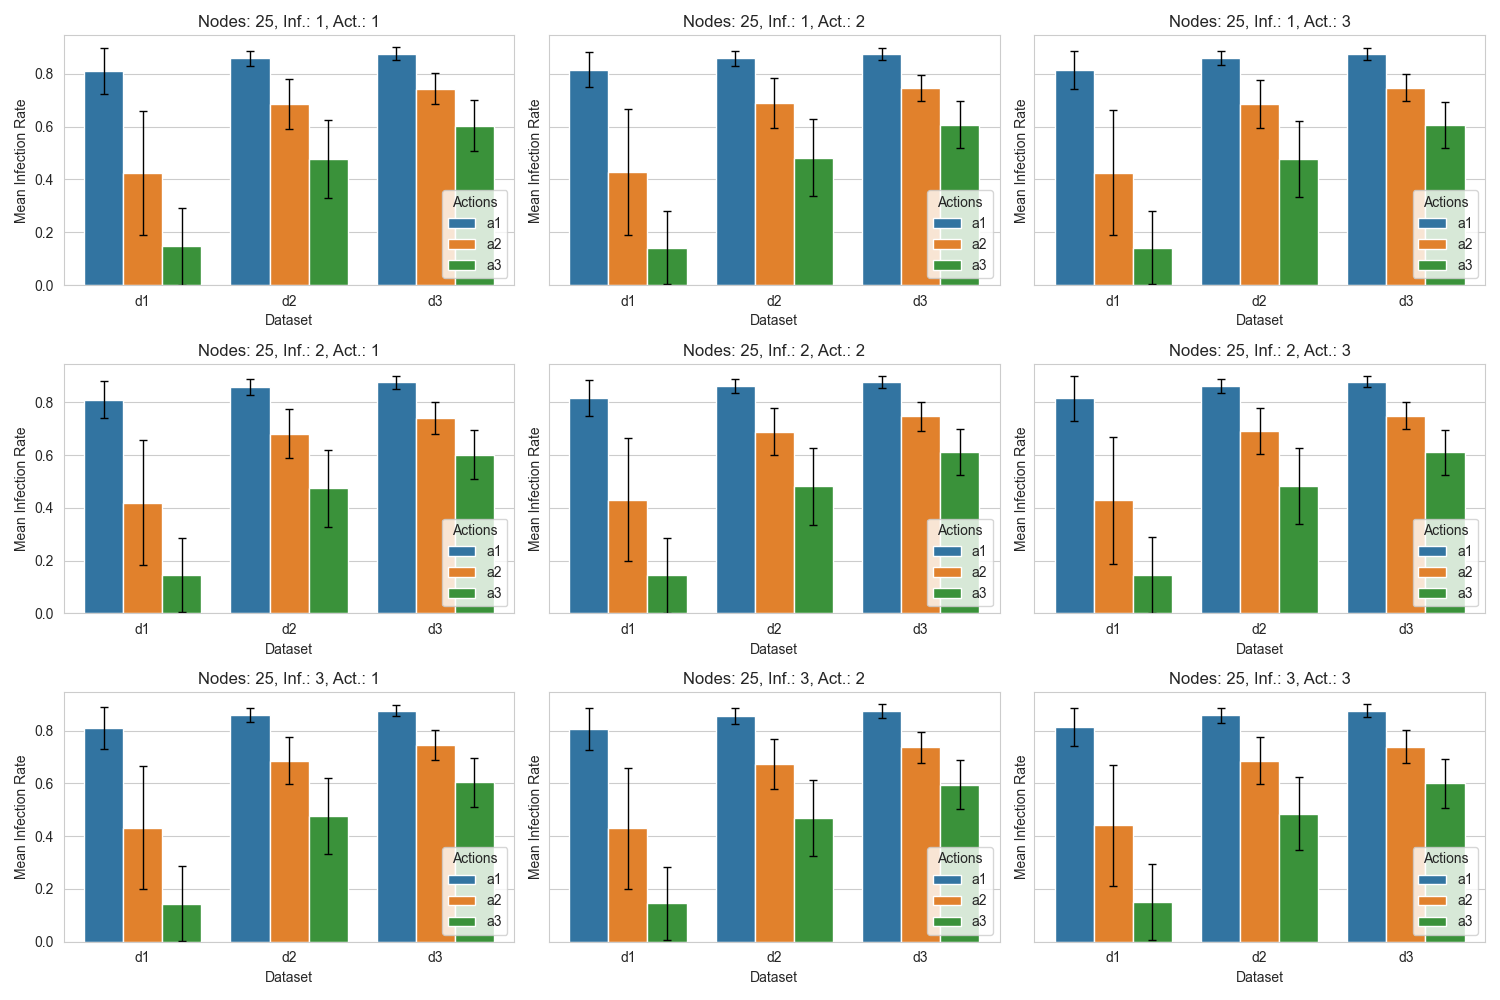}
    \caption{Case-2 using R2: Performance comparison of the RL policies trained using ResNet model for a 25-node network. The barplot displays the mean infection rate for datasets d1, d2, and d3 of Dataset v1 type, differentiated by the number of initial misinformation sources (Inf.) and action budgets (Act.: a1, a2, a3). Each subplot illustrates the performance of a policy trained with the parameters indicated in its title. Lower infection rates indicate more effective policy learning and misinformation containment.}
    \label{fig:inf_resnet_c2r2_25}
\end{figure}

\begin{figure}
    \centering
    \includegraphics[scale=0.34]{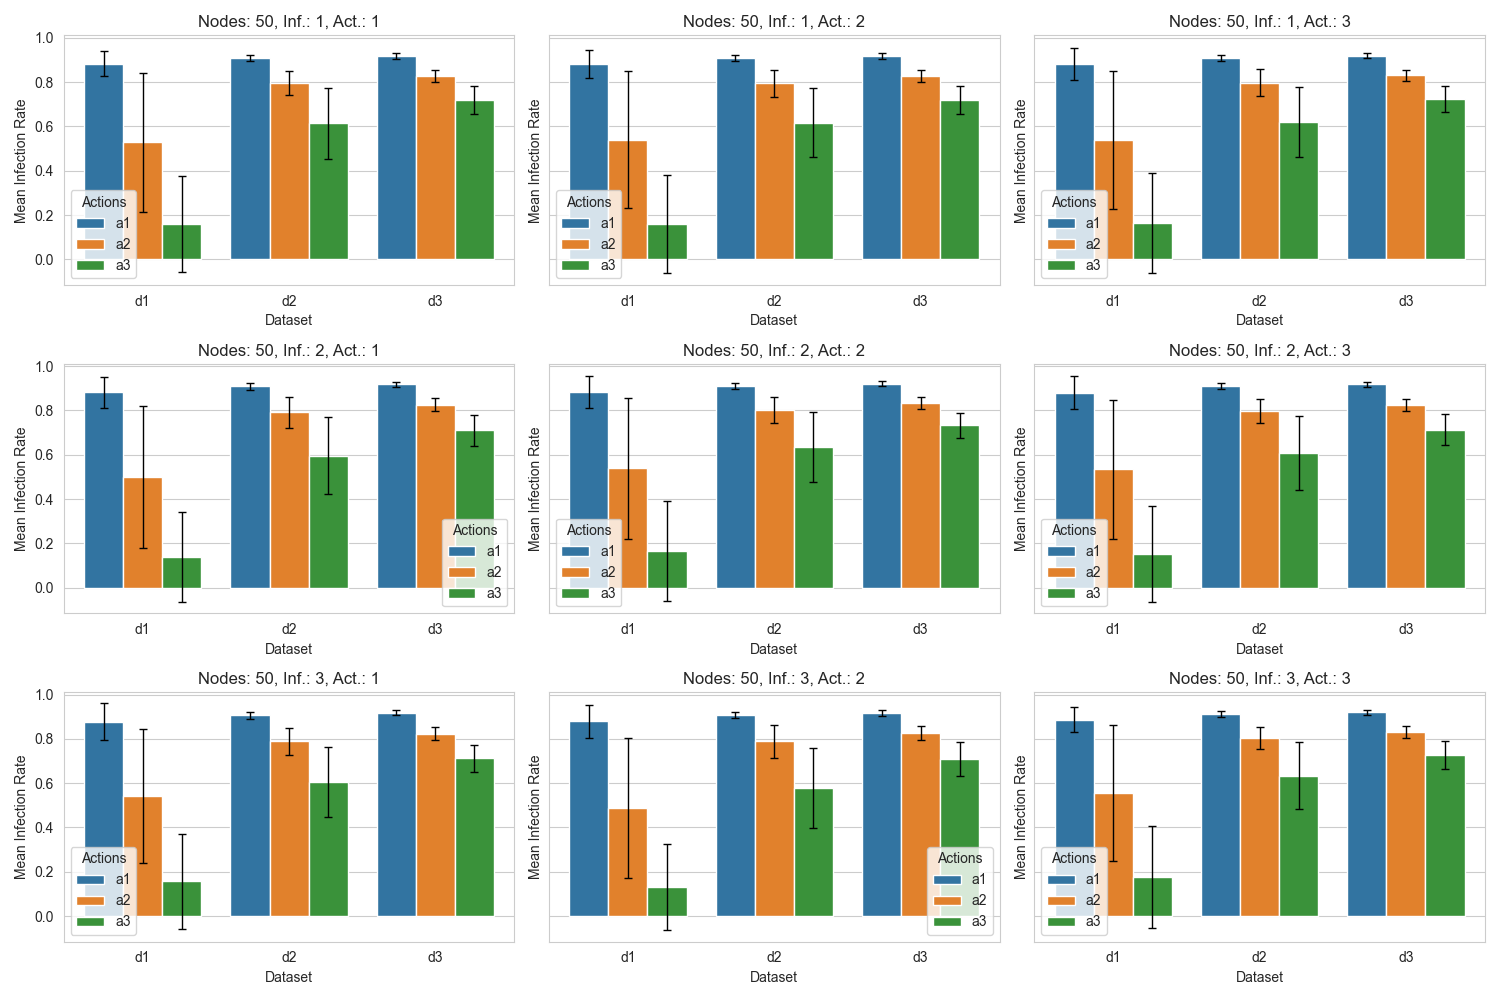}
    \caption{Case-2 using R2: Performance comparison of the RL policies trained using ResNet model for a 50-node network. The barplot displays the mean infection rate for datasets d1, d2, and d3 of Dataset v1 type, differentiated by the number of initial misinformation sources (Inf.) and action budgets (Act.: a1, a2, a3). Each subplot illustrates the performance of a policy trained with the parameters indicated in its title. Lower infection rates indicate more effective policy learning and misinformation containment.}
    \label{fig:inf_resnet_c2r2_50}
\end{figure}

%%%%%% R3 %%%%%%%%
\begin{figure}[!h]
    \centering
    \includegraphics[scale=0.34]{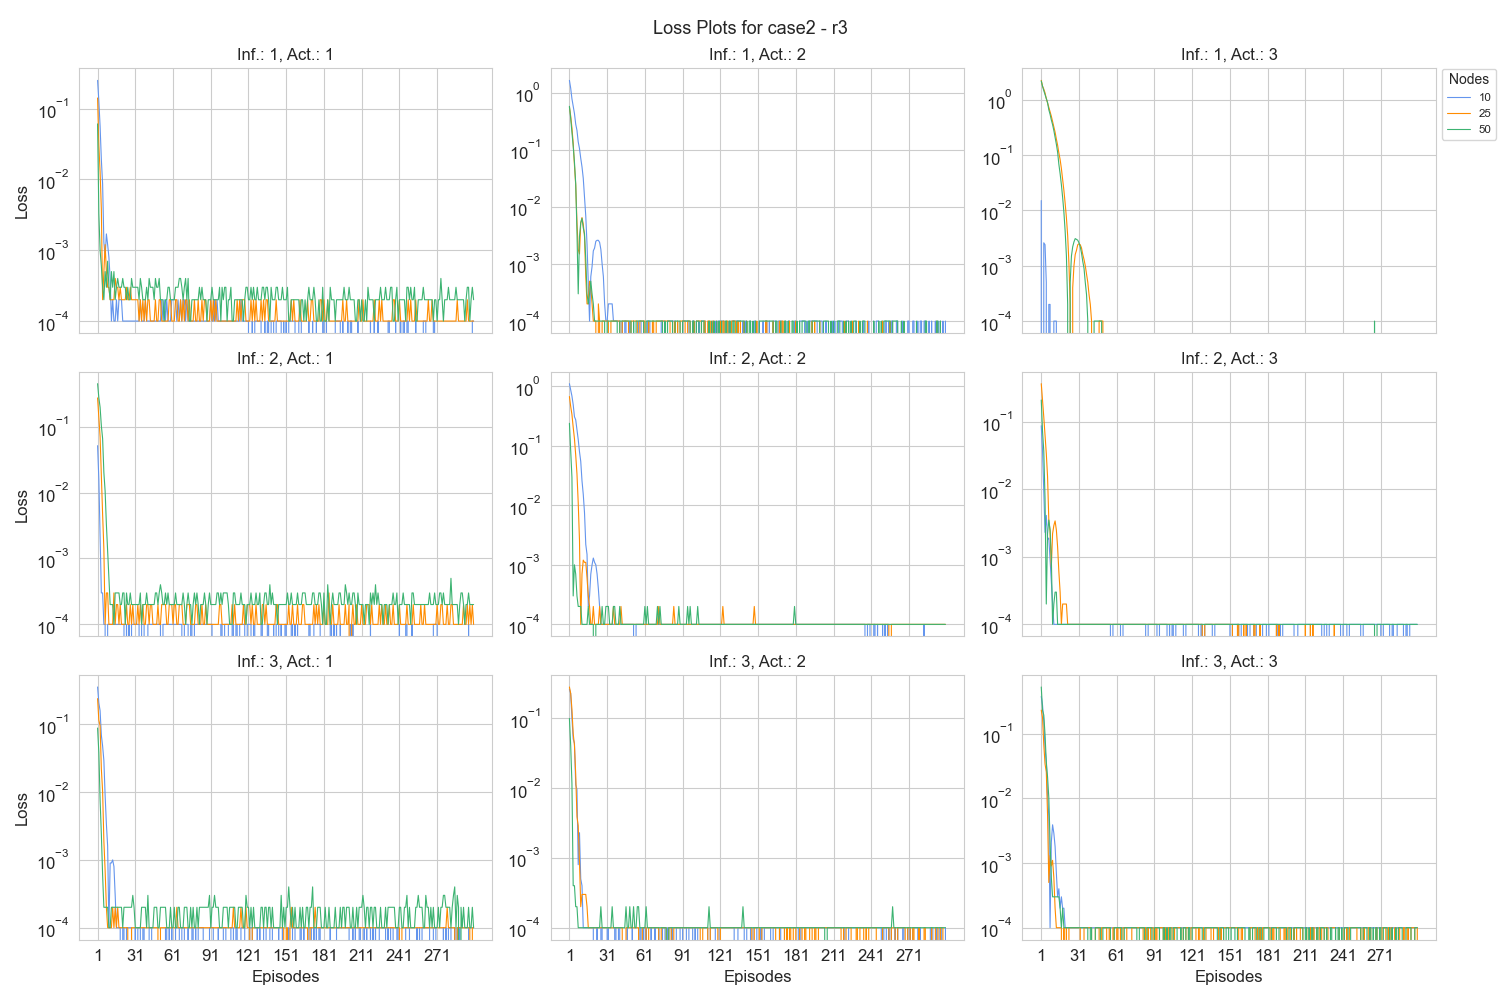}
    \caption{Case-2 using R3: Training MSE loss evolution for RL policy using ResNet model across networks of 10 (blue), 25 (orange), and 50 (green) nodes, for varying initial misinformation sources (Inf.) and action budgets (Act.). Plotted on a logarithmic scale, the loss decreases over episodes, indicating improved policy performance and adaptation across network sizes.}
    \label{fig:resnet_c2r3_loss}
\end{figure}

\begin{figure}
    \centering
    \includegraphics[scale=0.34]{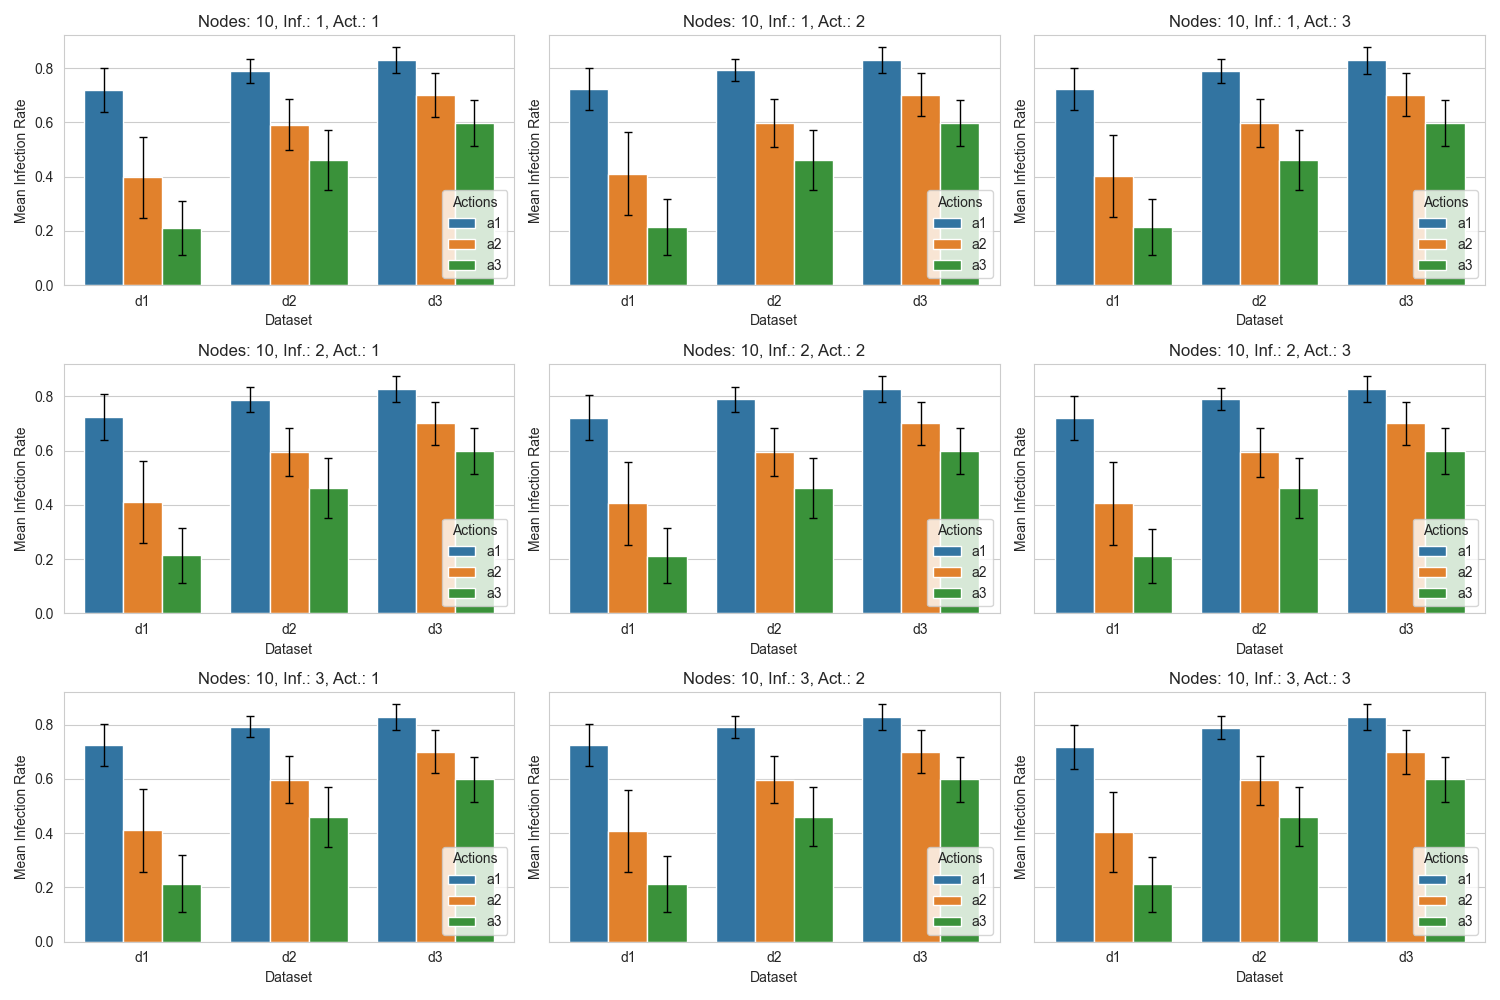}
    \caption{Case-2 using R3: Performance comparison of the RL policies trained using ResNet model for a 10-node network. The barplot displays the mean infection rate for datasets d1, d2, and d3 of Dataset v1 type, differentiated by the number of initial misinformation sources (Inf.) and action budgets (Act.: a1, a2, a3). Each subplot illustrates the performance of a policy trained with the parameters indicated in its title. Lower infection rates indicate more effective policy learning and misinformation containment.}
    \label{fig:inf_resnet_c2r3_10}
\end{figure}

\begin{figure}
    \centering
    \includegraphics[scale=0.34]{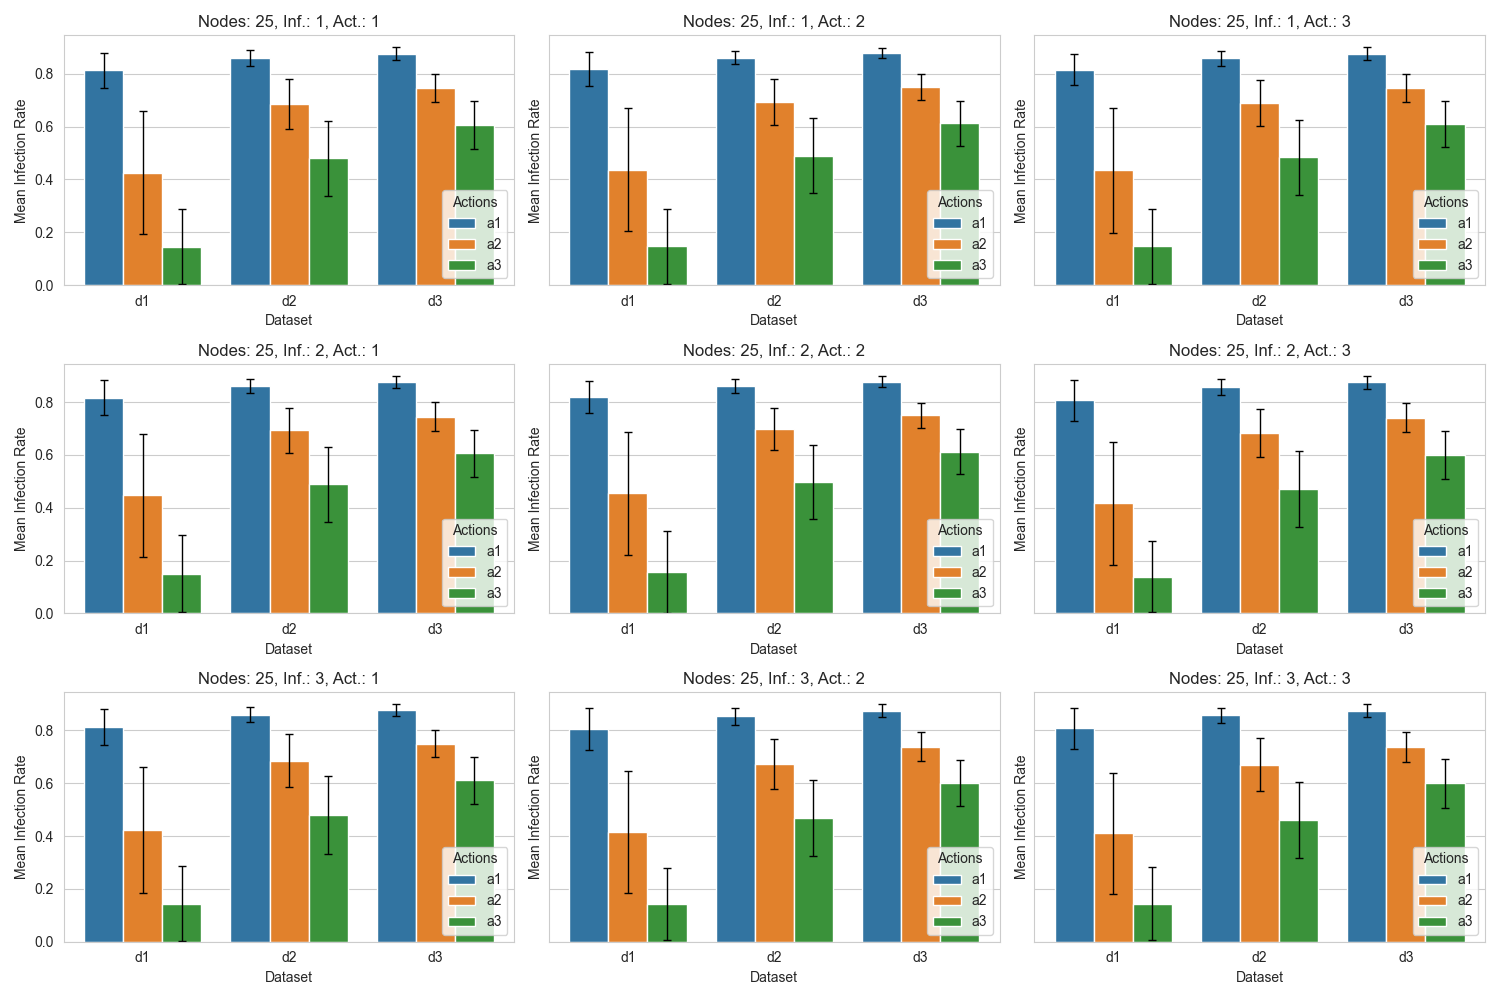}
    \caption{Case-2 using R3: Performance comparison of the RL policies trained using ResNet model for a 25-node network. The barplot displays the mean infection rate for datasets d1, d2, and d3 of Dataset v1 type, differentiated by the number of initial misinformation sources (Inf.) and action budgets (Act.: a1, a2, a3). Each subplot illustrates the performance of a policy trained with the parameters indicated in its title. Lower infection rates indicate more effective policy learning and misinformation containment.}
    \label{fig:inf_resnet_c2r3_25}
\end{figure}

\begin{figure}
    \centering
    \includegraphics[scale=0.34]{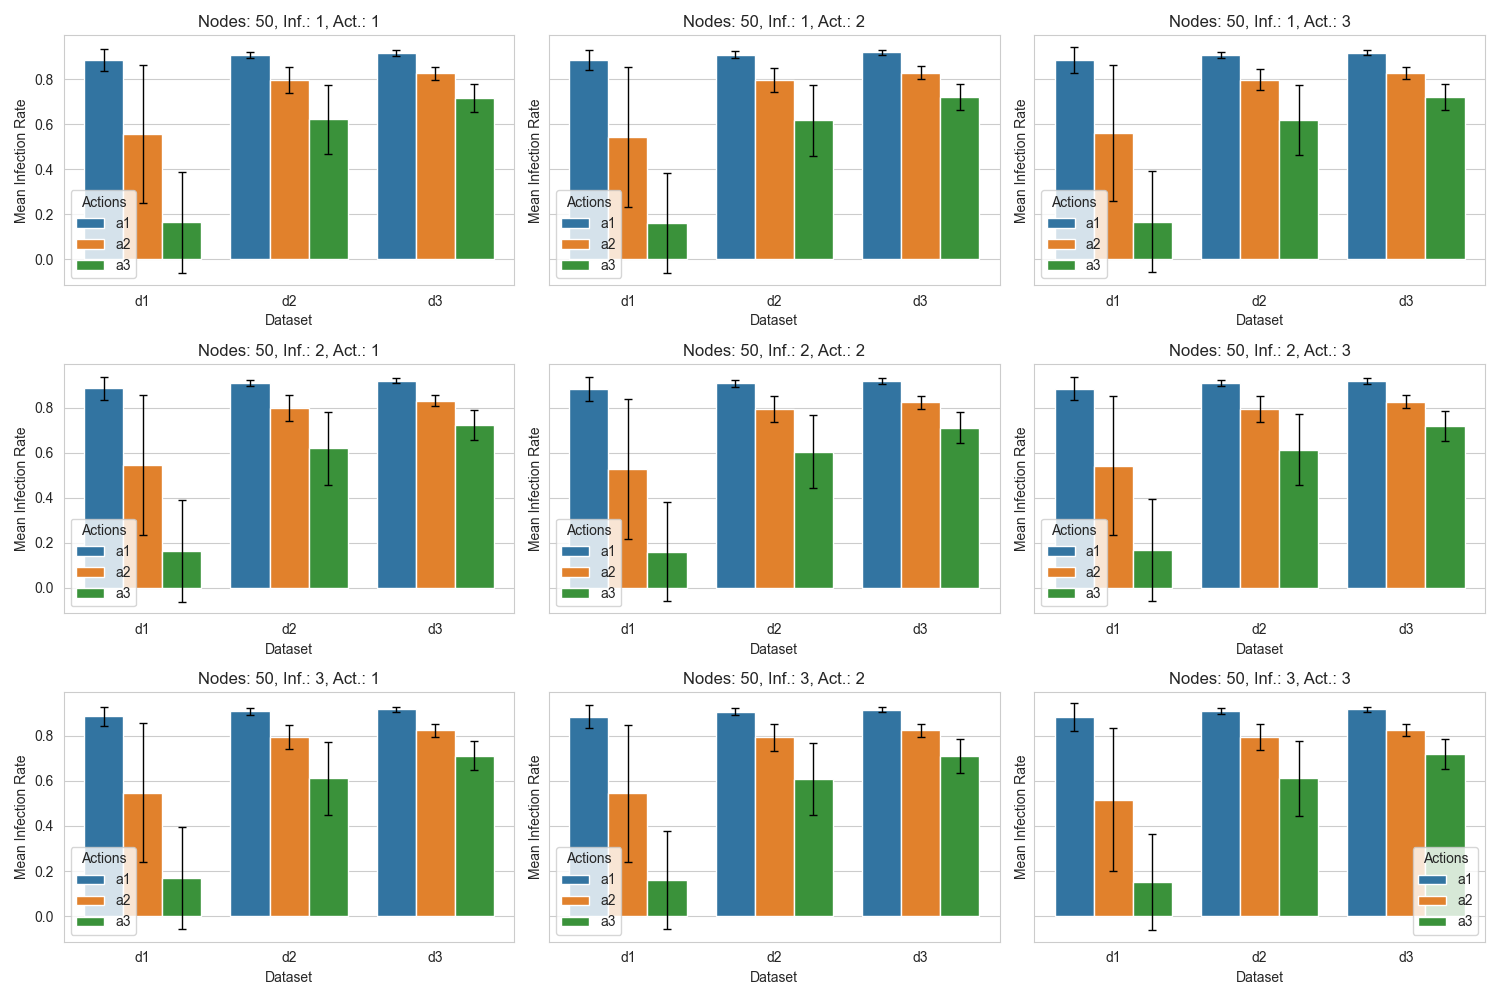}
    \caption{Case-2 using R3: Performance comparison of the RL policies trained using ResNet model for a 50-node network. The barplot displays the mean infection rate for datasets d1, d2, and d3 of Dataset v1 type, differentiated by the number of initial misinformation sources (Inf.) and action budgets (Act.: a1, a2, a3). Each subplot illustrates the performance of a policy trained with the parameters indicated in its title. Lower infection rates indicate more effective policy learning and misinformation containment.}
    \label{fig:inf_resnet_c2r3_50}
\end{figure}

%%%%%% R4 %%%%%%%%
\begin{figure}[!h]
    \centering
    \includegraphics[scale=0.34]{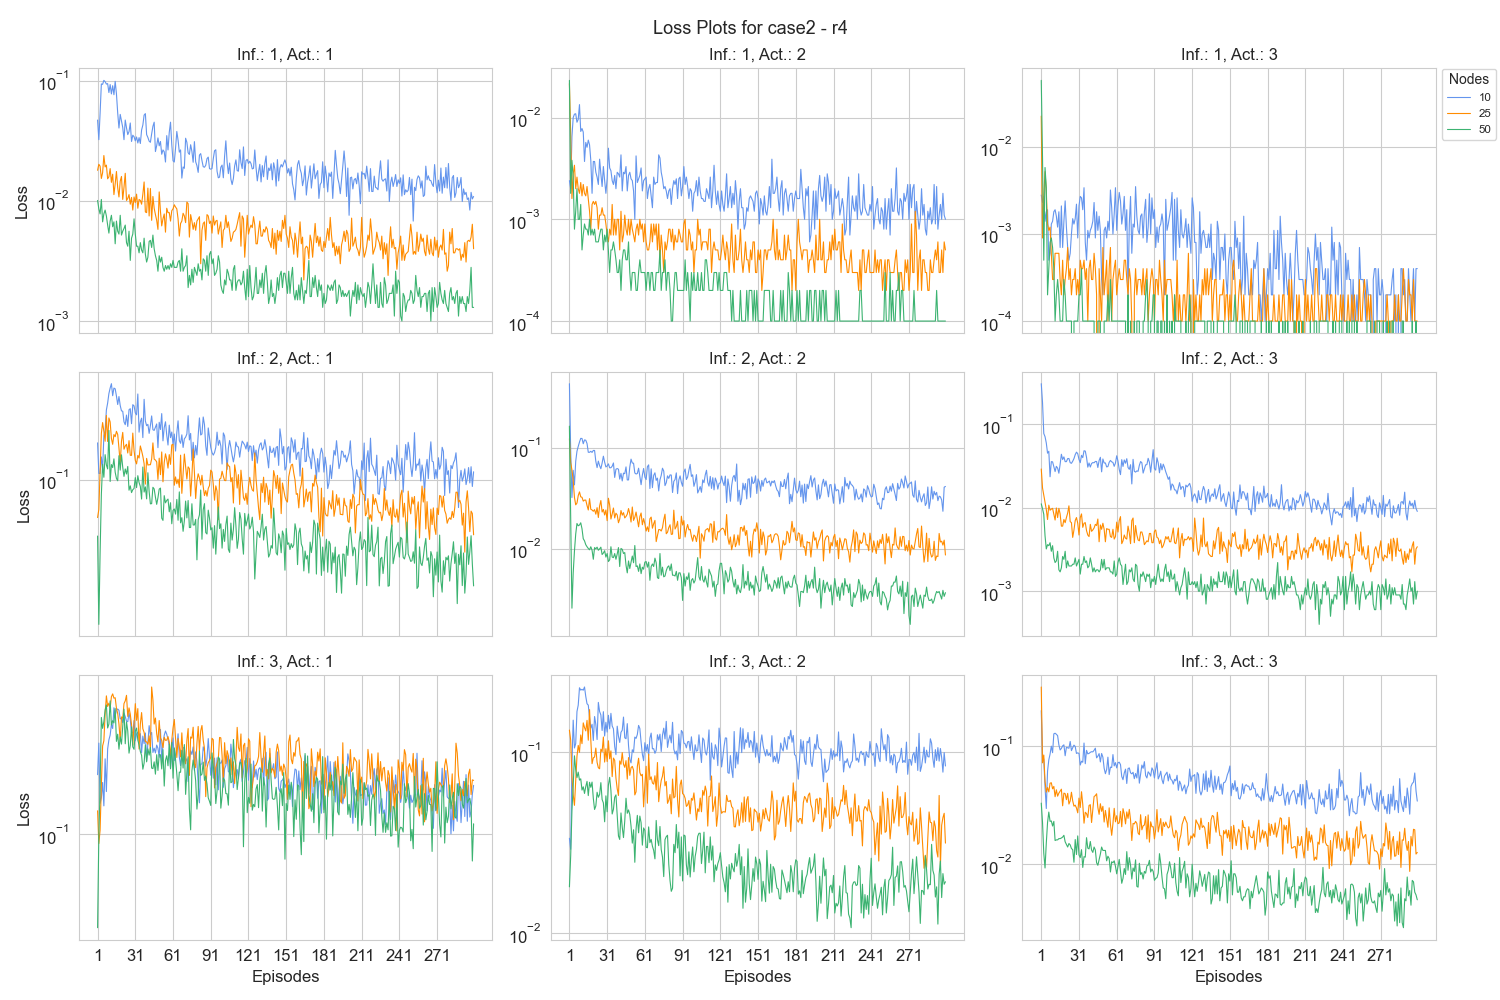}
    \caption{Case-2 using R4: Training MSE loss evolution for RL policy using ResNet model across networks of 10 (blue), 25 (orange), and 50 (green) nodes, for varying initial misinformation sources (Inf.) and action budgets (Act.). Plotted on a logarithmic scale, the loss decreases over episodes, indicating improved policy performance and adaptation across network sizes.}
    \label{fig:resnet_c2r4_loss}
\end{figure}

\begin{figure}
    \centering
    \includegraphics[scale=0.34]{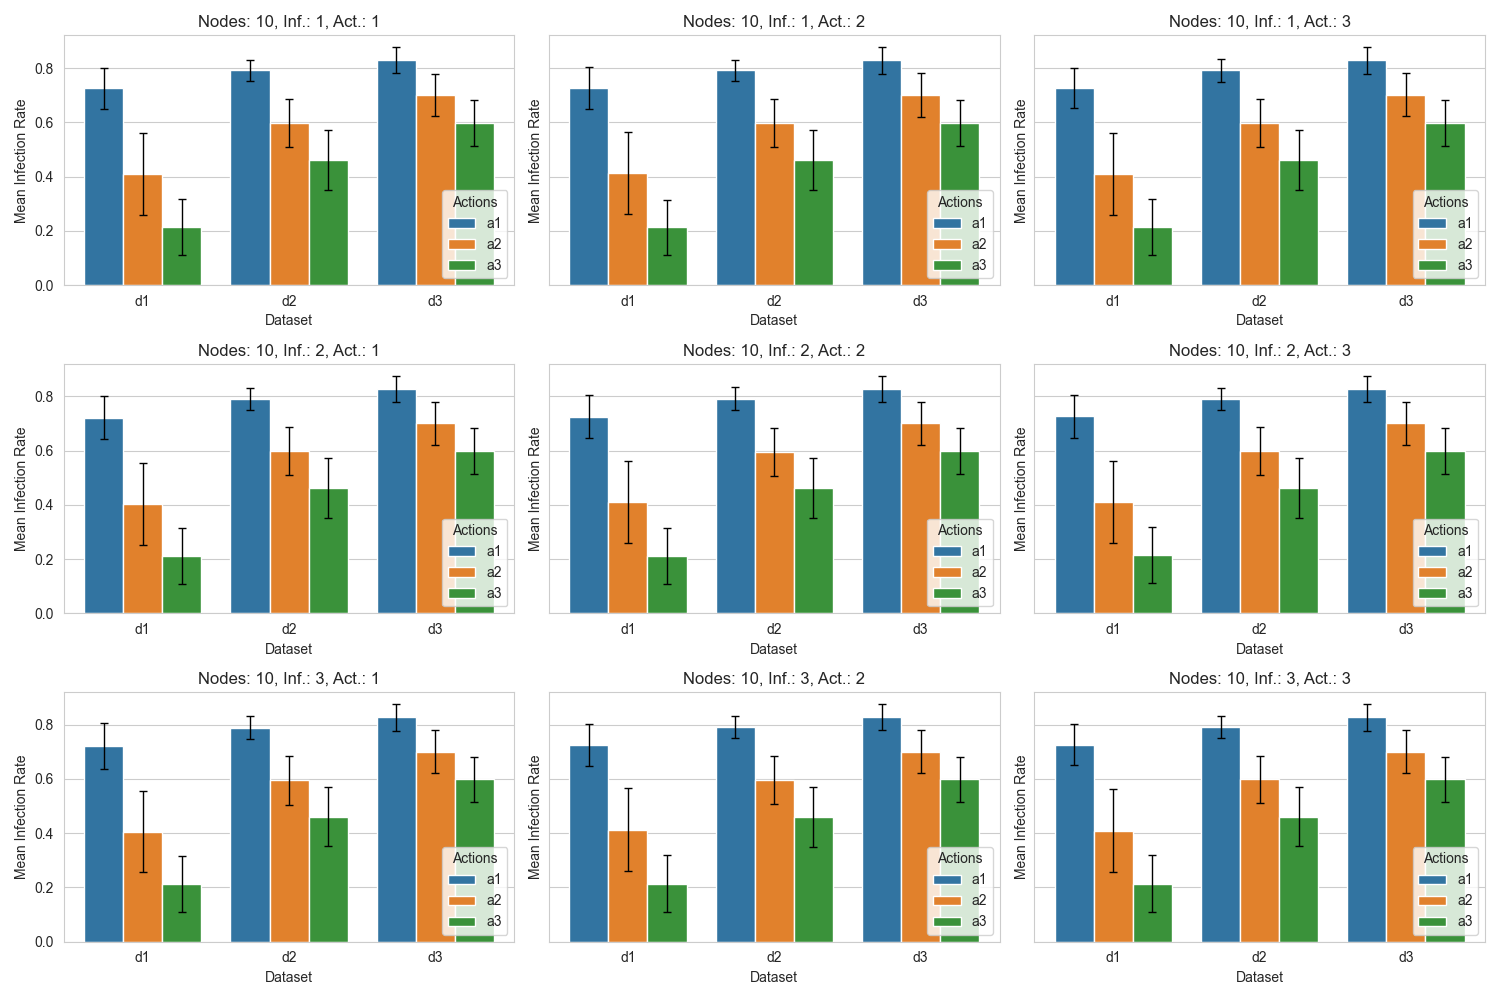}
    \caption{Case-2 using R4: Performance comparison of the RL policies trained using ResNet model for a 10-node network. The barplot displays the mean infection rate for datasets d1, d2, and d3 of Dataset v1 type, differentiated by the number of initial misinformation sources (Inf.) and action budgets (Act.: a1, a2, a3). Each subplot illustrates the performance of a policy trained with the parameters indicated in its title. Lower infection rates indicate more effective policy learning and misinformation containment.}
    \label{fig:inf_resnet_c2r4_10}
\end{figure}

\begin{figure}
    \centering
    \includegraphics[scale=0.34]{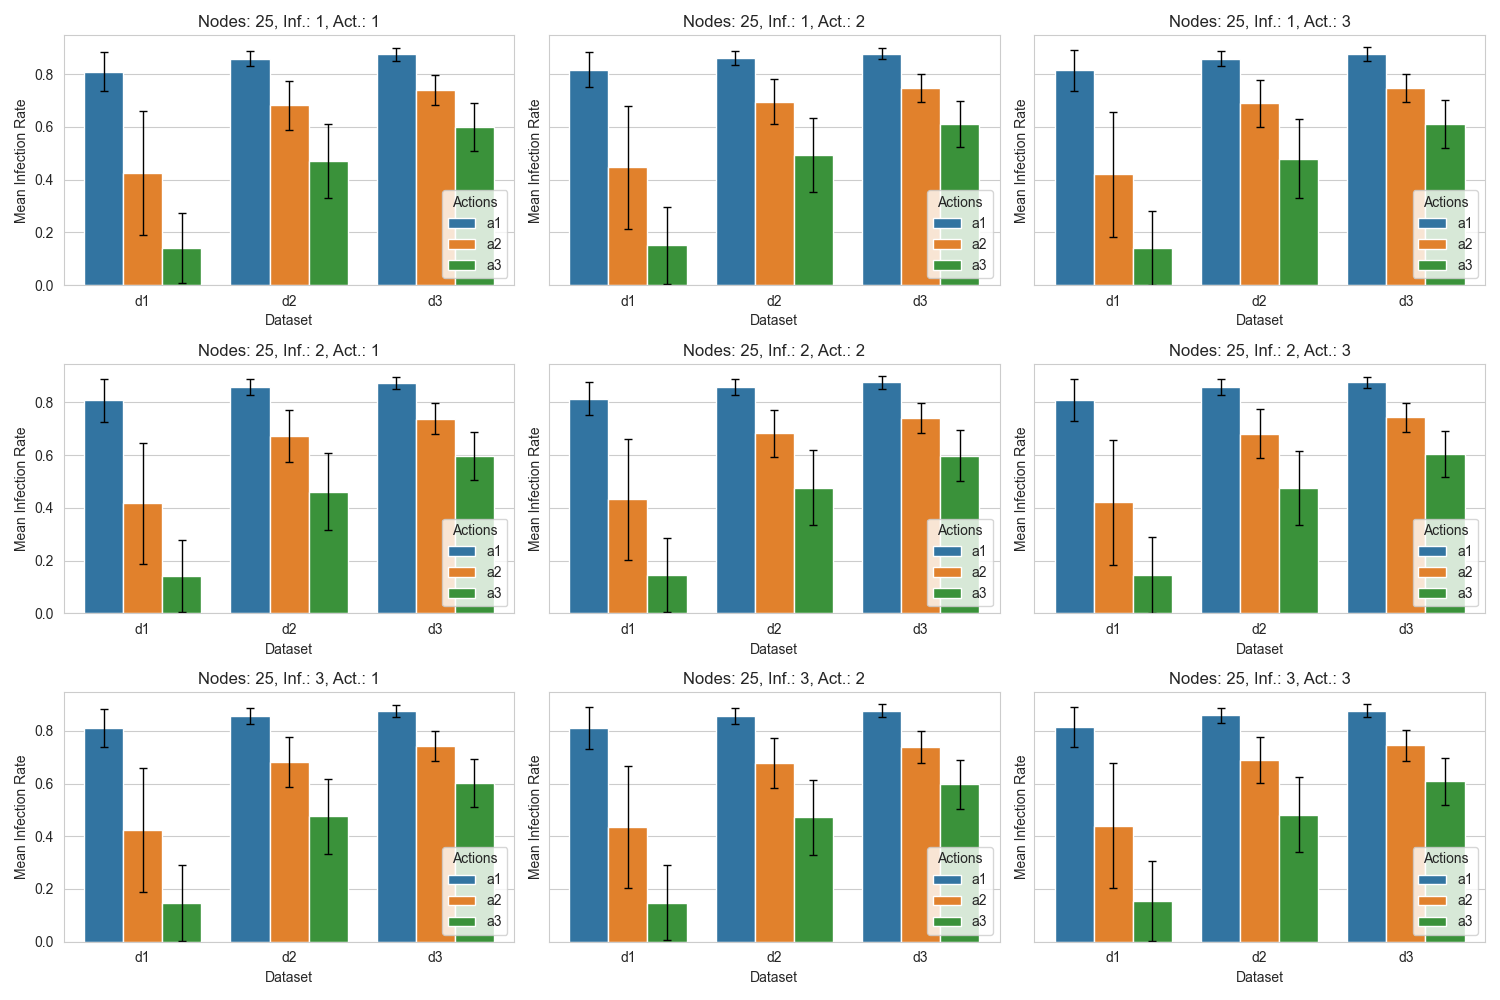}
    \caption{Case-2 using R4: Performance comparison of the RL policies trained using ResNet model for a 25-node network. The barplot displays the mean infection rate for datasets d1, d2, and d3 of Dataset v1 type, differentiated by the number of initial misinformation sources (Inf.) and action budgets (Act.: a1, a2, a3). Each subplot illustrates the performance of a policy trained with the parameters indicated in its title. Lower infection rates indicate more effective policy learning and misinformation containment.}
    \label{fig:inf_resnet_c2r4_25}
\end{figure}

\begin{figure}
    \centering
    \includegraphics[scale=0.34]{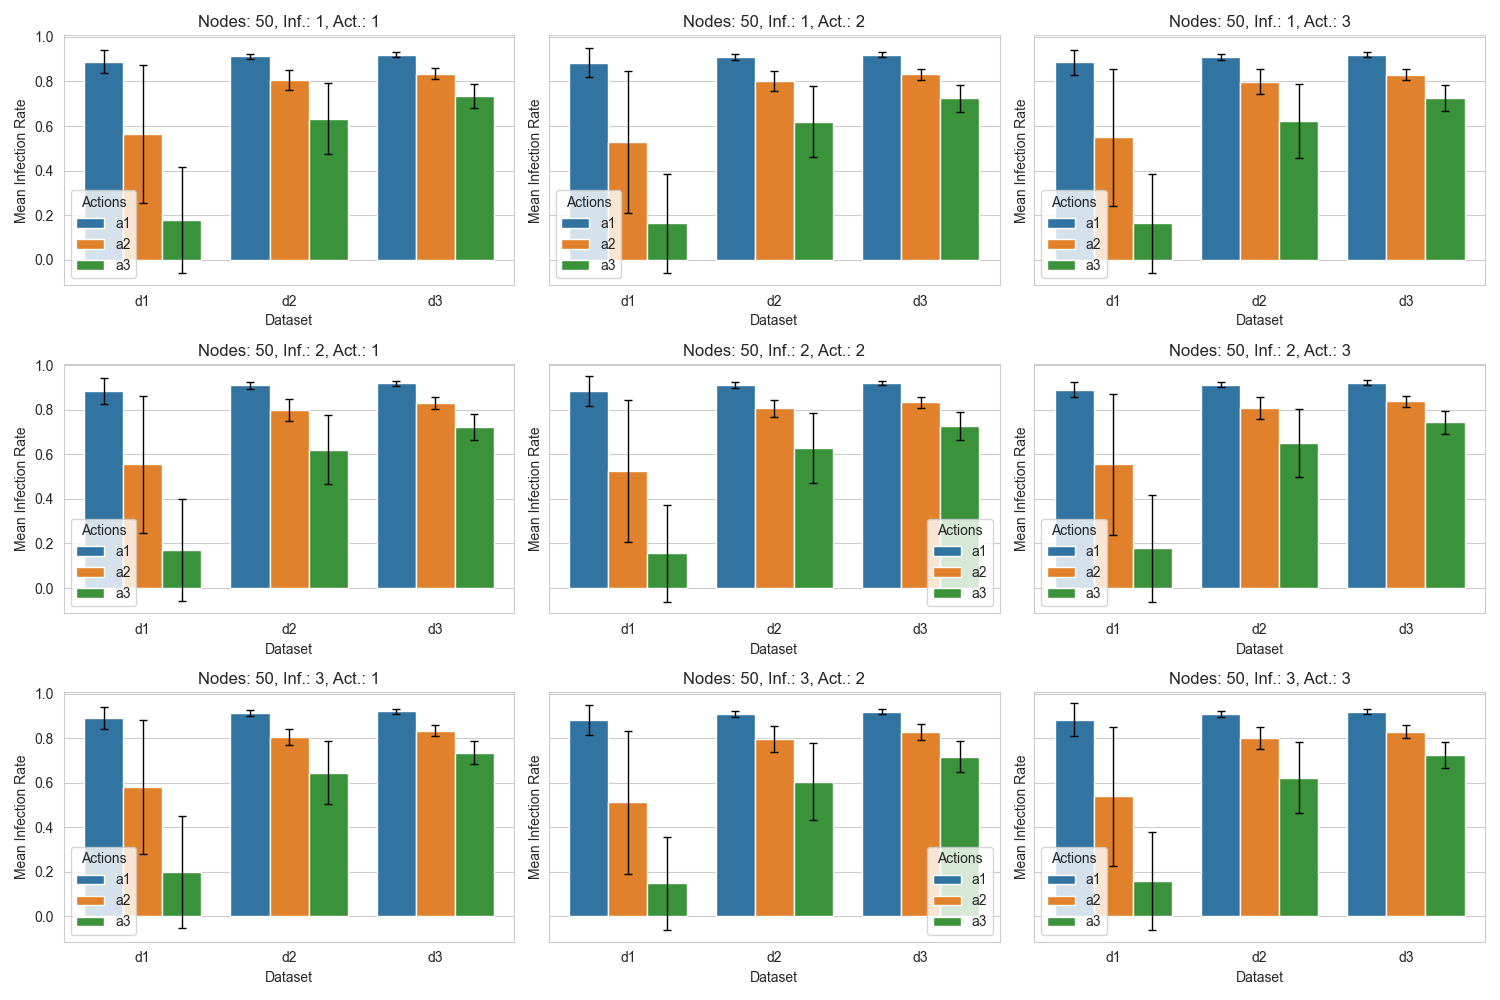}
    \caption{Case-2 using R4: Performance comparison of the RL policies trained using ResNet model for a 50-node network. The barplot displays the mean infection rate for datasets d1, d2, and d3 of Dataset v1 type, differentiated by the number of initial misinformation sources (Inf.) and action budgets (Act.: a1, a2, a3). Each subplot illustrates the performance of a policy trained with the parameters indicated in its title. Lower infection rates indicate more effective policy learning and misinformation containment.}
    \label{fig:inf_resnet_c2r4_50}
\end{figure}

%####################################

% ######### Case 3-v1 ResNet Figures ##########

%%%%%% R0 %%%%%%
\begin{figure}[!h]
    \centering
    \includegraphics[scale=0.34]{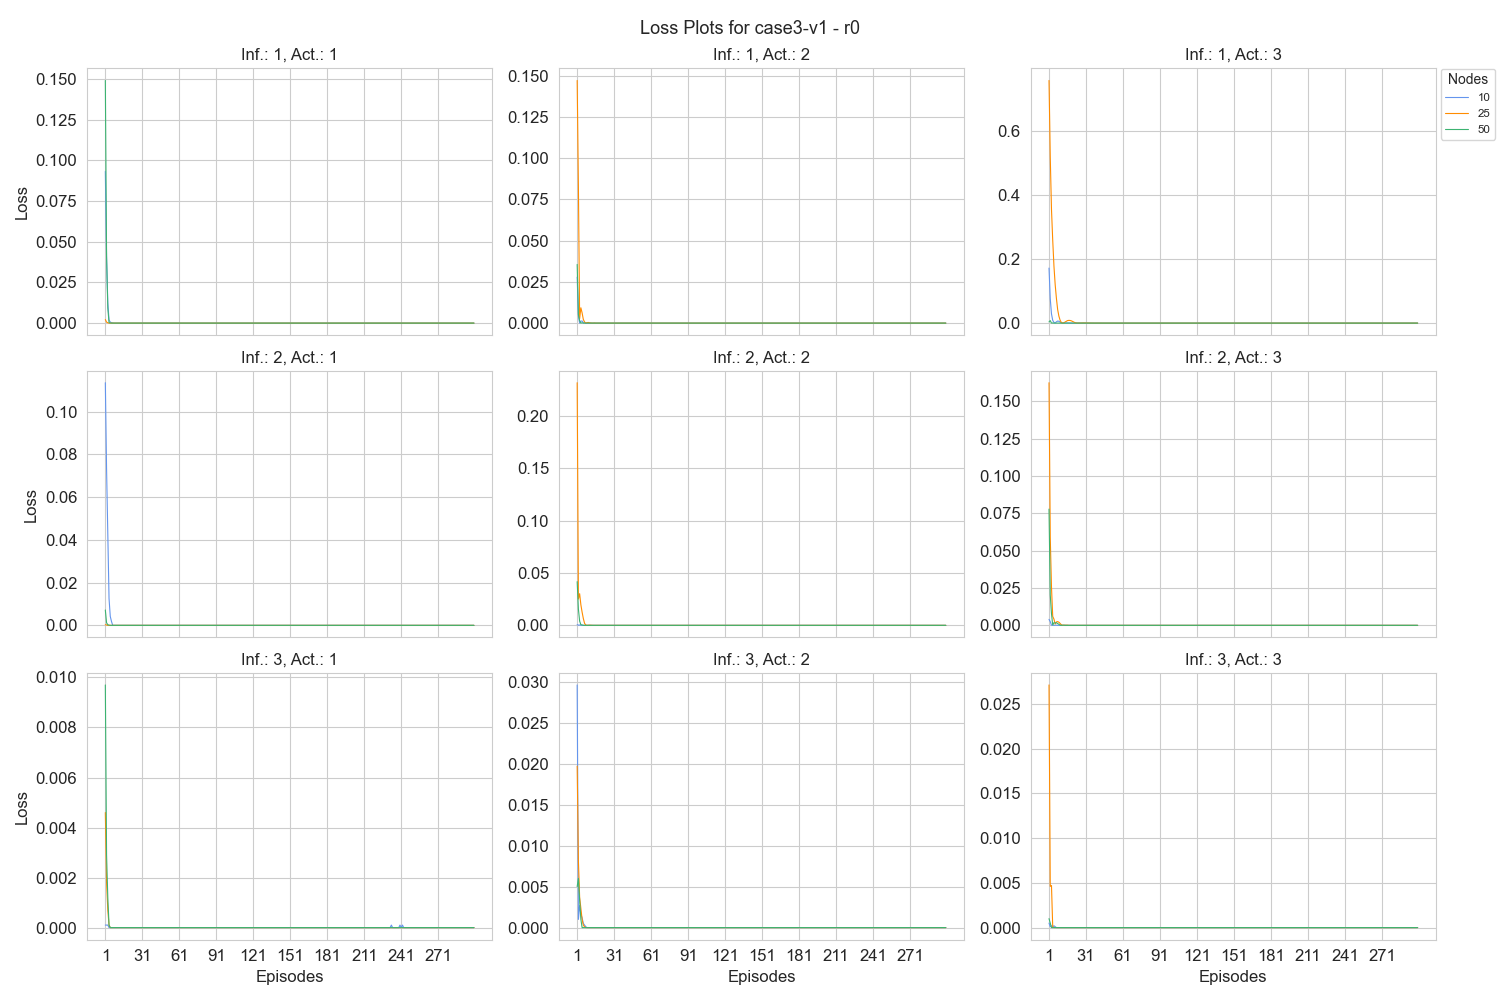}
    \caption{Case-3 v1 using R0: Training MSE loss evolution for RL policy using ResNet model across networks of 10 (blue), 25 (orange), and 50 (green) nodes, for varying initial misinformation sources (Inf.) and action budgets (Act.). The loss decreases over episodes, indicating improved policy performance and adaptation across network sizes.}
    \label{fig:resnet_c3v1r0_loss}
\end{figure}

\begin{figure}
    \centering
    \includegraphics[scale=0.34]{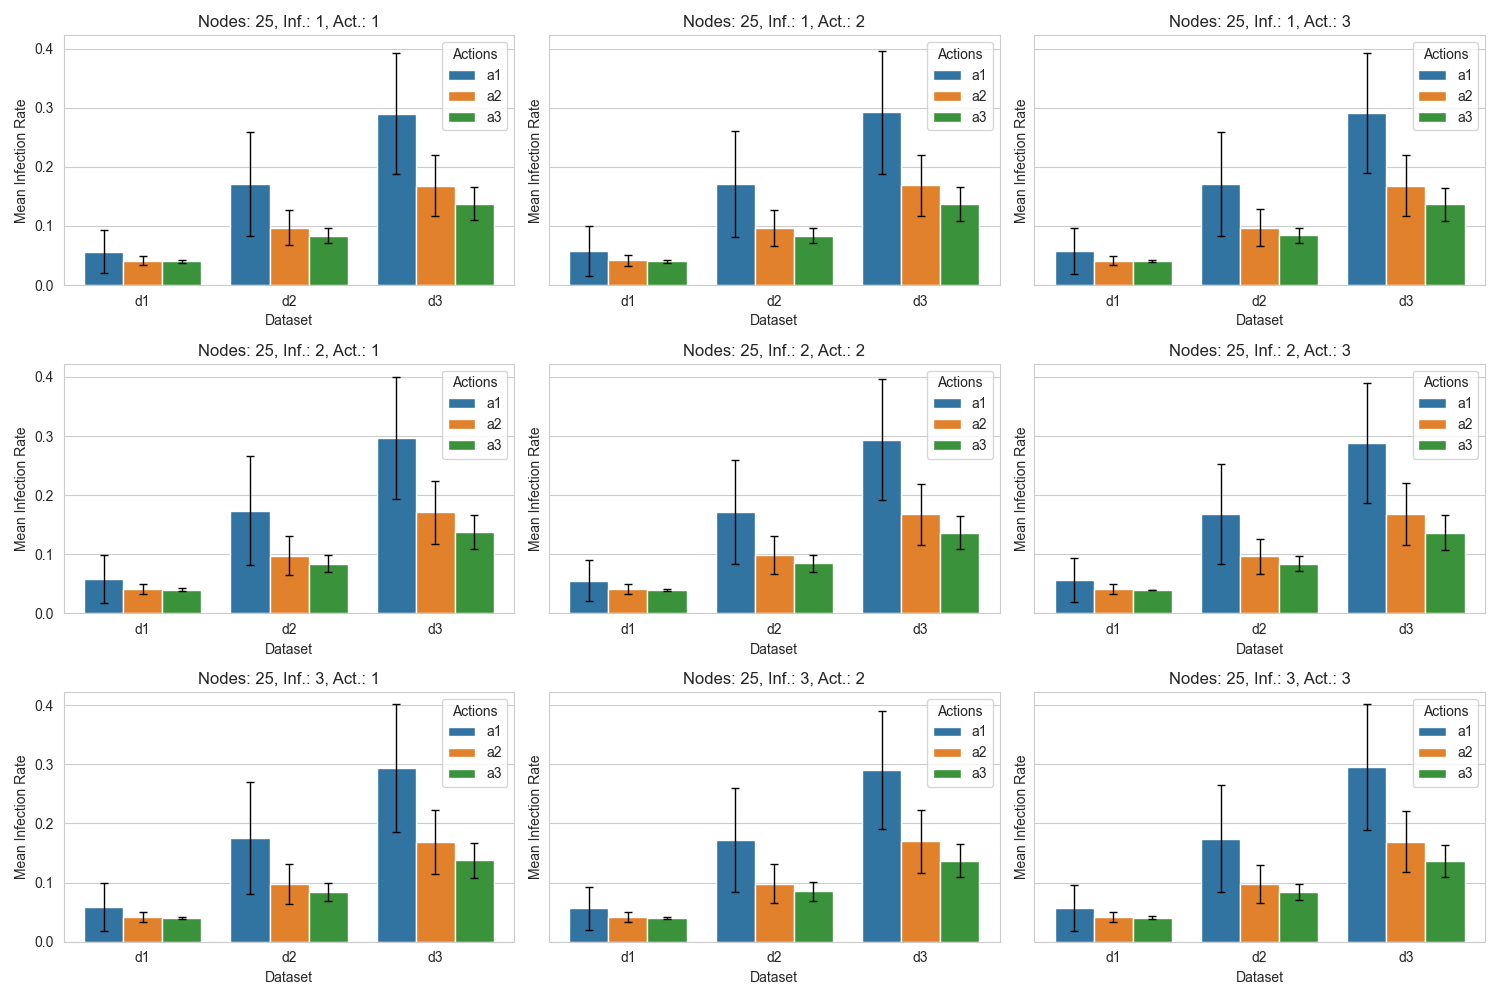}
    \caption{Case-3 v1 using R0: Performance comparison of the RL policies trained using ResNet model for a 25-node network. The barplot displays the mean infection rate for datasets d1, d2, and d3 of Dataset v1 type, differentiated by the number of initial misinformation sources (Inf.) and action budgets (Act.: a1, a2, a3). Each subplot illustrates the performance of a policy trained with the parameters indicated in its title. Lower infection rates indicate more effective policy learning and misinformation containment.}
    \label{fig:inf_resnet_c3v1r0_25}
\end{figure}

\begin{figure}
    \centering
    \includegraphics[scale=0.34]{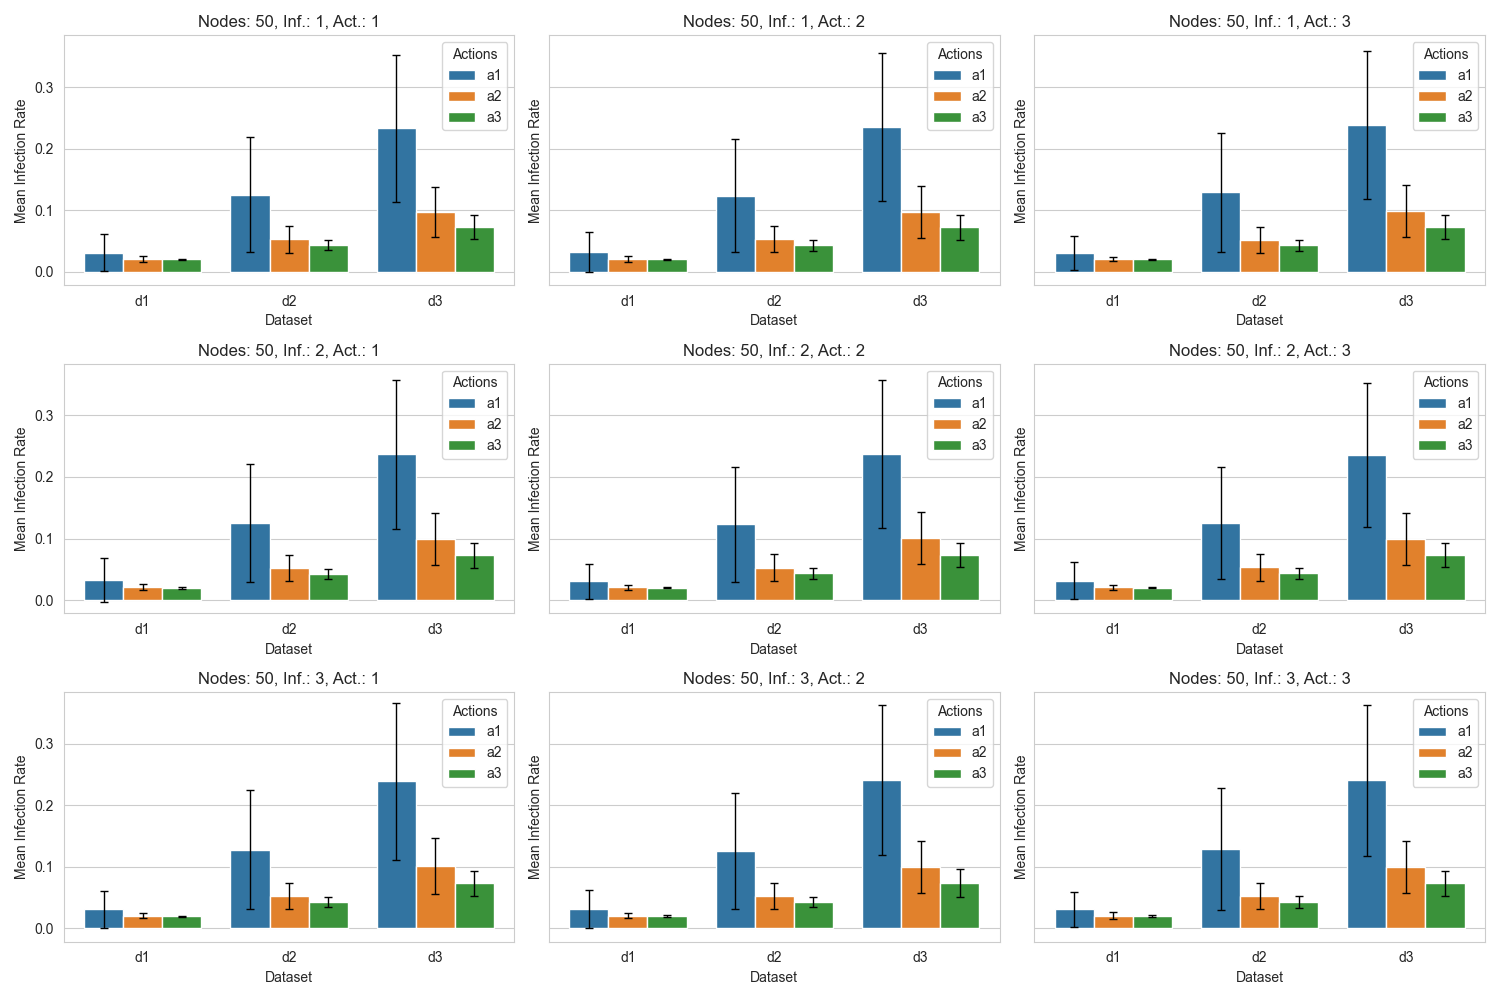}
    \caption{Case-3 v1 using R0: Performance comparison of the RL policies trained using ResNet model for a 50-node network. The barplot displays the mean infection rate for datasets d1, d2, and d3 of Dataset v1 type, differentiated by the number of initial misinformation sources (Inf.) and action budgets (Act.: a1, a2, a3). Each subplot illustrates the performance of a policy trained with the parameters indicated in its title. Lower infection rates indicate more effective policy learning and misinformation containment.}
    \label{fig:inf_resnet_c3v1r0_50}
\end{figure}

%%%%%% R1 %%%%%%%
\begin{figure}[!h]
    \centering
    \includegraphics[scale=0.34]{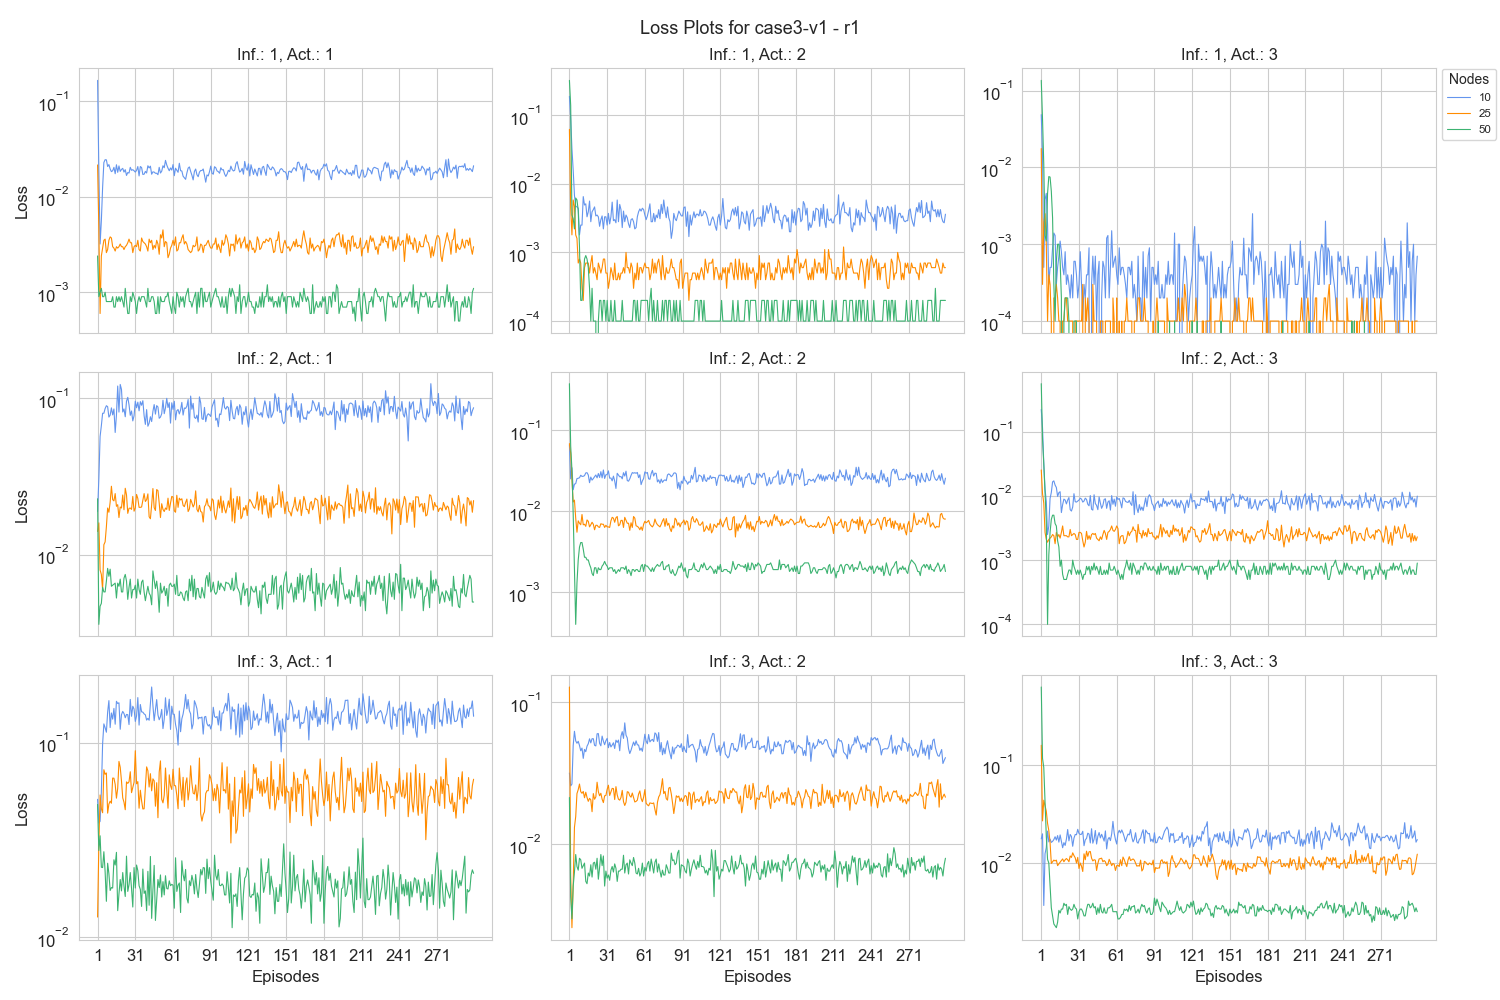}
    \caption{Case-3 v1 using R1: Training MSE loss evolution for RL policy using ResNet model across networks of 10 (blue), 25 (orange), and 50 (green) nodes, for varying initial misinformation sources (Inf.) and action budgets (Act.). Plotted on a logarithmic scale, the loss decreases over episodes, indicating improved policy performance and adaptation across network sizes.}
    \label{fig:resnet_c3v1r1_loss}
\end{figure}

\begin{figure}
    \centering
    \includegraphics[scale=0.34]{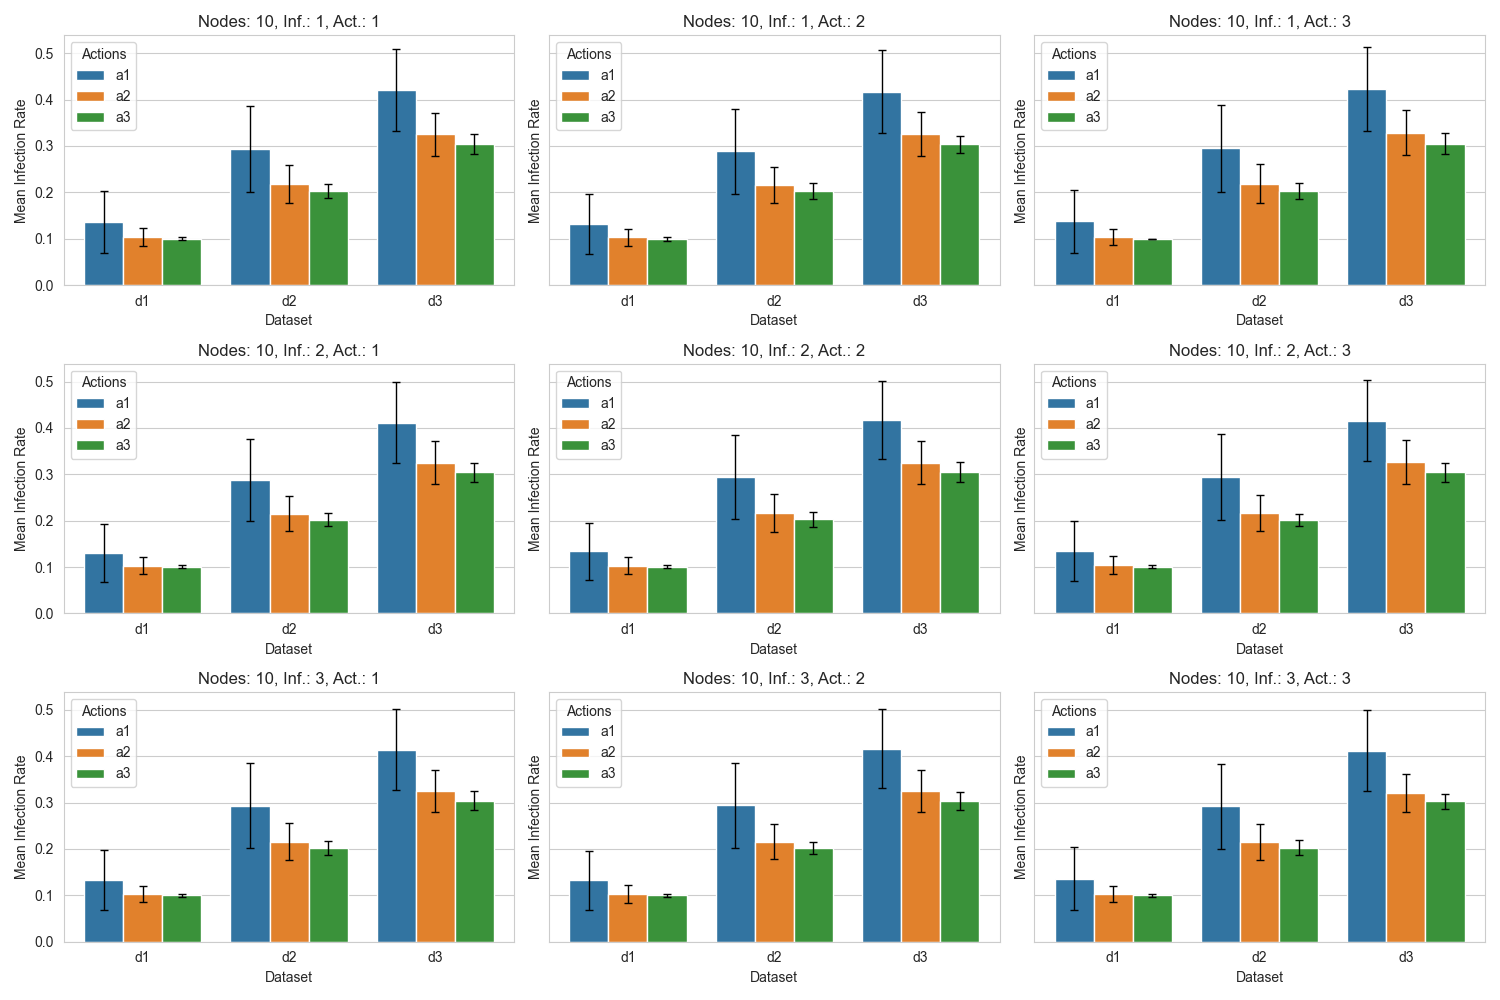}
    \caption{Case-3 v1 using R1: Performance comparison of the RL policies trained using ResNet model for a 10-node network. The barplot displays the mean infection rate for datasets d1, d2, and d3 of Dataset v1 type, differentiated by the number of initial misinformation sources (Inf.) and action budgets (Act.: a1, a2, a3). Each subplot illustrates the performance of a policy trained with the parameters indicated in its title. Lower infection rates indicate more effective policy learning and misinformation containment.}
    \label{fig:inf_resnet_c3v1r1_10}
\end{figure}

\begin{figure}
    \centering
    \includegraphics[scale=0.34]{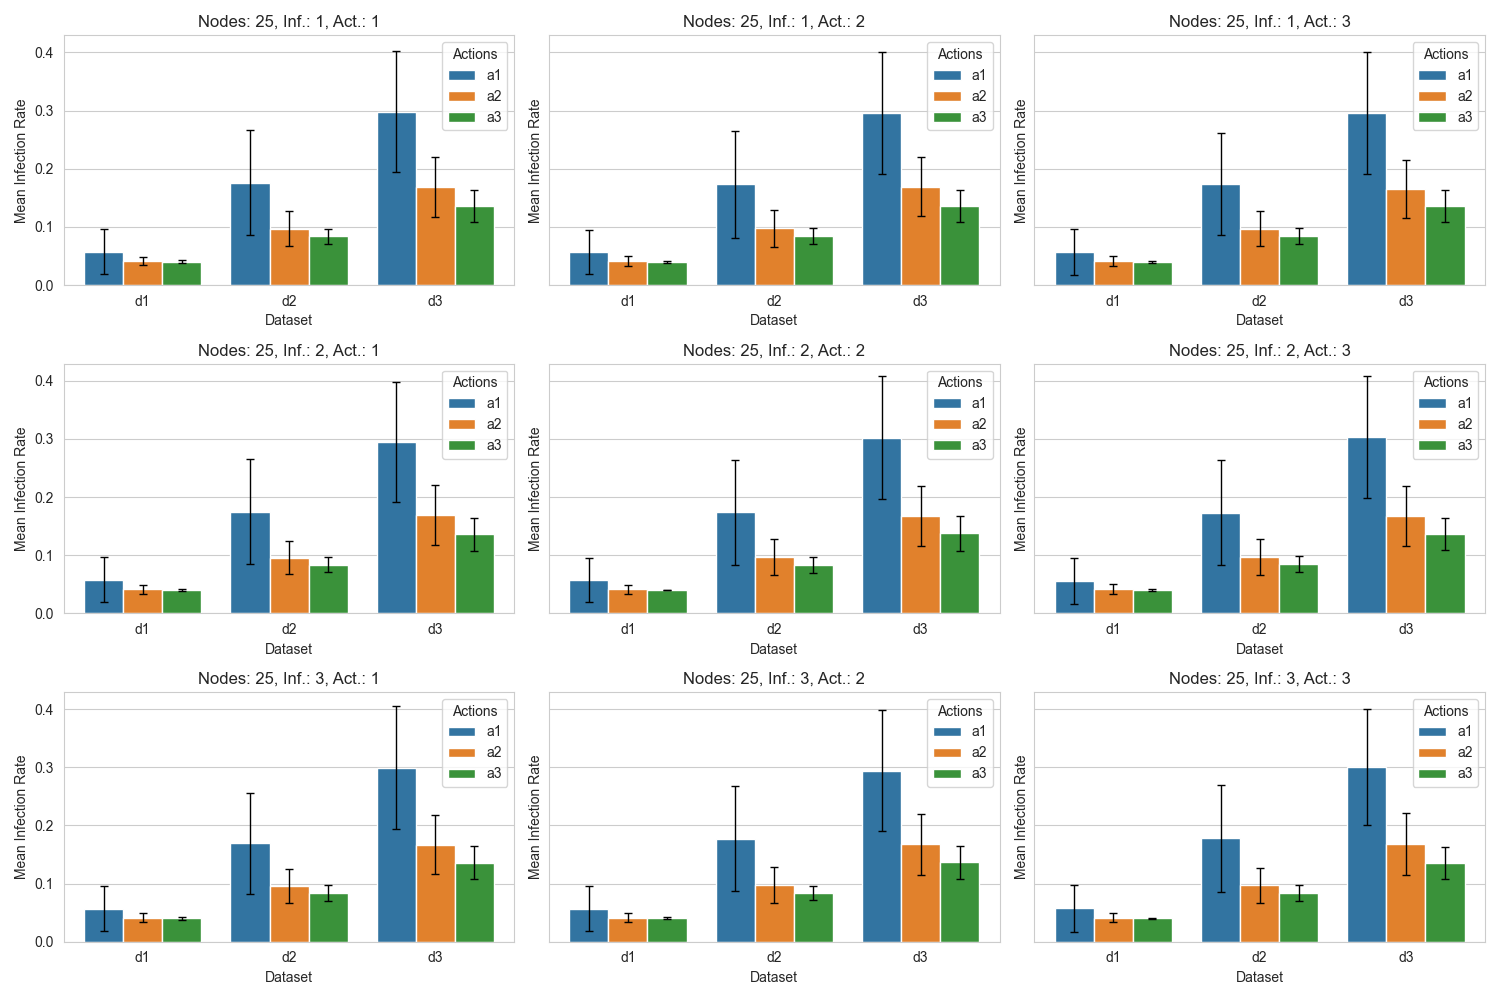}
    \caption{Case-3 v1 using R1: Performance comparison of the RL policies trained using ResNet model for a 25-node network. The barplot displays the mean infection rate for datasets d1, d2, and d3 of Dataset v1 type, differentiated by the number of initial misinformation sources (Inf.) and action budgets (Act.: a1, a2, a3). Each subplot illustrates the performance of a policy trained with the parameters indicated in its title. Lower infection rates indicate more effective policy learning and misinformation containment.}
    \label{fig:inf_resnet_c3v1r1_25}
\end{figure}

\begin{figure}
    \centering
    \includegraphics[scale=0.34]{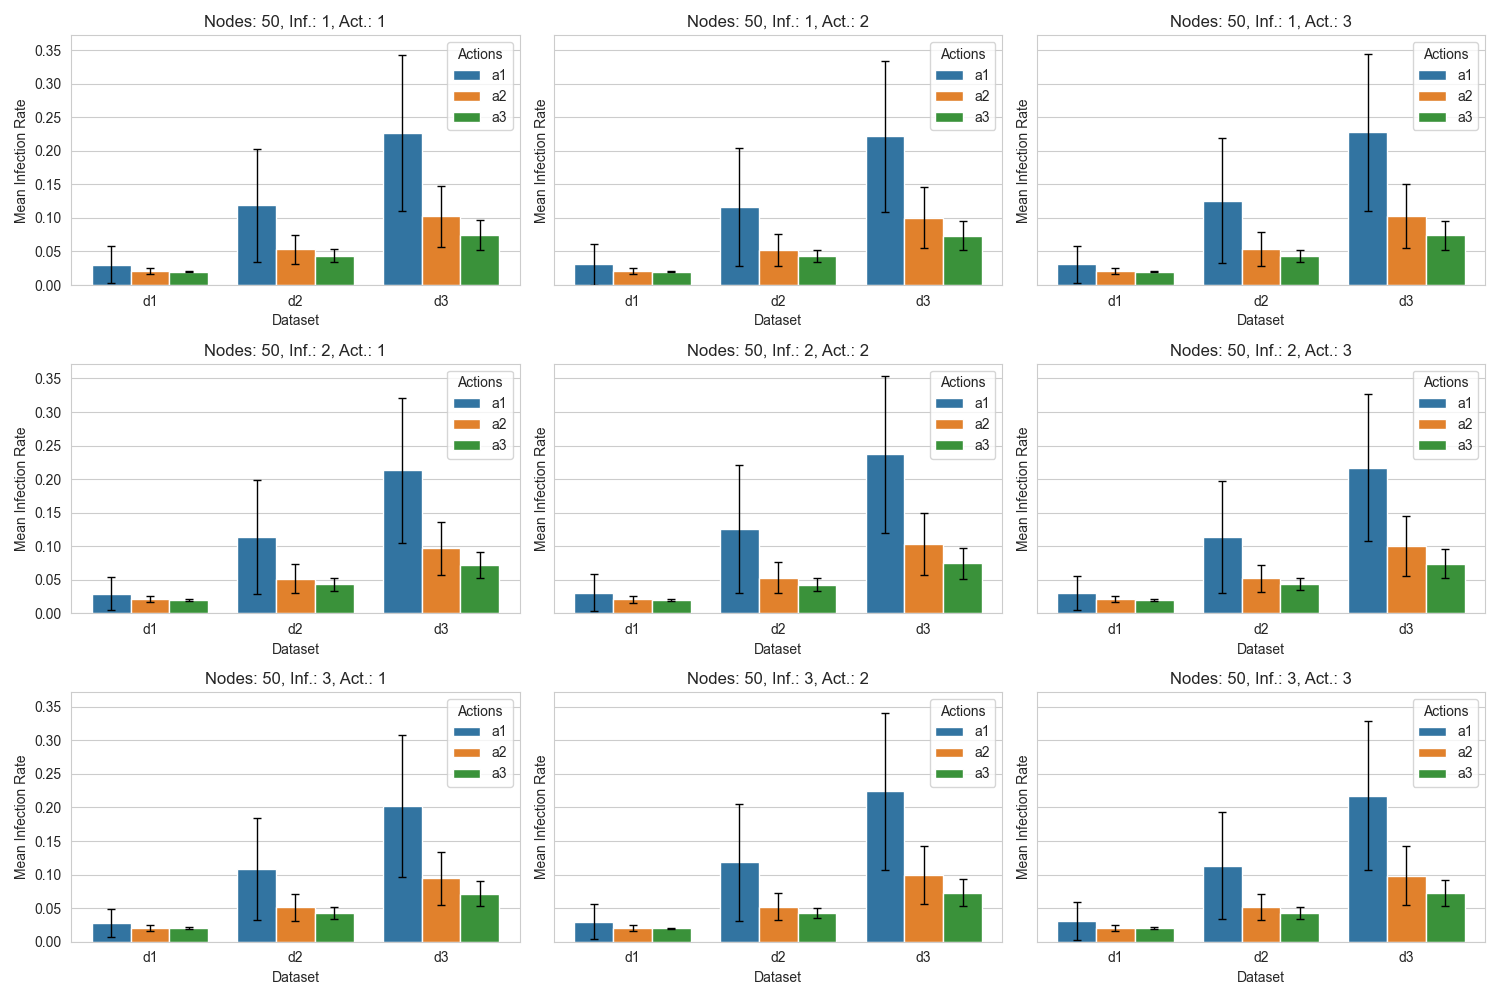}
    \caption{Case-3 v1 using R1: Performance comparison of the RL policies trained using ResNet model for a 50-node network. The barplot displays the mean infection rate for datasets d1, d2, and d3 of Dataset v1 type, differentiated by the number of initial misinformation sources (Inf.) and action budgets (Act.: a1, a2, a3). Each subplot illustrates the performance of a policy trained with the parameters indicated in its title. Lower infection rates indicate more effective policy learning and misinformation containment.}
    \label{fig:inf_resnet_c3v1r1_50}
\end{figure}

%%%%%% R2 %%%%%%%
\begin{figure}[!h]
    \centering
    \includegraphics[scale=0.34]{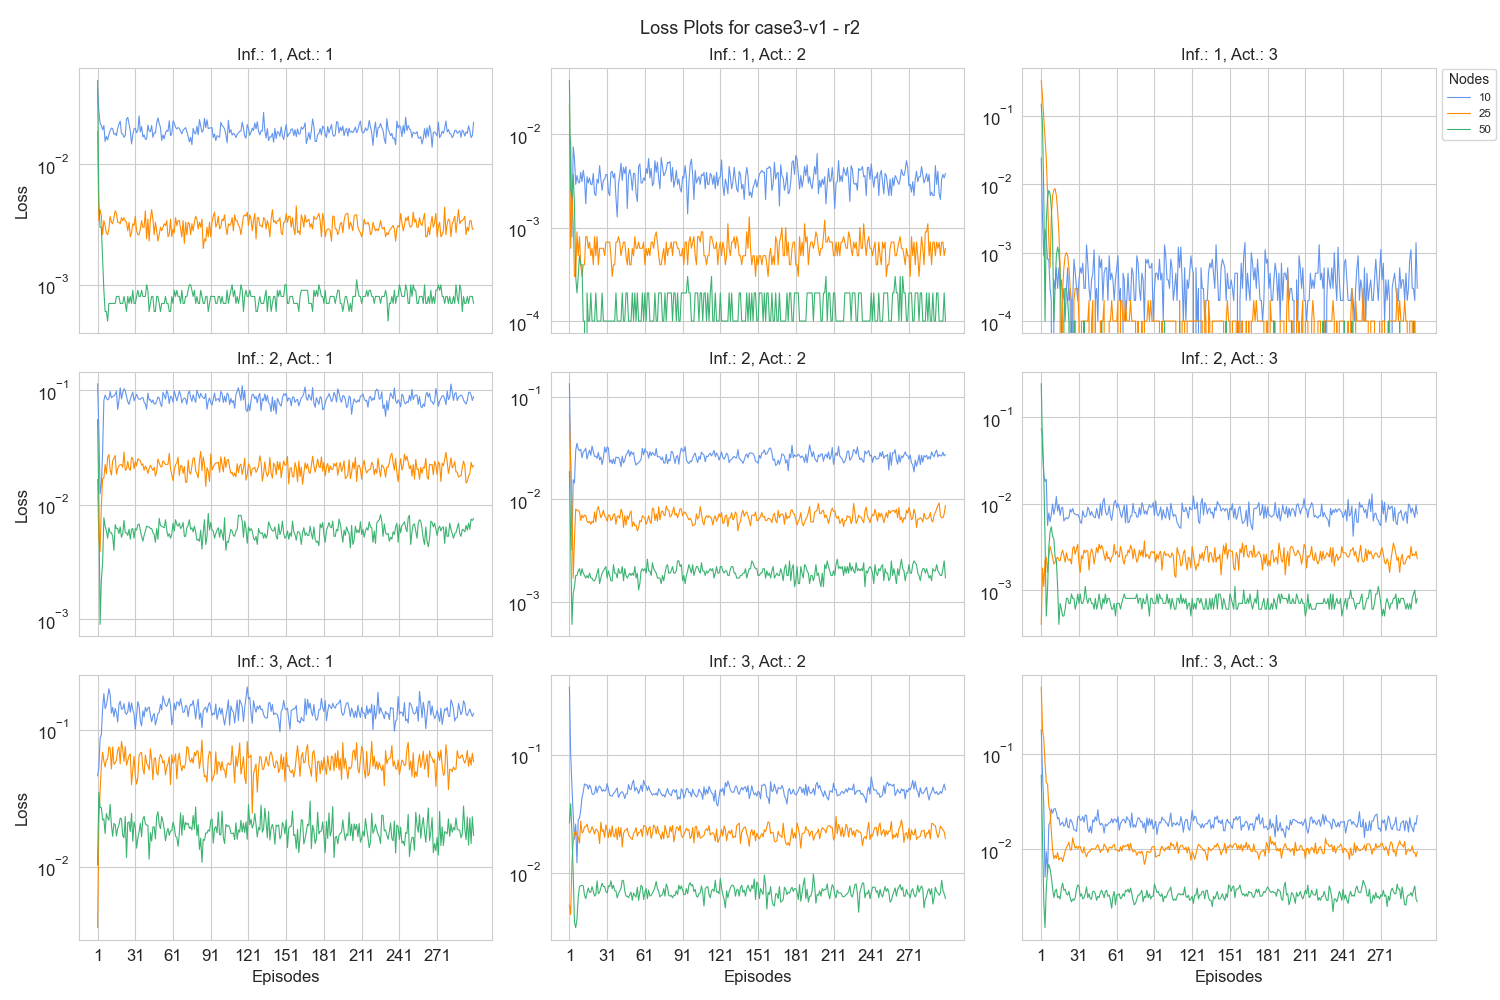}
    \caption{Case-3 v1 using R2: Training MSE loss evolution for RL policy using ResNet model across networks of 10 (blue), 25 (orange), and 50 (green) nodes, for varying initial misinformation sources (Inf.) and action budgets (Act.). Plotted on a logarithmic scale, the loss decreases over episodes, indicating improved policy performance and adaptation across network sizes.}
    \label{fig:resnet_c3v1r2_loss}
\end{figure}

\begin{figure}
    \centering
    \includegraphics[scale=0.34]{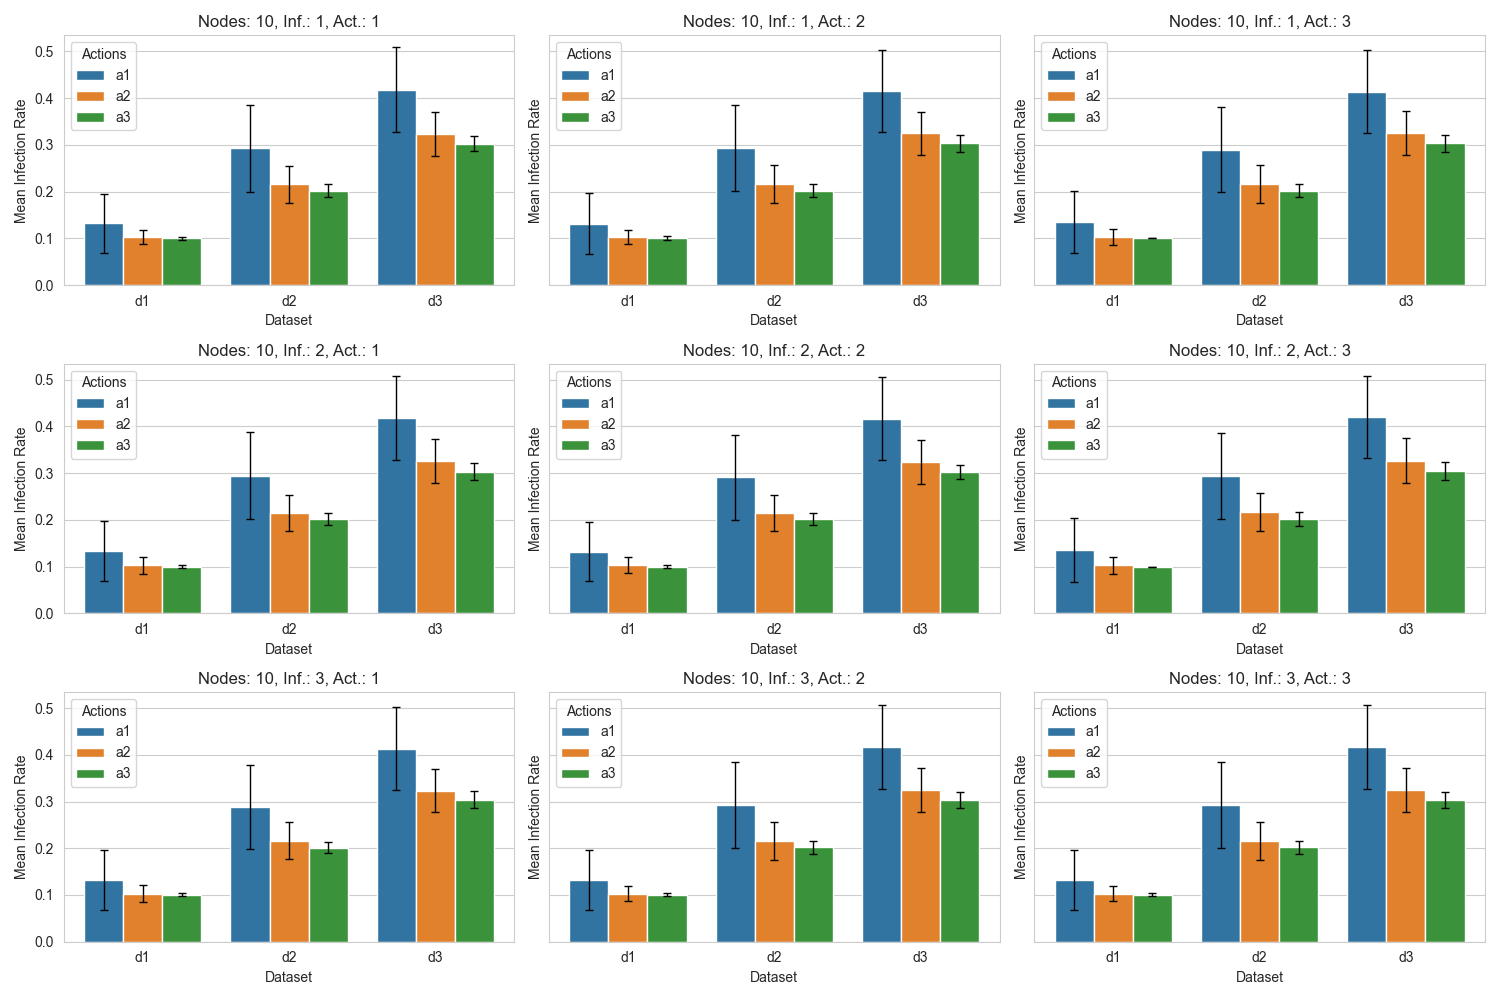}
    \caption{Case-3 v1 using R2: Performance comparison of the RL policies trained using ResNet model for a 10-node network. The barplot displays the mean infection rate for datasets d1, d2, and d3 of Dataset v1 type, differentiated by the number of initial misinformation sources (Inf.) and action budgets (Act.: a1, a2, a3). Each subplot illustrates the performance of a policy trained with the parameters indicated in its title. Lower infection rates indicate more effective policy learning and misinformation containment.}
    \label{fig:inf_resnet_c3v1r2_10}
\end{figure}

\begin{figure}
    \centering
    \includegraphics[scale=0.34]{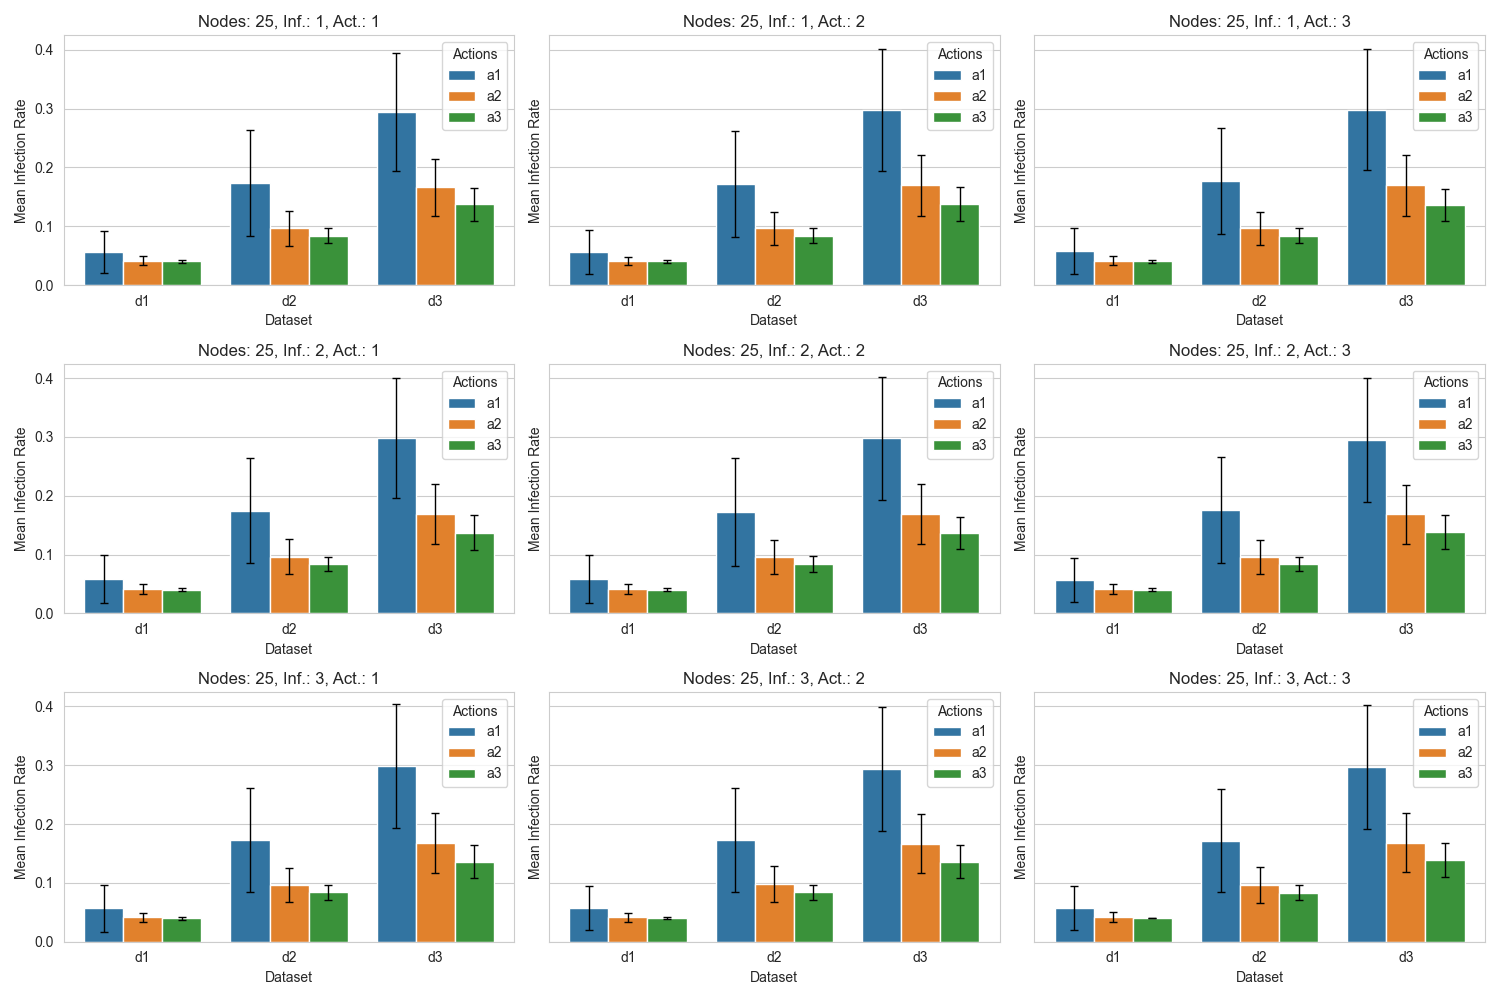}
    \caption{Case-3 v1 using R2: Performance comparison of the RL policies trained using ResNet model for a 25-node network. The barplot displays the mean infection rate for datasets d1, d2, and d3 of Dataset v1 type, differentiated by the number of initial misinformation sources (Inf.) and action budgets (Act.: a1, a2, a3). Each subplot illustrates the performance of a policy trained with the parameters indicated in its title. Lower infection rates indicate more effective policy learning and misinformation containment.}
    \label{fig:inf_resnet_c3v1r2_25}
\end{figure}

\begin{figure}
    \centering
    \includegraphics[scale=0.34]{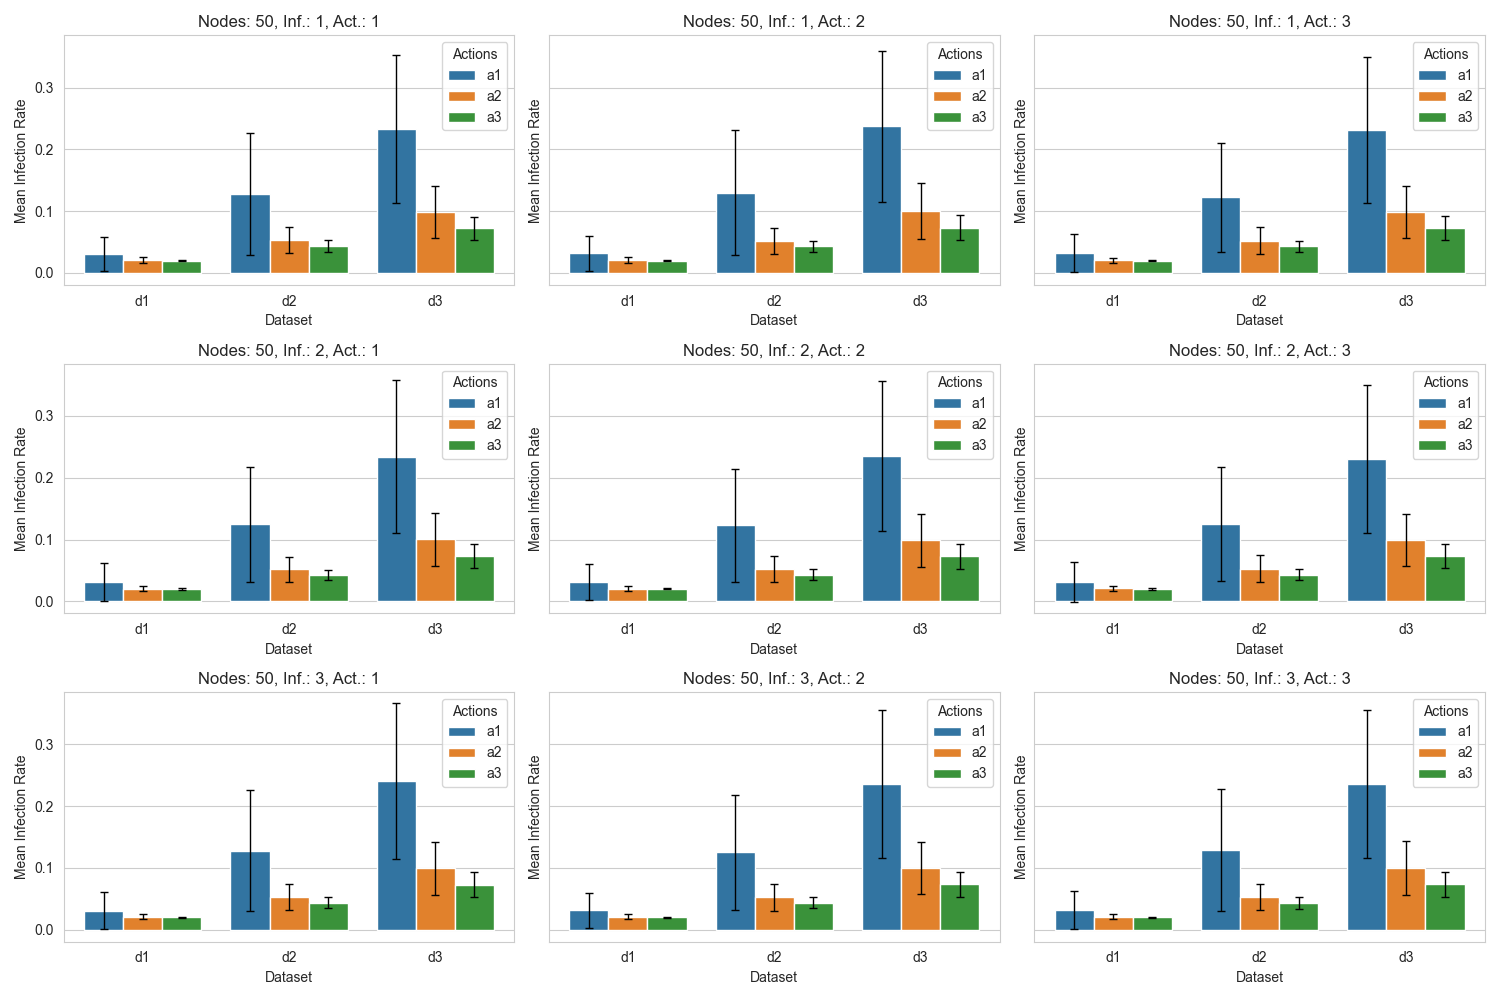}
    \caption{Case-3 v1 using R2: Performance comparison of the RL policies trained using ResNet model for a 50-node network. The barplot displays the mean infection rate for datasets d1, d2, and d3 of Dataset v1 type, differentiated by the number of initial misinformation sources (Inf.) and action budgets (Act.: a1, a2, a3). Each subplot illustrates the performance of a policy trained with the parameters indicated in its title. Lower infection rates indicate more effective policy learning and misinformation containment.}
    \label{fig:inf_resnet_c3v1r2_50}
\end{figure}

%%%%%% R3 %%%%%%%
\begin{figure}[!h]
    \centering
    \includegraphics[scale=0.34]{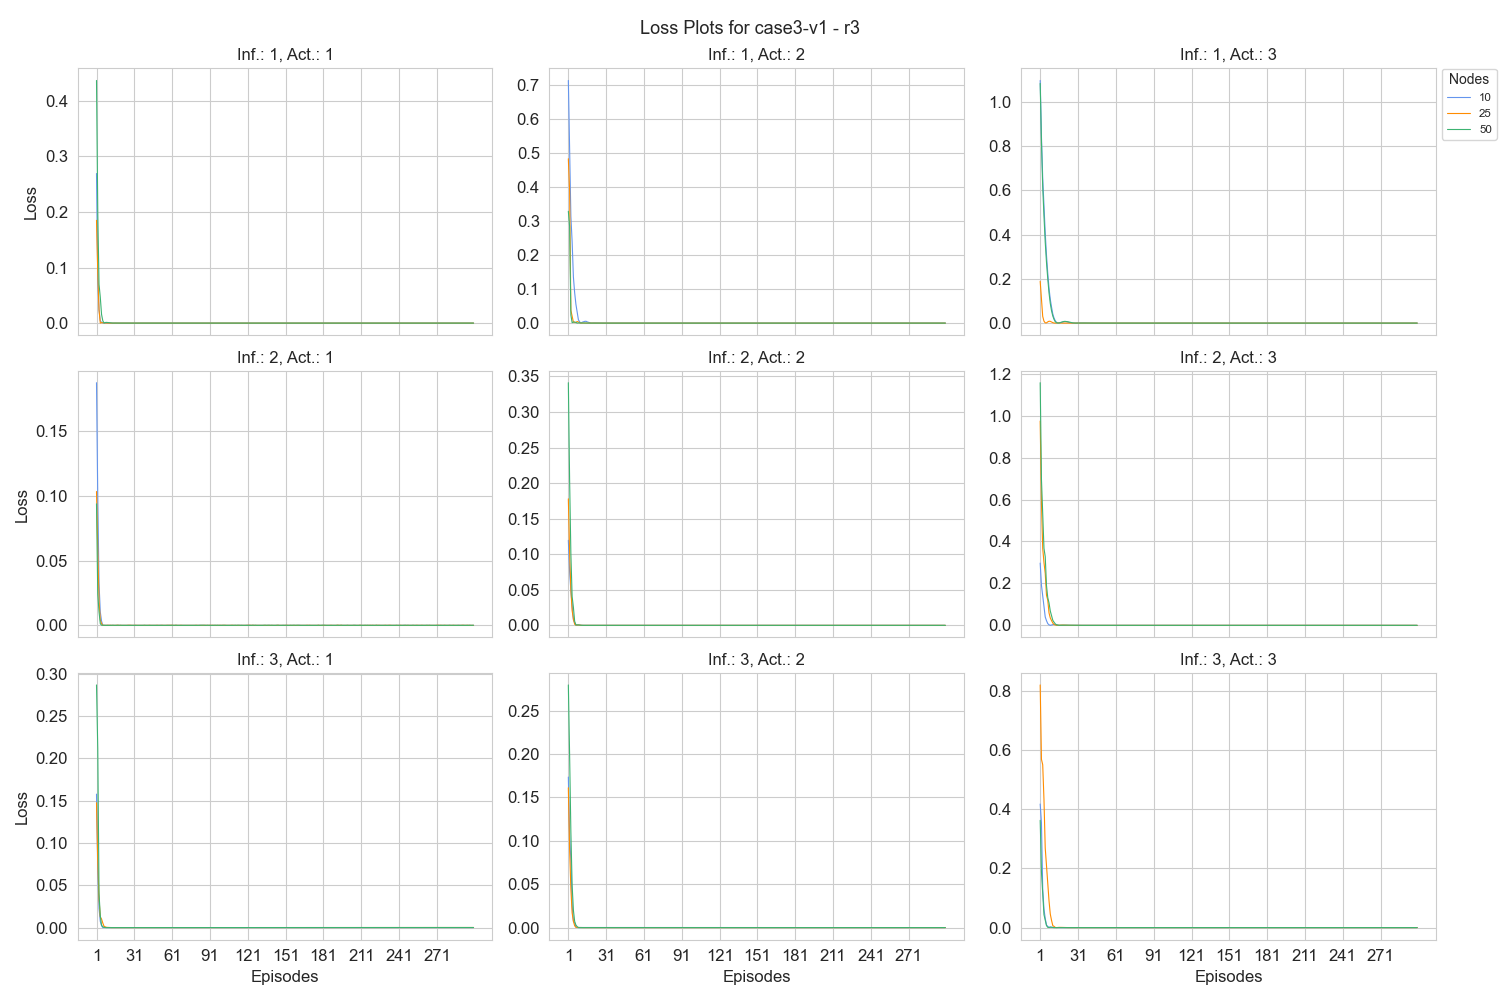}
    \caption{Case-3 v1 using R3: Training MSE loss evolution for RL policy using ResNet model across networks of 10 (blue), 25 (orange), and 50 (green) nodes, for varying initial misinformation sources (Inf.) and action budgets (Act.). The loss decreases over episodes, indicating improved policy performance and adaptation across network sizes.}
    \label{fig:resnet_c3v1r3_loss}
\end{figure}

\begin{figure}
    \centering
    \includegraphics[scale=0.34]{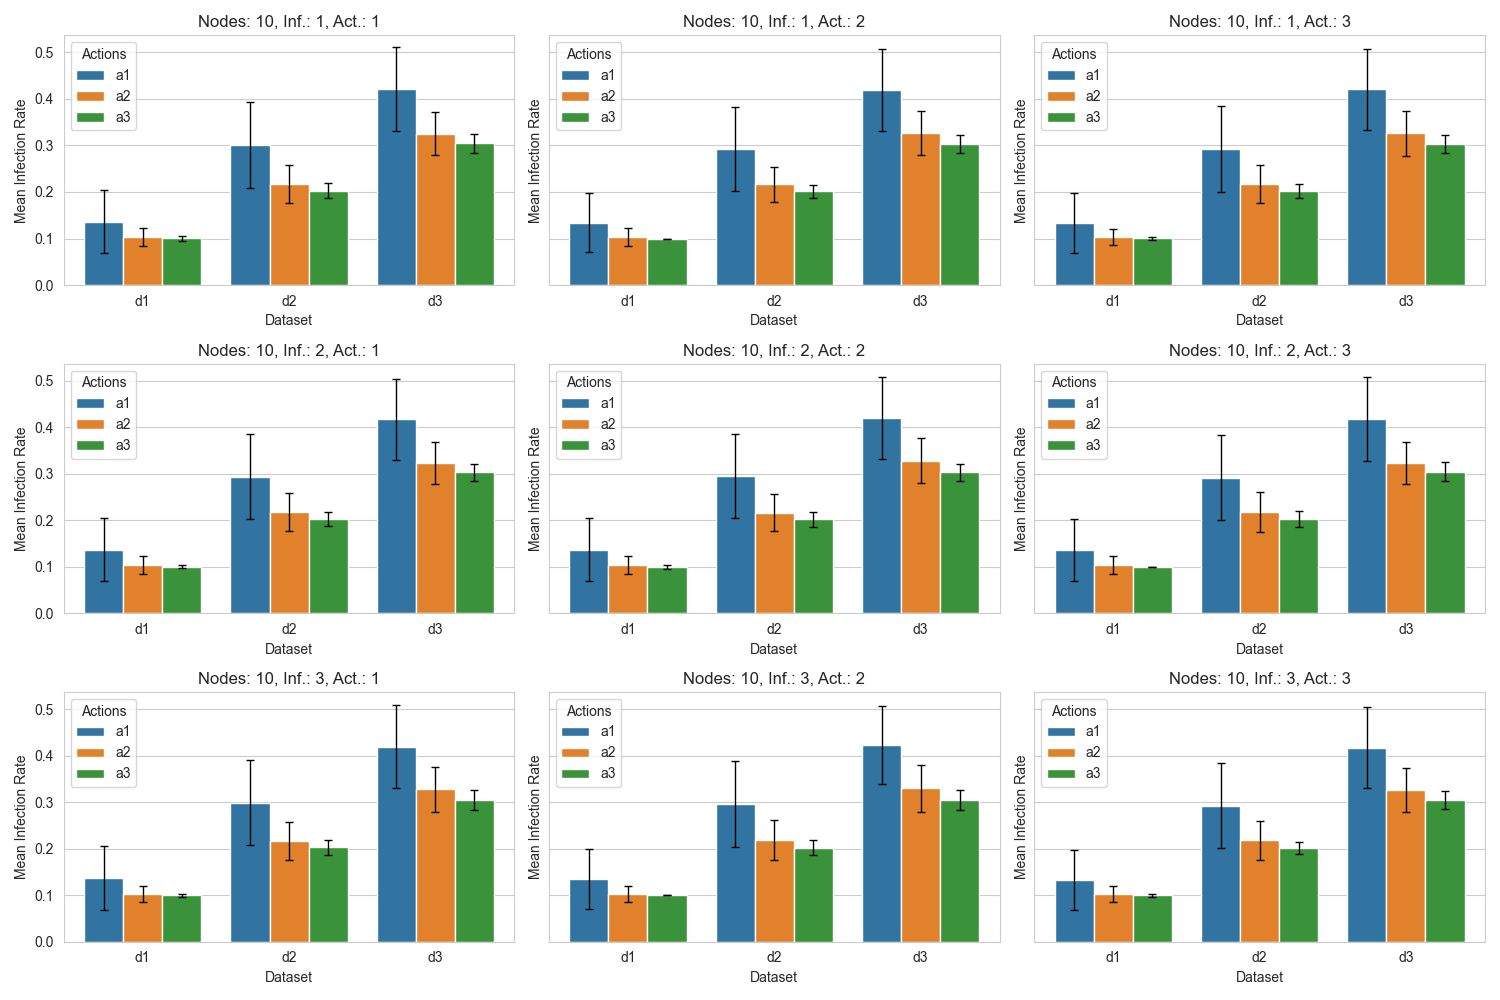}
    \caption{Case-3 v1 using R3: Performance comparison of the RL policies trained using ResNet model for a 10-node network. The barplot displays the mean infection rate for datasets d1, d2, and d3 of Dataset v1 type, differentiated by the number of initial misinformation sources (Inf.) and action budgets (Act.: a1, a2, a3). Each subplot illustrates the performance of a policy trained with the parameters indicated in its title. Lower infection rates indicate more effective policy learning and misinformation containment.}
    \label{fig:inf_resnet_c3v1r3_10}
\end{figure}

\begin{figure}
    \centering
    \includegraphics[scale=0.34]{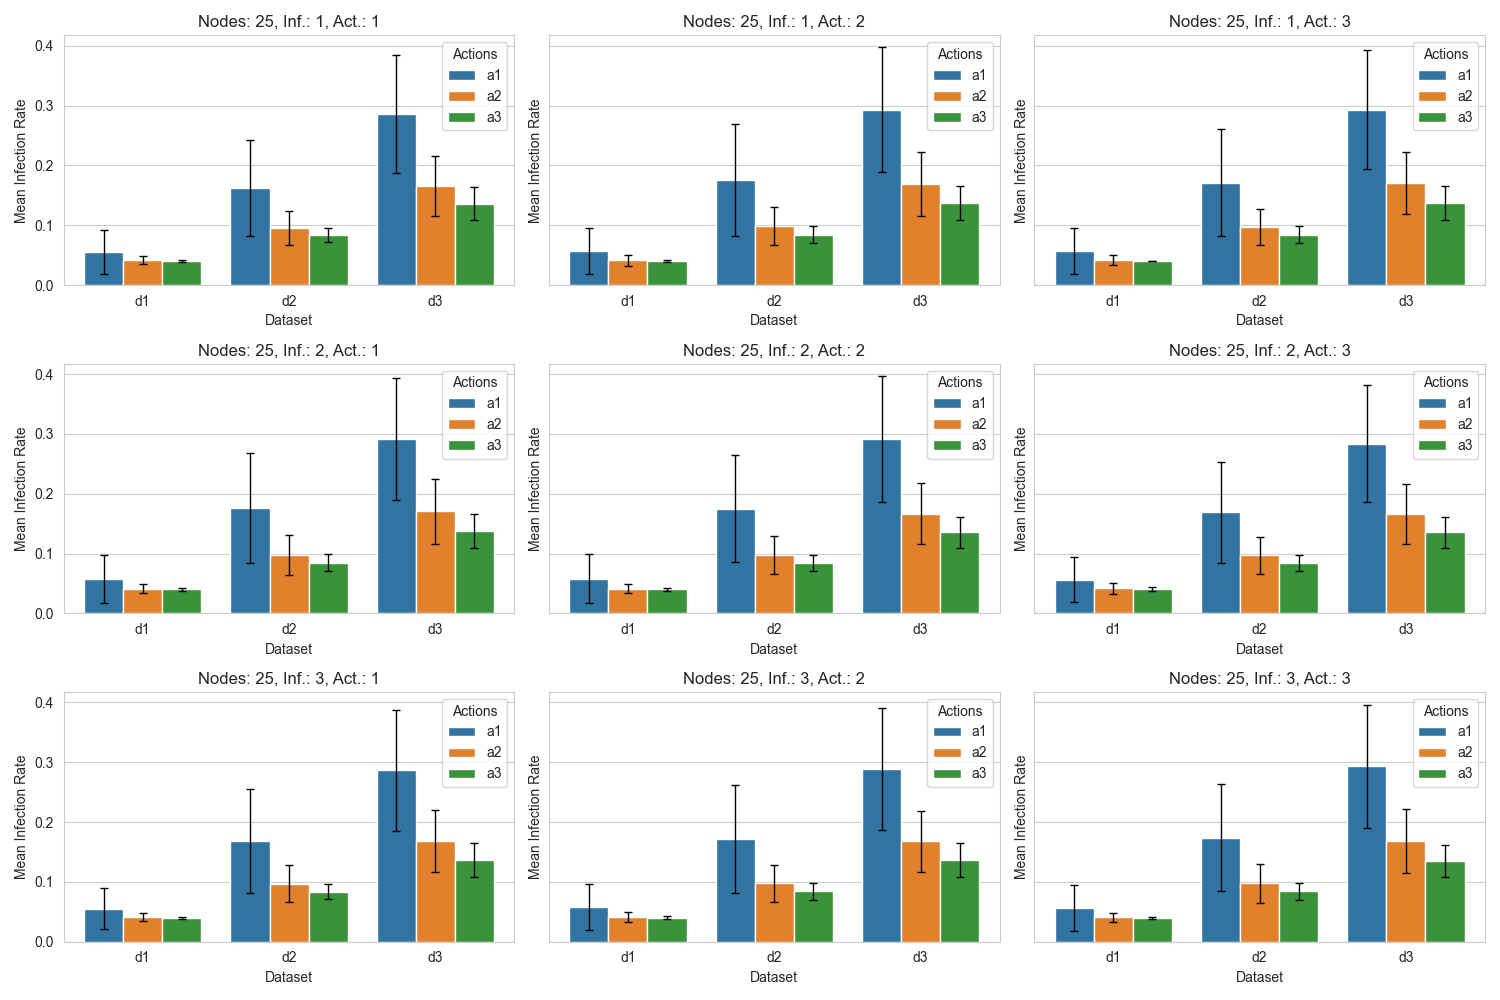}
    \caption{Case-3 v1 using R3: Performance comparison of the RL policies trained using ResNet model for a 25-node network. The barplot displays the mean infection rate for datasets d1, d2, and d3 of Dataset v1 type, differentiated by the number of initial misinformation sources (Inf.) and action budgets (Act.: a1, a2, a3). Each subplot illustrates the performance of a policy trained with the parameters indicated in its title. Lower infection rates indicate more effective policy learning and misinformation containment.}
    \label{fig:inf_resnet_c3v1r3_25}
\end{figure}

\begin{figure}
    \centering
    \includegraphics[scale=0.34]{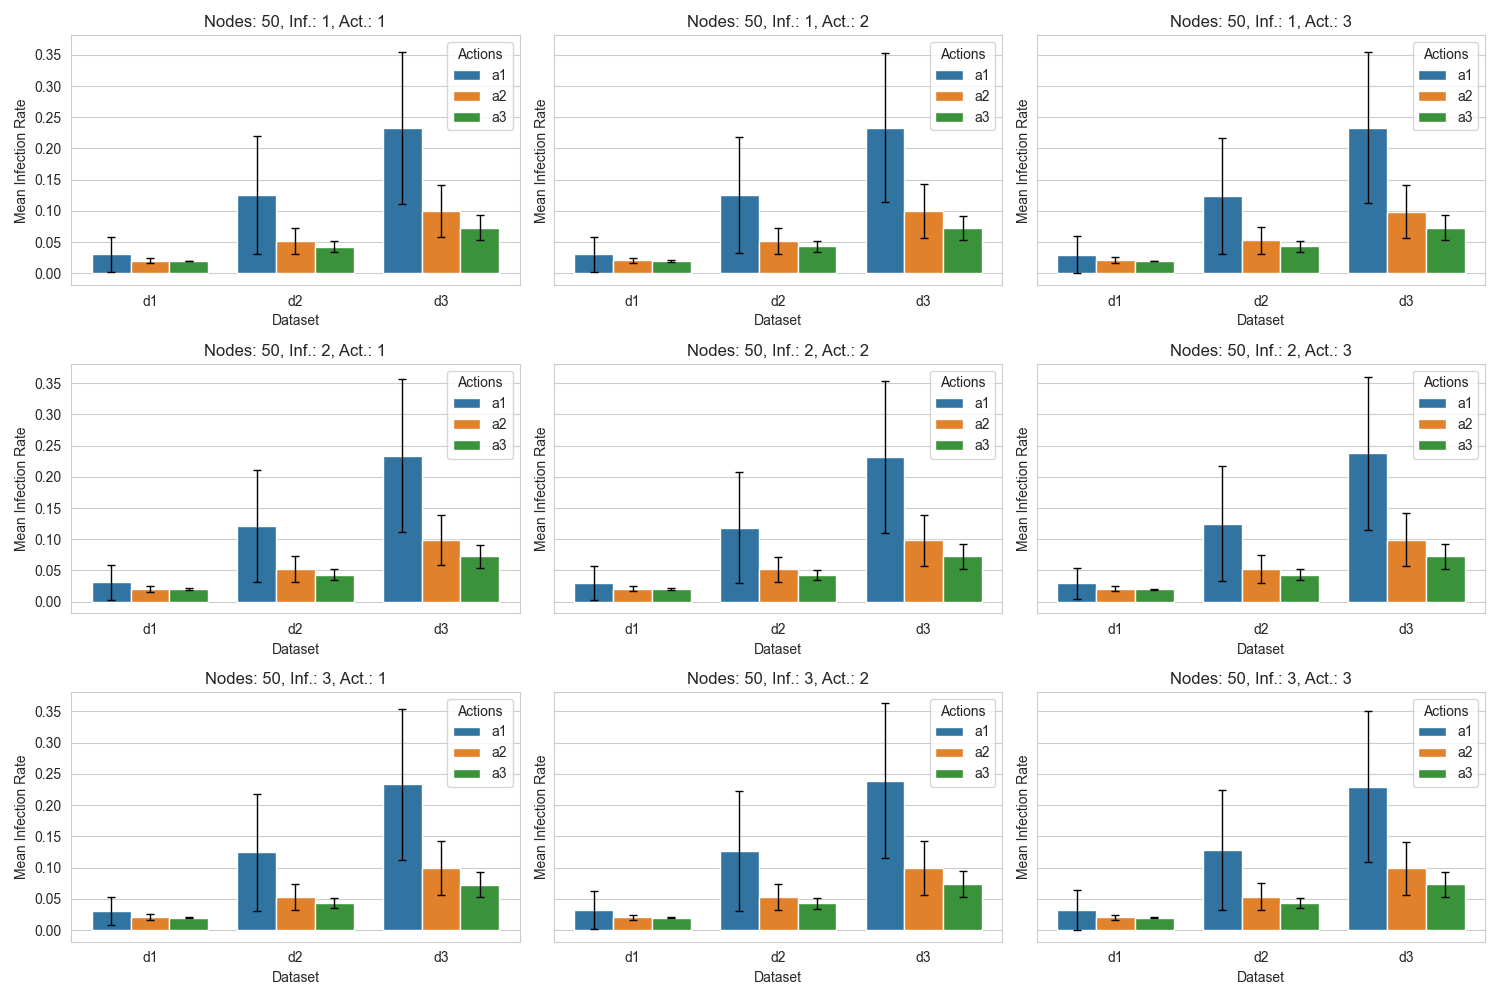}
    \caption{Case-3 v1 using R3: Performance comparison of the RL policies trained using ResNet model for a 50-node network. The barplot displays the mean infection rate for datasets d1, d2, and d3 of Dataset v1 type, differentiated by the number of initial misinformation sources (Inf.) and action budgets (Act.: a1, a2, a3). Each subplot illustrates the performance of a policy trained with the parameters indicated in its title. Lower infection rates indicate more effective policy learning and misinformation containment.}
    \label{fig:inf_resnet_c3v1r3_50}
\end{figure}

%%%%%% R4 %%%%%%%
\begin{figure}[!h]
    \centering
    \includegraphics[scale=0.34]{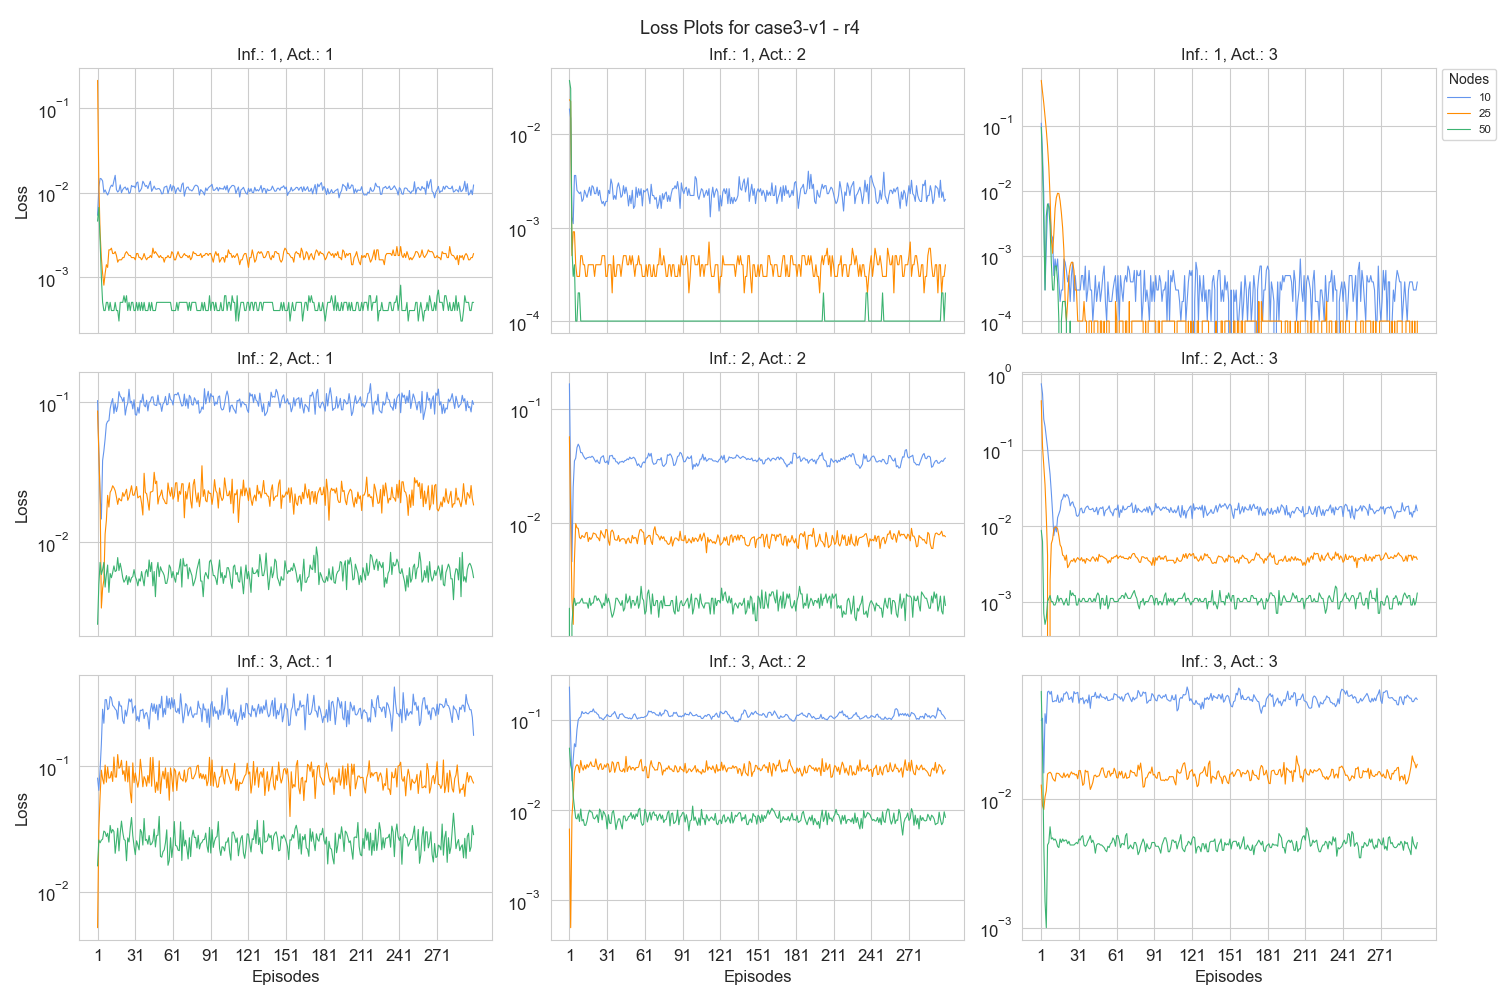}
    \caption{Case-3 v1 using R4: Training MSE loss evolution for RL policy using ResNet model across networks of 10 (blue), 25 (orange), and 50 (green) nodes, for varying initial misinformation sources (Inf.) and action budgets (Act.). Plotted on a logarithmic scale, the loss decreases over episodes, indicating improved policy performance and adaptation across network sizes.}
    \label{fig:resnet_c3v1r4_loss}
\end{figure}

\begin{figure}
    \centering
    \includegraphics[scale=0.34]{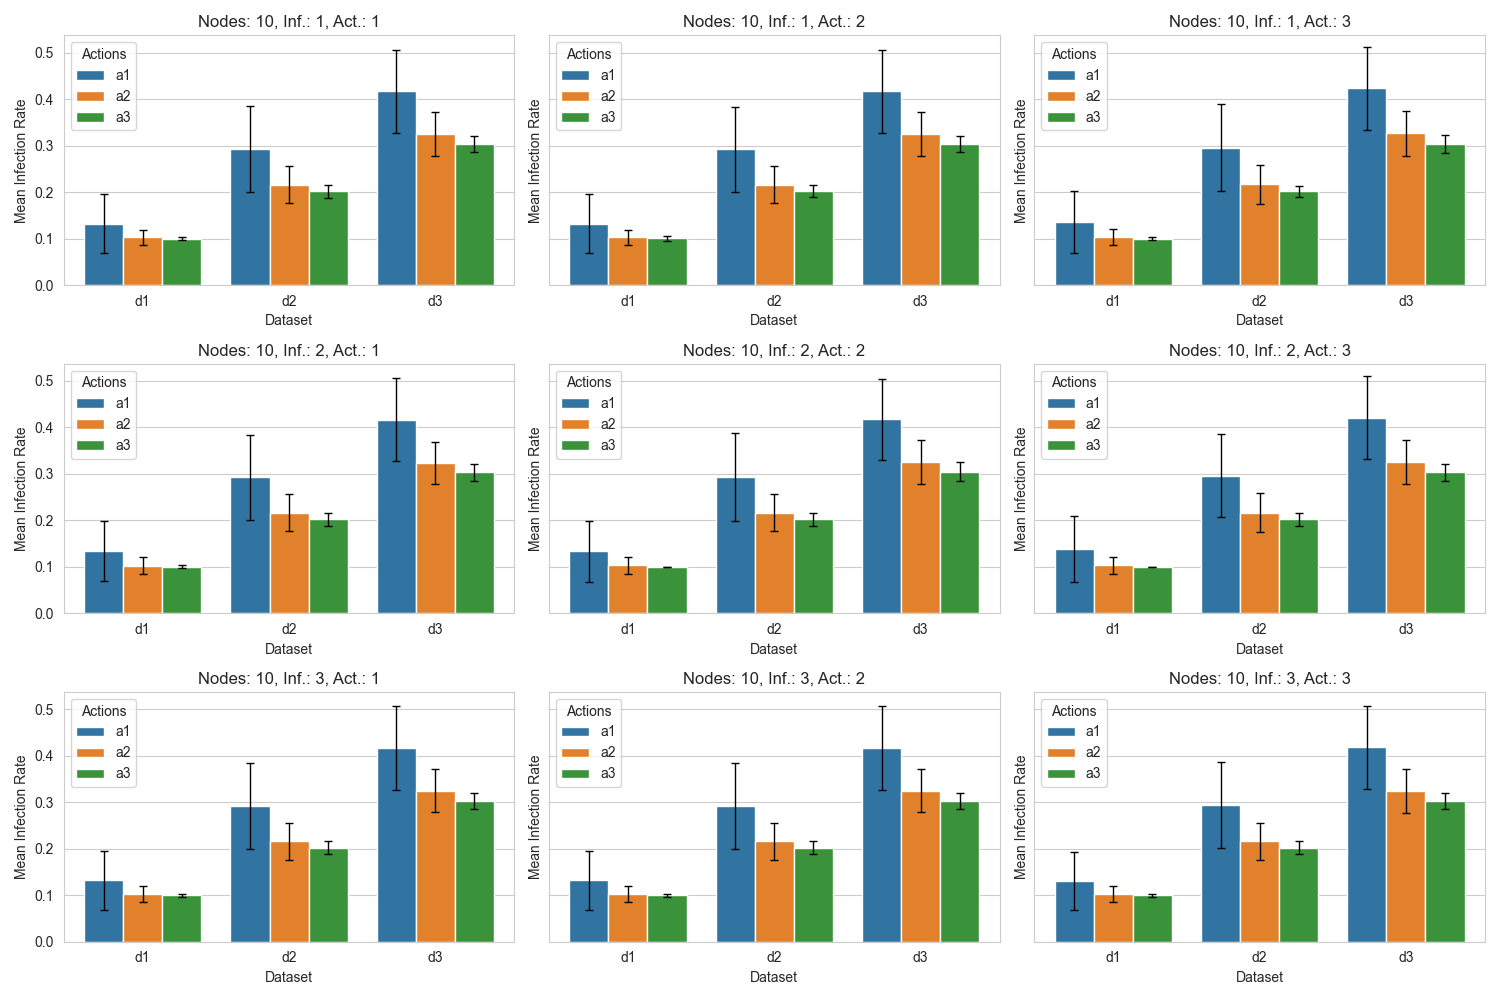}
    \caption{Case-3 v1 using R4: Performance comparison of the RL policies trained using ResNet model for a 10-node network. The barplot displays the mean infection rate for datasets d1, d2, and d3 of Dataset v1 type, differentiated by the number of initial misinformation sources (Inf.) and action budgets (Act.: a1, a2, a3). Each subplot illustrates the performance of a policy trained with the parameters indicated in its title. Lower infection rates indicate more effective policy learning and misinformation containment.}
    \label{fig:inf_resnet_c3v1r4_10}
\end{figure}

\begin{figure}
    \centering
    \includegraphics[scale=0.34]{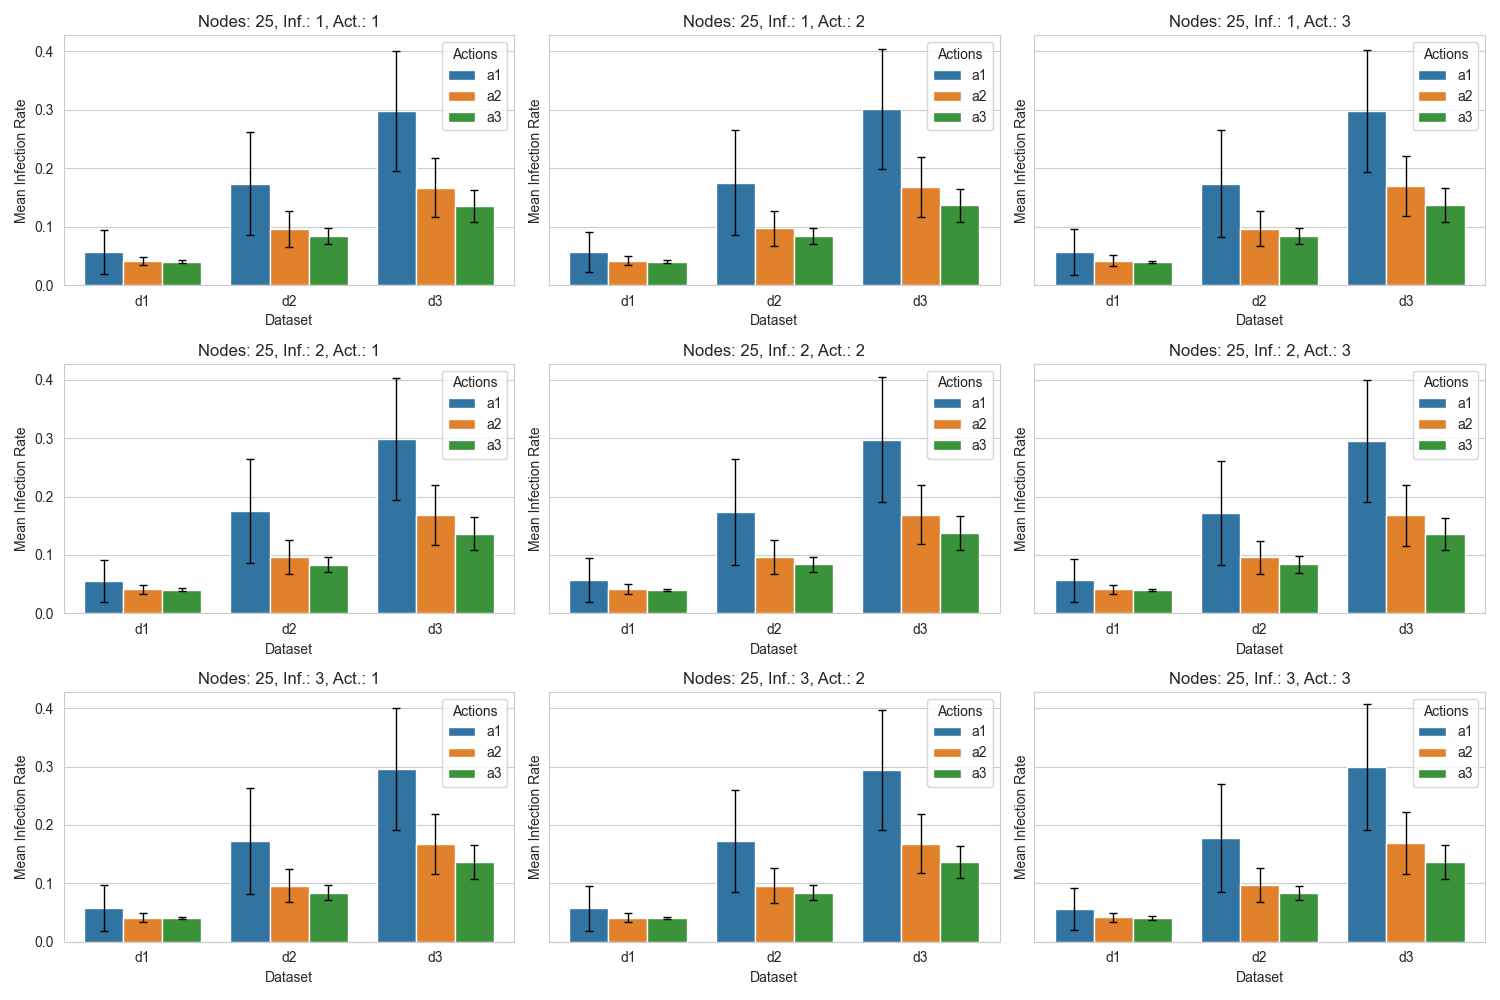}
    \caption{Case-3 v1 using R4: Performance comparison of the RL policies trained using ResNet model for a 25-node network. The barplot displays the mean infection rate for datasets d1, d2, and d3 of Dataset v1 type, differentiated by the number of initial misinformation sources (Inf.) and action budgets (Act.: a1, a2, a3). Each subplot illustrates the performance of a policy trained with the parameters indicated in its title. Lower infection rates indicate more effective policy learning and misinformation containment.}
    \label{fig:inf_resnet_c3v1r4_25}
\end{figure}

\begin{figure}
    \centering
    \includegraphics[scale=0.34]{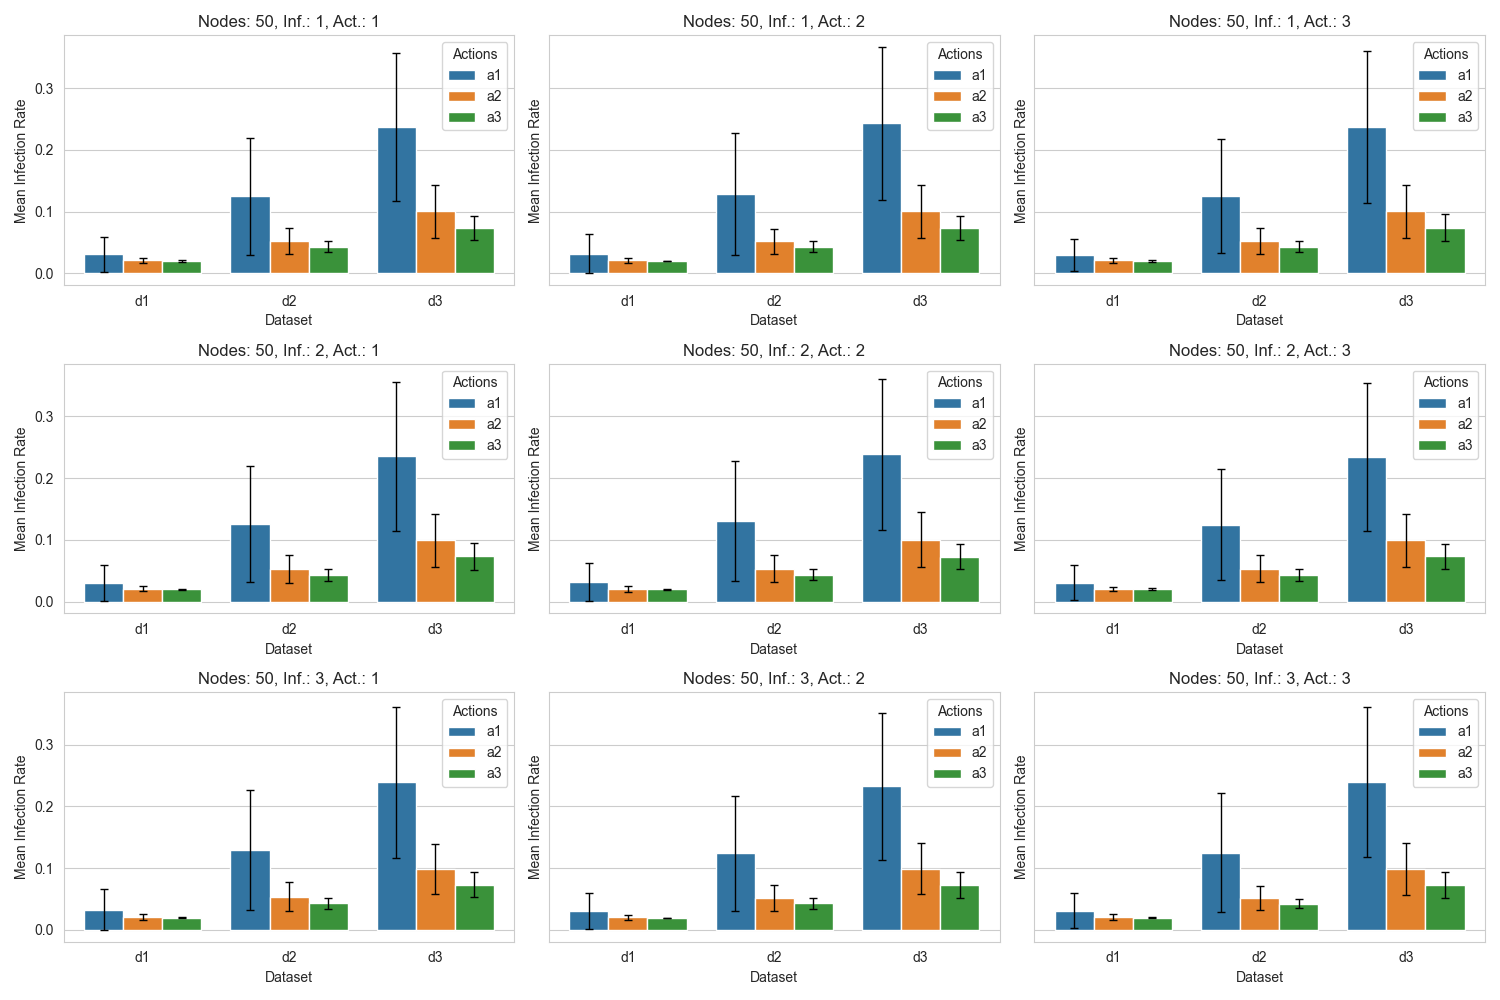}
    \caption{Case-3 v1 using R4: Performance comparison of the RL policies trained using ResNet model for a 50-node network. The barplot displays the mean infection rate for datasets d1, d2, and d3 of Dataset v1 type, differentiated by the number of initial misinformation sources (Inf.) and action budgets (Act.: a1, a2, a3). Each subplot illustrates the performance of a policy trained with the parameters indicated in its title. Lower infection rates indicate more effective policy learning and misinformation containment.}
    \label{fig:inf_resnet_c3v1r4_50}
\end{figure}

% #############################################

% ##################### GCN Figures ######################

%###### Case 1 GCN Figures #######
\begin{figure}[!h]
    \centering
    \includegraphics[scale=0.34]{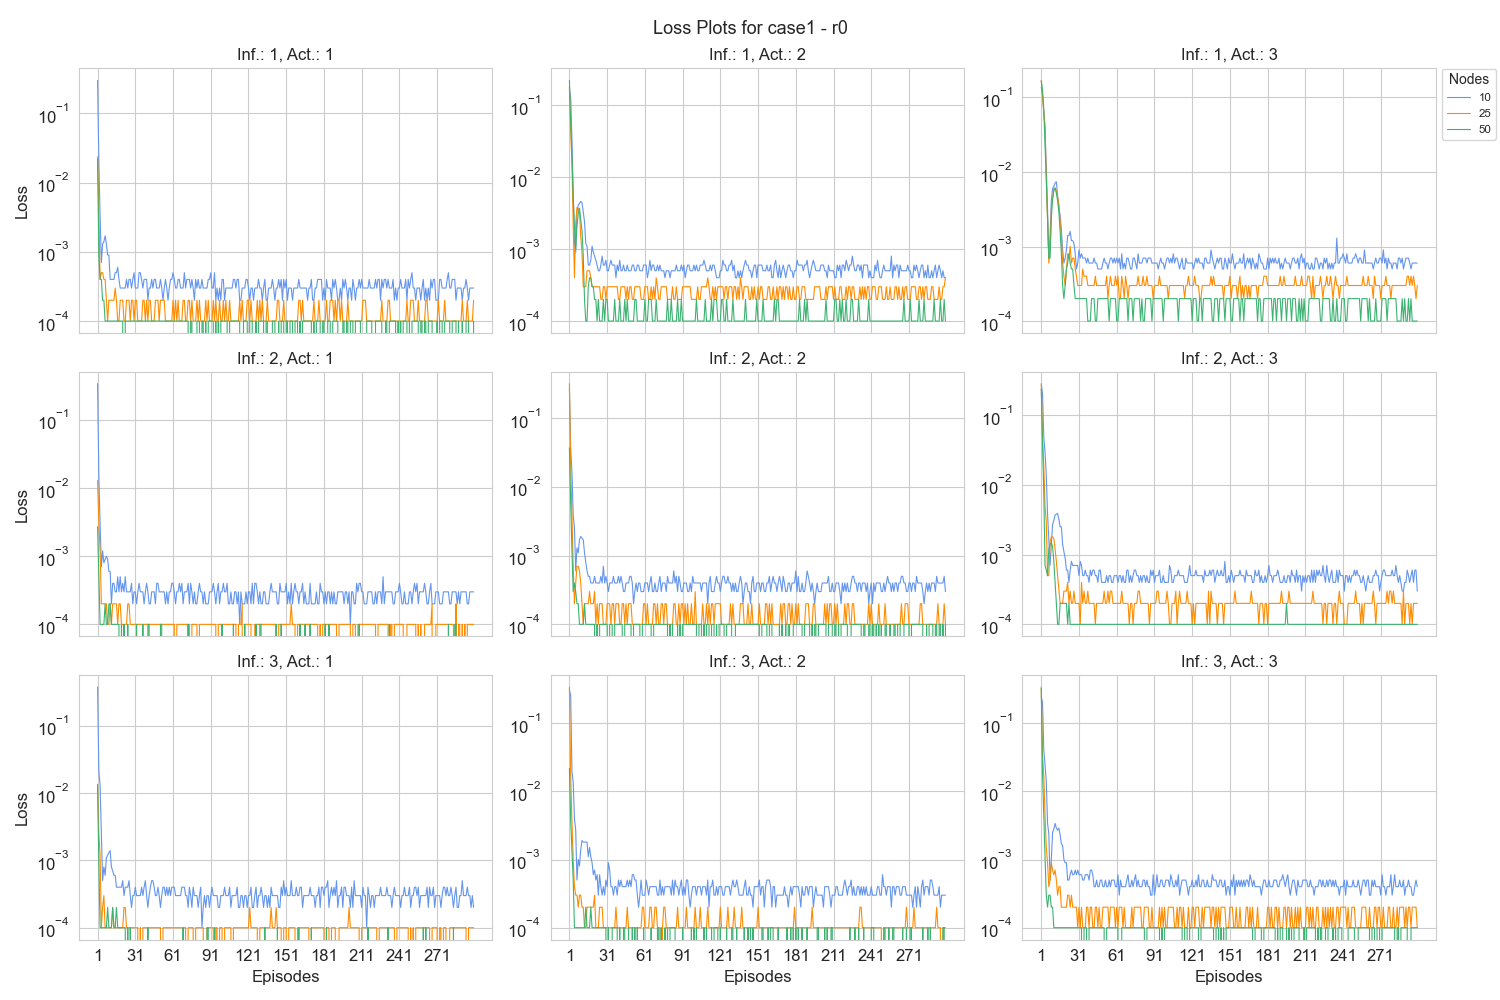}
    \caption{Case-1 using R0: Training MSE loss evolution for RL policy using GCN model across networks of 10 (blue), 25 (orange), and 50 (green) nodes, for varying initial misinformation sources (Inf.) and action budgets (Act.). Plotted on a logarithmic scale, the loss decreases over episodes, indicating improved policy performance and adaptation across network sizes.}
    \label{fig:gcn_c1r0_loss}
\end{figure}

\begin{figure}[!h]
    \centering
    \includegraphics[scale=0.34]{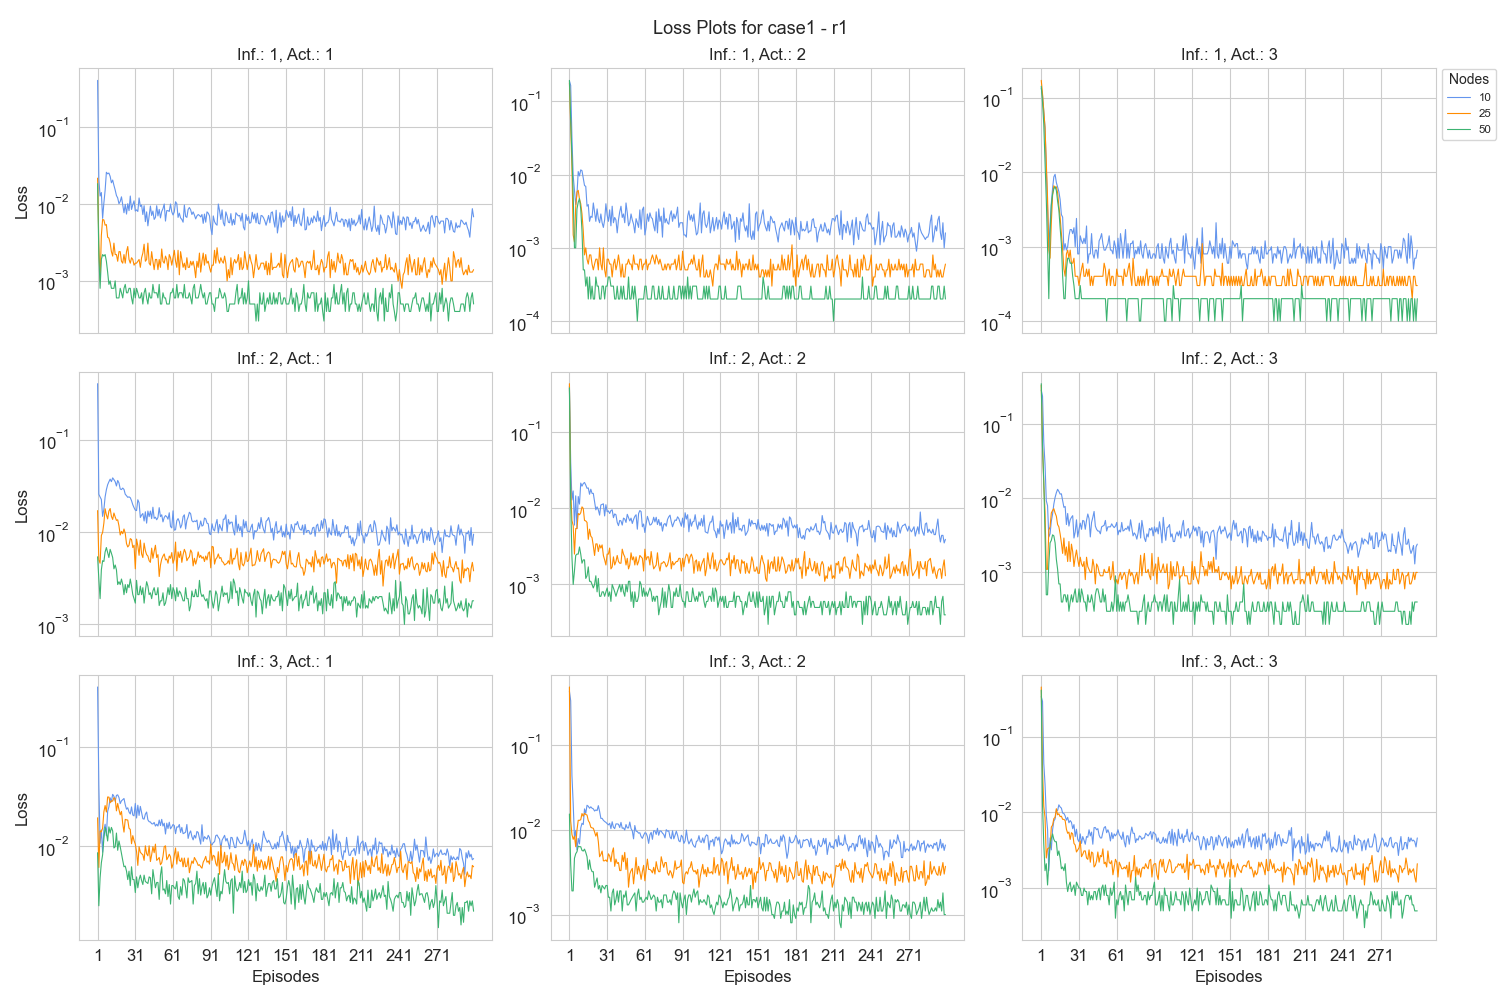}
    \caption{Case-1 using R1: Training MSE loss evolution for RL policy using GCN model across networks of 10 (blue), 25 (orange), and 50 (green) nodes, for varying initial misinformation sources (Inf.) and action budgets (Act.). Plotted on a logarithmic scale, the loss decreases over episodes, indicating improved policy performance and adaptation across network sizes.}
    \label{fig:gcn_c1r1_loss}
\end{figure}

\begin{figure}[!h]
    \centering
    \includegraphics[scale=0.34]{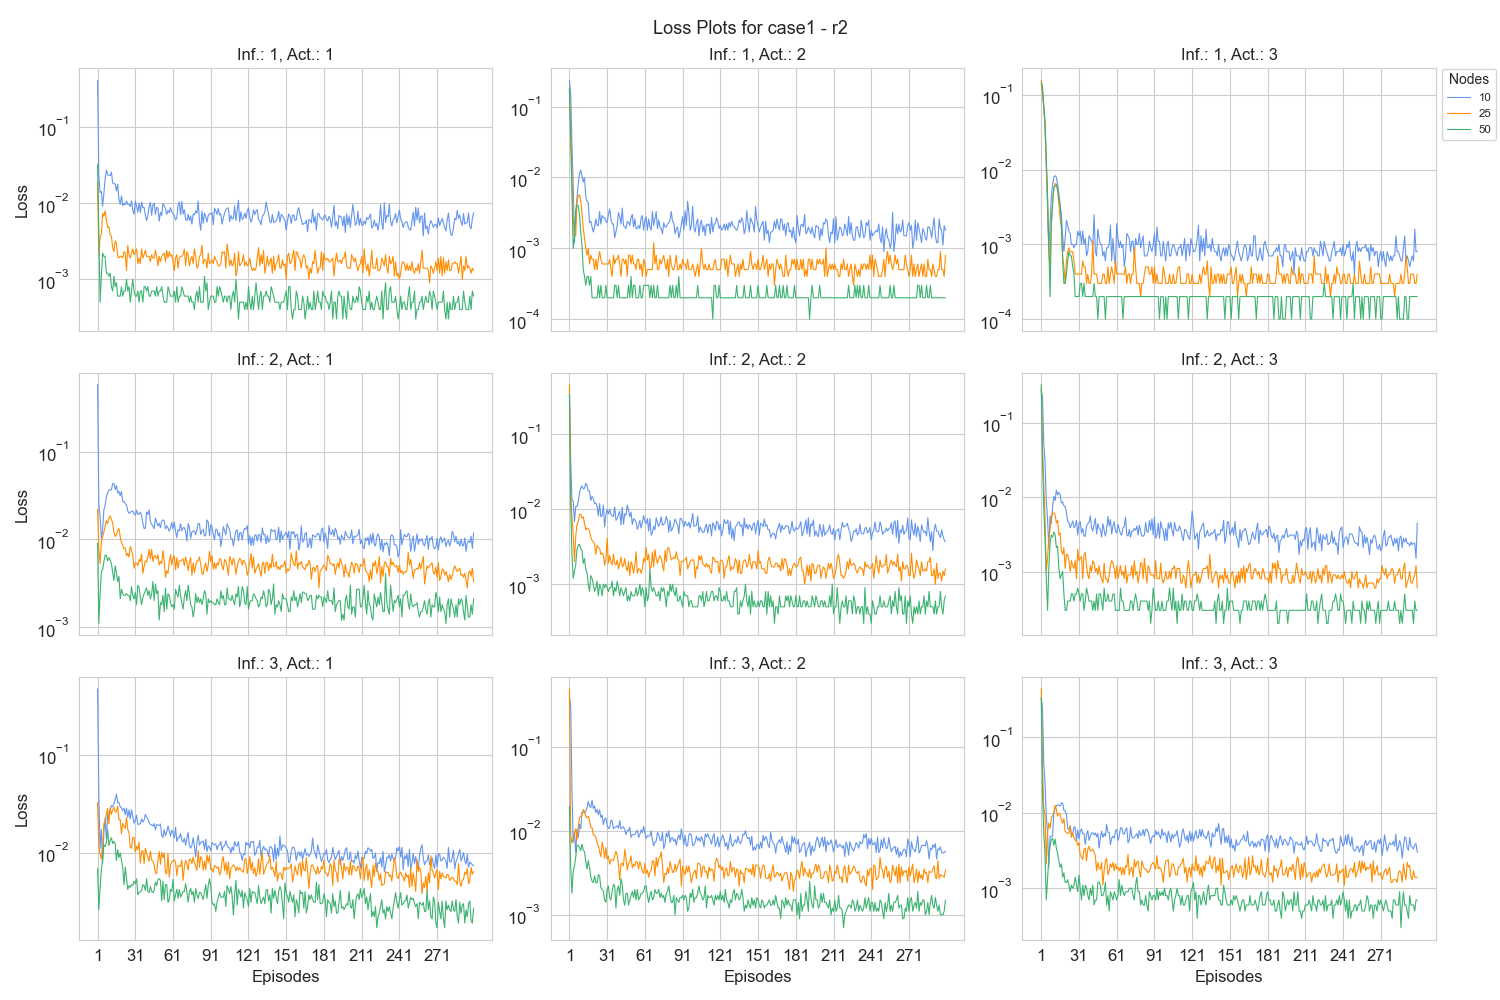}
    \caption{Case-1 using R2: Training MSE loss evolution for RL policy using GCN model across networks of 10 (blue), 25 (orange), and 50 (green) nodes, for varying initial misinformation sources (Inf.) and action budgets (Act.). Plotted on a logarithmic scale, the loss decreases over episodes, indicating improved policy performance and adaptation across network sizes.}
    \label{fig:gcn_c1r2_loss}
\end{figure}

\begin{figure}[!h]
    \centering
    \includegraphics[scale=0.34]{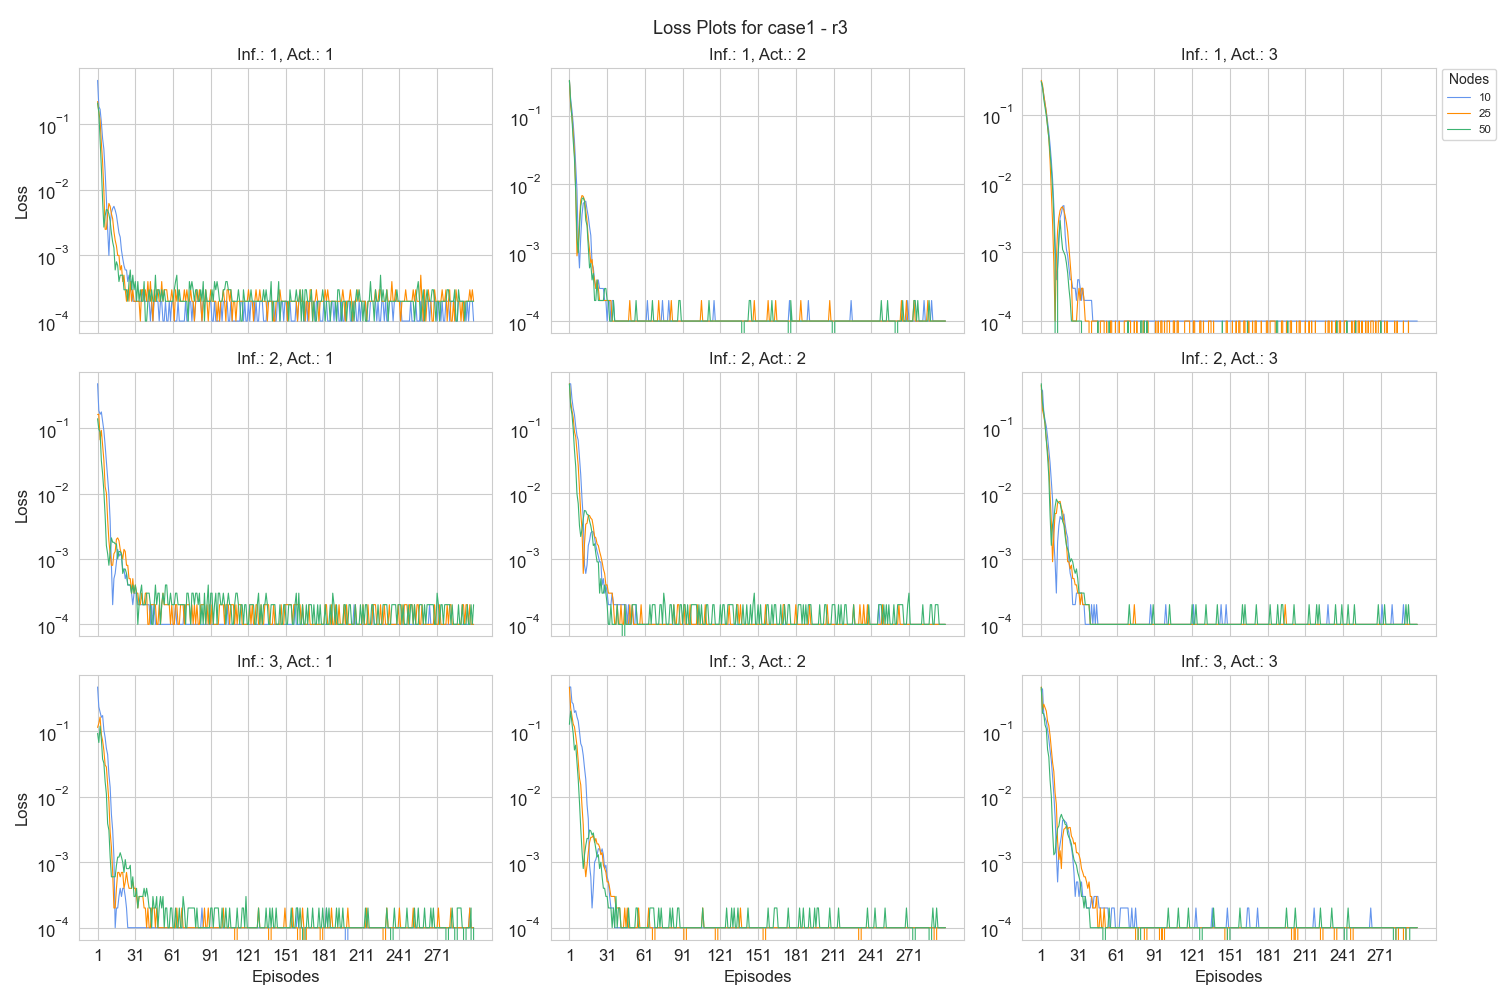}
    \caption{Case-1 using R3: Training MSE loss evolution for RL policy using GCN model across networks of 10 (blue), 25 (orange), and 50 (green) nodes, for varying initial misinformation sources (Inf.) and action budgets (Act.). Plotted on a logarithmic scale, the loss decreases over episodes, indicating improved policy performance and adaptation across network sizes.}
    \label{fig:gcn_c1r3_loss}
\end{figure}

\begin{figure}[!h]
    \centering
    \includegraphics[scale=0.34]{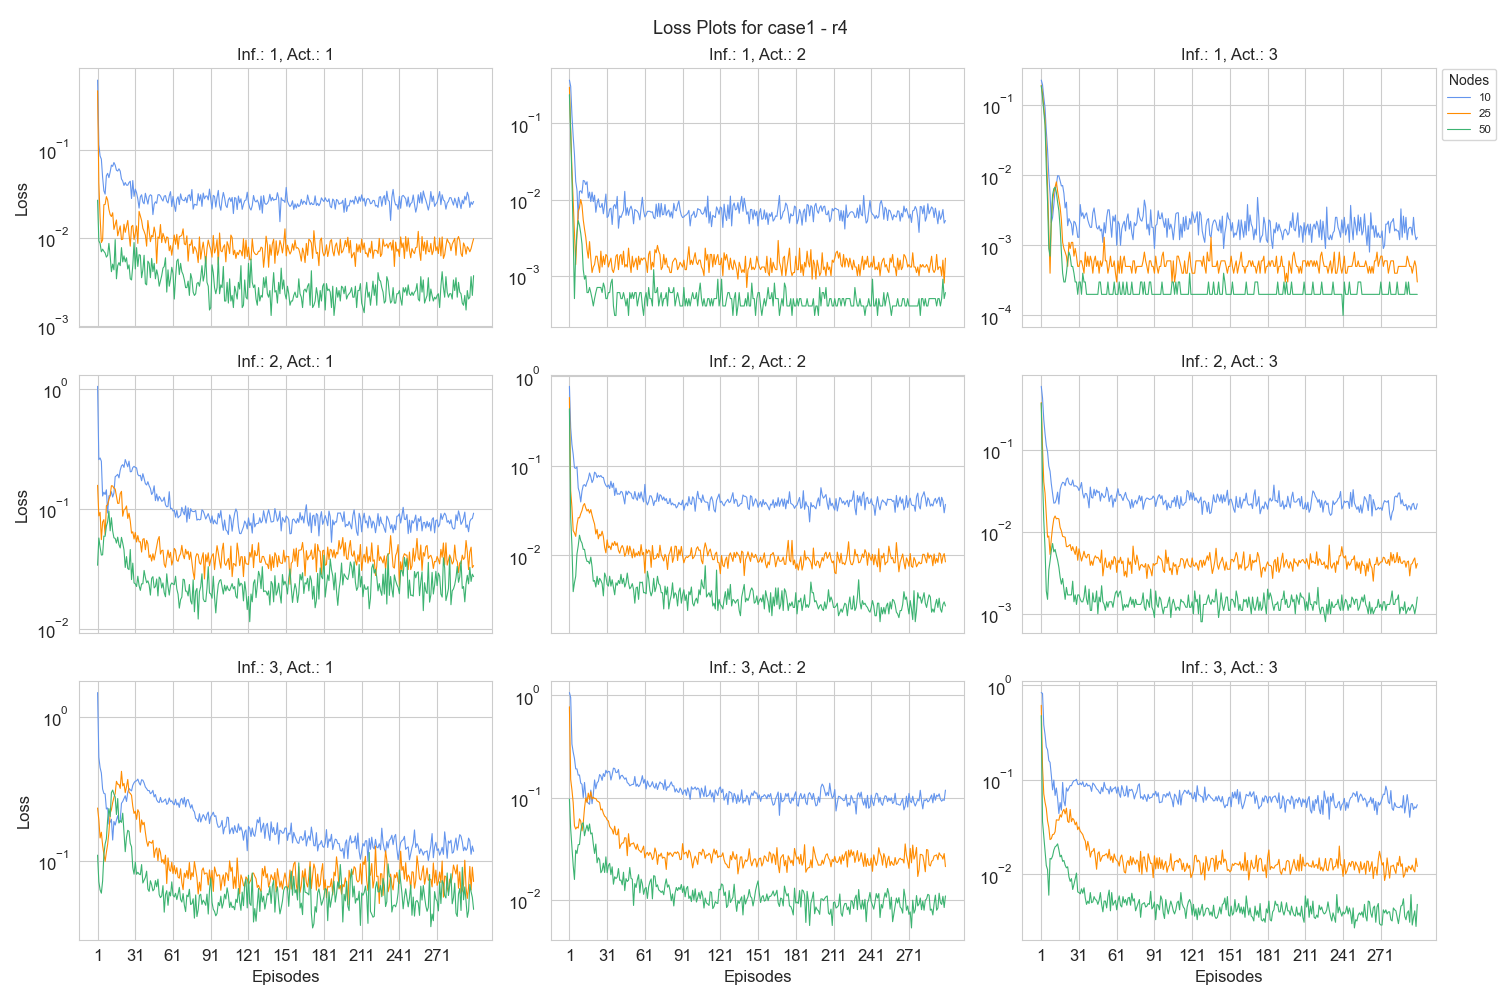}
    \caption{Case-1 using R4: Training MSE loss evolution for RL policy using GCN model across networks of 10 (blue), 25 (orange), and 50 (green) nodes, for varying initial misinformation sources (Inf.) and action budgets (Act.). Plotted on a logarithmic scale, the loss decreases over episodes, indicating improved policy performance and adaptation across network sizes.}
    \label{fig:gcn_c1r4_loss}
\end{figure}

%###########################

%###### Case 2 GCN Figures #######
\begin{figure}[!h]
    \centering
    \includegraphics[scale=0.34]{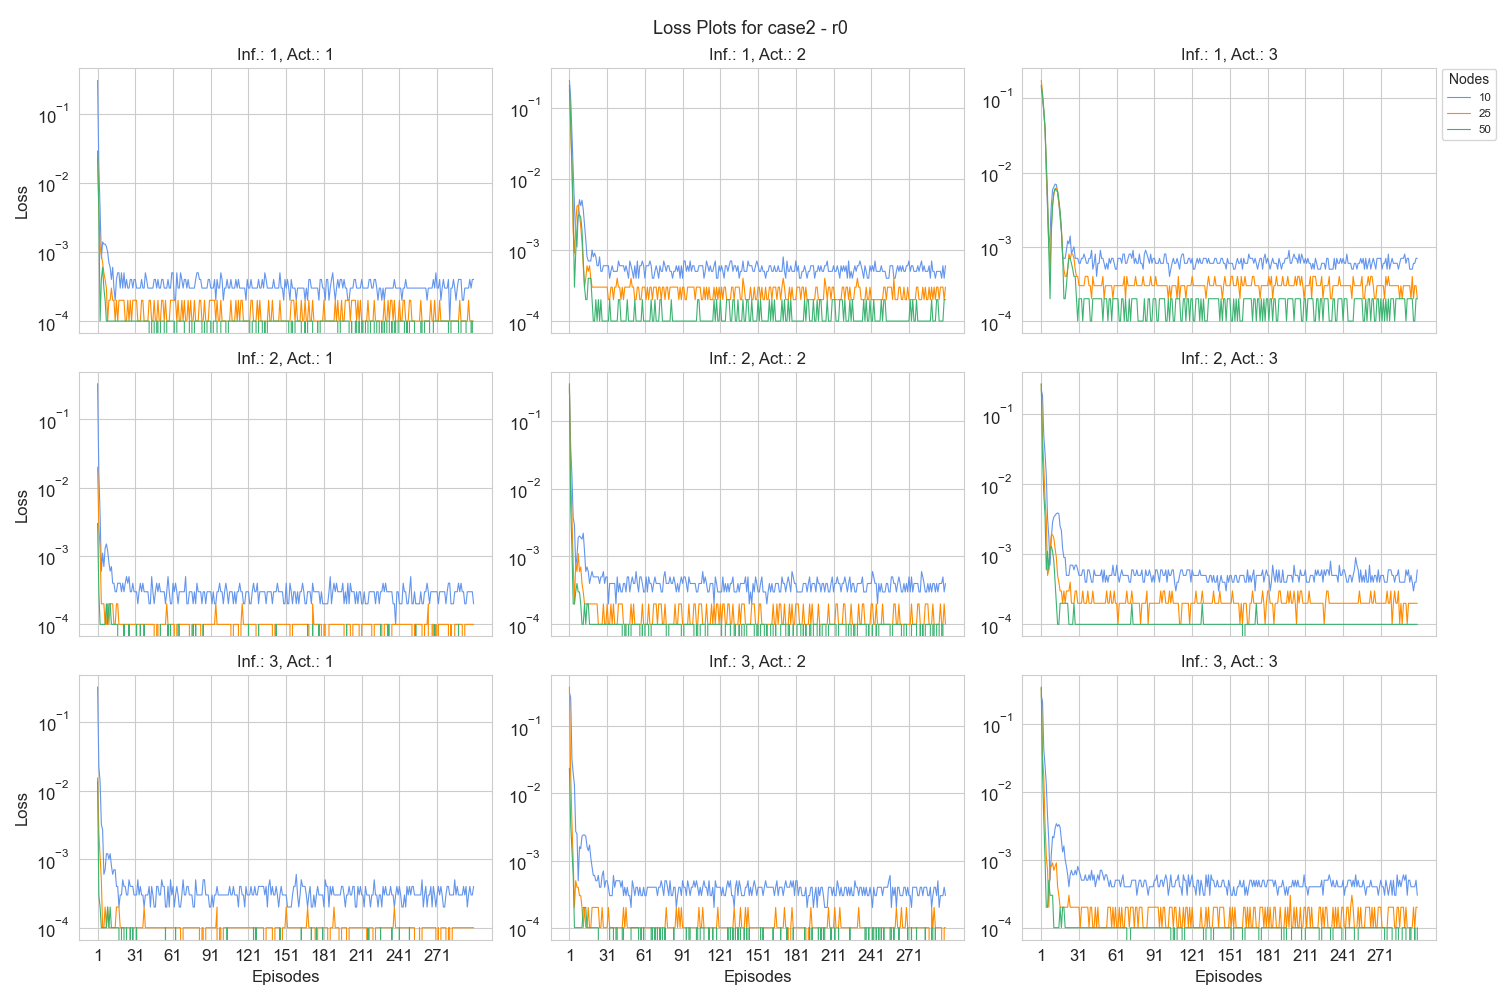}
    \caption{Case-2 using R0: Training MSE loss evolution for RL policy using GCN model across networks of 10 (blue), 25 (orange), and 50 (green) nodes, for varying initial misinformation sources (Inf.) and action budgets (Act.). Plotted on a logarithmic scale, the loss decreases over episodes, indicating improved policy performance and adaptation across network sizes.}
    \label{fig:gcn_c2r0_loss}
\end{figure}

\begin{figure}[!h]
    \centering
    \includegraphics[scale=0.34]{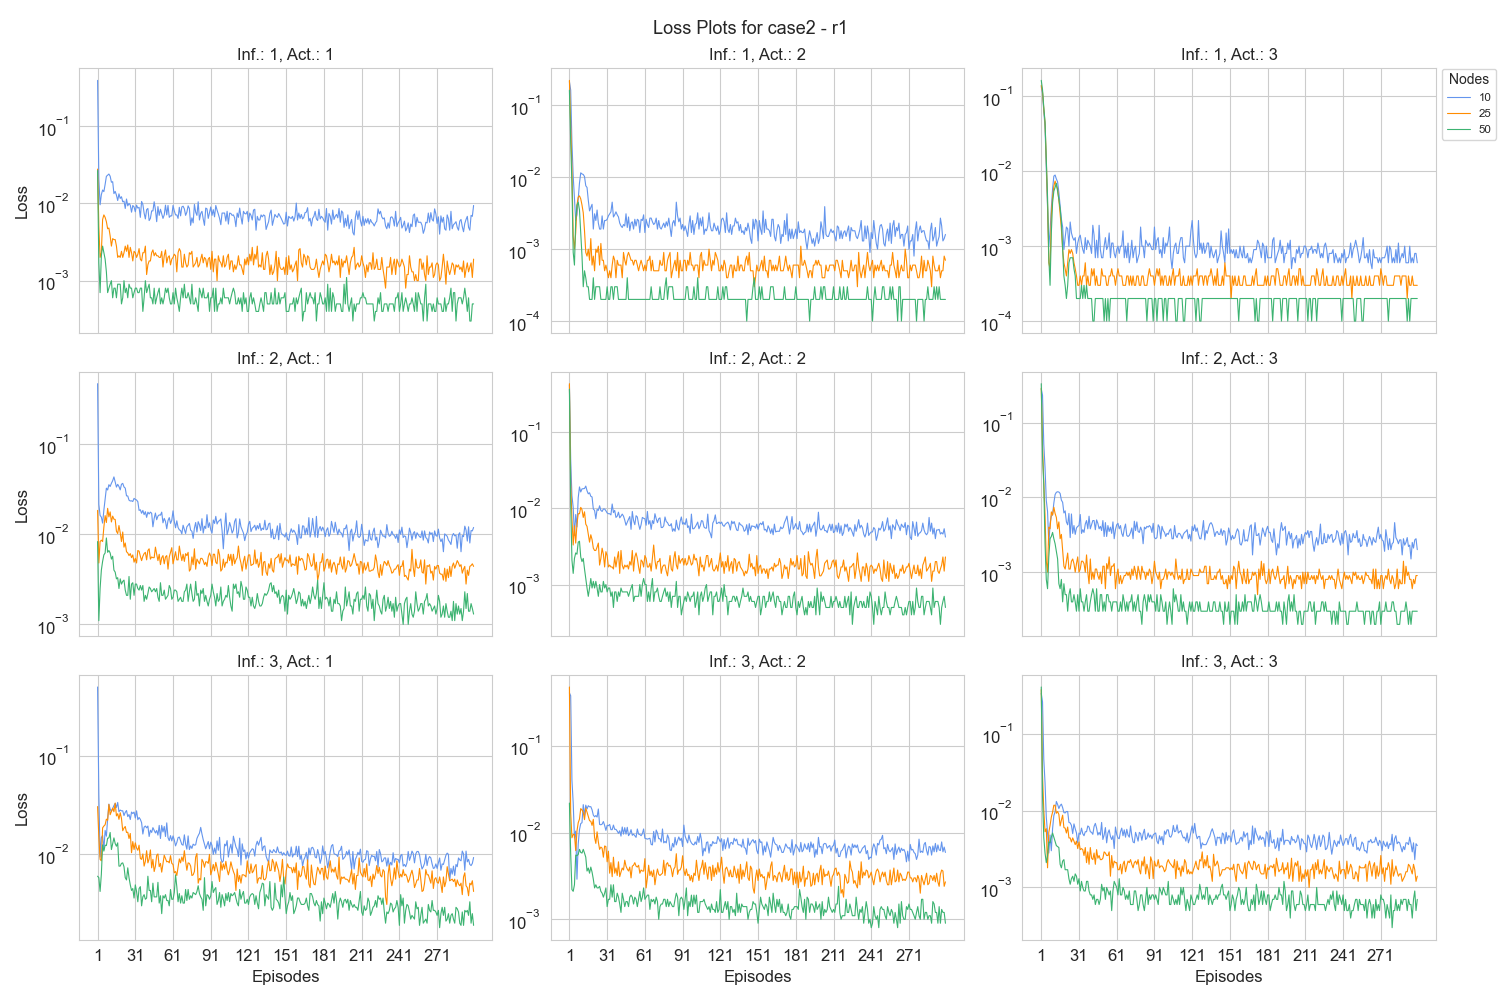}
    \caption{Case-2 using R1: Training MSE loss evolution for RL policy using GCN model across networks of 10 (blue), 25 (orange), and 50 (green) nodes, for varying initial misinformation sources (Inf.) and action budgets (Act.). Plotted on a logarithmic scale, the loss decreases over episodes, indicating improved policy performance and adaptation across network sizes.}
    \label{fig:gcn_c2r1_loss}
\end{figure}

\begin{figure}[!h]
    \centering
    \includegraphics[scale=0.34]{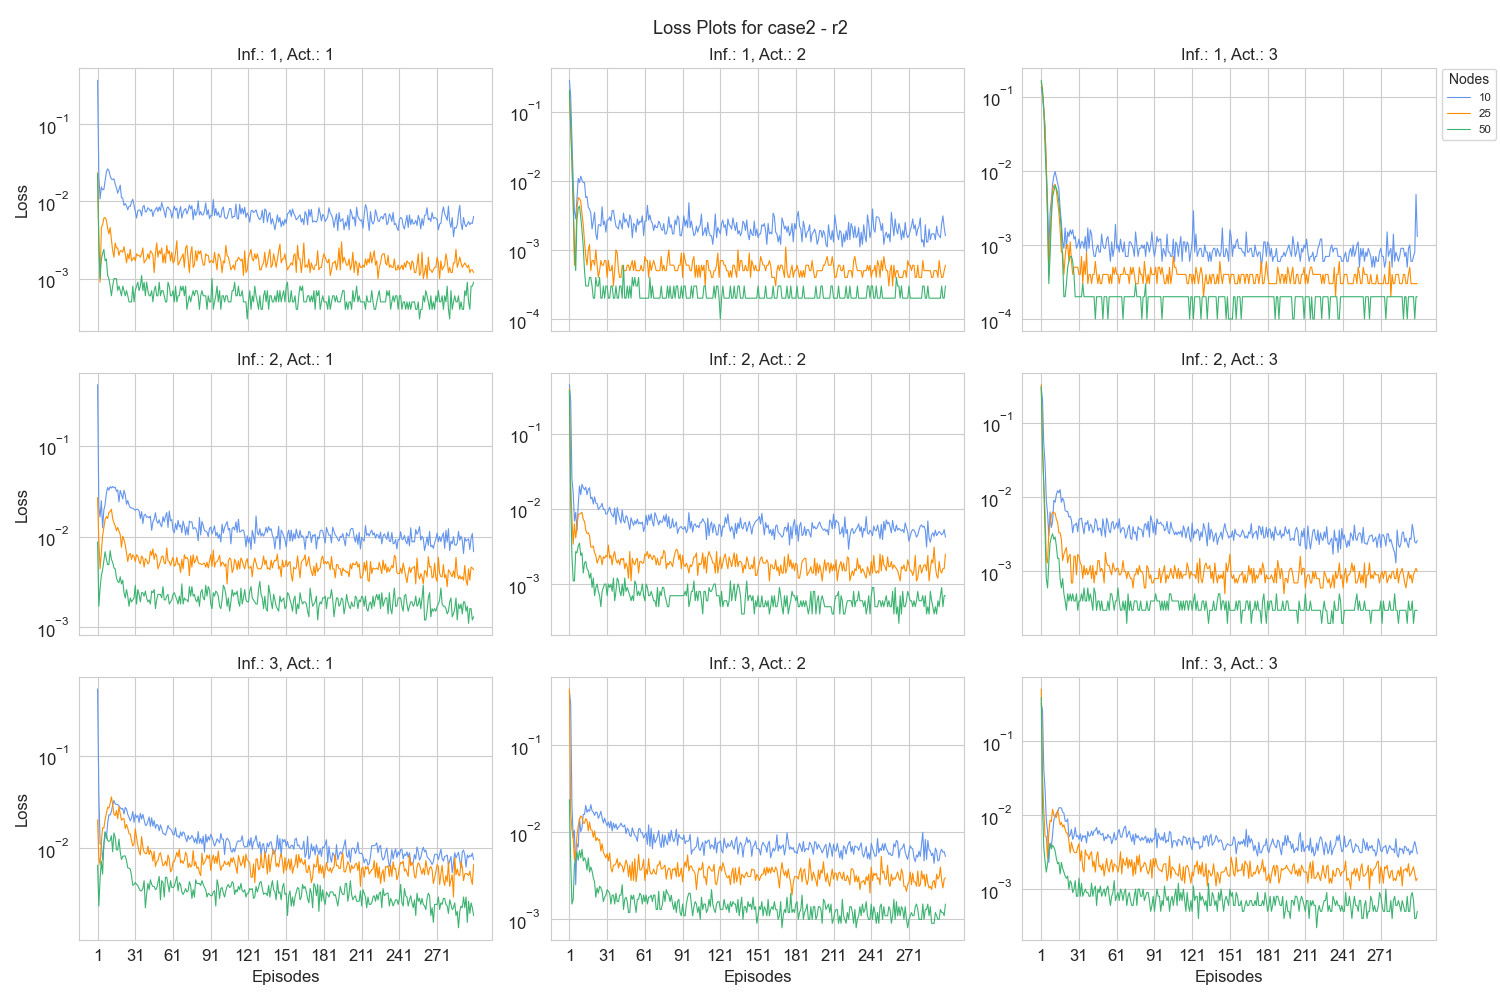}
    \caption{Case-2 using R2: Training MSE loss evolution for RL policy using GCN model across networks of 10 (blue), 25 (orange), and 50 (green) nodes, for varying initial misinformation sources (Inf.) and action budgets (Act.). Plotted on a logarithmic scale, the loss decreases over episodes, indicating improved policy performance and adaptation across network sizes.}
    \label{fig:gcn_c2r2_loss}
\end{figure}

\begin{figure}[!h]
    \centering
    \includegraphics[scale=0.34]{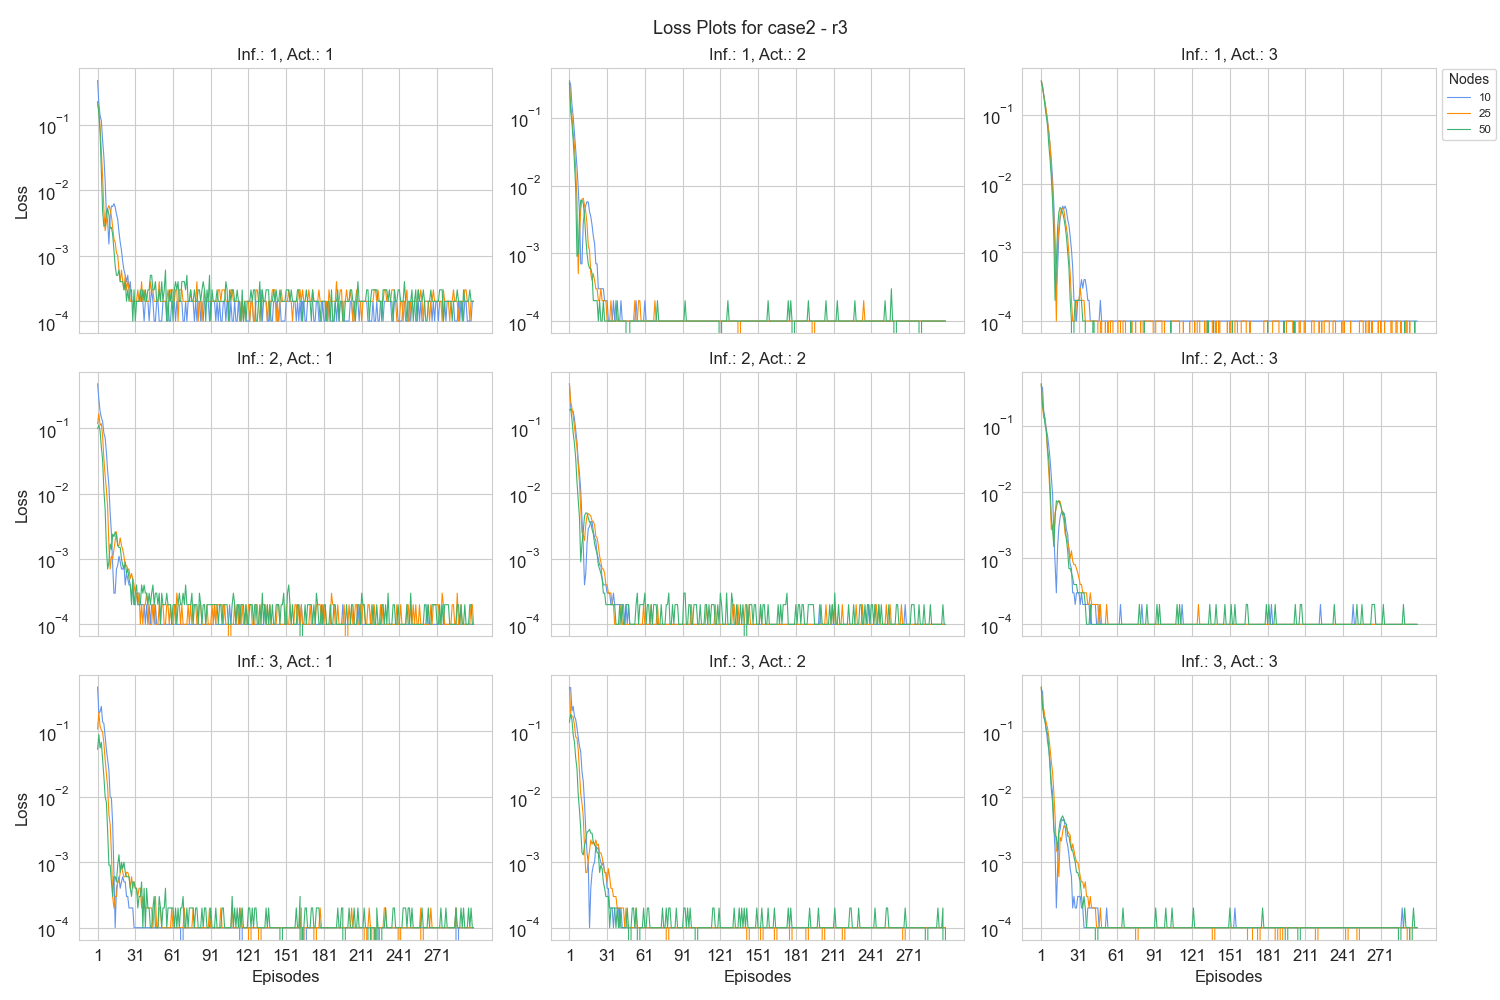}
    \caption{Case-2 using R3: Training MSE loss evolution for RL policy using GCN model across networks of 10 (blue), 25 (orange), and 50 (green) nodes, for varying initial misinformation sources (Inf.) and action budgets (Act.). Plotted on a logarithmic scale, the loss decreases over episodes, indicating improved policy performance and adaptation across network sizes.}
    \label{fig:gcn_c2r3_loss}
\end{figure}

\begin{figure}[!h]
    \centering
    \includegraphics[scale=0.34]{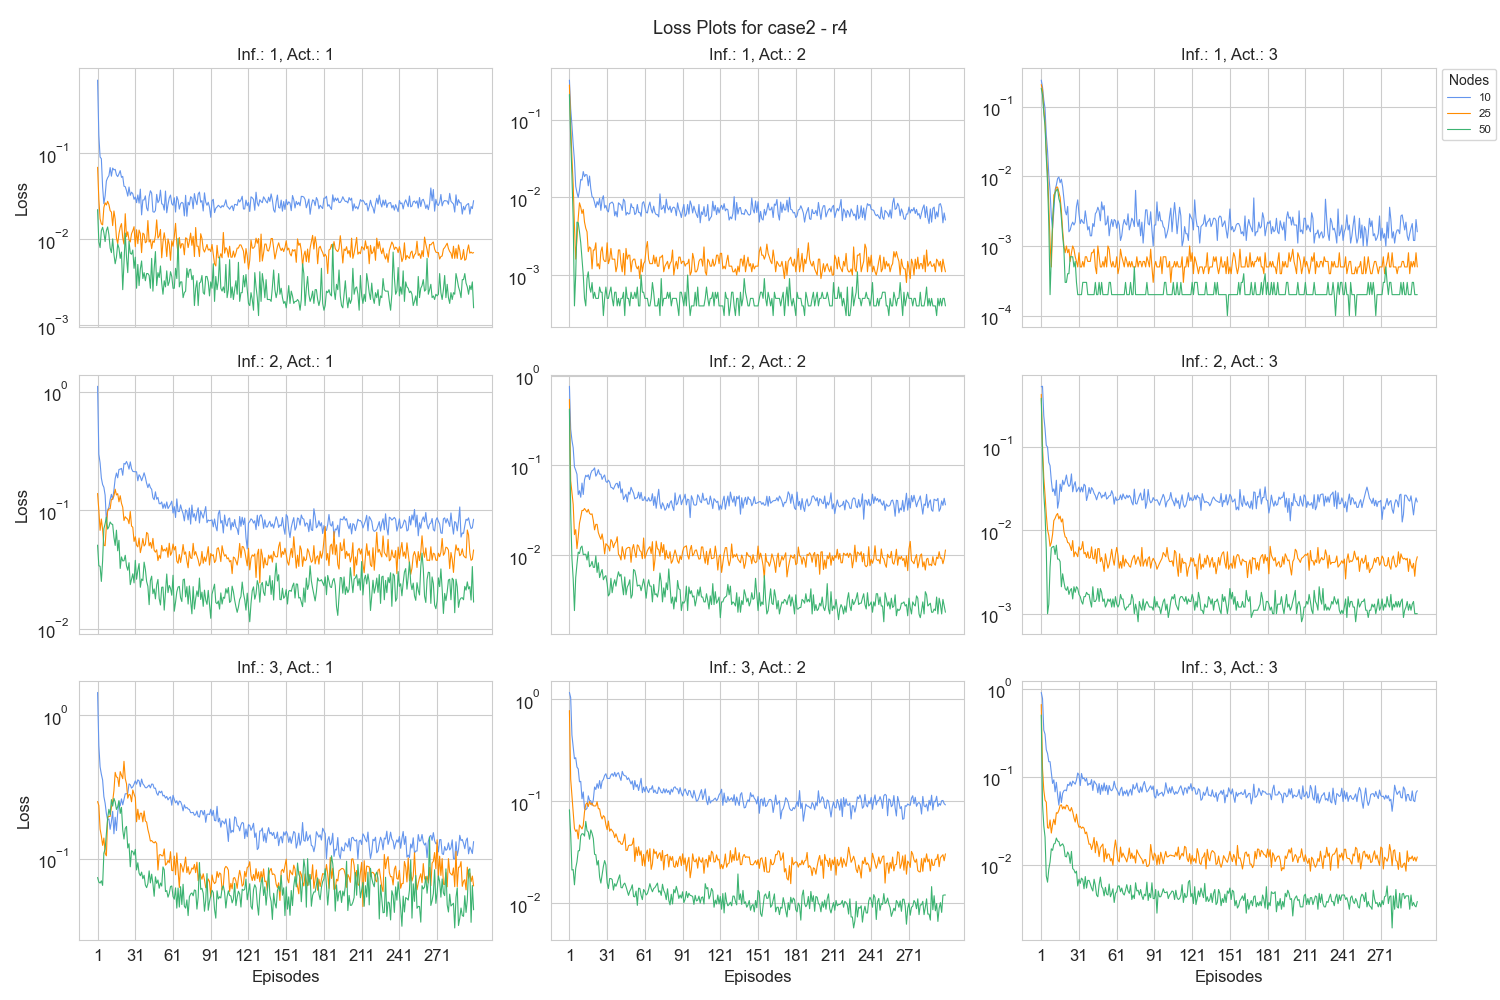}
    \caption{Case-2 using R4: Training MSE loss evolution for RL policy using GCN model across networks of 10 (blue), 25 (orange), and 50 (green) nodes, for varying initial misinformation sources (Inf.) and action budgets (Act.). Plotted on a logarithmic scale, the loss decreases over episodes, indicating improved policy performance and adaptation across network sizes.}
    \label{fig:gcn_c2r4_loss}
\end{figure}
%####################################

% 3 different analysis needed
% 1. Comparison across reward functions, loss, and infection rate
% 2. Comparison of average infection rate and trust distribution.
% 3. The difference is action selection strategies across reward functions.
