# Supplementary material for: Towards Effective Planning Strategies for Dynamic Opinion Networks
Source: arXiv:2410.14091 source file (2024-11-03)
Supplement: Supplementary file 3 [file appendix_figures.tex]

% ######################################
% ################ SL ##################
% ######################################

%%%%%%%%%%%% Figures %%%%%%%%%%%%%

% ###### Case 1 ##########

\begin{figure}[!h]
    \centering
    \includegraphics[scale=0.3]{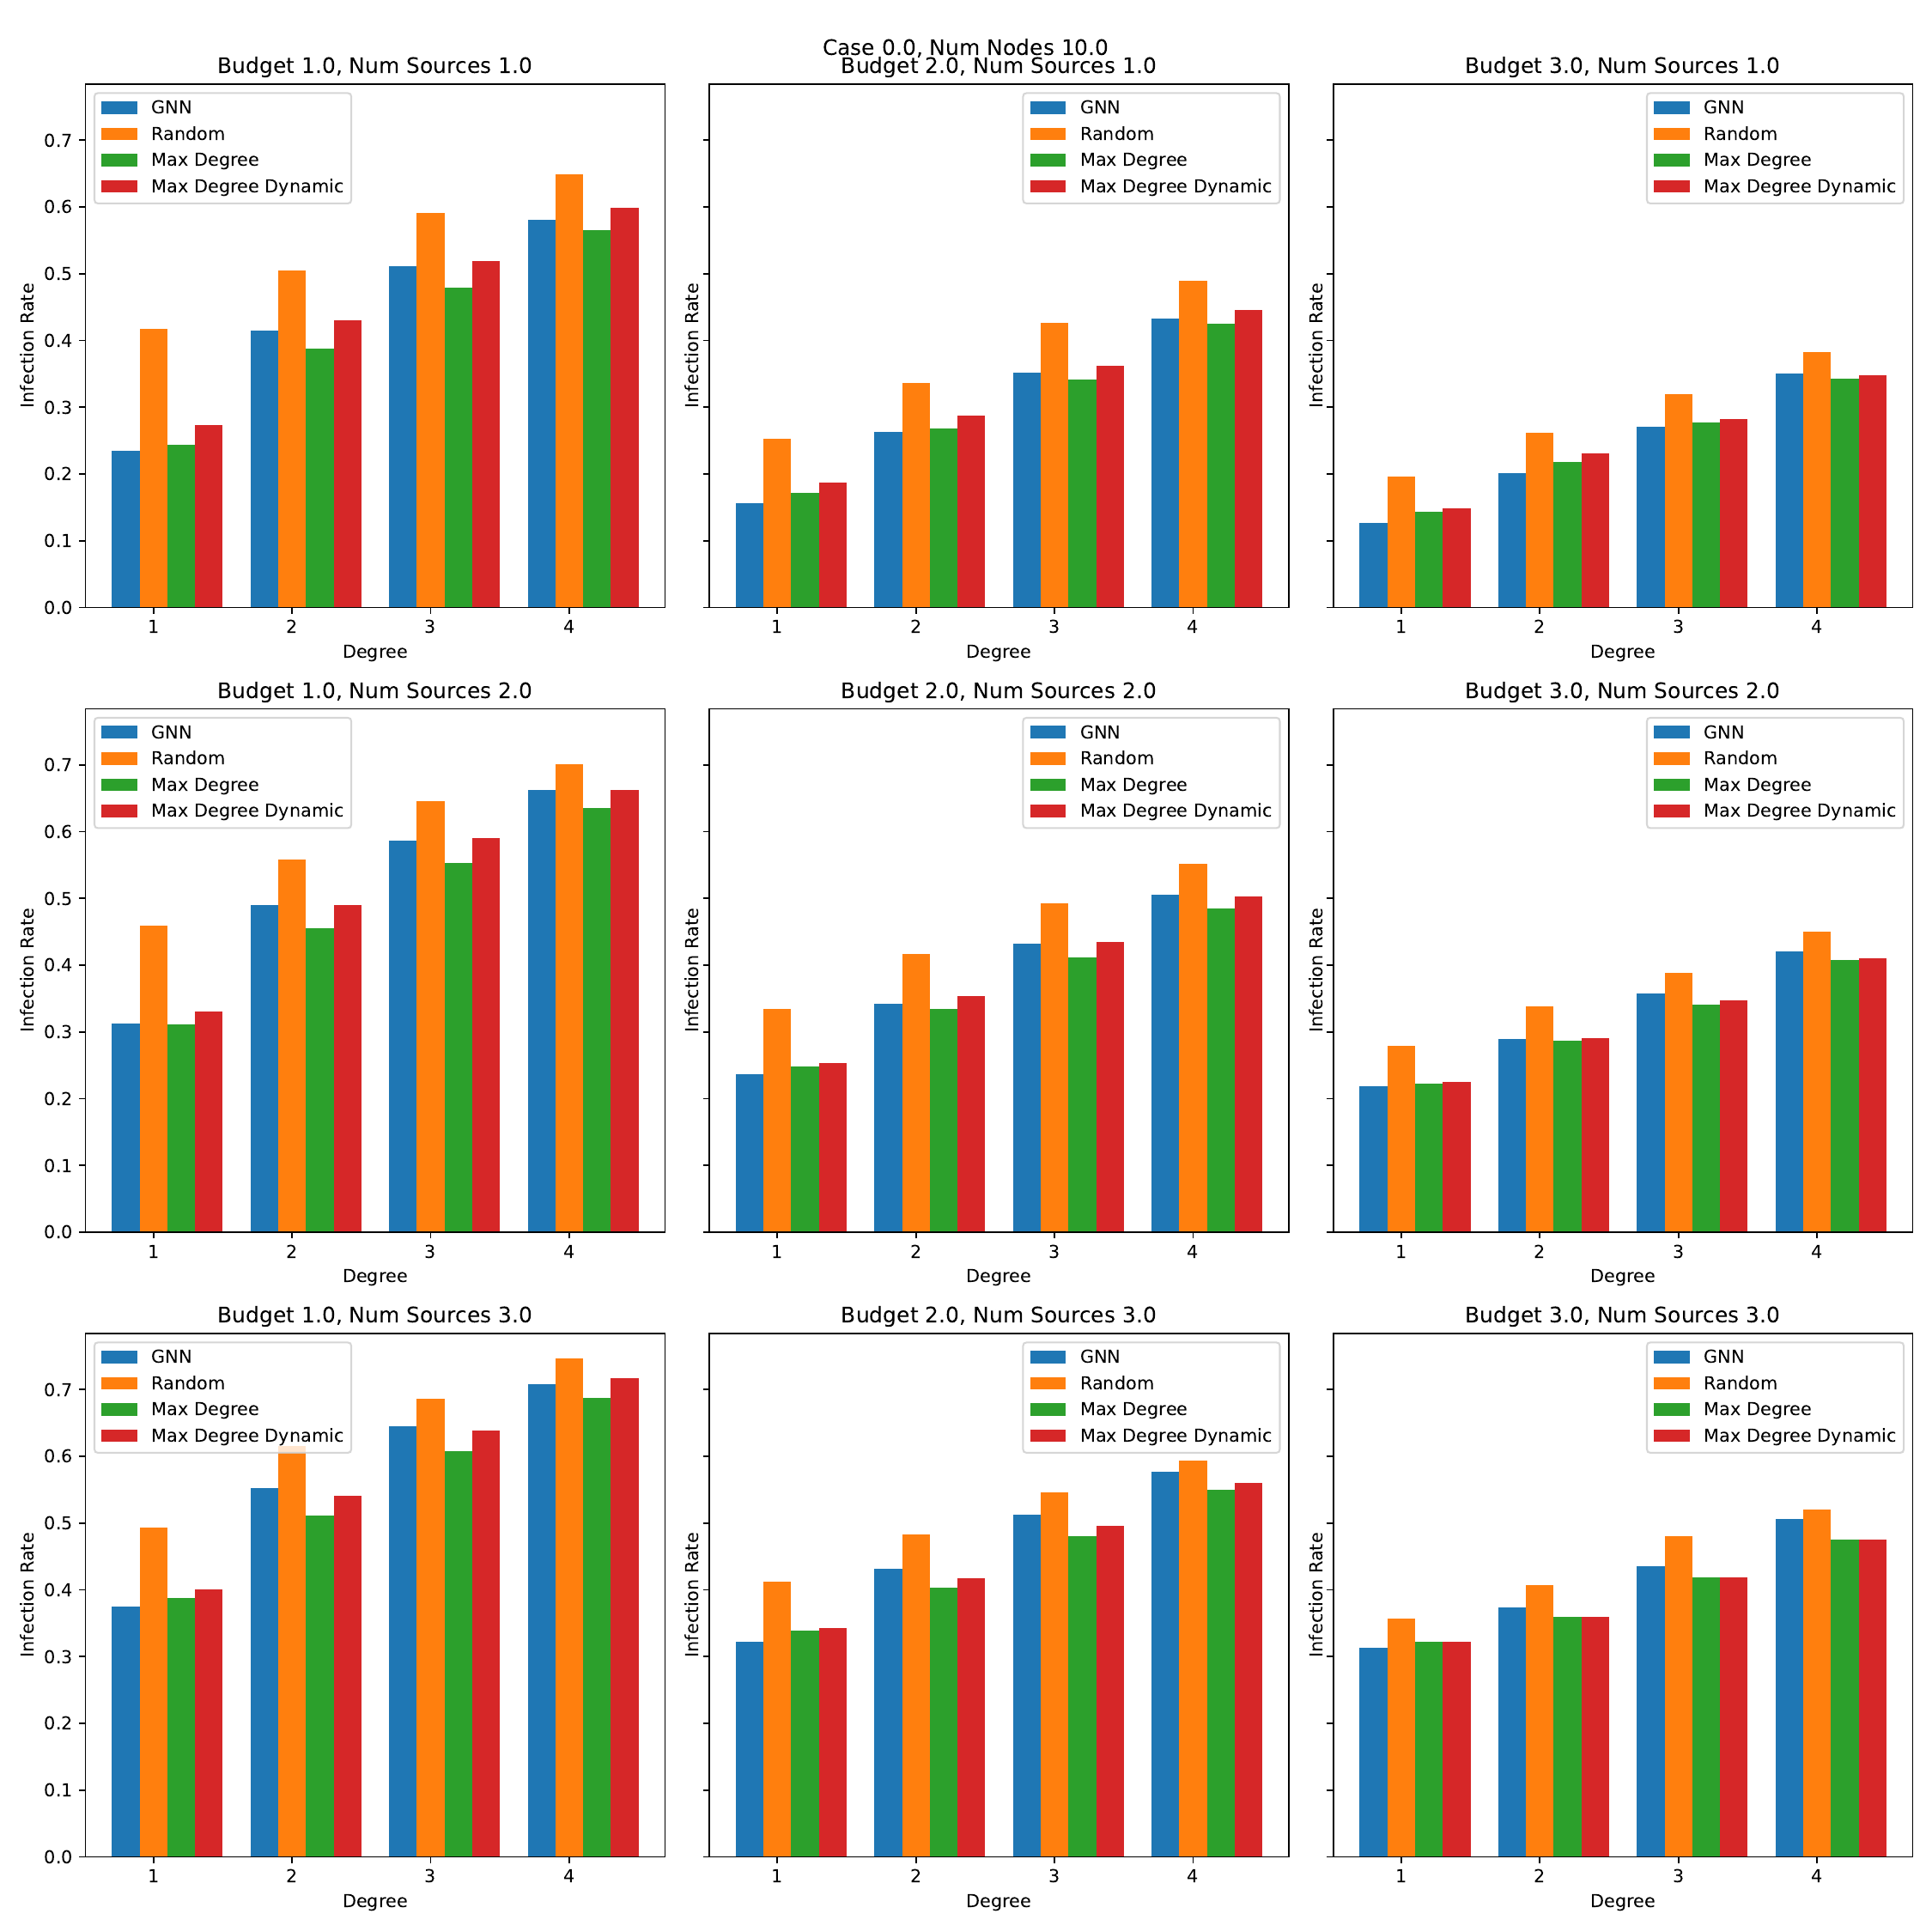}
    \caption{\footnotesize Dataset: Watts-Strogatz, Case-1 Node-10: Performance Evaluation of GCN-Based Supervised Learning Model: This series of bar plots presents a comparative analysis between our GCN-based SL model (blue), Randomized Policy model(yellow), Max Degree Policy model (Static) (green) and Max Degree Policy model (Dynamic) (red) on 10-node network environment. Progressing from left to right, the plots depict scenarios with increasing action budgets, ranging from 1 to 3 actions permitted. Vertically, the plots are ordered to show the effect of varying the initial count of infected nodes, starting with one and increasing to three. Each set of bars within the plots is categorized by the average connectivity (degree) of the infected nodes.}
    \label{fig:c1n10}
\end{figure}

\begin{figure}[!h]
    \centering
    \includegraphics[scale=0.3]{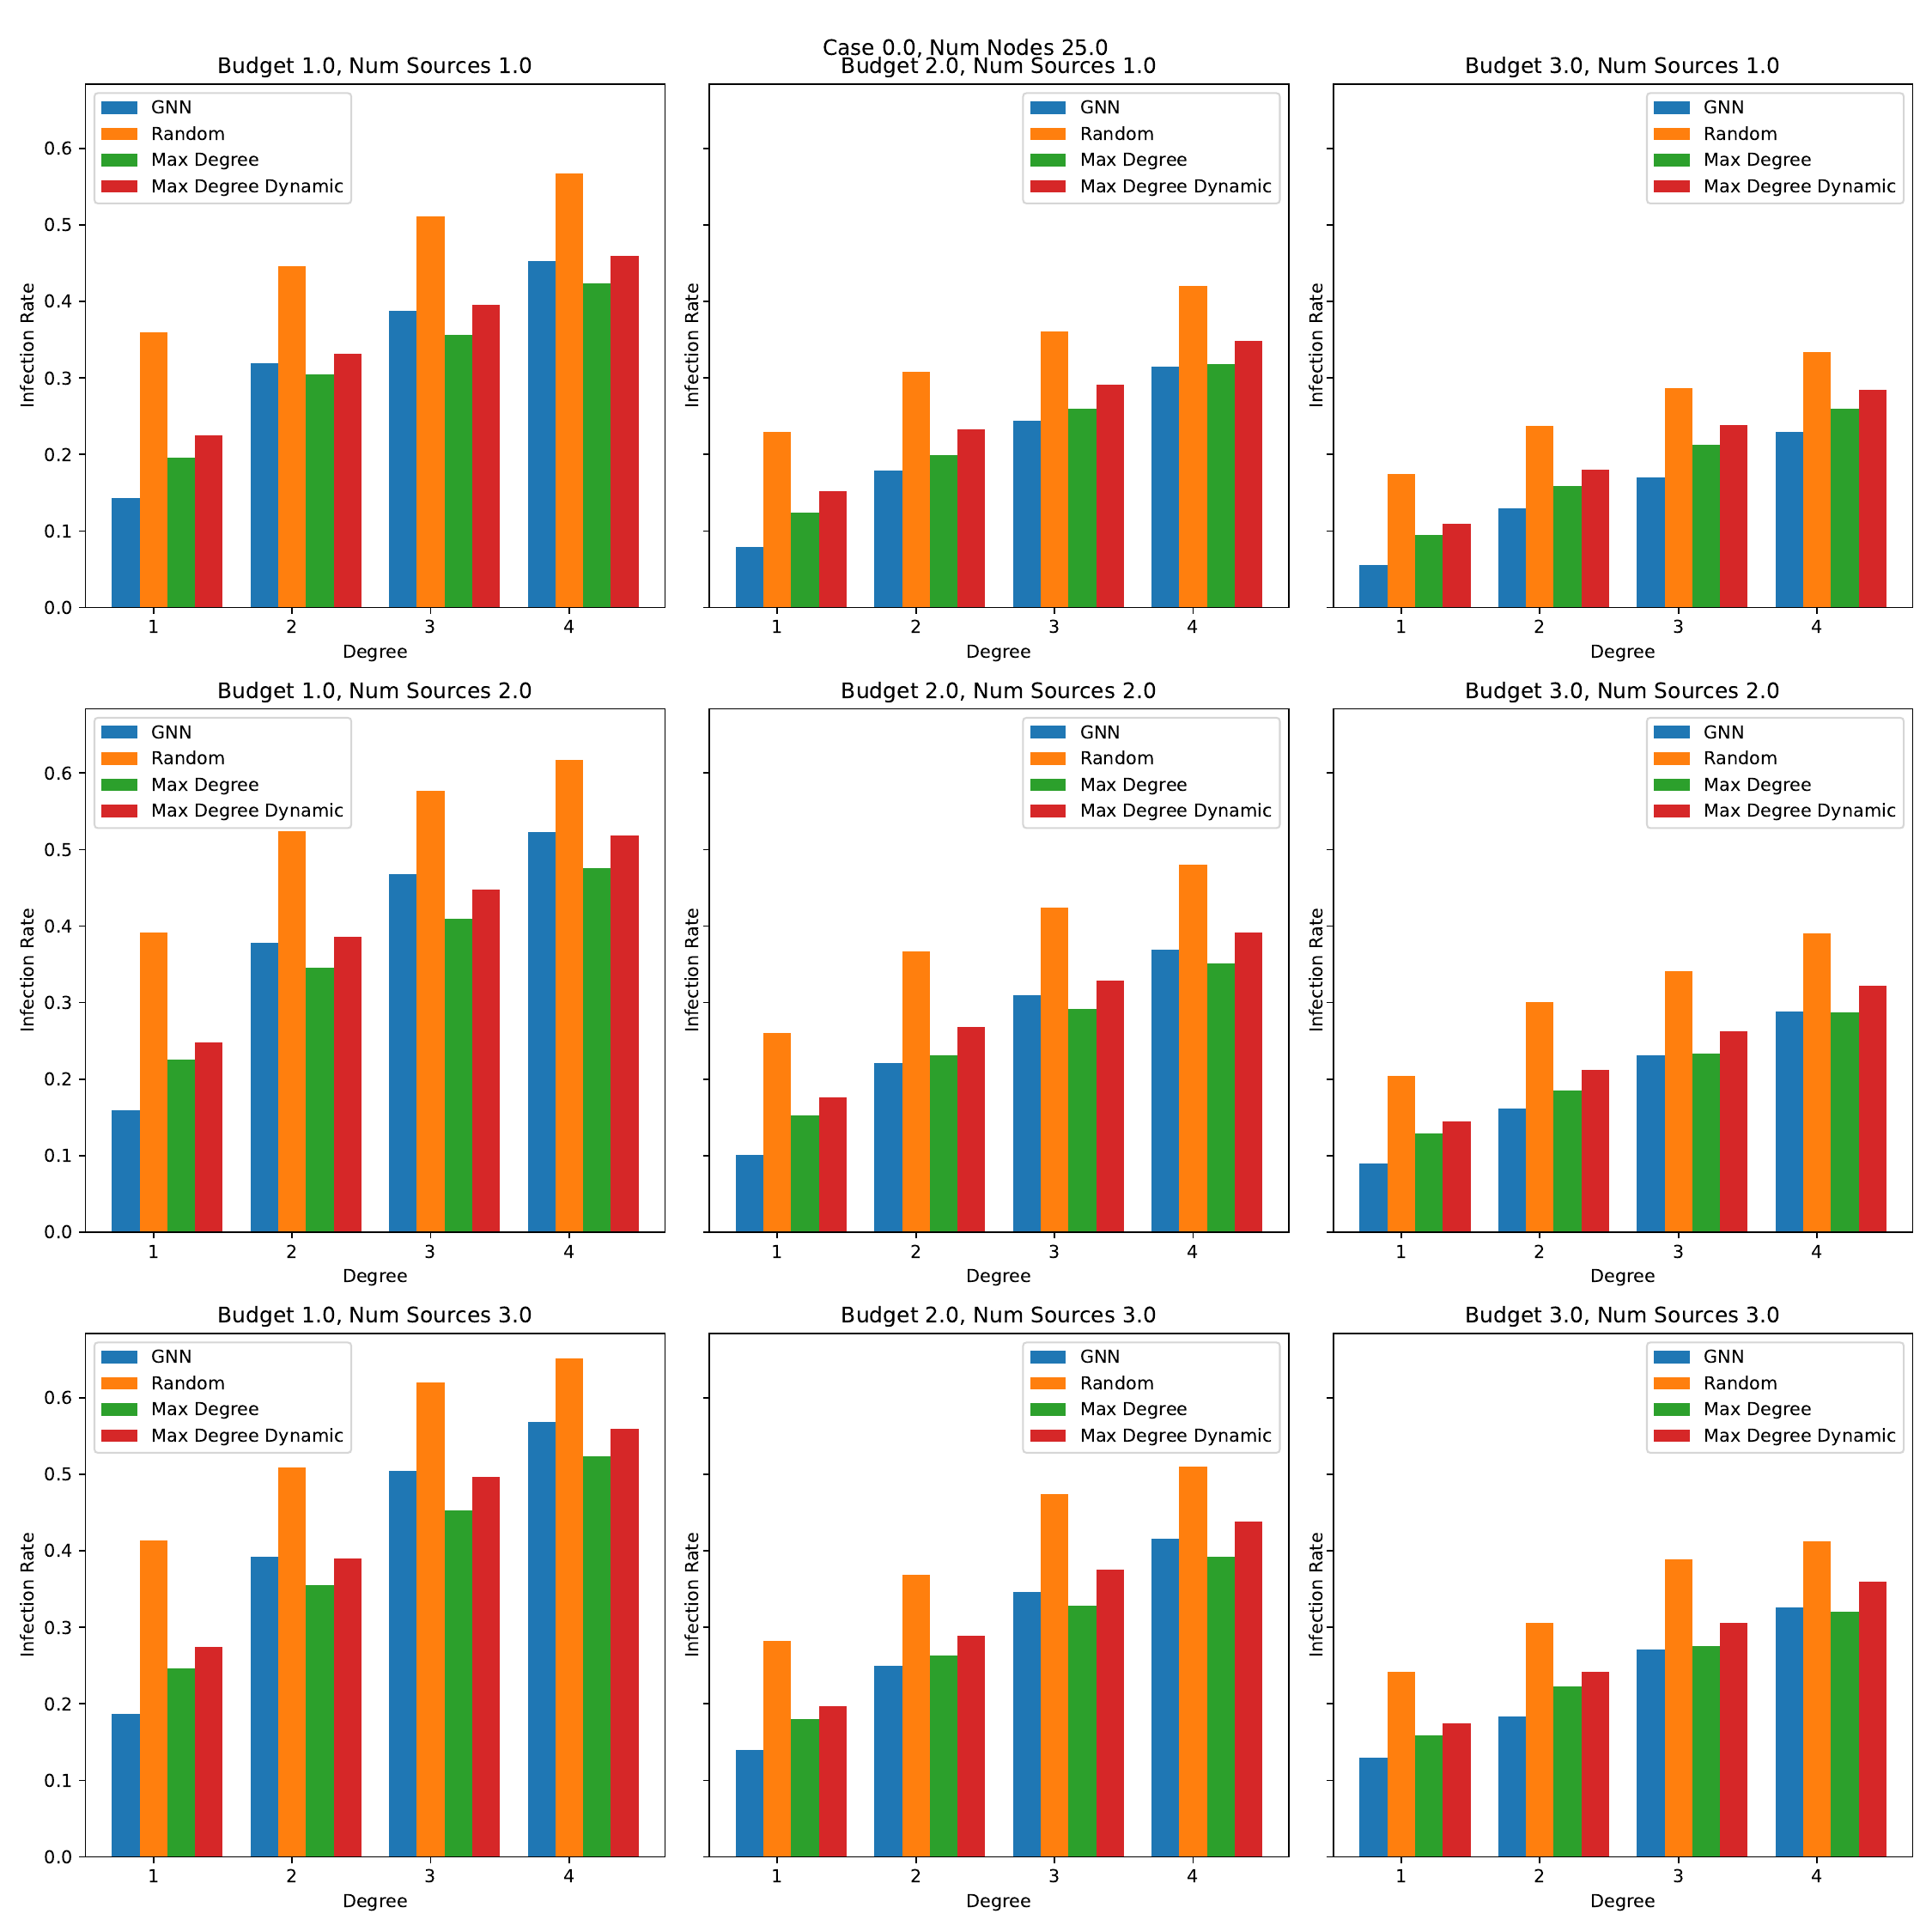}
    \caption{\footnotesize Dataset: Watts-Strogatz, Case-1 Node-25: Performance Evaluation of GCN-Based Supervised Learning Model: This series of bar plots presents a comparative analysis between our GCN-based SL model (blue), Randomized Policy model(yellow), Max Degree Policy model (Static) (green) and Max Degree Policy model (Dynamic) (red) on 25-node network environment. Progressing from left to right, the plots depict scenarios with increasing action budgets, ranging from 1 to 3 actions permitted. Vertically, the plots are ordered to show the effect of varying the initial count of infected nodes, starting with one and increasing to three. Each set of bars within the plots is categorized by the average connectivity (degree) of the infected nodes.}
    \label{fig:c1n25}
\end{figure}

\begin{figure}[!h]
    \centering
    \includegraphics[scale=0.3]{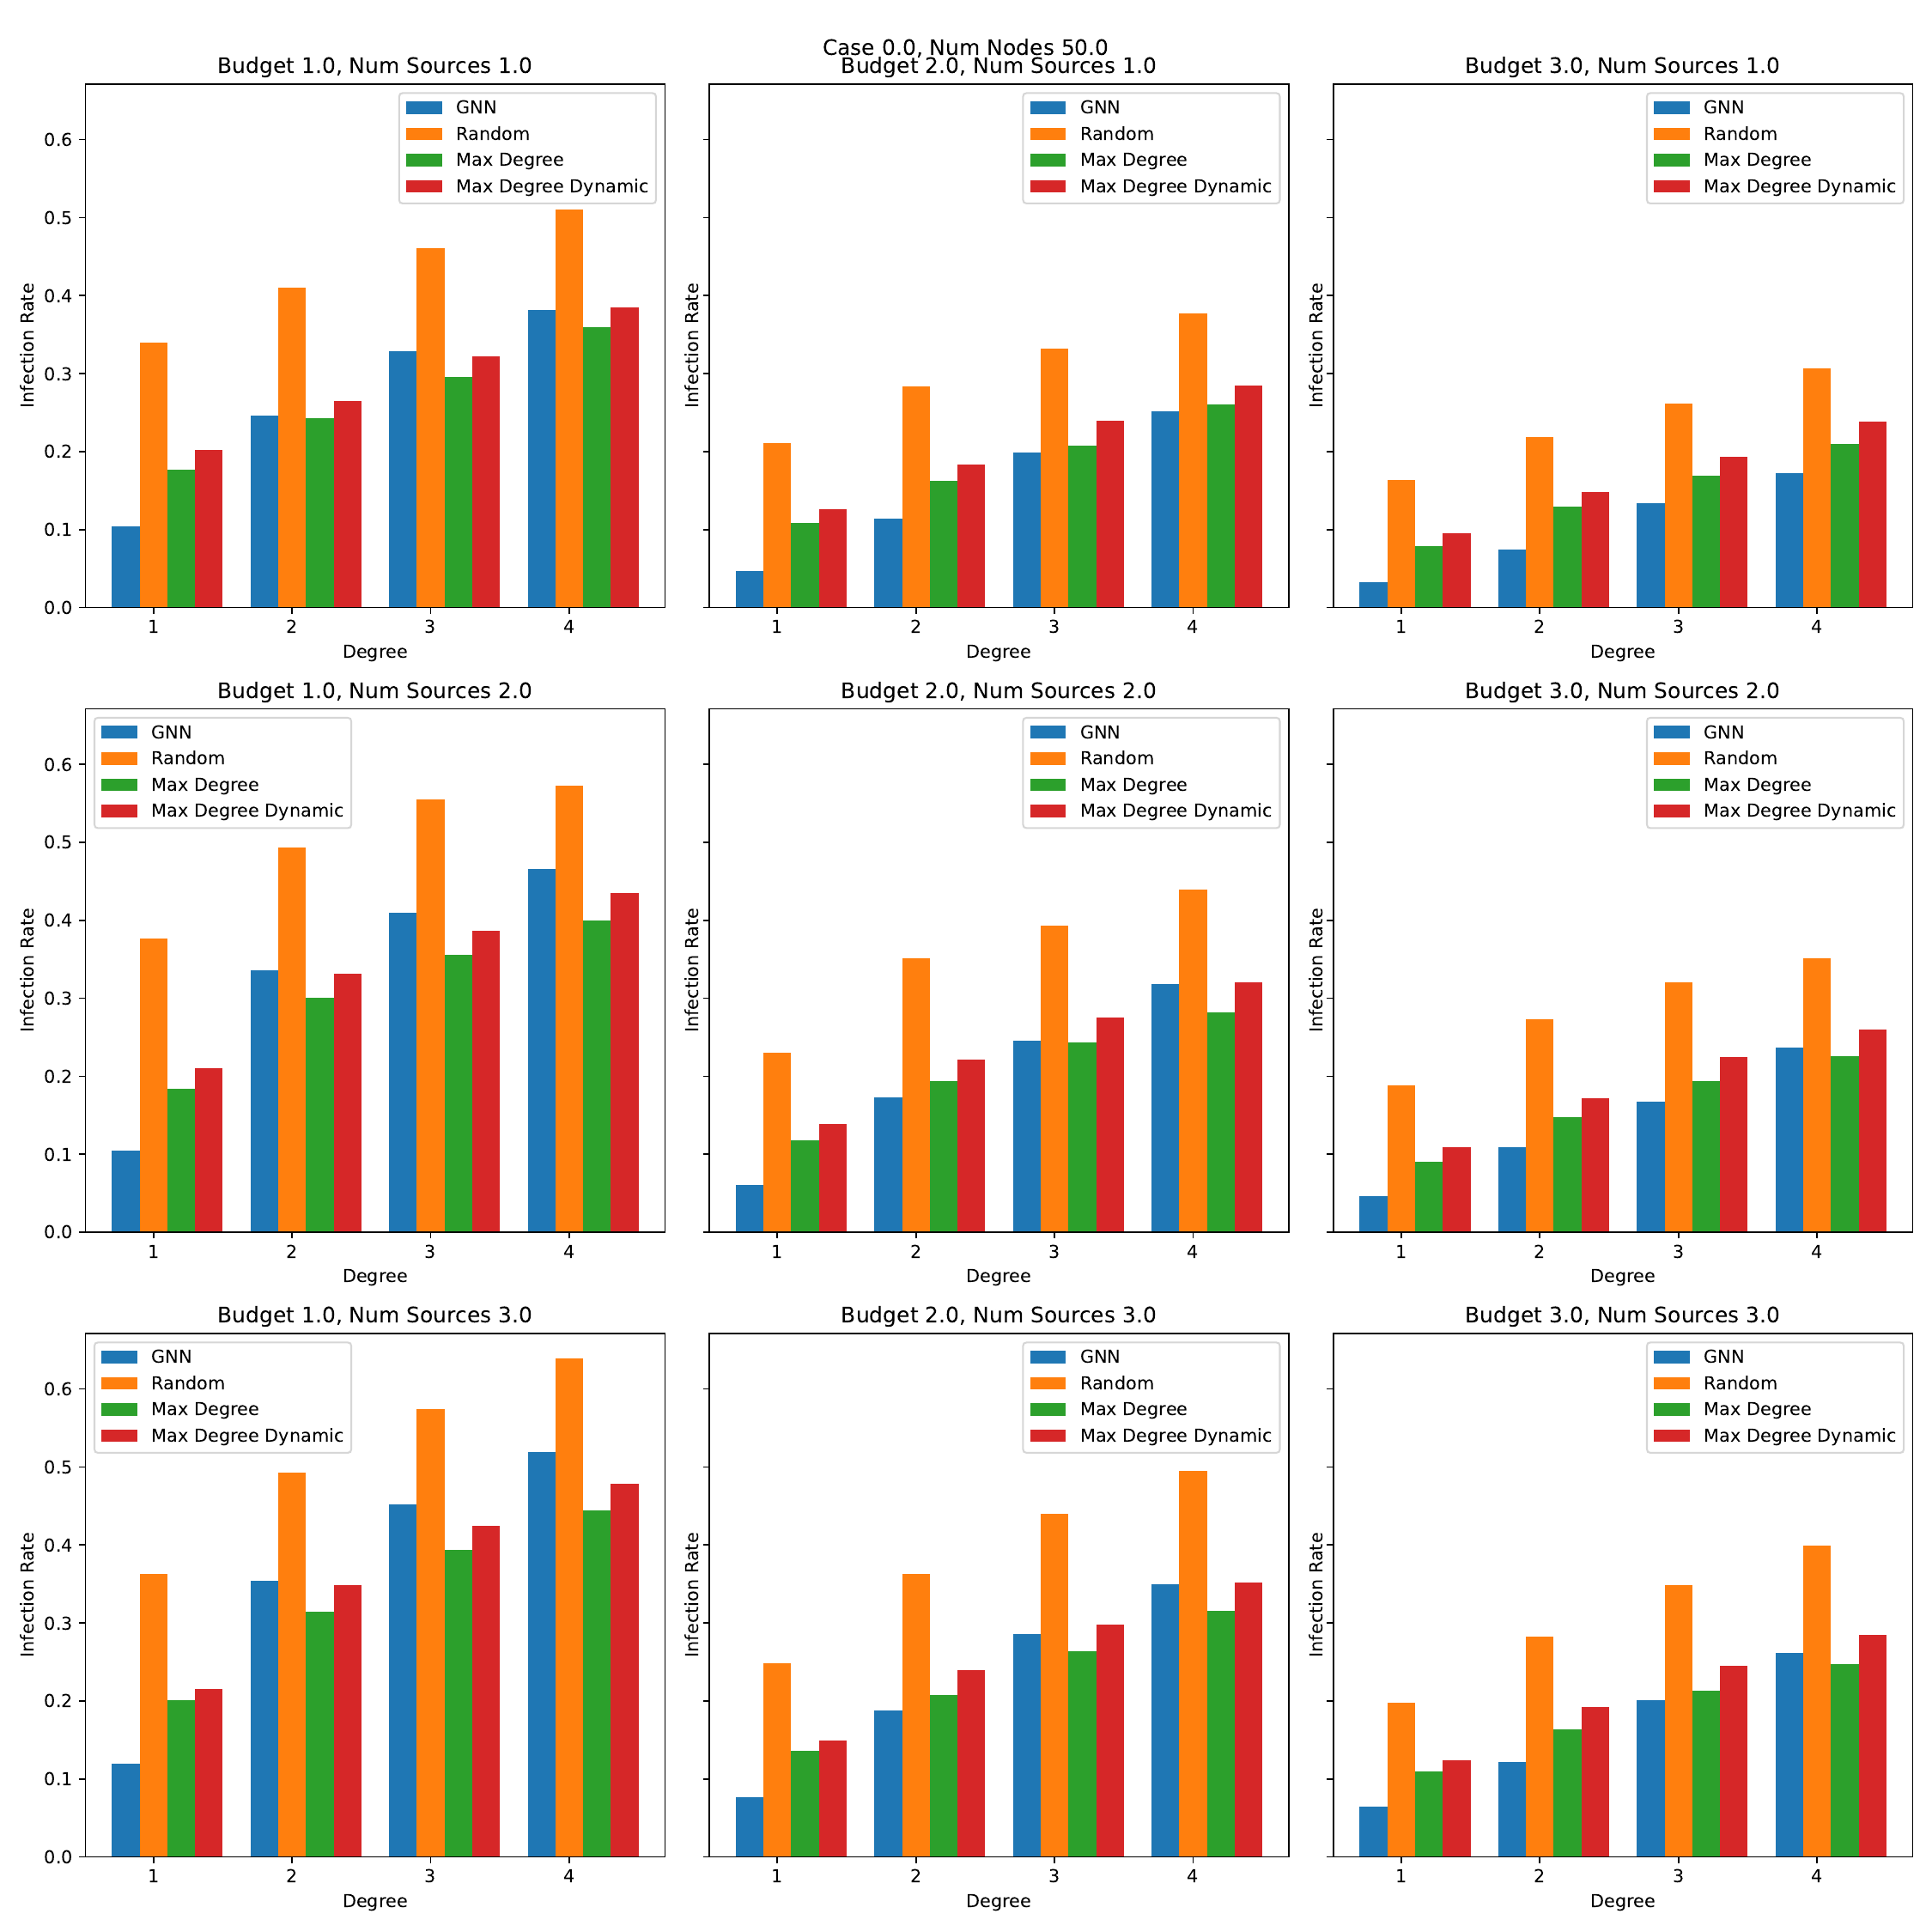}
    \caption{\footnotesize Dataset: Watts-Strogatz, Case-1 Node-50: Performance Evaluation of GCN-Based Supervised Learning Model: This series of bar plots presents a comparative analysis between our GCN-based SL model (blue), Randomized Policy model(yellow), Max Degree Policy model (Static) (green) and Max Degree Policy model (Dynamic) (red) on 50-node network environment. Progressing from left to right, the plots depict scenarios with increasing action budgets, ranging from 1 to 3 actions permitted. Vertically, the plots are ordered to show the effect of varying the initial count of infected nodes, starting with one and increasing to three. Each set of bars within the plots is categorized by the average connectivity (degree) of the infected nodes.}
    \label{fig:c1n50}
\end{figure}

\begin{figure}[!h]
    \centering
    \includegraphics[scale=0.3]{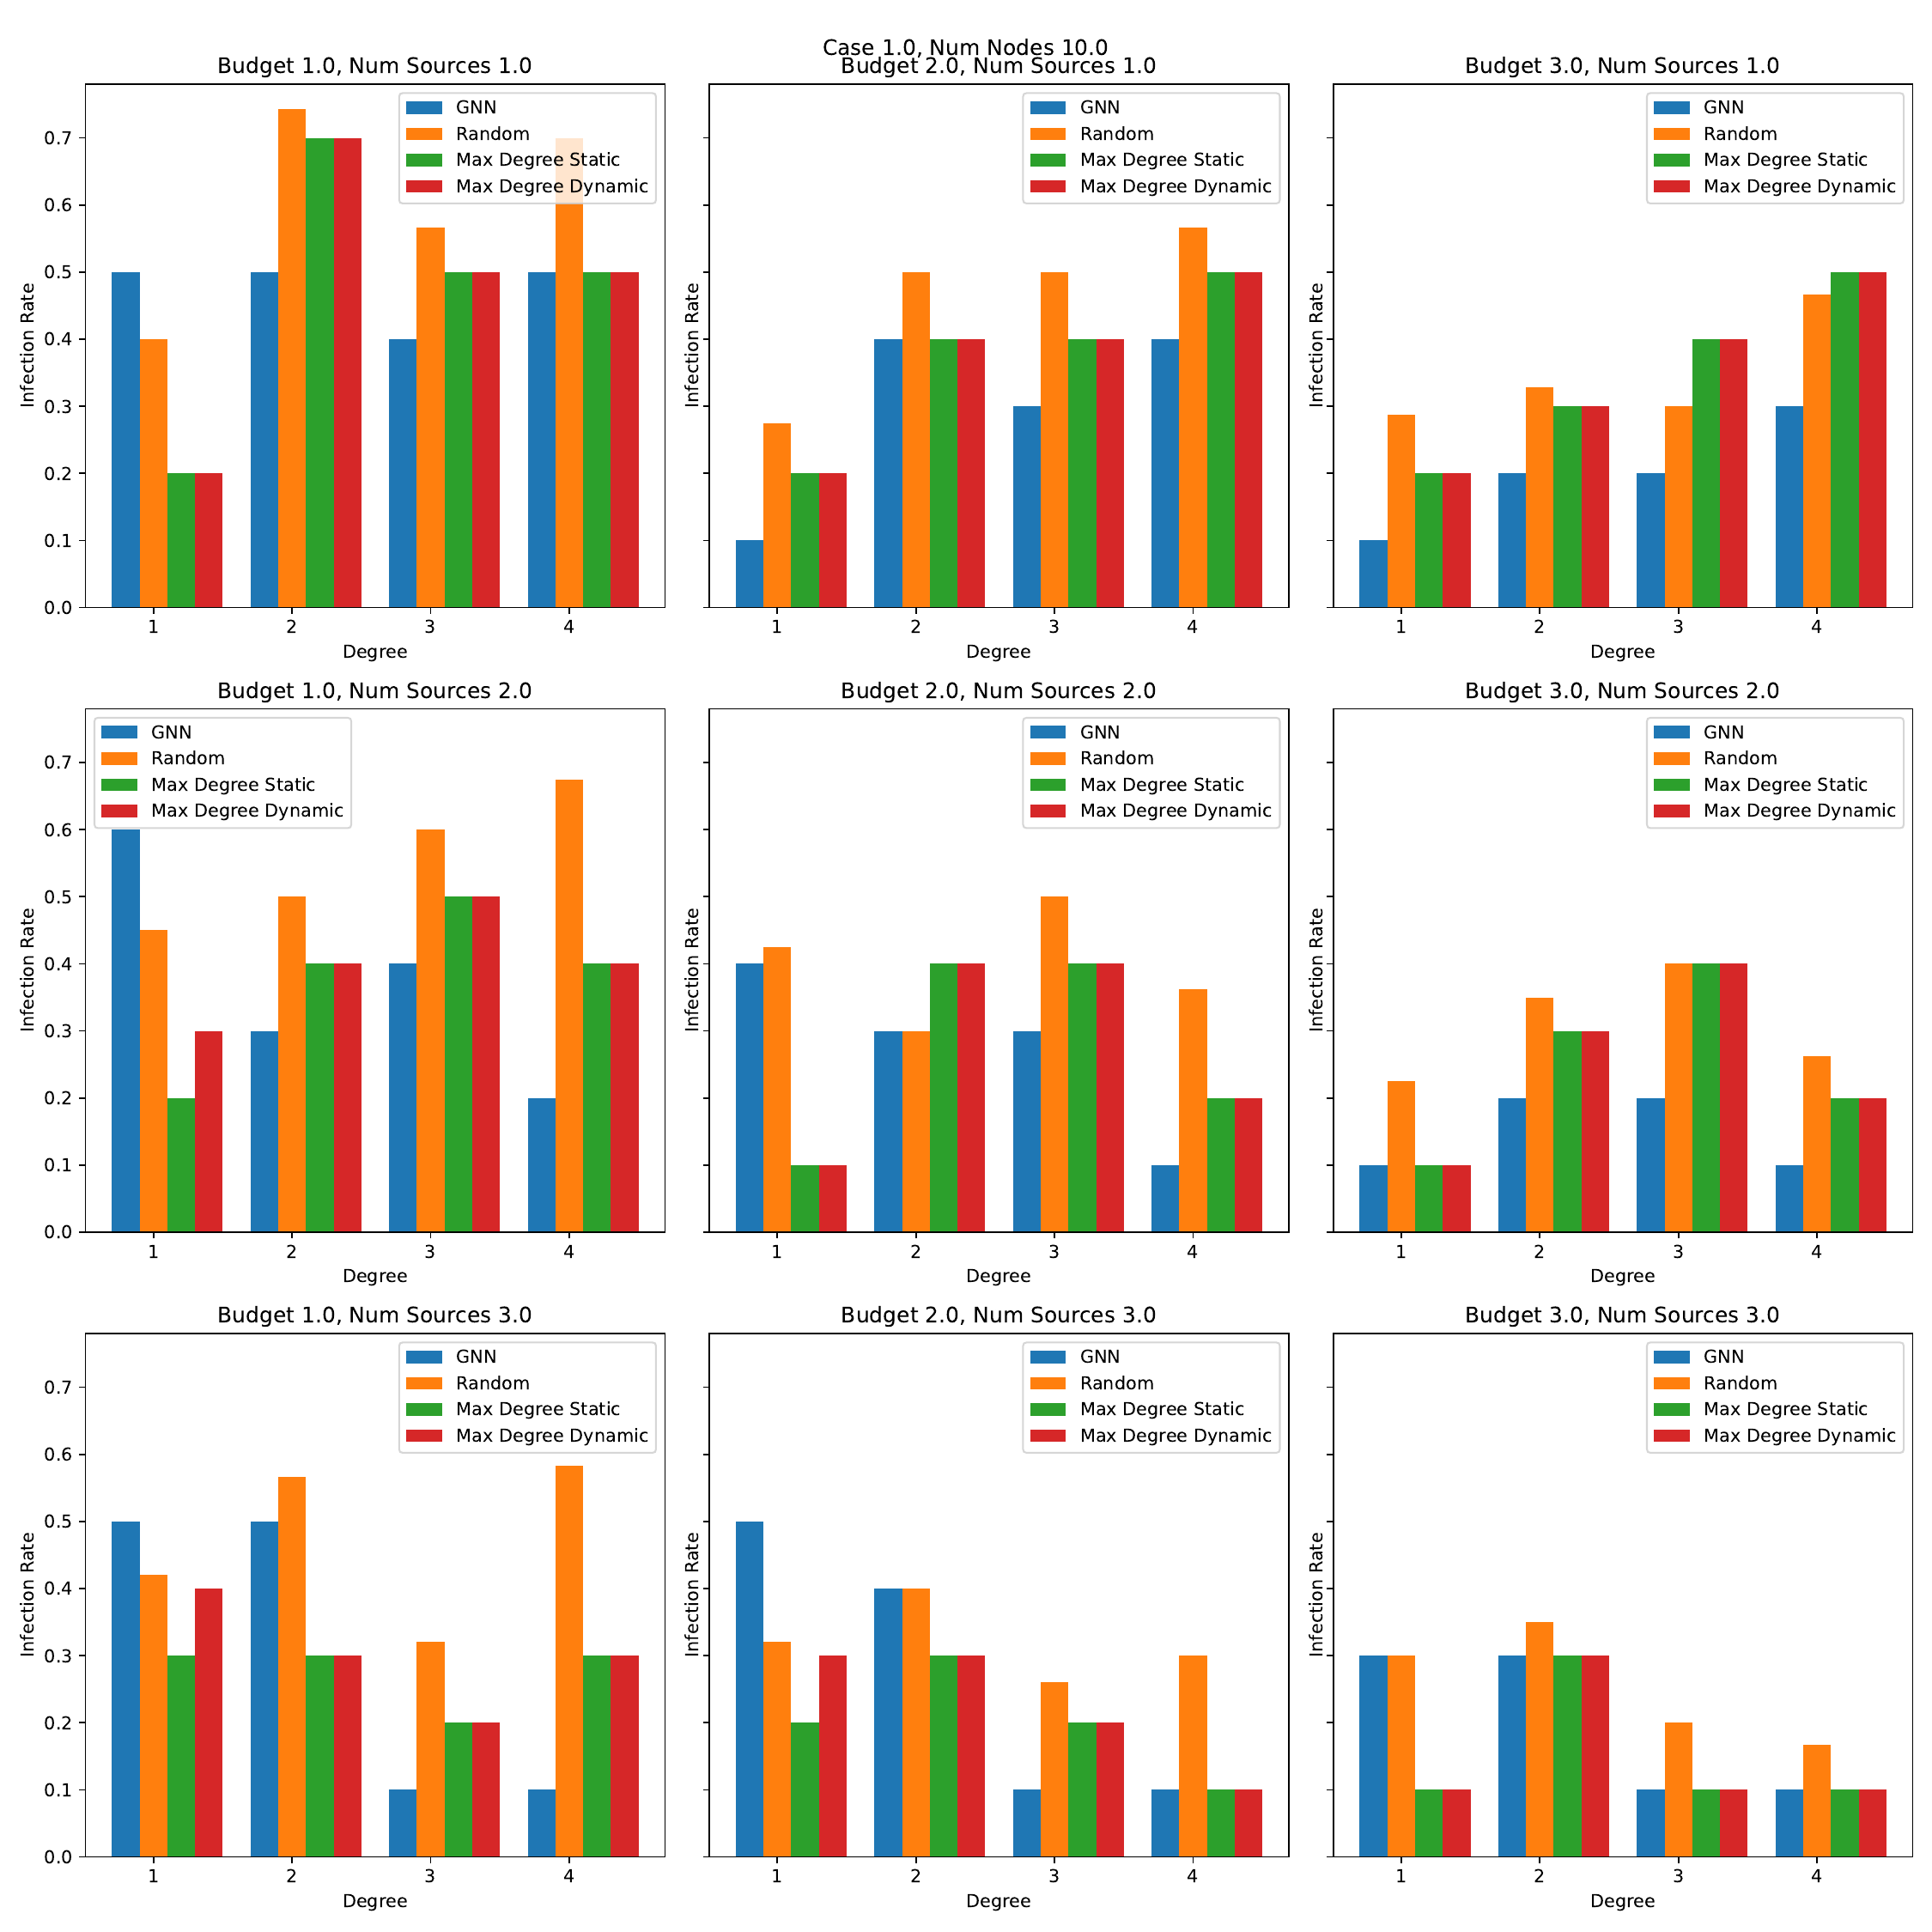}
    \caption{\footnotesize Dataset: Tree, Case-1 Node-10: Performance Evaluation of GCN-Based Supervised Learning Model: This series of bar plots presents a comparative analysis between our GCN-based SL model (blue), Randomized Policy model(yellow), Max Degree Policy model (Static) (green) and Max Degree Policy model (Dynamic) (red) on 10-node network environment. Progressing from left to right, the plots depict scenarios with increasing action budgets, ranging from 1 to 3 actions permitted. Vertically, the plots are ordered to show the effect of varying the initial count of infected nodes, starting with one and increasing to three. Each set of bars within the plots is categorized by the average connectivity (degree) of the infected nodes.}
    \label{fig:Treec1n10}
\end{figure}

\begin{figure}[!h]
    \centering
    \includegraphics[scale=0.3]{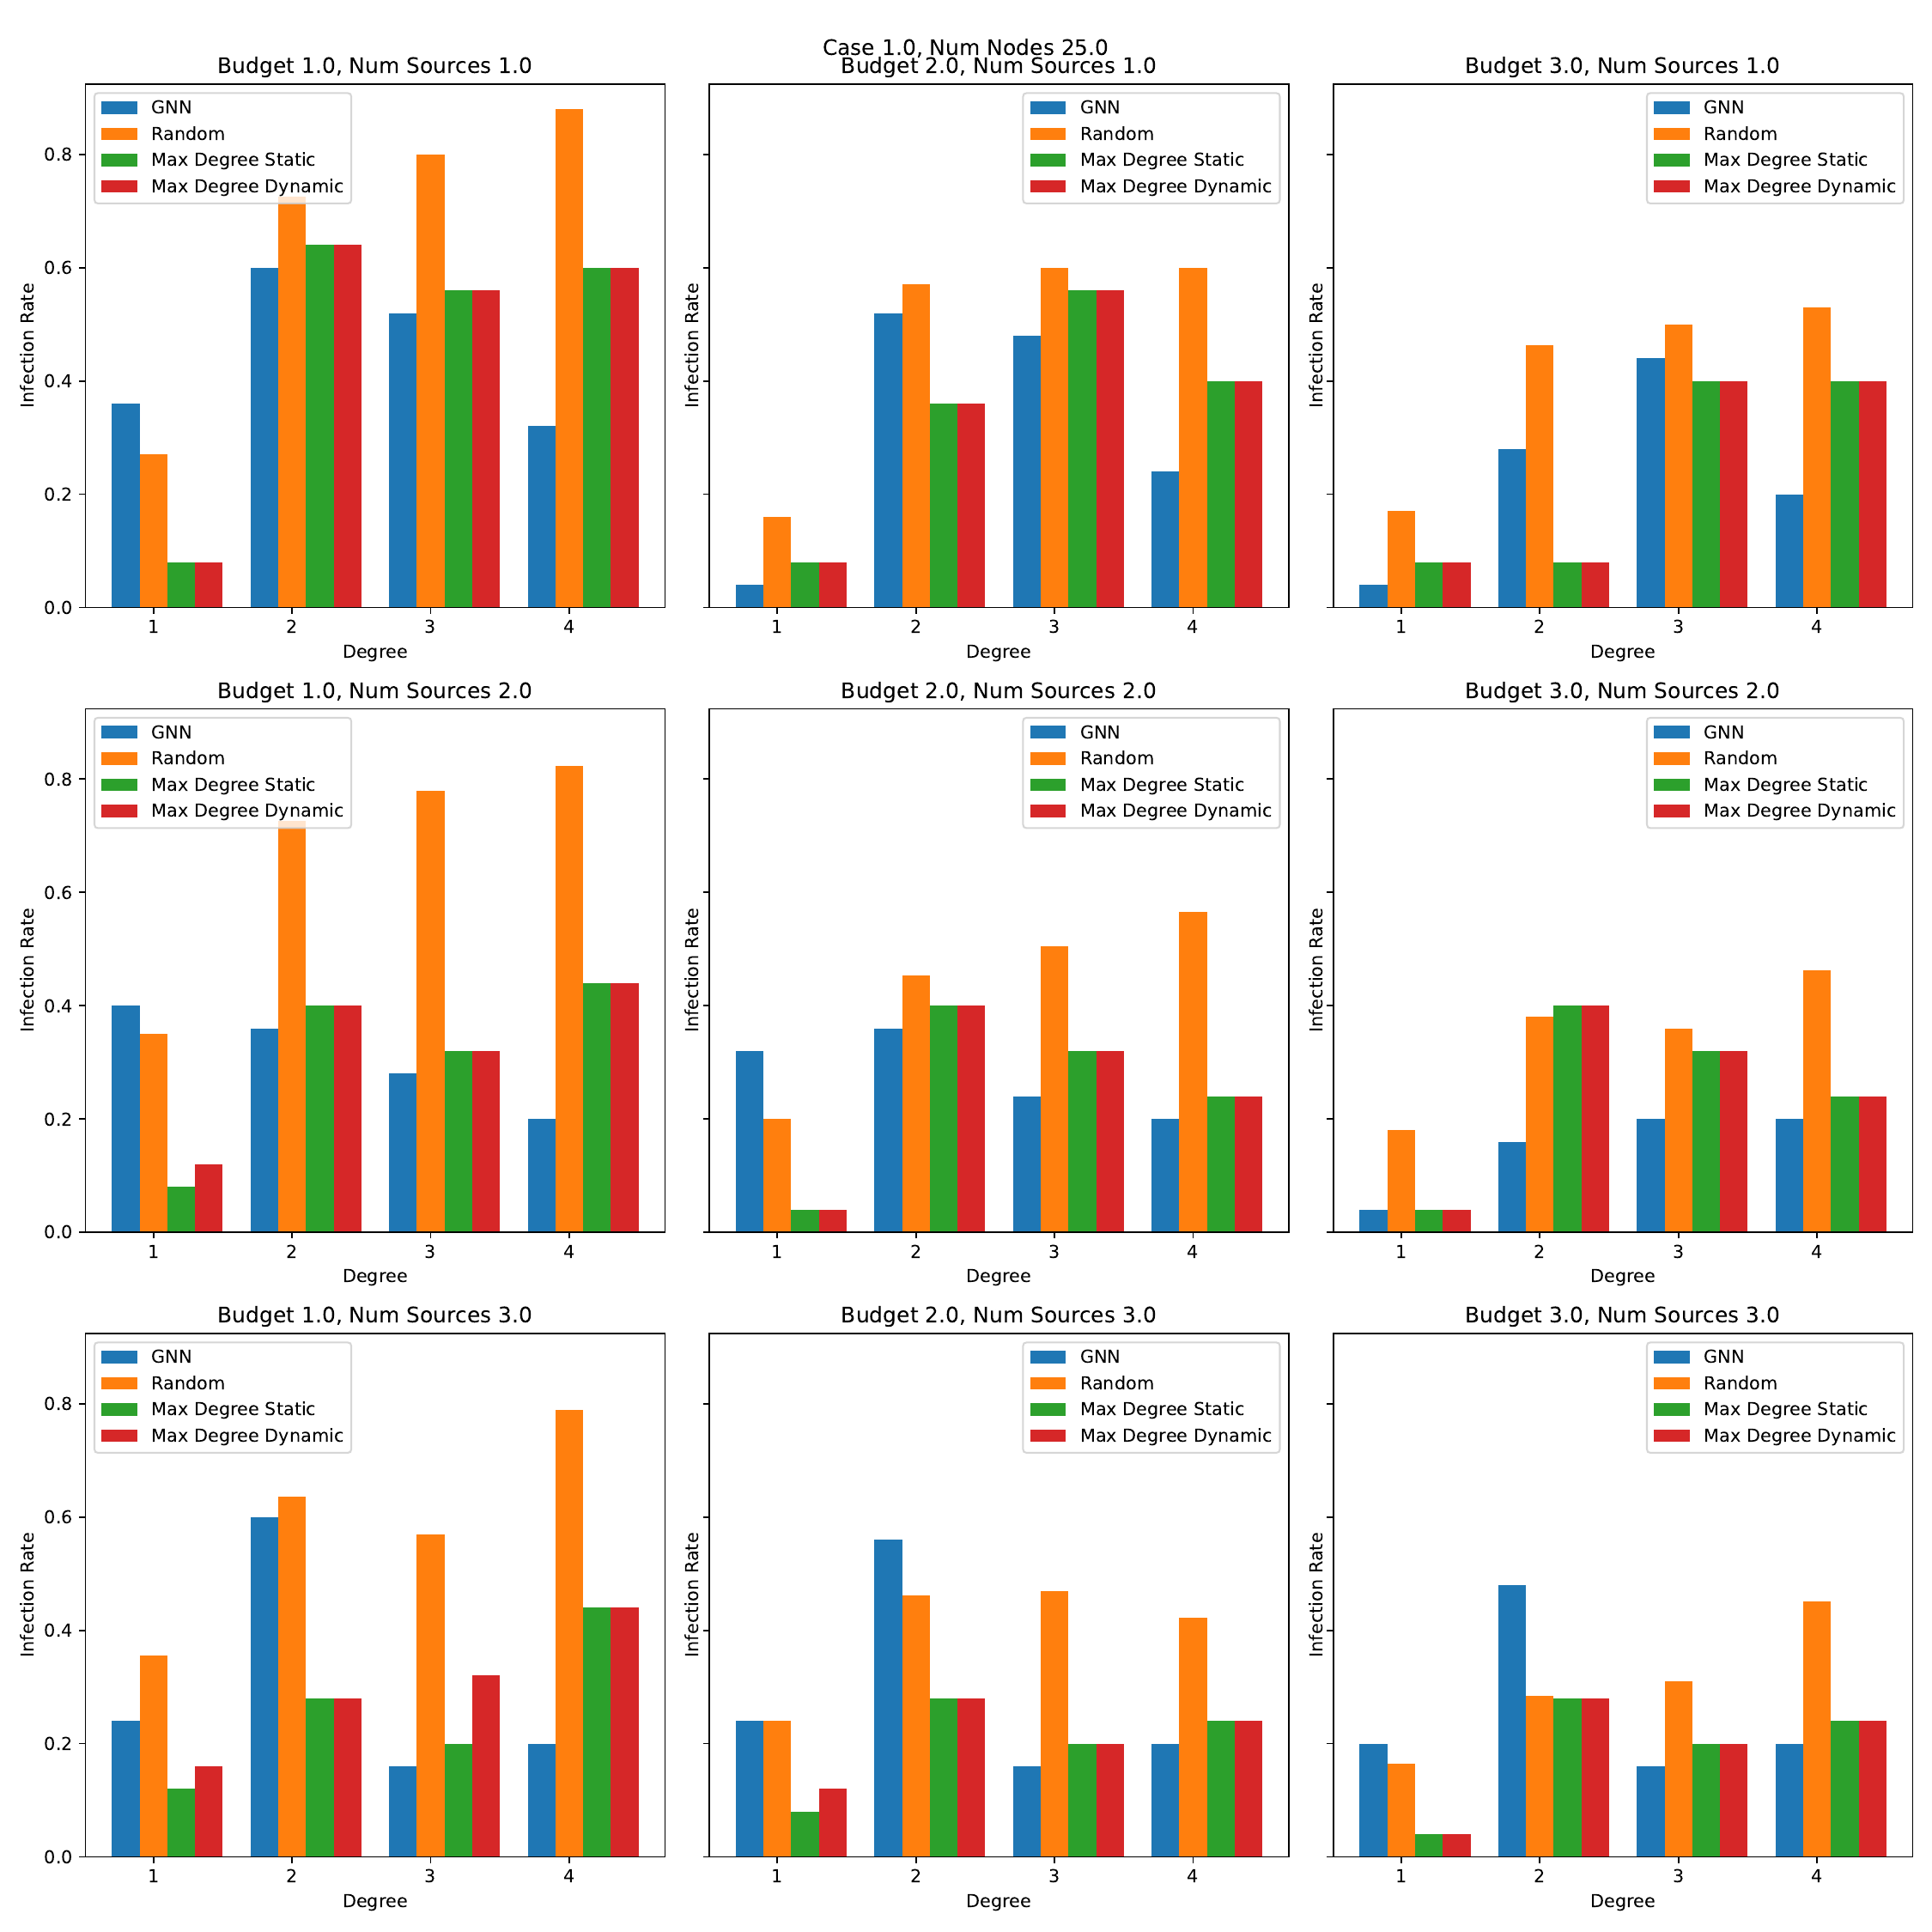}
    \caption{\footnotesize Dataset: Tree, Case-1 Node-25: Performance Evaluation of GCN-Based Supervised Learning Model: This series of bar plots presents a comparative analysis between our GCN-based SL model (blue), Randomized Policy model(yellow), Max Degree Policy model (Static) (green) and Max Degree Policy model (Dynamic) (red) on 25-node network environment. Progressing from left to right, the plots depict scenarios with increasing action budgets, ranging from 1 to 3 actions permitted. Vertically, the plots are ordered to show the effect of varying the initial count of infected nodes, starting with one and increasing to three. Each set of bars within the plots is categorized by the average connectivity (degree) of the infected nodes.}
    \label{fig:Treec1n25}
\end{figure}

\begin{figure}[!h]
    \centering
    \includegraphics[scale=0.3]{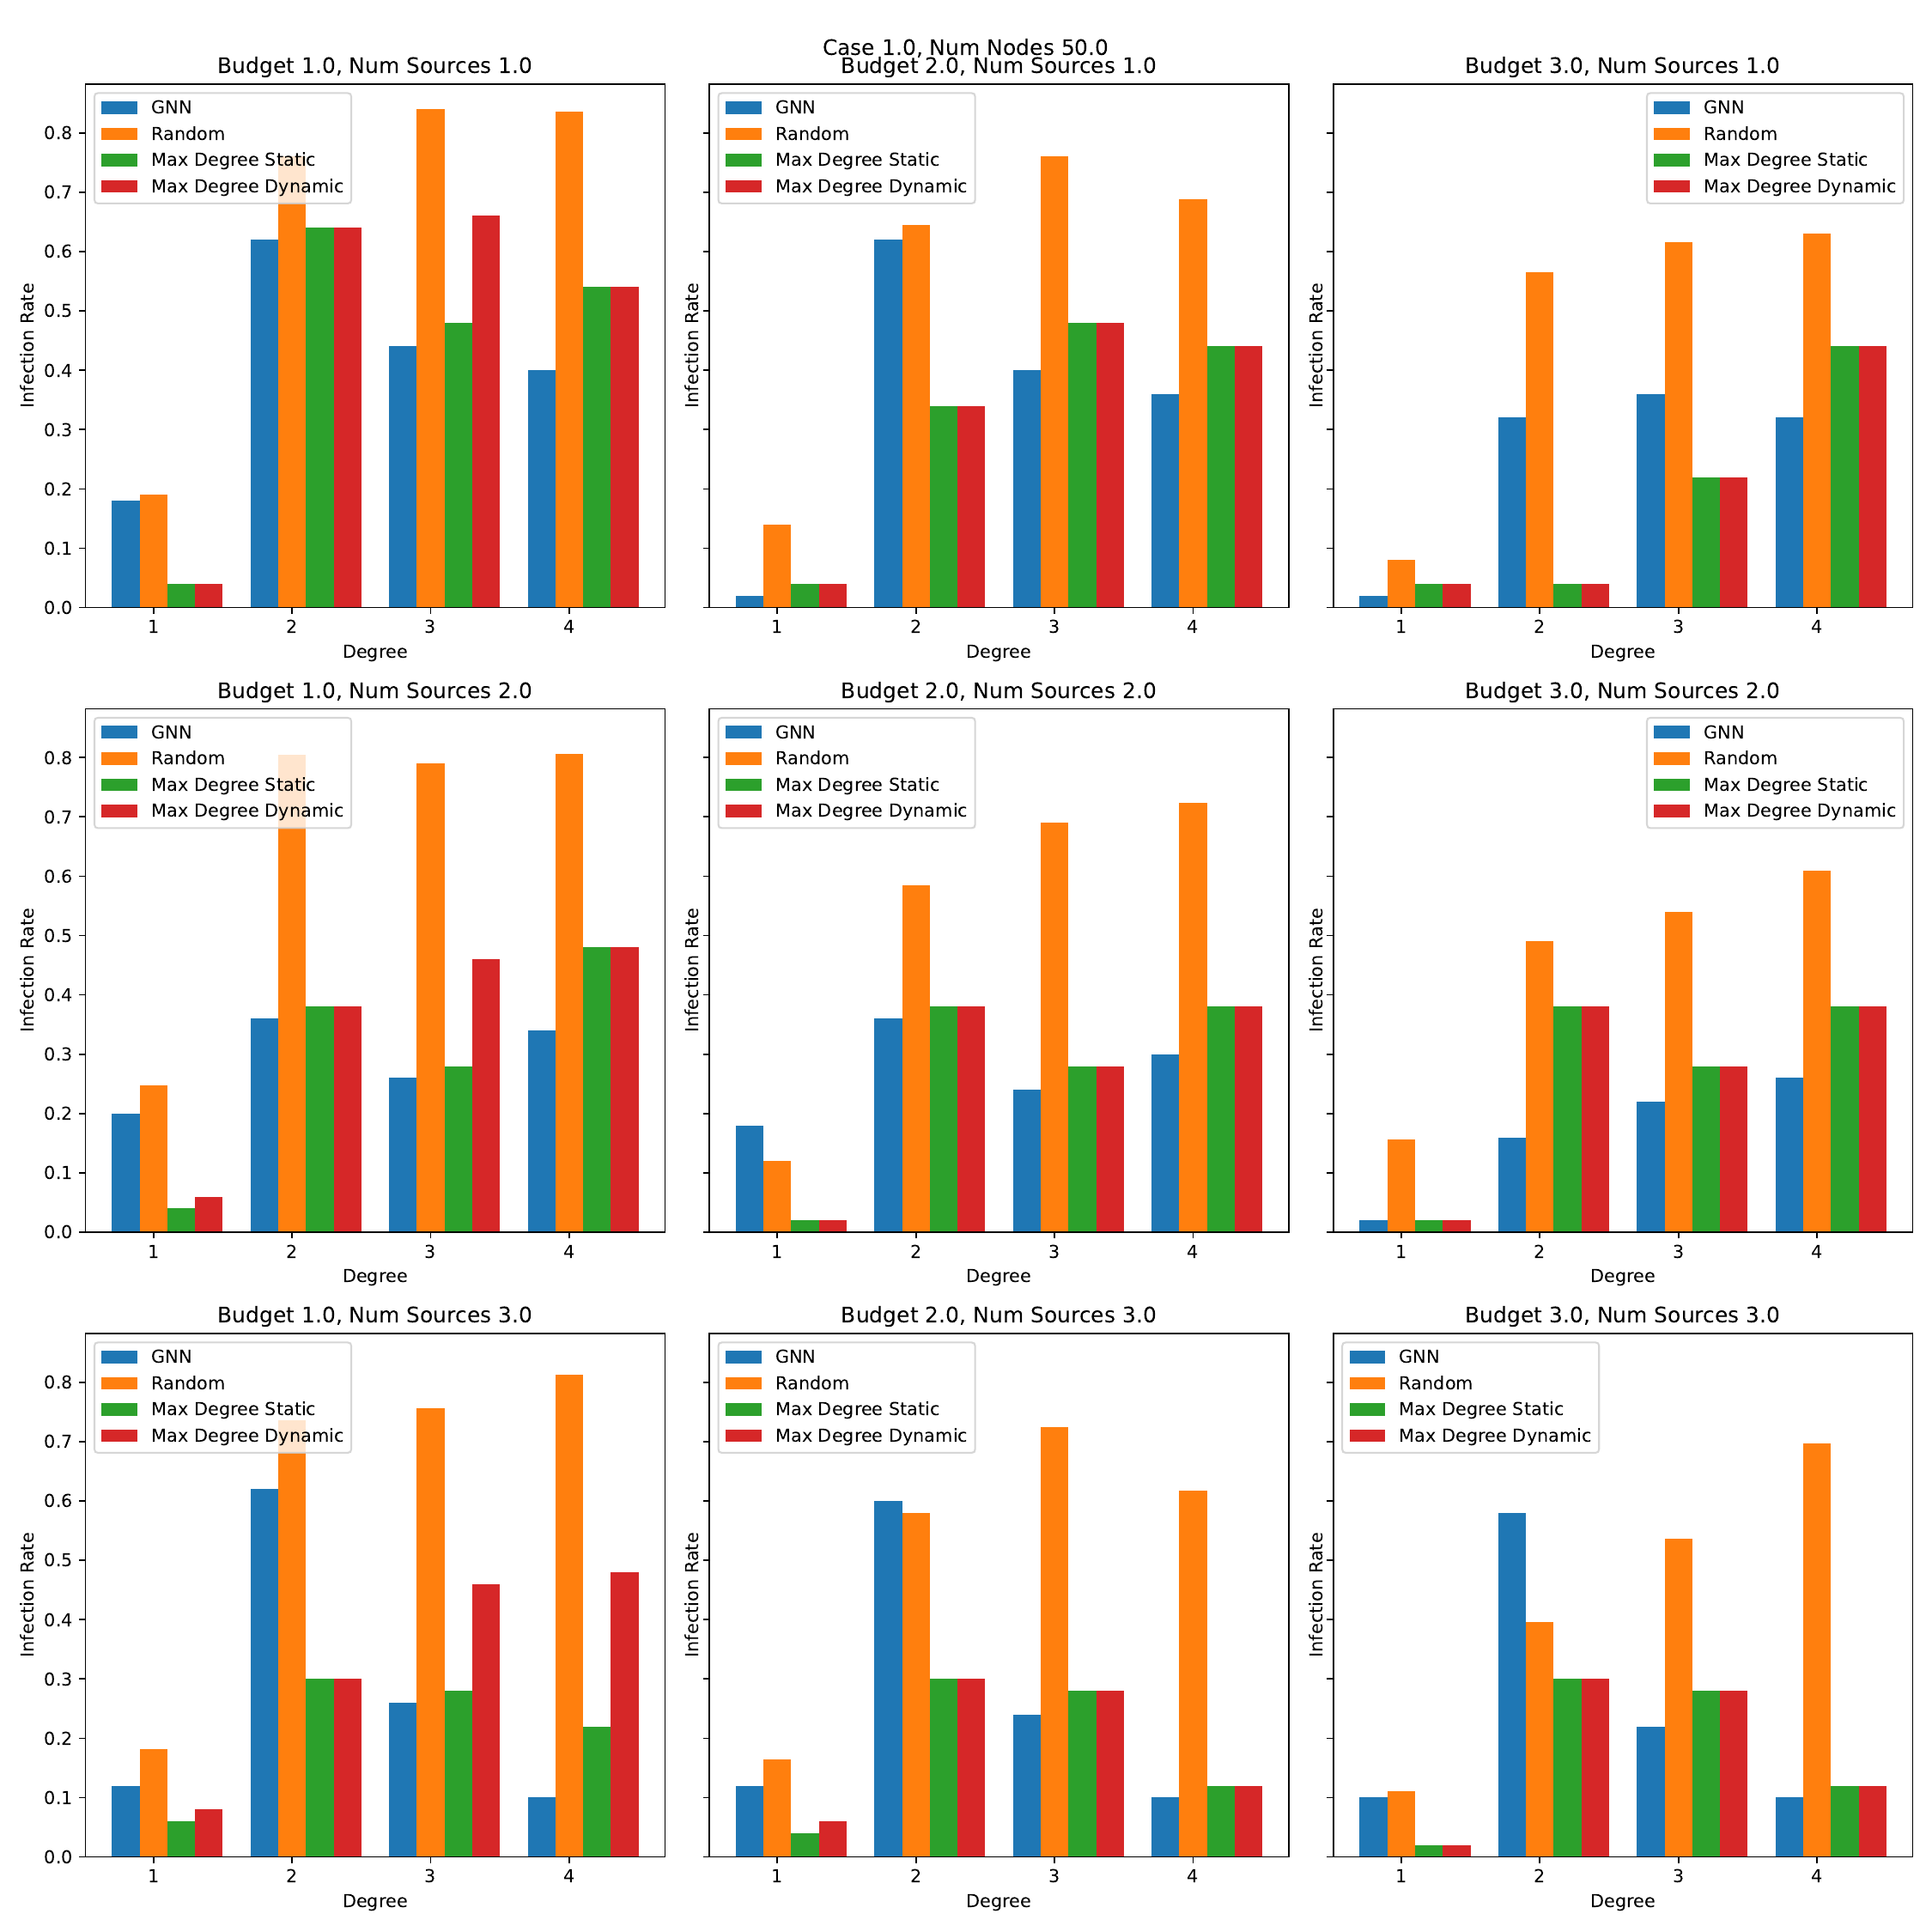}
    \caption{\footnotesize Dataset: Tree, Case-1 Node-50: Performance Evaluation of GCN-Based Supervised Learning Model: This series of bar plots presents a comparative analysis between our GCN-based SL model (blue), Randomized Policy model(yellow), Max Degree Policy model (Static) (green) and Max Degree Policy model (Dynamic) (red) on 25-node network environment. Progressing from left to right, the plots depict scenarios with increasing action budgets, ranging from 1 to 3 actions permitted. Vertically, the plots are ordered to show the effect of varying the initial count of infected nodes, starting with one and increasing to three. Each set of bars within the plots is categorized by the average connectivity (degree) of the infected nodes.}
    \label{fig:Treec1n50}
\end{figure}

\begin{figure}[!h]
    \centering
    \includegraphics[scale=0.3]{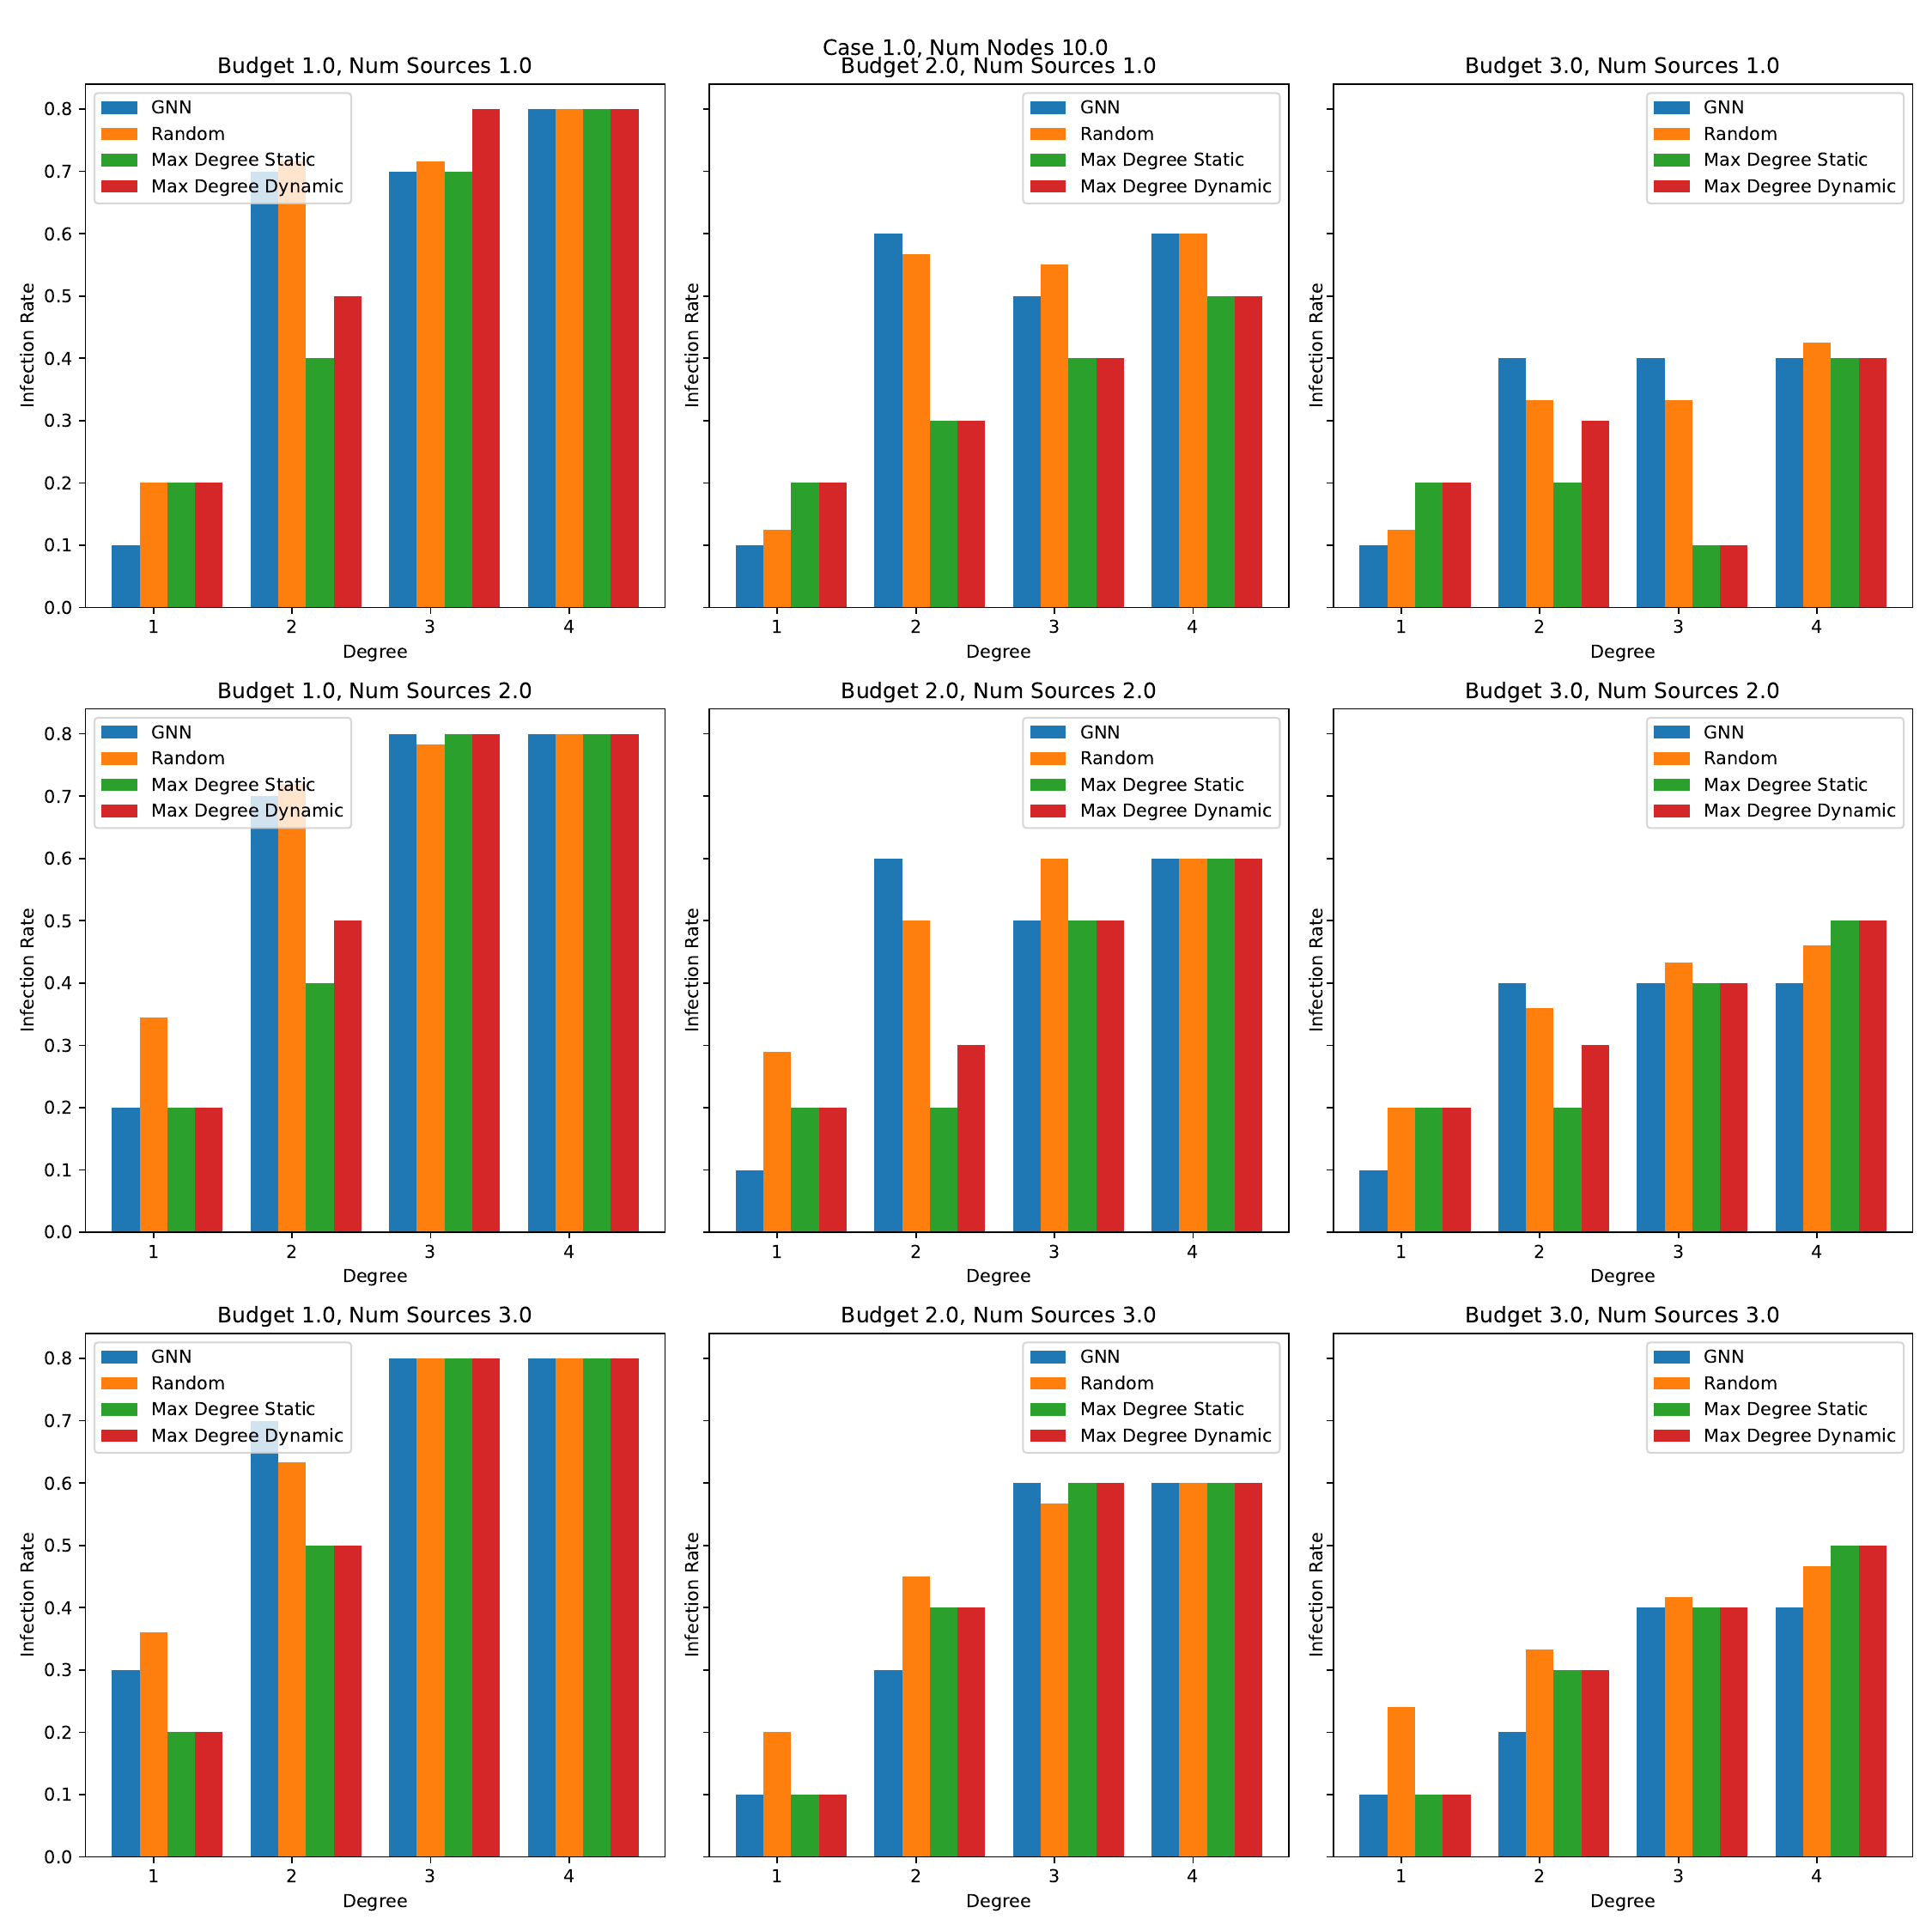}
    \caption{\footnotesize Dataset: Erdos-Renyi, Case-1 Node-10: Performance Evaluation of GCN-Based Supervised Learning Model: This series of bar plots presents a comparative analysis between our GCN-based SL model (blue), Randomized Policy model(yellow), Max Degree Policy model (Static) (green) and Max Degree Policy model (Dynamic) (red) on 10-node network environment. Progressing from left to right, the plots depict scenarios with increasing action budgets, ranging from 1 to 3 actions permitted. Vertically, the plots are ordered to show the effect of varying the initial count of infected nodes, starting with one and increasing to three. Each set of bars within the plots is categorized by the average connectivity (degree) of the infected nodes.}
    \label{fig:ERc1n10}
\end{figure}

\begin{figure}[!h]
    \centering
    \includegraphics[scale=0.3]{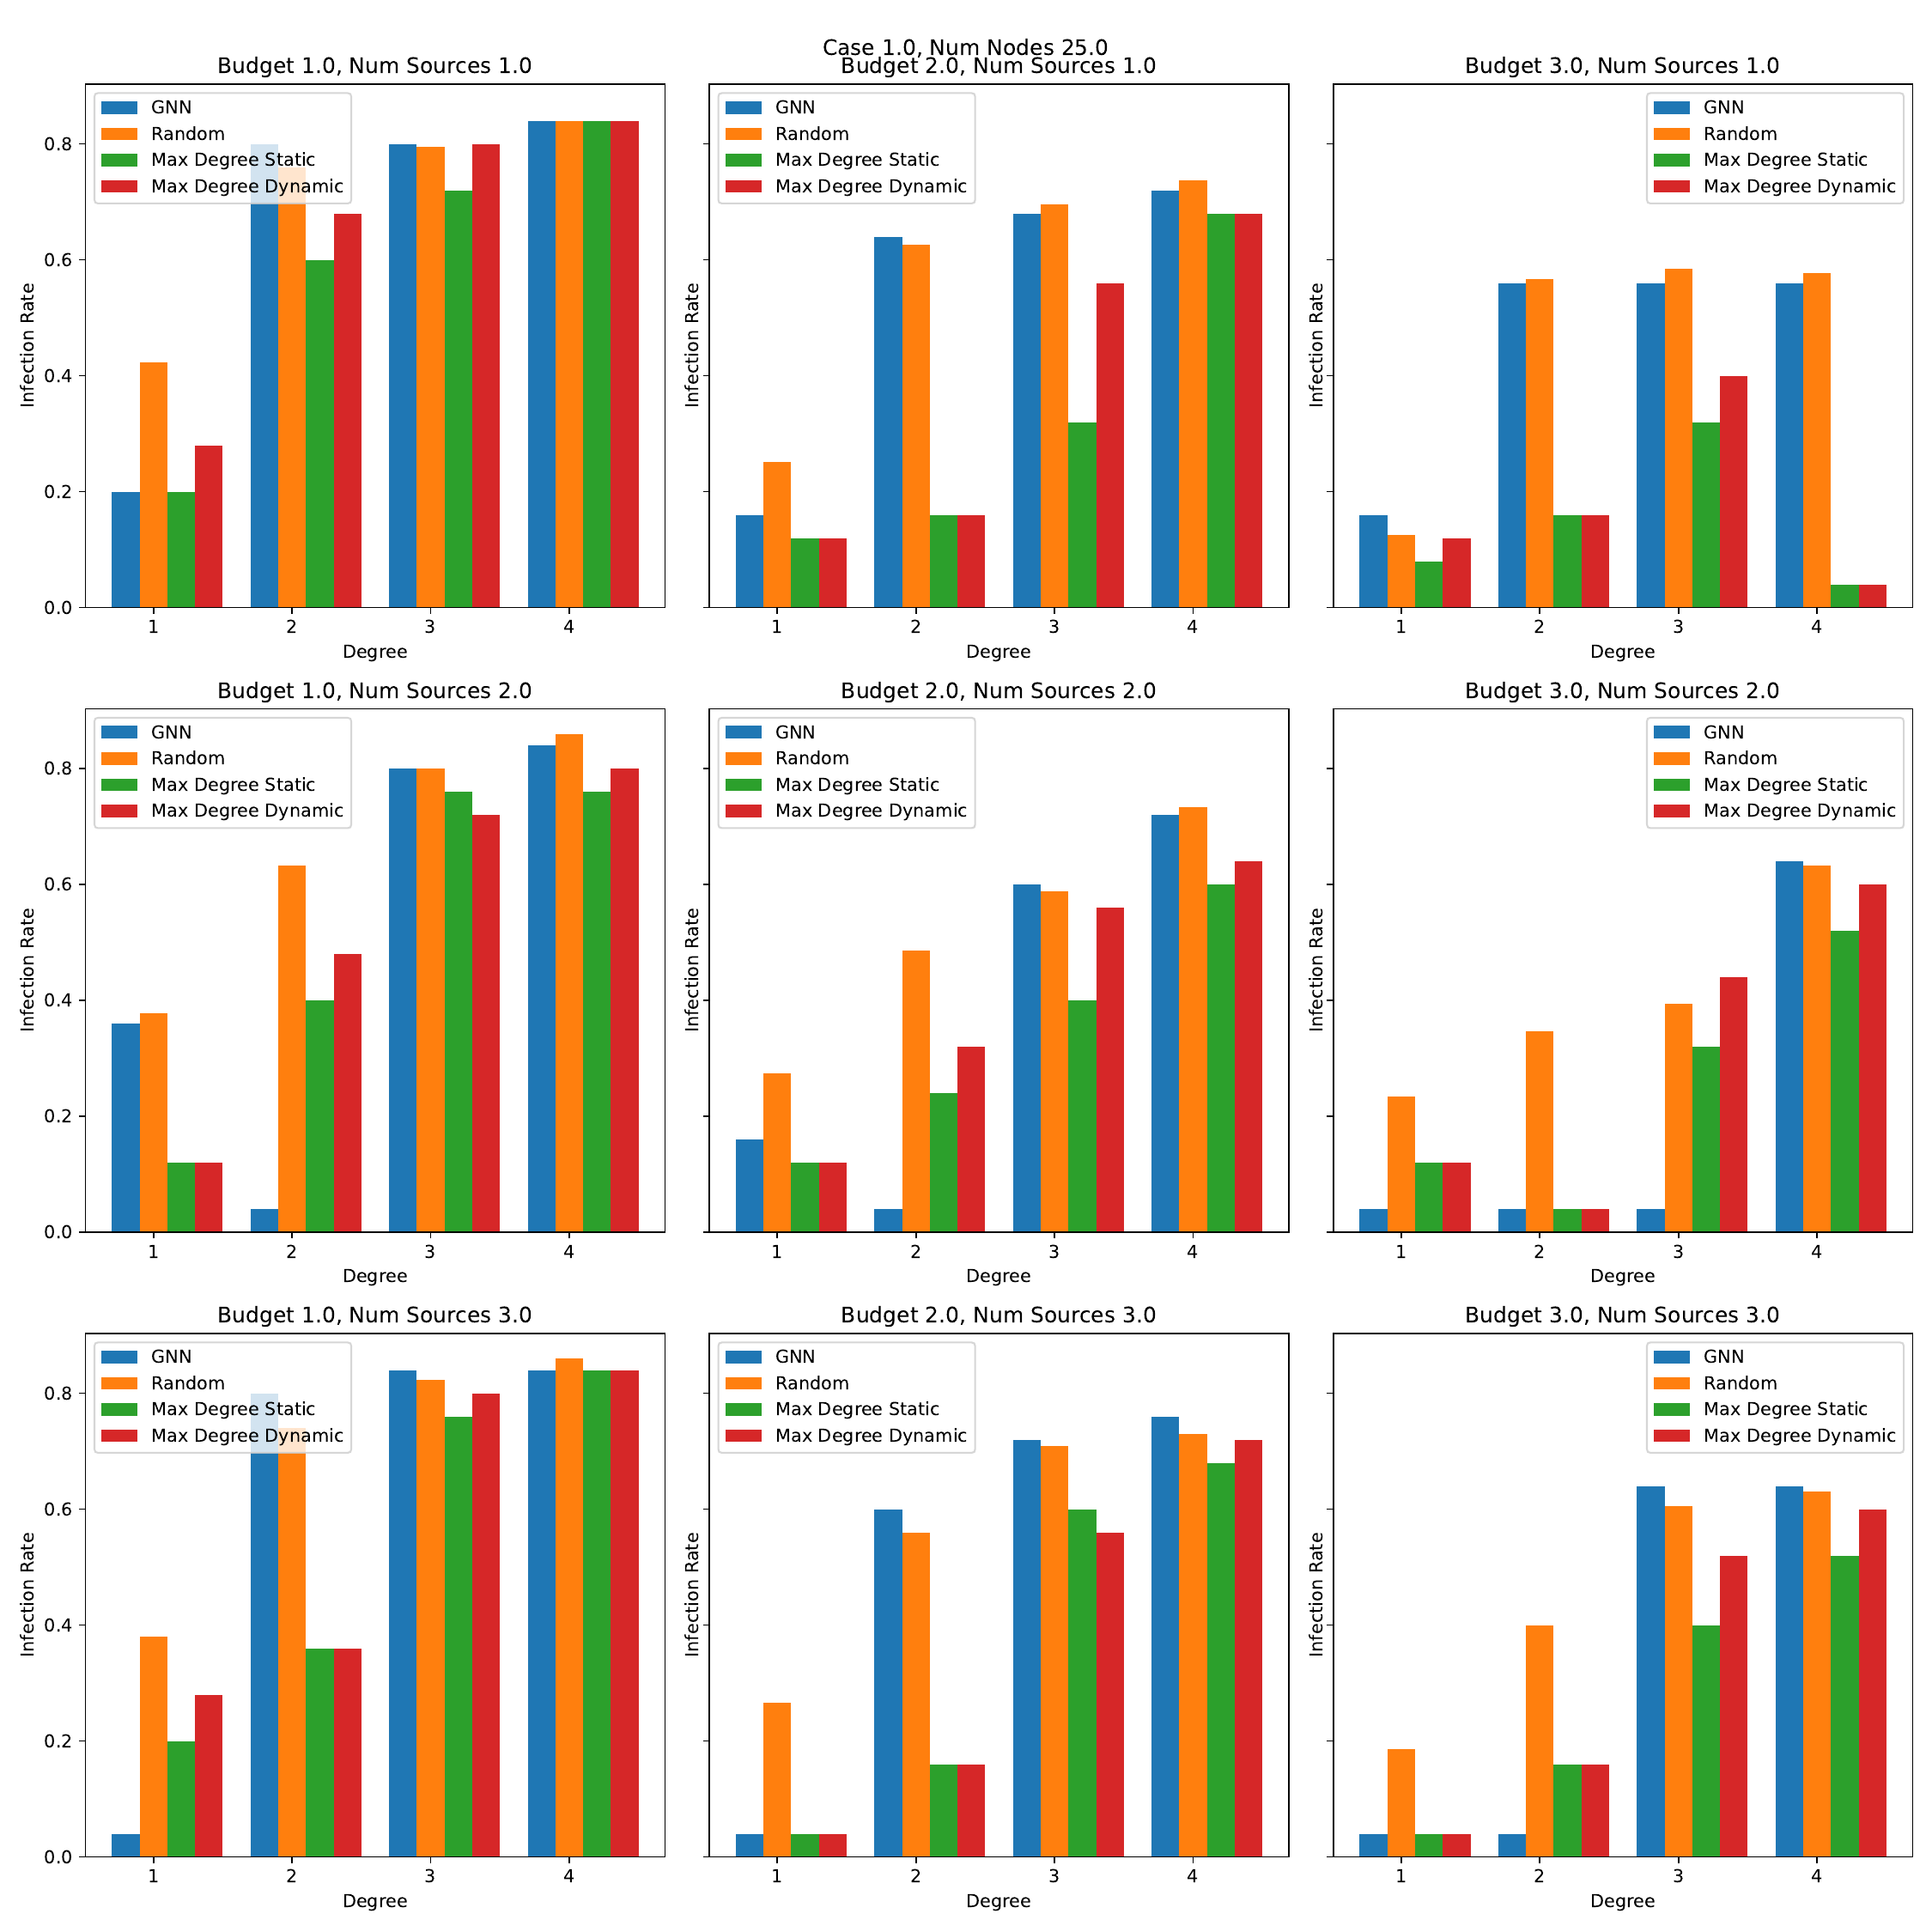}
    \caption{\footnotesize Dataset: Erdos-Renyi, Case-1 Node-25: Performance Evaluation of GCN-Based Supervised Learning Model: This series of bar plots presents a comparative analysis between our GCN-based SL model (blue), Randomized Policy model(yellow), Max Degree Policy model (Static) (green) and Max Degree Policy model (Dynamic) (red) on 25-node network environment. Progressing from left to right, the plots depict scenarios with increasing action budgets, ranging from 1 to 3 actions permitted. Vertically, the plots are ordered to show the effect of varying the initial count of infected nodes, starting with one and increasing to three. Each set of bars within the plots is categorized by the average connectivity (degree) of the infected nodes.}
    \label{fig:ERc1n25}
\end{figure}

\begin{figure}[!h]
    \centering
    \includegraphics[scale=0.3]{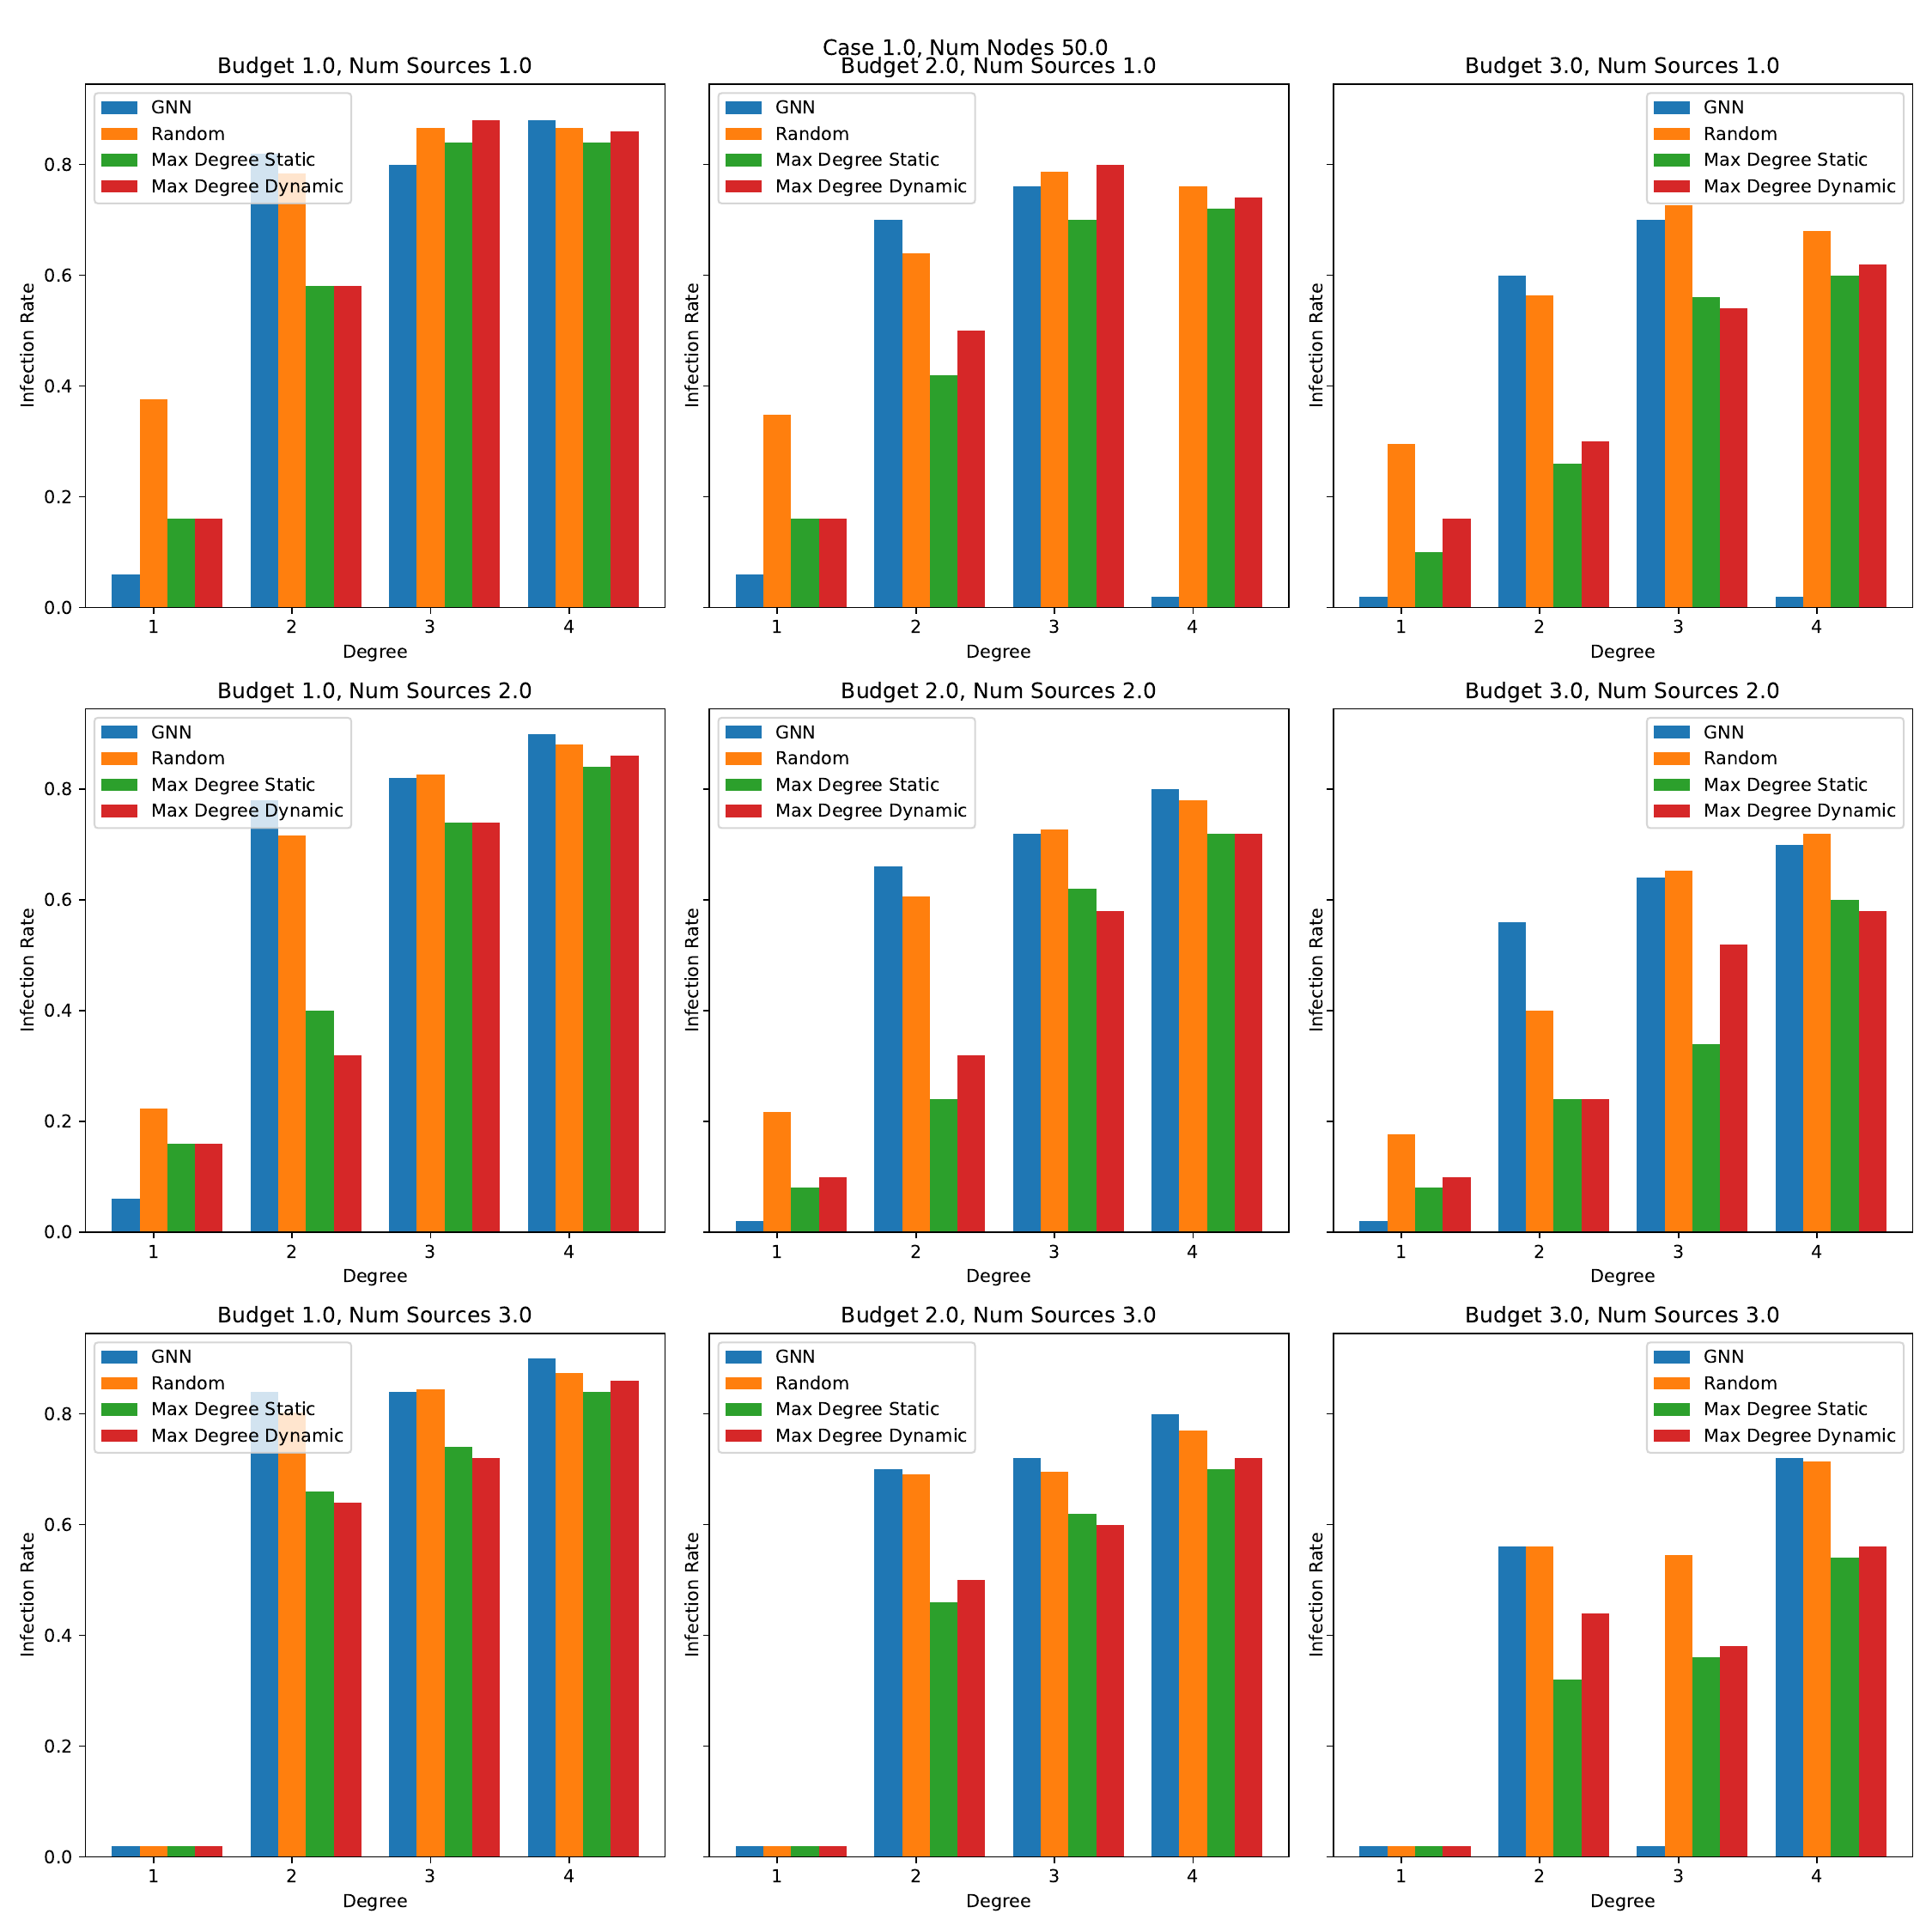}
    \caption{\footnotesize Dataset: Erdos-Renyi, Case-1 Node-50: Performance Evaluation of GCN-Based Supervised Learning Model: This series of bar plots presents a comparative analysis between our GCN-based SL model (blue), Randomized Policy model(yellow), Max Degree Policy model (Static) (green) and Max Degree Policy model (Dynamic) (red) on 25-node network environment. Progressing from left to right, the plots depict scenarios with increasing action budgets, ranging from 1 to 3 actions permitted. Vertically, the plots are ordered to show the effect of varying the initial count of infected nodes, starting with one and increasing to three. Each set of bars within the plots is categorized by the average connectivity (degree) of the infected nodes.}
    \label{fig:ERc1n50}
\end{figure}

% ######## Case 2 #########

\begin{figure}[!h]
    \centering
    \includegraphics[scale=0.3]{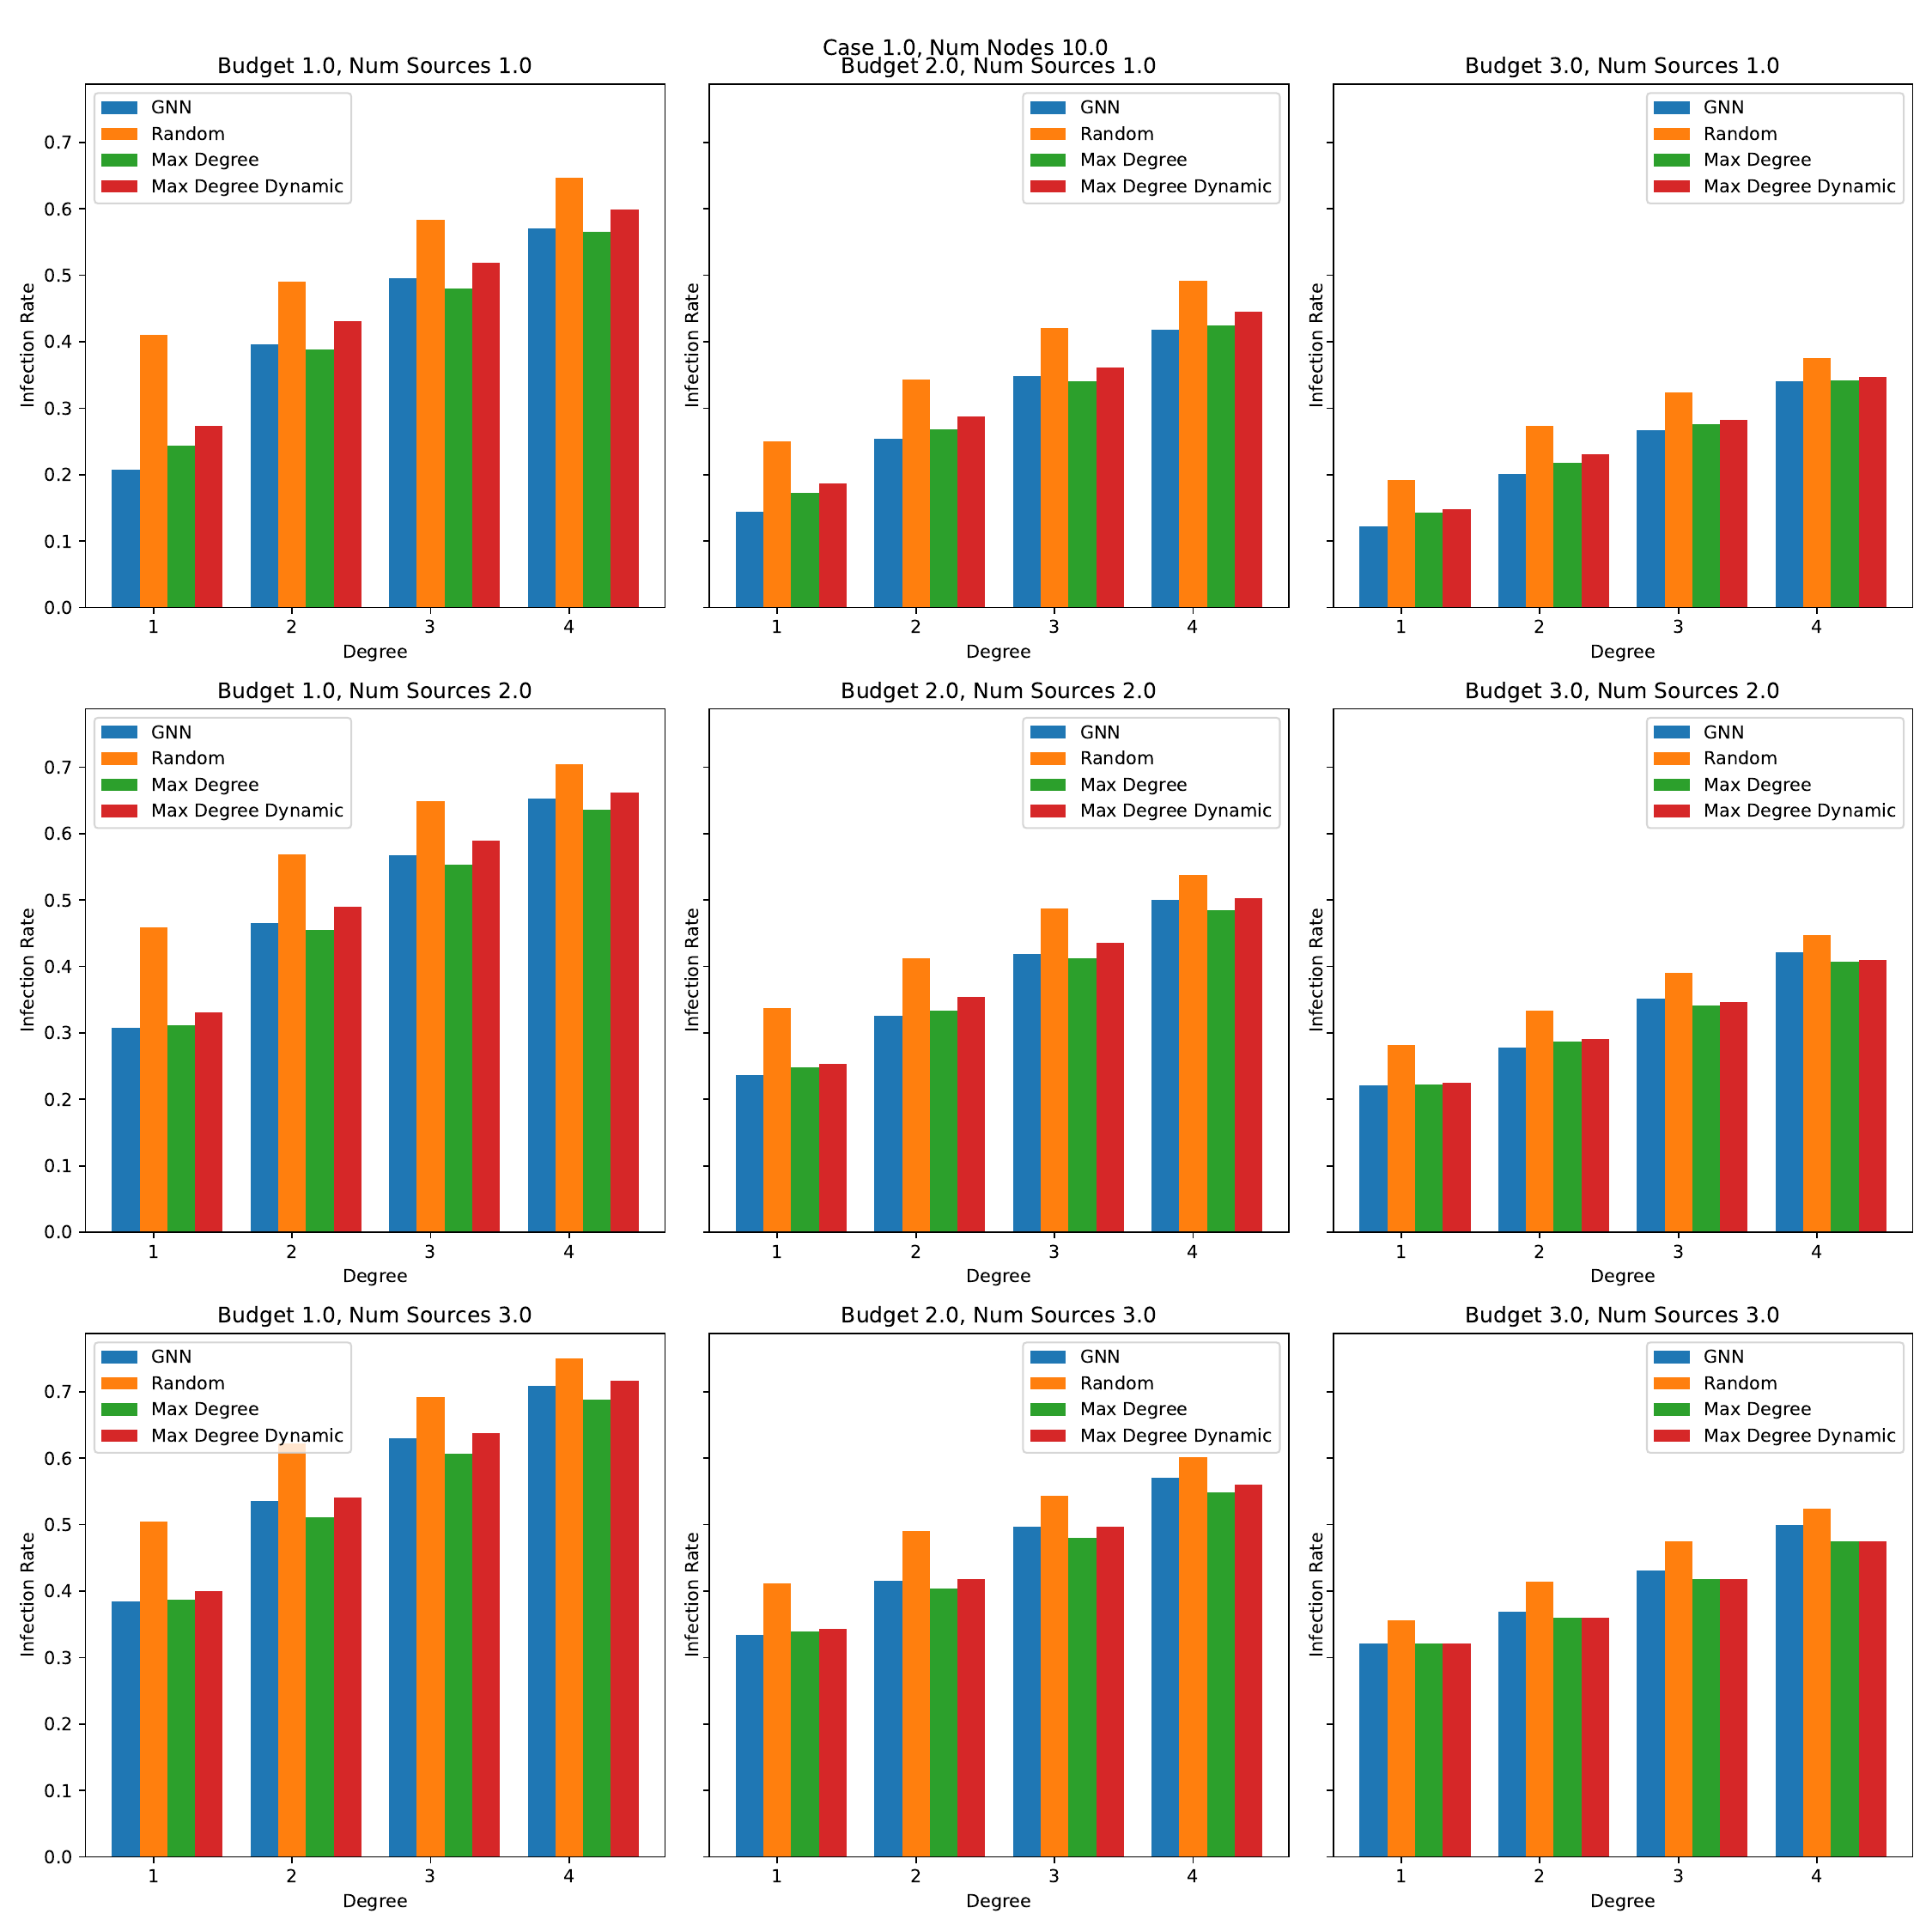}
    \caption{\footnotesize Dataset: Watts-Strogatz, Case-2 Node-10: Performance Evaluation of GCN-Based Supervised Learning Model: This series of bar plots presents a comparative analysis between our GCN-based SL model (blue), Randomized Policy model(yellow), Max Degree Policy model (Static) (green) and Max Degree Policy model (Dynamic) (red) on 10-node network environment. Progressing from left to right, the plots depict scenarios with increasing action budgets, ranging from 1 to 3 actions permitted. Vertically, the plots are ordered to show the effect of varying the initial count of infected nodes, starting with one and increasing to three. Each set of bars within the plots is categorized by the average connectivity (degree) of the infected nodes.}
    \label{fig:c2n10}
\end{figure}

\begin{figure}[!h]
    \centering
    \includegraphics[scale=0.3]{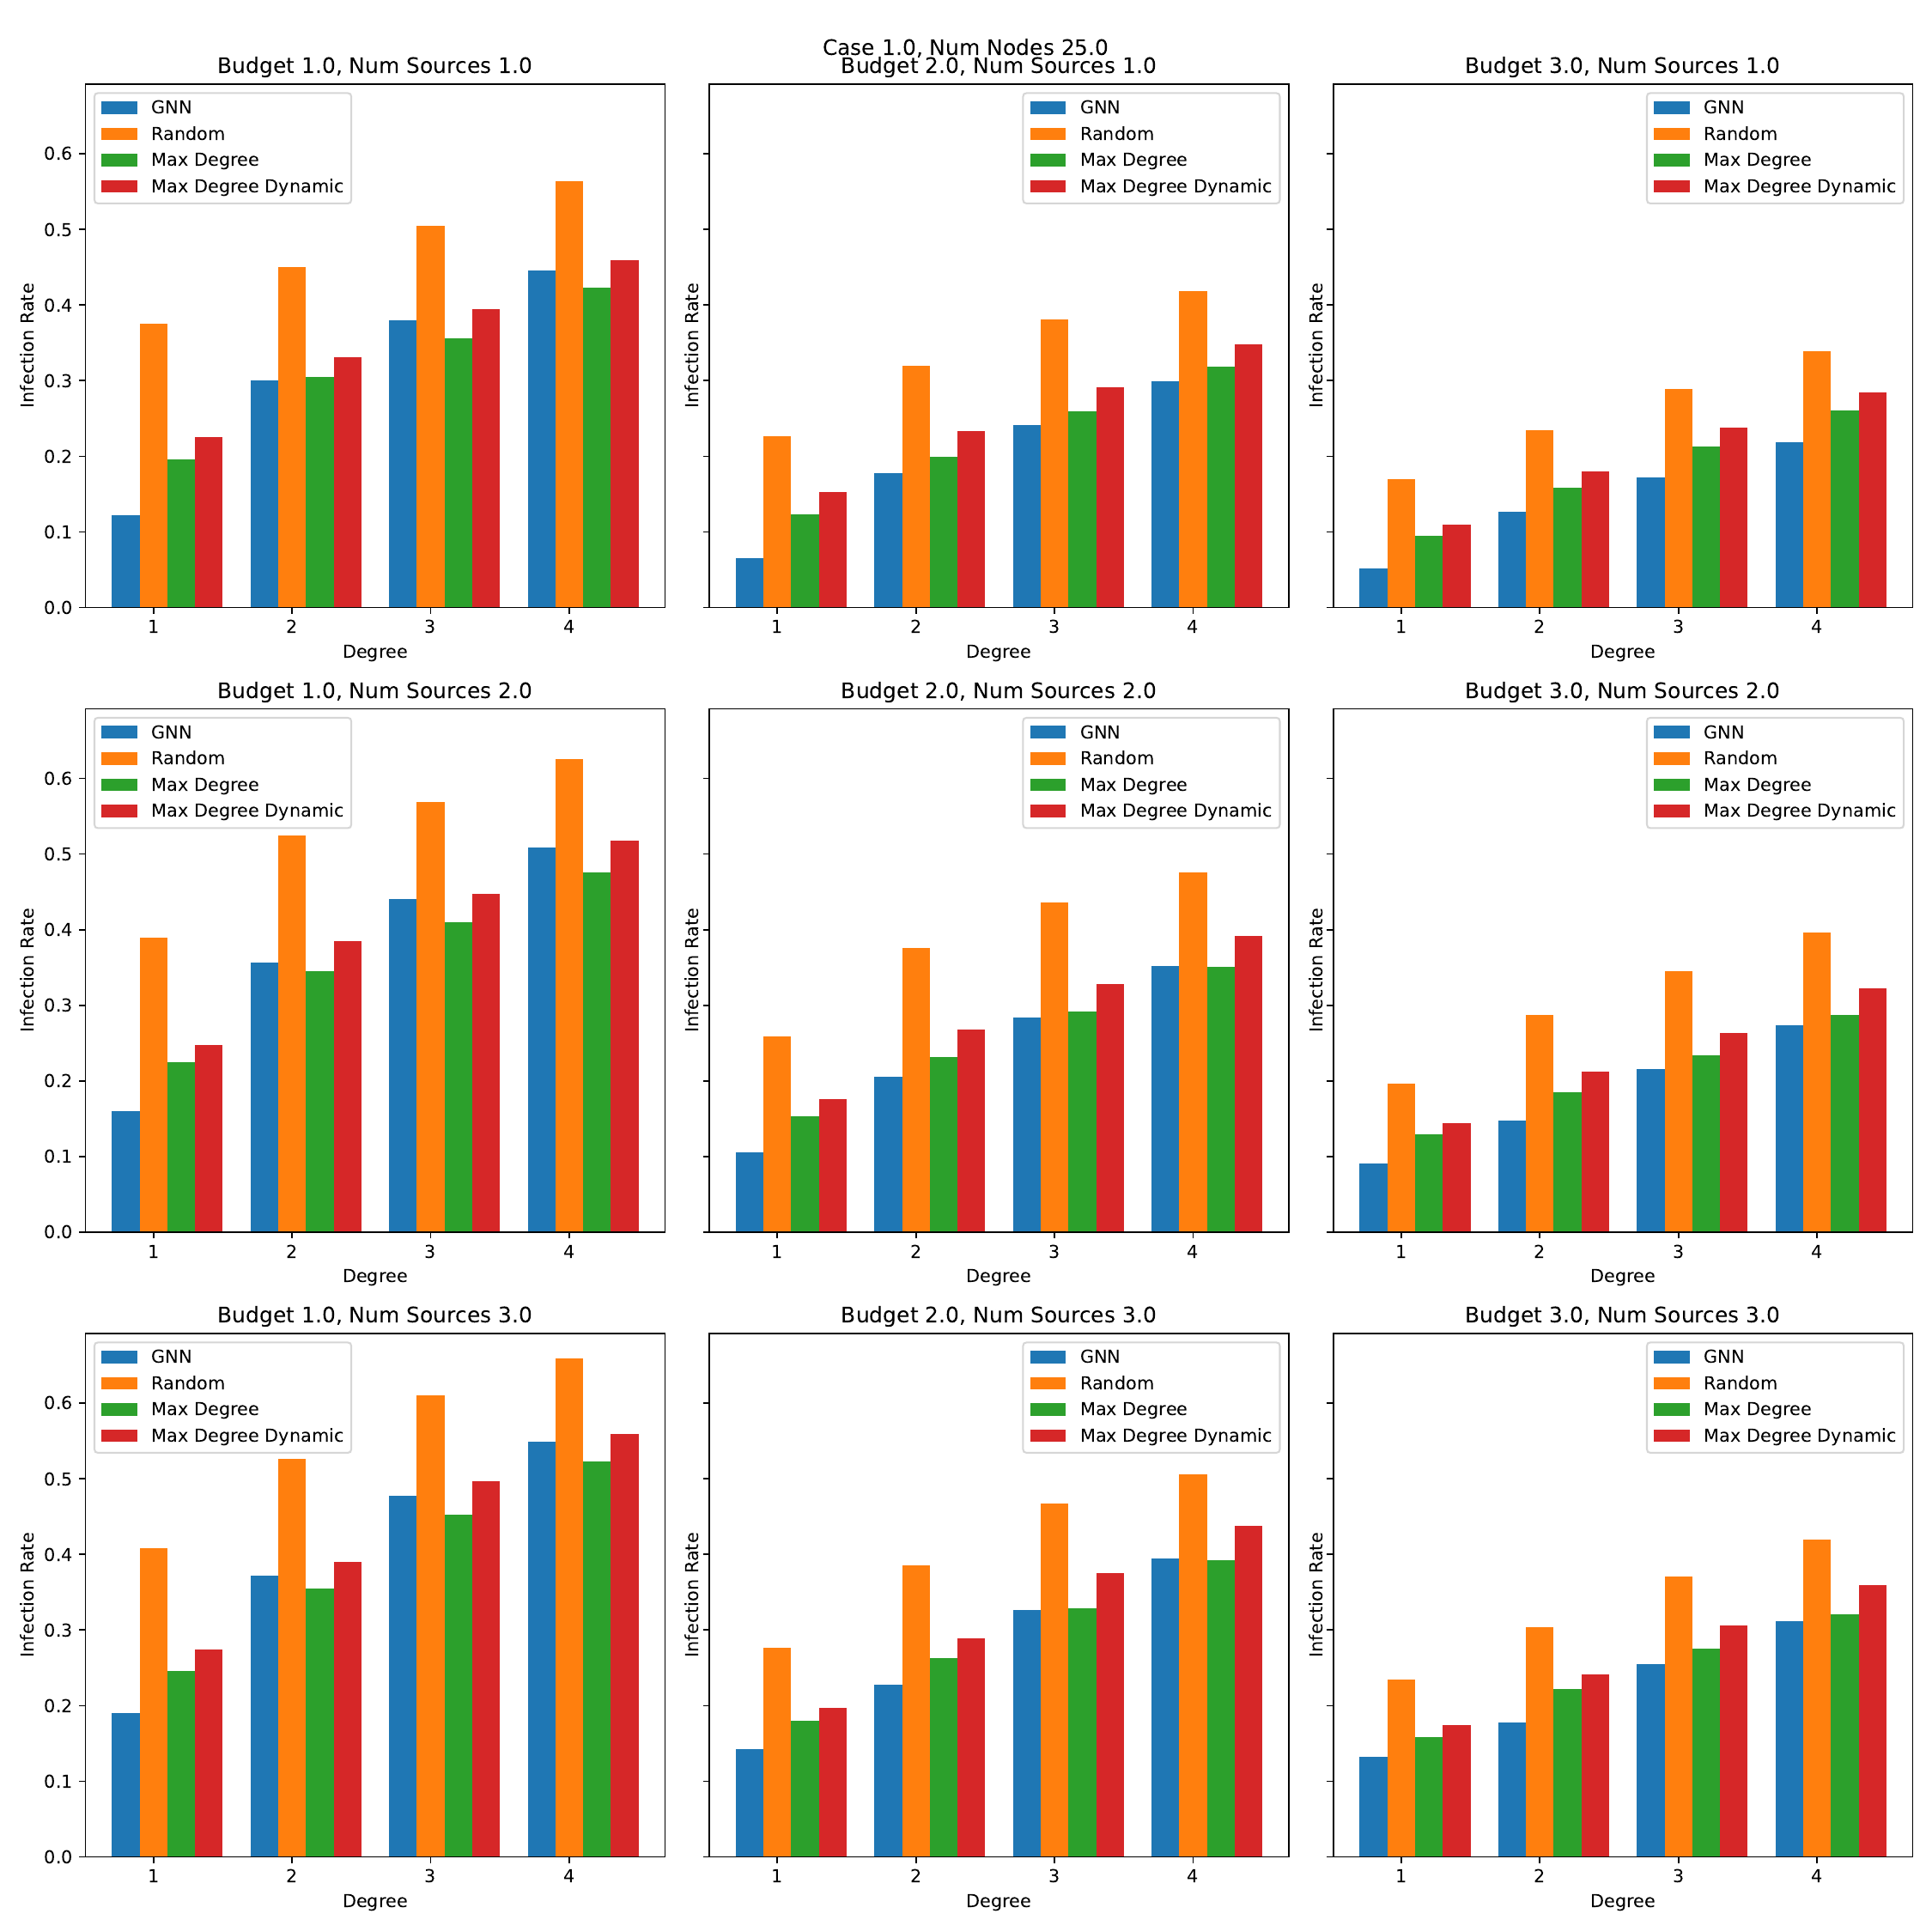}
    \caption{\footnotesize Dataset: Watts-Strogatz, Case-2 Node-25: Performance Evaluation of GCN-Based Supervised Learning Model: This series of bar plots presents a comparative analysis between our GCN-based SL model (blue), Randomized Policy model(yellow), Max Degree Policy model (Static) (green) and Max Degree Policy model (Dynamic) (red) on 25-node network environment. Progressing from left to right, the plots depict scenarios with increasing action budgets, ranging from 1 to 3 actions permitted. Vertically, the plots are ordered to show the effect of varying the initial count of infected nodes, starting with one and increasing to three. Each set of bars within the plots is categorized by the average connectivity (degree) of the infected nodes.}
    \label{fig:c2n25}
\end{figure}

\begin{figure}[!h]
    \centering
    \includegraphics[scale=0.3]{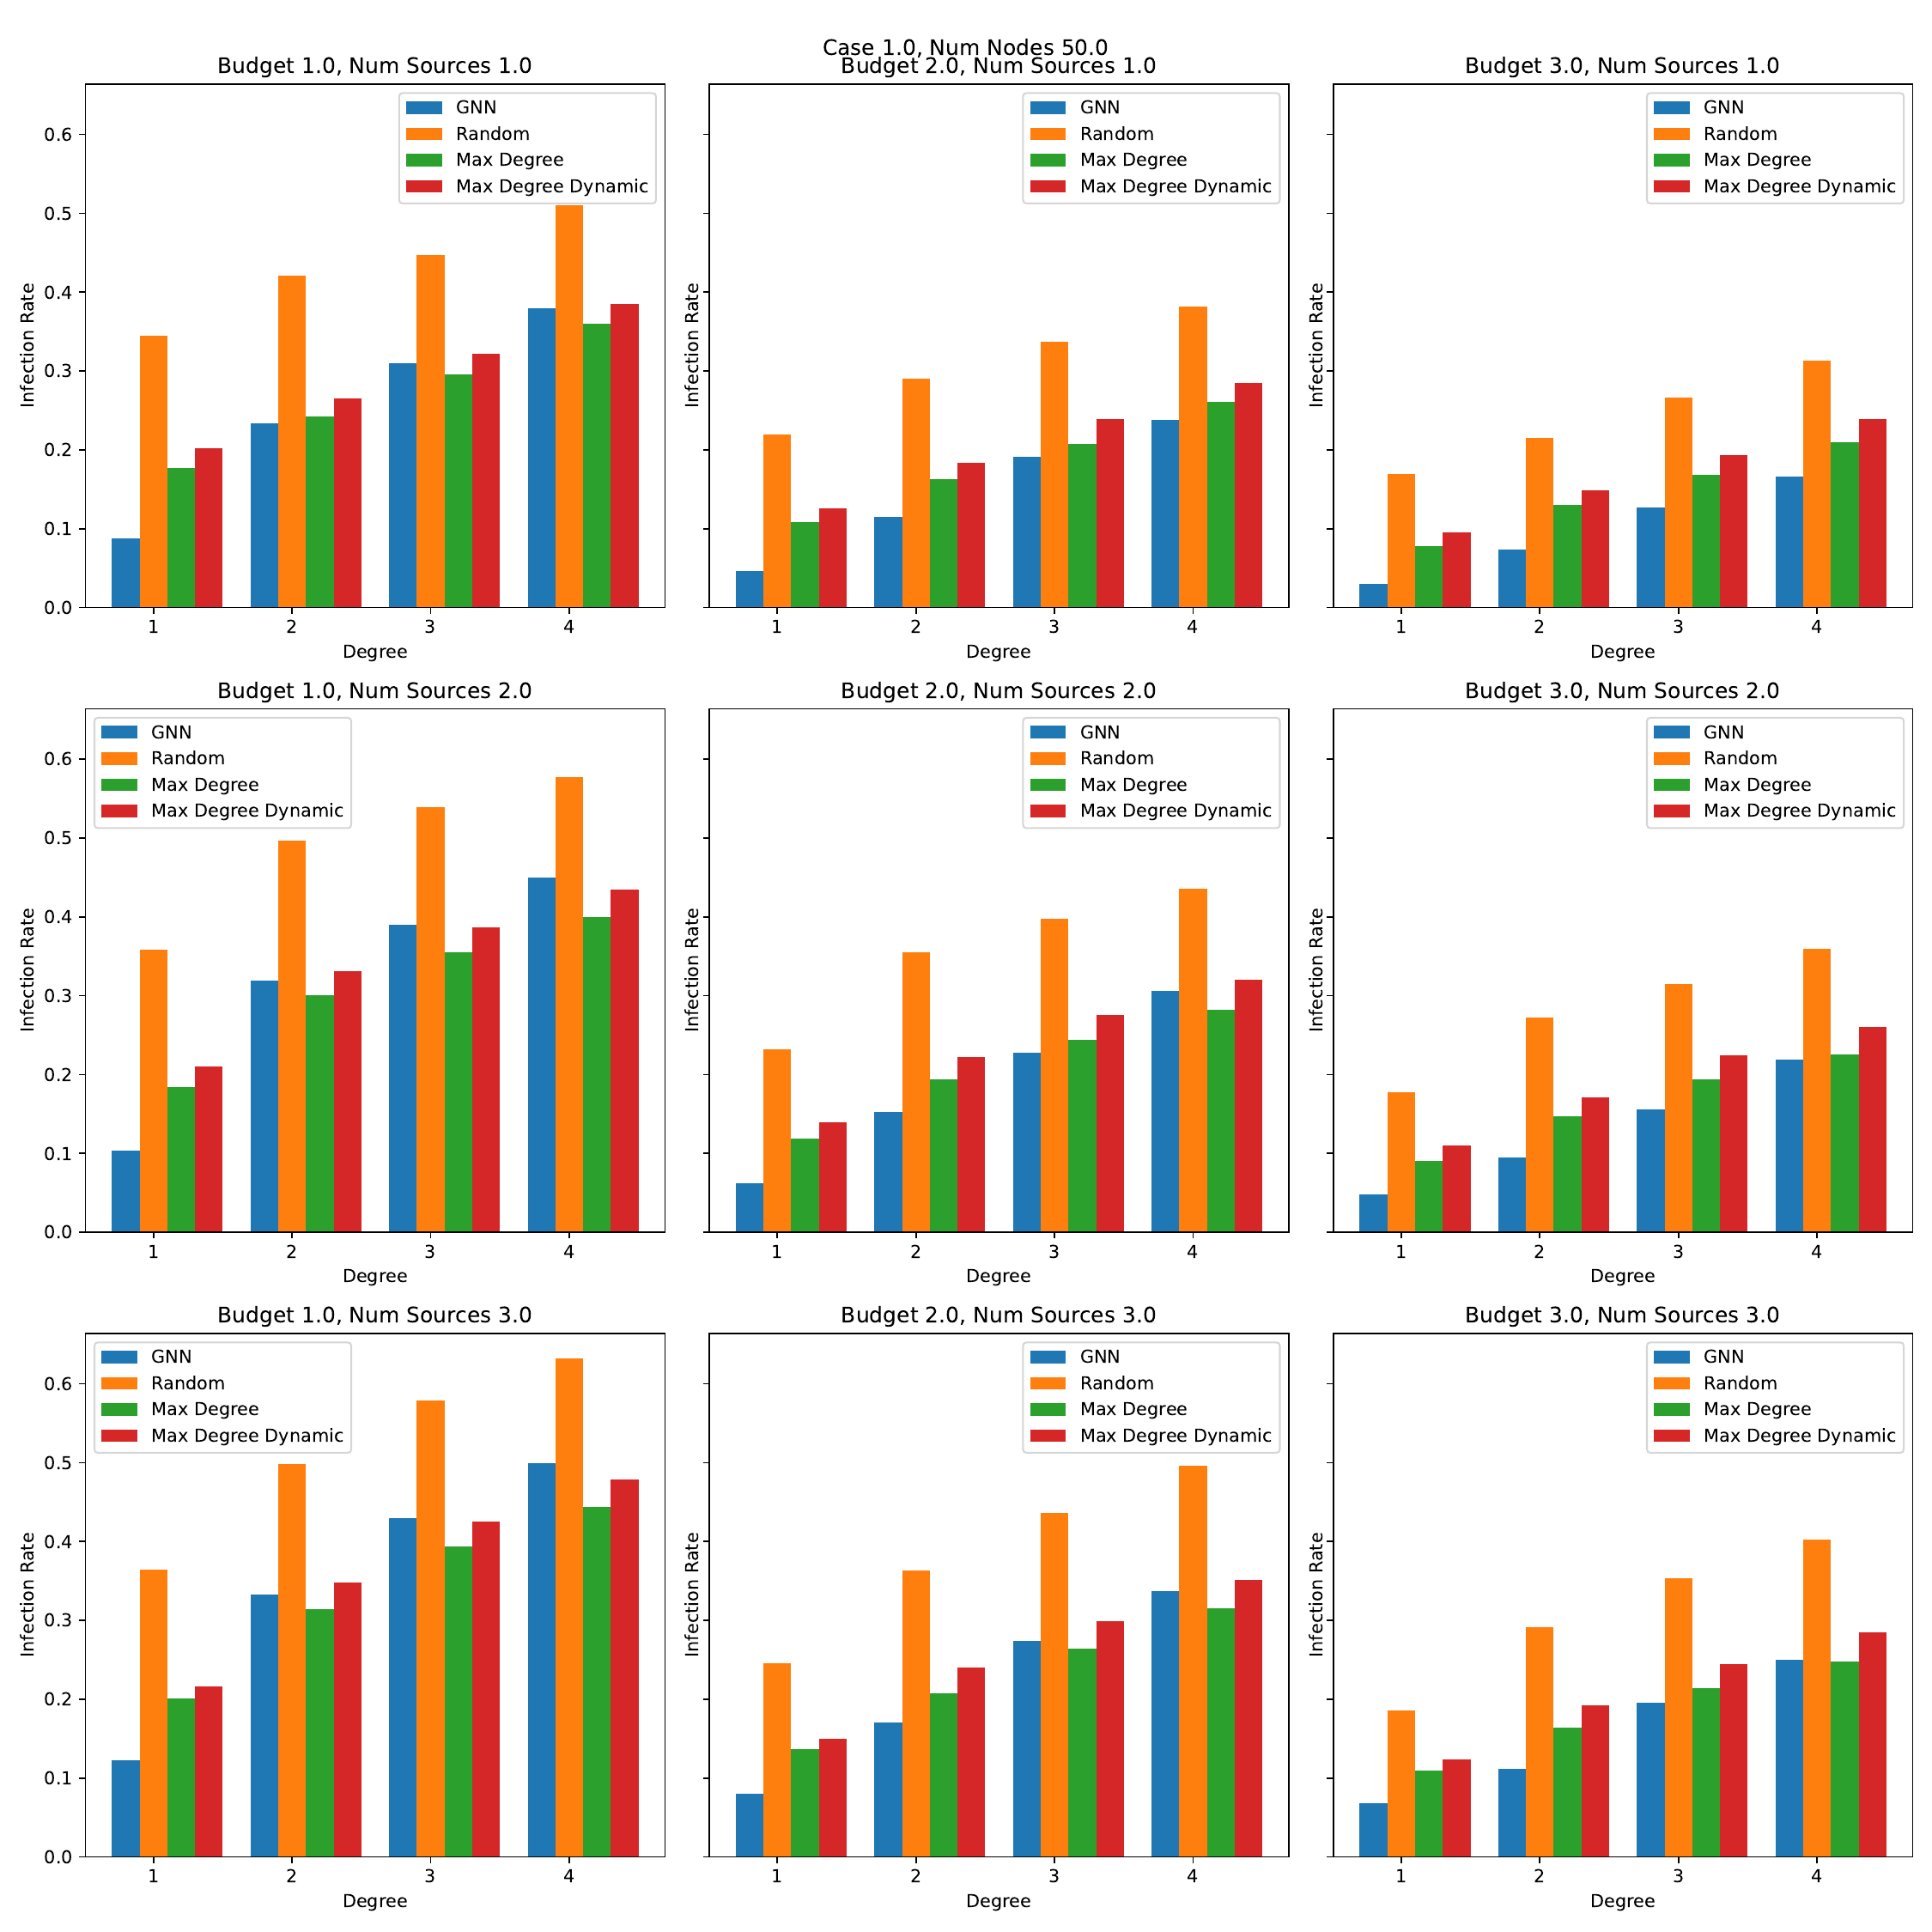}
    \caption{\footnotesize Dataset: Watts-Strogatz, Case-2 Node-50: Performance Evaluation of GCN-Based Supervised Learning Model: This series of bar plots presents a comparative analysis between our GCN-based SL model (blue), Randomized Policy model(yellow), Max Degree Policy model (Static) (green) and Max Degree Policy model (Dynamic) (red) on 50-node network environment. Progressing from left to right, the plots depict scenarios with increasing action budgets, ranging from 1 to 3 actions permitted. Vertically, the plots are ordered to show the effect of varying the initial count of infected nodes, starting with one and increasing to three. Each set of bars within the plots is categorized by the average connectivity (degree) of the infected nodes.}
    \label{fig:c2n50}
\end{figure}

\begin{figure}[!h]
    \centering
    \includegraphics[scale=0.3]{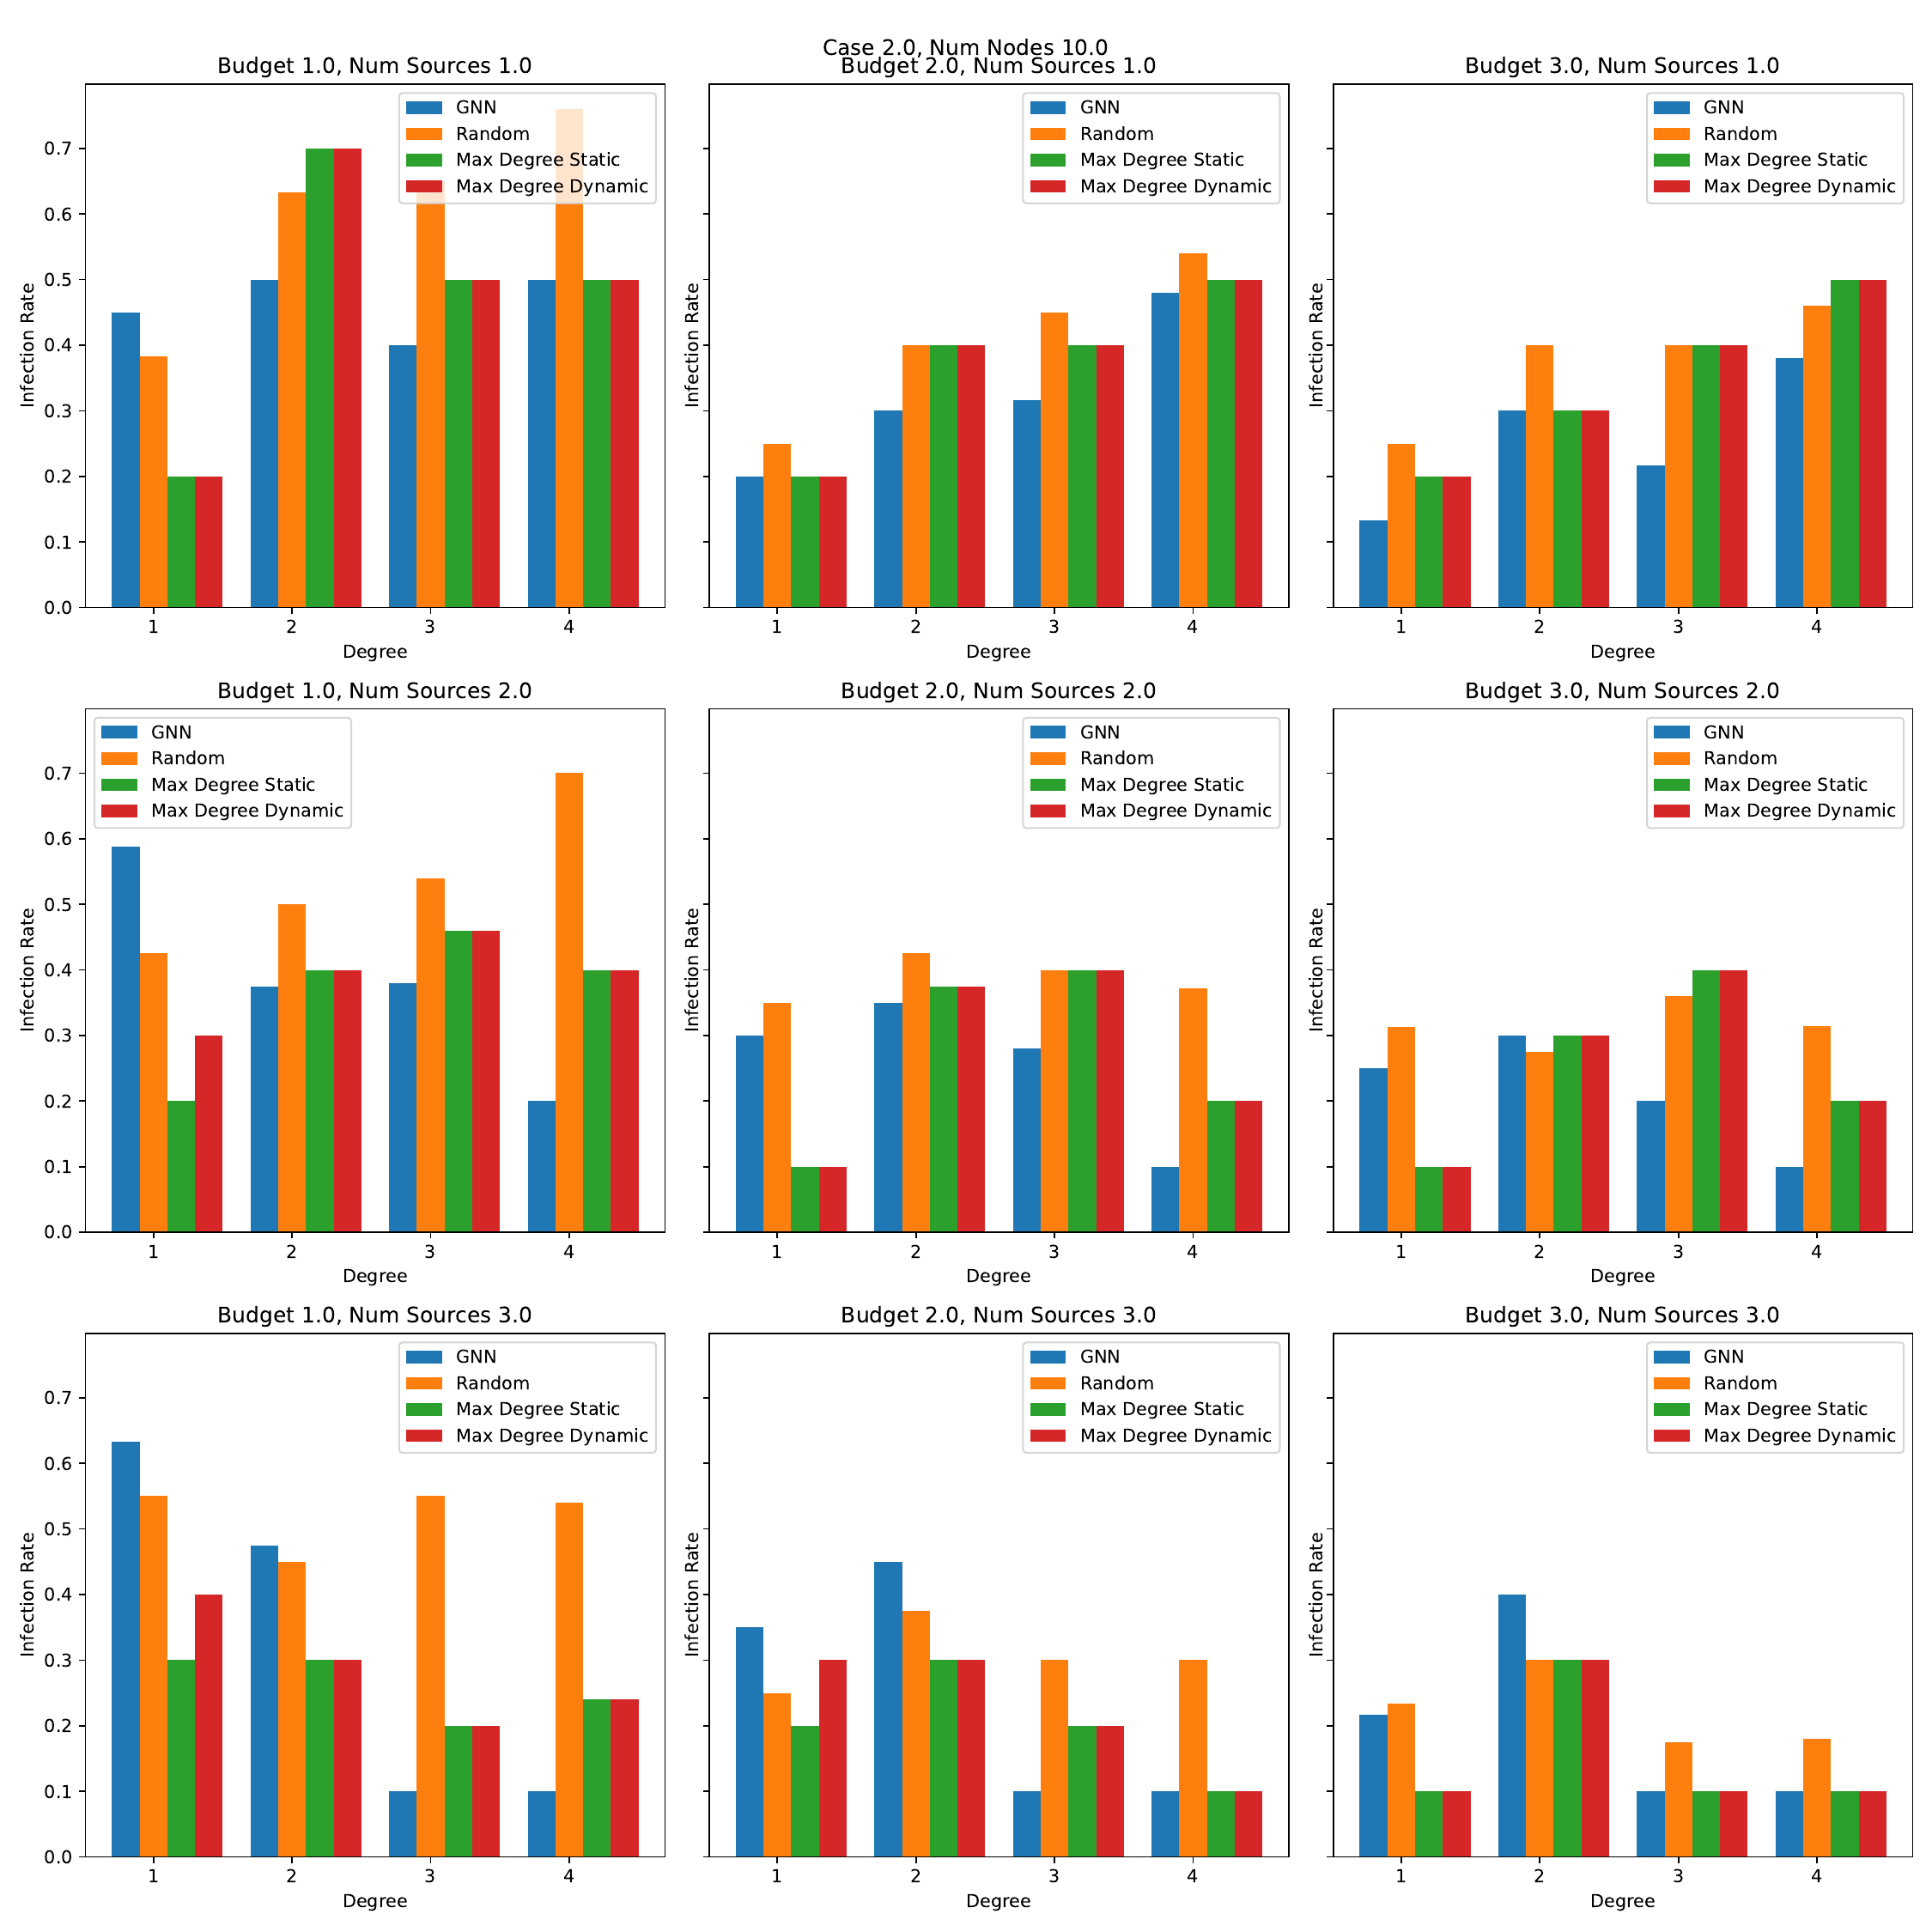}
    \caption{\footnotesize Dataset: Tree, Case-2 Node-10: Performance Evaluation of GCN-Based Supervised Learning Model: This series of bar plots presents a comparative analysis between our GCN-based SL model (blue), Randomized Policy model(yellow), Max Degree Policy model (Static) (green) and Max Degree Policy model (Dynamic) (red) on 10-node network environment. Progressing from left to right, the plots depict scenarios with increasing action budgets, ranging from 1 to 3 actions permitted. Vertically, the plots are ordered to show the effect of varying the initial count of infected nodes, starting with one and increasing to three. Each set of bars within the plots is categorized by the average connectivity (degree) of the infected nodes.}
    \label{fig:Treec2n10}
\end{figure}

\begin{figure}[!h]
    \centering
    \includegraphics[scale=0.3]{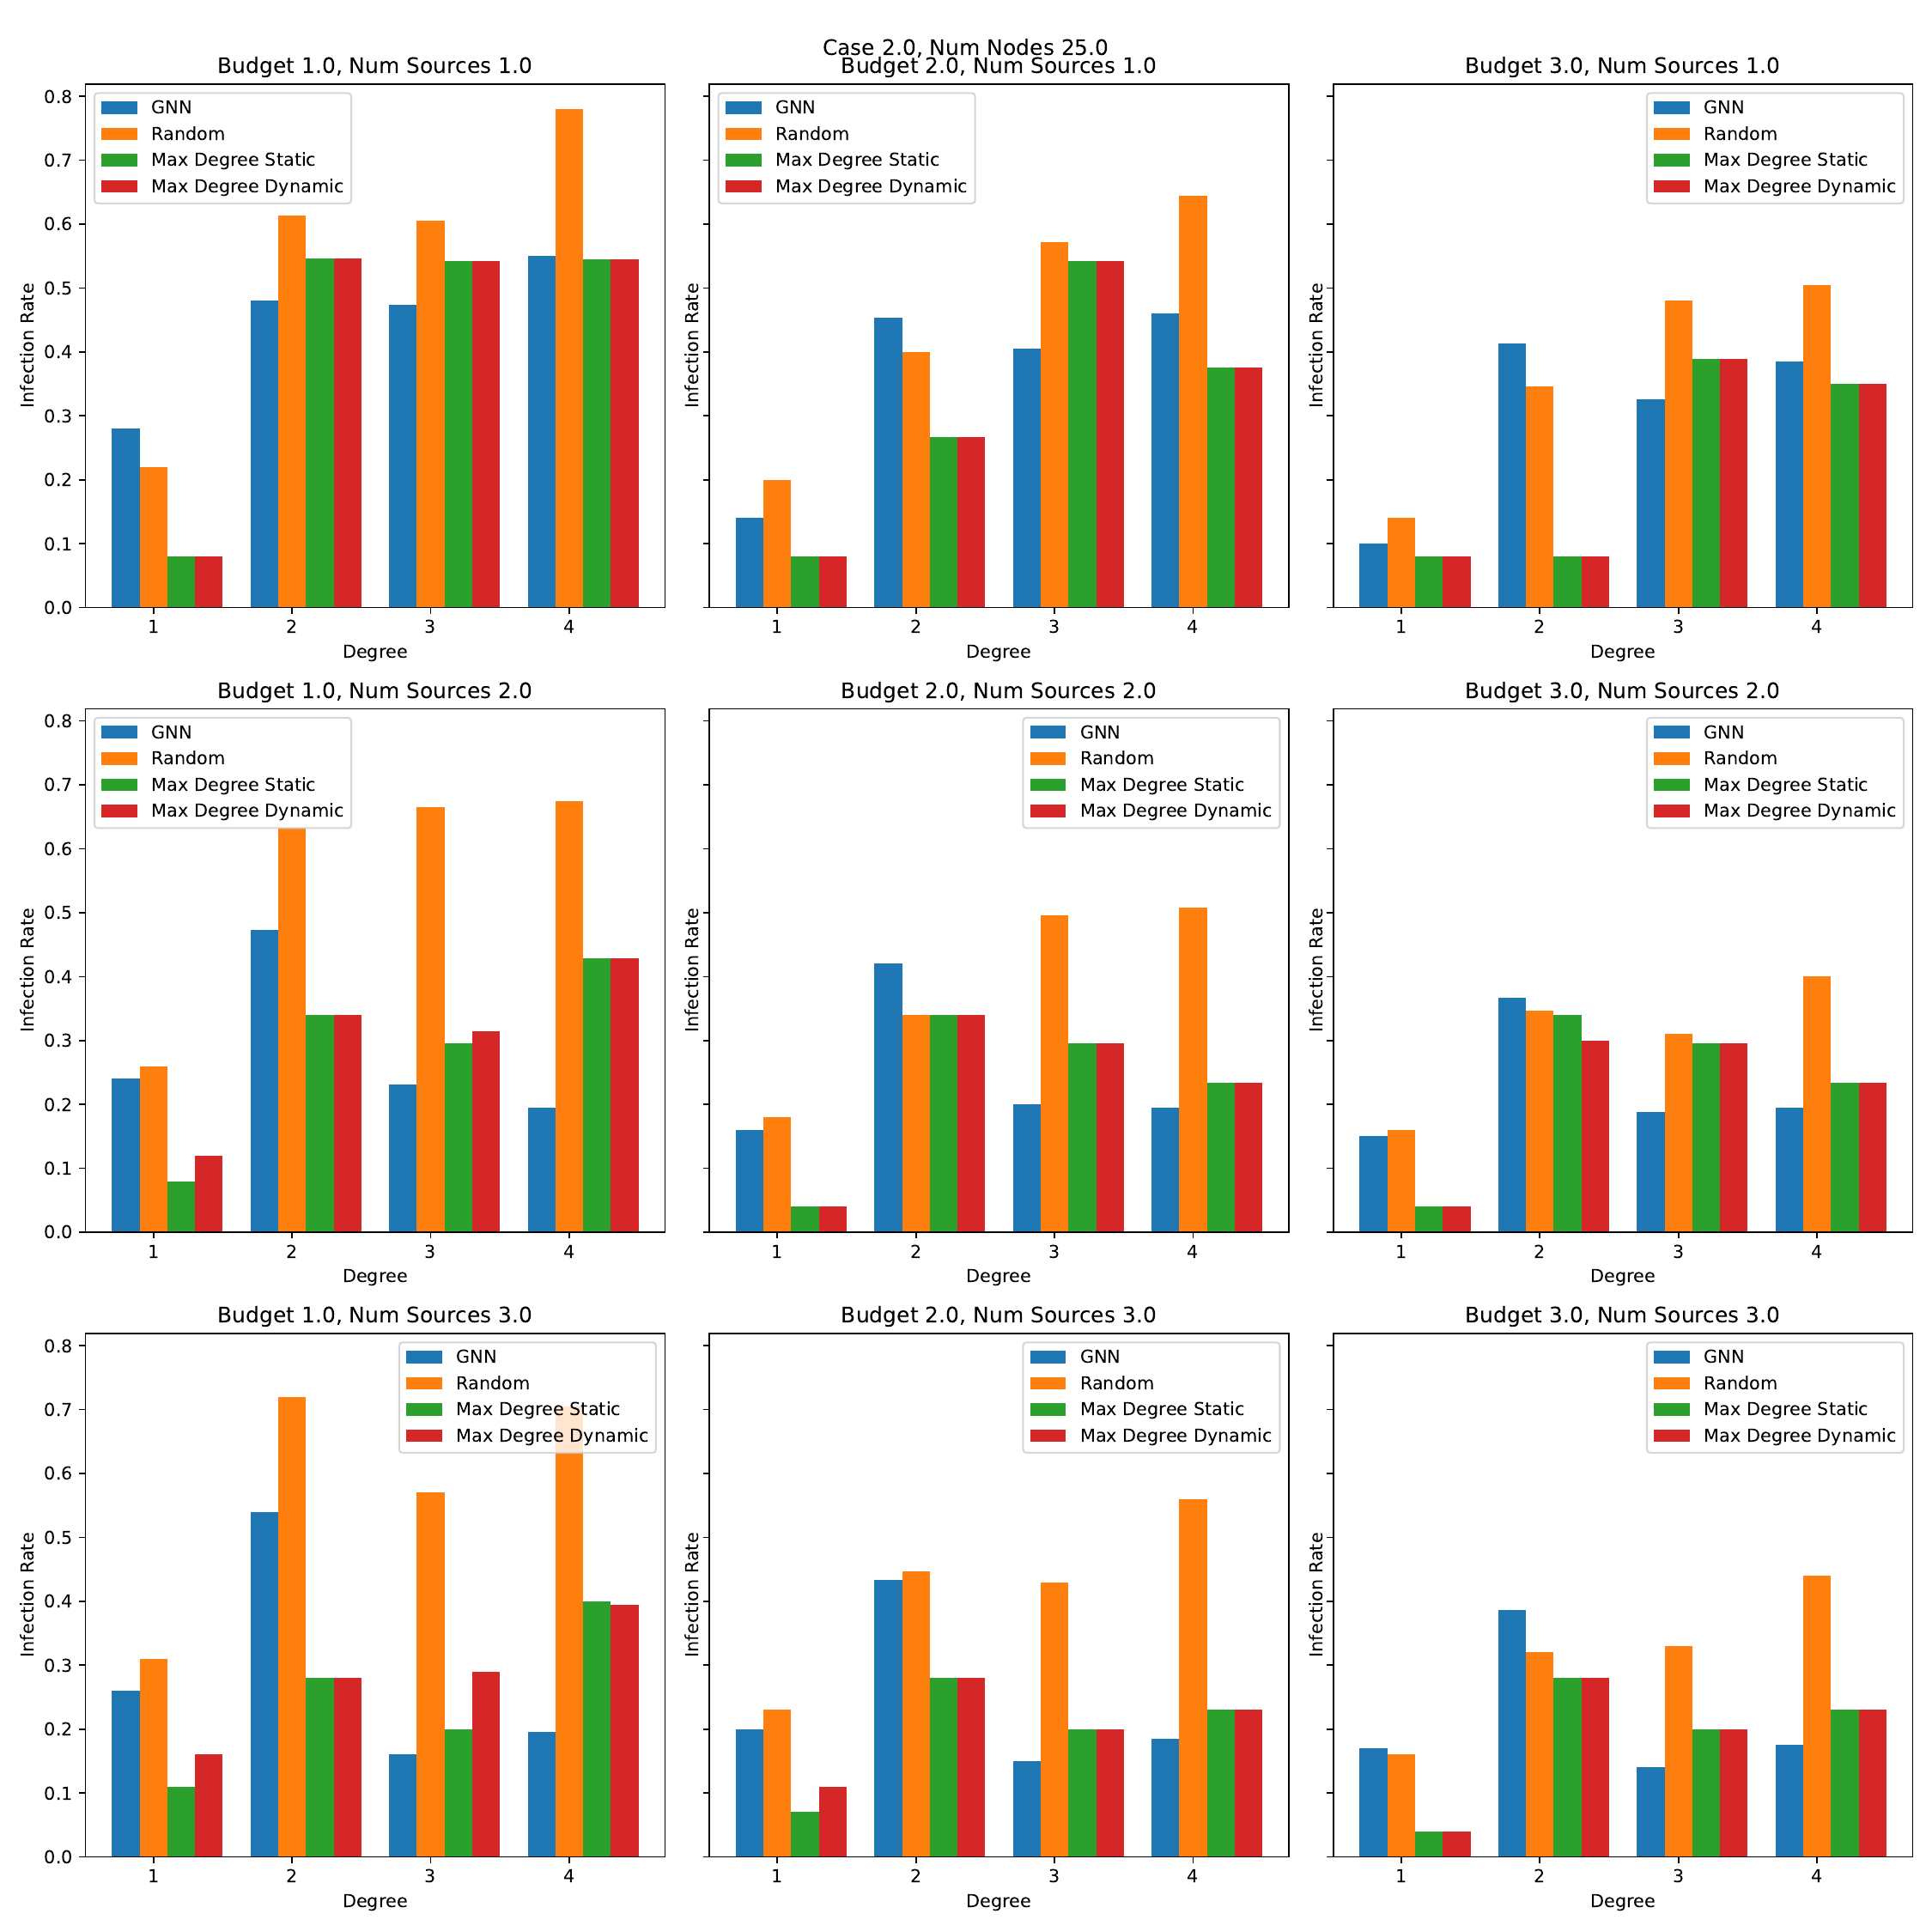}
    \caption{\footnotesize Dataset: Tree, Case-2 Node-25: Performance Evaluation of GCN-Based Supervised Learning Model: This series of bar plots presents a comparative analysis between our GCN-based SL model (blue), Randomized Policy model(yellow), Max Degree Policy model (Static) (green) and Max Degree Policy model (Dynamic) (red) on 25-node network environment. Progressing from left to right, the plots depict scenarios with increasing action budgets, ranging from 1 to 3 actions permitted. Vertically, the plots are ordered to show the effect of varying the initial count of infected nodes, starting with one and increasing to three. Each set of bars within the plots is categorized by the average connectivity (degree) of the infected nodes.}
    \label{fig:Treec2n25}
\end{figure}

\begin{figure}[!h]
    \centering
    \includegraphics[scale=0.3]{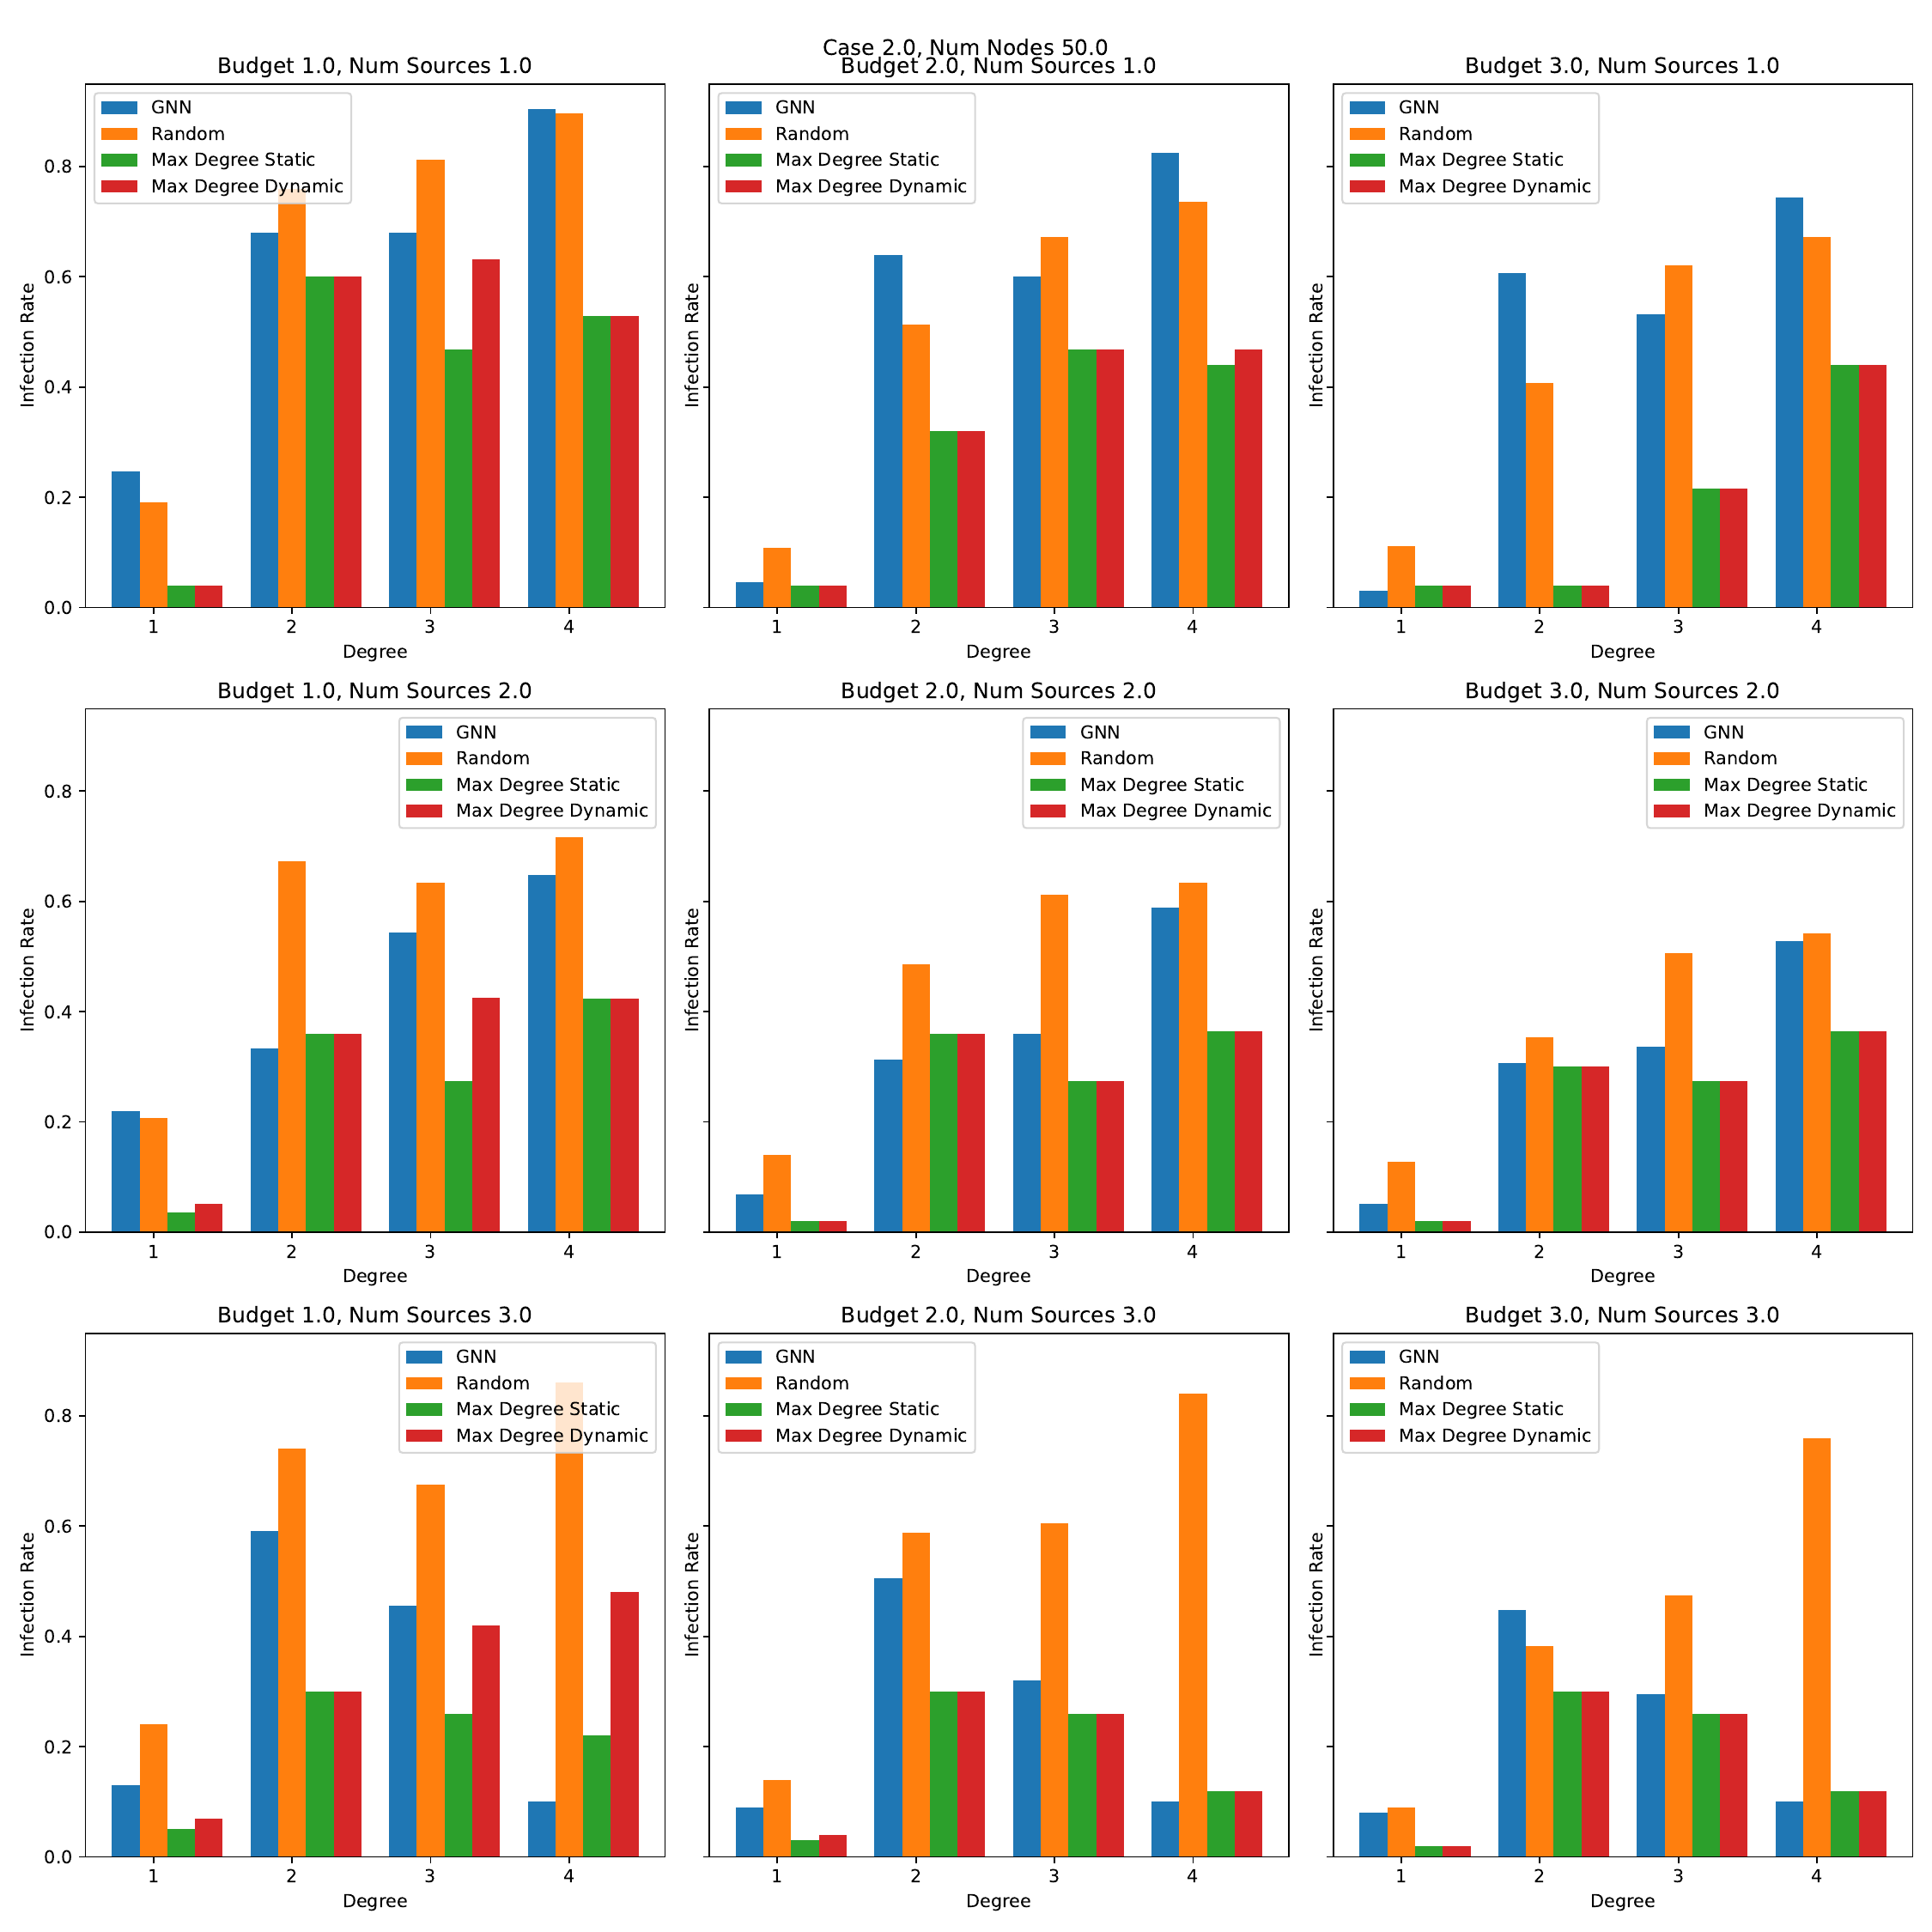}
    \caption{\footnotesize Dataset: Tree, Case-2 Node-50: Performance Evaluation of GCN-Based Supervised Learning Model: This series of bar plots presents a comparative analysis between our GCN-based SL model (blue), Randomized Policy model(yellow), Max Degree Policy model (Static) (green) and Max Degree Policy model (Dynamic) (red) on 25-node network environment. Progressing from left to right, the plots depict scenarios with increasing action budgets, ranging from 1 to 3 actions permitted. Vertically, the plots are ordered to show the effect of varying the initial count of infected nodes, starting with one and increasing to three. Each set of bars within the plots is categorized by the average connectivity (degree) of the infected nodes.}
    \label{fig:Treec2n50}
\end{figure}

\begin{figure}[!h]
    \centering
    \includegraphics[scale=0.3]{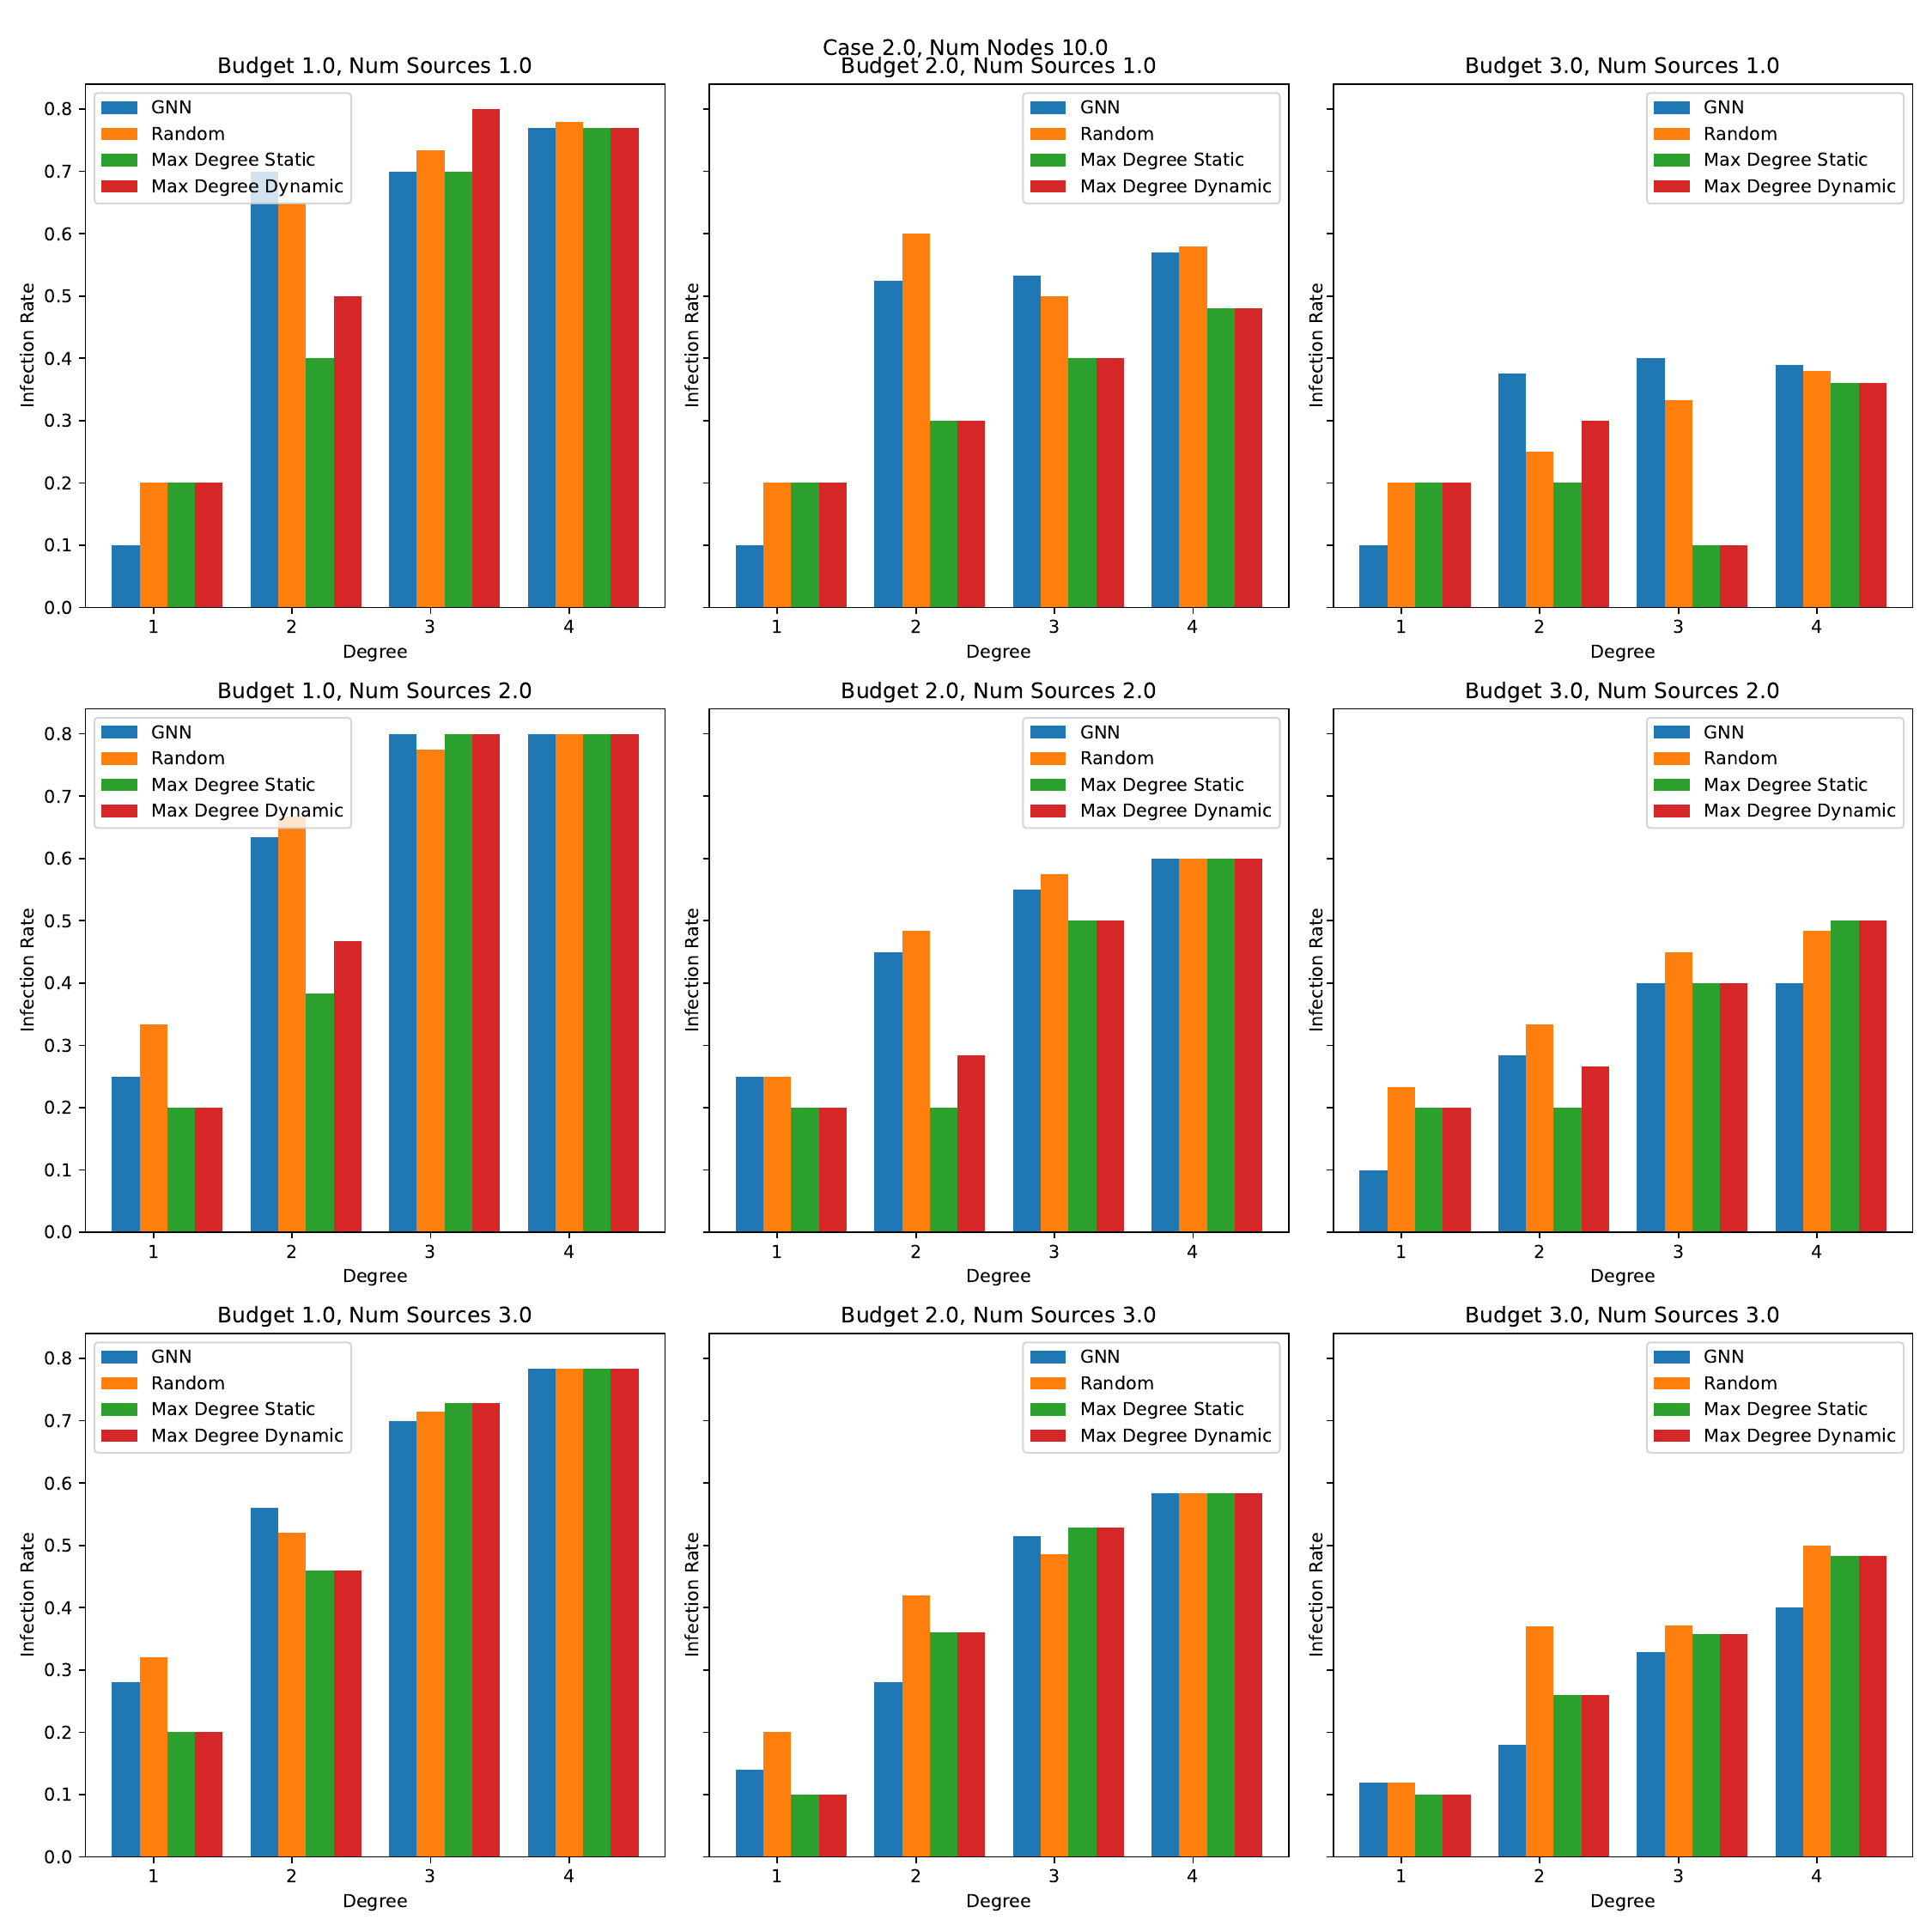}
    \caption{\footnotesize Dataset: Erdos-Renyi, Case-2 Node-10: Performance Evaluation of GCN-Based Supervised Learning Model: This series of bar plots presents a comparative analysis between our GCN-based SL model (blue), Randomized Policy model(yellow), Max Degree Policy model (Static) (green) and Max Degree Policy model (Dynamic) (red) on 10-node network environment. Progressing from left to right, the plots depict scenarios with increasing action budgets, ranging from 1 to 3 actions permitted. Vertically, the plots are ordered to show the effect of varying the initial count of infected nodes, starting with one and increasing to three. Each set of bars within the plots is categorized by the average connectivity (degree) of the infected nodes.}
    \label{fig:ERc2n10}
\end{figure}

\begin{figure}[!h]
    \centering
    \includegraphics[scale=0.3]{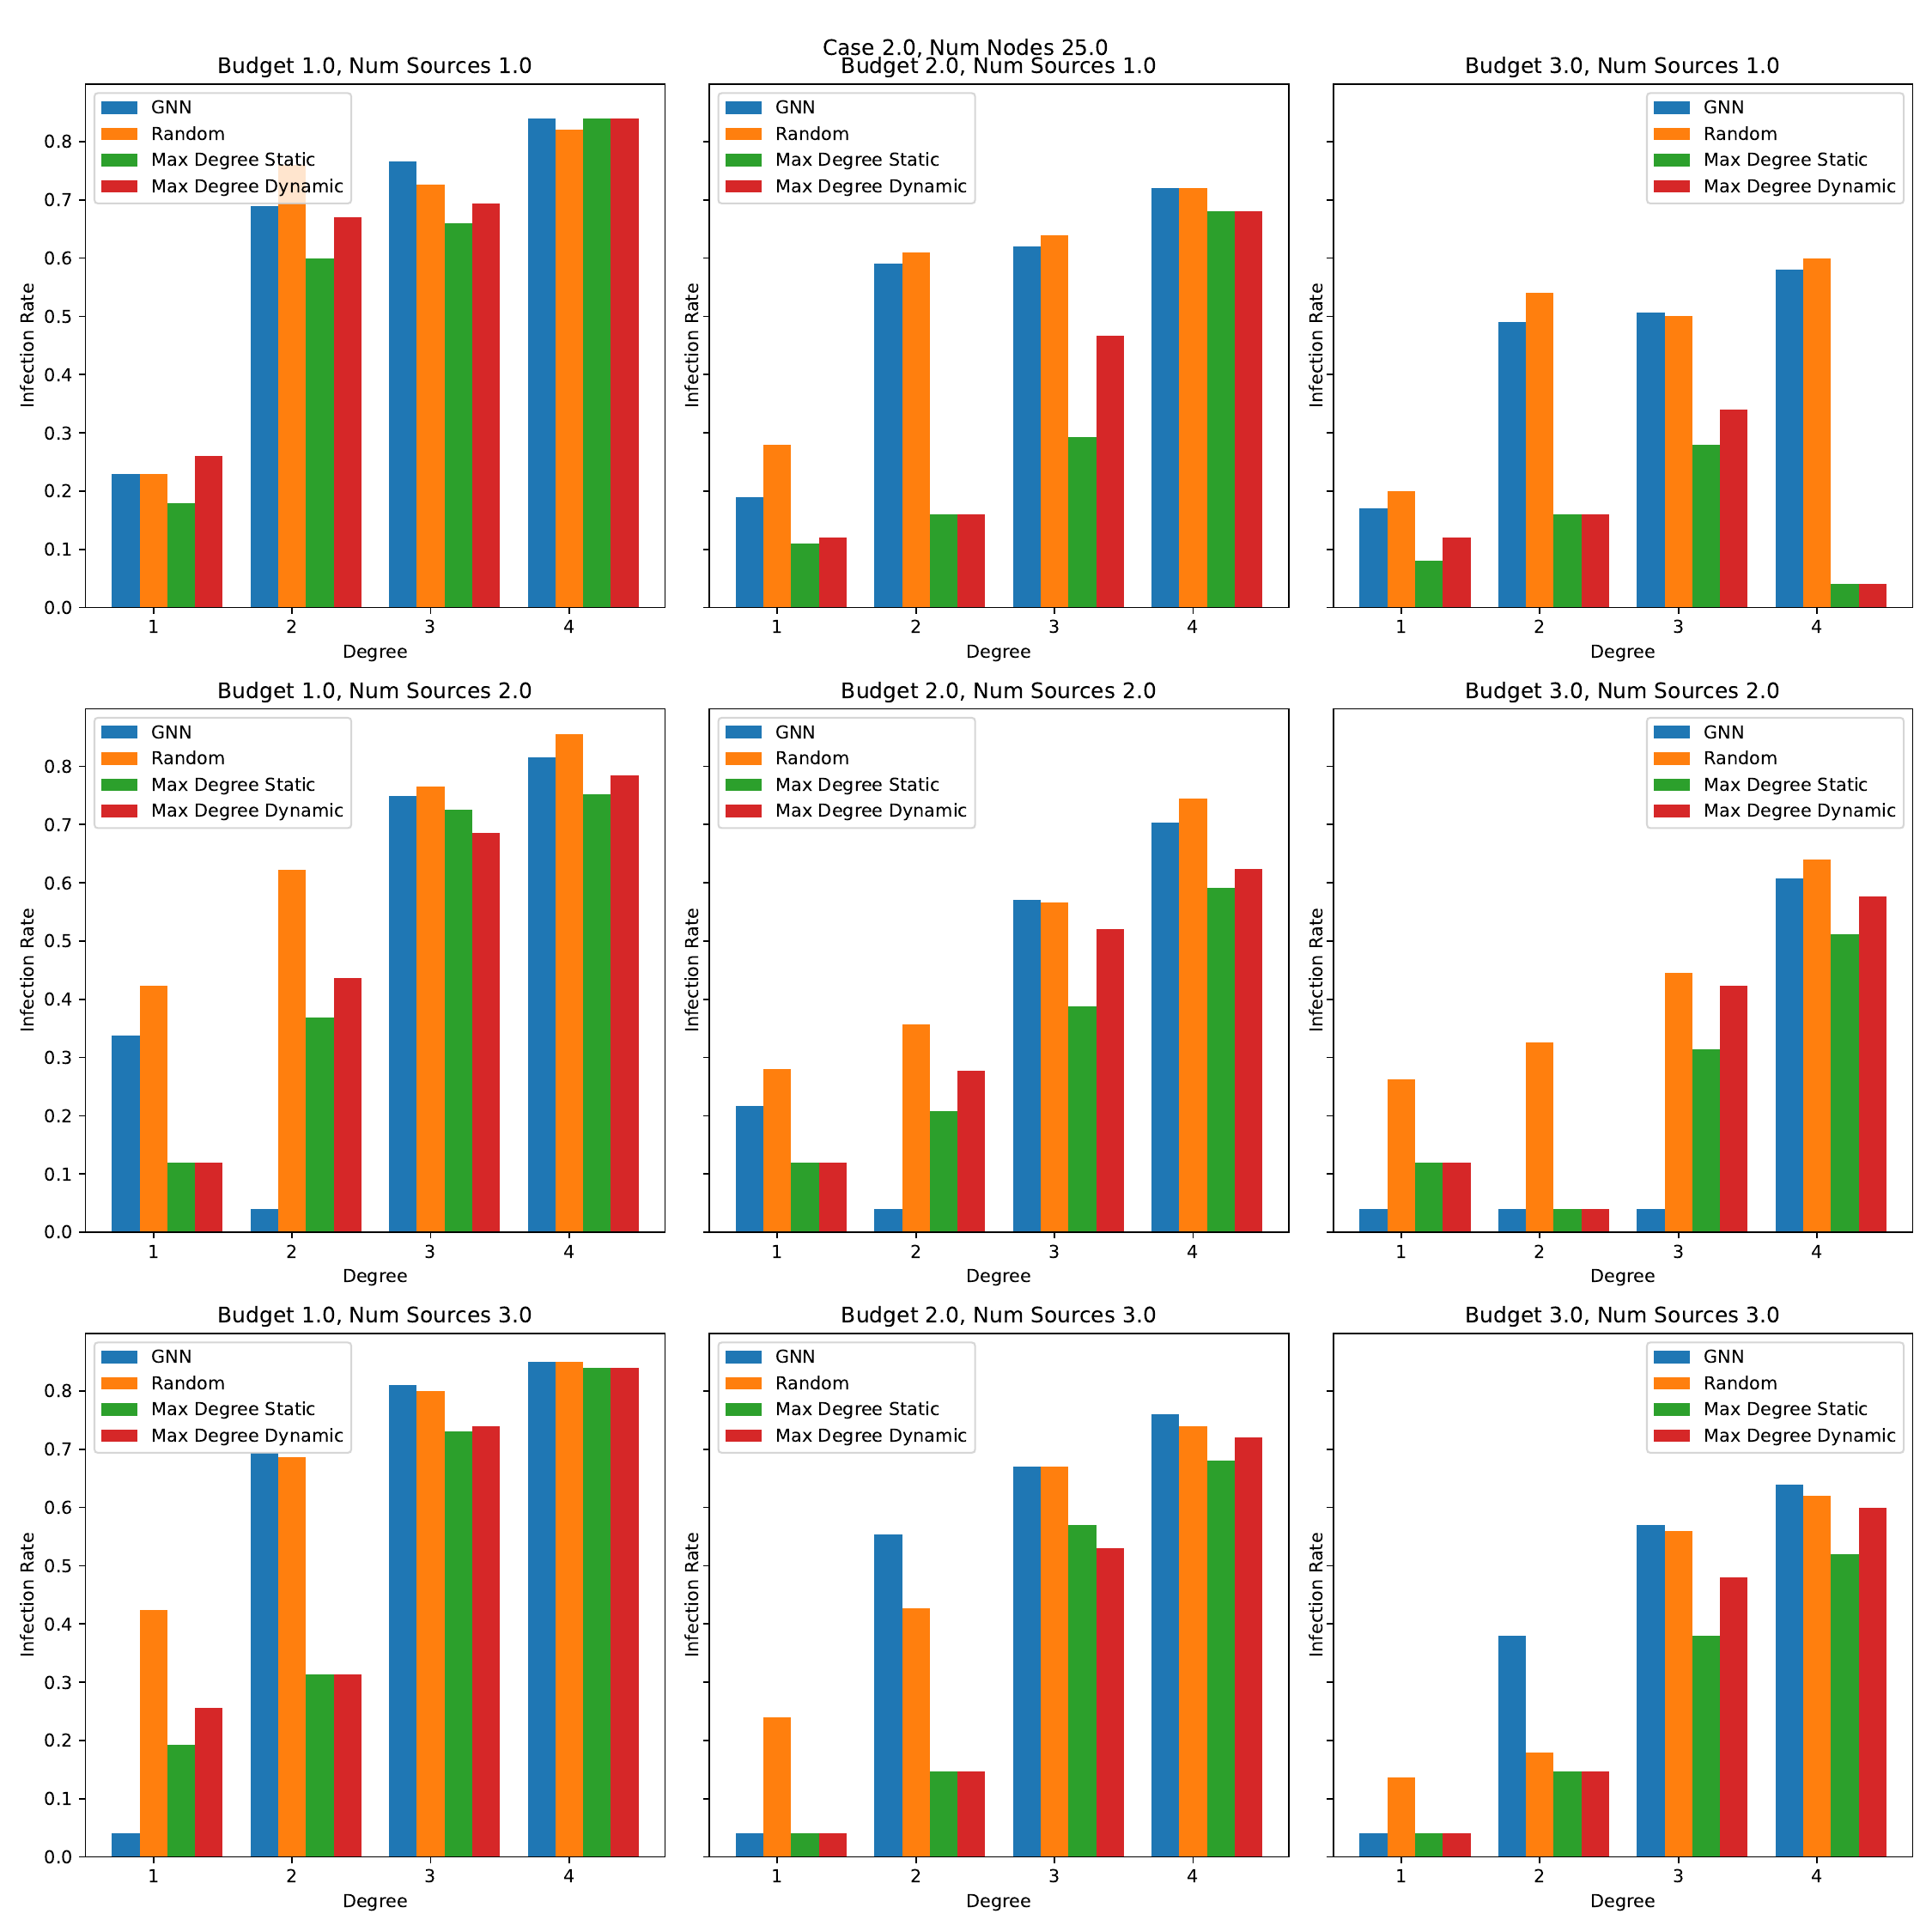}
    \caption{\footnotesize Dataset: Erdos-Renyi, Case-2 Node-25: Performance Evaluation of GCN-Based Supervised Learning Model: This series of bar plots presents a comparative analysis between our GCN-based SL model (blue), Randomized Policy model(yellow), Max Degree Policy model (Static) (green) and Max Degree Policy model (Dynamic) (red) on 10-node network environment. Progressing from left to right, the plots depict scenarios with increasing action budgets, ranging from 1 to 3 actions permitted. Vertically, the plots are ordered to show the effect of varying the initial count of infected nodes, starting with one and increasing to three. Each set of bars within the plots is categorized by the average connectivity (degree) of the infected nodes.}
    \label{fig:ERc2n25}
\end{figure}

\begin{figure}[!h]
    \centering
    \includegraphics[scale=0.3]{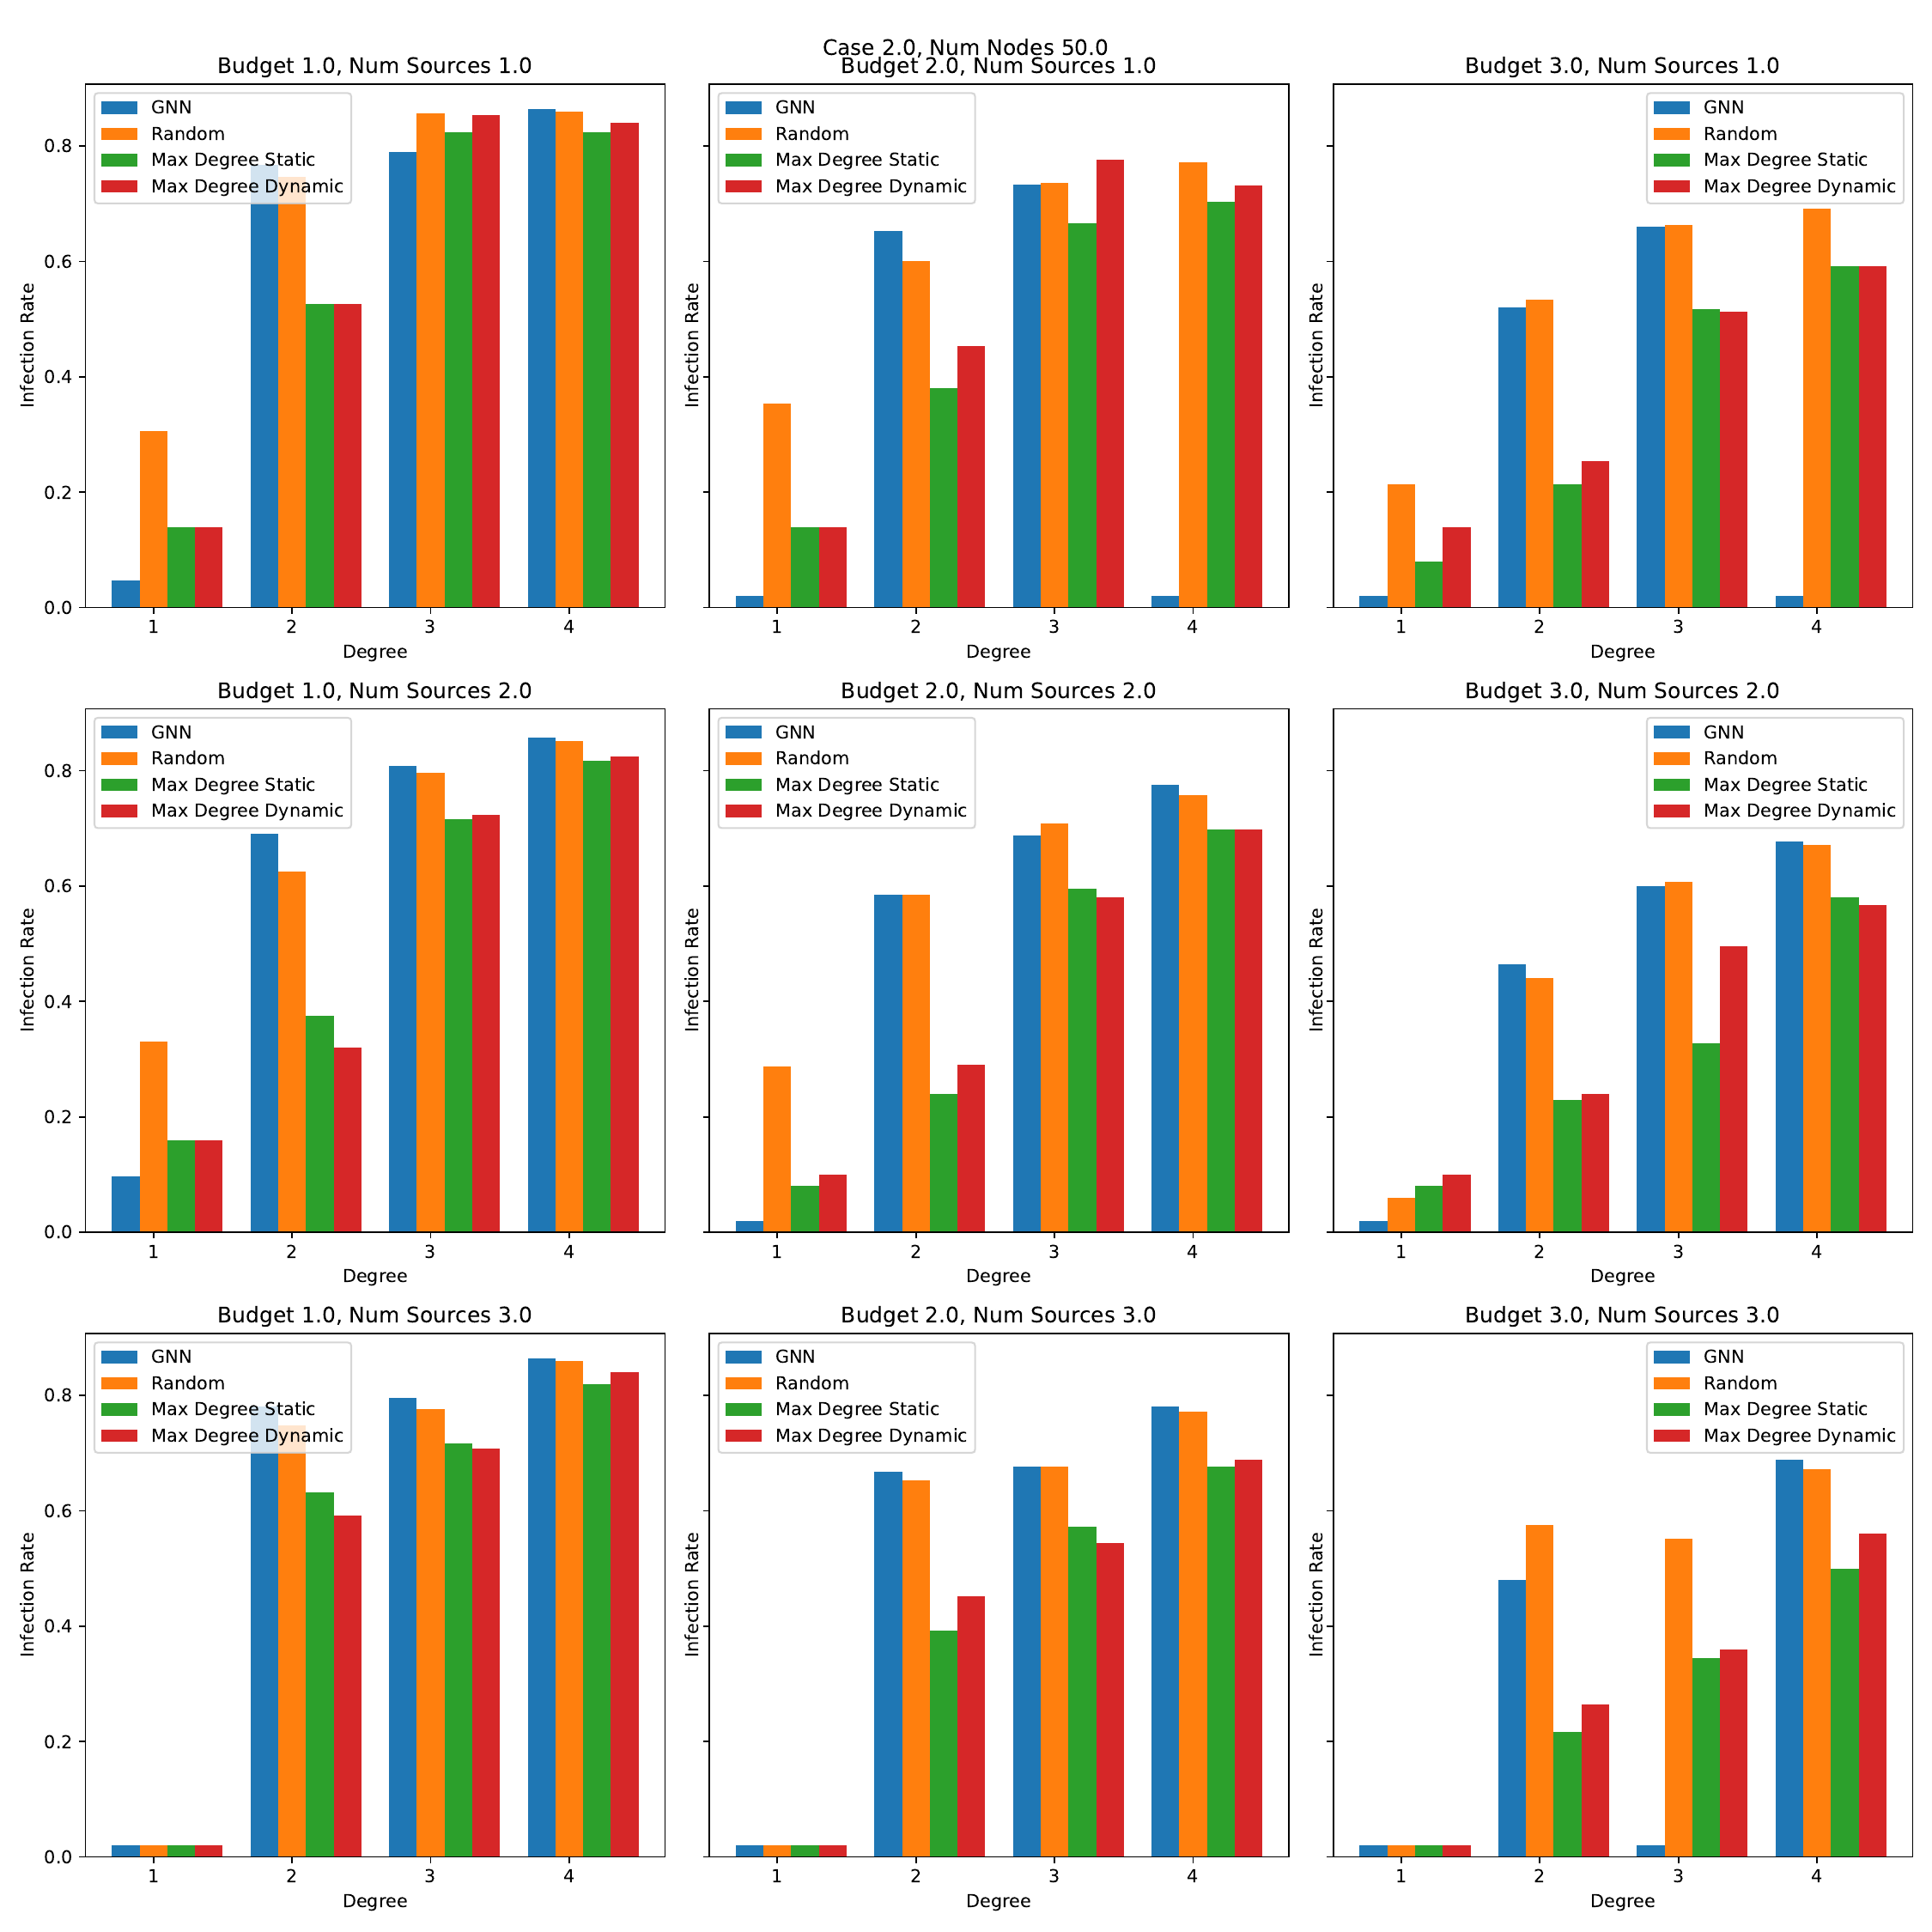}
    \caption{\footnotesize Dataset: Erdos-Renyi, Case-2 Node-50: Performance Evaluation of GCN-Based Supervised Learning Model: This series of bar plots presents a comparative analysis between our GCN-based SL model (blue), Randomized Policy model(yellow), Max Degree Policy model (Static) (green) and Max Degree Policy model (Dynamic) (red) on 10-node network environment. Progressing from left to right, the plots depict scenarios with increasing action budgets, ranging from 1 to 3 actions permitted. Vertically, the plots are ordered to show the effect of varying the initial count of infected nodes, starting with one and increasing to three. Each set of bars within the plots is categorized by the average connectivity (degree) of the infected nodes.}
    \label{fig:ERc2n50}
\end{figure}

% ######## Case 3 #########

\begin{figure}[!h]
    \centering
    \includegraphics[scale=0.3]{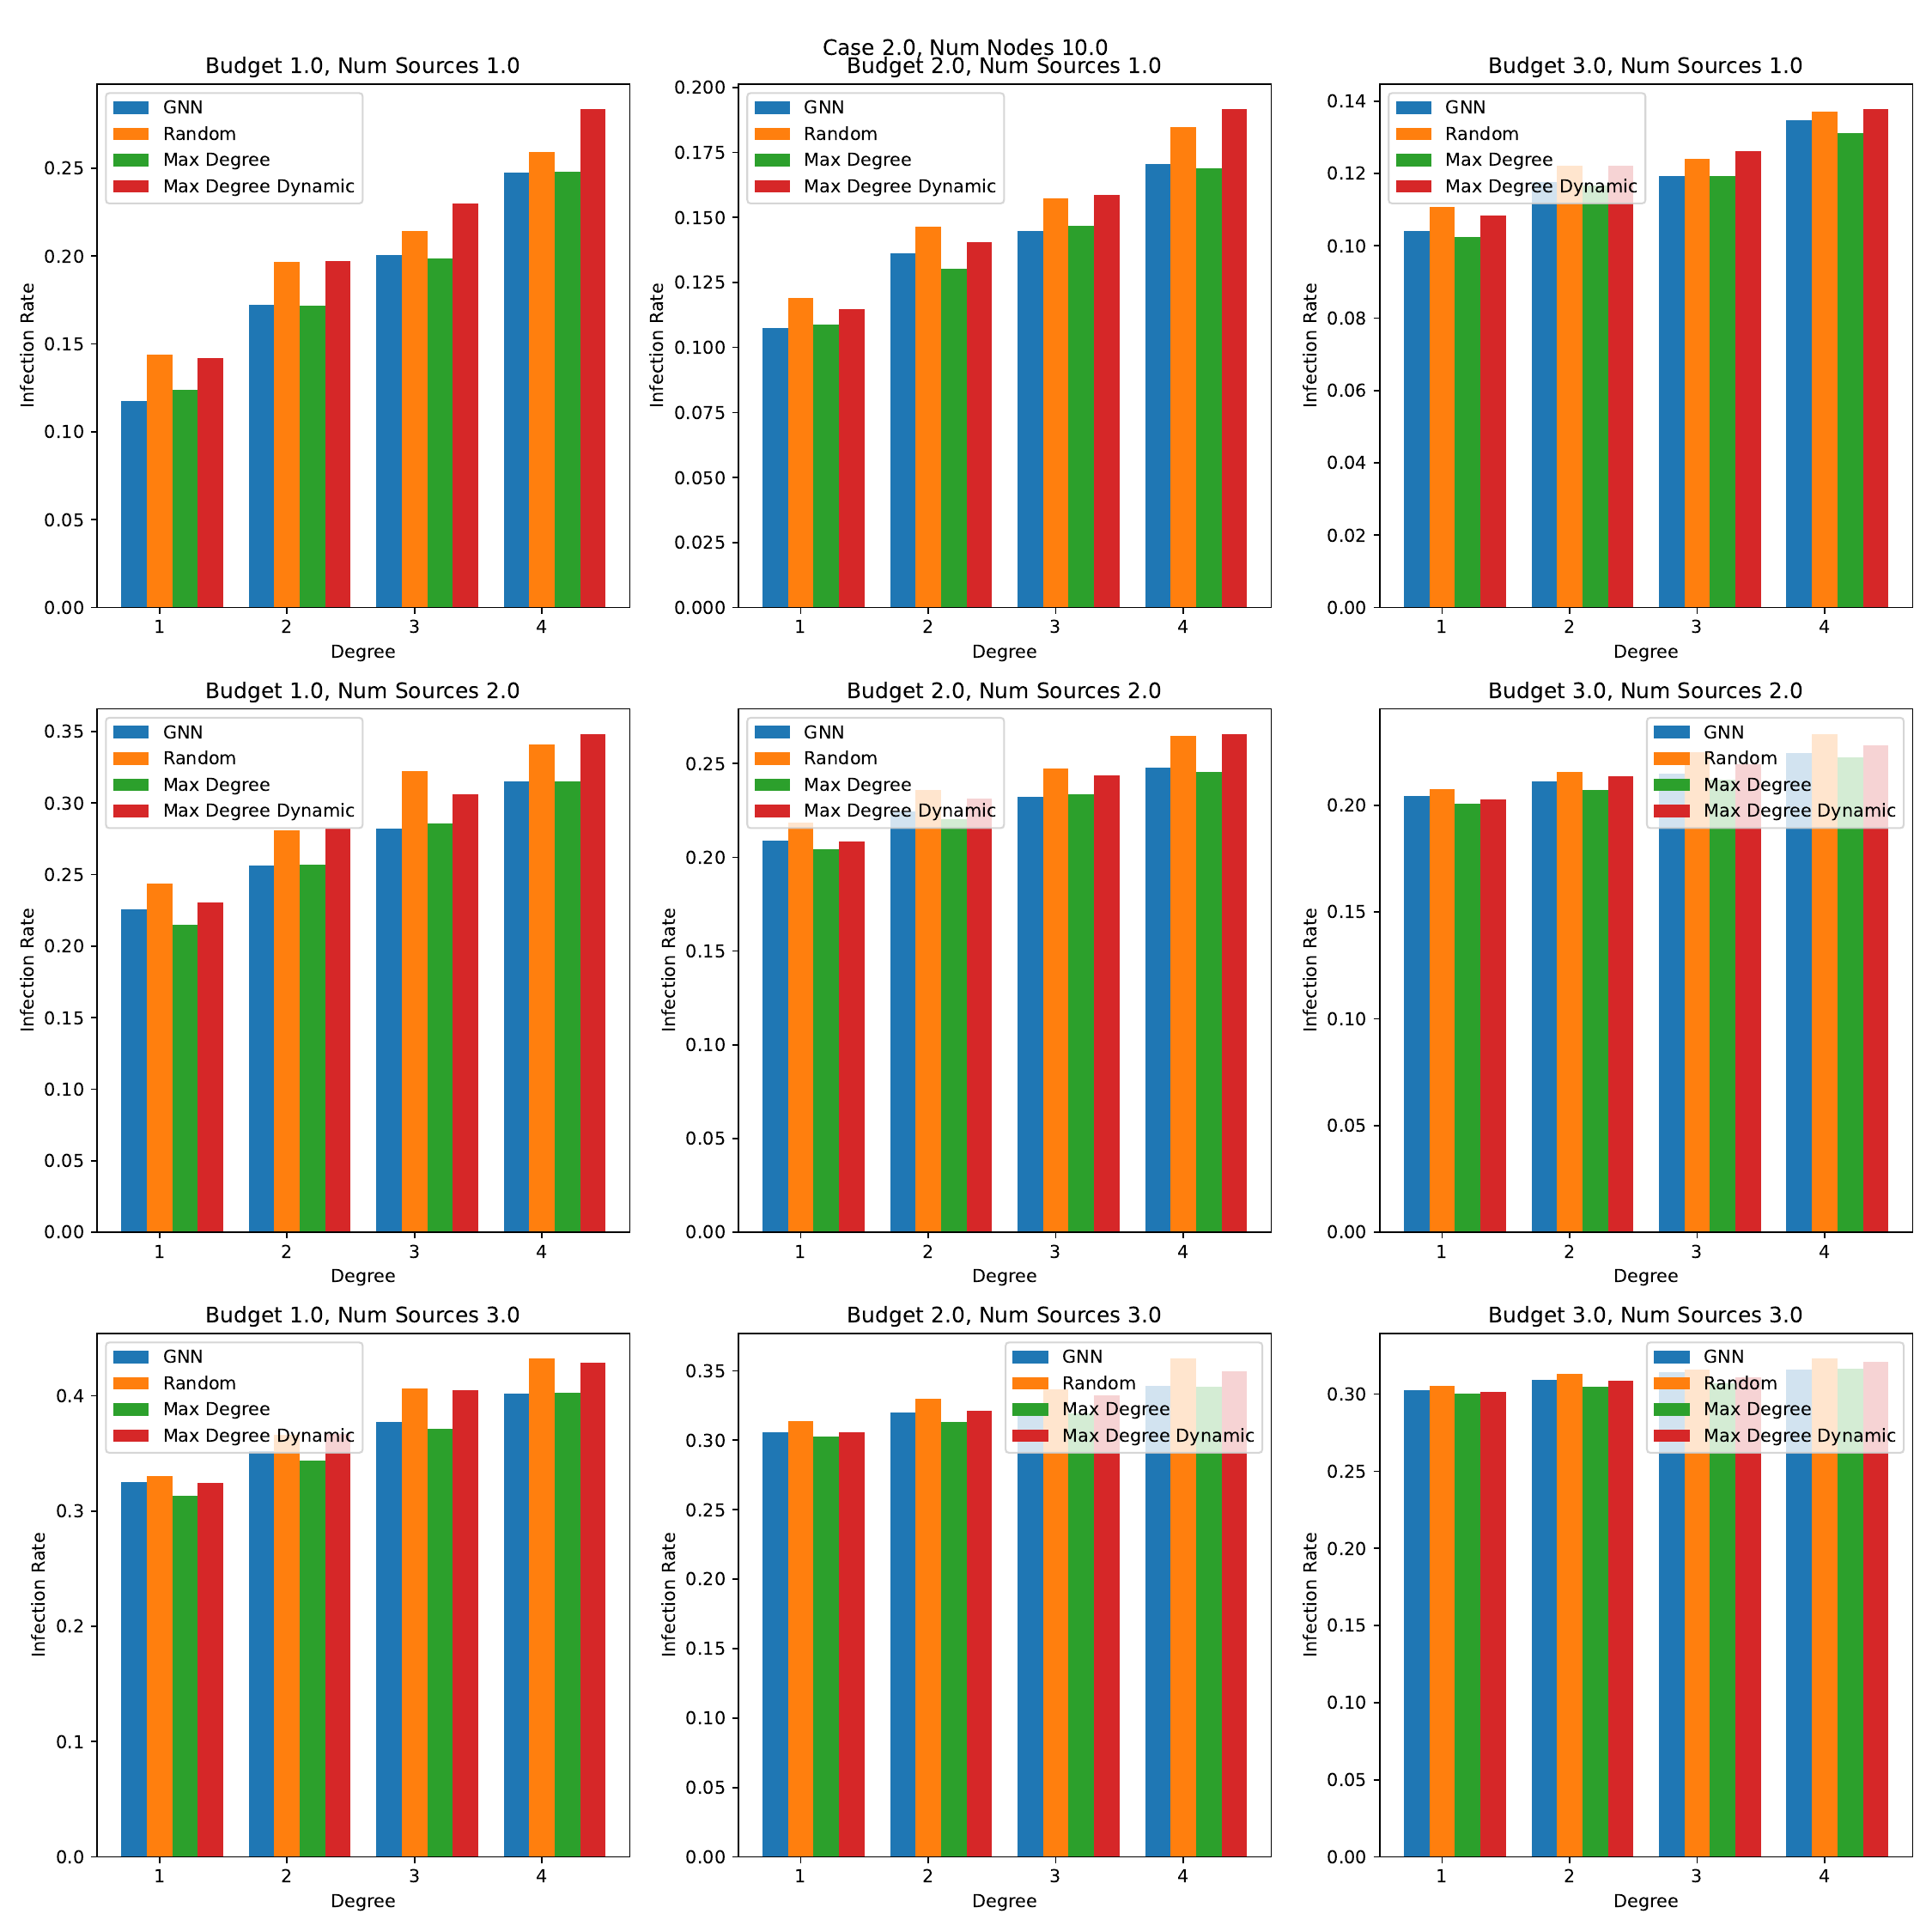}
    \caption{\footnotesize Dataset: Watts\_Strogatz, Case-3 Node-10: Performance Evaluation of GCN-Based Supervised Learning Model: This series of bar plots presents a comparative analysis between our GCN-based SL model (blue), Randomized Policy model(yellow), Max Degree Policy model (Static) (green) and Max Degree Policy model (Dynamic) (red) on 10-node network environment. Progressing from left to right, the plots depict scenarios with increasing action budgets, ranging from 1 to 3 actions permitted. Vertically, the plots are ordered to show the effect of varying the initial count of infected nodes, starting with one and increasing to three. Each set of bars within the plots is categorized by the average connectivity (degree) of the infected nodes.}
    \label{fig:c3n10}
\end{figure}

\begin{figure}[!h]
    \centering
    \includegraphics[scale=0.3]{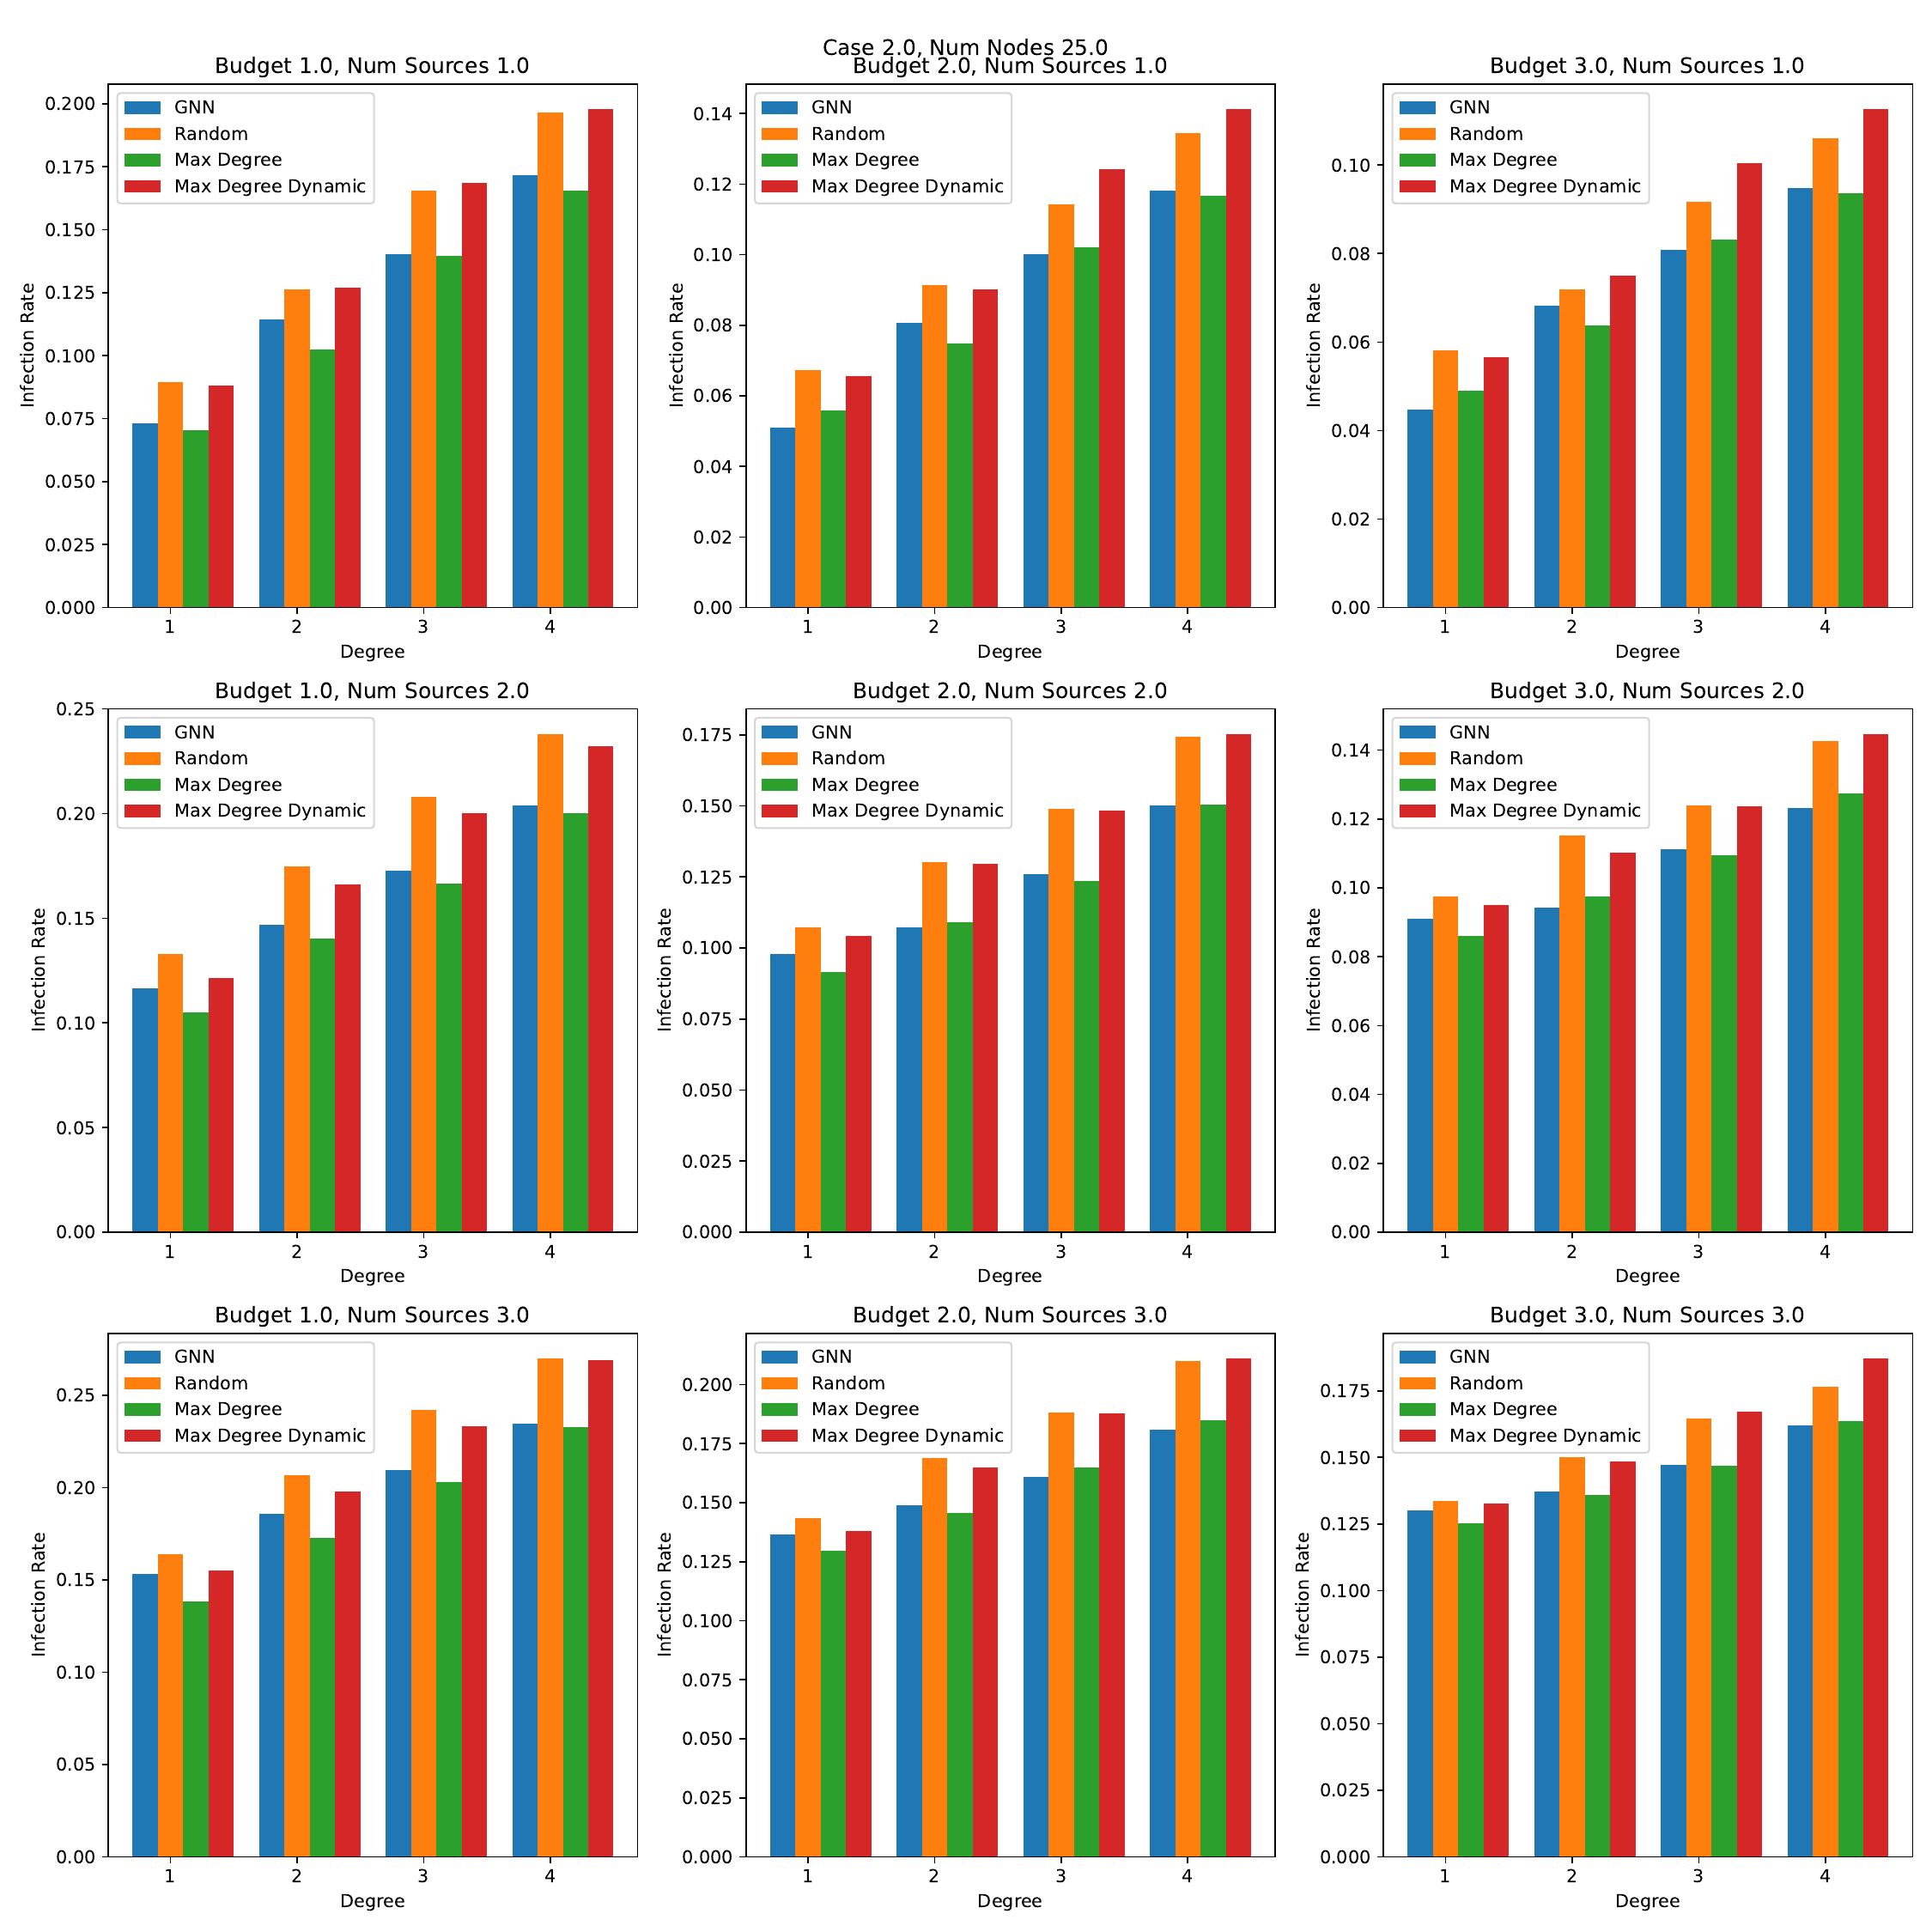}
    \caption{\footnotesize Dataset: Watts\_Strogatz, Case-3 Node-25: Performance Evaluation of GCN-Based Supervised Learning Model: This series of bar plots presents a comparative analysis between our GCN-based SL model (blue), Randomized Policy model(yellow), Max Degree Policy model (Static) (green) and Max Degree Policy model (Dynamic) (red) on 25-node network environment. Progressing from left to right, the plots depict scenarios with increasing action budgets, ranging from 1 to 3 actions permitted. Vertically, the plots are ordered to show the effect of varying the initial count of infected nodes, starting with one and increasing to three. Each set of bars within the plots is categorized by the average connectivity (degree) of the infected nodes.}
    \label{fig:c3n25}
\end{figure}

\begin{figure}[!h]
    \centering
    \includegraphics[scale=0.3]{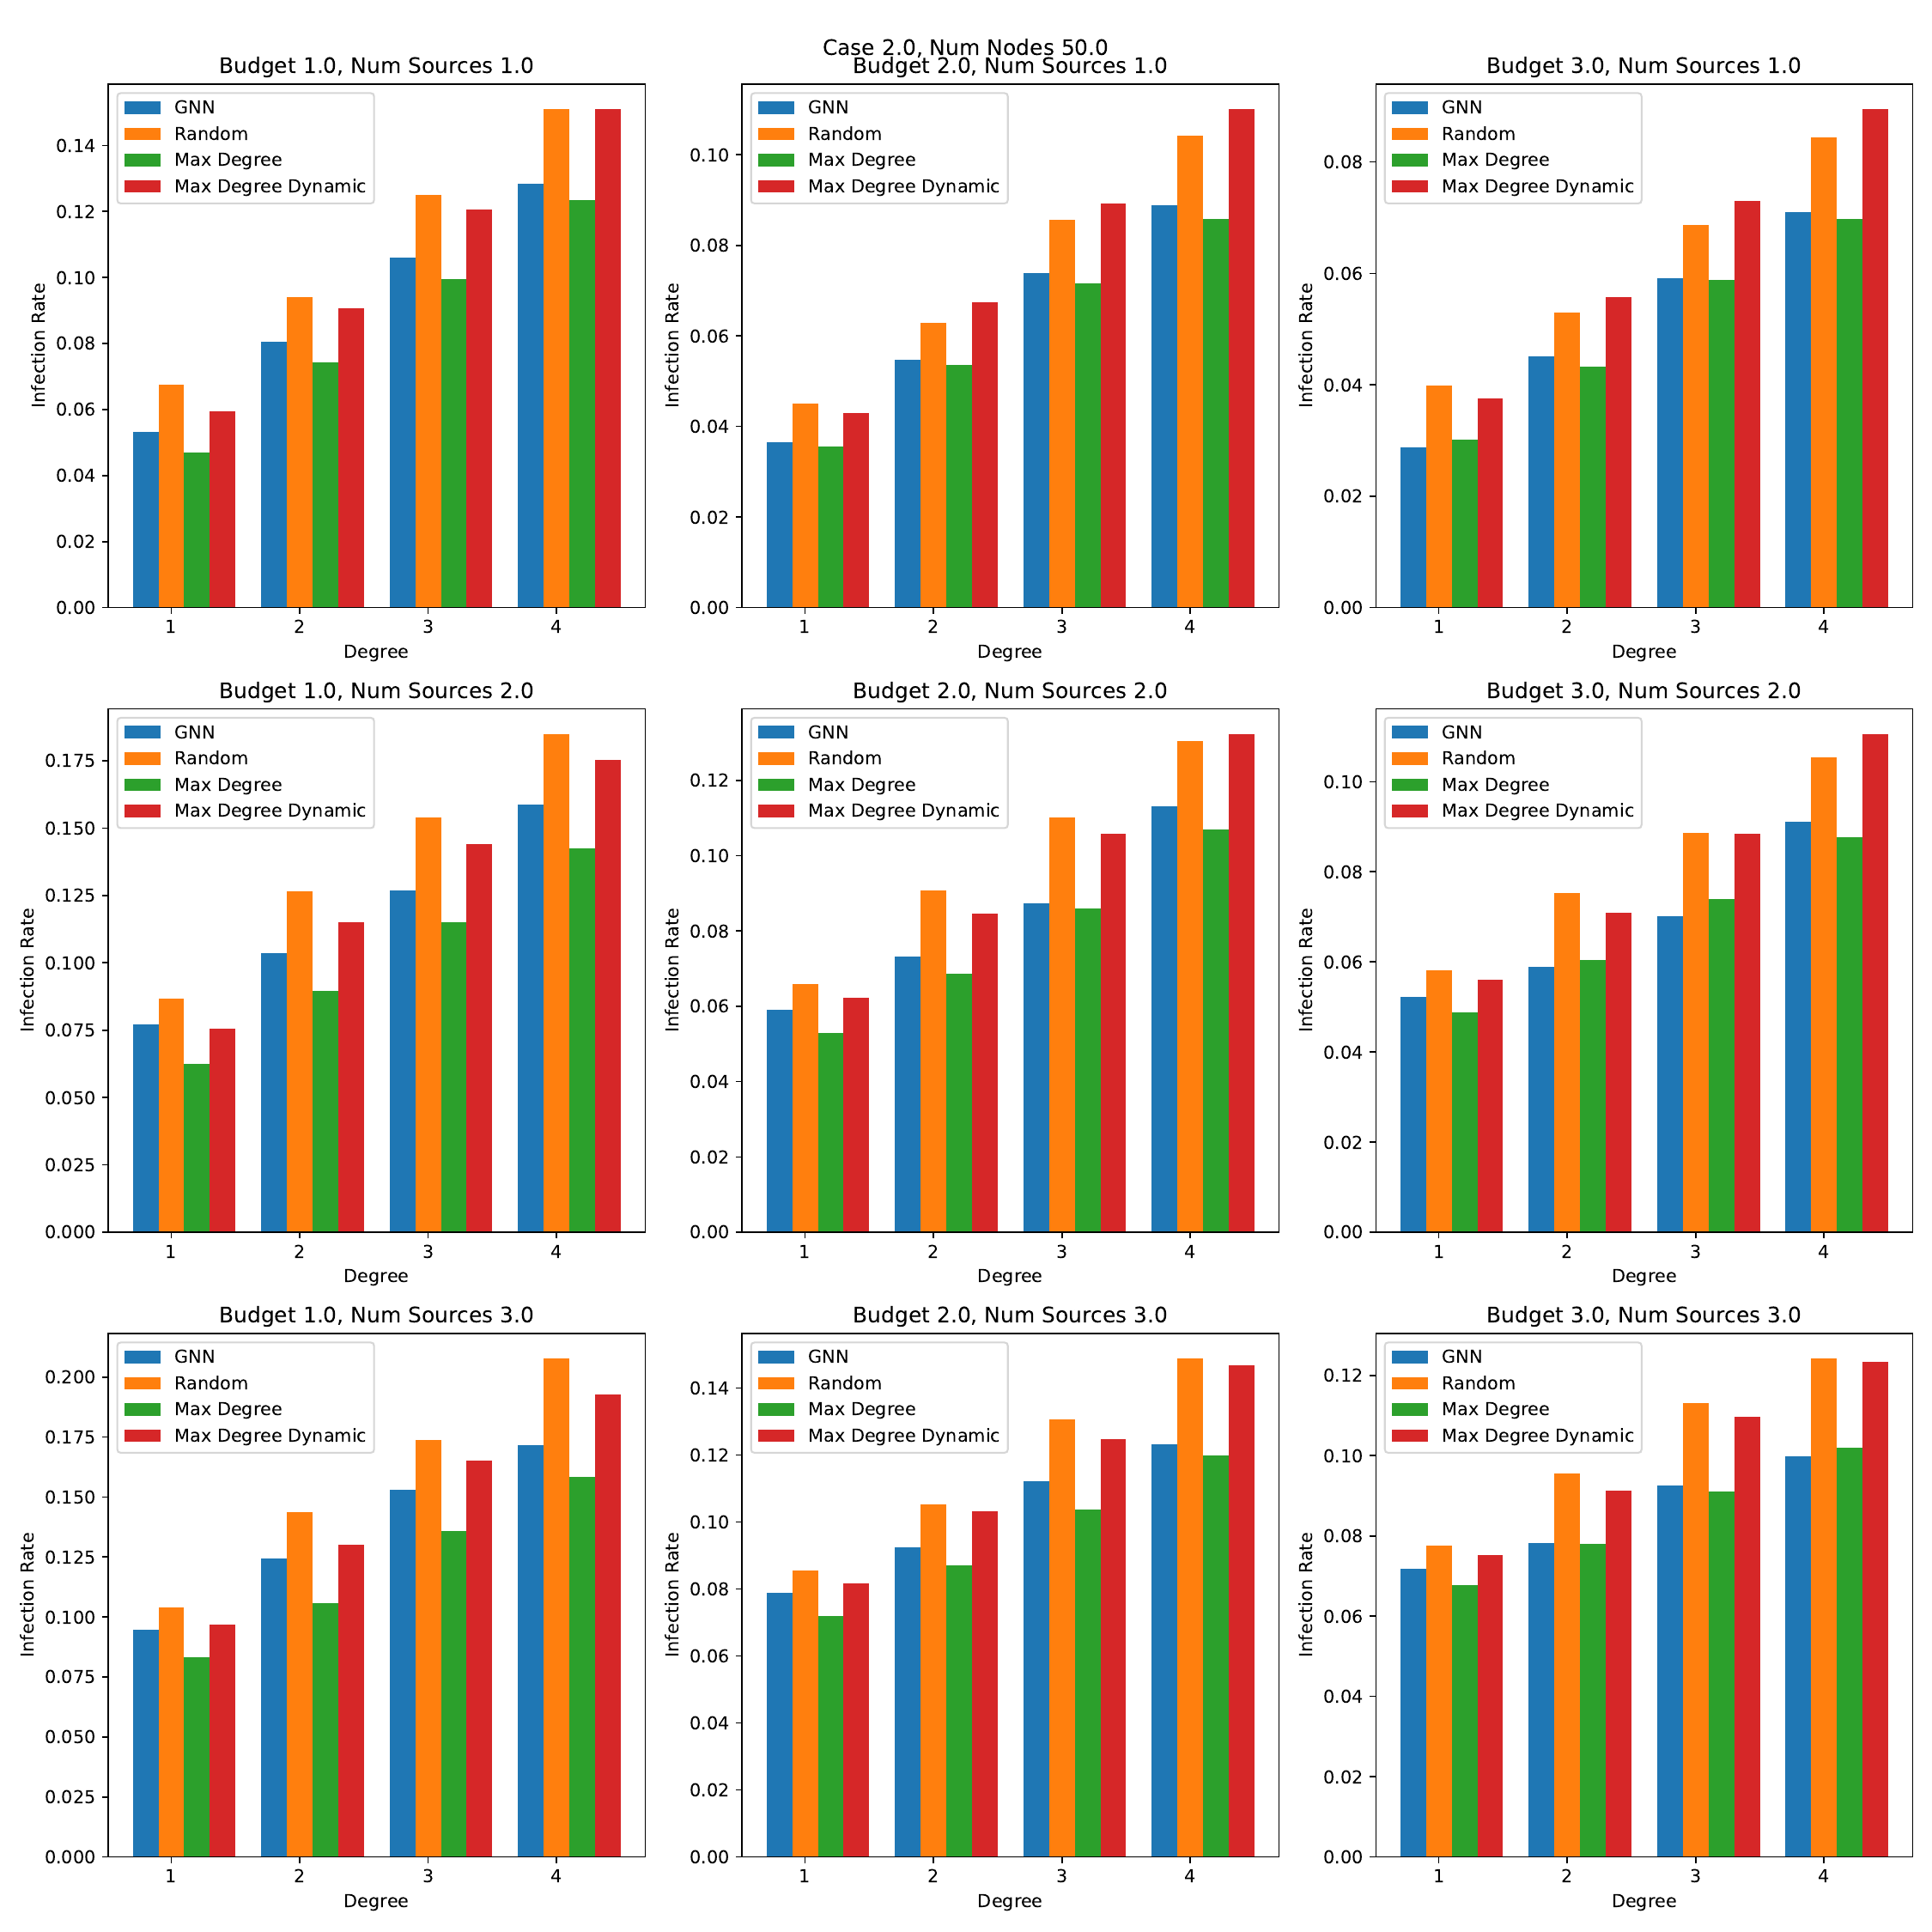}
    \caption{\footnotesize Dataset: Watts\_Strogatz, Case-3 Node-50: Performance Evaluation of GCN-Based Supervised Learning Model: This series of bar plots presents a comparative analysis between our GCN-based SL model (blue), Randomized Policy model(yellow), Max Degree Policy model (Static) (green) and Max Degree Policy model (Dynamic) (red) on 25-node network environment. Progressing from left to right, the plots depict scenarios with increasing action budgets, ranging from 1 to 3 actions permitted. Vertically, the plots are ordered to show the effect of varying the initial count of infected nodes, starting with one and increasing to three. Each set of bars within the plots is categorized by the average connectivity (degree) of the infected nodes.}
    \label{fig:c3n50}
\end{figure}

\begin{figure}[!h]
    \centering
    \includegraphics[scale=0.3]{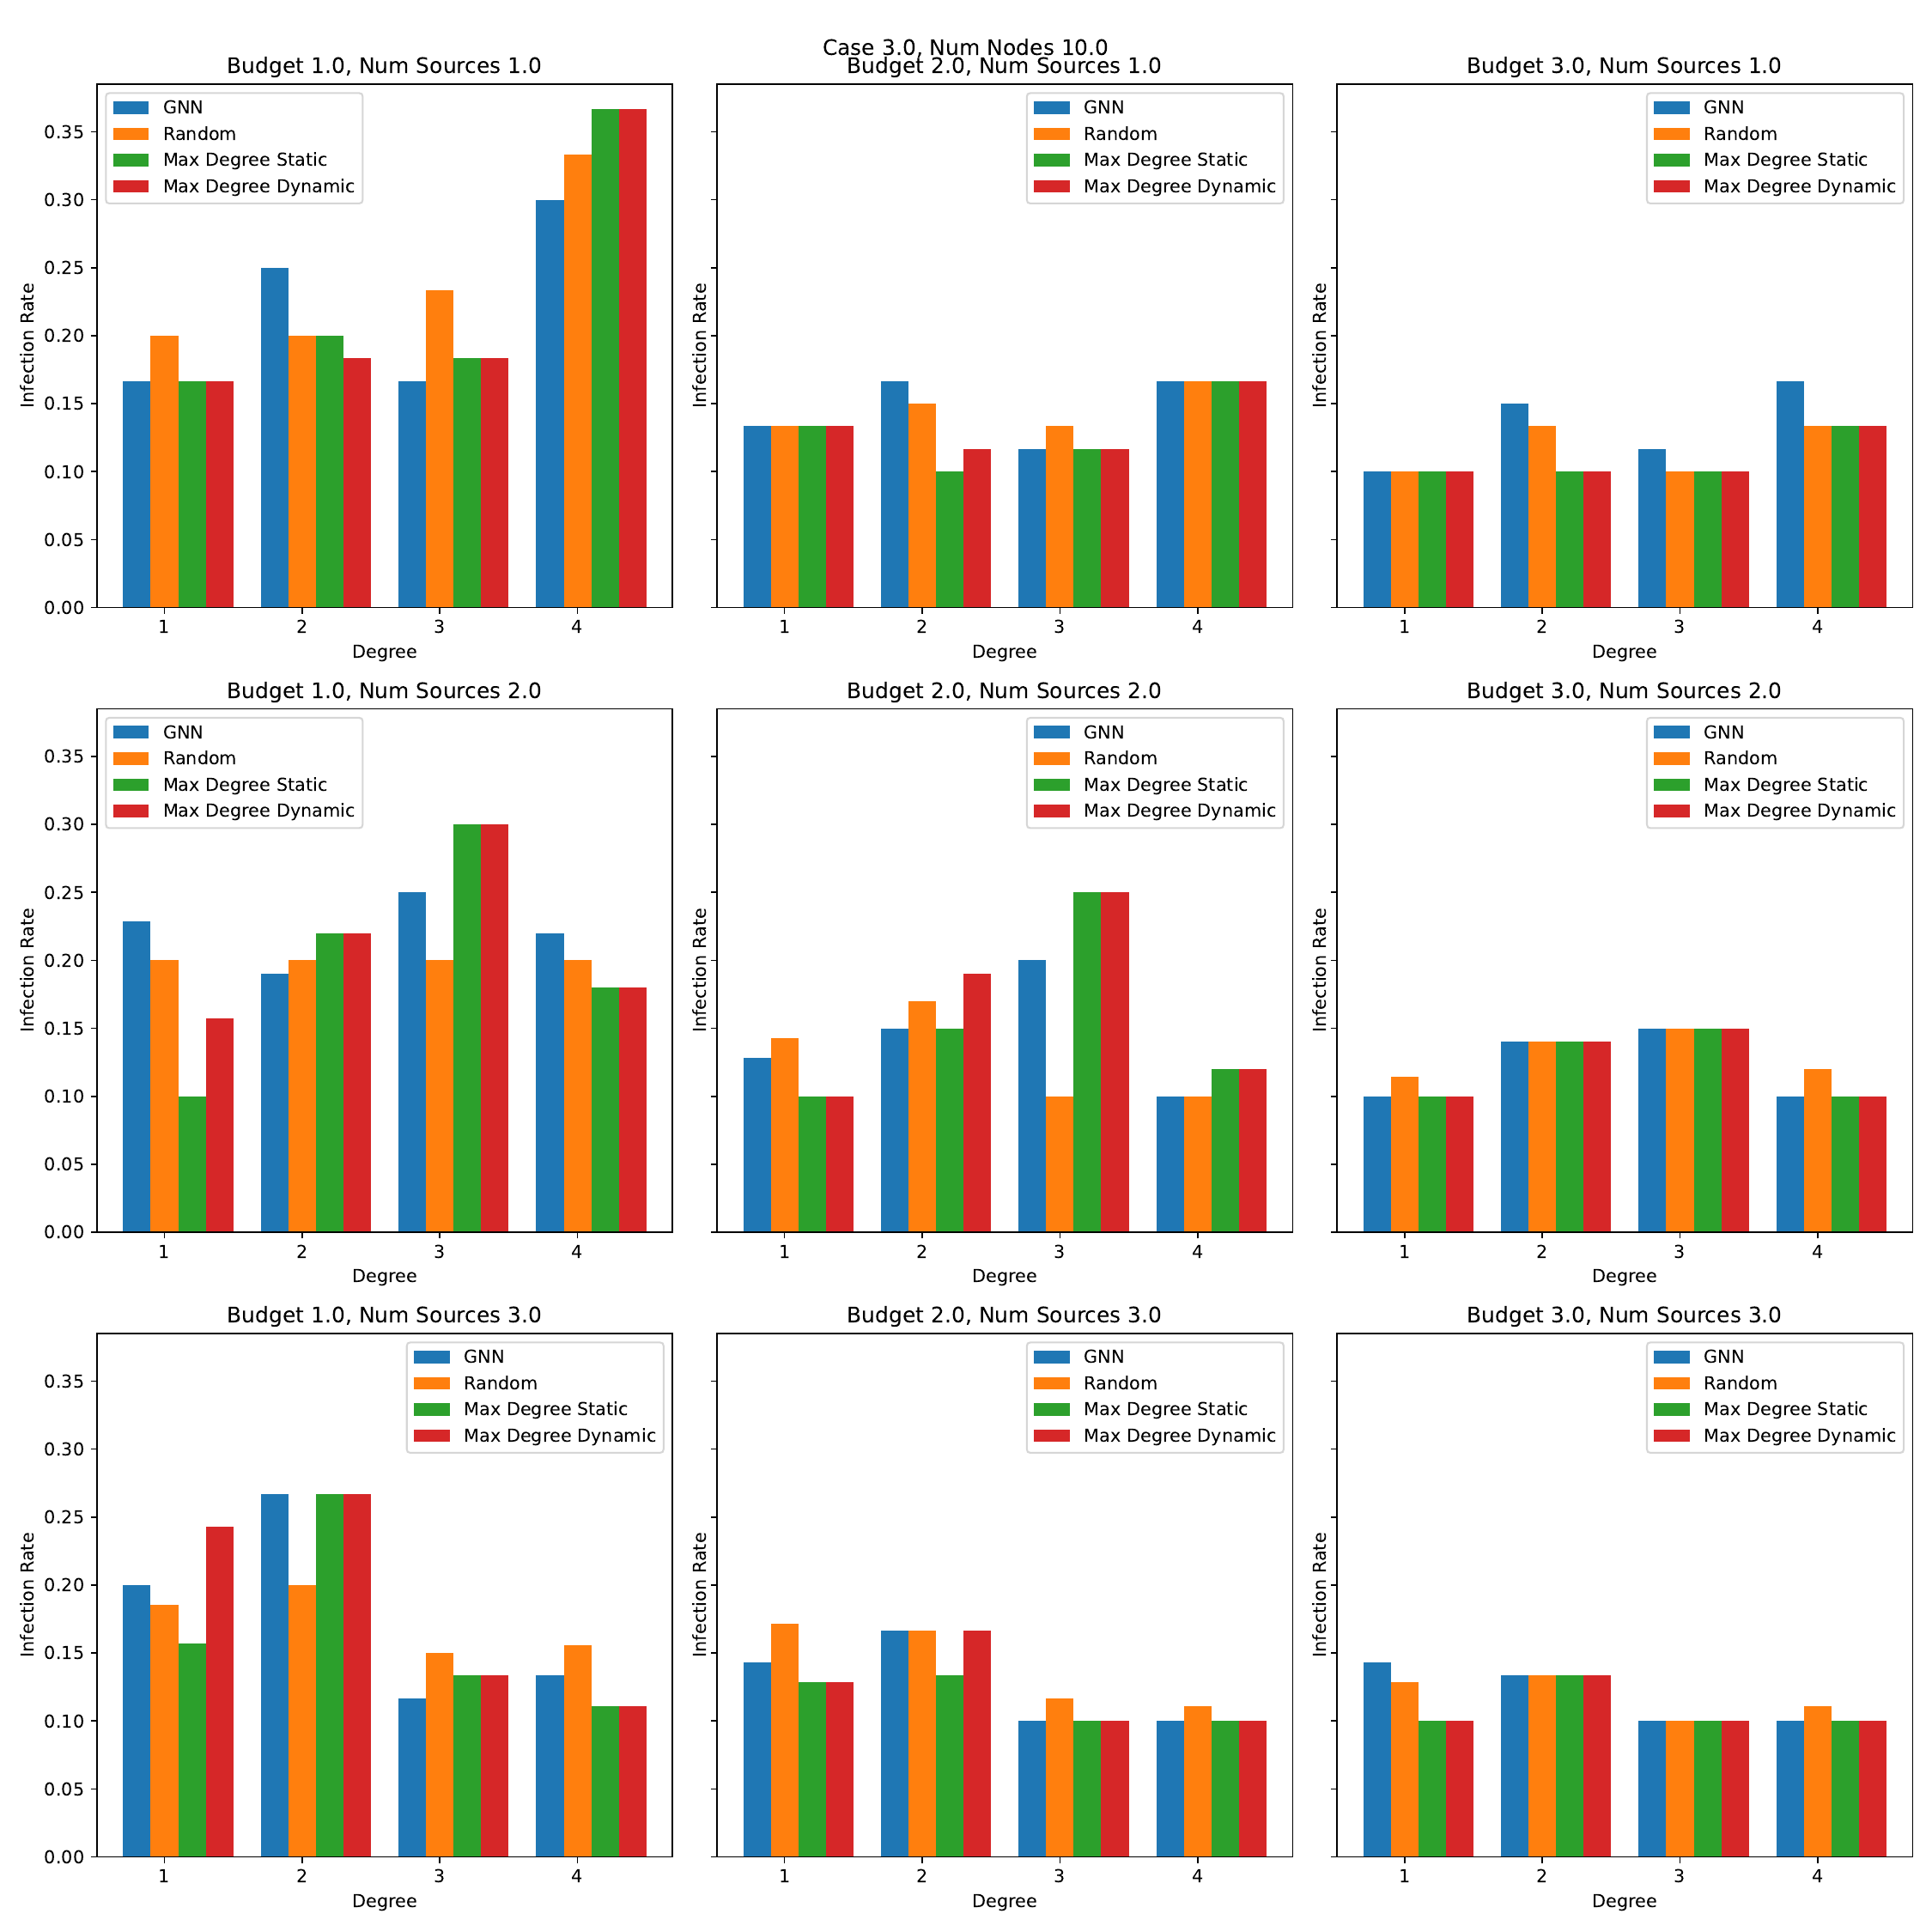}
    \caption{\footnotesize Dataset: Tree, Case-3 Node-10: Performance Evaluation of GCN-Based Supervised Learning Model: This series of bar plots presents a comparative analysis between our GCN-based SL model (blue), Randomized Policy model(yellow), Max Degree Policy model (Static) (green) and Max Degree Policy model (Dynamic) (red) on 10-node network environment. Progressing from left to right, the plots depict scenarios with increasing action budgets, ranging from 1 to 3 actions permitted. Vertically, the plots are ordered to show the effect of varying the initial count of infected nodes, starting with one and increasing to three. Each set of bars within the plots is categorized by the average connectivity (degree) of the infected nodes.}
    \label{fig:Treec3n10}
\end{figure}

\begin{figure}[!h]
    \centering
    \includegraphics[scale=0.3]{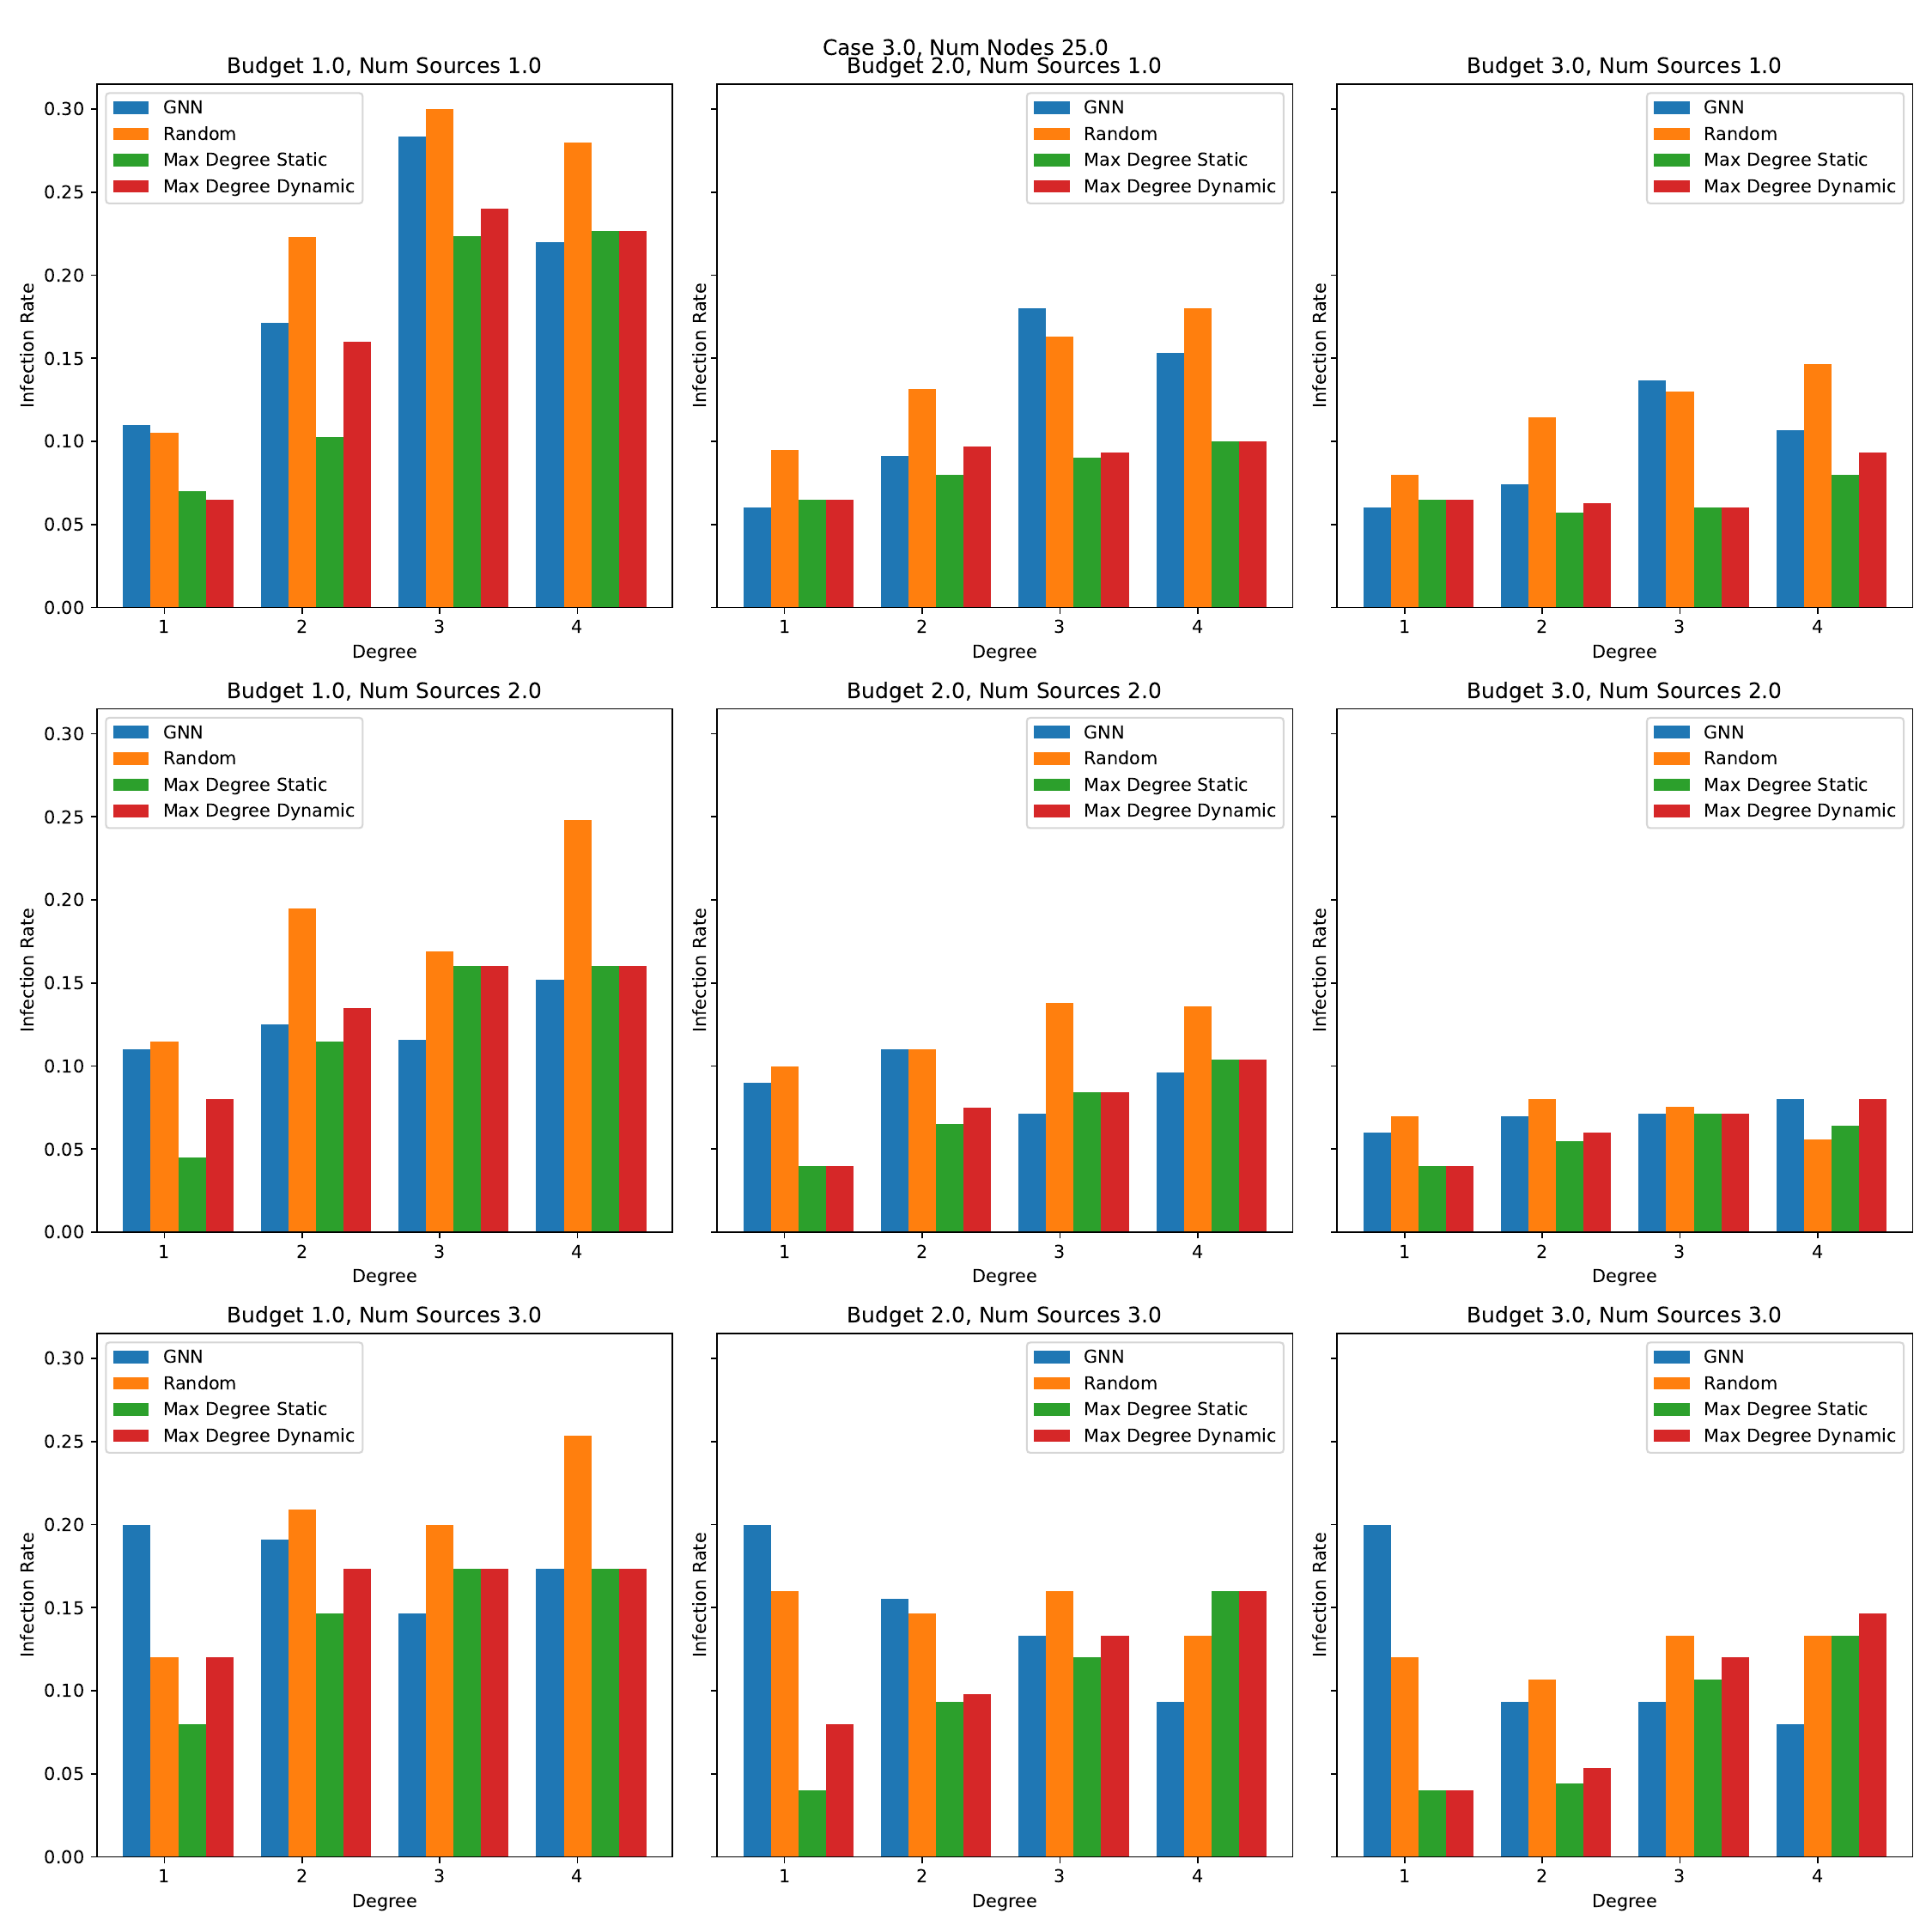}
    \caption{\footnotesize Dataset: Tree, Case-3 Node-25: Performance Evaluation of GCN-Based Supervised Learning Model: This series of bar plots presents a comparative analysis between our GCN-based SL model (blue), Randomized Policy model(yellow), Max Degree Policy model (Static) (green) and Max Degree Policy model (Dynamic) (red) on 25-node network environment. Progressing from left to right, the plots depict scenarios with increasing action budgets, ranging from 1 to 3 actions permitted. Vertically, the plots are ordered to show the effect of varying the initial count of infected nodes, starting with one and increasing to three. Each set of bars within the plots is categorized by the average connectivity (degree) of the infected nodes.}
    \label{fig:Treec3n25}
\end{figure}

\begin{figure}[!h]
    \centering
    \includegraphics[scale=0.3]{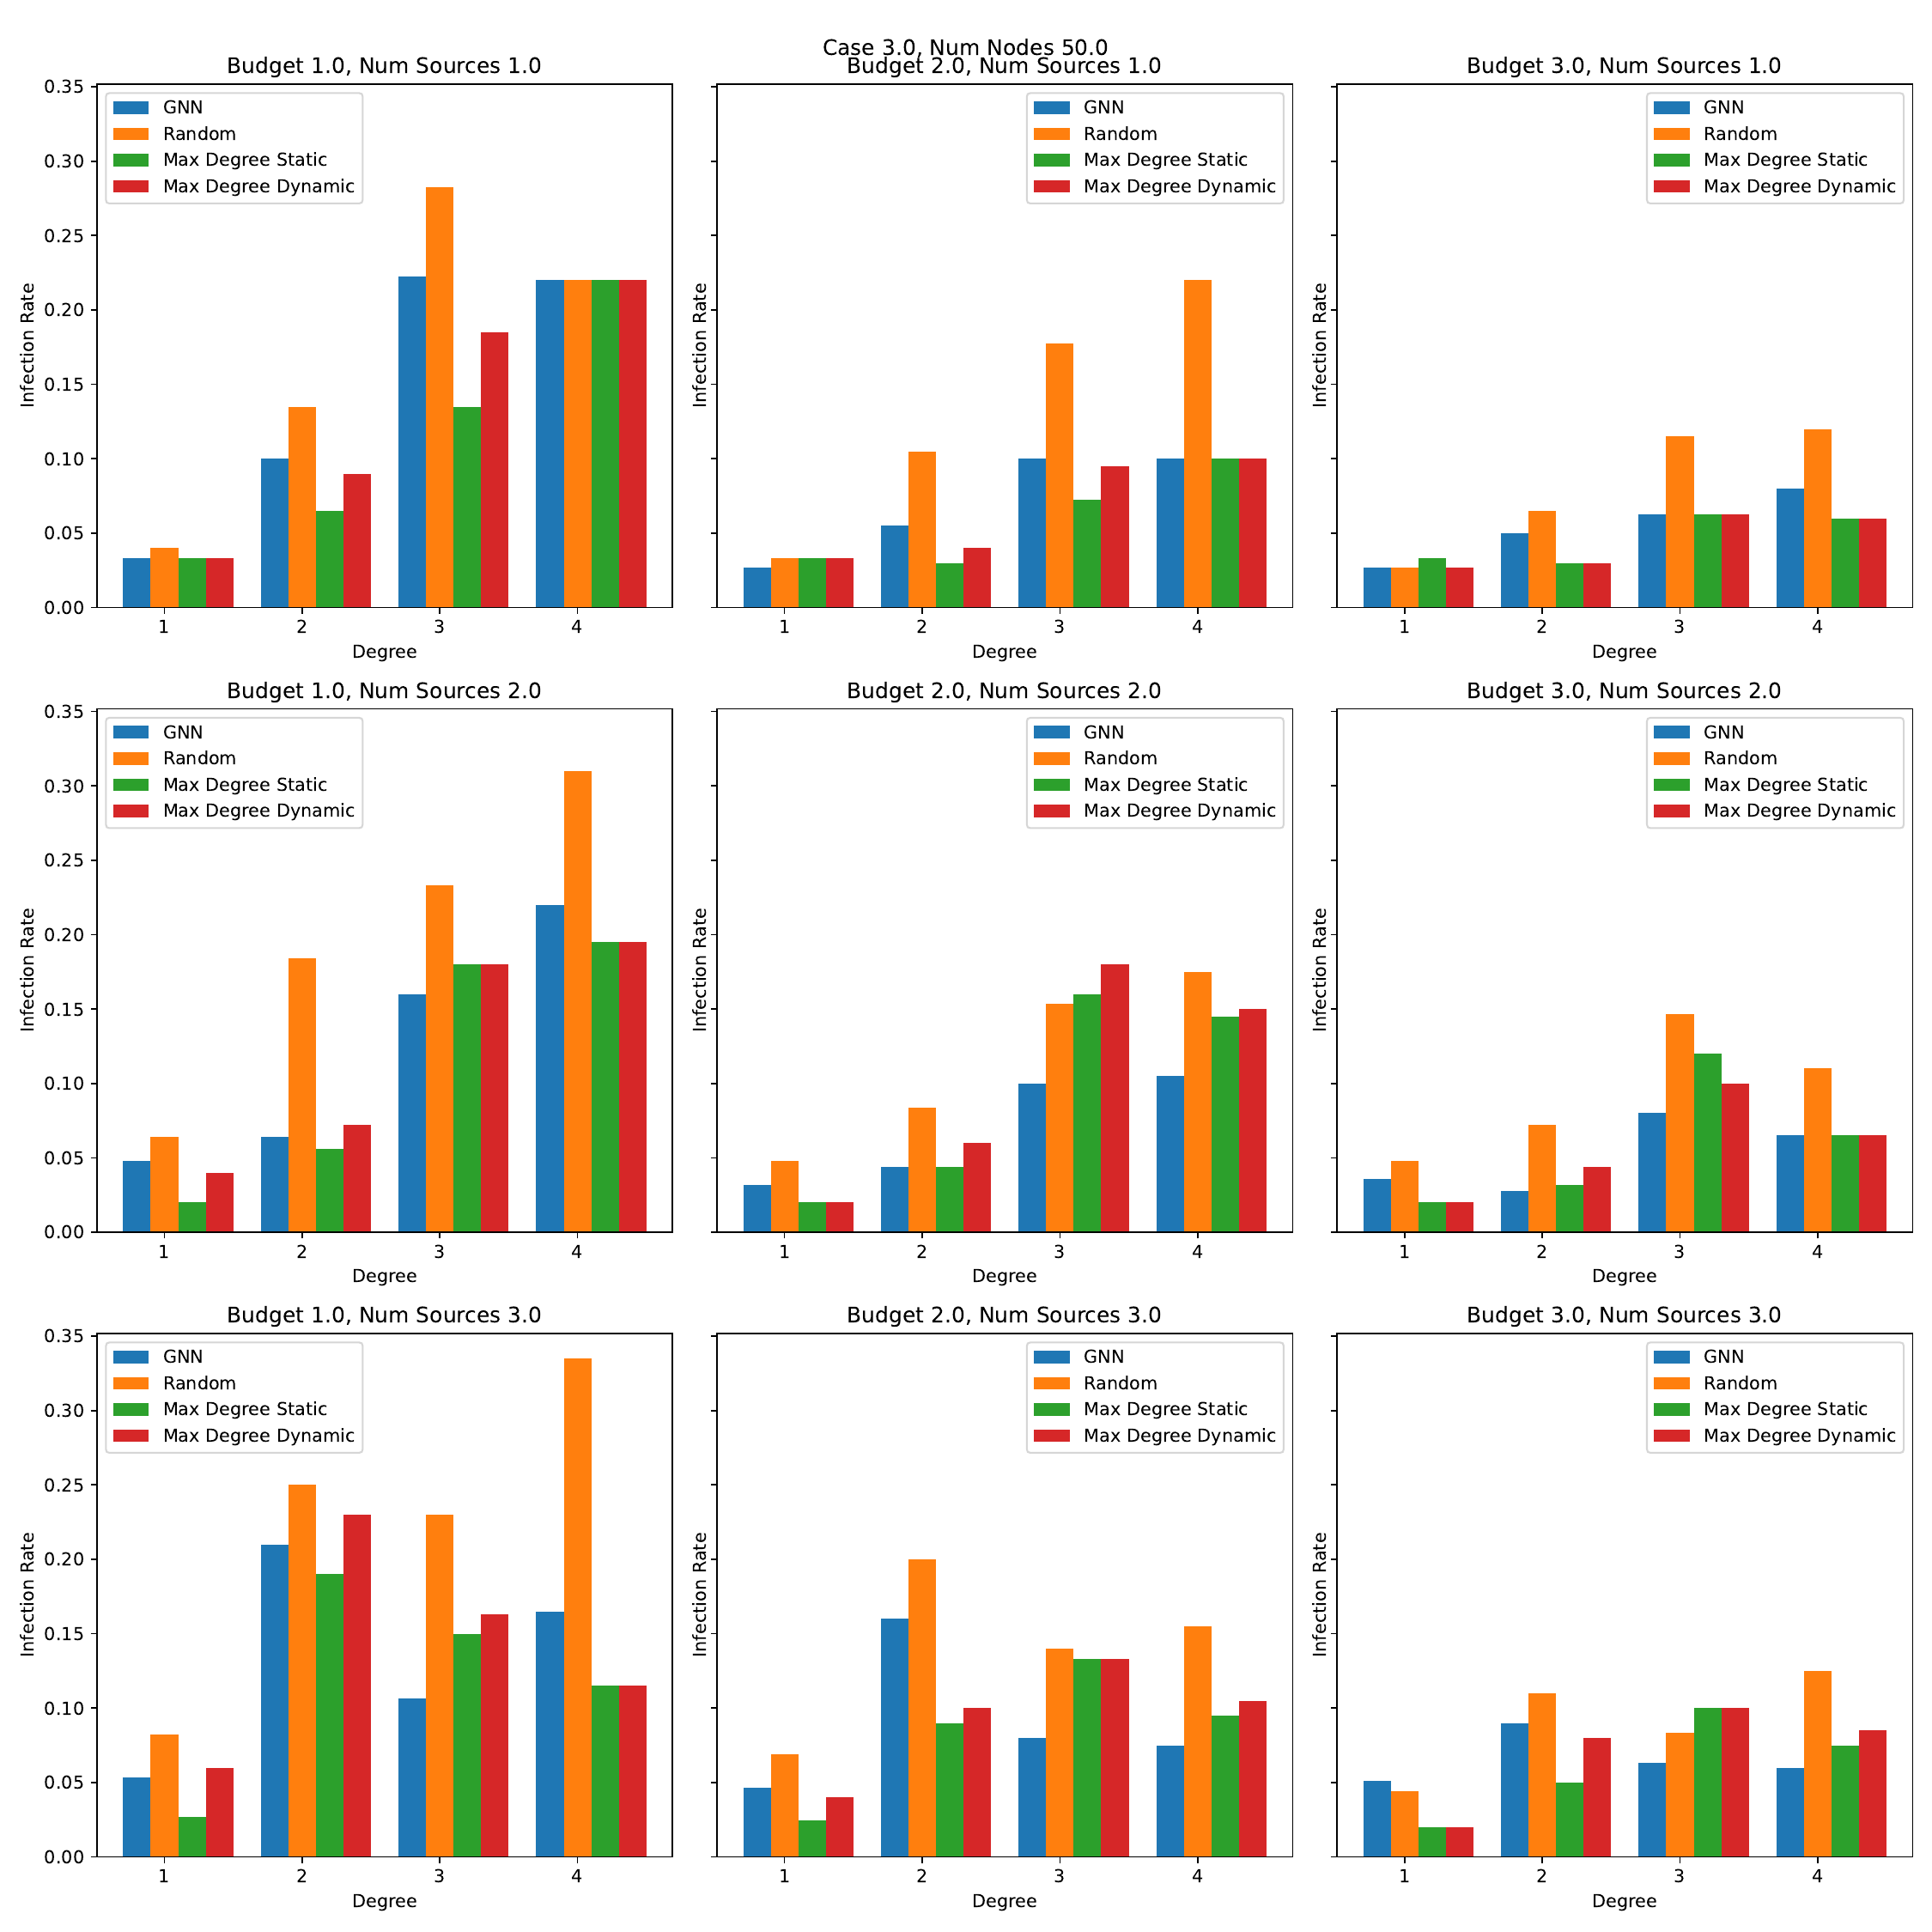}
    \caption{\footnotesize Dataset: Tree, Case-3 Node-50: Performance Evaluation of GCN-Based Supervised Learning Model: This series of bar plots presents a comparative analysis between our GCN-based SL model (blue), Randomized Policy model(yellow), Max Degree Policy model (Static) (green) and Max Degree Policy model (Dynamic) (red) on 25-node network environment. Progressing from left to right, the plots depict scenarios with increasing action budgets, ranging from 1 to 3 actions permitted. Vertically, the plots are ordered to show the effect of varying the initial count of infected nodes, starting with one and increasing to three. Each set of bars within the plots is categorized by the average connectivity (degree) of the infected nodes.}
    \label{fig:Treec3n50}
\end{figure}

\begin{figure}[!h]
    \centering
    \includegraphics[scale=0.3]{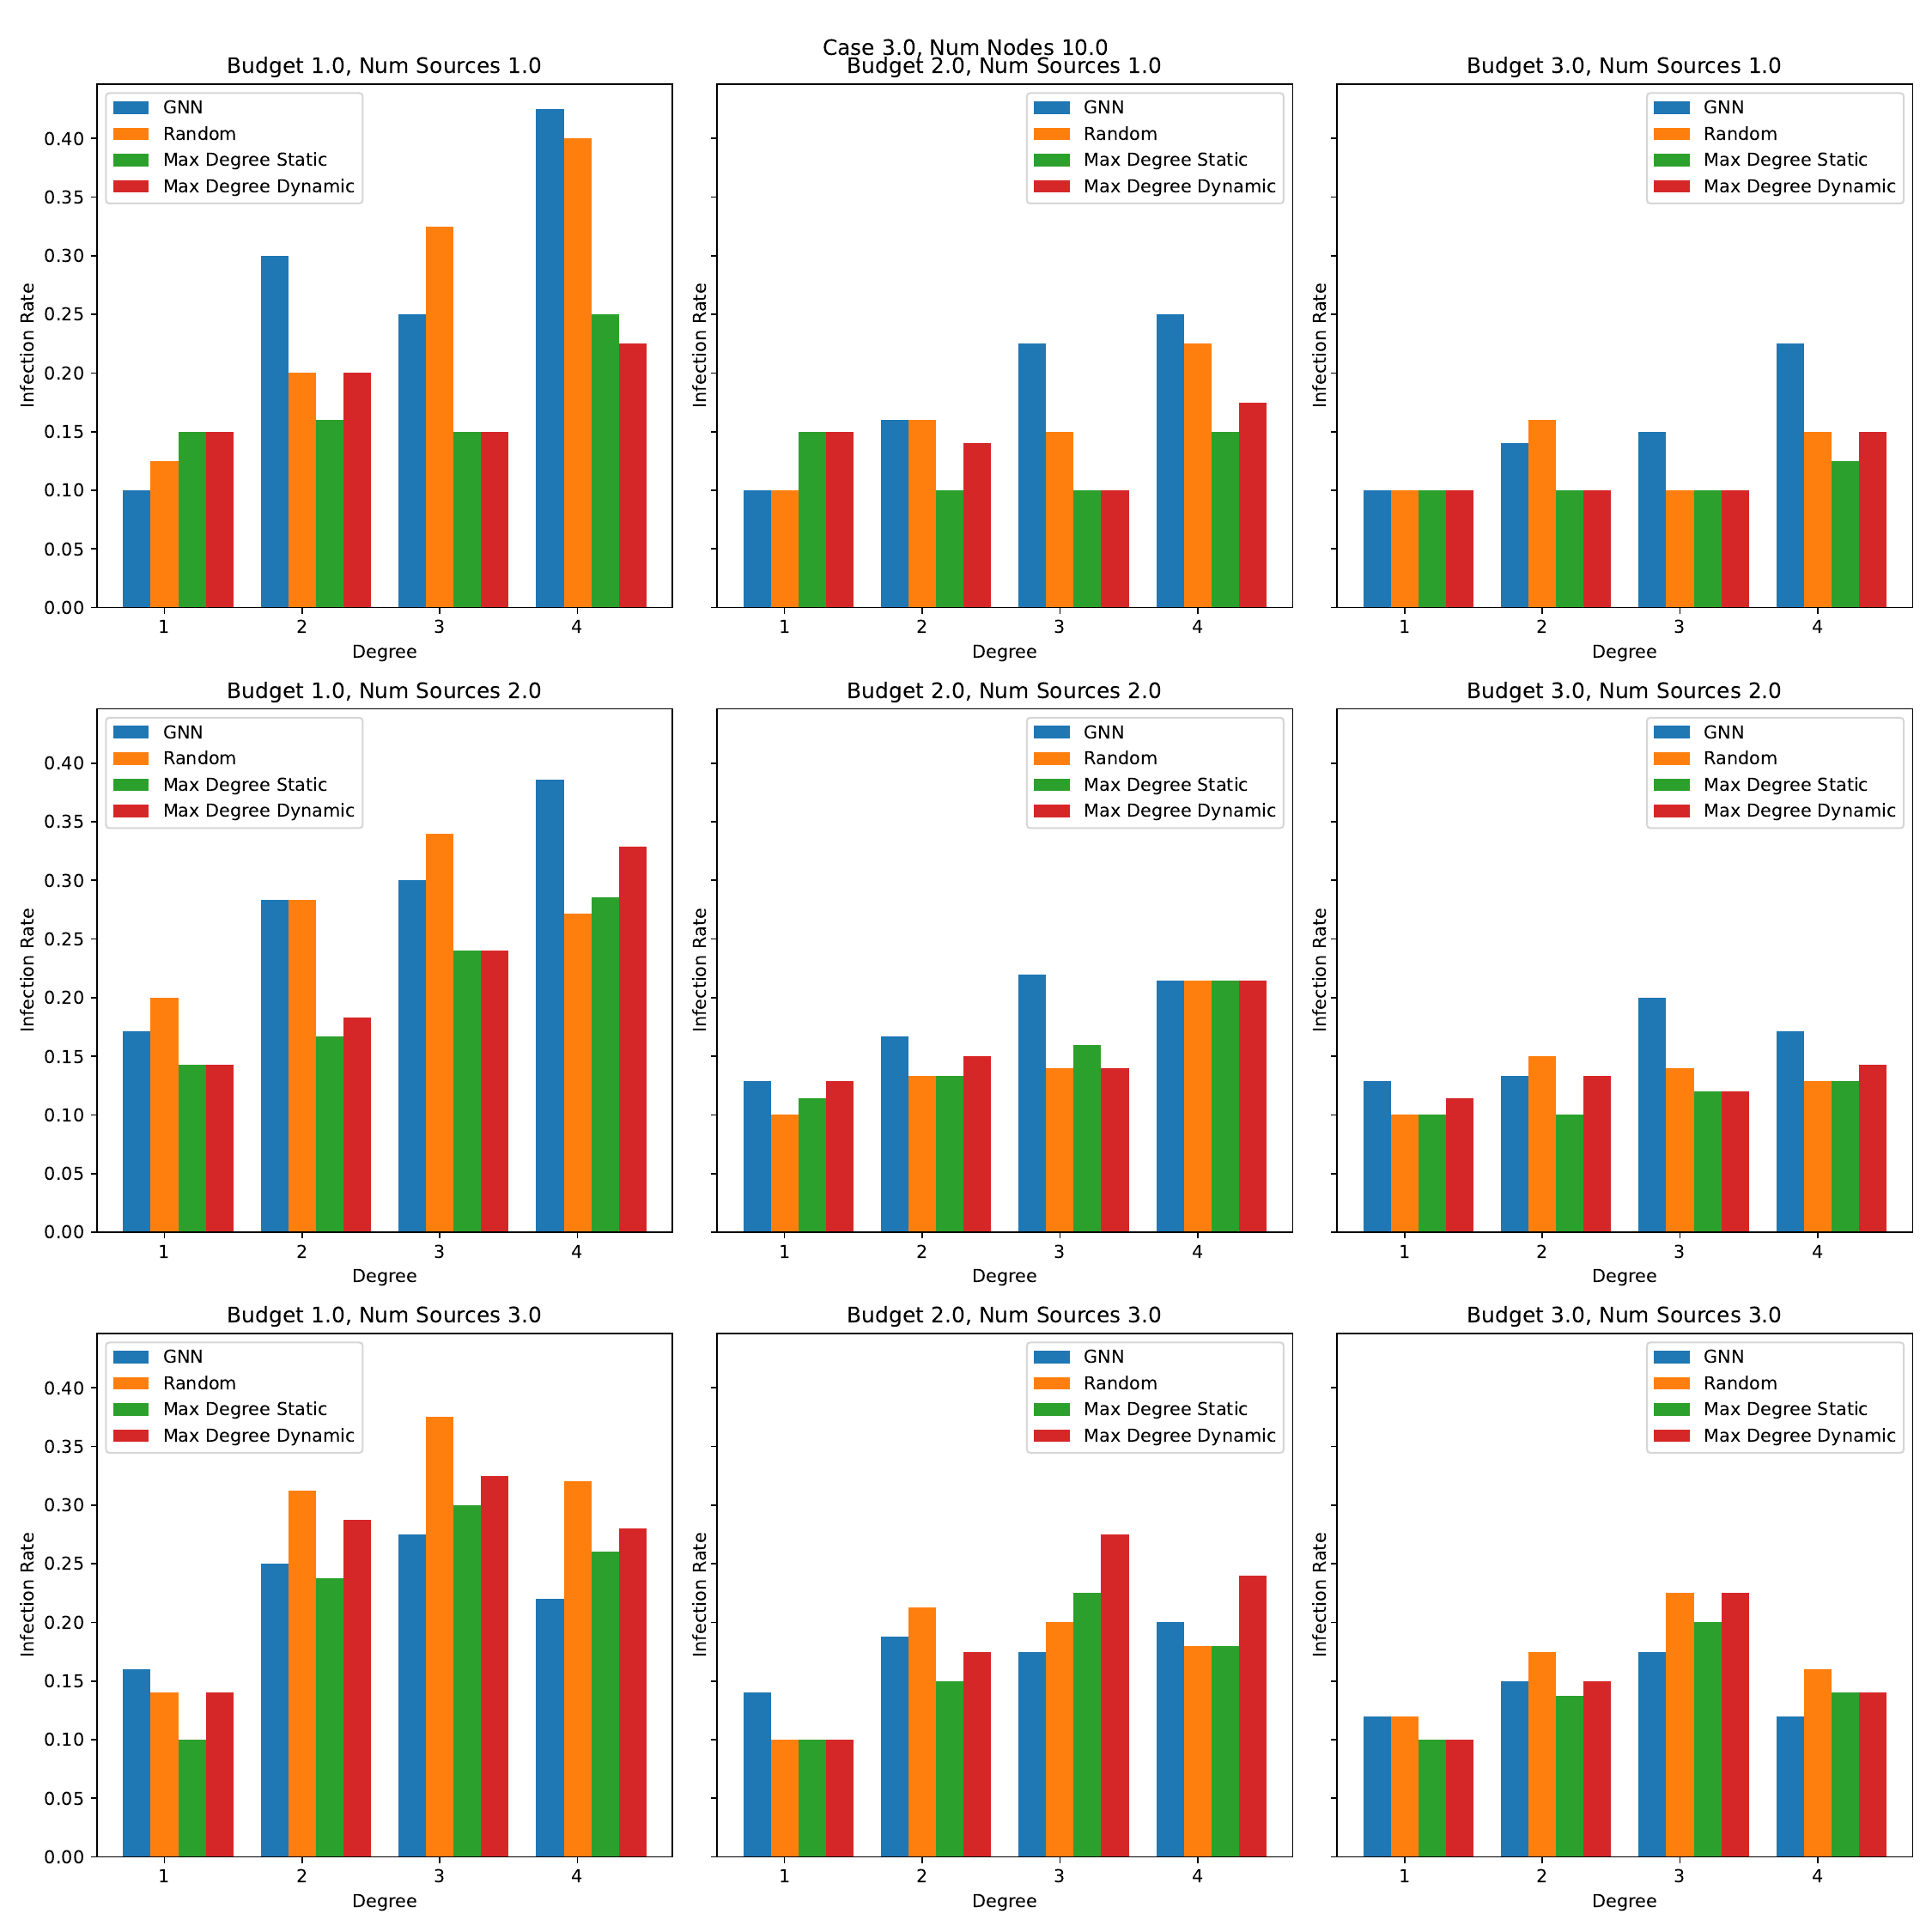}
    \caption{\footnotesize Dataset: Erdos-Renyi, Case-3 Node-10: Performance Evaluation of GCN-Based Supervised Learning Model: This series of bar plots presents a comparative analysis between our GCN-based SL model (blue), Randomized Policy model(yellow), Max Degree Policy model (Static) (green) and Max Degree Policy model (Dynamic) (red) on 25-node network environment. Progressing from left to right, the plots depict scenarios with increasing action budgets, ranging from 1 to 3 actions permitted. Vertically, the plots are ordered to show the effect of varying the initial count of infected nodes, starting with one and increasing to three. Each set of bars within the plots is categorized by the average connectivity (degree) of the infected nodes.}
    \label{fig:ERc3n10}
\end{figure}

\begin{figure}[!h]
    \centering
    \includegraphics[scale=0.3]{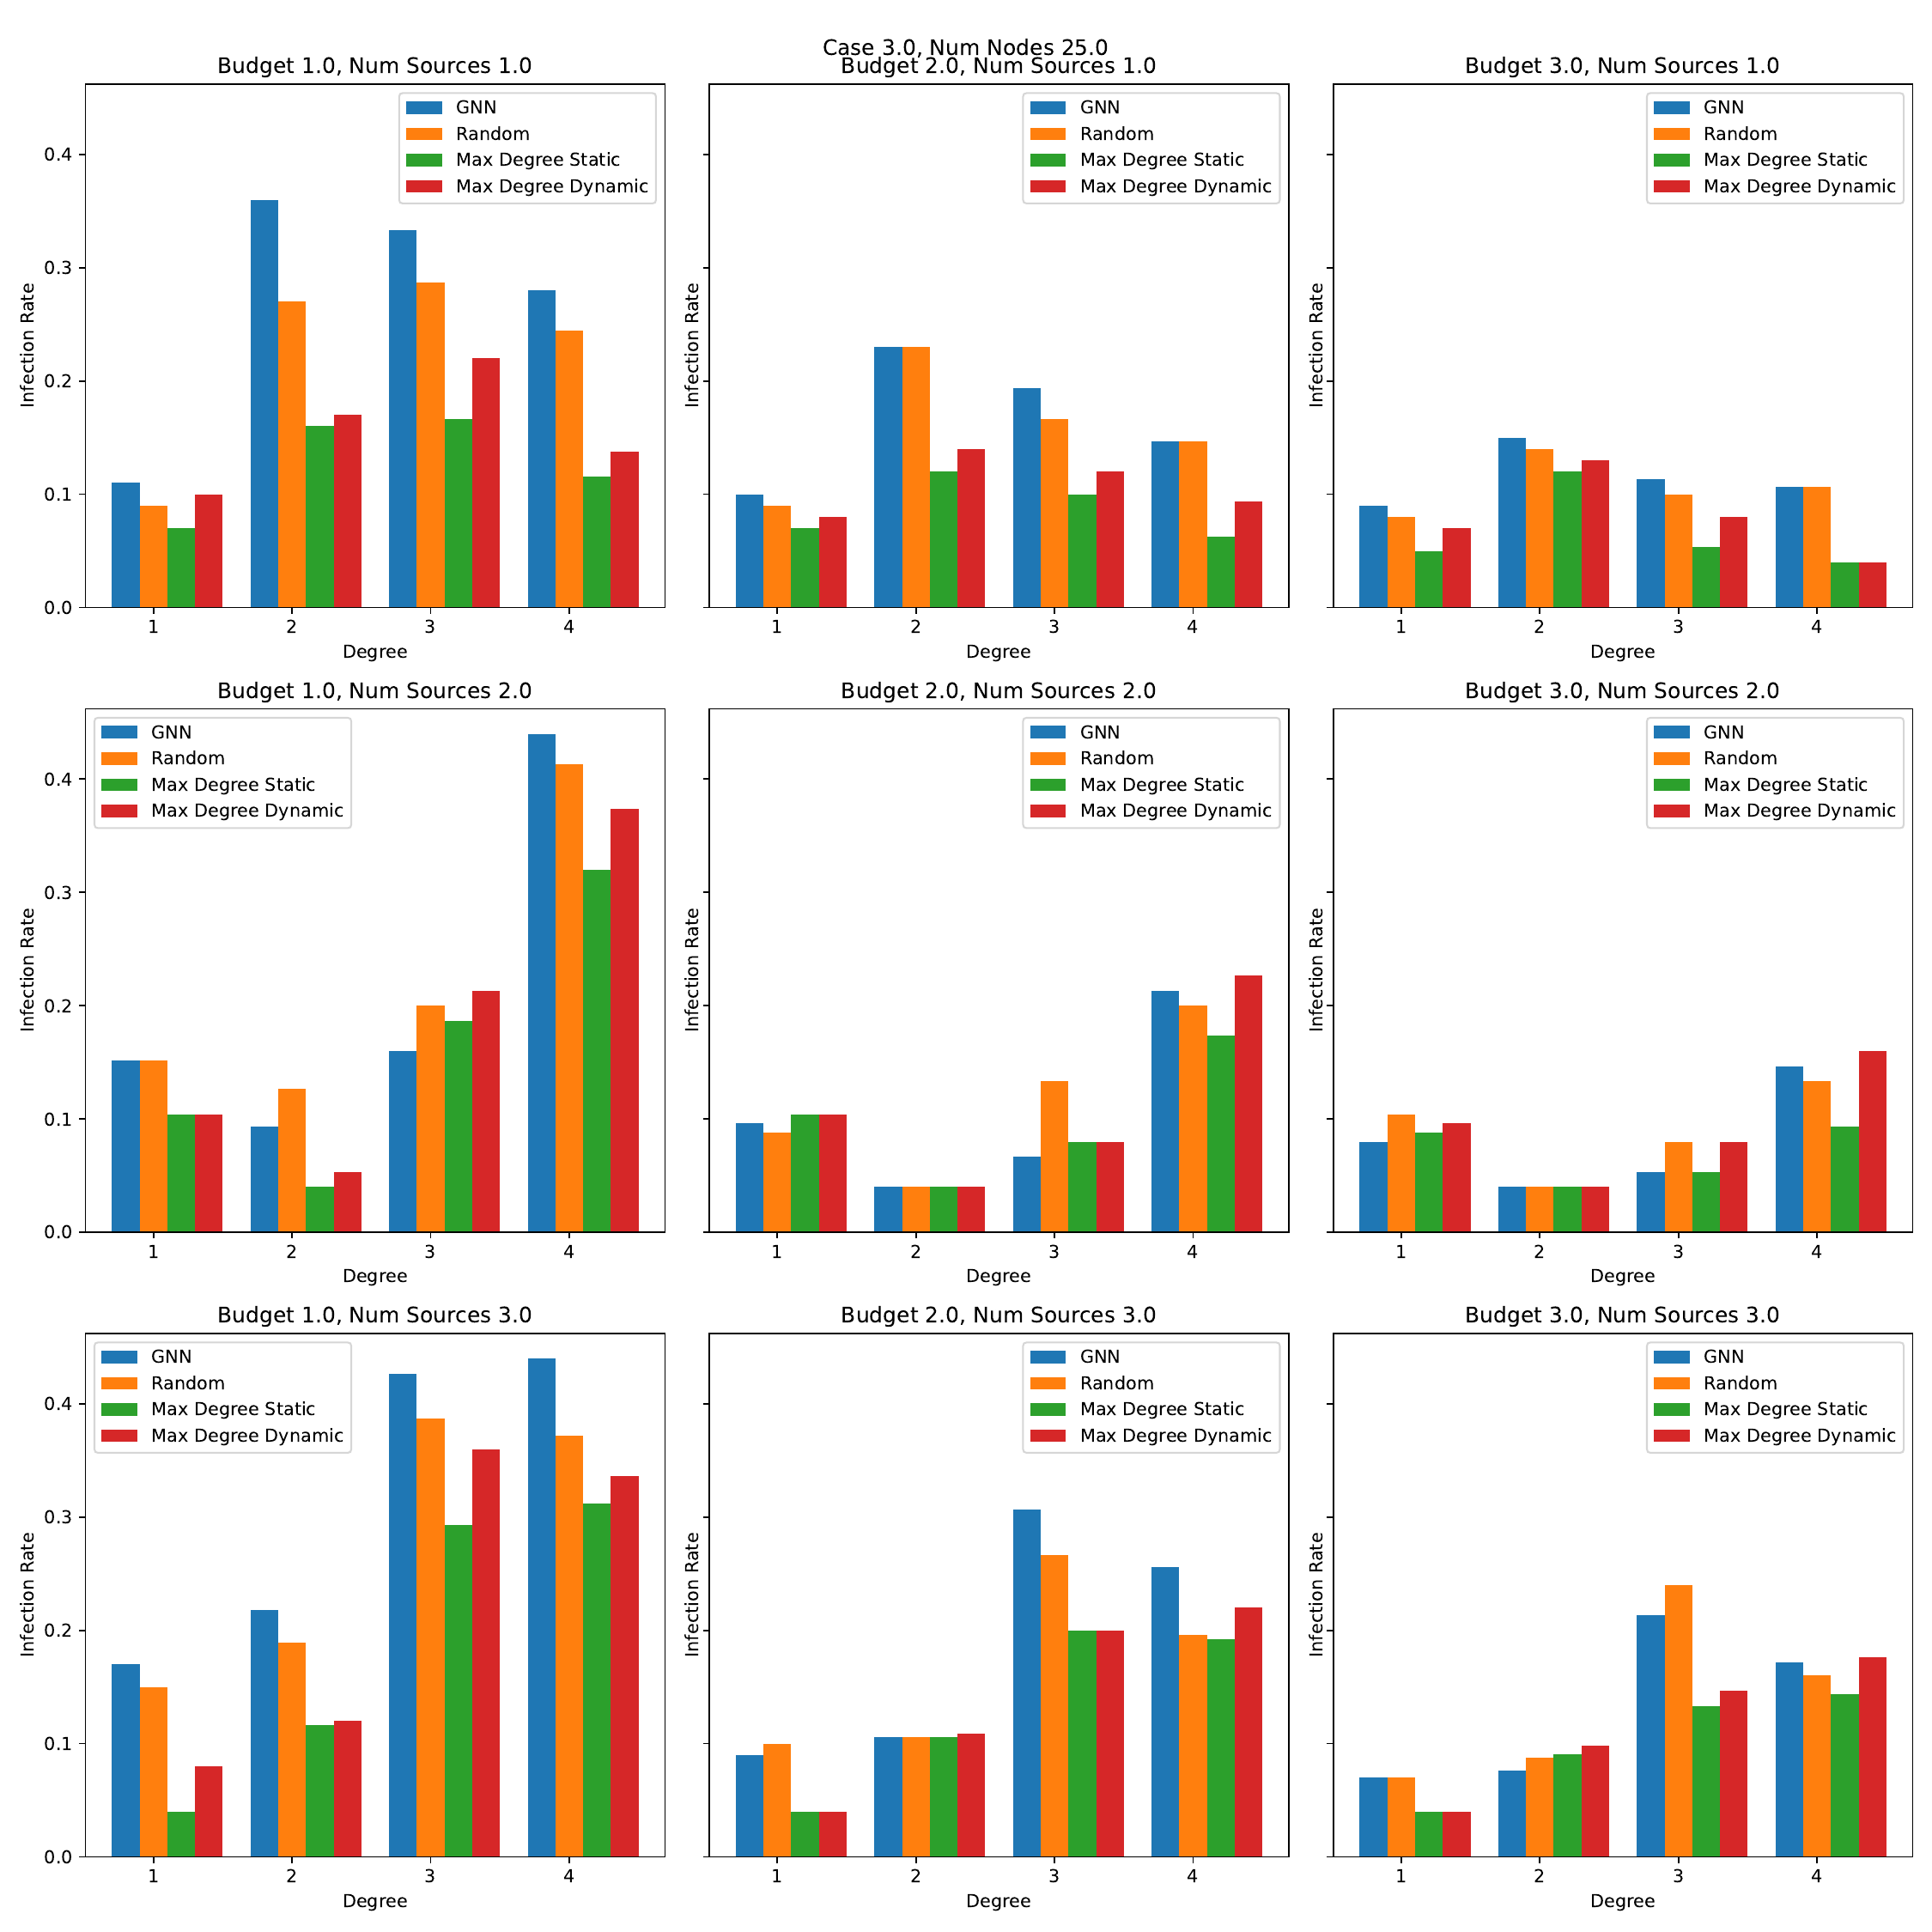}
    \caption{\footnotesize Dataset: Erdos-Renyi, Case-3 Node-25: Performance Evaluation of GCN-Based Supervised Learning Model: This series of bar plots presents a comparative analysis between our GCN-based SL model (blue), Randomized Policy model(yellow), Max Degree Policy model (Static) (green) and Max Degree Policy model (Dynamic) (red) on 25-node network environment. Progressing from left to right, the plots depict scenarios with increasing action budgets, ranging from 1 to 3 actions permitted. Vertically, the plots are ordered to show the effect of varying the initial count of infected nodes, starting with one and increasing to three. Each set of bars within the plots is categorized by the average connectivity (degree) of the infected nodes.}
    \label{fig:ERc3n25}
\end{figure}

\begin{figure}[!h]
    \centering
    \includegraphics[scale=0.3]{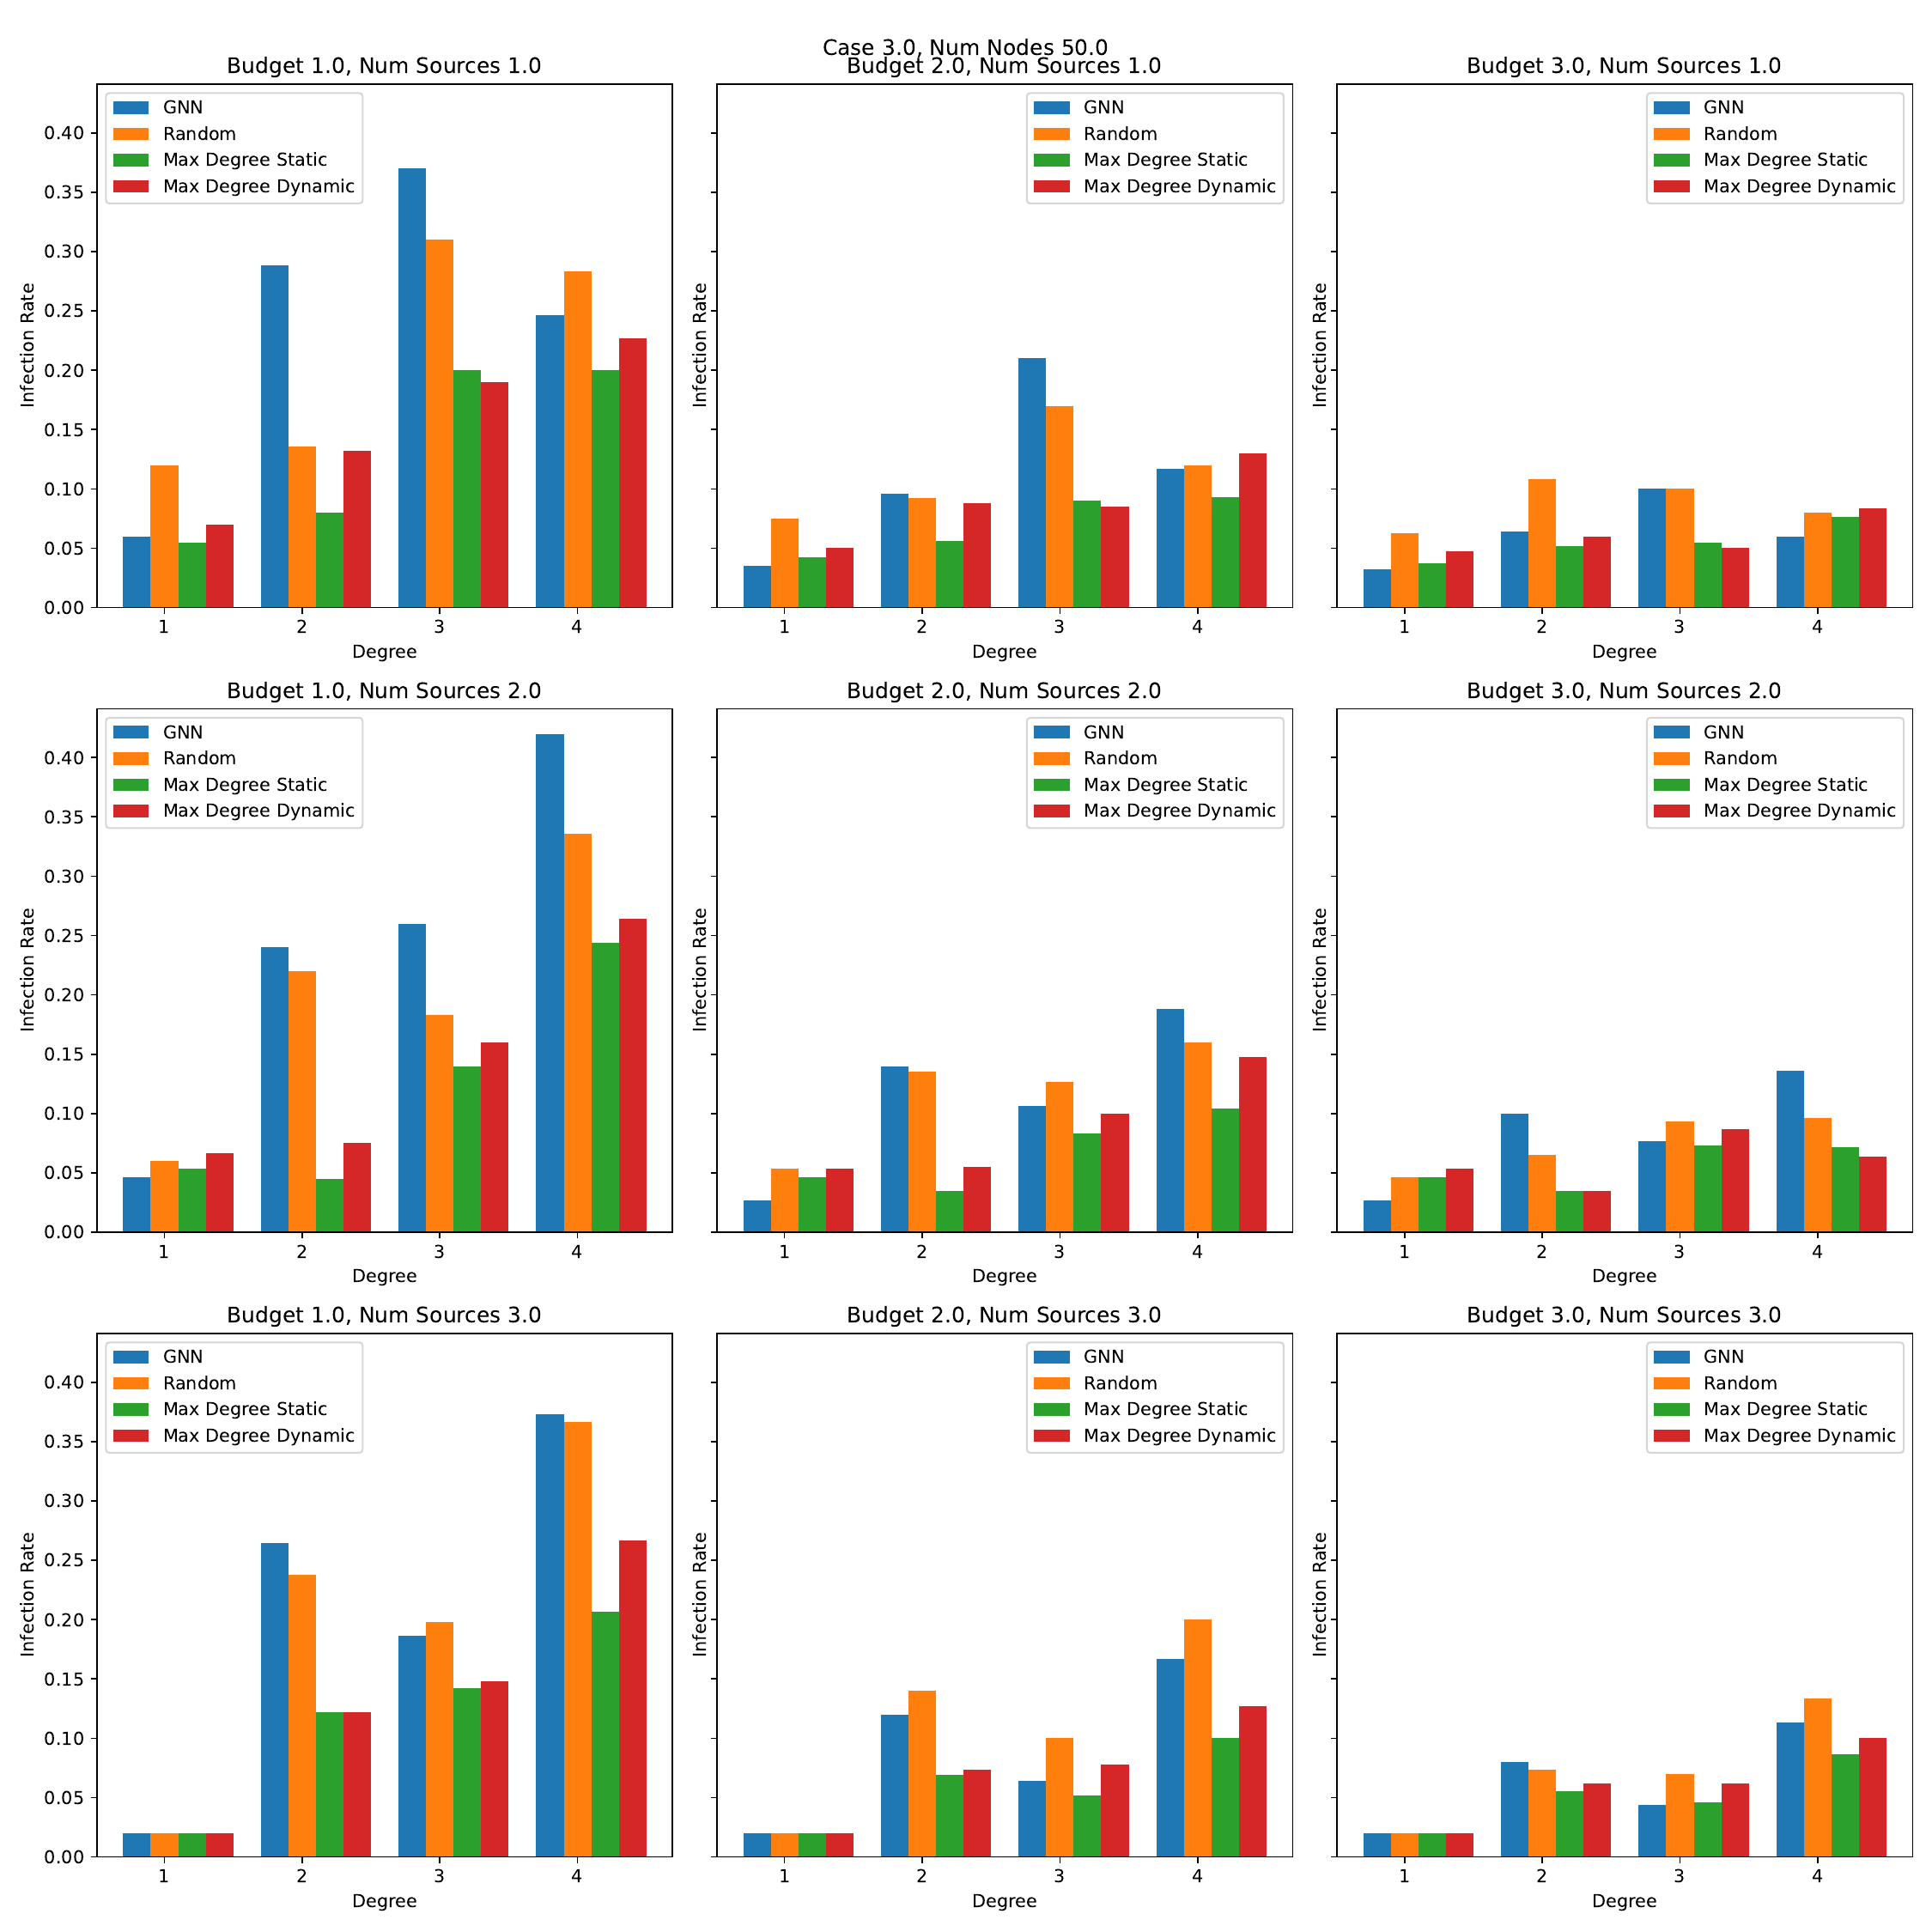}
    \caption{\footnotesize Dataset: Erdos-Renyi, Case-3 Node-50: Performance Evaluation of GCN-Based Supervised Learning Model: This series of bar plots presents a comparative analysis between our GCN-based SL model (blue), Randomized Policy model(yellow), Max Degree Policy model (Static) (green) and Max Degree Policy model (Dynamic) (red) on 25-node network environment. Progressing from left to right, the plots depict scenarios with increasing action budgets, ranging from 1 to 3 actions permitted. Vertically, the plots are ordered to show the effect of varying the initial count of infected nodes, starting with one and increasing to three. Each set of bars within the plots is categorized by the average connectivity (degree) of the infected nodes.}
    \label{fig:ERc3n50}
\end{figure}

%%%%%%%%%%%%%%%%%%%%%%%%%%%%%%%%%%

% ######################################
% ################ RL ##################
% ######################################

%###### Case 1 ResNet Figures #######

%%%%% R0 %%%%%%%%
\begin{figure}[!h]
    \centering
    \includegraphics[scale=0.34]{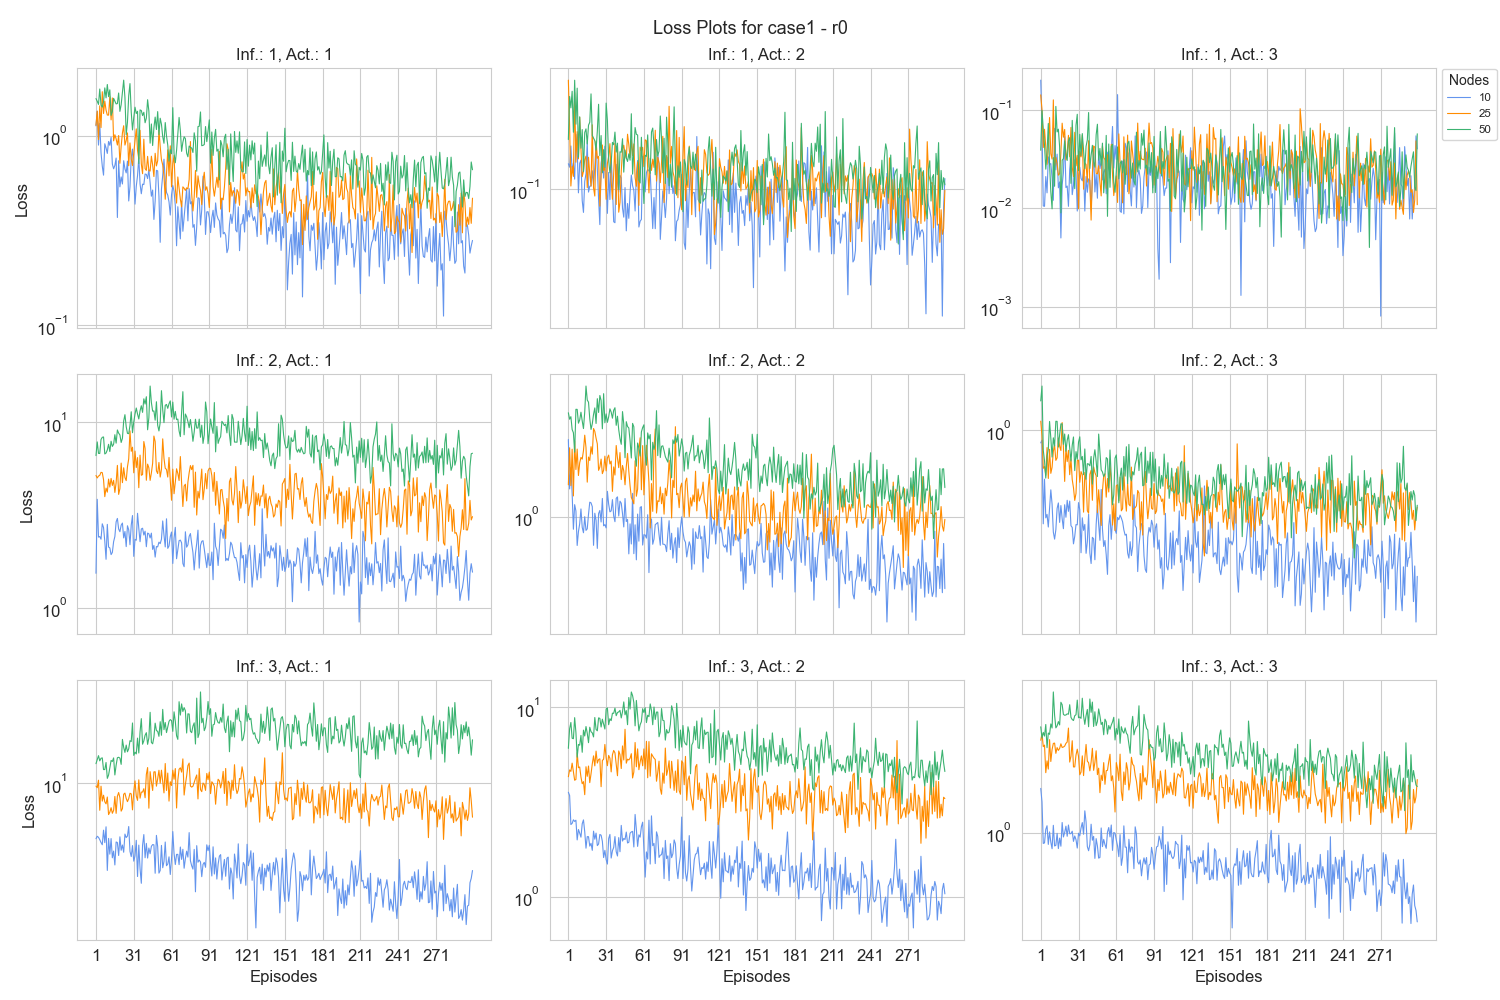}
    \caption{\footnotesize Case-1 using R0: Training MSE loss evolution for RL policy using ResNet model across networks of 10 (blue), 25 (orange), and 50 (green) nodes, for varying initial misinformation sources (Inf.) and action budgets (Act.). Plotted on a logarithmic scale, the loss decreases over episodes, indicating improved policy performance and adaptation across network sizes.}
    \label{fig:resnet_c1r0_loss}
\end{figure}

\begin{figure}
    \centering
    \includegraphics[scale=0.34]{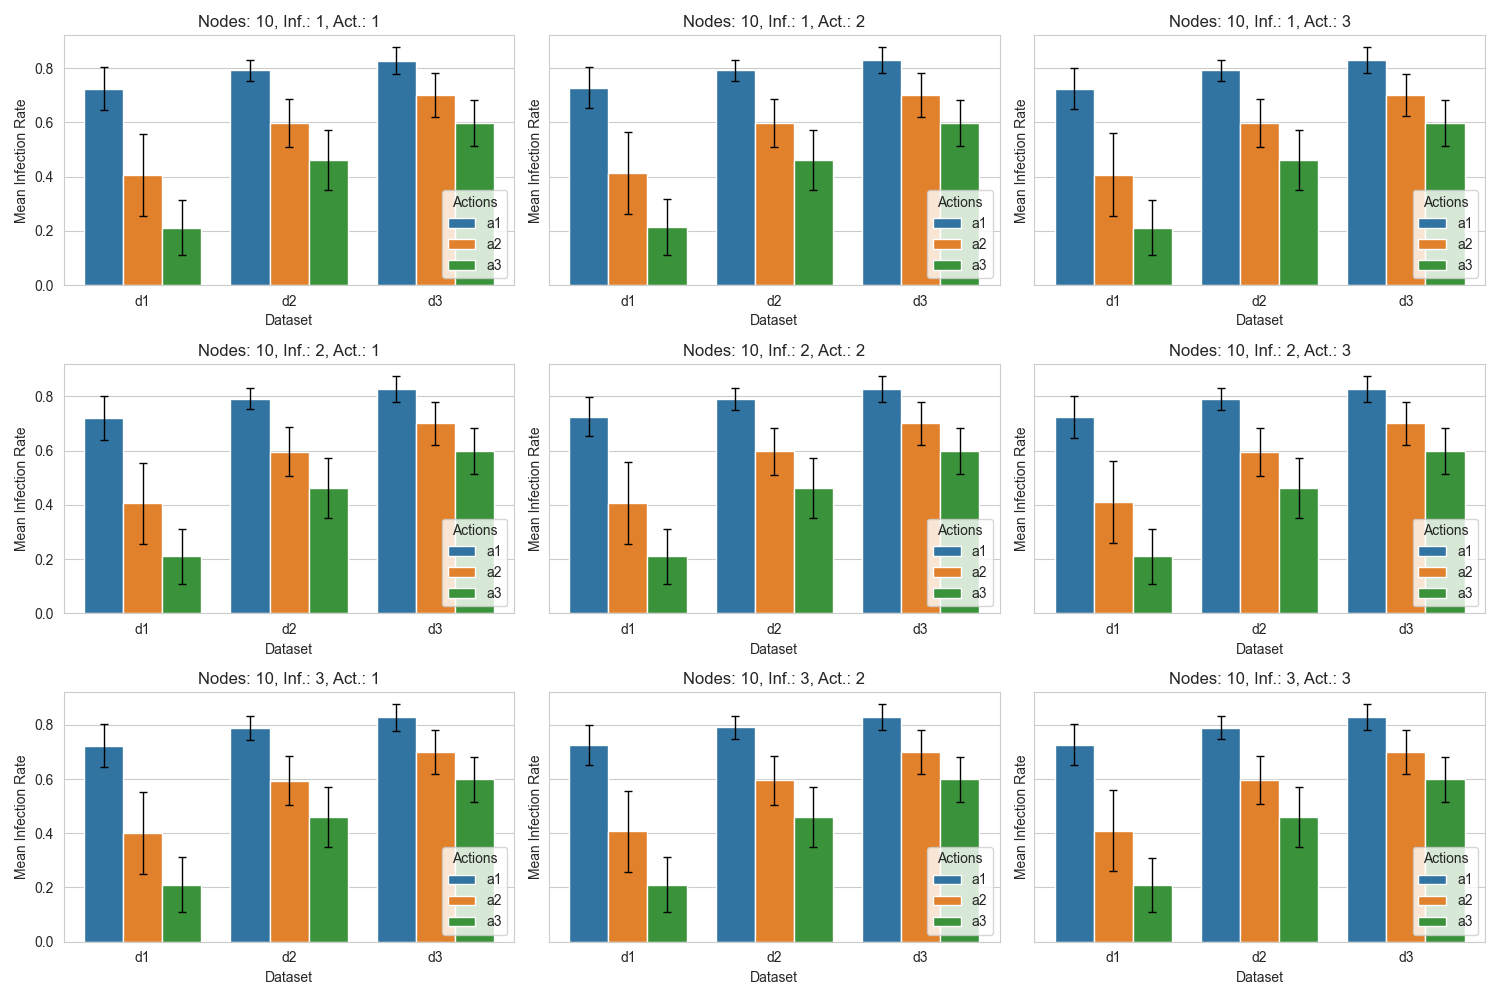}
    \caption{Case-1 using R0: Performance comparison of the RL policies trained using ResNet model for a 10-node network. The barplot displays the mean infection rate for datasets d1, d2, and d3 of Dataset v1 type, differentiated by the number of initial misinformation sources (Inf.) and action budgets (Act.: a1, a2, a3). Each subplot illustrates the performance of a policy trained with the parameters indicated in its title. Lower infection rates indicate more effective policy learning and misinformation containment.}
    \label{fig:inf_resnet_c1r0_10}
\end{figure}

\begin{figure}
    \centering
    \includegraphics[scale=0.34]{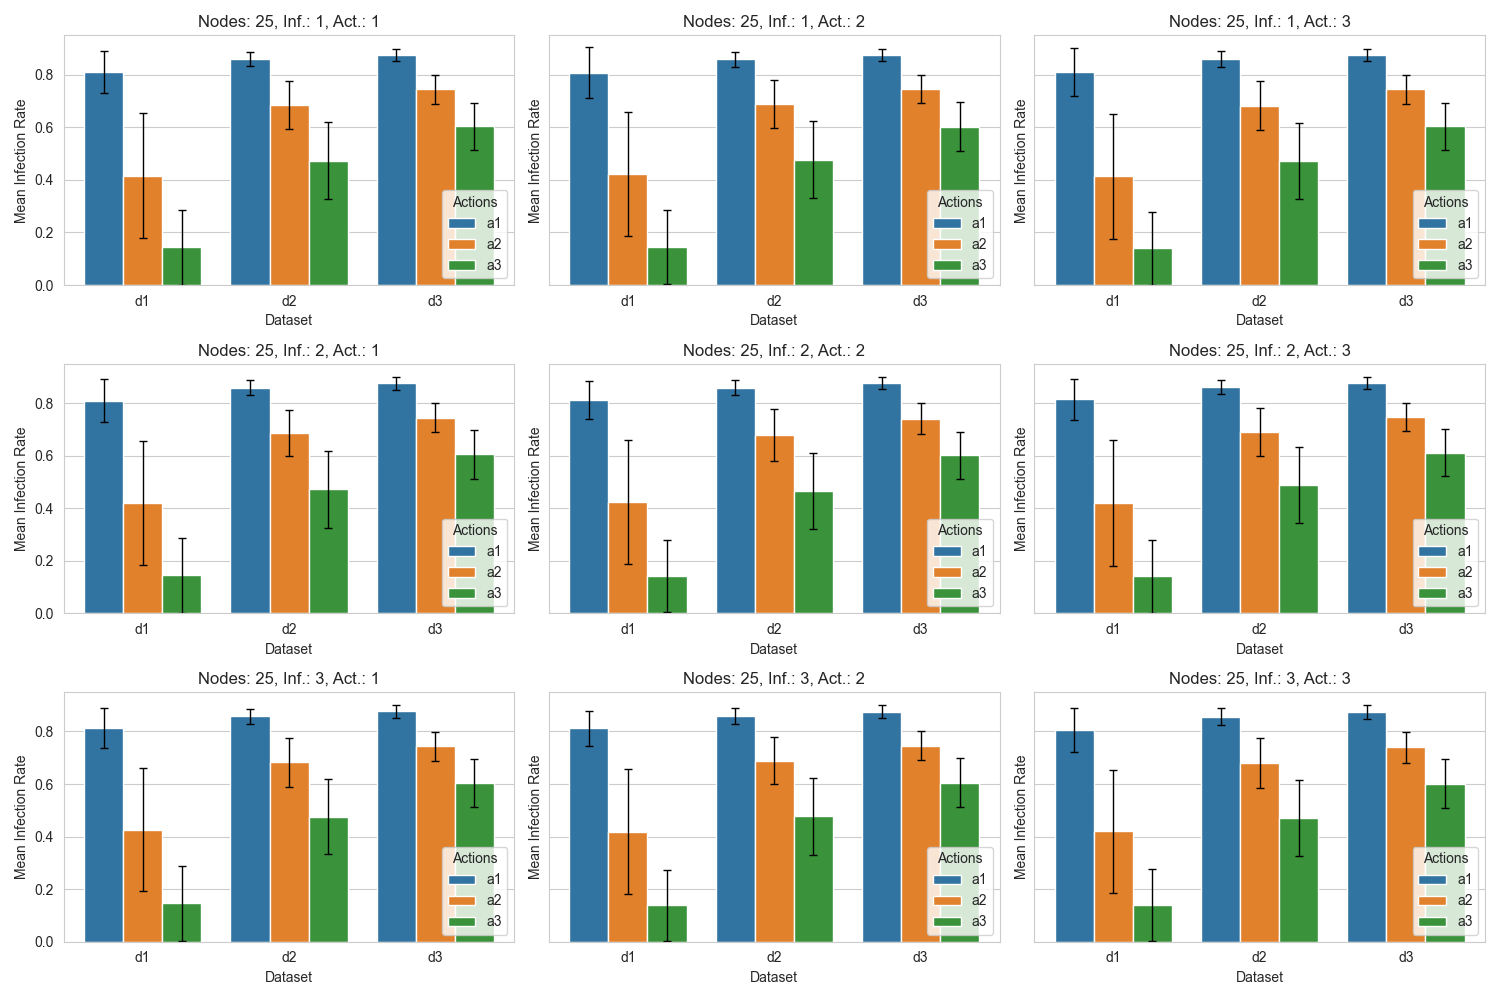}
    \caption{Case-1 using R0: Performance comparison of the RL policies trained using ResNet model for a 25-node network. The barplot displays the mean infection rate for datasets d1, d2, and d3 of Dataset v1 type, differentiated by the number of initial misinformation sources (Inf.) and action budgets (Act.: a1, a2, a3). Each subplot illustrates the performance of a policy trained with the parameters indicated in its title. Lower infection rates indicate more effective policy learning and misinformation containment.}
    \label{fig:inf_resnet_c1r0_25}
\end{figure}

\begin{figure}
    \centering
    \includegraphics[scale=0.34]{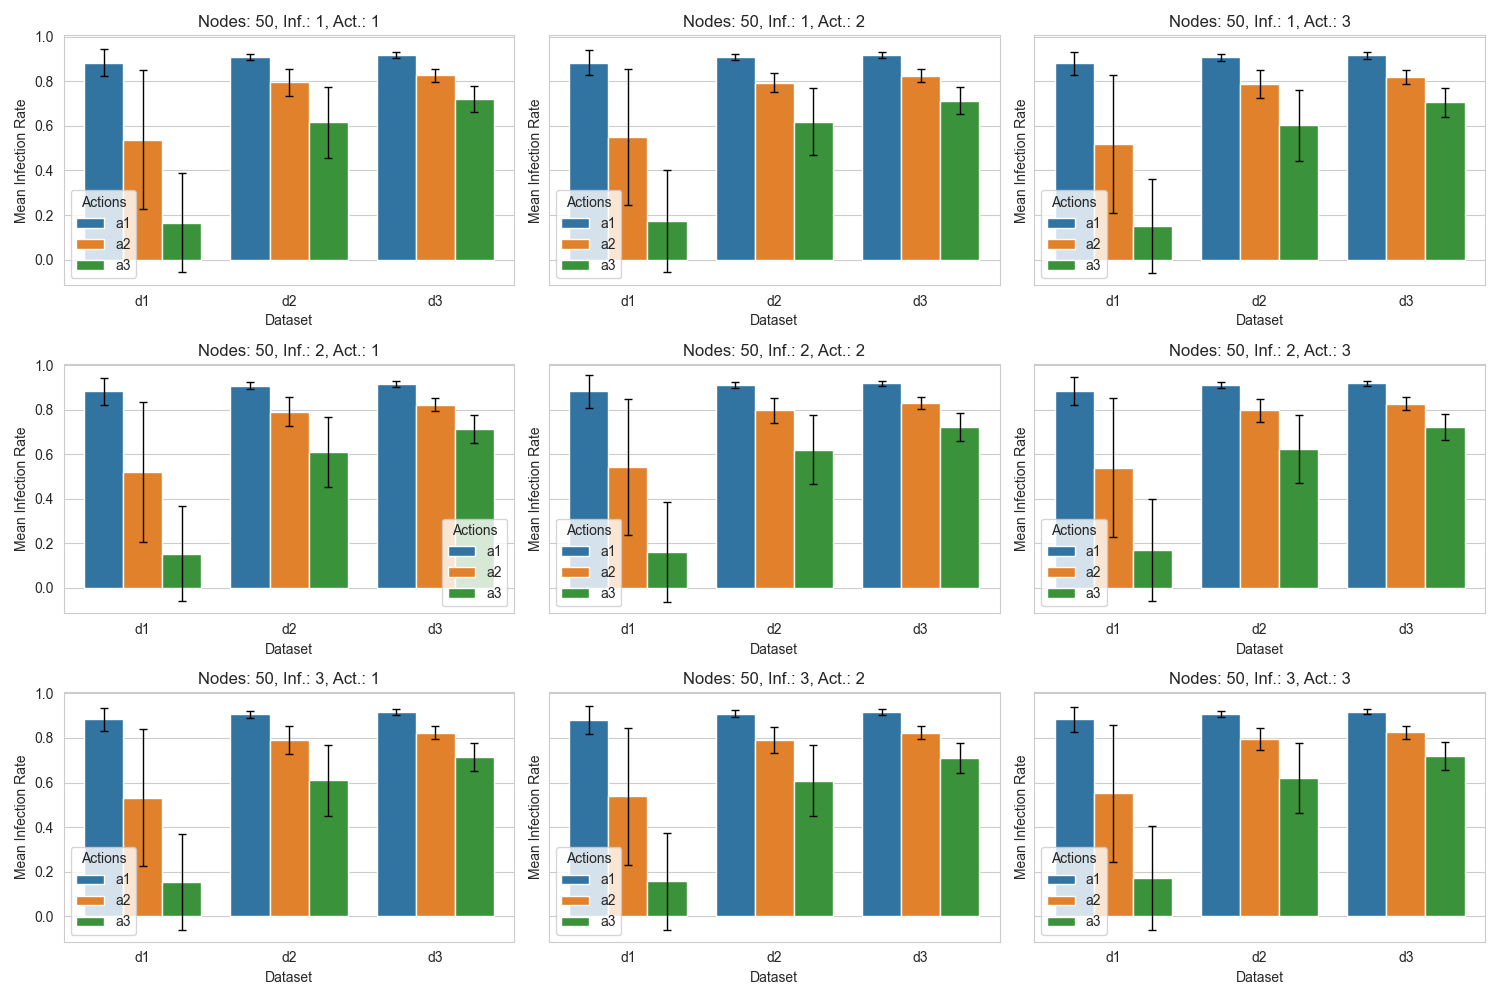}
    \caption{Case-1 using R0: Performance comparison of the RL policies trained using ResNet model for a 50-node network. The barplot displays the mean infection rate for datasets d1, d2, and d3 of Dataset v1 type, differentiated by the number of initial misinformation sources (Inf.) and action budgets (Act.: a1, a2, a3). Each subplot illustrates the performance of a policy trained with the parameters indicated in its title. Lower infection rates indicate more effective policy learning and misinformation containment.}
    \label{fig:inf_resnet_c1r0_50}
\end{figure}

%%%%%% R1 %%%%%%%%

\begin{figure}[!h]
    \centering
    \includegraphics[scale=0.34]{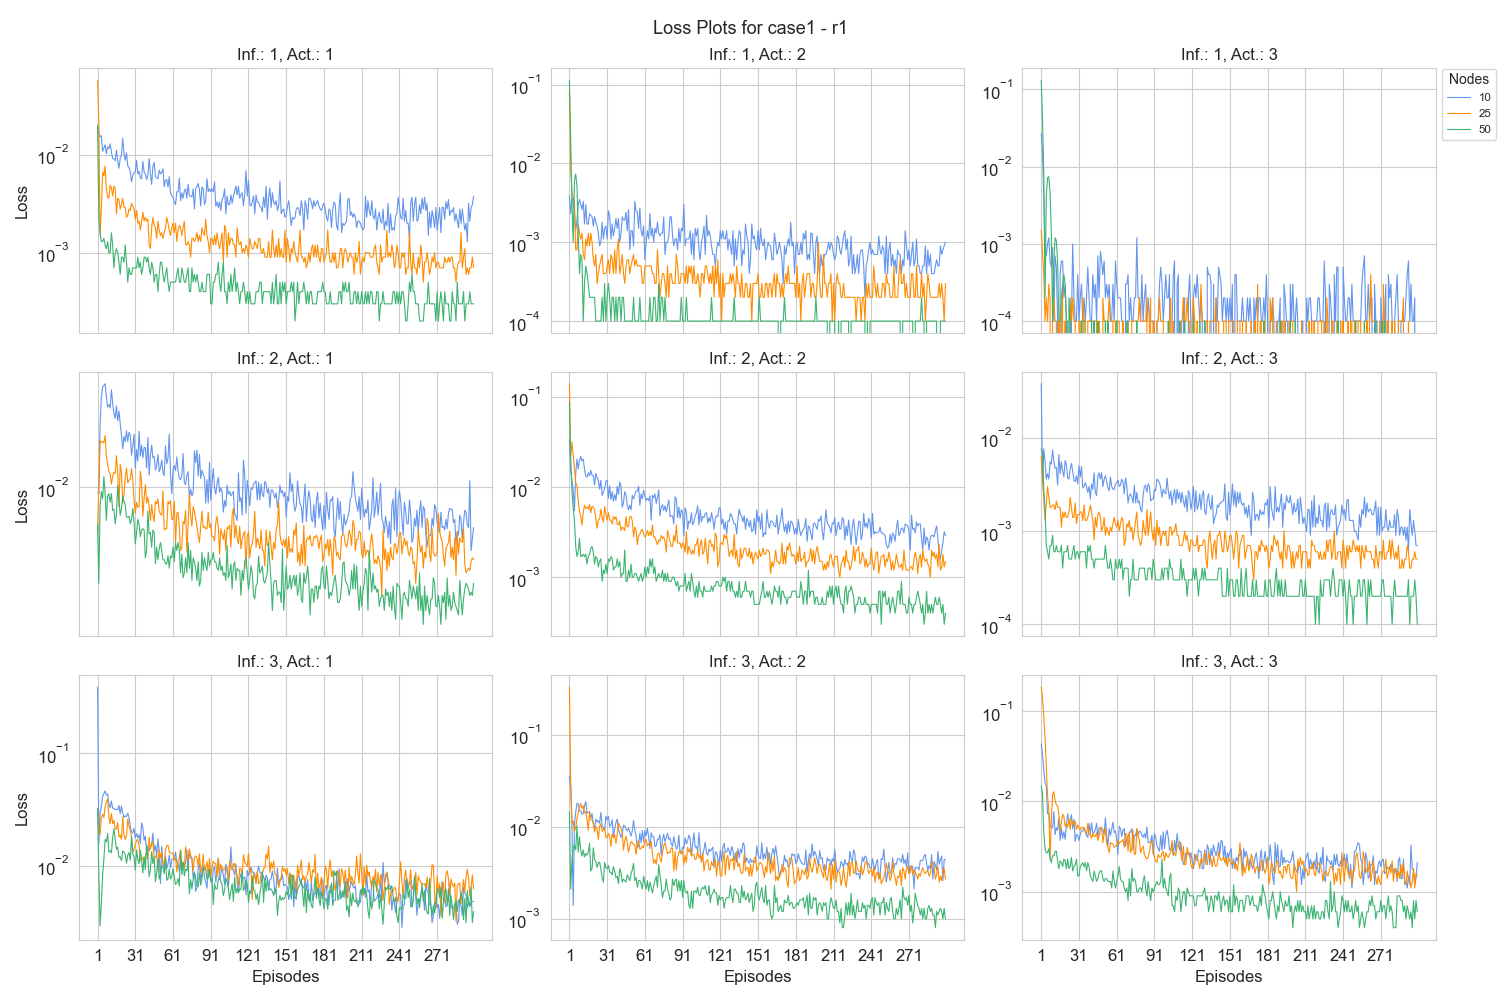}
    \caption{Case-1 using R1: Training MSE loss evolution for RL policy using ResNet model across networks of 10 (blue), 25 (orange), and 50 (green) nodes, for varying initial misinformation sources (Inf.) and action budgets (Act.). Plotted on a logarithmic scale, the loss decreases over episodes, indicating improved policy performance and adaptation across network sizes.}
    \label{fig:resnet_c1r1_loss}
\end{figure}

\begin{figure}
    \centering
    \includegraphics[scale=0.34]{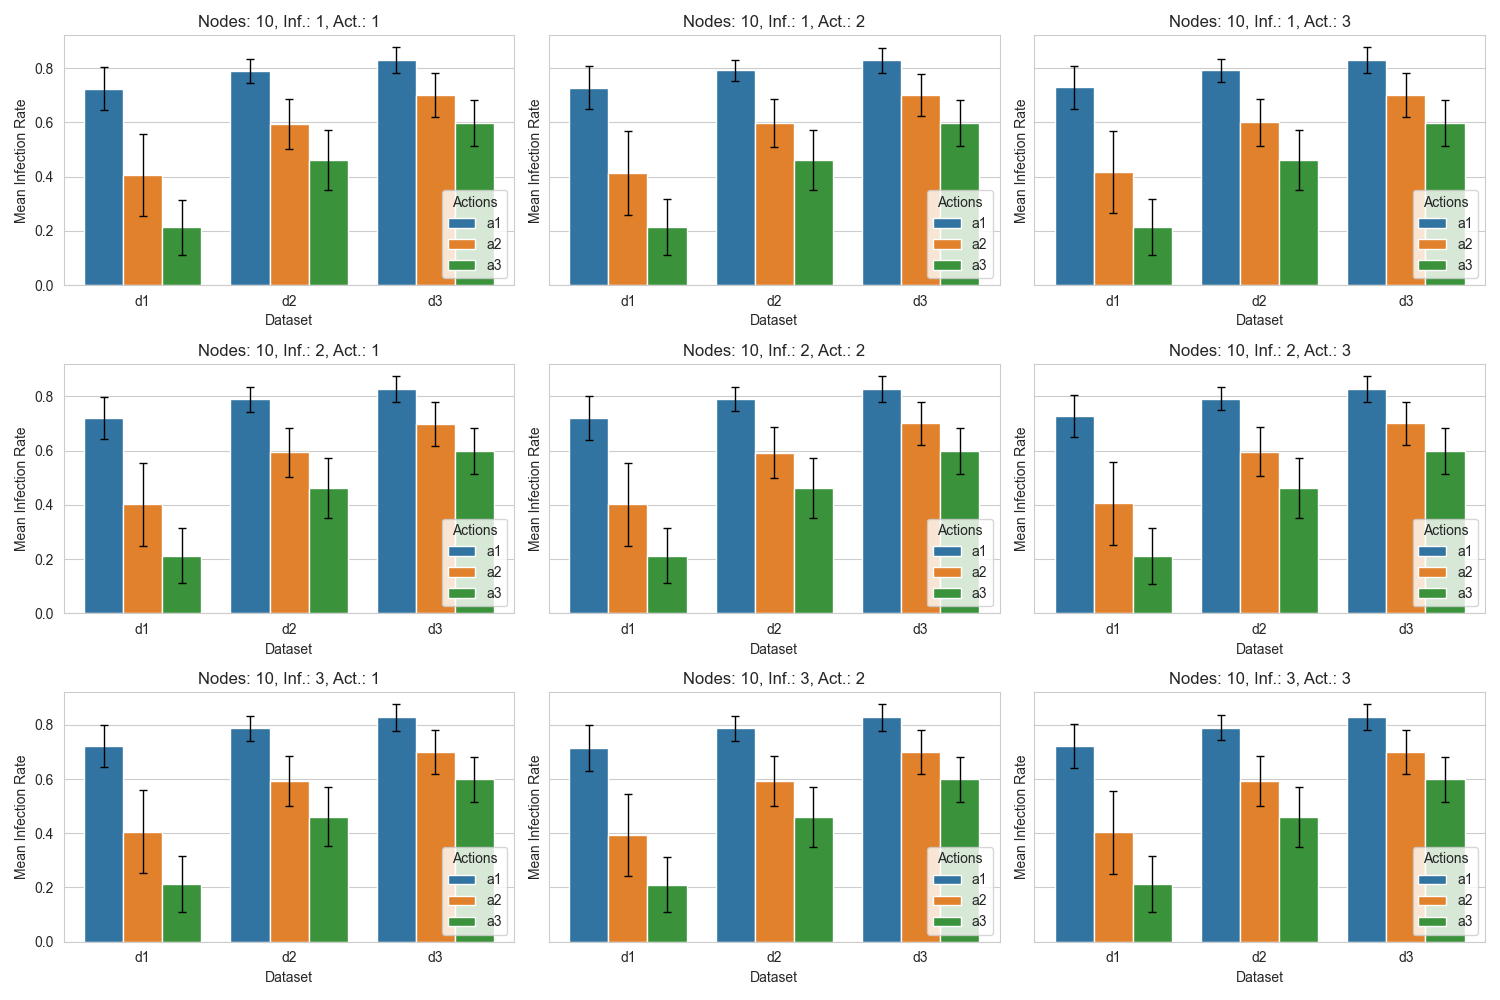}
    \caption{Case-1 using R1: Performance comparison of the RL policies trained using ResNet model for a 10-node network. The barplot displays the mean infection rate for datasets d1, d2, and d3 of Dataset v1 type, differentiated by the number of initial misinformation sources (Inf.) and action budgets (Act.: a1, a2, a3). Each subplot illustrates the performance of a policy trained with the parameters indicated in its title. Lower infection rates indicate more effective policy learning and misinformation containment.}
    \label{fig:inf_resnet_c1r1_10}
\end{figure}

\begin{figure}
    \centering
    \includegraphics[scale=0.34]{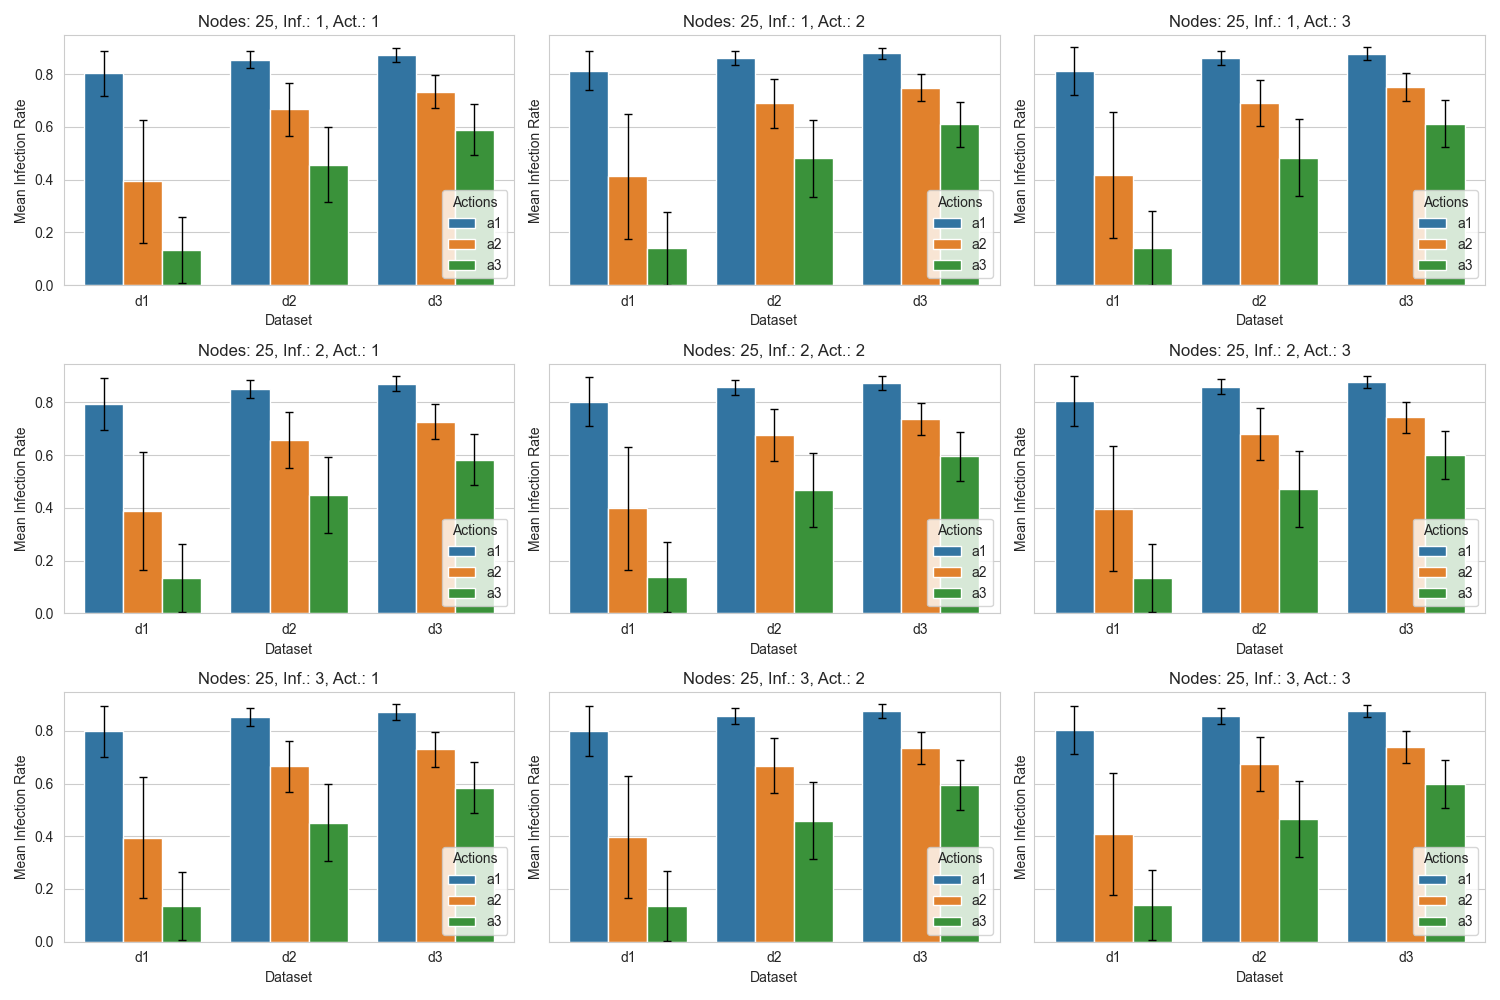}
    \caption{Case-1 using R1: Performance comparison of the RL policies trained using ResNet model for a 25-node network. The barplot displays the mean infection rate for datasets d1, d2, and d3 of Dataset v1 type, differentiated by the number of initial misinformation sources (Inf.) and action budgets (Act.: a1, a2, a3). Each subplot illustrates the performance of a policy trained with the parameters indicated in its title. Lower infection rates indicate more effective policy learning and misinformation containment.}
    \label{fig:inf_resnet_c1r1_25}
\end{figure}

\begin{figure}
    \centering
    \includegraphics[scale=0.34]{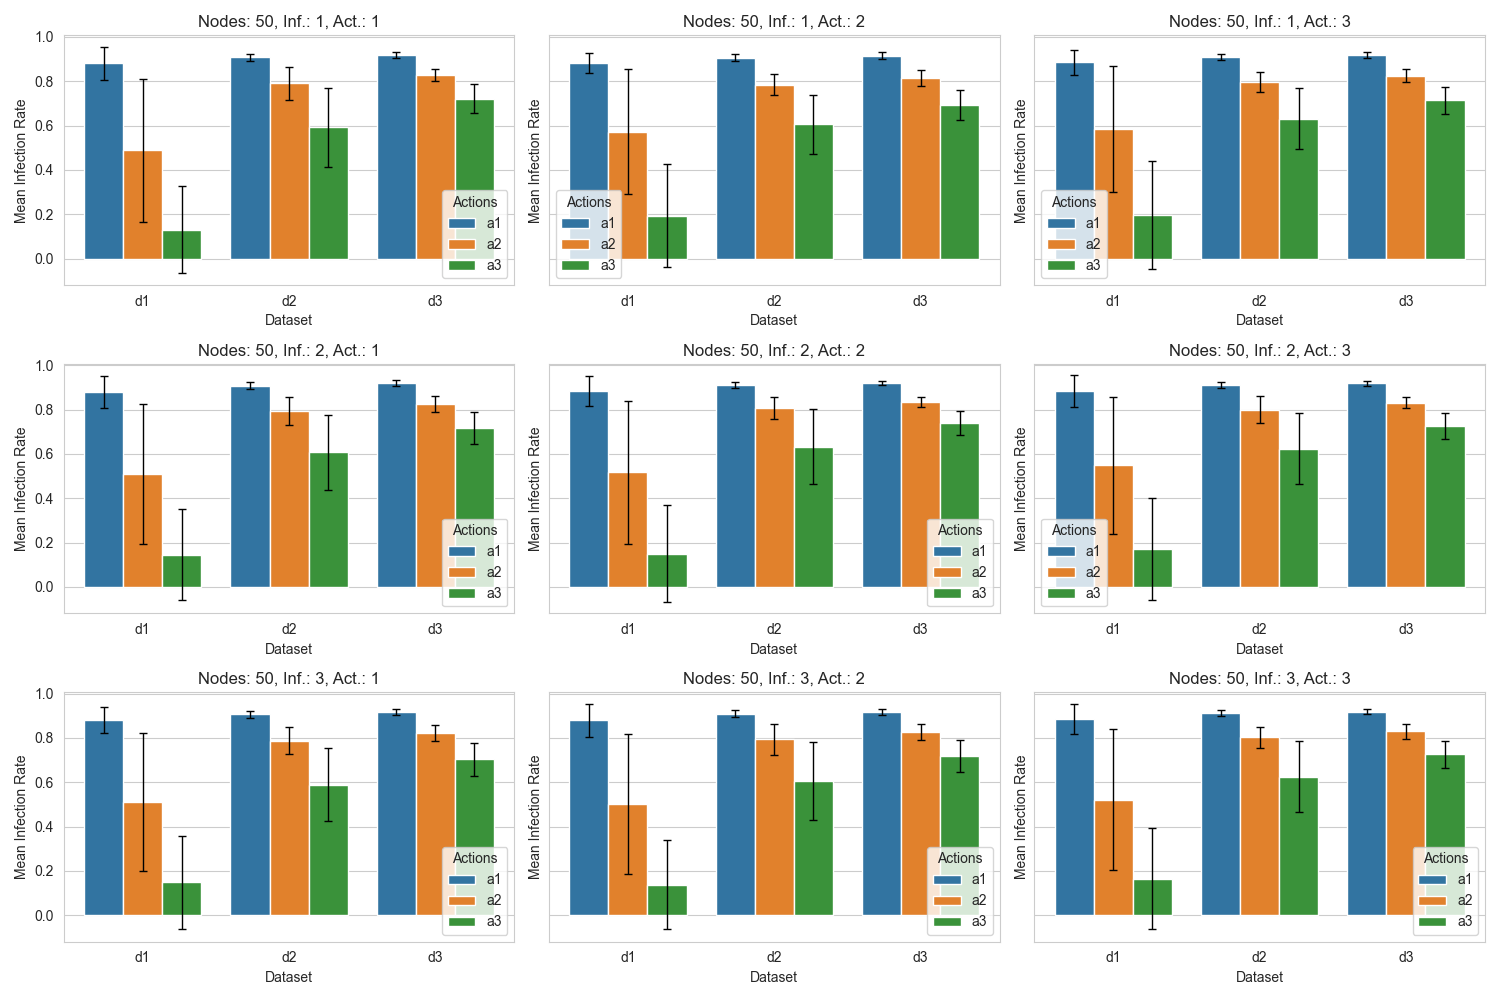}
    \caption{Case-1 using R1: Performance comparison of the RL policies trained using ResNet model for a 50-node network. The barplot displays the mean infection rate for datasets d1, d2, and d3 of Dataset v1 type, differentiated by the number of initial misinformation sources (Inf.) and action budgets (Act.: a1, a2, a3). Each subplot illustrates the performance of a policy trained with the parameters indicated in its title. Lower infection rates indicate more effective policy learning and misinformation containment.}
    \label{fig:inf_resnet_c1r1_50}
\end{figure}

%%%%%% R2 %%%%%%%%

\begin{figure}[!h]
    \centering
    \includegraphics[scale=0.34]{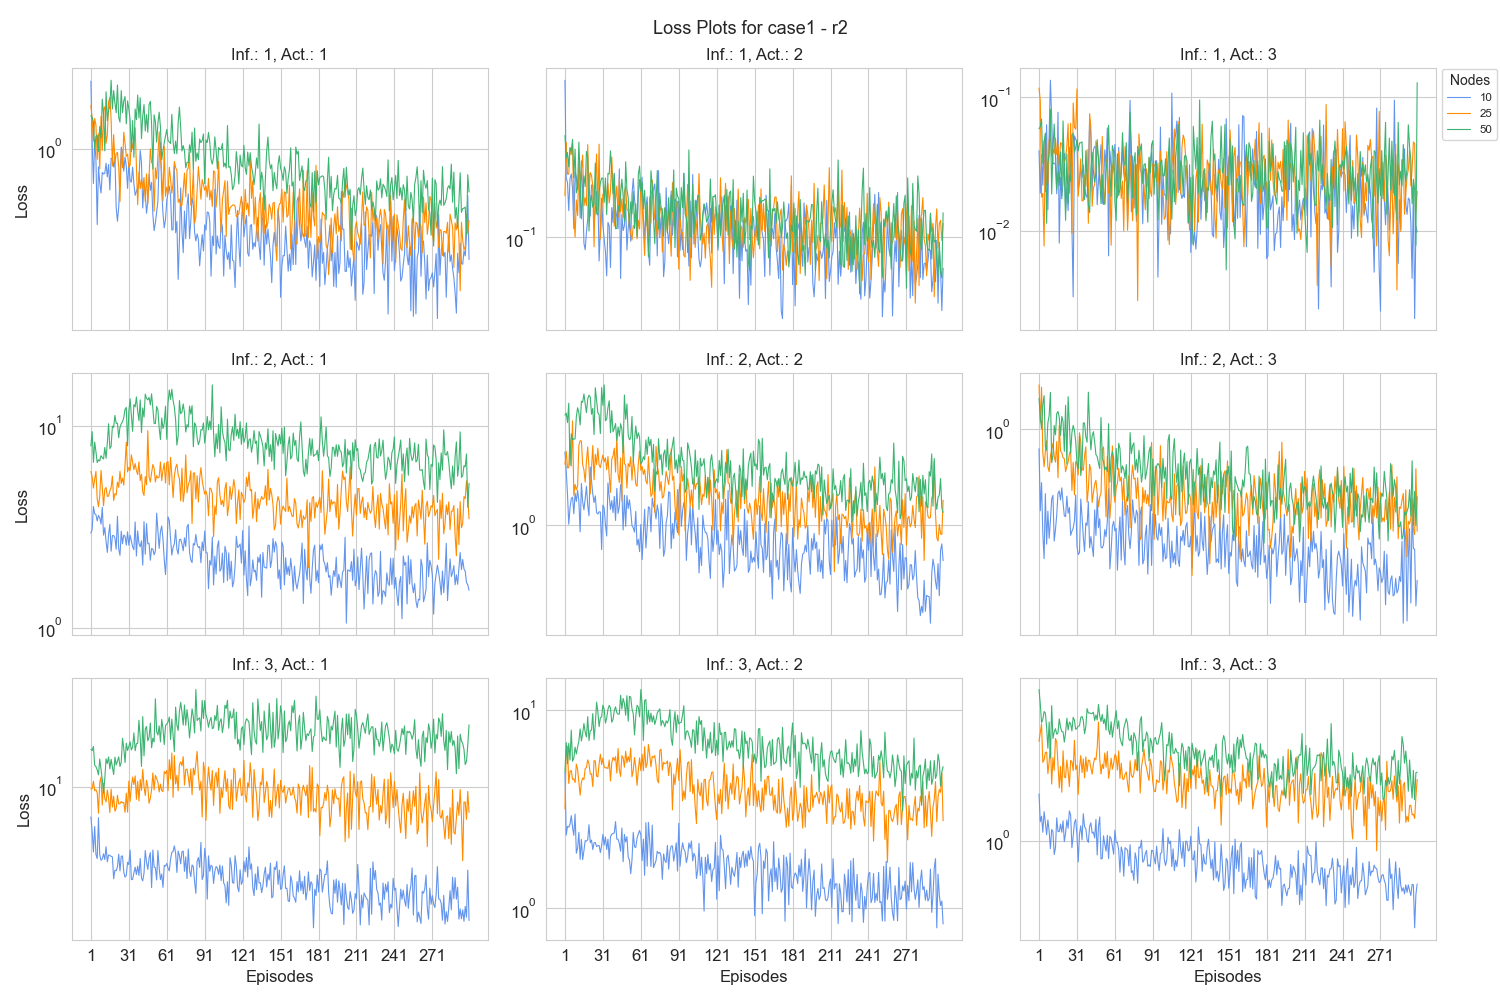}
    \caption{Case-1 using R2: Training MSE loss evolution for RL policy using ResNet model across networks of 10 (blue), 25 (orange), and 50 (green) nodes, for varying initial misinformation sources (Inf.) and action budgets (Act.). Plotted on a logarithmic scale, the loss decreases over episodes, indicating improved policy performance and adaptation across network sizes.}
    \label{fig:resnet_c1r2_loss}
\end{figure}

\begin{figure}
    \centering
    \includegraphics[scale=0.34]{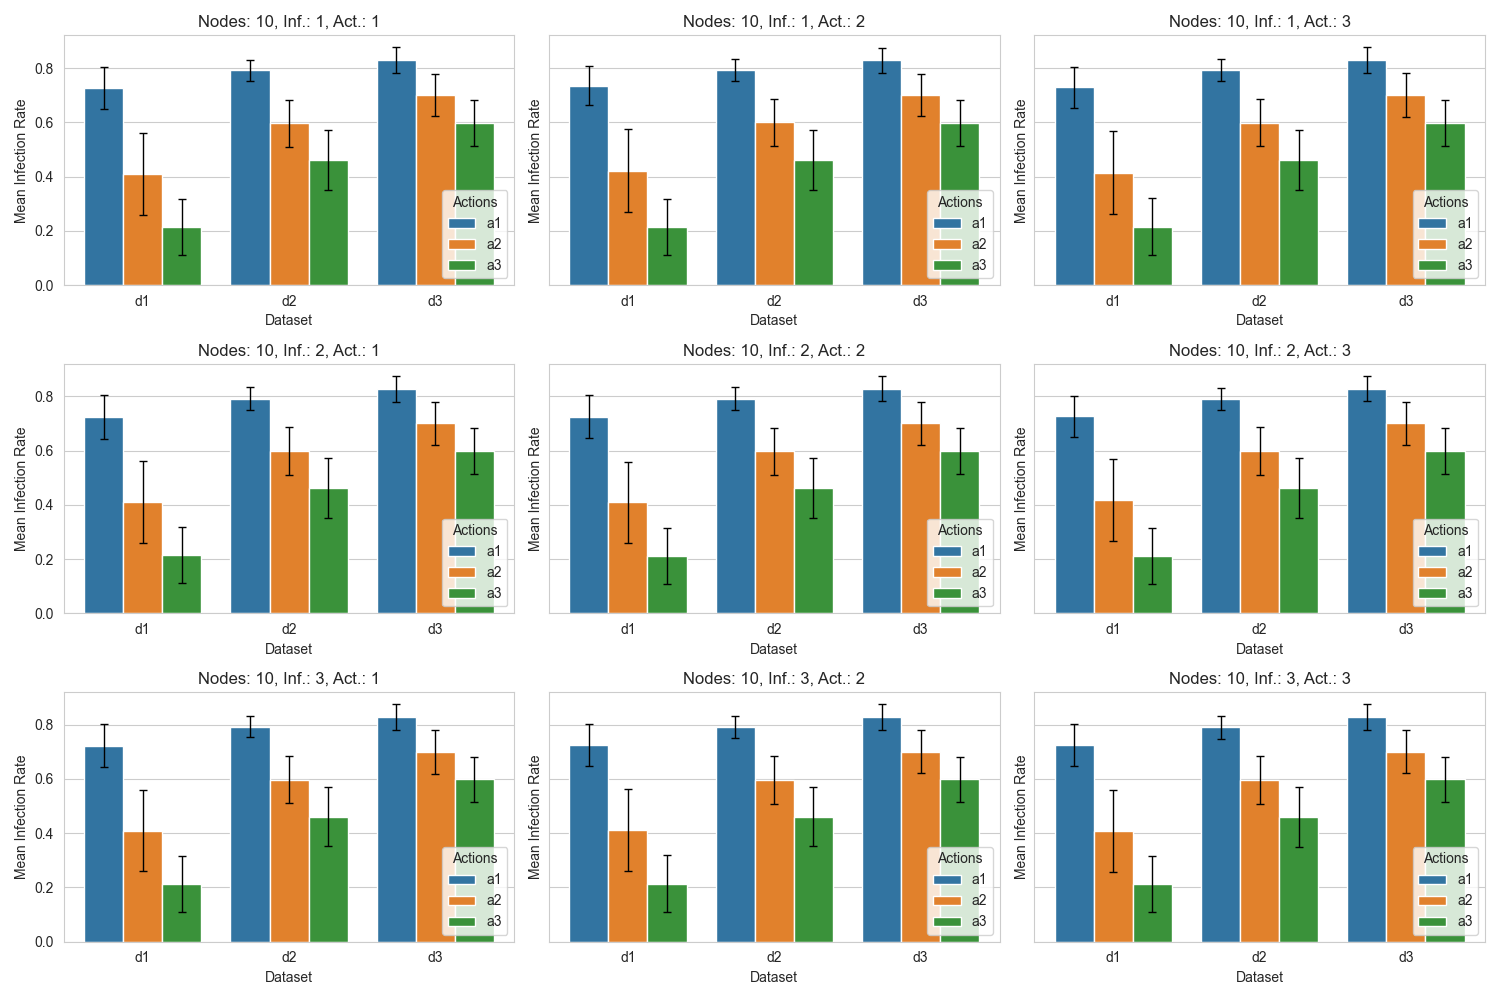}
    \caption{Case-1 using R2: Performance comparison of the RL policies trained using ResNet model for a 10-node network. The barplot displays the mean infection rate for datasets d1, d2, and d3 of Dataset v1 type, differentiated by the number of initial misinformation sources (Inf.) and action budgets (Act.: a1, a2, a3). Each subplot illustrates the performance of a policy trained with the parameters indicated in its title. Lower infection rates indicate more effective policy learning and misinformation containment.}
    \label{fig:inf_resnet_c1r2_10}
\end{figure}

\begin{figure}
    \centering
    \includegraphics[scale=0.34]{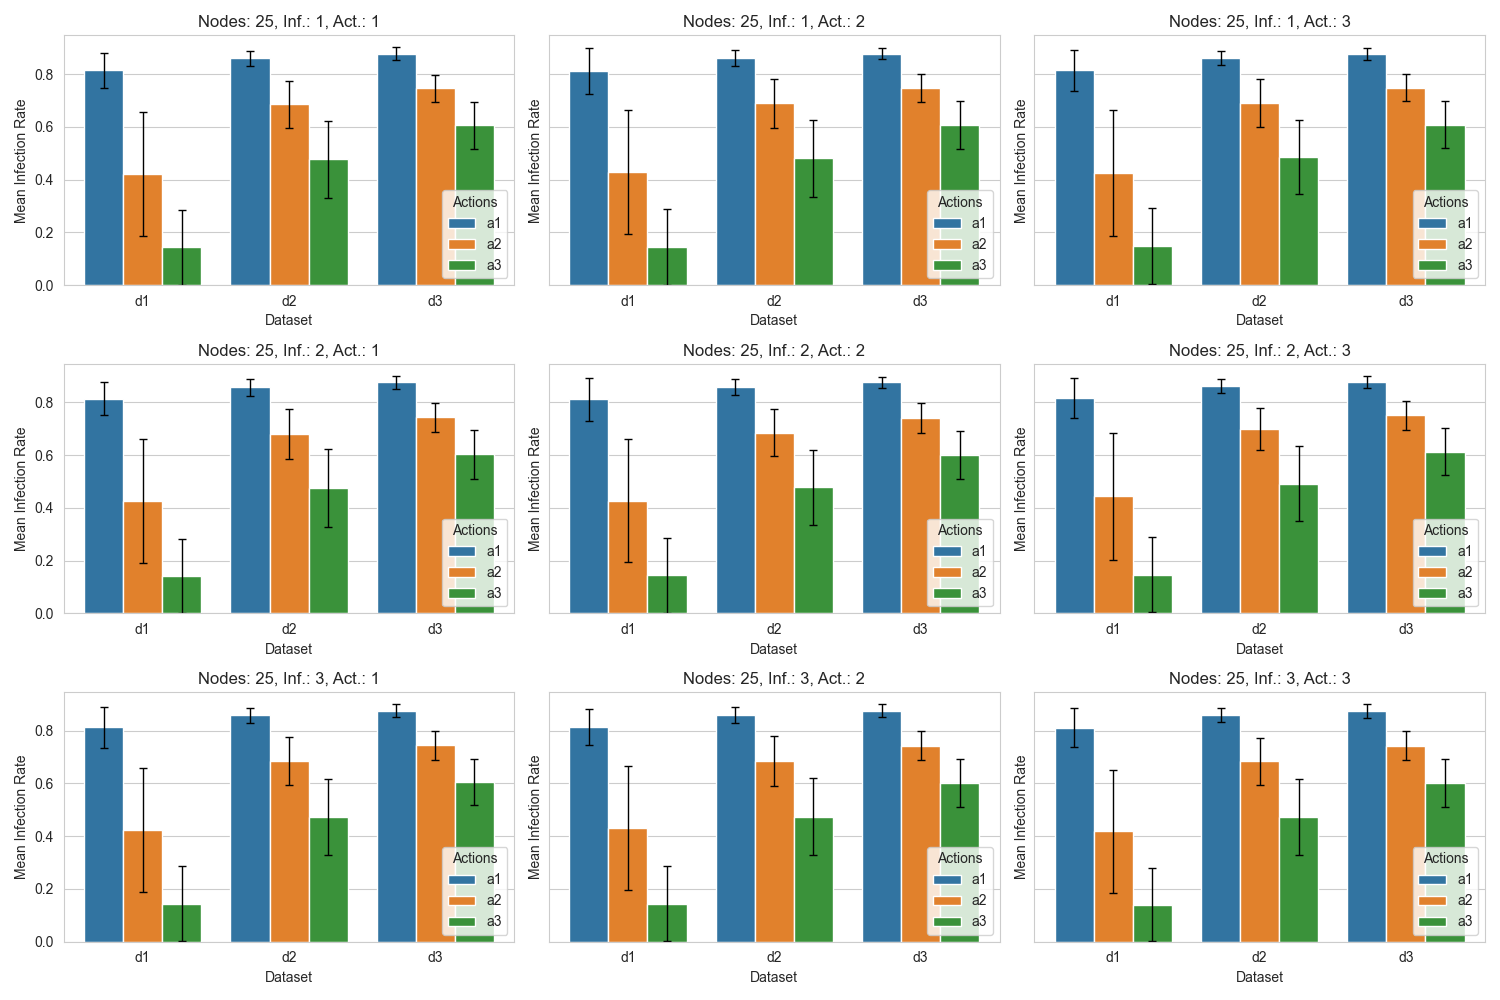}
    \caption{Case-1 using R2: Performance comparison of the RL policies trained using ResNet model for a 25-node network. The barplot displays the mean infection rate for datasets d1, d2, and d3 of Dataset v1 type, differentiated by the number of initial misinformation sources (Inf.) and action budgets (Act.: a1, a2, a3). Each subplot illustrates the performance of a policy trained with the parameters indicated in its title. Lower infection rates indicate more effective policy learning and misinformation containment.}
    \label{fig:inf_resnet_c1r2_25}
\end{figure}

\begin{figure}
    \centering
    \includegraphics[scale=0.34]{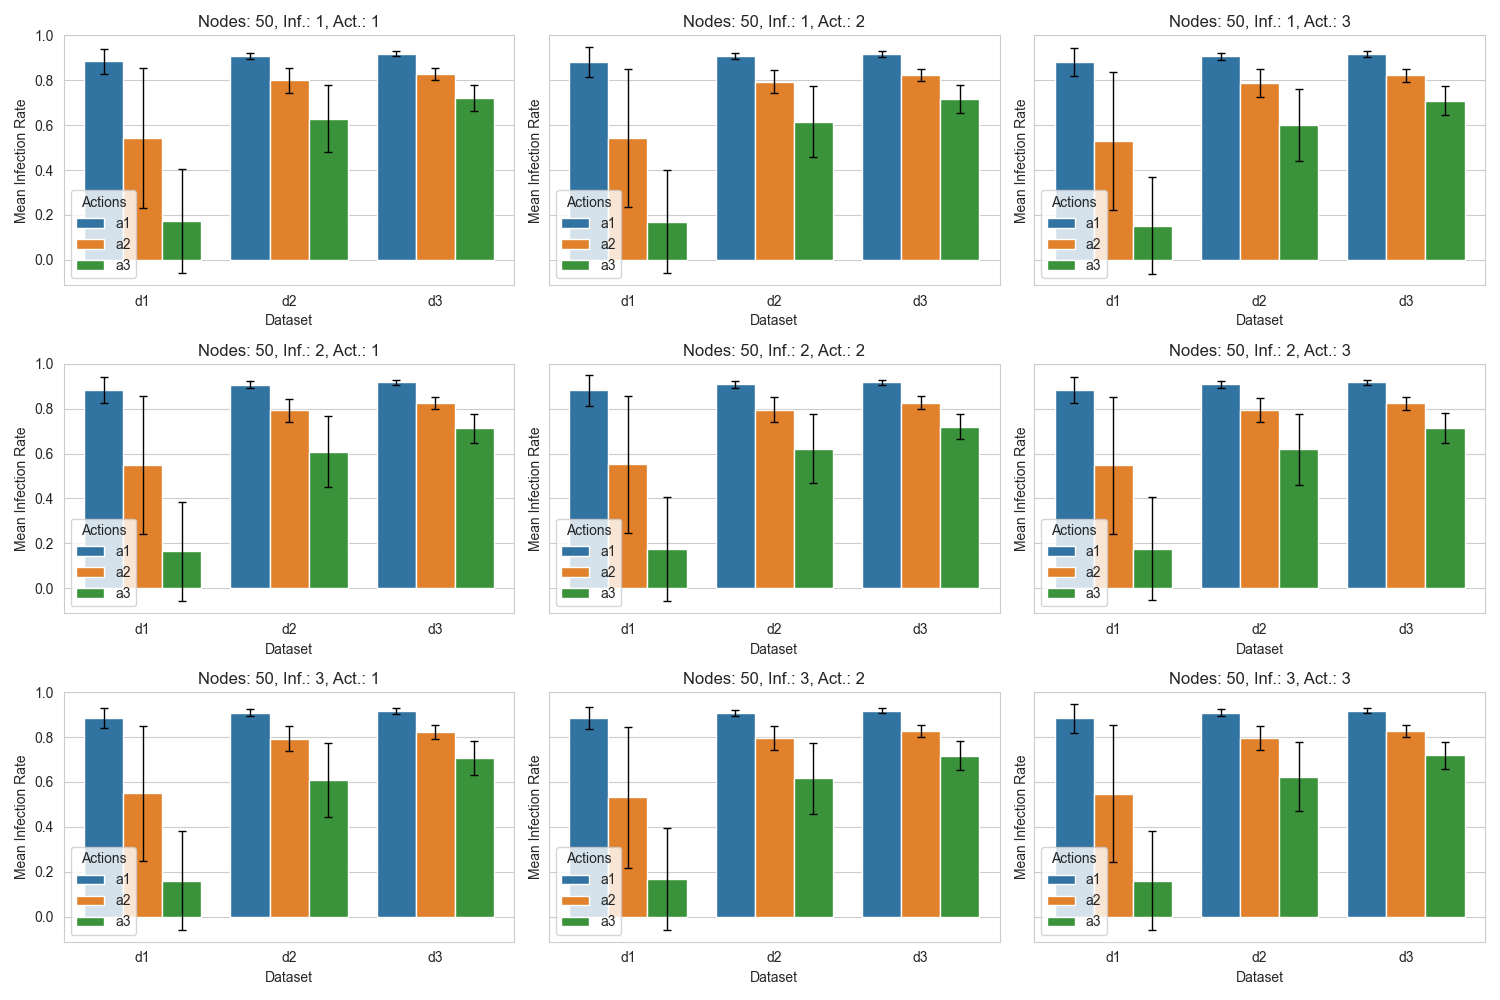}
    \caption{Case-1 using R2: Performance comparison of the RL policies trained using ResNet model for a 50-node network. The barplot displays the mean infection rate for datasets d1, d2, and d3 of Dataset v1 type, differentiated by the number of initial misinformation sources (Inf.) and action budgets (Act.: a1, a2, a3). Each subplot illustrates the performance of a policy trained with the parameters indicated in its title. Lower infection rates indicate more effective policy learning and misinformation containment.}
    \label{fig:inf_resnet_c1r2_50}
\end{figure}

%%%%%% R3 %%%%%%%%

\begin{figure}[!h]
    \centering
    \includegraphics[scale=0.34]{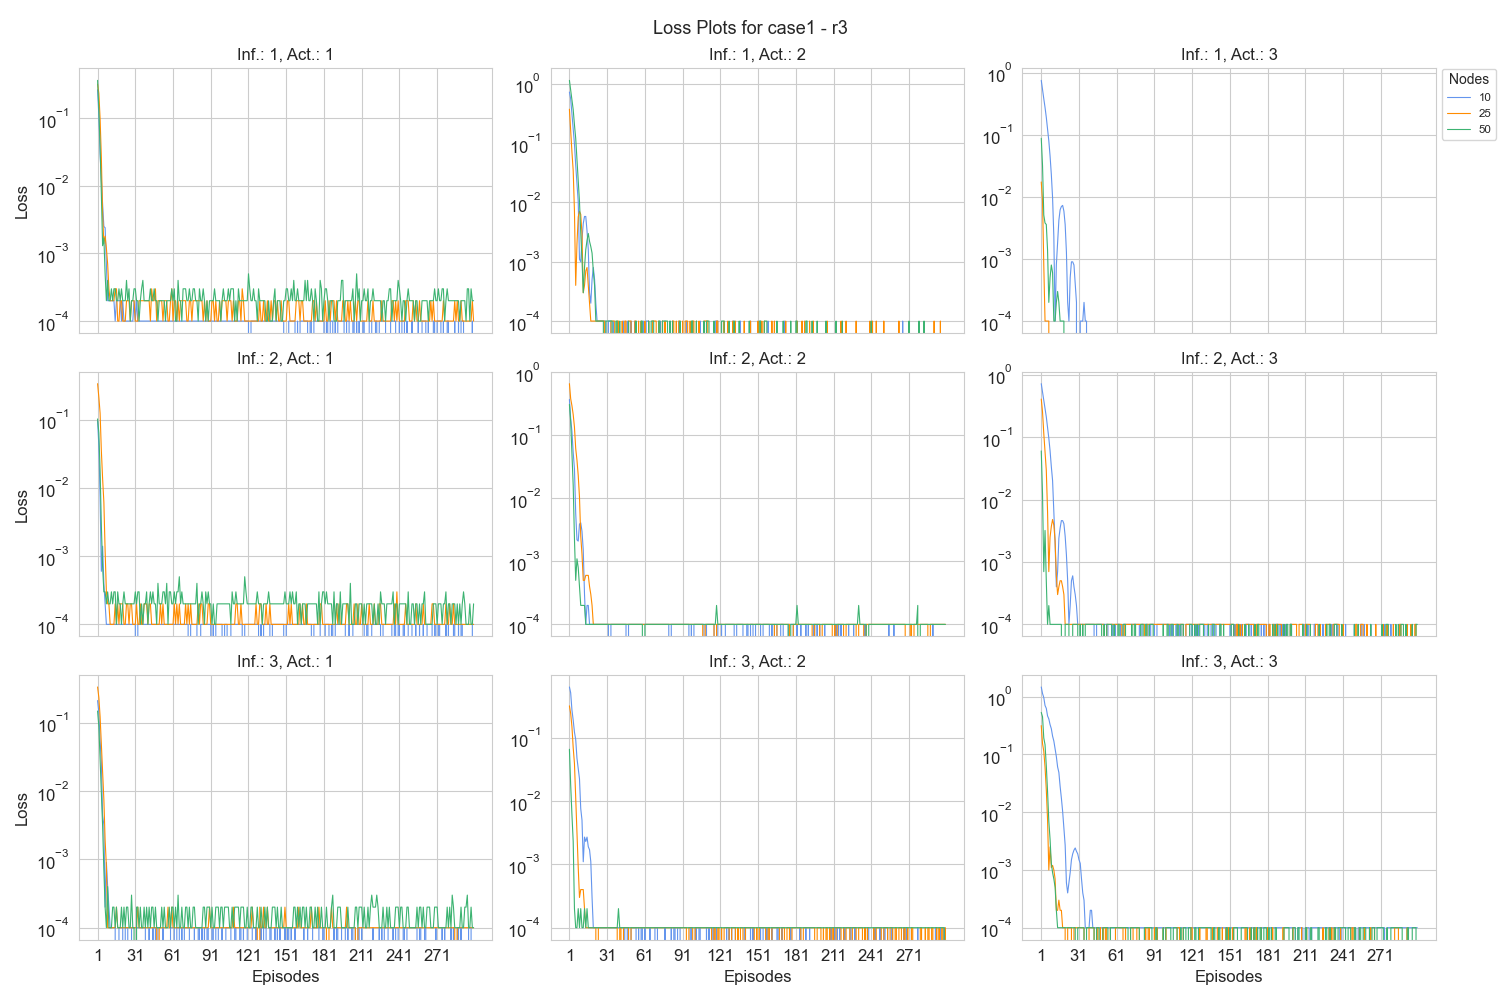}
    \caption{Case-1 using R3: Training MSE loss evolution for RL policy using ResNet model across networks of 10 (blue), 25 (orange), and 50 (green) nodes, for varying initial misinformation sources (Inf.) and action budgets (Act.). Plotted on a logarithmic scale, the loss decreases over episodes, indicating improved policy performance and adaptation across network sizes.}
    \label{fig:resnet_c1r3_loss}
\end{figure}

\begin{figure}
    \centering
    \includegraphics[scale=0.34]{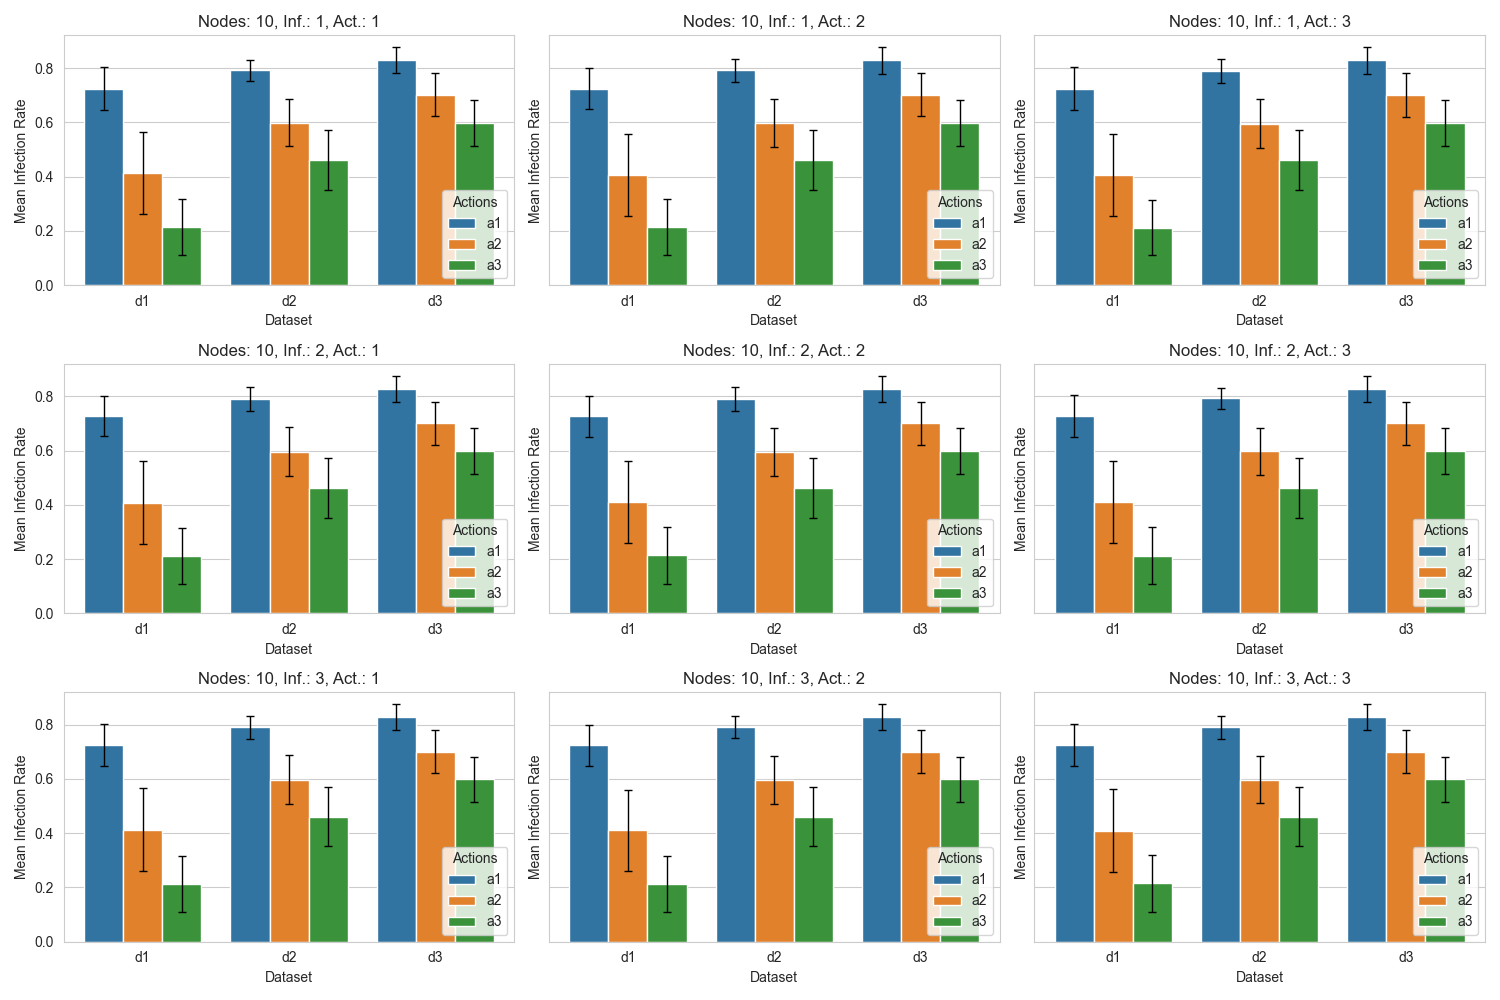}
    \caption{Case-1 using R3: Performance comparison of the RL policies trained using ResNet model for a 10-node network. The barplot displays the mean infection rate for datasets d1, d2, and d3 of Dataset v1 type, differentiated by the number of initial misinformation sources (Inf.) and action budgets (Act.: a1, a2, a3). Each subplot illustrates the performance of a policy trained with the parameters indicated in its title. Lower infection rates indicate more effective policy learning and misinformation containment.}
    \label{fig:inf_resnet_c1r3_10}
\end{figure}

\begin{figure}
    \centering
    \includegraphics[scale=0.34]{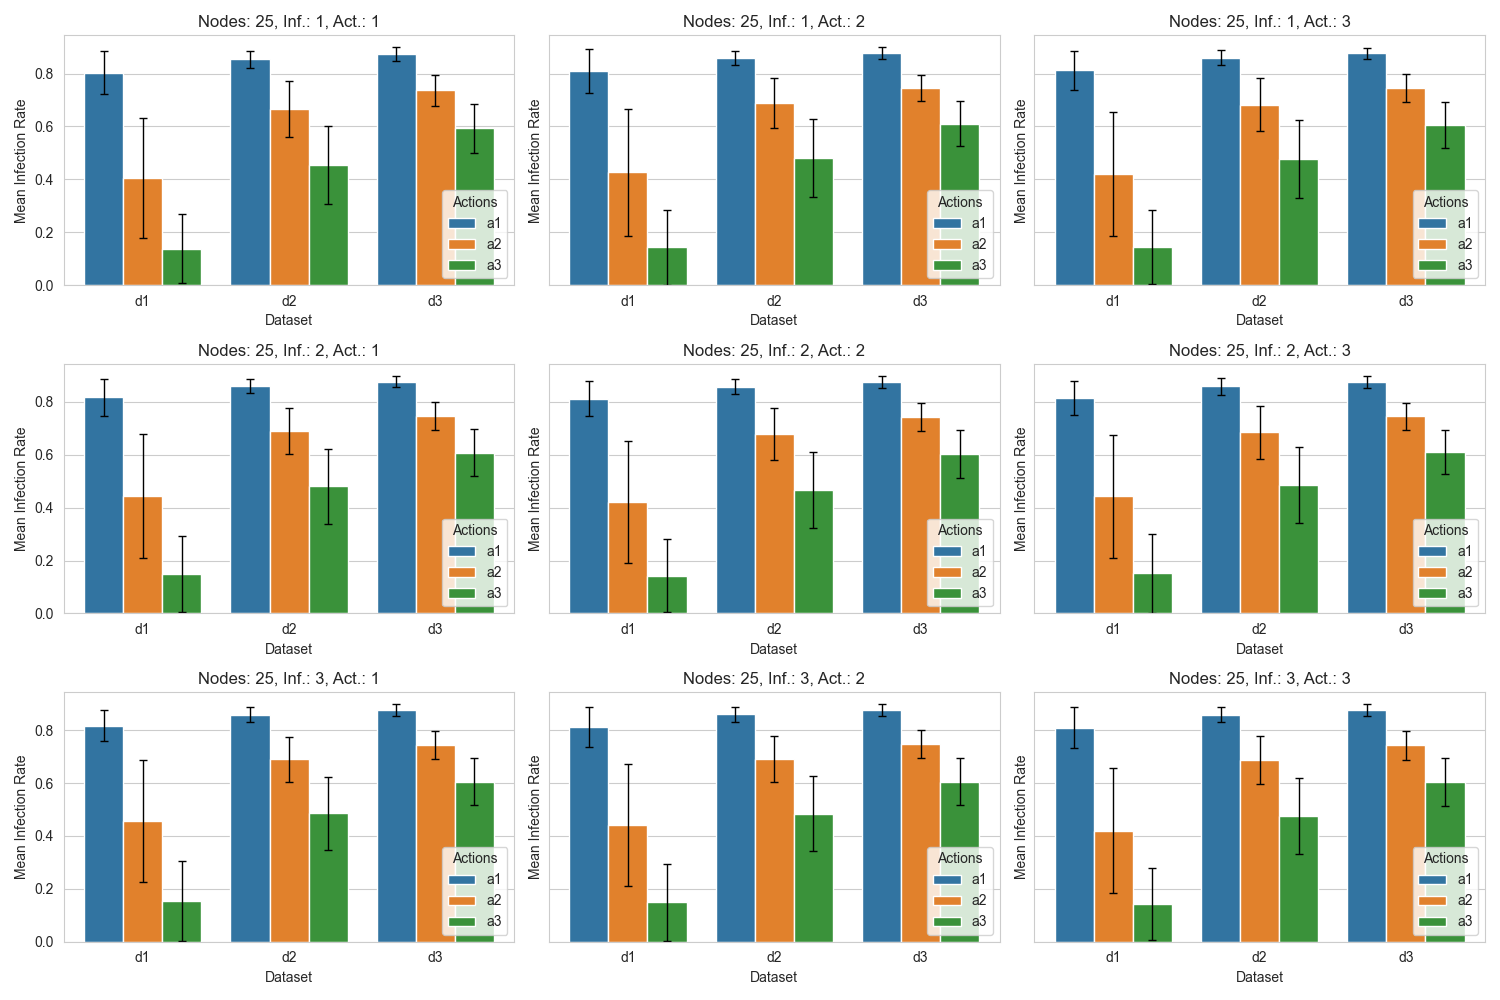}
    \caption{Case-1 using R3: Performance comparison of the RL policies trained using ResNet model for a 25-node network. The barplot displays the mean infection rate for datasets d1, d2, and d3 of Dataset v1 type, differentiated by the number of initial misinformation sources (Inf.) and action budgets (Act.: a1, a2, a3). Each subplot illustrates the performance of a policy trained with the parameters indicated in its title. Lower infection rates indicate more effective policy learning and misinformation containment.}
    \label{fig:inf_resnet_c1r3_25}
\end{figure}

\begin{figure}
    \centering
    \includegraphics[scale=0.34]{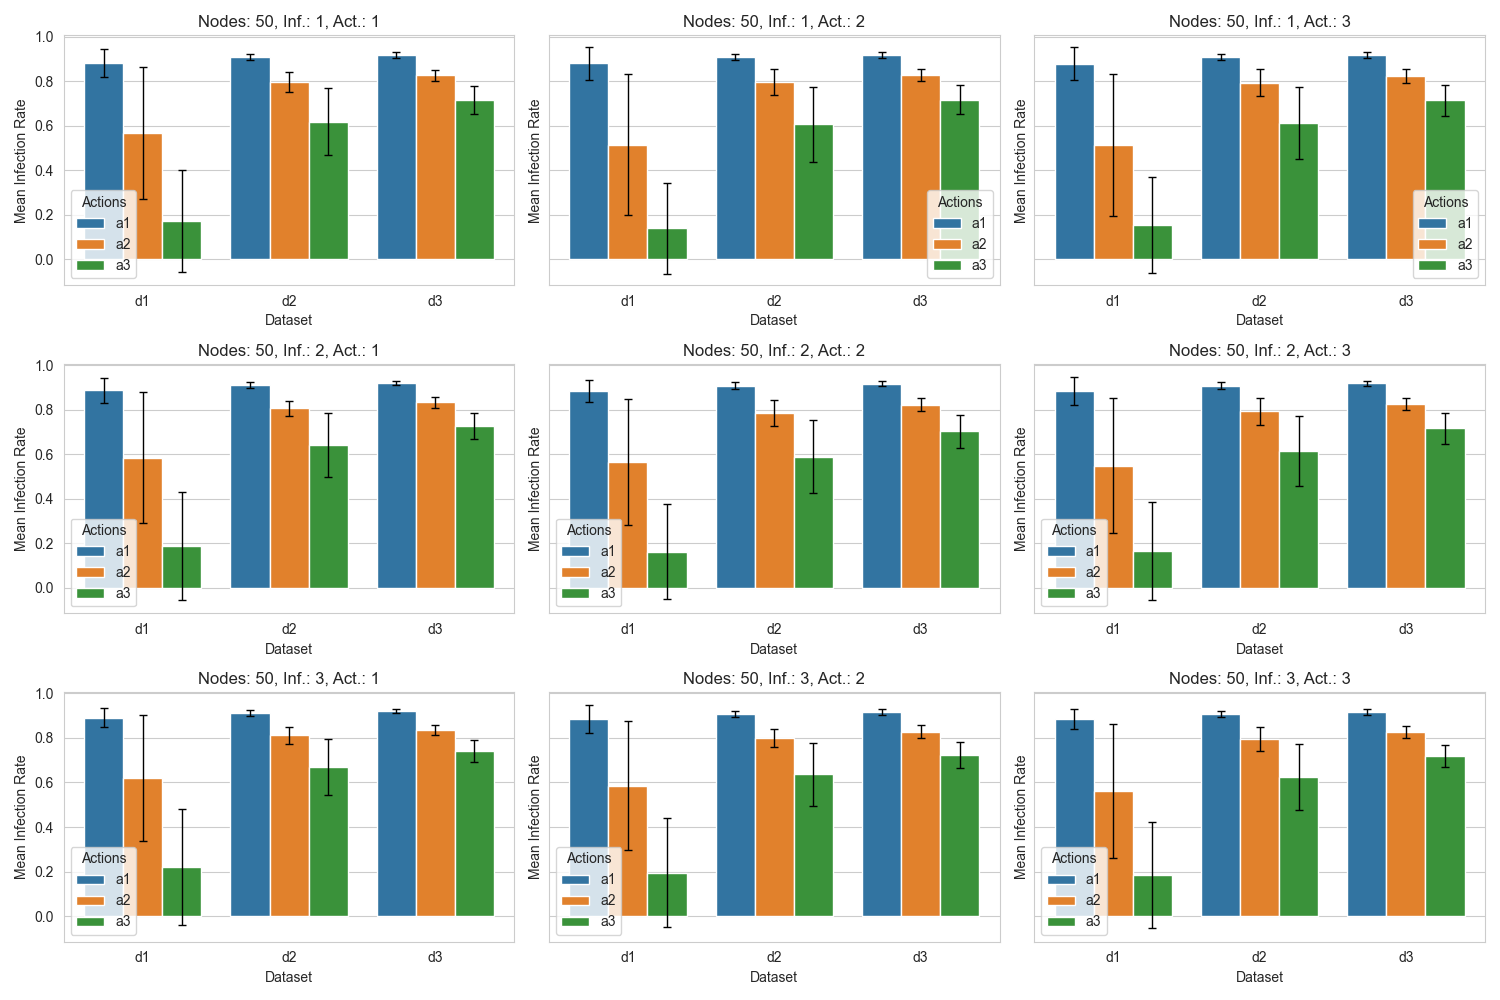}
    \caption{Case-1 using R3: Performance comparison of the RL policies trained using ResNet model for a 50-node network. The barplot displays the mean infection rate for datasets d1, d2, and d3 of Dataset v1 type, differentiated by the number of initial misinformation sources (Inf.) and action budgets (Act.: a1, a2, a3). Each subplot illustrates the performance of a policy trained with the parameters indicated in its title. Lower infection rates indicate more effective policy learning and misinformation containment.}
    \label{fig:inf_resnet_c1r3_50}
\end{figure}

%%%%%% R4 %%%%%%%%

\begin{figure}[!h]
    \centering
    \includegraphics[scale=0.34]{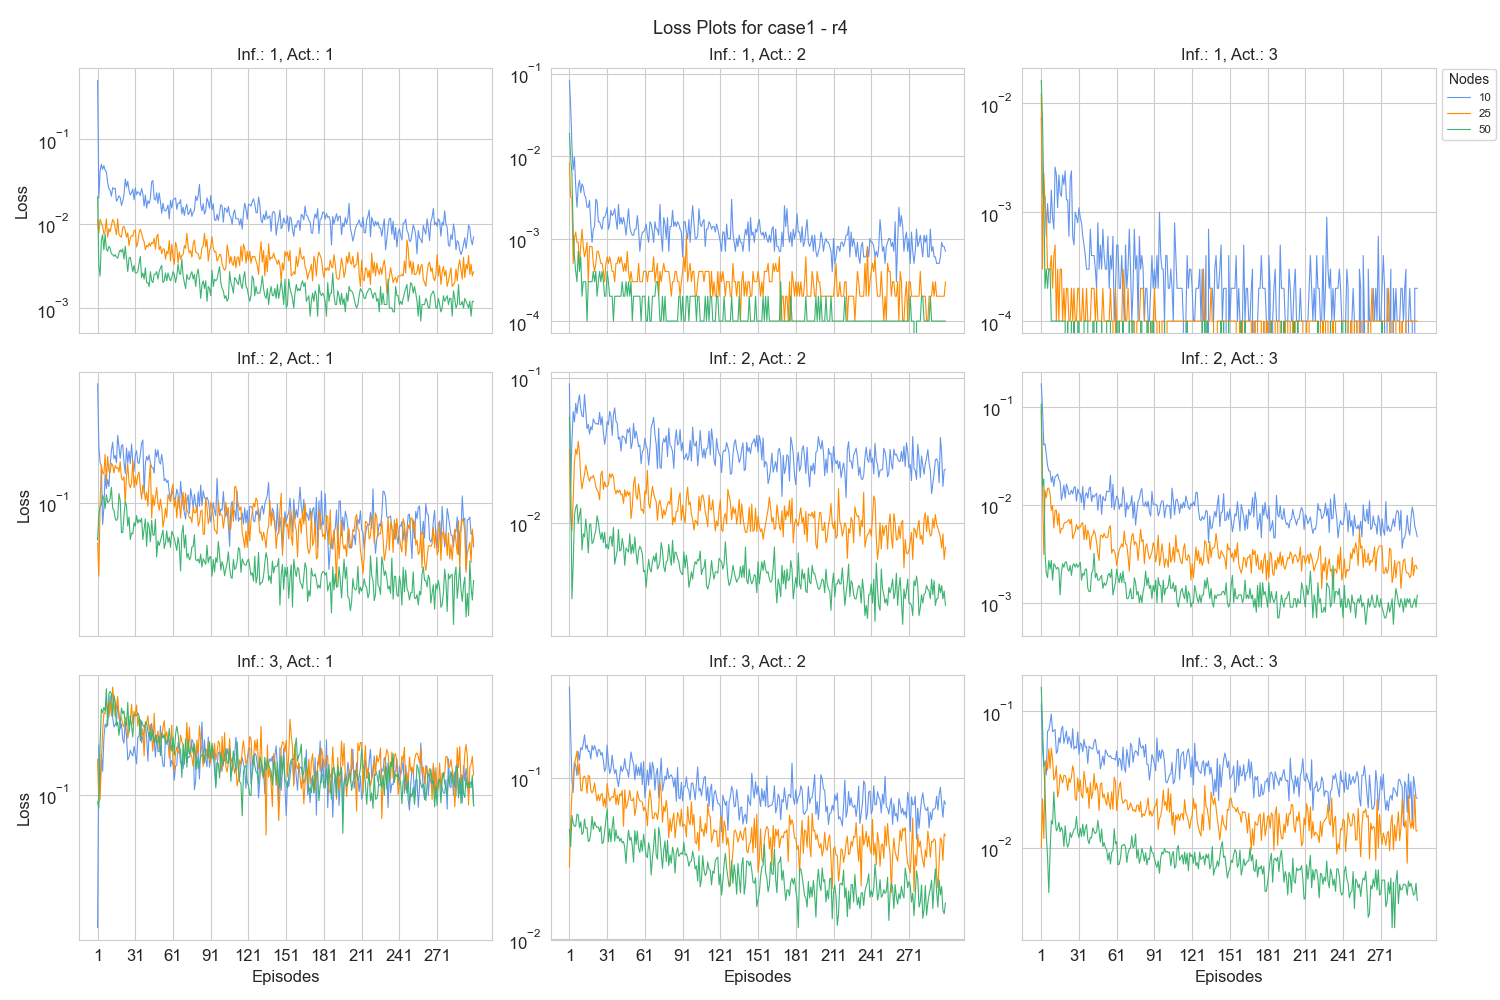}
    \caption{Case-1 using R4: Training MSE loss evolution for RL policy using ResNet model across networks of 10 (blue), 25 (orange), and 50 (green) nodes, for varying initial misinformation sources (Inf.) and action budgets (Act.). Plotted on a logarithmic scale, the loss decreases over episodes, indicating improved policy performance and adaptation across network sizes.}
    \label{fig:resnet_c1r4_loss}
\end{figure}

\begin{figure}
    \centering
    \includegraphics[scale=0.34]{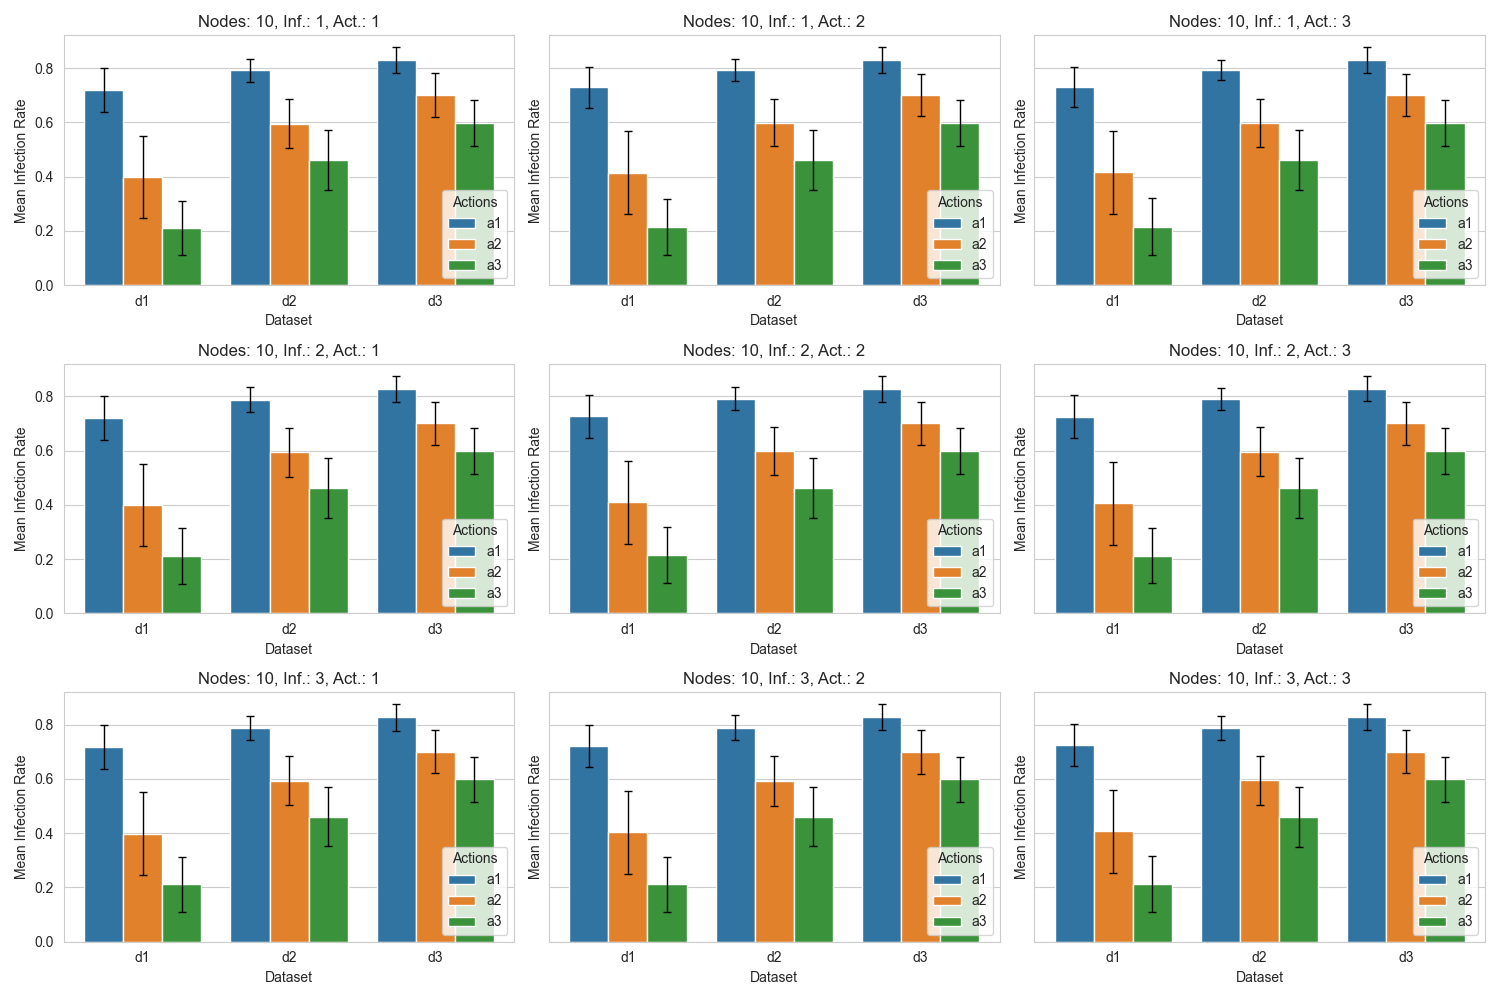}
    \caption{Case-1 using R4: Performance comparison of the RL policies trained using ResNet model for a 10-node network. The barplot displays the mean infection rate for datasets d1, d2, and d3 of Dataset v1 type, differentiated by the number of initial misinformation sources (Inf.) and action budgets (Act.: a1, a2, a3). Each subplot illustrates the performance of a policy trained with the parameters indicated in its title. Lower infection rates indicate more effective policy learning and misinformation containment.}
    \label{fig:inf_resnet_c1r4_10}
\end{figure}

\begin{figure}
    \centering
    \includegraphics[scale=0.34]{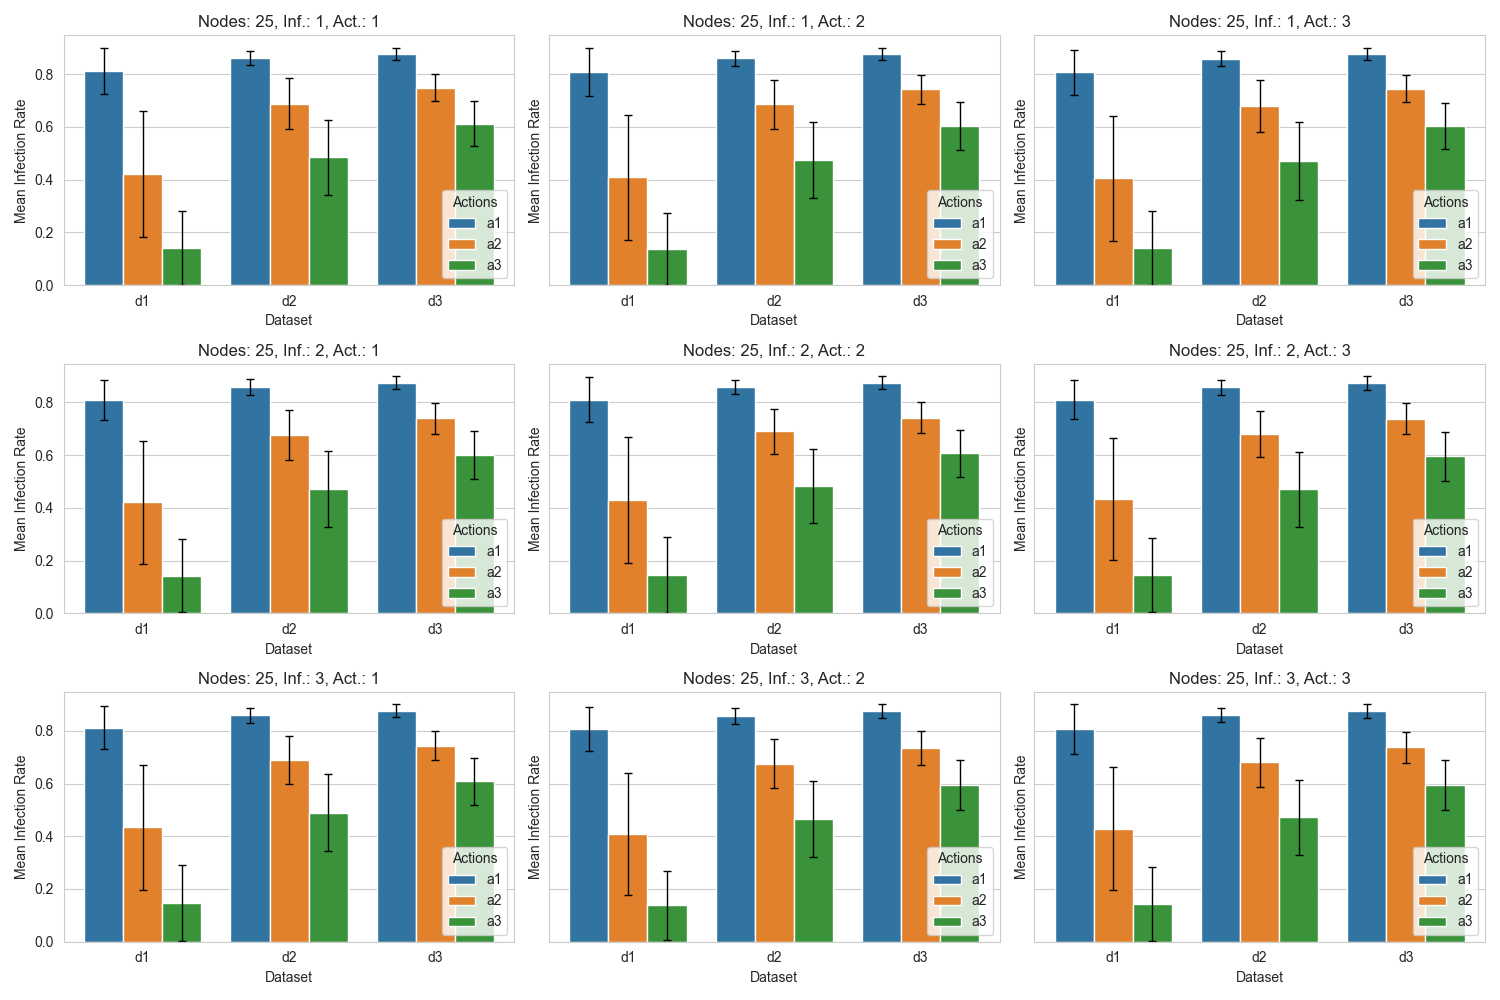}
    \caption{Case-1 using R4: Performance comparison of the RL policies trained using ResNet model for a 25-node network. The barplot displays the mean infection rate for datasets d1, d2, and d3 of Dataset v1 type, differentiated by the number of initial misinformation sources (Inf.) and action budgets (Act.: a1, a2, a3). Each subplot illustrates the performance of a policy trained with the parameters indicated in its title. Lower infection rates indicate more effective policy learning and misinformation containment.}
    \label{fig:inf_resnet_c1r4_25}
\end{figure}

\begin{figure}
    \centering
    \includegraphics[scale=0.34]{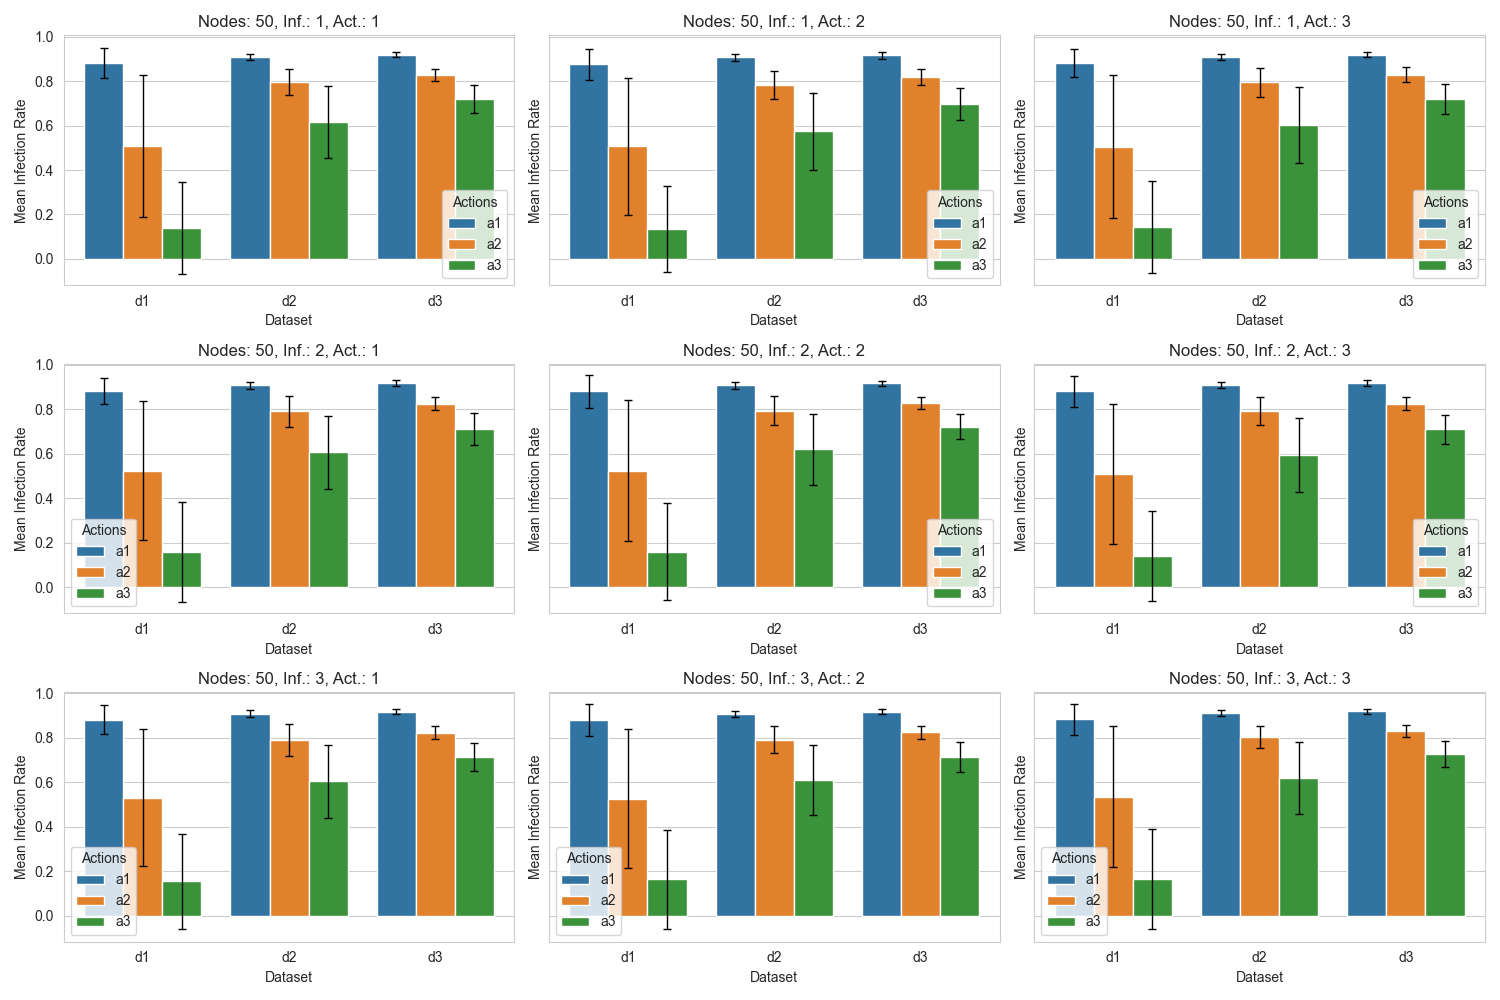}
    \caption{Case-1 using R4: Performance comparison of the RL policies trained using ResNet model for a 50-node network. The barplot displays the mean infection rate for datasets d1, d2, and d3 of Dataset v1 type, differentiated by the number of initial misinformation sources (Inf.) and action budgets (Act.: a1, a2, a3). Each subplot illustrates the performance of a policy trained with the parameters indicated in its title. Lower infection rates indicate more effective policy learning and misinformation containment.}
    \label{fig:inf_resnet_c1r4_50}
\end{figure}

% --------------------Inference------------------------

%###########################

%###### Case 2 ResNet Figures #######

%%%%%% R0 %%%%%%%%
\begin{figure}[!h]
    \centering
    \includegraphics[scale=0.34]{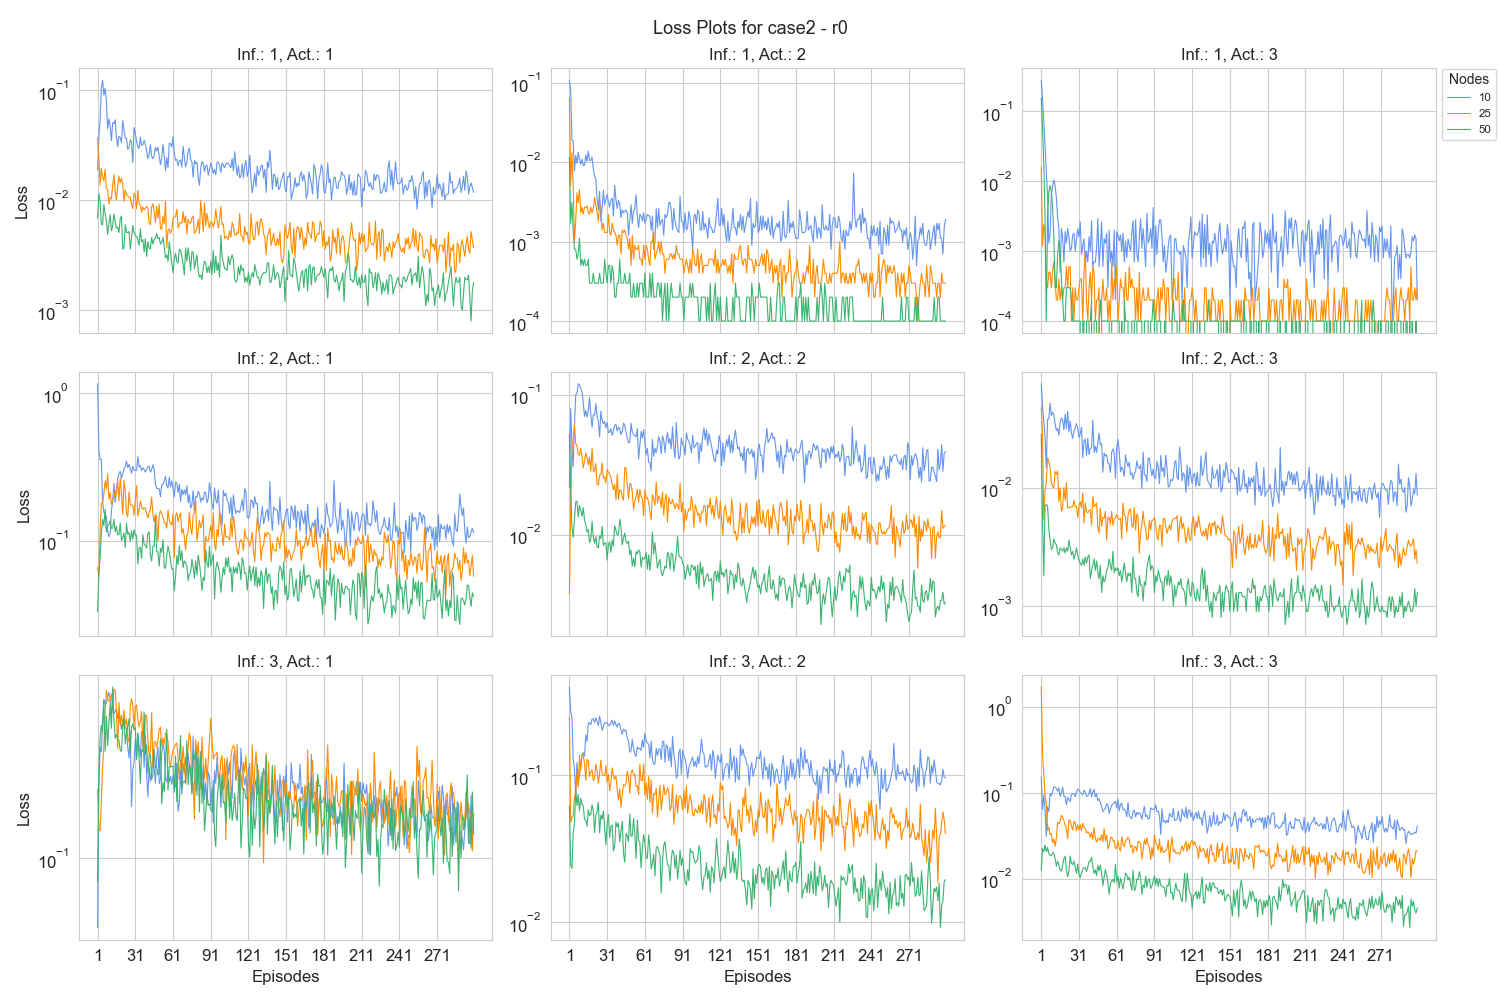}
    \caption{Case-2 using R0: Training MSE loss evolution for RL policy using ResNet model across networks of 10 (blue), 25 (orange), and 50 (green) nodes, for varying initial misinformation sources (Inf.) and action budgets (Act.). Plotted on a logarithmic scale, the loss decreases over episodes, indicating improved policy performance and adaptation across network sizes.}
    \label{fig:resnet_c2r0_loss}
\end{figure}

\begin{figure}
    \centering
    \includegraphics[scale=0.34]{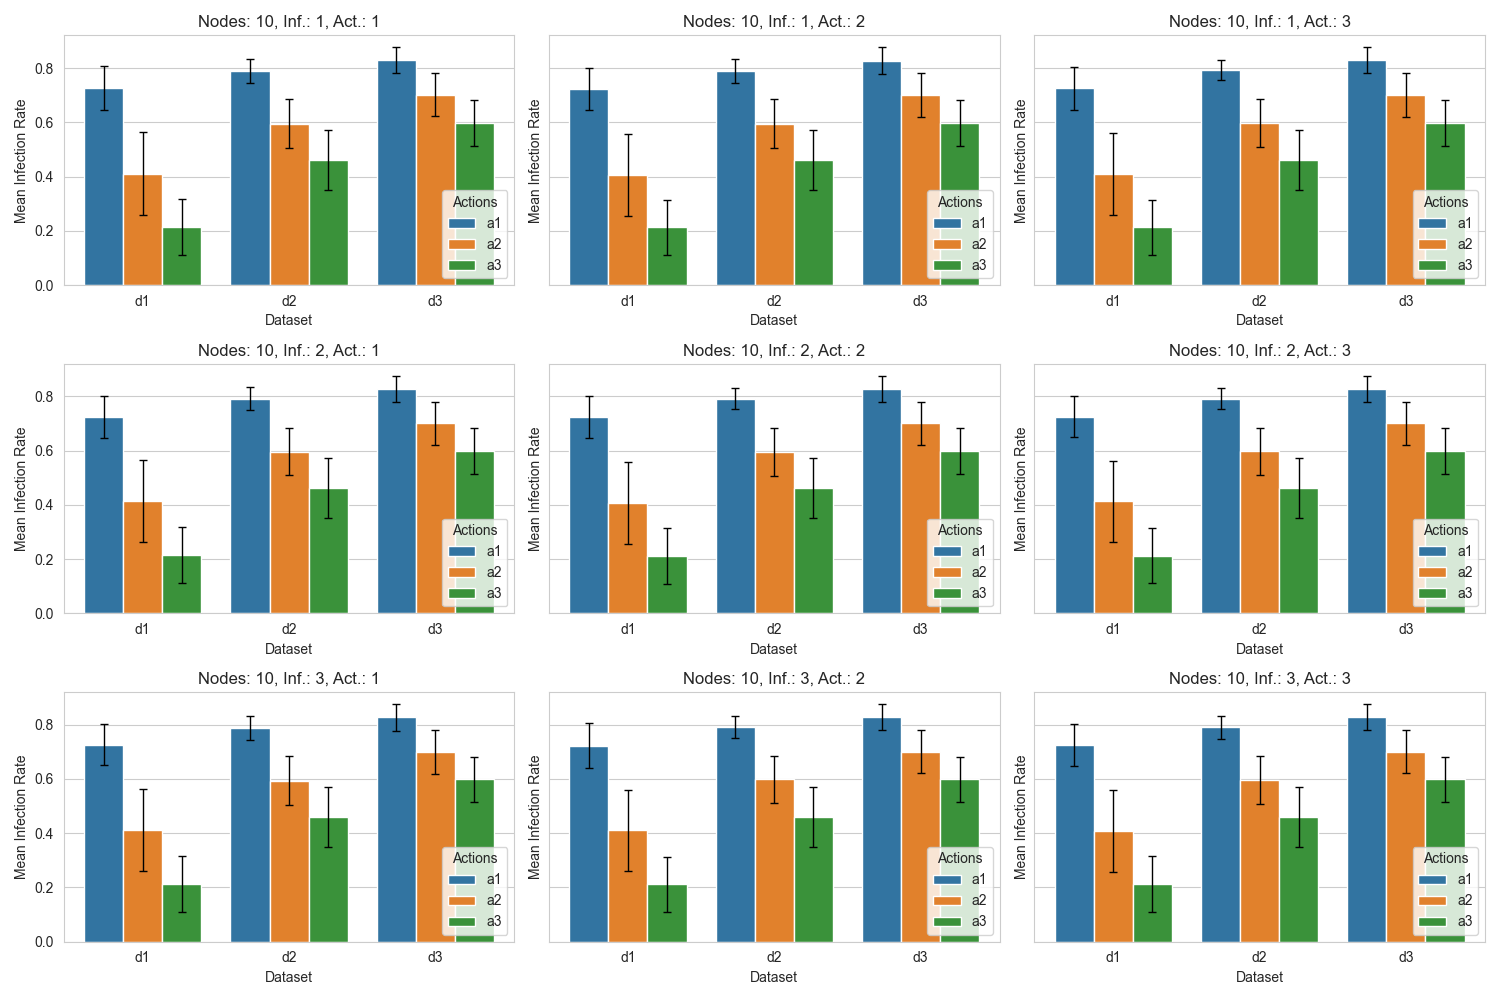}
    \caption{Case-2 using R0: Performance comparison of the RL policies trained using ResNet model for a 10-node network. The barplot displays the mean infection rate for datasets d1, d2, and d3 of Dataset v1 type, differentiated by the number of initial misinformation sources (Inf.) and action budgets (Act.: a1, a2, a3). Each subplot illustrates the performance of a policy trained with the parameters indicated in its title. Lower infection rates indicate more effective policy learning and misinformation containment.}
    \label{fig:inf_resnet_c2r0_10}
\end{figure}

\begin{figure}
    \centering
    \includegraphics[scale=0.34]{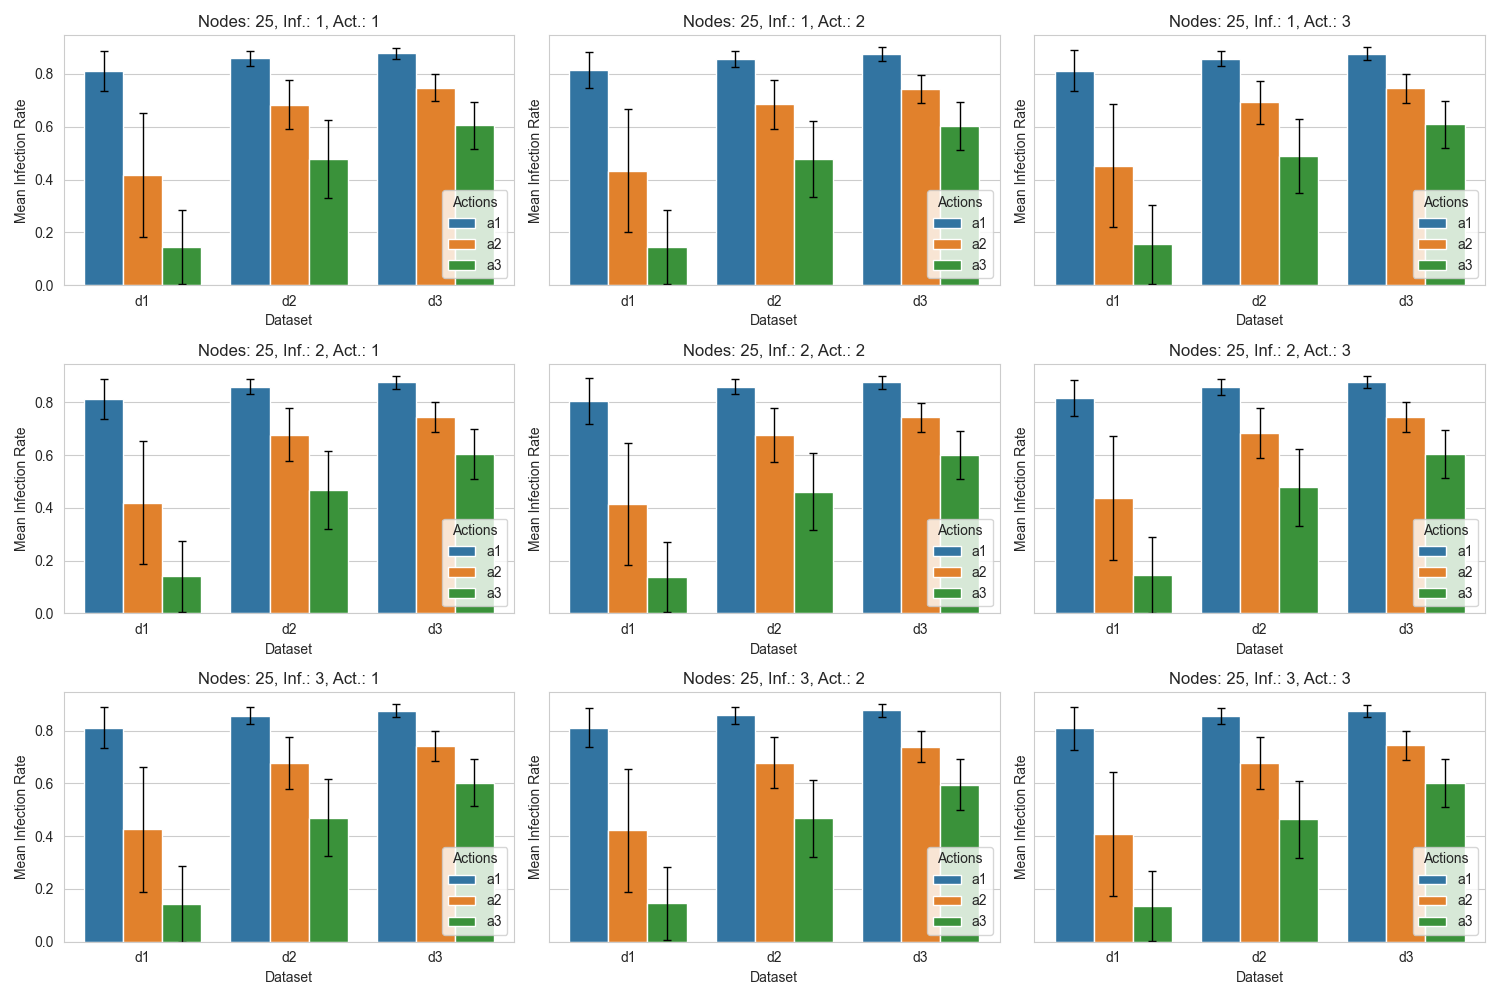}
    \caption{Case-2 using R0: Performance comparison of the RL policies trained using ResNet model for a 25-node network. The barplot displays the mean infection rate for datasets d1, d2, and d3 of Dataset v1 type, differentiated by the number of initial misinformation sources (Inf.) and action budgets (Act.: a1, a2, a3). Each subplot illustrates the performance of a policy trained with the parameters indicated in its title. Lower infection rates indicate more effective policy learning and misinformation containment.}
    \label{fig:inf_resnet_c2r0_25}
\end{figure}

\begin{figure}
    \centering
    \includegraphics[scale=0.34]{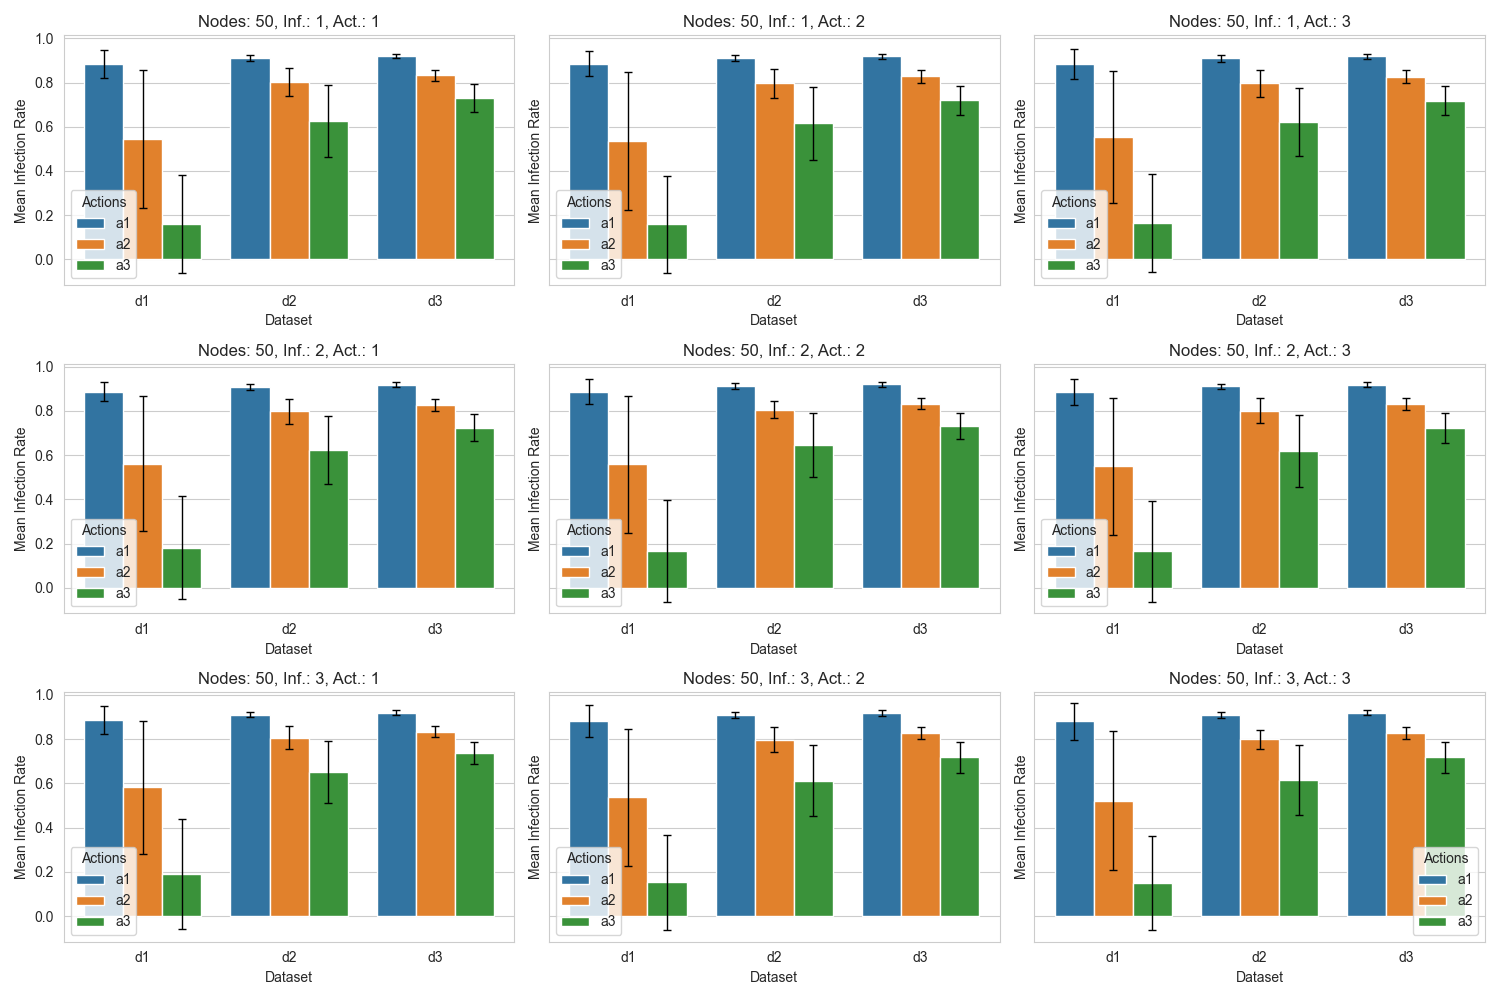}
    \caption{Case-2 using R0: Performance comparison of the RL policies trained using ResNet model for a 50-node network. The barplot displays the mean infection rate for datasets d1, d2, and d3 of Dataset v1 type, differentiated by the number of initial misinformation sources (Inf.) and action budgets (Act.: a1, a2, a3). Each subplot illustrates the performance of a policy trained with the parameters indicated in its title. Lower infection rates indicate more effective policy learning and misinformation containment.}
    \label{fig:inf_resnet_c2r0_50}
\end{figure}

%%%%%% R1 %%%%%%%%
\begin{figure}[!h]
    \centering
    \includegraphics[scale=0.34]{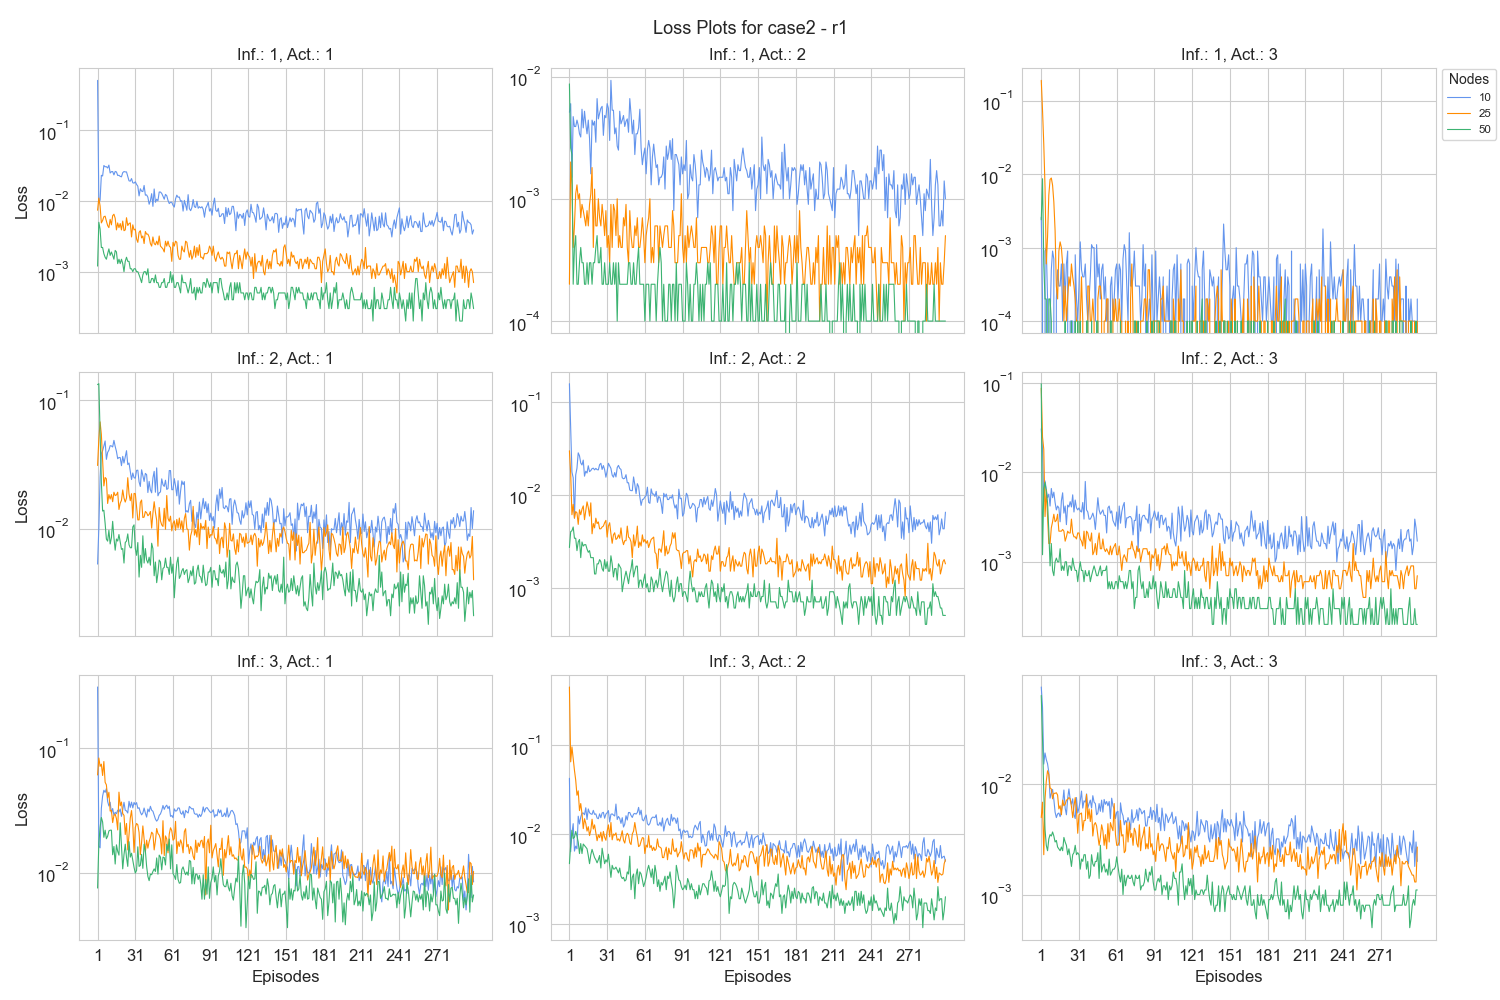}
    \caption{Case-2 using R1: Training MSE loss evolution for RL policy using ResNet model across networks of 10 (blue), 25 (orange), and 50 (green) nodes, for varying initial misinformation sources (Inf.) and action budgets (Act.). Plotted on a logarithmic scale, the loss decreases over episodes, indicating improved policy performance and adaptation across network sizes.}
    \label{fig:resnet_c2r1_loss}
\end{figure}

\begin{figure}
    \centering
    \includegraphics[scale=0.34]{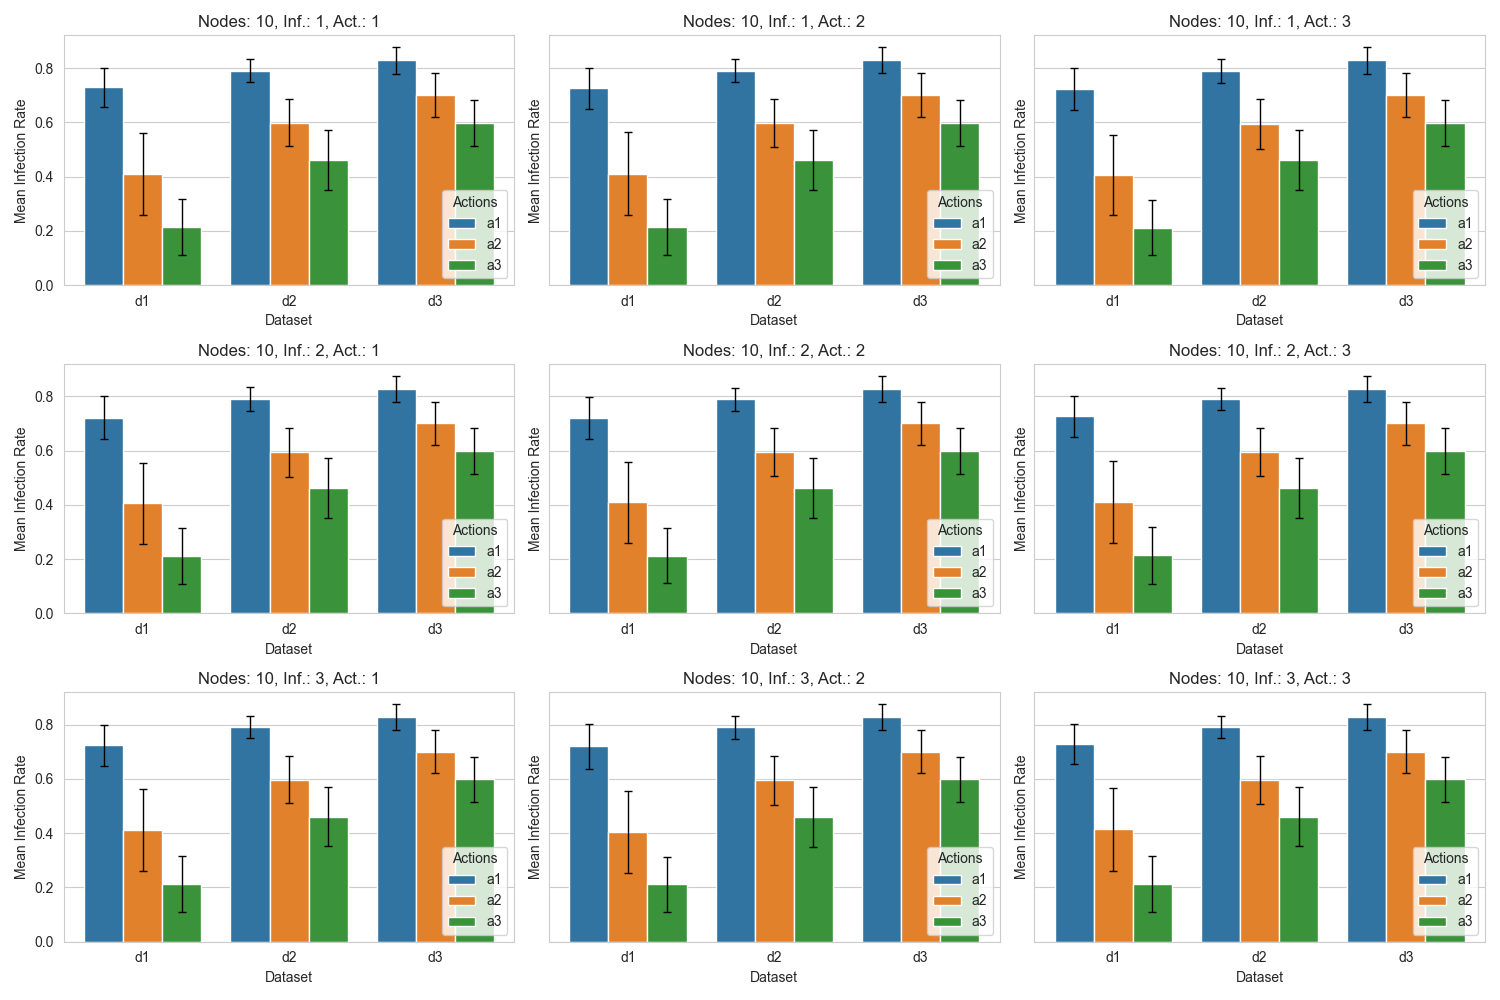}
    \caption{Case-2 using R1: Performance comparison of the RL policies trained using ResNet model for a 10-node network. The barplot displays the mean infection rate for datasets d1, d2, and d3 of Dataset v1 type, differentiated by the number of initial misinformation sources (Inf.) and action budgets (Act.: a1, a2, a3). Each subplot illustrates the performance of a policy trained with the parameters indicated in its title. Lower infection rates indicate more effective policy learning and misinformation containment.}
    \label{fig:inf_resnet_c2r1_10}
\end{figure}

\begin{figure}
    \centering
    \includegraphics[scale=0.34]{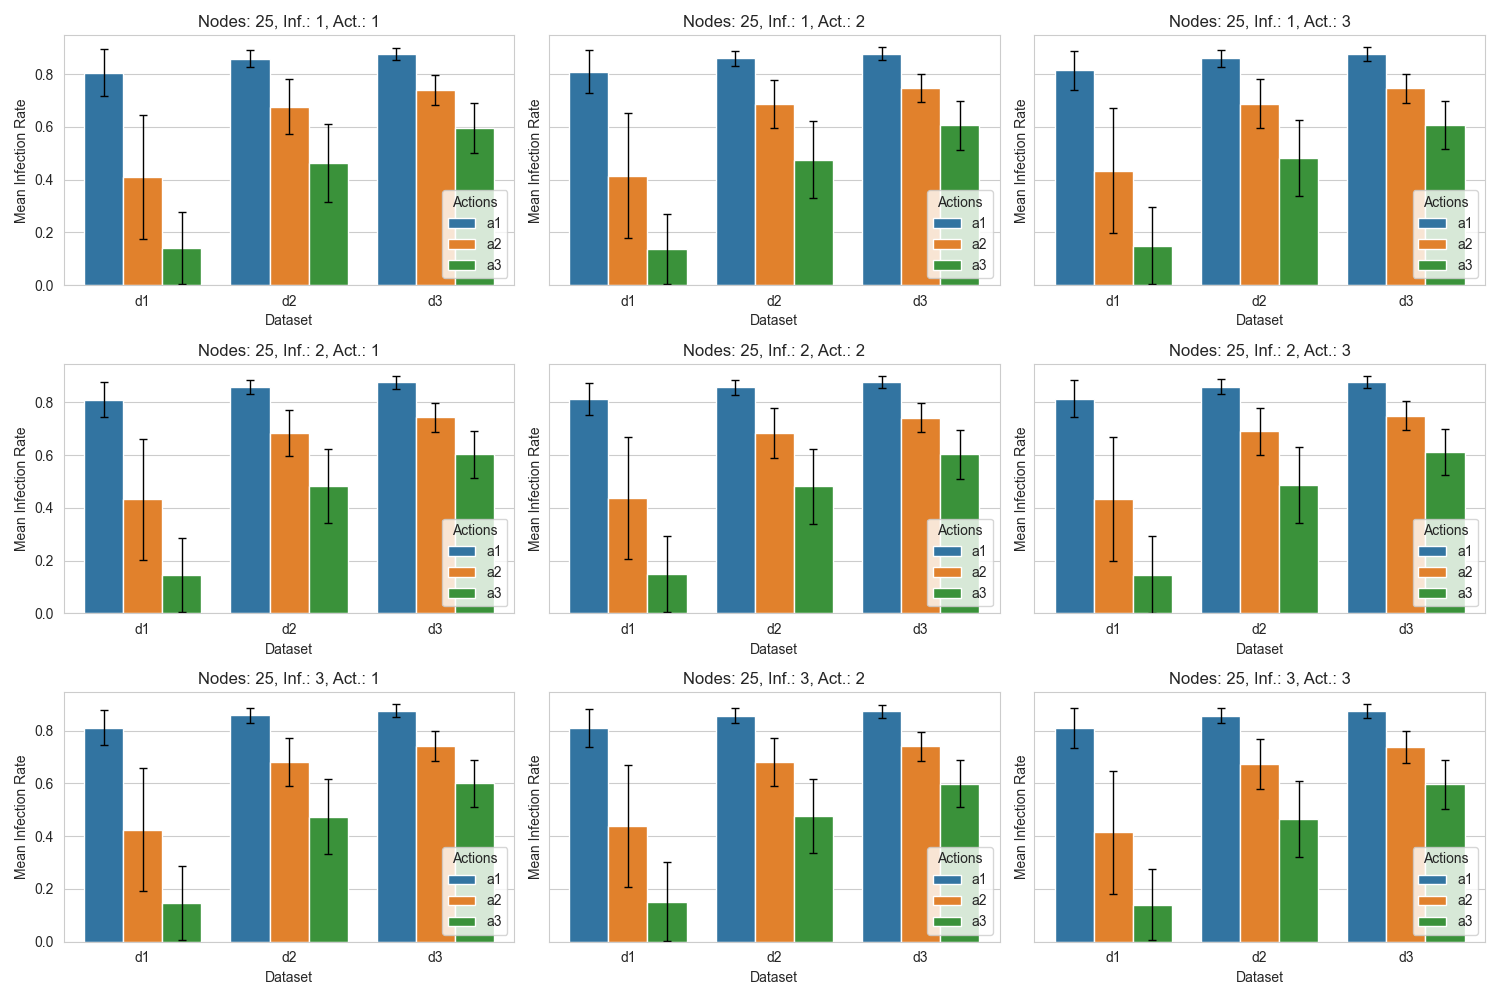}
    \caption{Case-2 using R1: Performance comparison of the RL policies trained using ResNet model for a 25-node network. The barplot displays the mean infection rate for datasets d1, d2, and d3 of Dataset v1 type, differentiated by the number of initial misinformation sources (Inf.) and action budgets (Act.: a1, a2, a3). Each subplot illustrates the performance of a policy trained with the parameters indicated in its title. Lower infection rates indicate more effective policy learning and misinformation containment.}
    \label{fig:inf_resnet_c2r1_25}
\end{figure}

\begin{figure}
    \centering
    \includegraphics[scale=0.34]{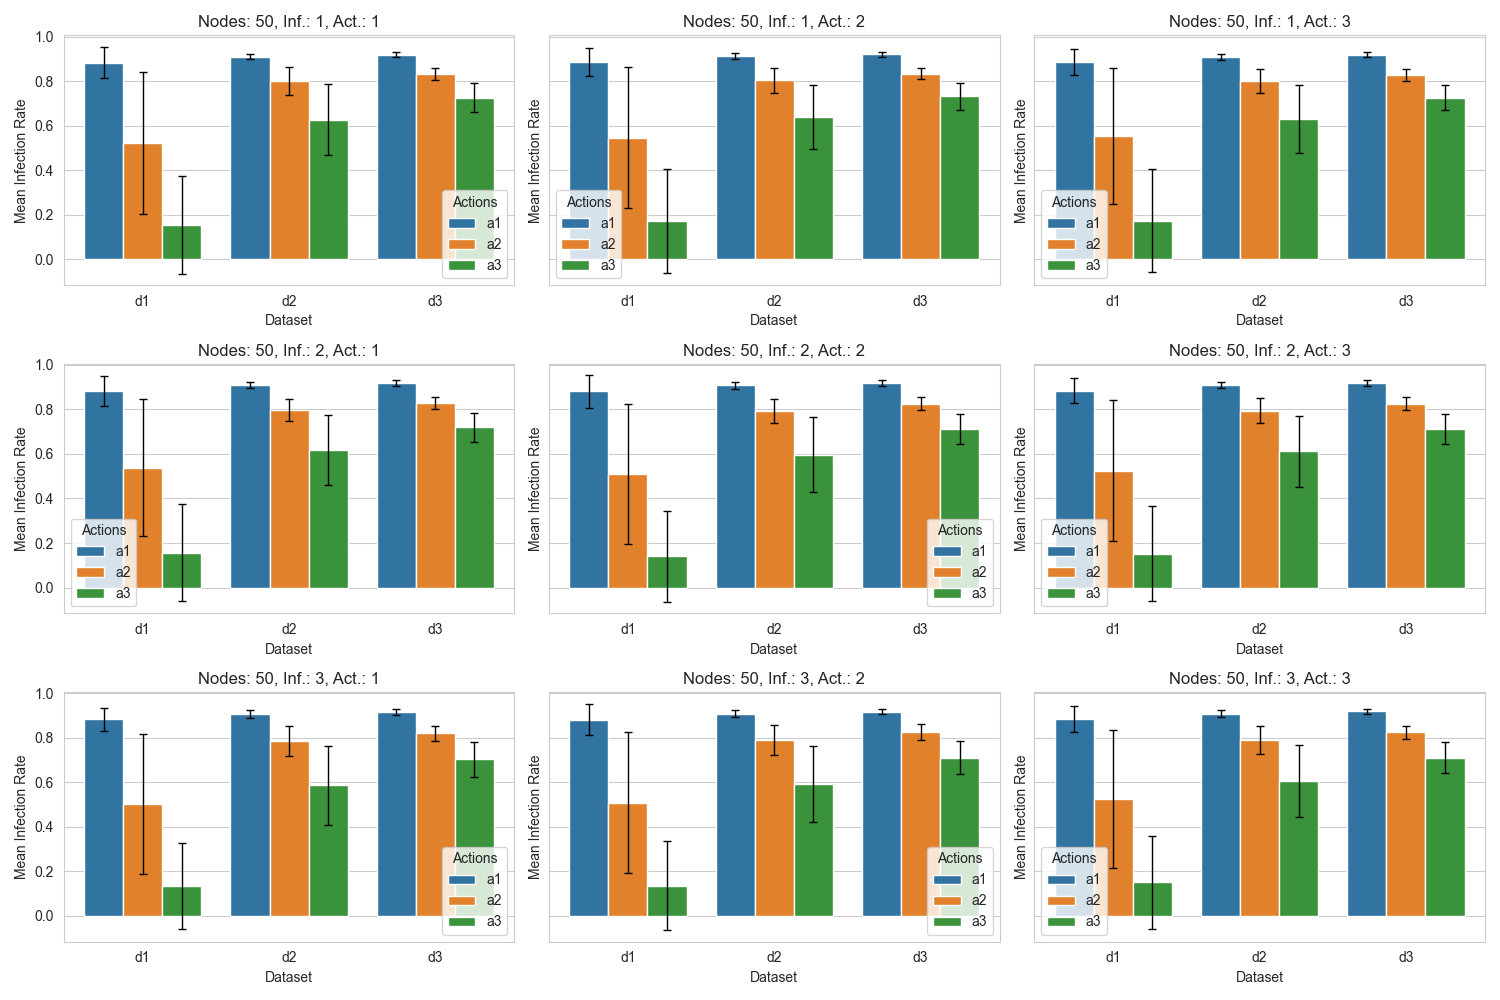}
    \caption{Case-2 using R1: Performance comparison of the RL policies trained using ResNet model for a 50-node network. The barplot displays the mean infection rate for datasets d1, d2, and d3 of Dataset v1 type, differentiated by the number of initial misinformation sources (Inf.) and action budgets (Act.: a1, a2, a3). Each subplot illustrates the performance of a policy trained with the parameters indicated in its title. Lower infection rates indicate more effective policy learning and misinformation containment.}
    \label{fig:inf_resnet_c2r1_50}
\end{figure}

%%%%%% R2 %%%%%%%%
\begin{figure}[!h]
    \centering
    \includegraphics[scale=0.34]{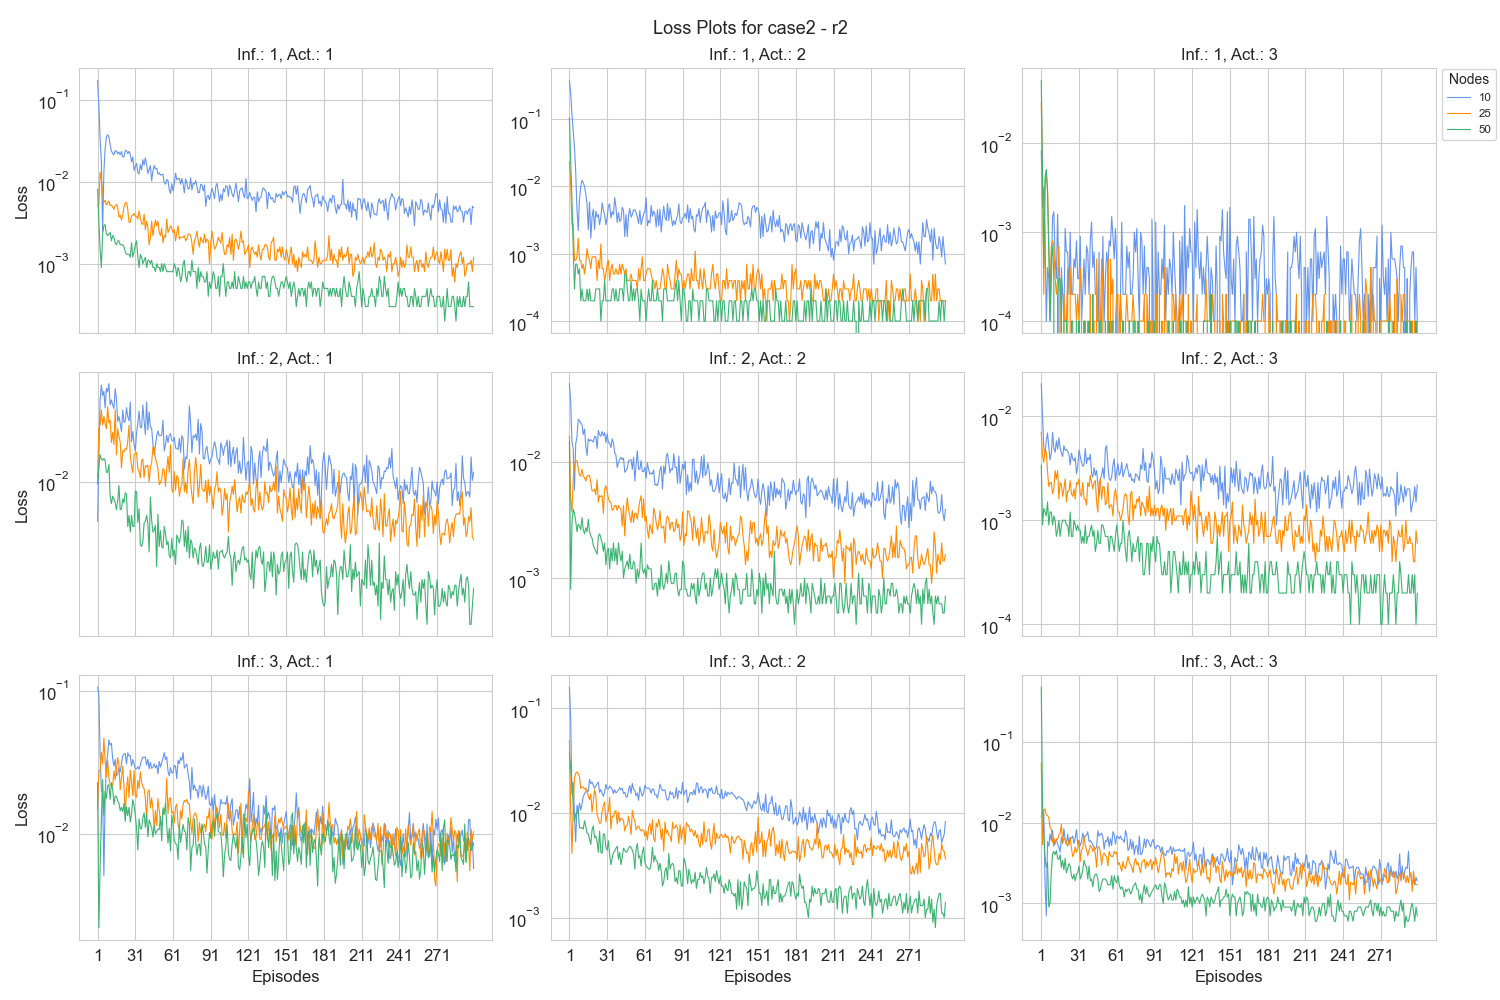}
    \caption{Case-2 using R2: Training MSE loss evolution for RL policy using ResNet model across networks of 10 (blue), 25 (orange), and 50 (green) nodes, for varying initial misinformation sources (Inf.) and action budgets (Act.). Plotted on a logarithmic scale, the loss decreases over episodes, indicating improved policy performance and adaptation across network sizes.}
    \label{fig:resnet_c2r2_loss}
\end{figure}

\begin{figure}
    \centering
    \includegraphics[scale=0.34]{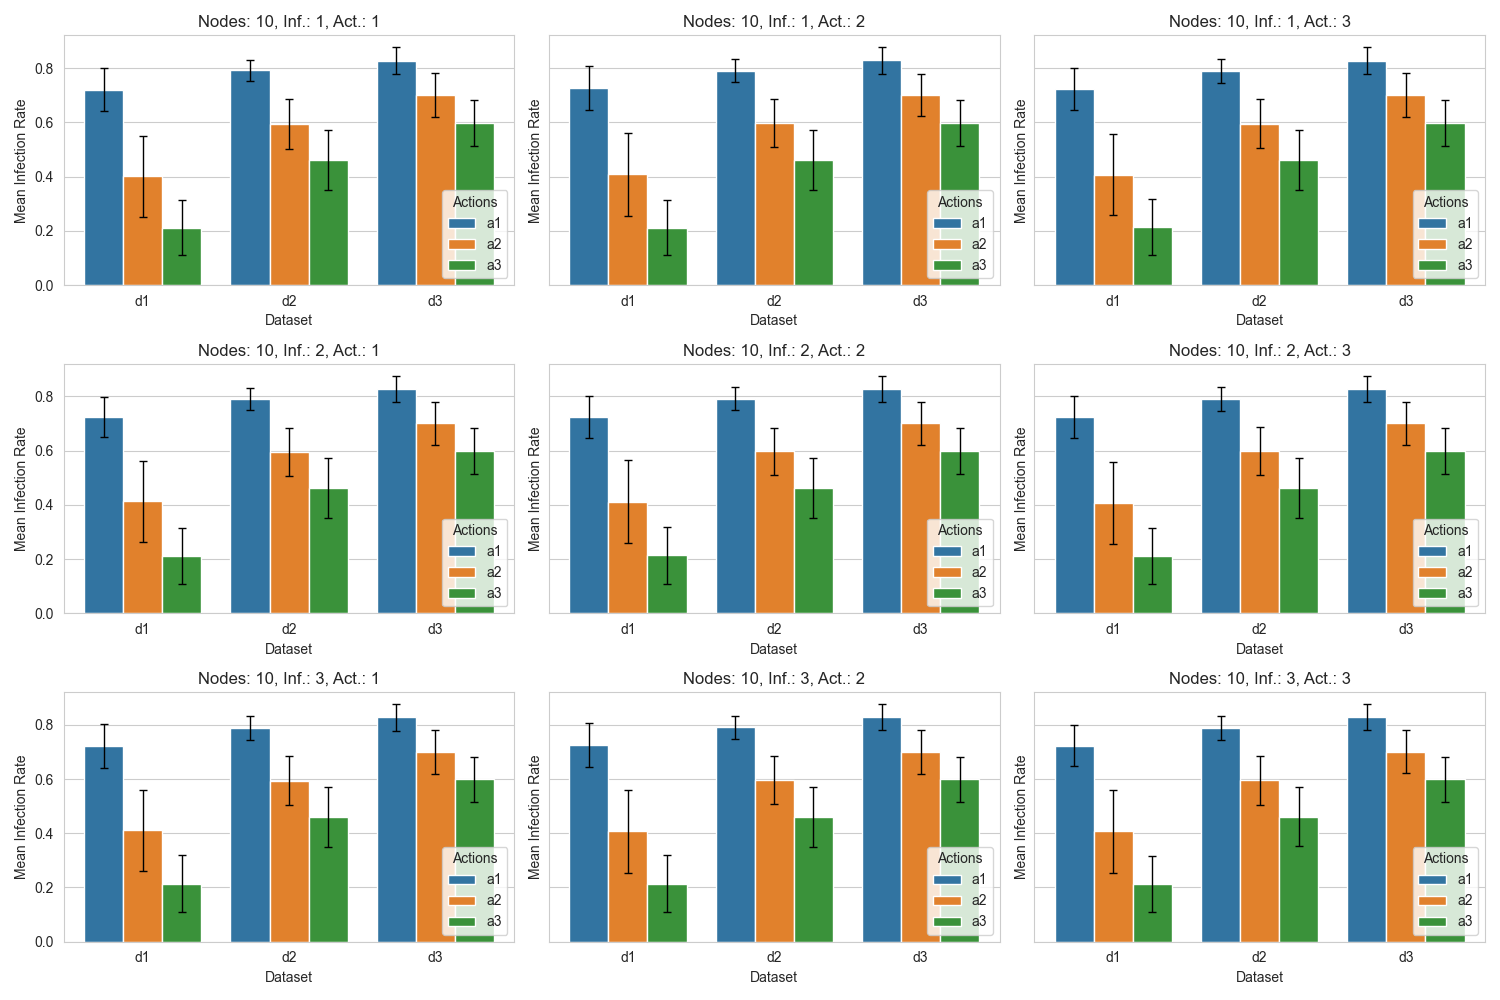}
    \caption{Case-2 using R2: Performance comparison of the RL policies trained using ResNet model for a 10-node network. The barplot displays the mean infection rate for datasets d1, d2, and d3 of Dataset v1 type, differentiated by the number of initial misinformation sources (Inf.) and action budgets (Act.: a1, a2, a3). Each subplot illustrates the performance of a policy trained with the parameters indicated in its title. Lower infection rates indicate more effective policy learning and misinformation containment.}
    \label{fig:inf_resnet_c2r2_10}
\end{figure}

\begin{figure}
    \centering
    \includegraphics[scale=0.34]{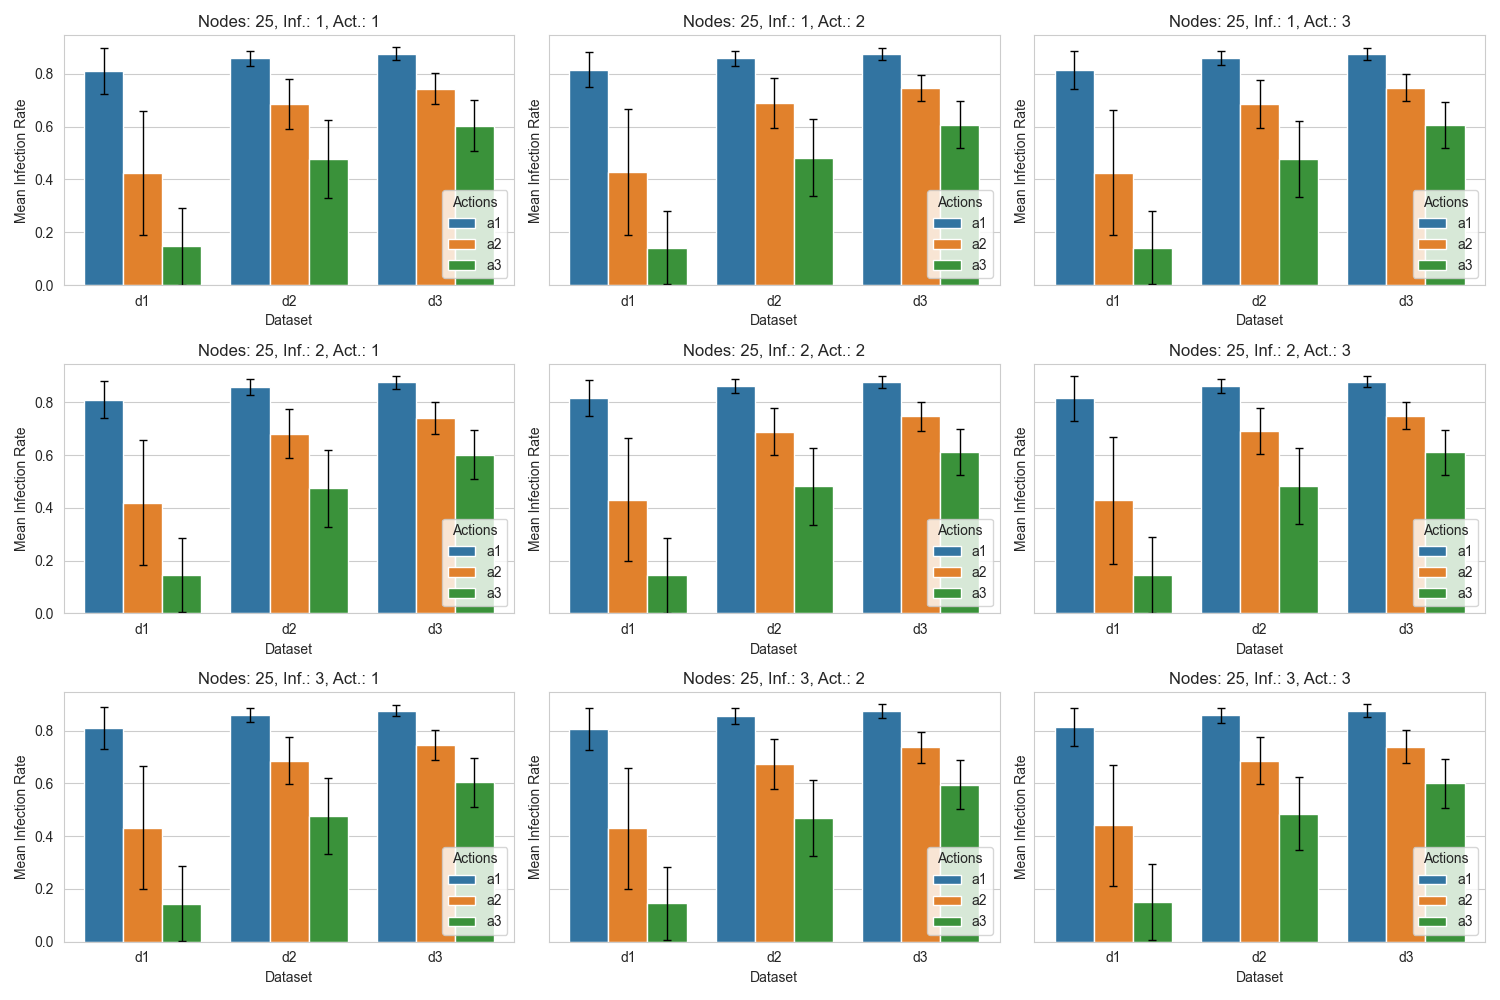}
    \caption{Case-2 using R2: Performance comparison of the RL policies trained using ResNet model for a 25-node network. The barplot displays the mean infection rate for datasets d1, d2, and d3 of Dataset v1 type, differentiated by the number of initial misinformation sources (Inf.) and action budgets (Act.: a1, a2, a3). Each subplot illustrates the performance of a policy trained with the parameters indicated in its title. Lower infection rates indicate more effective policy learning and misinformation containment.}
    \label{fig:inf_resnet_c2r2_25}
\end{figure}

\begin{figure}
    \centering
    \includegraphics[scale=0.34]{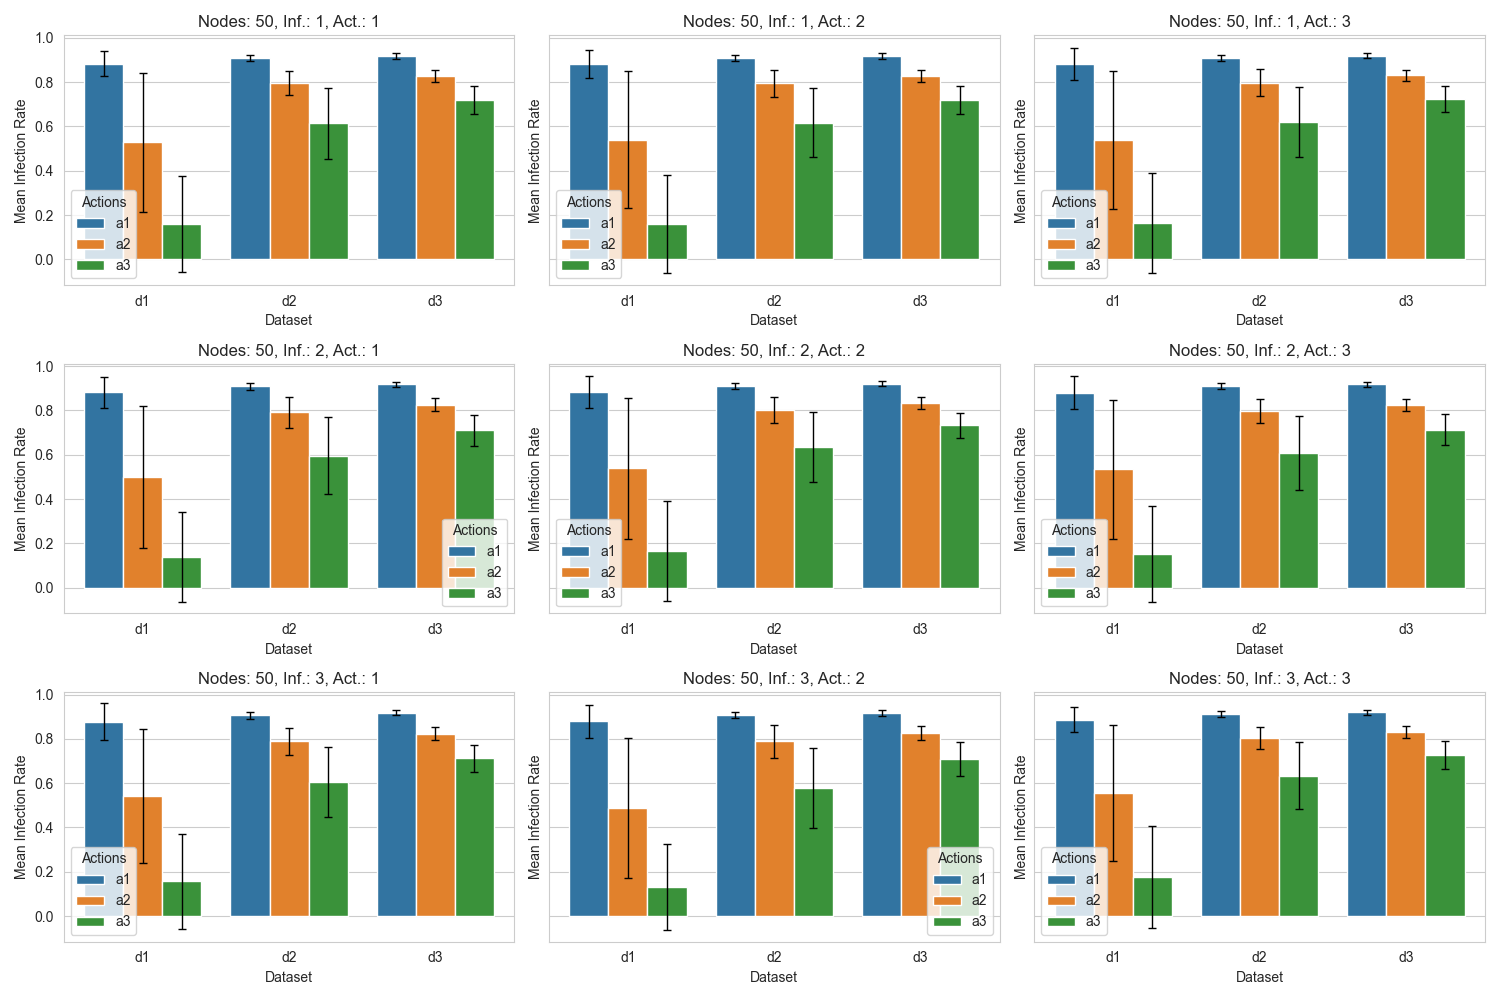}
    \caption{Case-2 using R2: Performance comparison of the RL policies trained using ResNet model for a 50-node network. The barplot displays the mean infection rate for datasets d1, d2, and d3 of Dataset v1 type, differentiated by the number of initial misinformation sources (Inf.) and action budgets (Act.: a1, a2, a3). Each subplot illustrates the performance of a policy trained with the parameters indicated in its title. Lower infection rates indicate more effective policy learning and misinformation containment.}
    \label{fig:inf_resnet_c2r2_50}
\end{figure}

%%%%%% R3 %%%%%%%%
\begin{figure}[!h]
    \centering
    \includegraphics[scale=0.34]{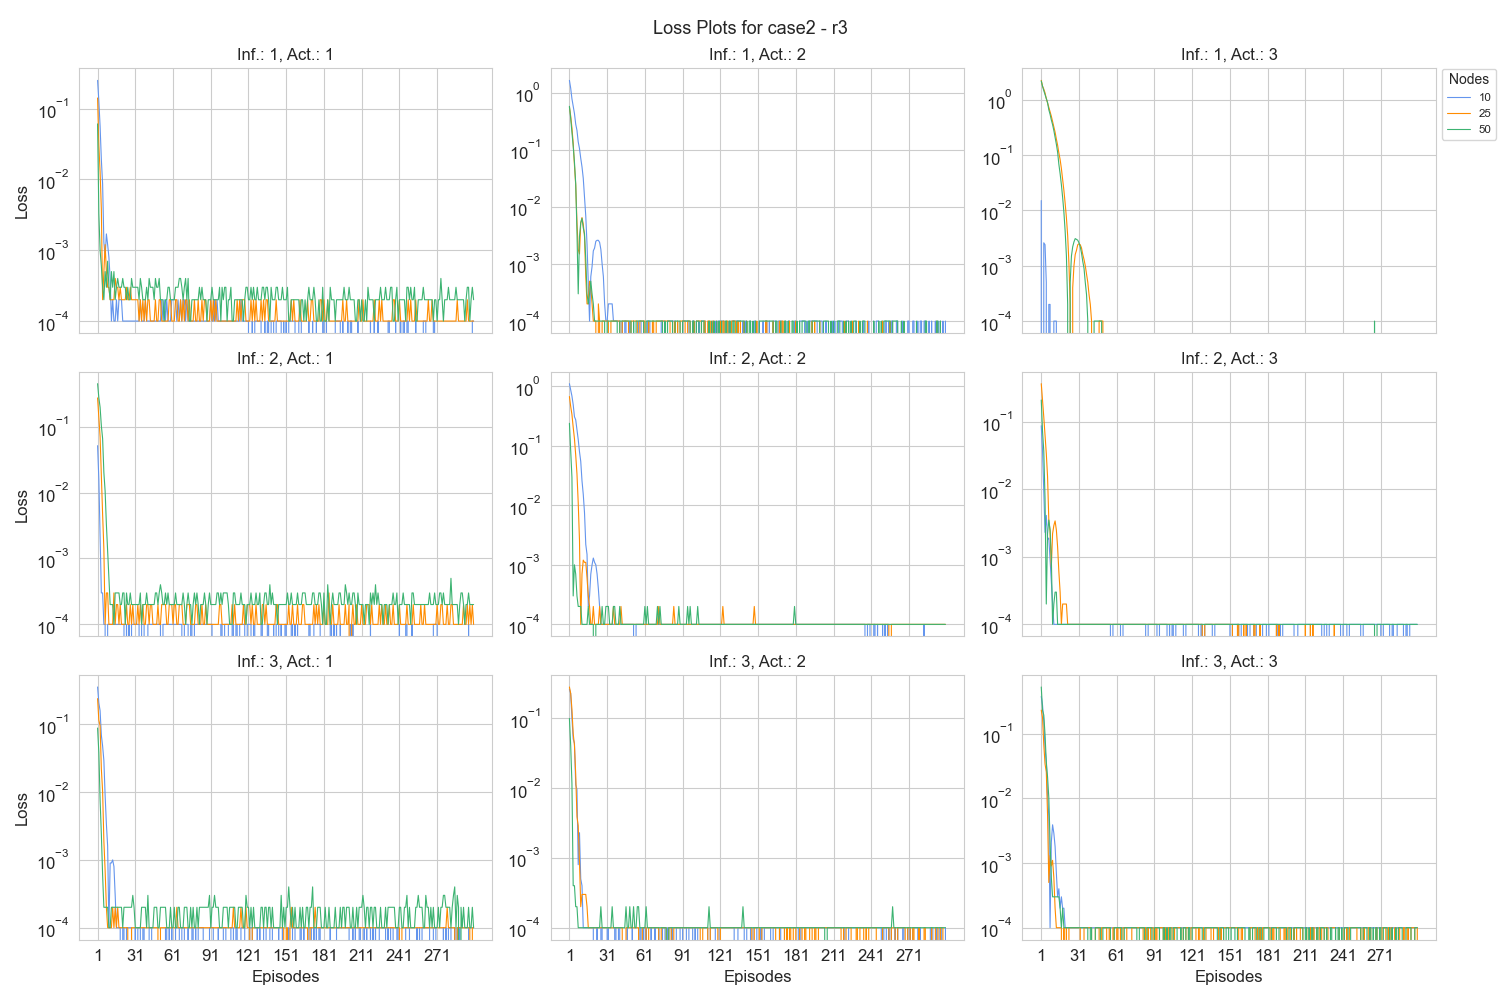}
    \caption{Case-2 using R3: Training MSE loss evolution for RL policy using ResNet model across networks of 10 (blue), 25 (orange), and 50 (green) nodes, for varying initial misinformation sources (Inf.) and action budgets (Act.). Plotted on a logarithmic scale, the loss decreases over episodes, indicating improved policy performance and adaptation across network sizes.}
    \label{fig:resnet_c2r3_loss}
\end{figure}

\begin{figure}
    \centering
    \includegraphics[scale=0.34]{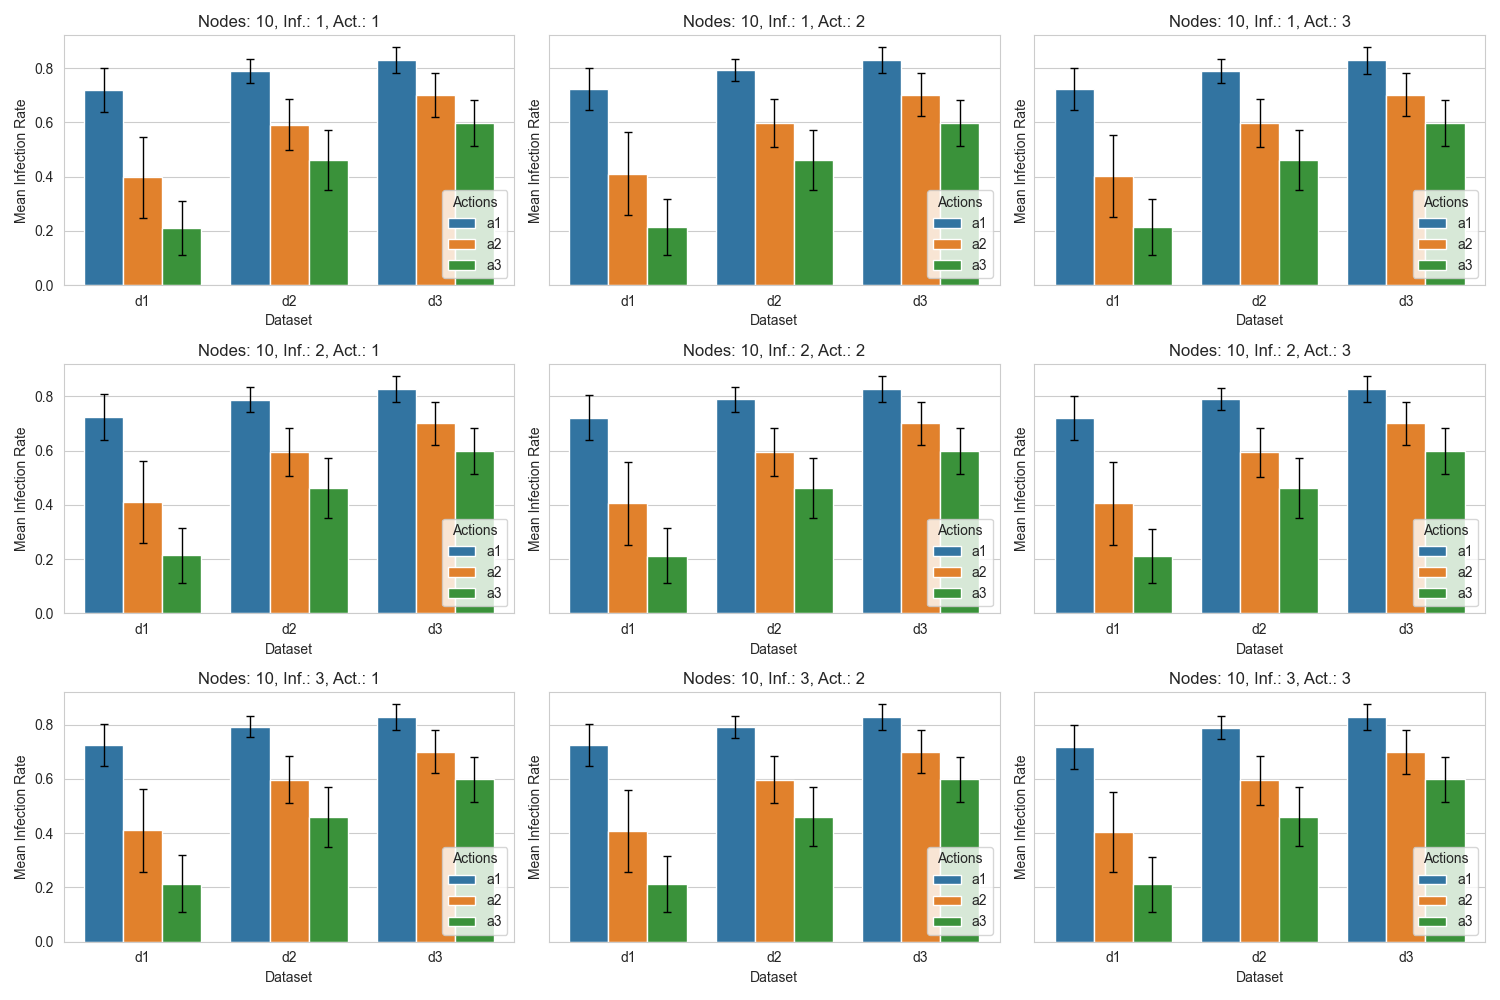}
    \caption{Case-2 using R3: Performance comparison of the RL policies trained using ResNet model for a 10-node network. The barplot displays the mean infection rate for datasets d1, d2, and d3 of Dataset v1 type, differentiated by the number of initial misinformation sources (Inf.) and action budgets (Act.: a1, a2, a3). Each subplot illustrates the performance of a policy trained with the parameters indicated in its title. Lower infection rates indicate more effective policy learning and misinformation containment.}
    \label{fig:inf_resnet_c2r3_10}
\end{figure}

\begin{figure}
    \centering
    \includegraphics[scale=0.34]{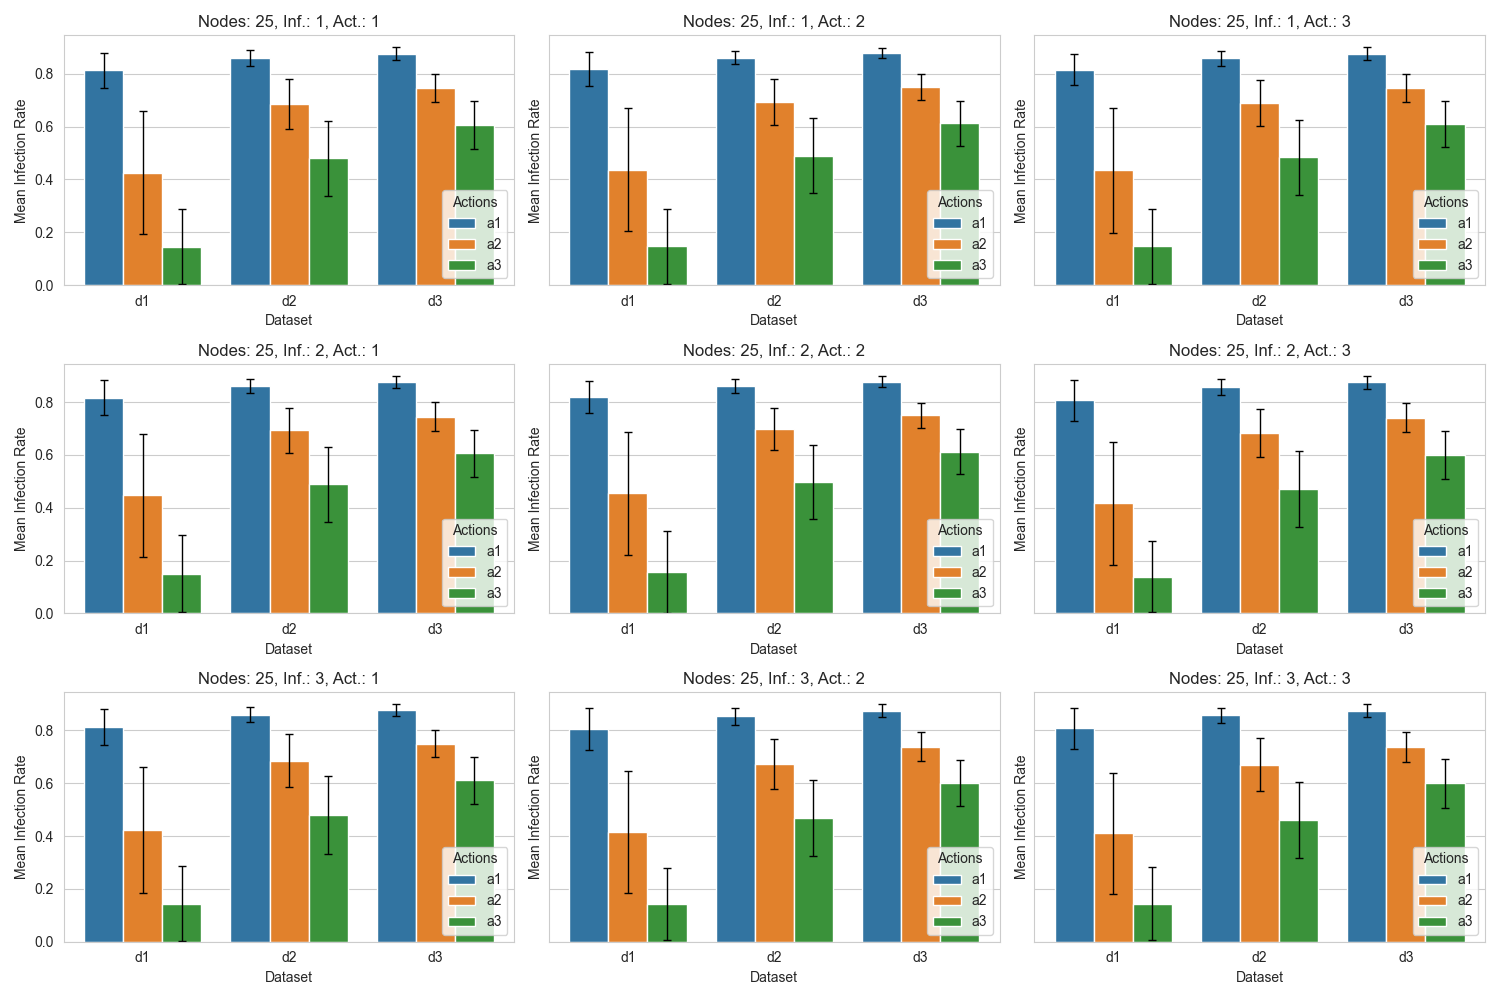}
    \caption{Case-2 using R3: Performance comparison of the RL policies trained using ResNet model for a 25-node network. The barplot displays the mean infection rate for datasets d1, d2, and d3 of Dataset v1 type, differentiated by the number of initial misinformation sources (Inf.) and action budgets (Act.: a1, a2, a3). Each subplot illustrates the performance of a policy trained with the parameters indicated in its title. Lower infection rates indicate more effective policy learning and misinformation containment.}
    \label{fig:inf_resnet_c2r3_25}
\end{figure}

\begin{figure}
    \centering
    \includegraphics[scale=0.34]{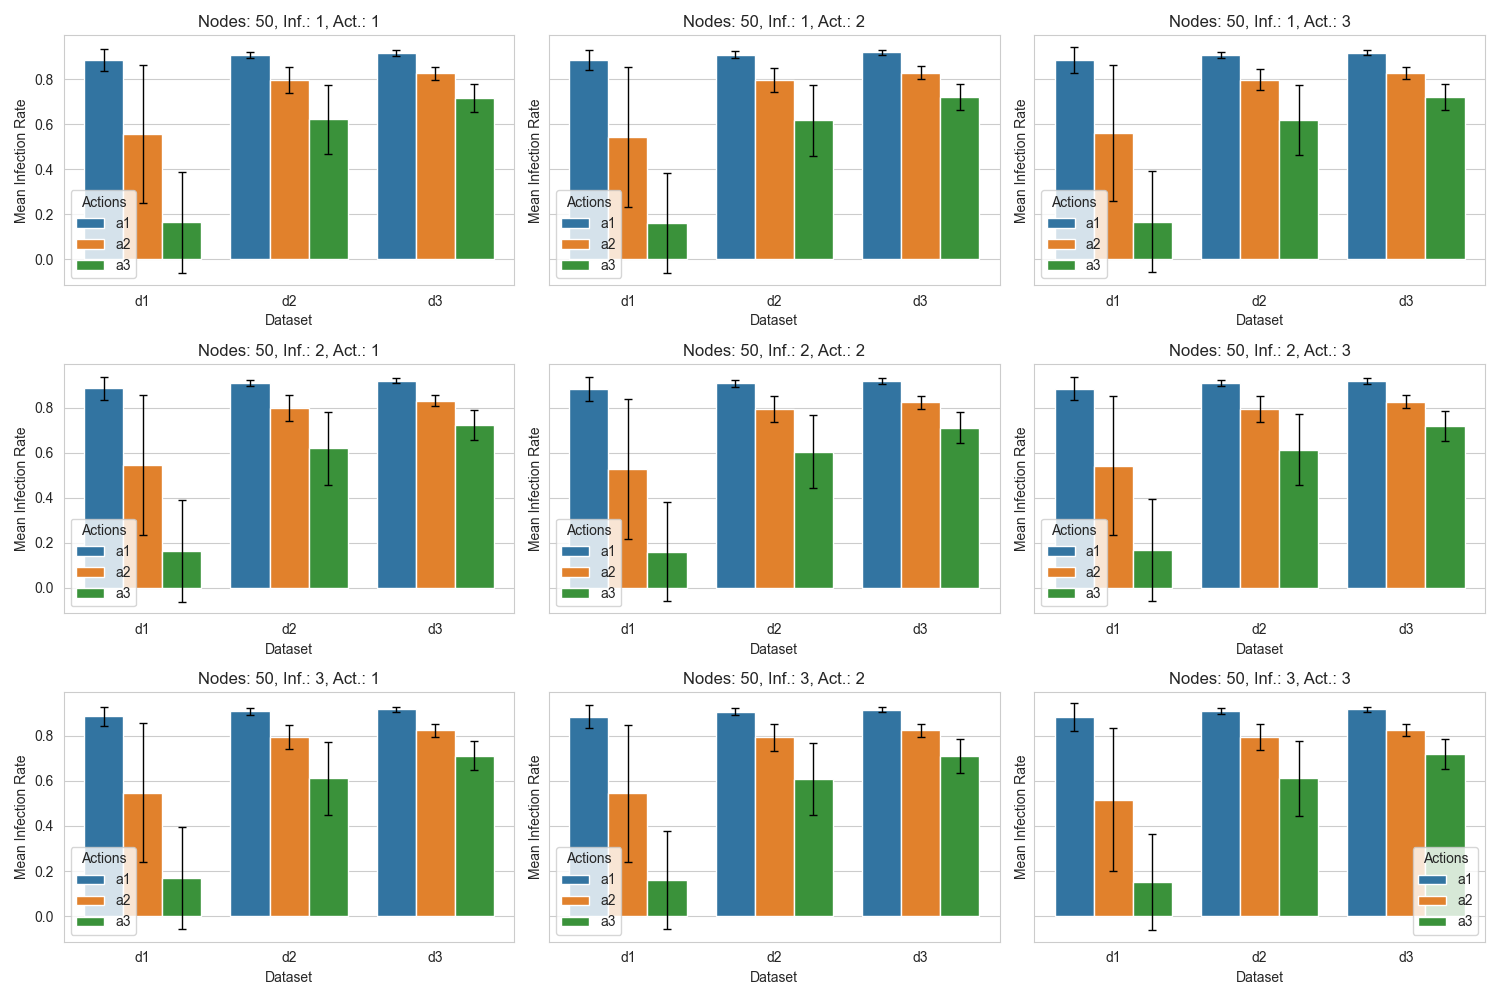}
    \caption{Case-2 using R3: Performance comparison of the RL policies trained using ResNet model for a 50-node network. The barplot displays the mean infection rate for datasets d1, d2, and d3 of Dataset v1 type, differentiated by the number of initial misinformation sources (Inf.) and action budgets (Act.: a1, a2, a3). Each subplot illustrates the performance of a policy trained with the parameters indicated in its title. Lower infection rates indicate more effective policy learning and misinformation containment.}
    \label{fig:inf_resnet_c2r3_50}
\end{figure}

%%%%%% R4 %%%%%%%%
\begin{figure}[!h]
    \centering
    \includegraphics[scale=0.34]{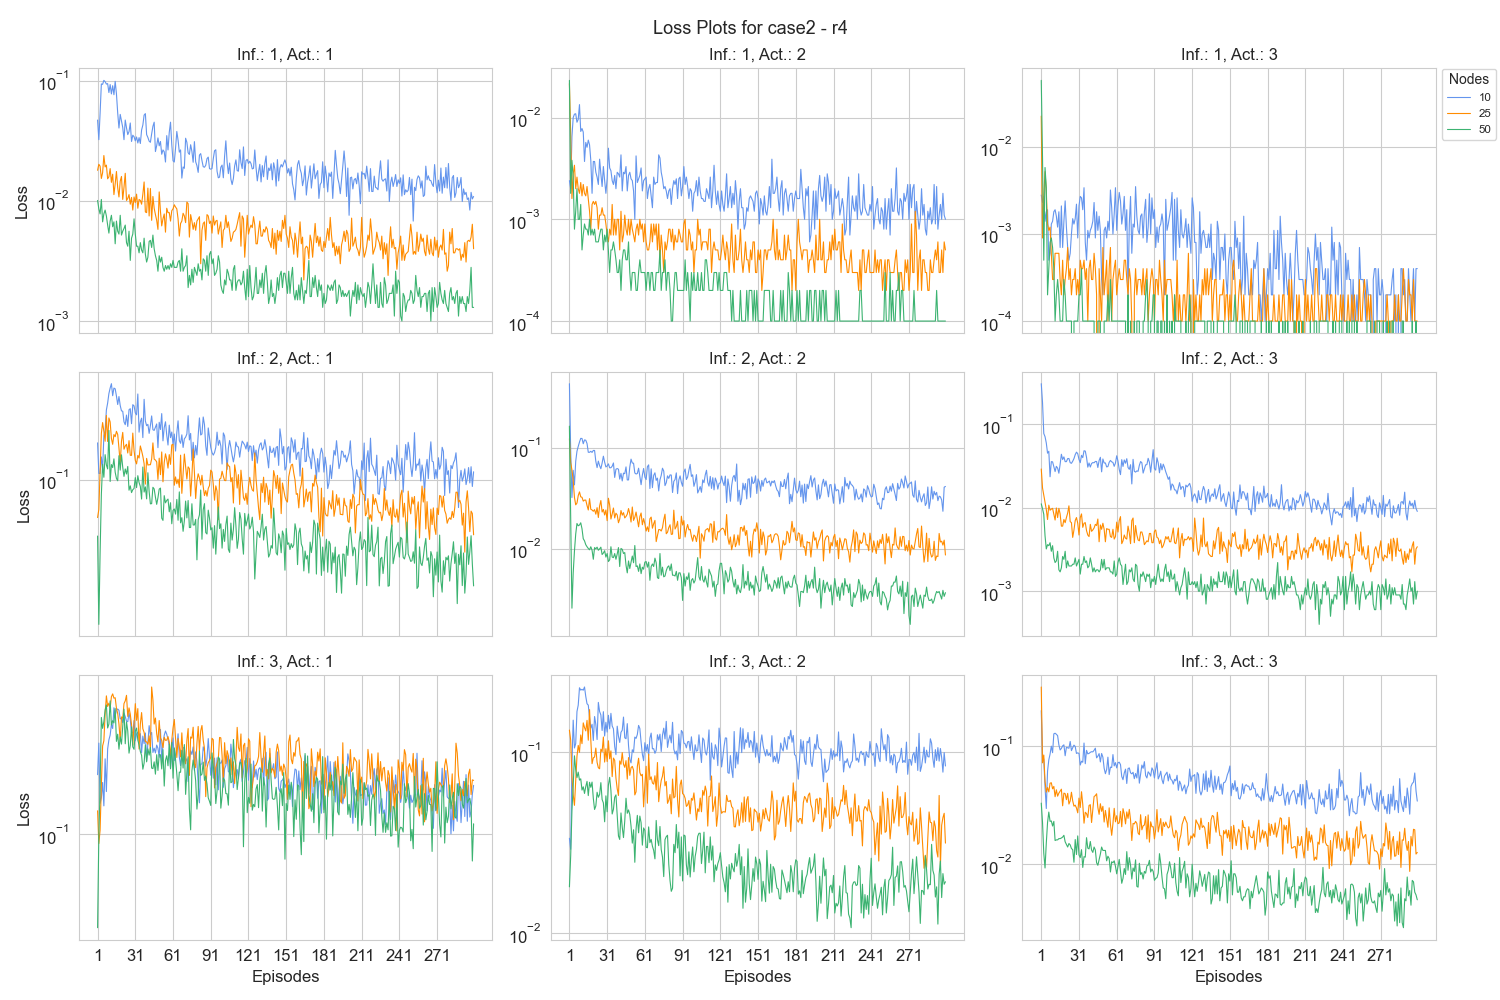}
    \caption{Case-2 using R4: Training MSE loss evolution for RL policy using ResNet model across networks of 10 (blue), 25 (orange), and 50 (green) nodes, for varying initial misinformation sources (Inf.) and action budgets (Act.). Plotted on a logarithmic scale, the loss decreases over episodes, indicating improved policy performance and adaptation across network sizes.}
    \label{fig:resnet_c2r4_loss}
\end{figure}

\begin{figure}
    \centering
    \includegraphics[scale=0.34]{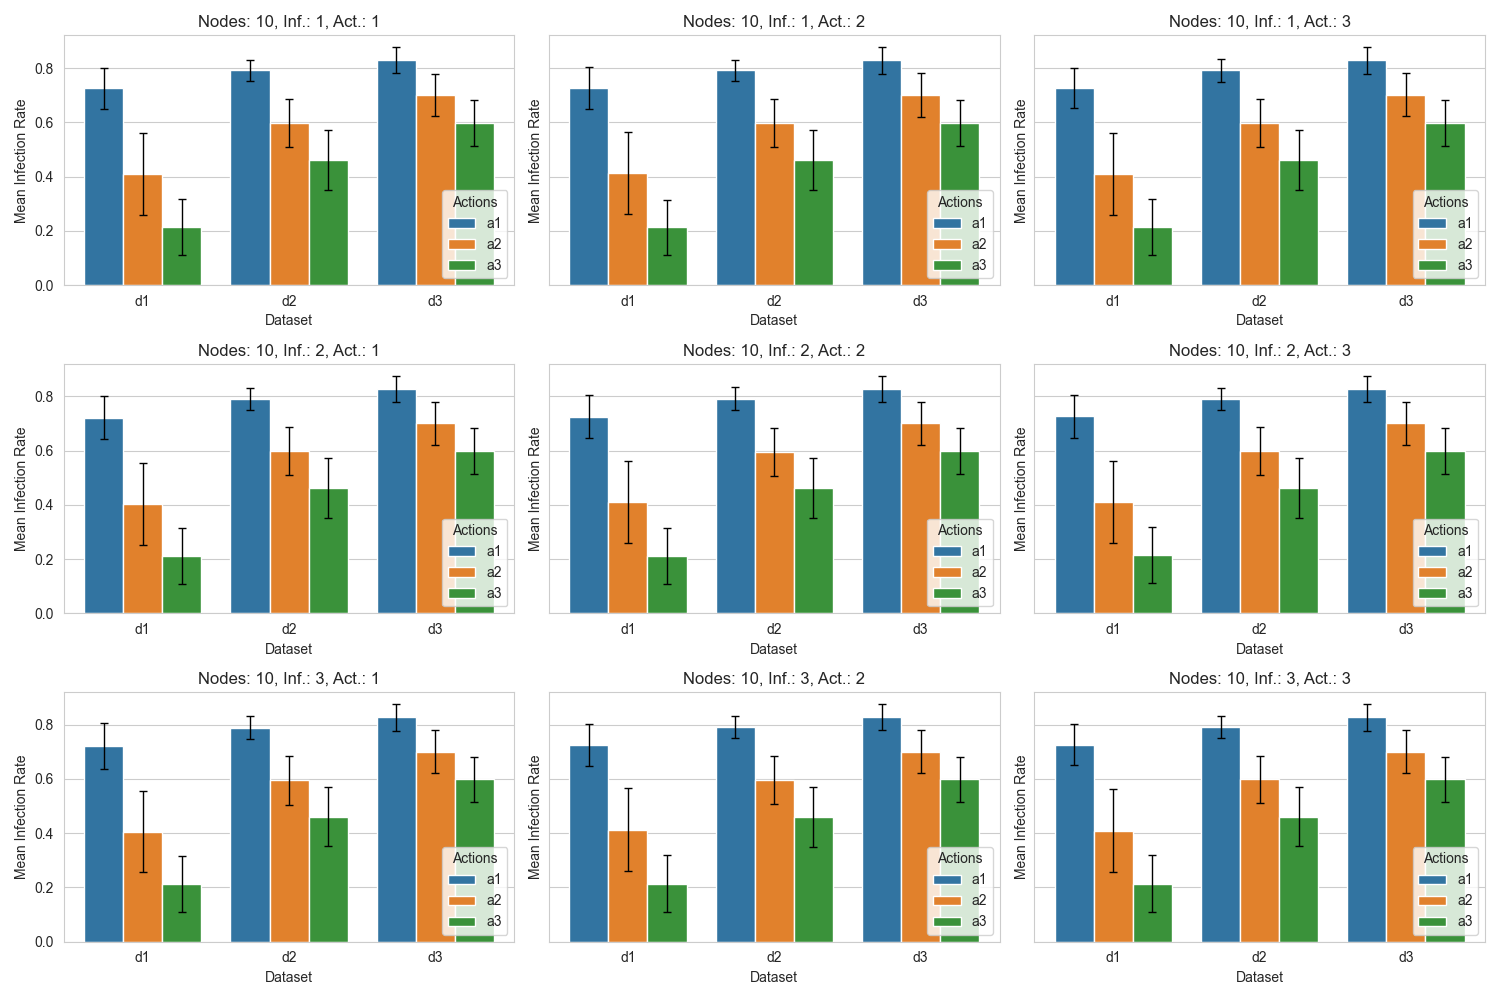}
    \caption{Case-2 using R4: Performance comparison of the RL policies trained using ResNet model for a 10-node network. The barplot displays the mean infection rate for datasets d1, d2, and d3 of Dataset v1 type, differentiated by the number of initial misinformation sources (Inf.) and action budgets (Act.: a1, a2, a3). Each subplot illustrates the performance of a policy trained with the parameters indicated in its title. Lower infection rates indicate more effective policy learning and misinformation containment.}
    \label{fig:inf_resnet_c2r4_10}
\end{figure}

\begin{figure}
    \centering
    \includegraphics[scale=0.34]{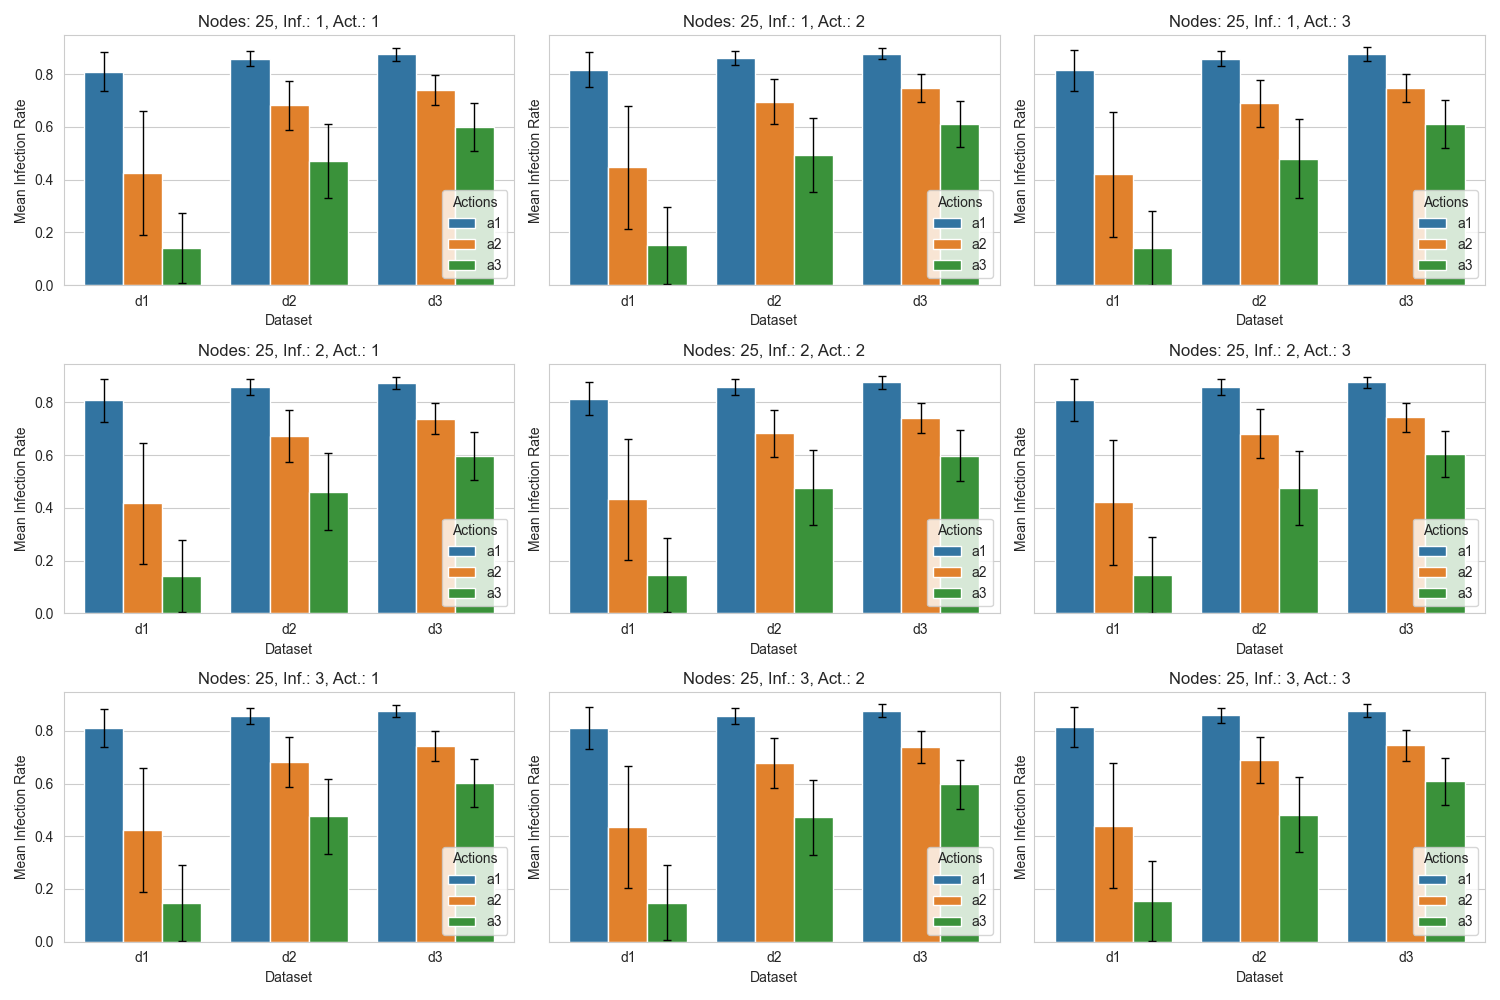}
    \caption{Case-2 using R4: Performance comparison of the RL policies trained using ResNet model for a 25-node network. The barplot displays the mean infection rate for datasets d1, d2, and d3 of Dataset v1 type, differentiated by the number of initial misinformation sources (Inf.) and action budgets (Act.: a1, a2, a3). Each subplot illustrates the performance of a policy trained with the parameters indicated in its title. Lower infection rates indicate more effective policy learning and misinformation containment.}
    \label{fig:inf_resnet_c2r4_25}
\end{figure}

\begin{figure}
    \centering
    \includegraphics[scale=0.34]{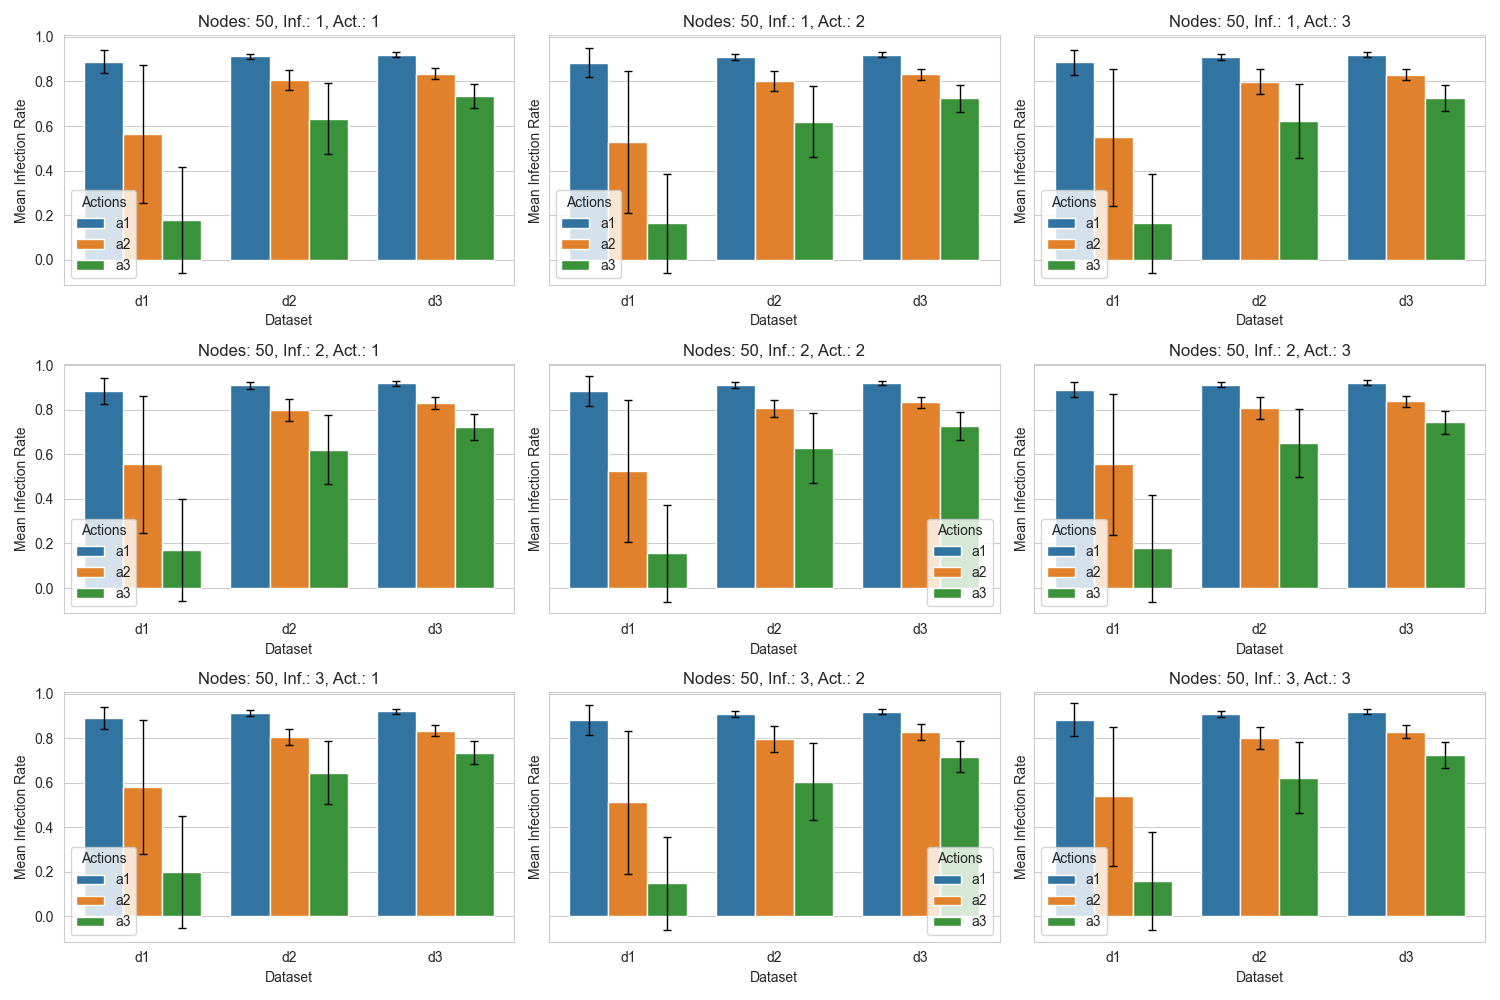}
    \caption{Case-2 using R4: Performance comparison of the RL policies trained using ResNet model for a 50-node network. The barplot displays the mean infection rate for datasets d1, d2, and d3 of Dataset v1 type, differentiated by the number of initial misinformation sources (Inf.) and action budgets (Act.: a1, a2, a3). Each subplot illustrates the performance of a policy trained with the parameters indicated in its title. Lower infection rates indicate more effective policy learning and misinformation containment.}
    \label{fig:inf_resnet_c2r4_50}
\end{figure}

%####################################

% ######### Case 3-v1 ResNet Figures ##########

%%%%%% R0 %%%%%%
\begin{figure}[!h]
    \centering
    \includegraphics[scale=0.34]{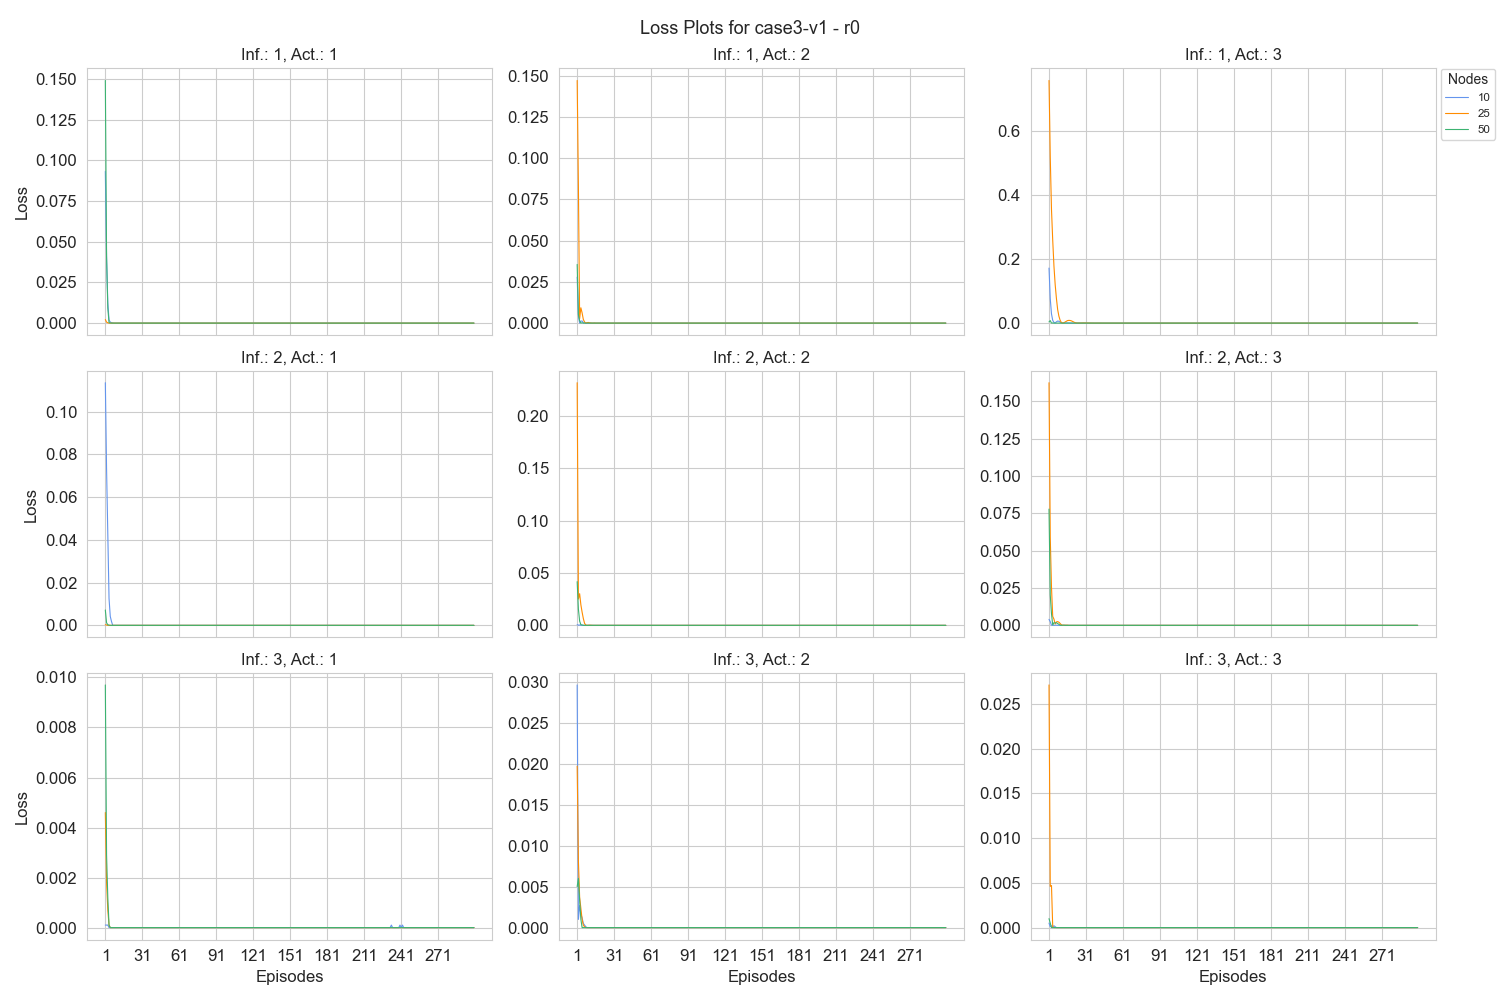}
    \caption{Case-3 v1 using R0: Training MSE loss evolution for RL policy using ResNet model across networks of 10 (blue), 25 (orange), and 50 (green) nodes, for varying initial misinformation sources (Inf.) and action budgets (Act.). The loss decreases over episodes, indicating improved policy performance and adaptation across network sizes.}
    \label{fig:resnet_c3v1r0_loss}
\end{figure}

\begin{figure}
    \centering
    \includegraphics[scale=0.34]{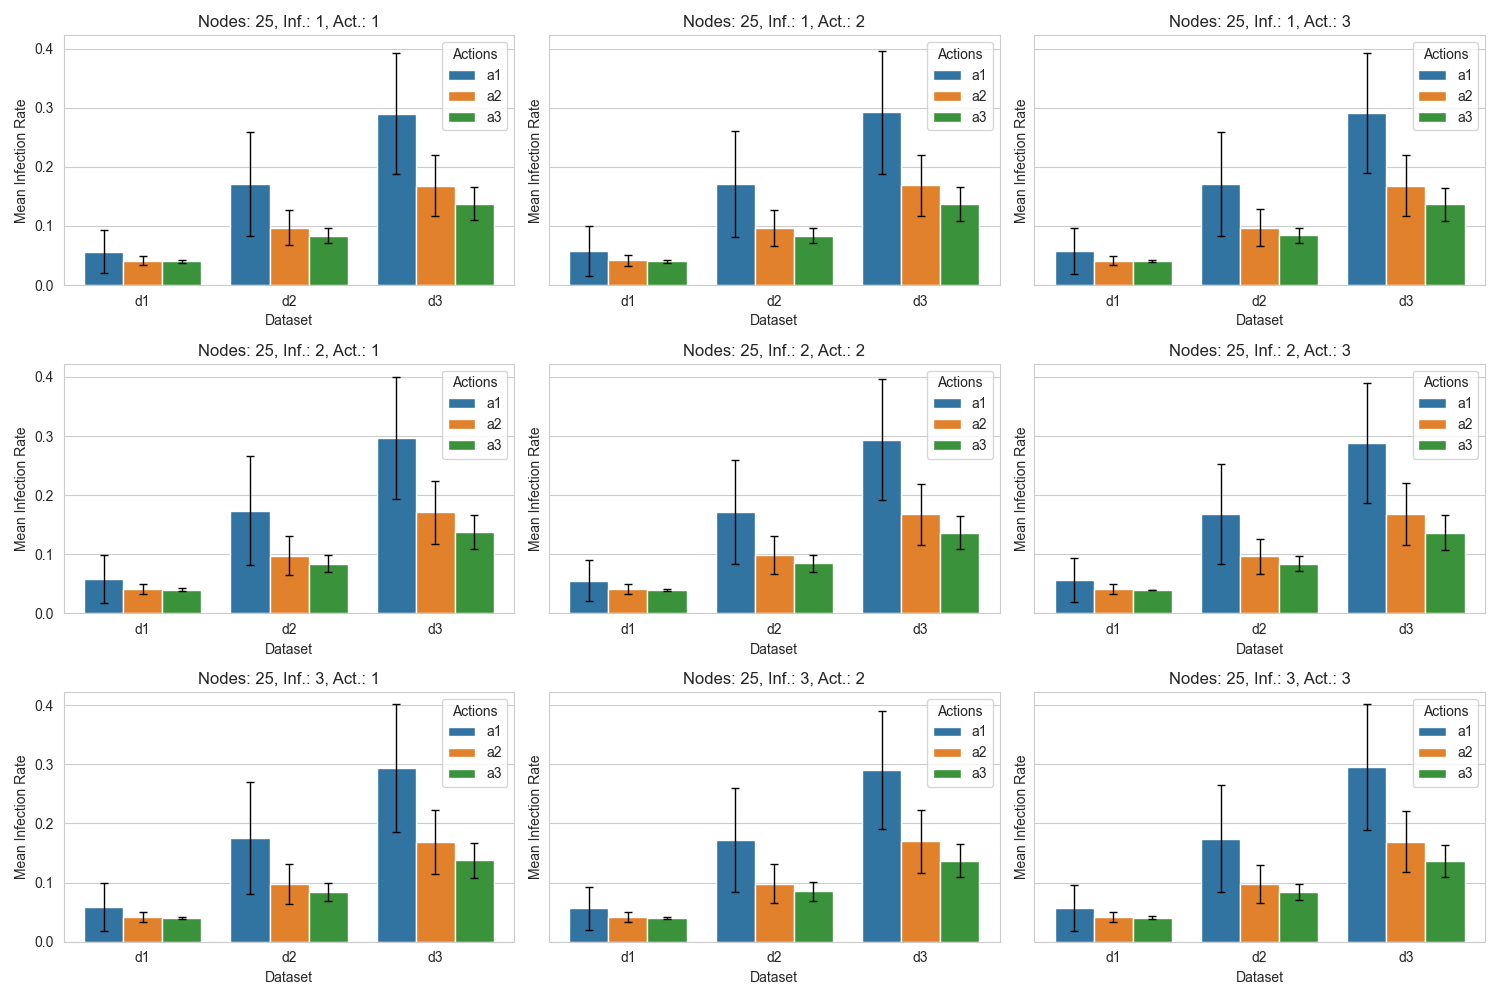}
    \caption{Case-3 v1 using R0: Performance comparison of the RL policies trained using ResNet model for a 25-node network. The barplot displays the mean infection rate for datasets d1, d2, and d3 of Dataset v1 type, differentiated by the number of initial misinformation sources (Inf.) and action budgets (Act.: a1, a2, a3). Each subplot illustrates the performance of a policy trained with the parameters indicated in its title. Lower infection rates indicate more effective policy learning and misinformation containment.}
    \label{fig:inf_resnet_c3v1r0_25}
\end{figure}

\begin{figure}
    \centering
    \includegraphics[scale=0.34]{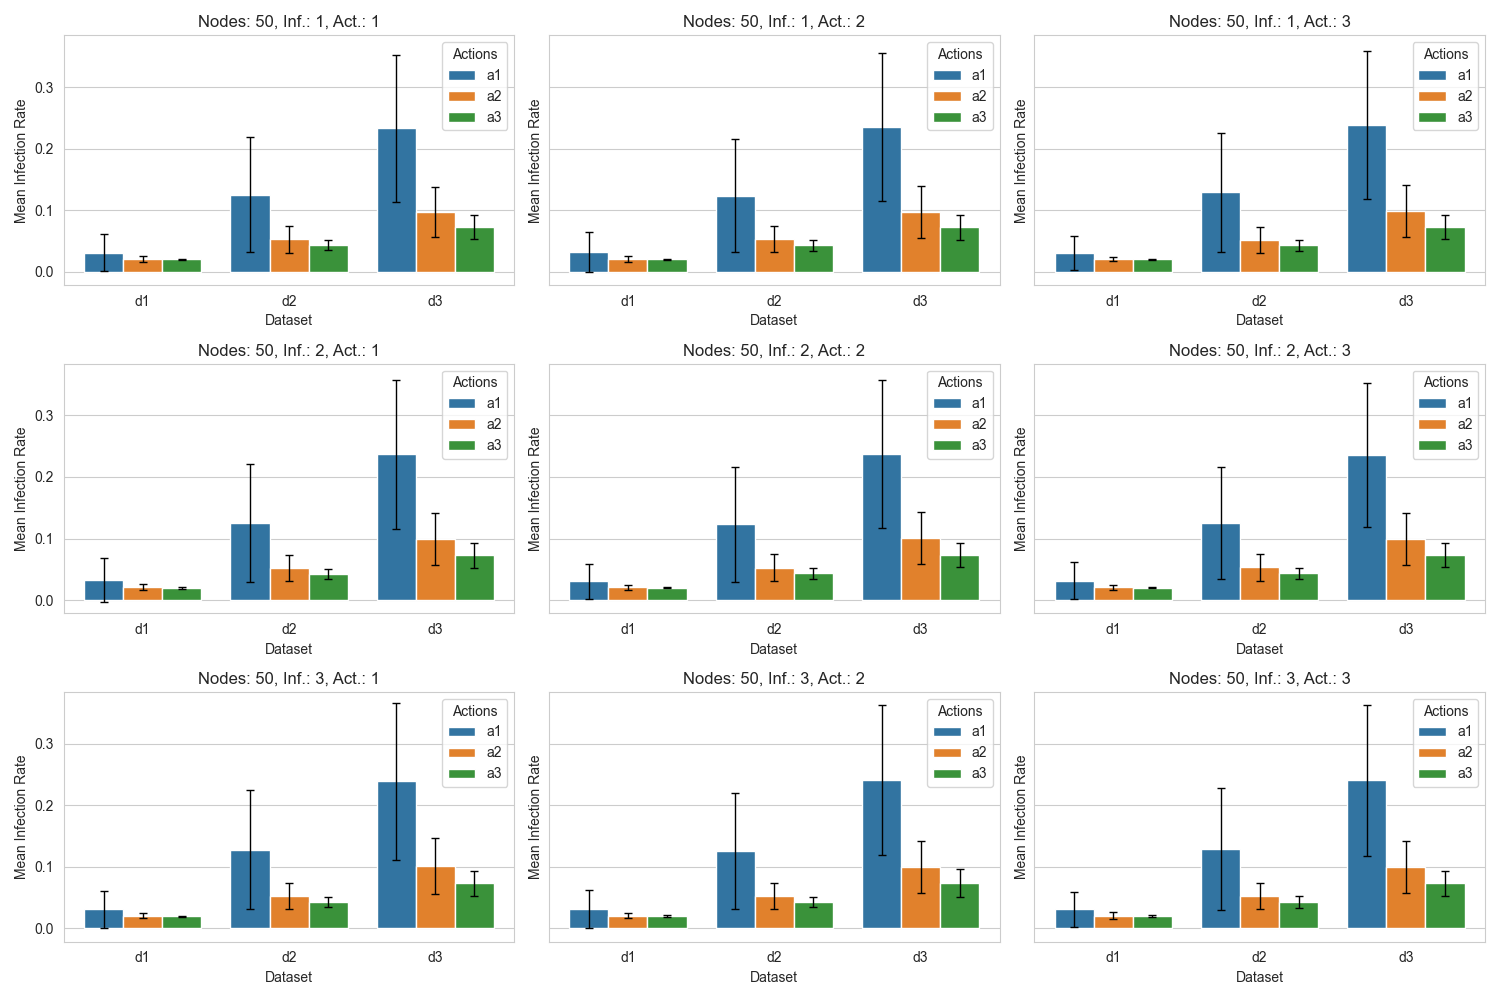}
    \caption{Case-3 v1 using R0: Performance comparison of the RL policies trained using ResNet model for a 50-node network. The barplot displays the mean infection rate for datasets d1, d2, and d3 of Dataset v1 type, differentiated by the number of initial misinformation sources (Inf.) and action budgets (Act.: a1, a2, a3). Each subplot illustrates the performance of a policy trained with the parameters indicated in its title. Lower infection rates indicate more effective policy learning and misinformation containment.}
    \label{fig:inf_resnet_c3v1r0_50}
\end{figure}

%%%%%% R1 %%%%%%%
\begin{figure}[!h]
    \centering
    \includegraphics[scale=0.34]{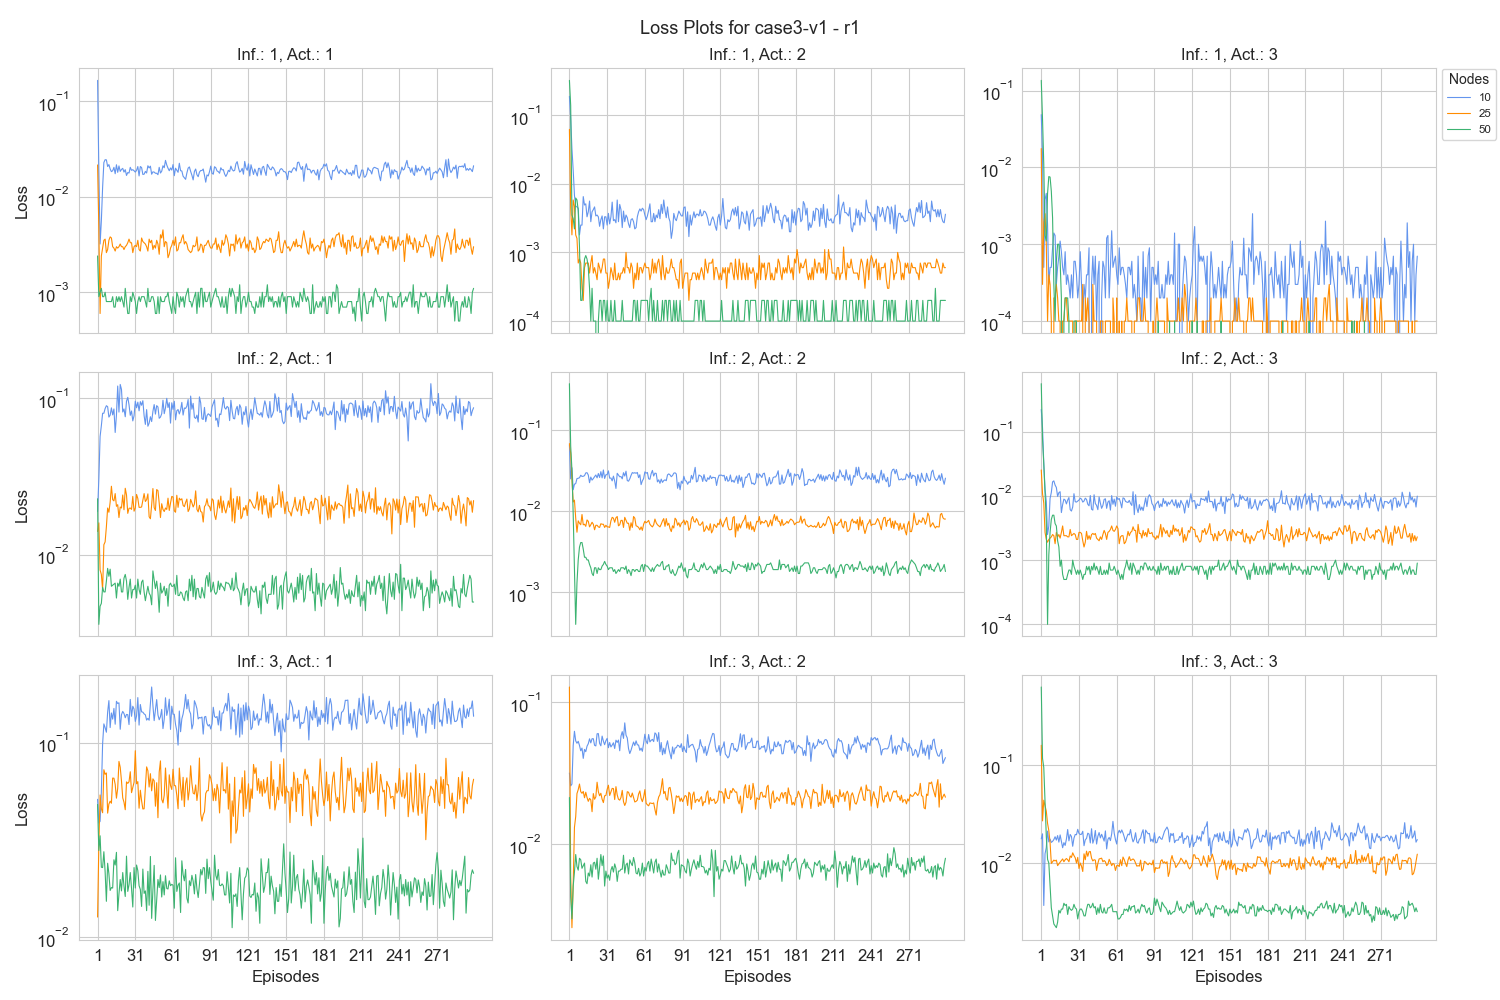}
    \caption{Case-3 v1 using R1: Training MSE loss evolution for RL policy using ResNet model across networks of 10 (blue), 25 (orange), and 50 (green) nodes, for varying initial misinformation sources (Inf.) and action budgets (Act.). Plotted on a logarithmic scale, the loss decreases over episodes, indicating improved policy performance and adaptation across network sizes.}
    \label{fig:resnet_c3v1r1_loss}
\end{figure}

\begin{figure}
    \centering
    \includegraphics[scale=0.34]{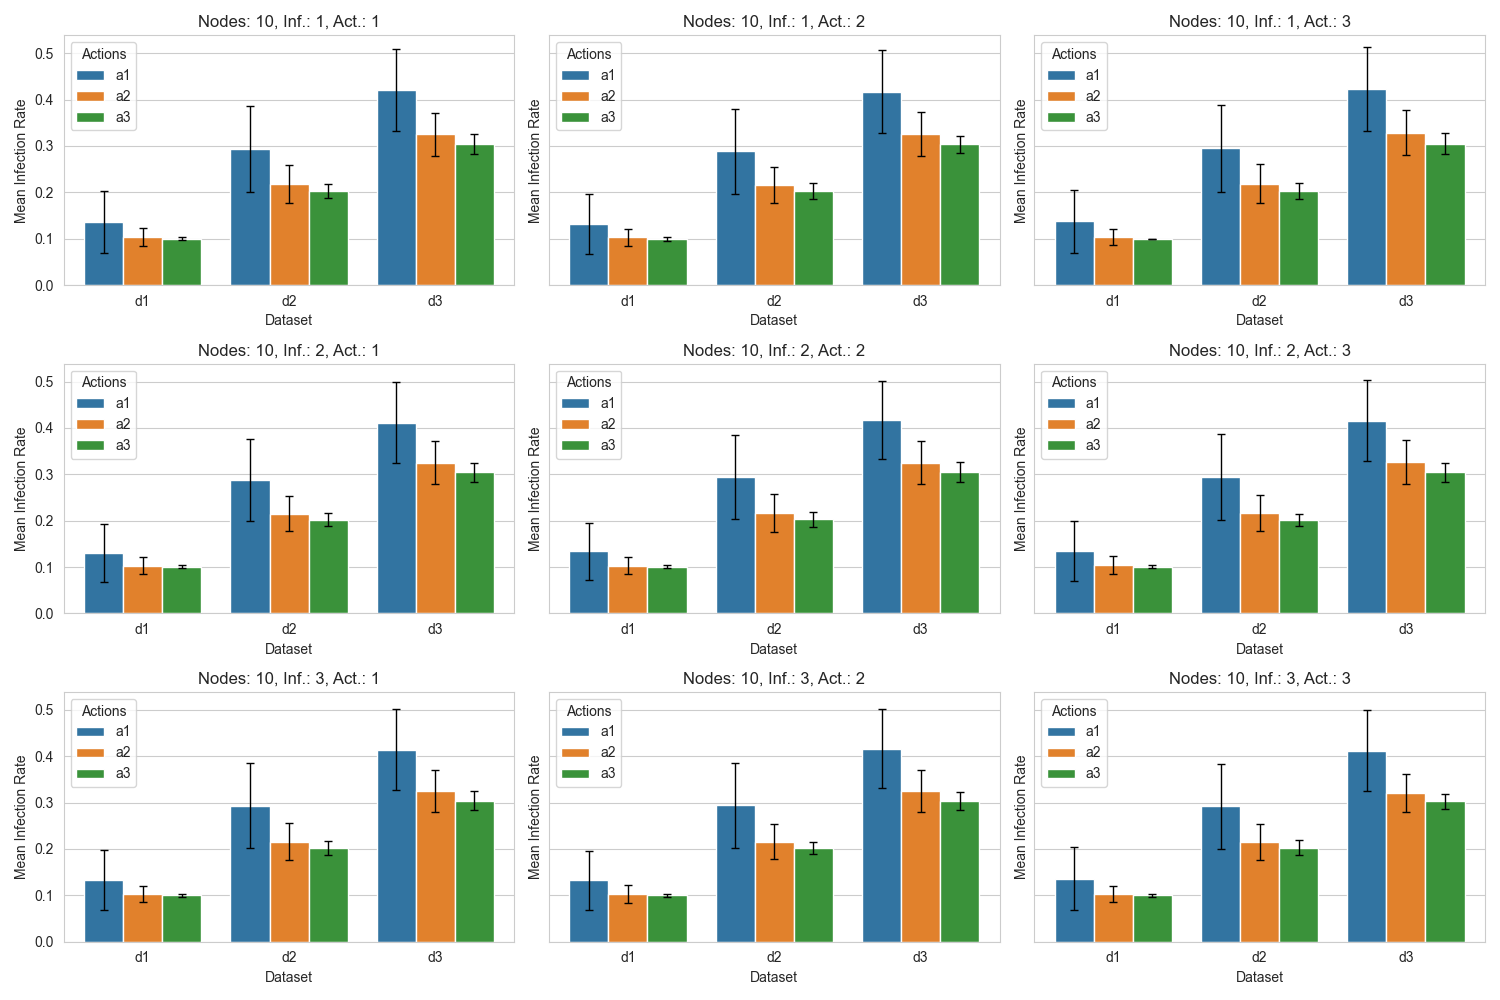}
    \caption{Case-3 v1 using R1: Performance comparison of the RL policies trained using ResNet model for a 10-node network. The barplot displays the mean infection rate for datasets d1, d2, and d3 of Dataset v1 type, differentiated by the number of initial misinformation sources (Inf.) and action budgets (Act.: a1, a2, a3). Each subplot illustrates the performance of a policy trained with the parameters indicated in its title. Lower infection rates indicate more effective policy learning and misinformation containment.}
    \label{fig:inf_resnet_c3v1r1_10}
\end{figure}

\begin{figure}
    \centering
    \includegraphics[scale=0.34]{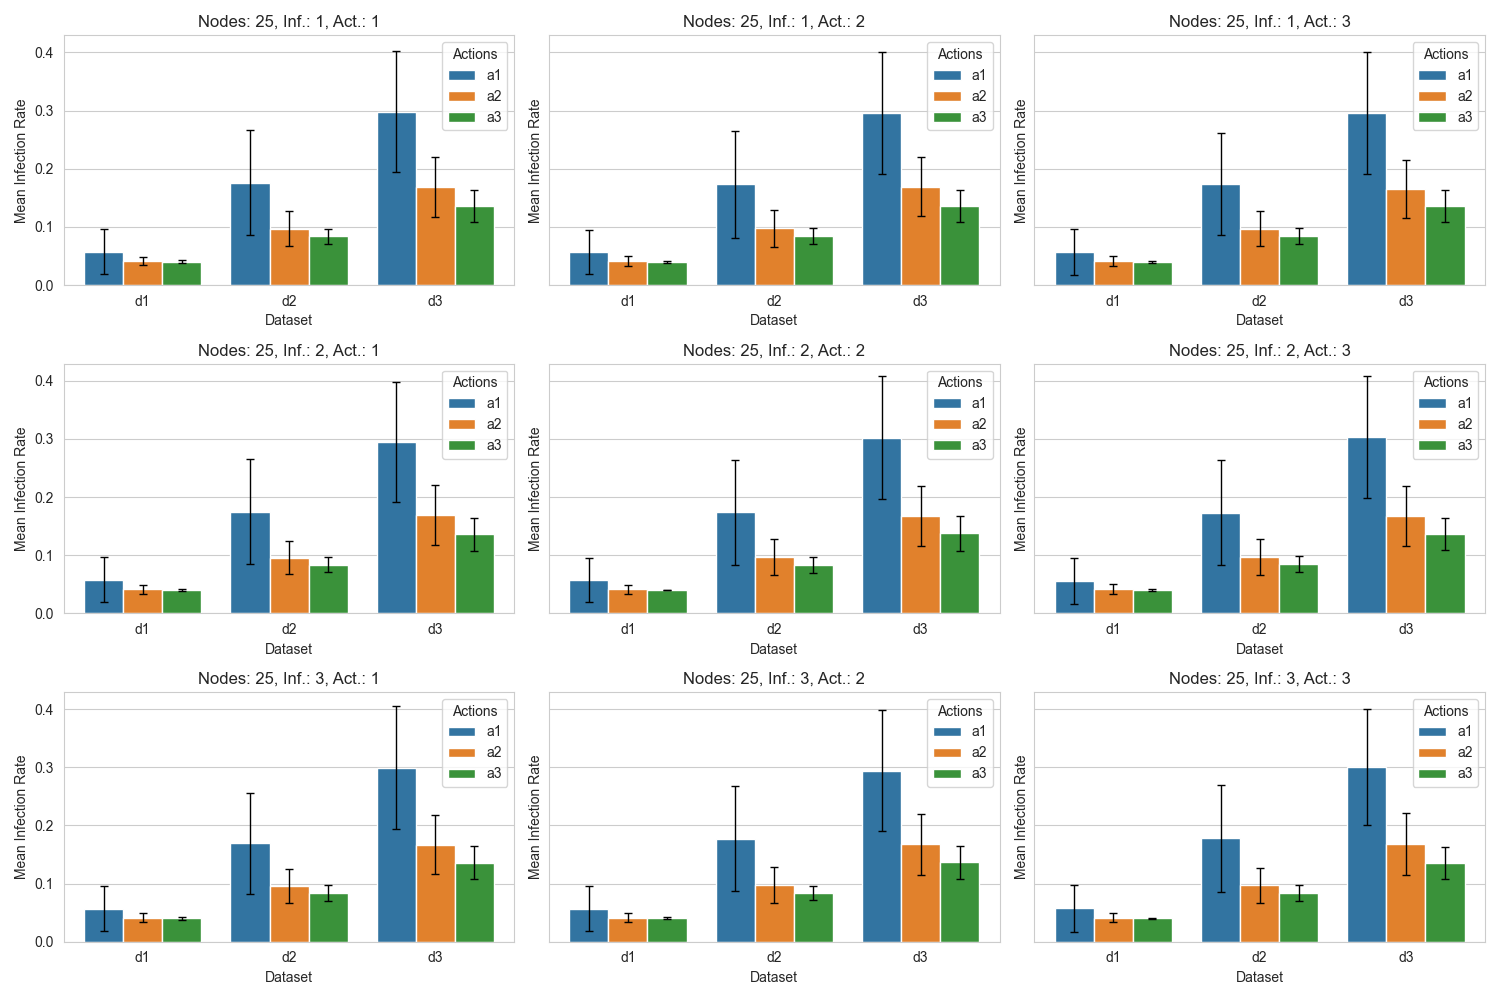}
    \caption{Case-3 v1 using R1: Performance comparison of the RL policies trained using ResNet model for a 25-node network. The barplot displays the mean infection rate for datasets d1, d2, and d3 of Dataset v1 type, differentiated by the number of initial misinformation sources (Inf.) and action budgets (Act.: a1, a2, a3). Each subplot illustrates the performance of a policy trained with the parameters indicated in its title. Lower infection rates indicate more effective policy learning and misinformation containment.}
    \label{fig:inf_resnet_c3v1r1_25}
\end{figure}

\begin{figure}
    \centering
    \includegraphics[scale=0.34]{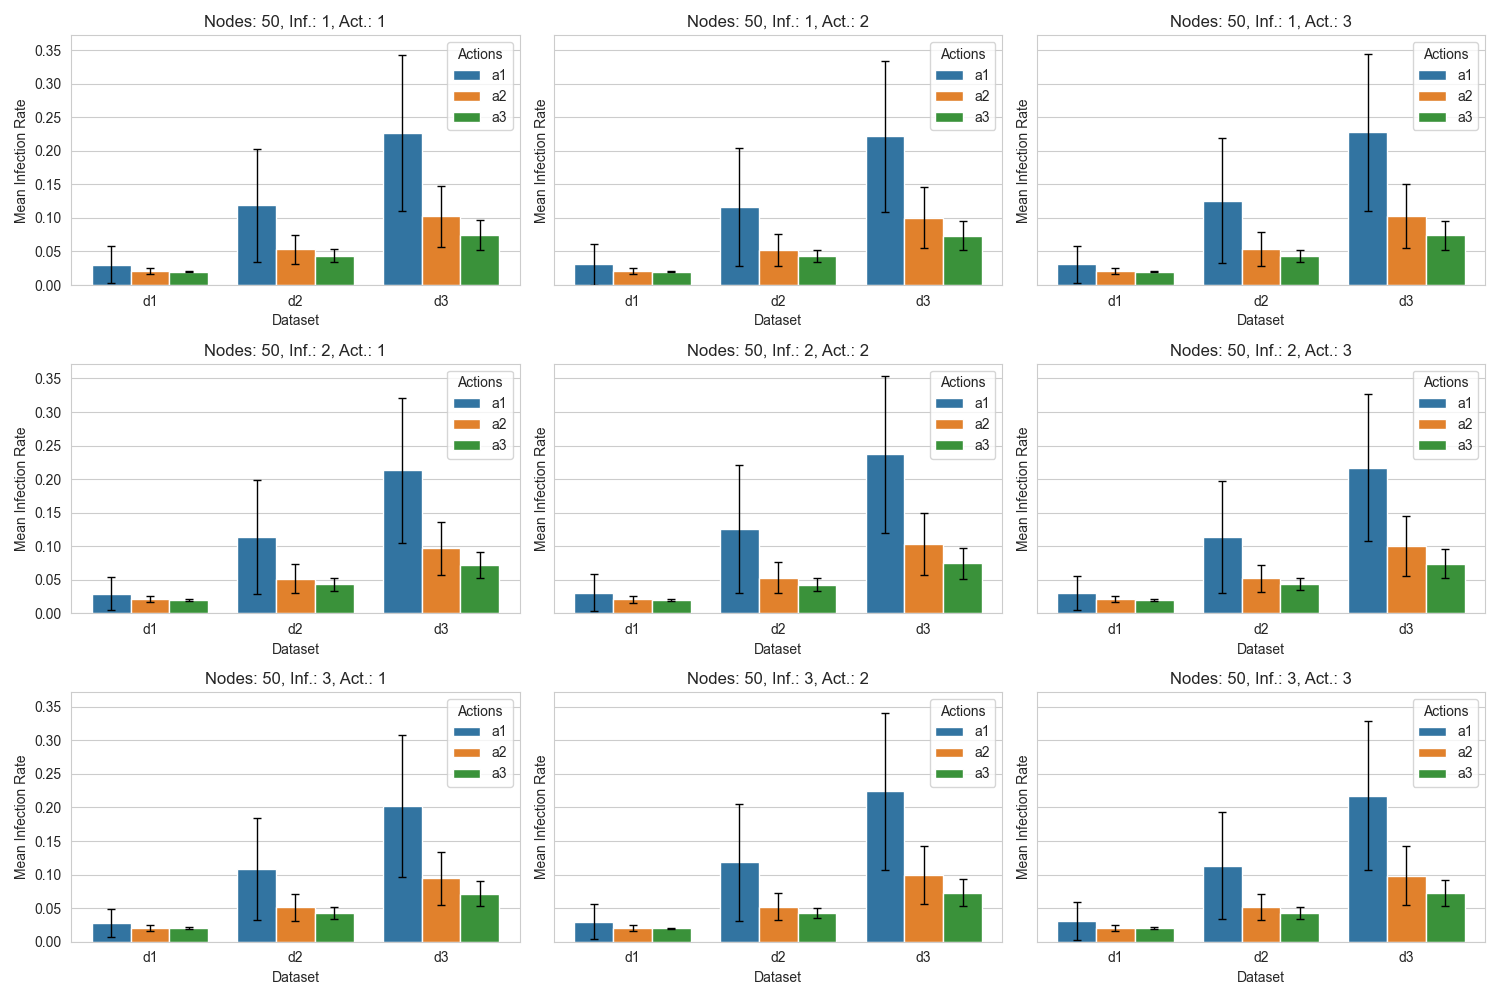}
    \caption{Case-3 v1 using R1: Performance comparison of the RL policies trained using ResNet model for a 50-node network. The barplot displays the mean infection rate for datasets d1, d2, and d3 of Dataset v1 type, differentiated by the number of initial misinformation sources (Inf.) and action budgets (Act.: a1, a2, a3). Each subplot illustrates the performance of a policy trained with the parameters indicated in its title. Lower infection rates indicate more effective policy learning and misinformation containment.}
    \label{fig:inf_resnet_c3v1r1_50}
\end{figure}

%%%%%% R2 %%%%%%%
\begin{figure}[!h]
    \centering
    \includegraphics[scale=0.34]{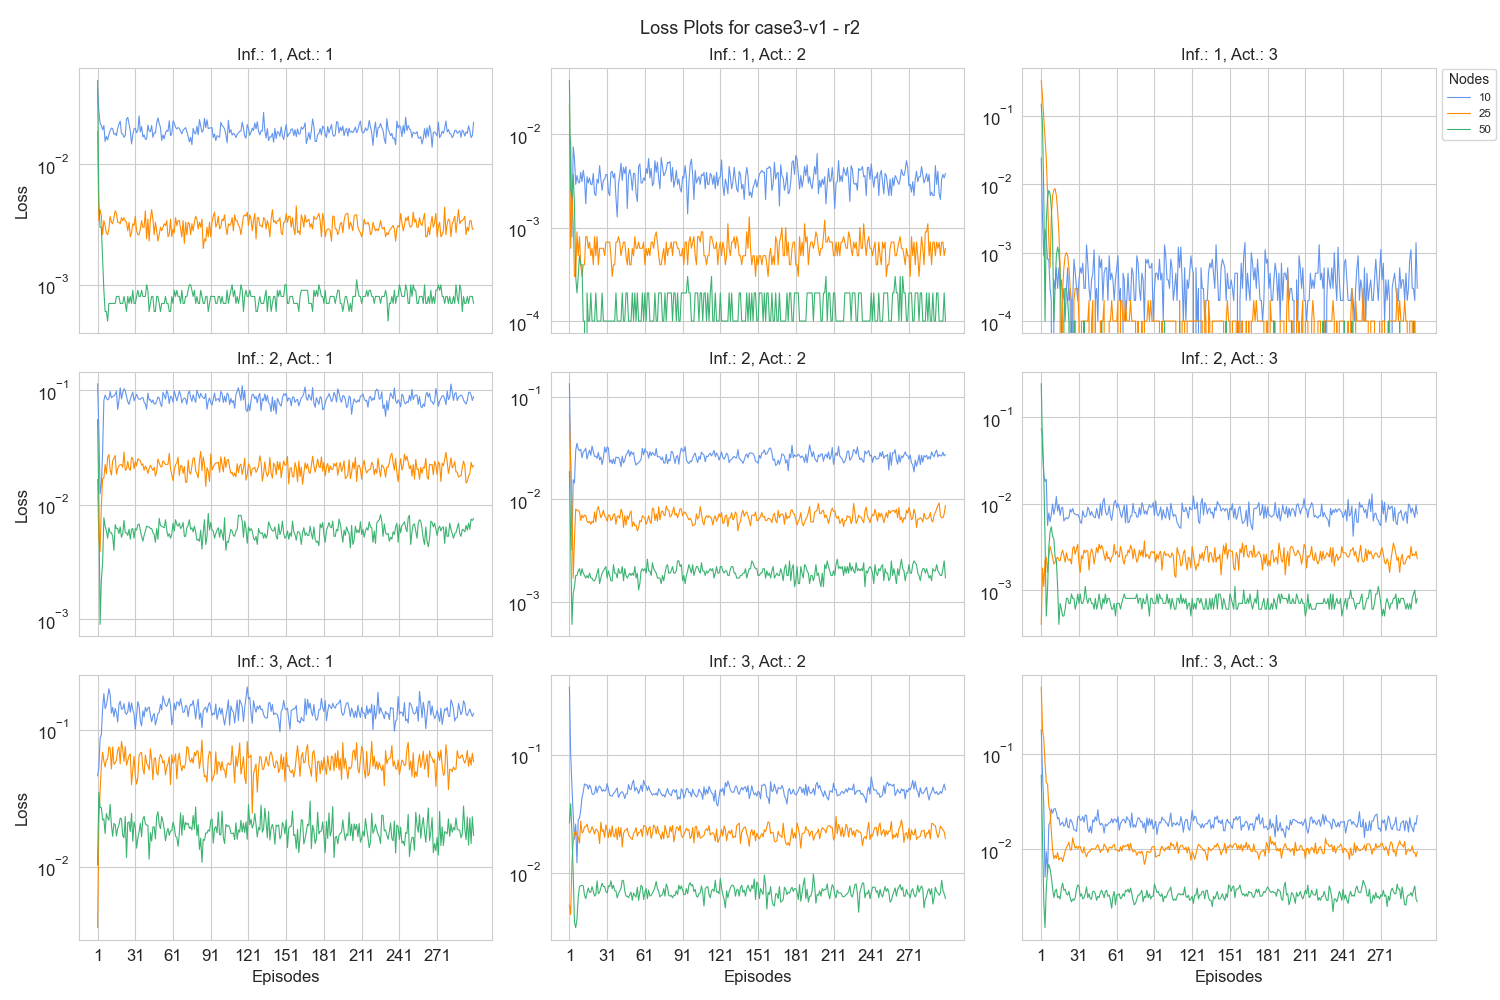}
    \caption{Case-3 v1 using R2: Training MSE loss evolution for RL policy using ResNet model across networks of 10 (blue), 25 (orange), and 50 (green) nodes, for varying initial misinformation sources (Inf.) and action budgets (Act.). Plotted on a logarithmic scale, the loss decreases over episodes, indicating improved policy performance and adaptation across network sizes.}
    \label{fig:resnet_c3v1r2_loss}
\end{figure}

\begin{figure}
    \centering
    \includegraphics[scale=0.34]{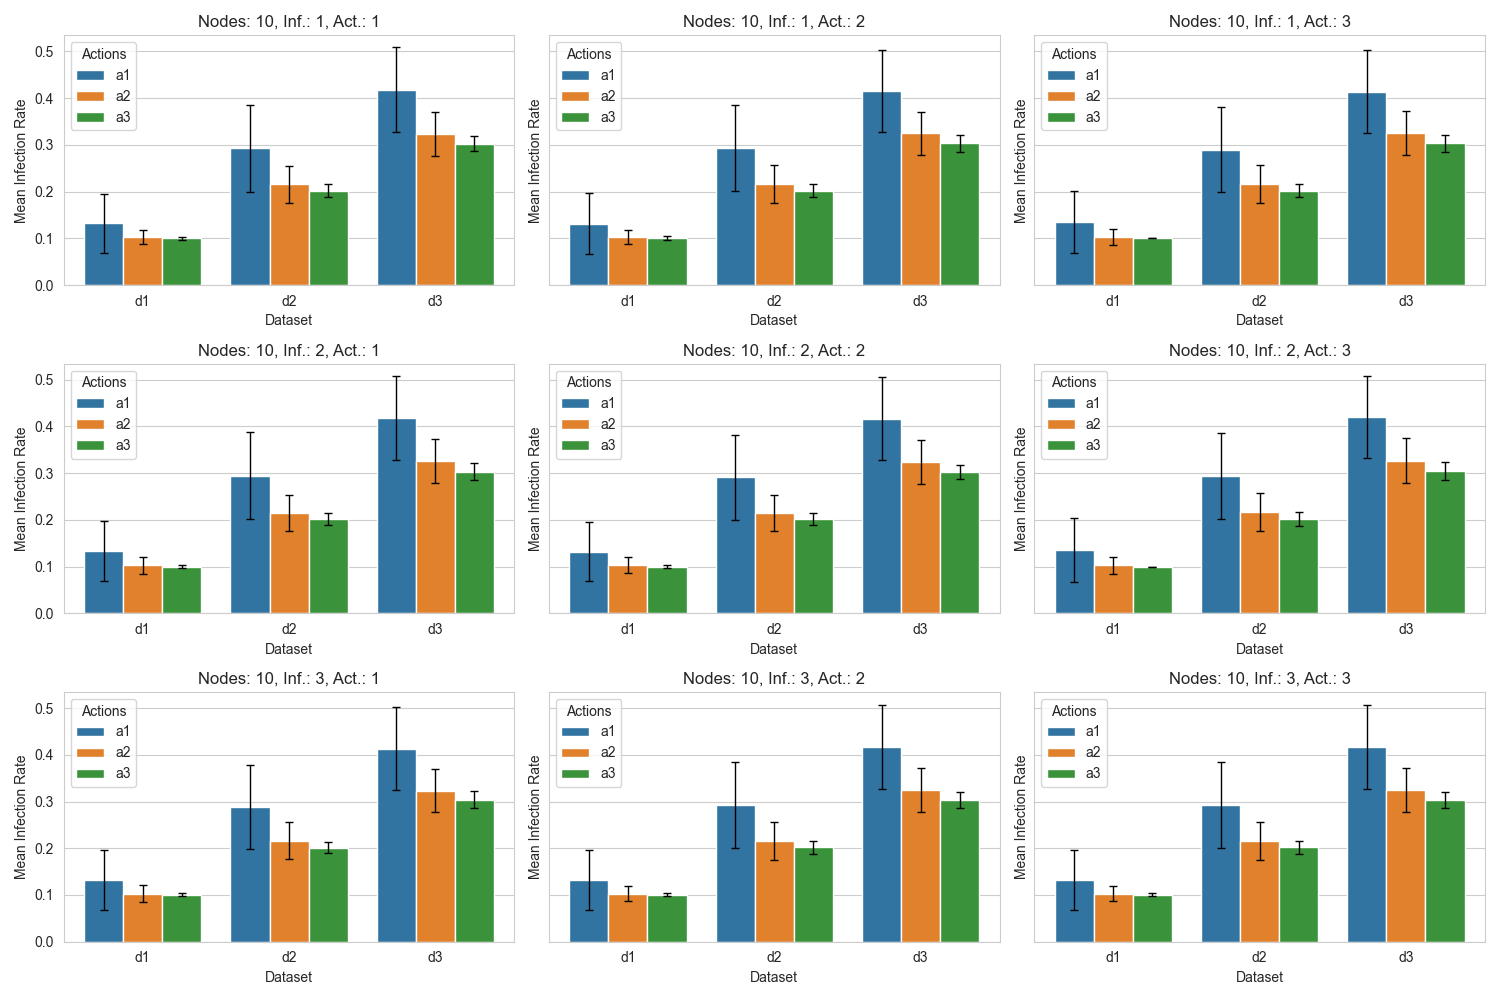}
    \caption{Case-3 v1 using R2: Performance comparison of the RL policies trained using ResNet model for a 10-node network. The barplot displays the mean infection rate for datasets d1, d2, and d3 of Dataset v1 type, differentiated by the number of initial misinformation sources (Inf.) and action budgets (Act.: a1, a2, a3). Each subplot illustrates the performance of a policy trained with the parameters indicated in its title. Lower infection rates indicate more effective policy learning and misinformation containment.}
    \label{fig:inf_resnet_c3v1r2_10}
\end{figure}

\begin{figure}
    \centering
    \includegraphics[scale=0.34]{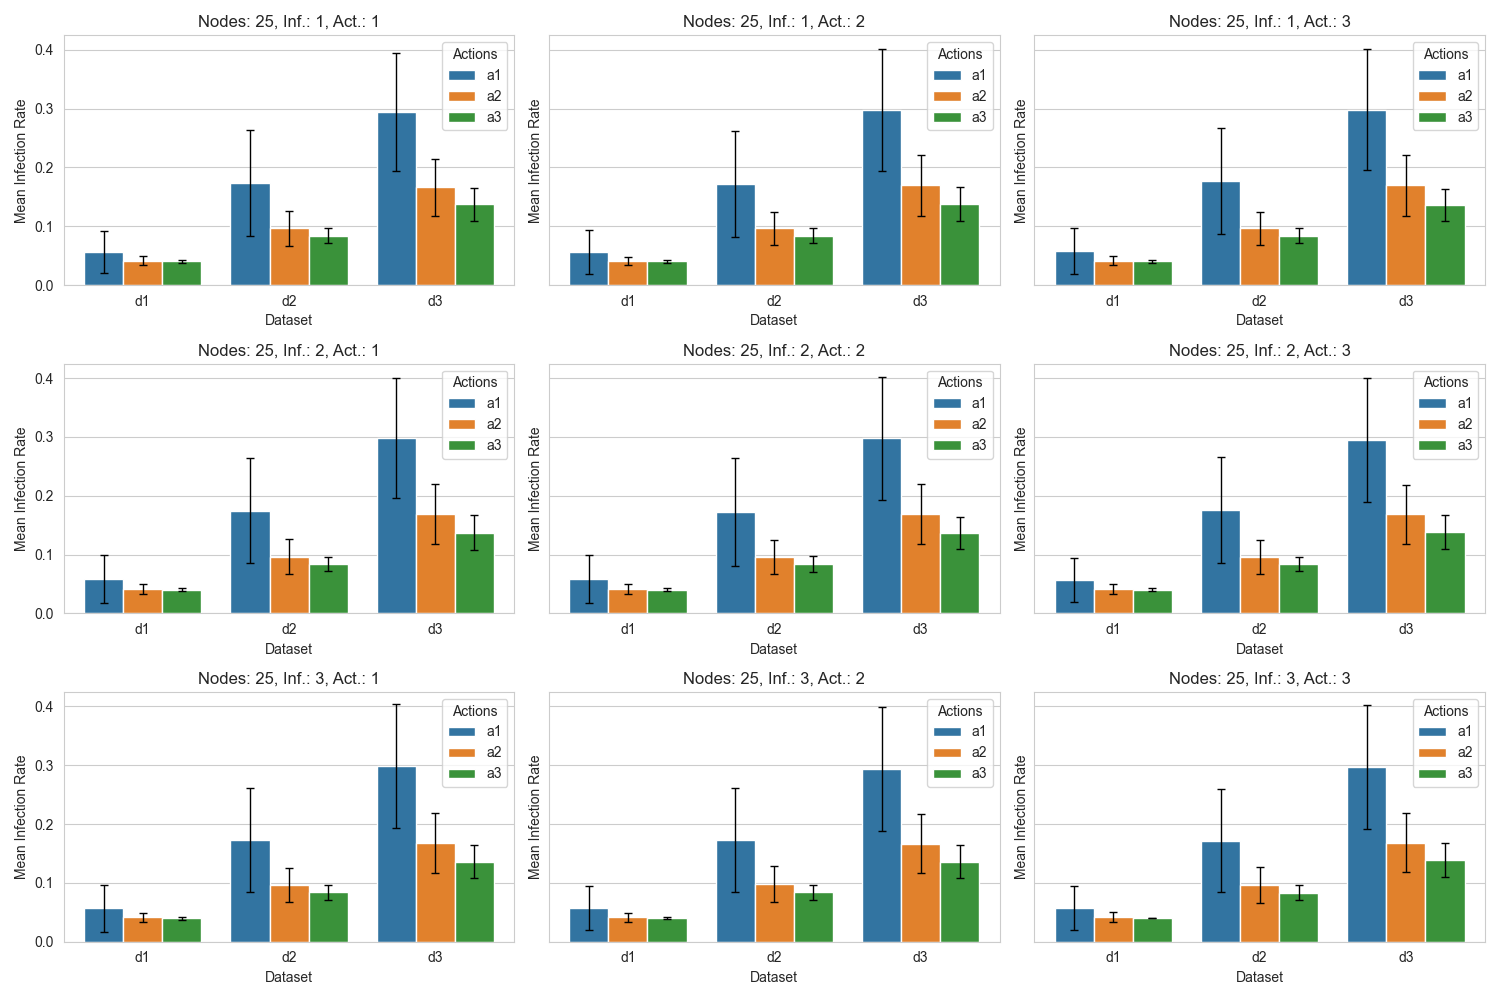}
    \caption{Case-3 v1 using R2: Performance comparison of the RL policies trained using ResNet model for a 25-node network. The barplot displays the mean infection rate for datasets d1, d2, and d3 of Dataset v1 type, differentiated by the number of initial misinformation sources (Inf.) and action budgets (Act.: a1, a2, a3). Each subplot illustrates the performance of a policy trained with the parameters indicated in its title. Lower infection rates indicate more effective policy learning and misinformation containment.}
    \label{fig:inf_resnet_c3v1r2_25}
\end{figure}

\begin{figure}
    \centering
    \includegraphics[scale=0.34]{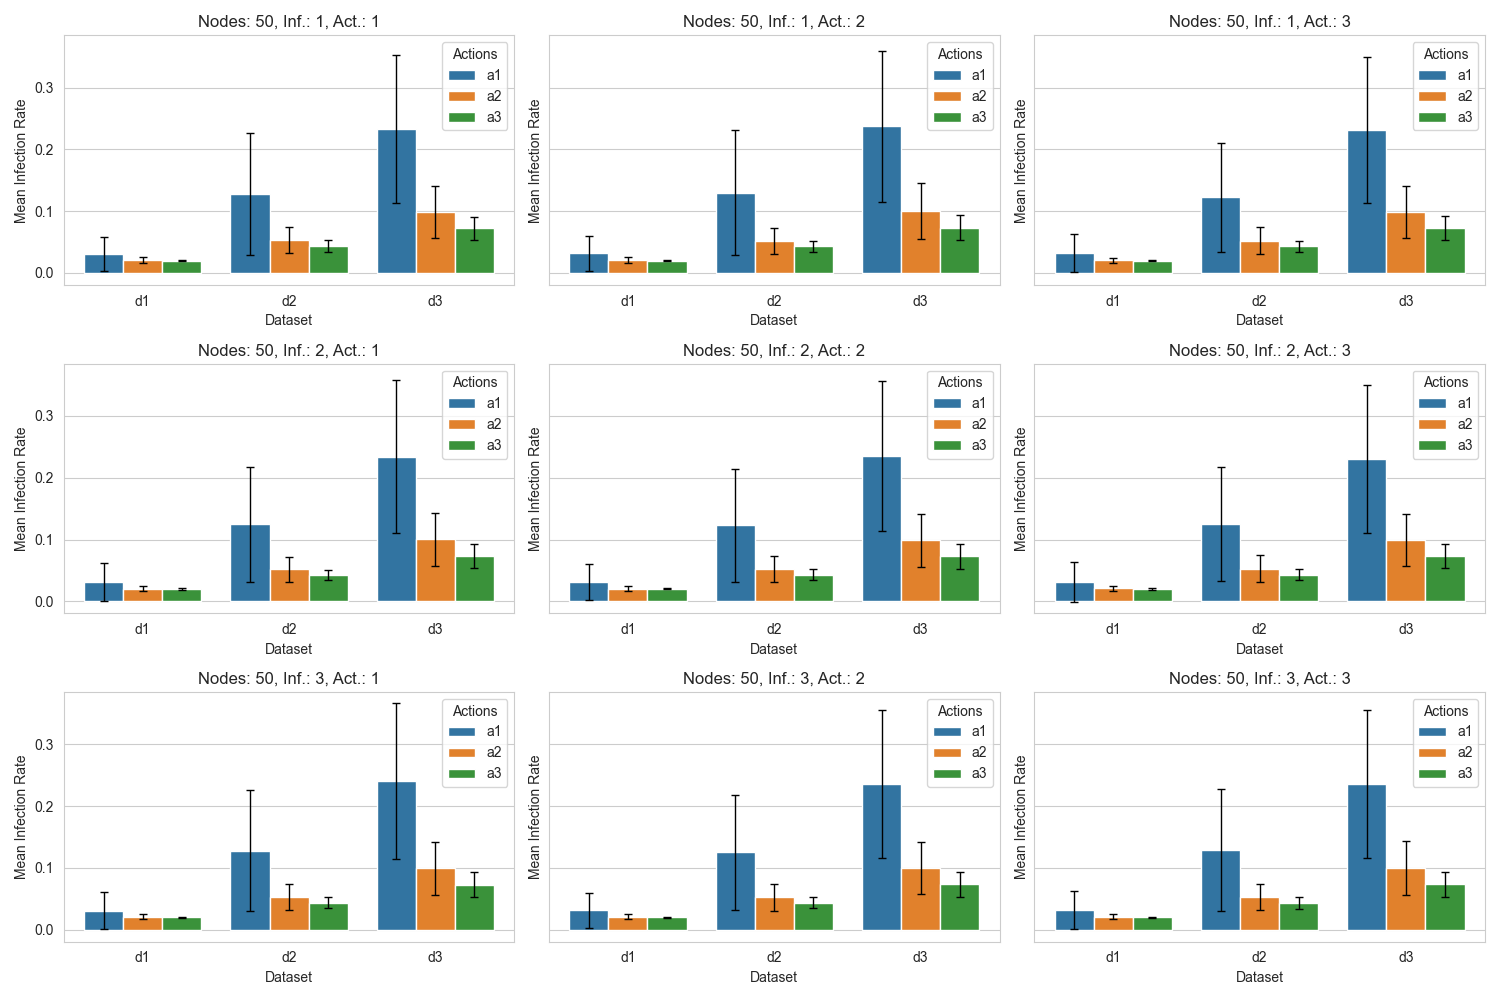}
    \caption{Case-3 v1 using R2: Performance comparison of the RL policies trained using ResNet model for a 50-node network. The barplot displays the mean infection rate for datasets d1, d2, and d3 of Dataset v1 type, differentiated by the number of initial misinformation sources (Inf.) and action budgets (Act.: a1, a2, a3). Each subplot illustrates the performance of a policy trained with the parameters indicated in its title. Lower infection rates indicate more effective policy learning and misinformation containment.}
    \label{fig:inf_resnet_c3v1r2_50}
\end{figure}

%%%%%% R3 %%%%%%%
\begin{figure}[!h]
    \centering
    \includegraphics[scale=0.34]{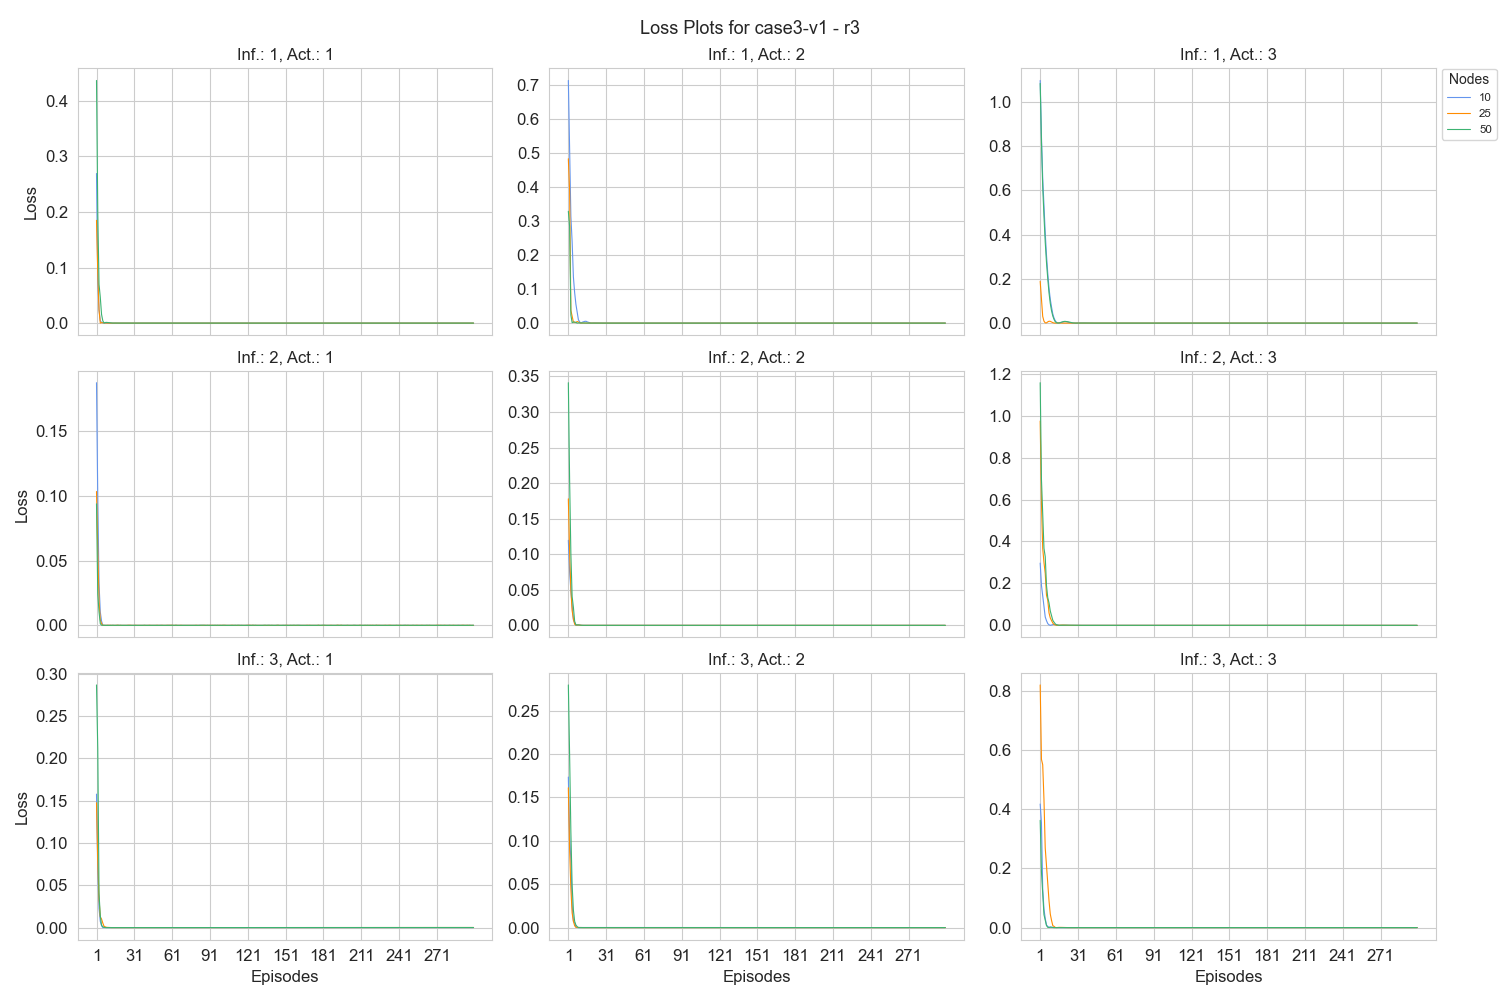}
    \caption{Case-3 v1 using R3: Training MSE loss evolution for RL policy using ResNet model across networks of 10 (blue), 25 (orange), and 50 (green) nodes, for varying initial misinformation sources (Inf.) and action budgets (Act.). The loss decreases over episodes, indicating improved policy performance and adaptation across network sizes.}
    \label{fig:resnet_c3v1r3_loss}
\end{figure}

\begin{figure}
    \centering
    \includegraphics[scale=0.34]{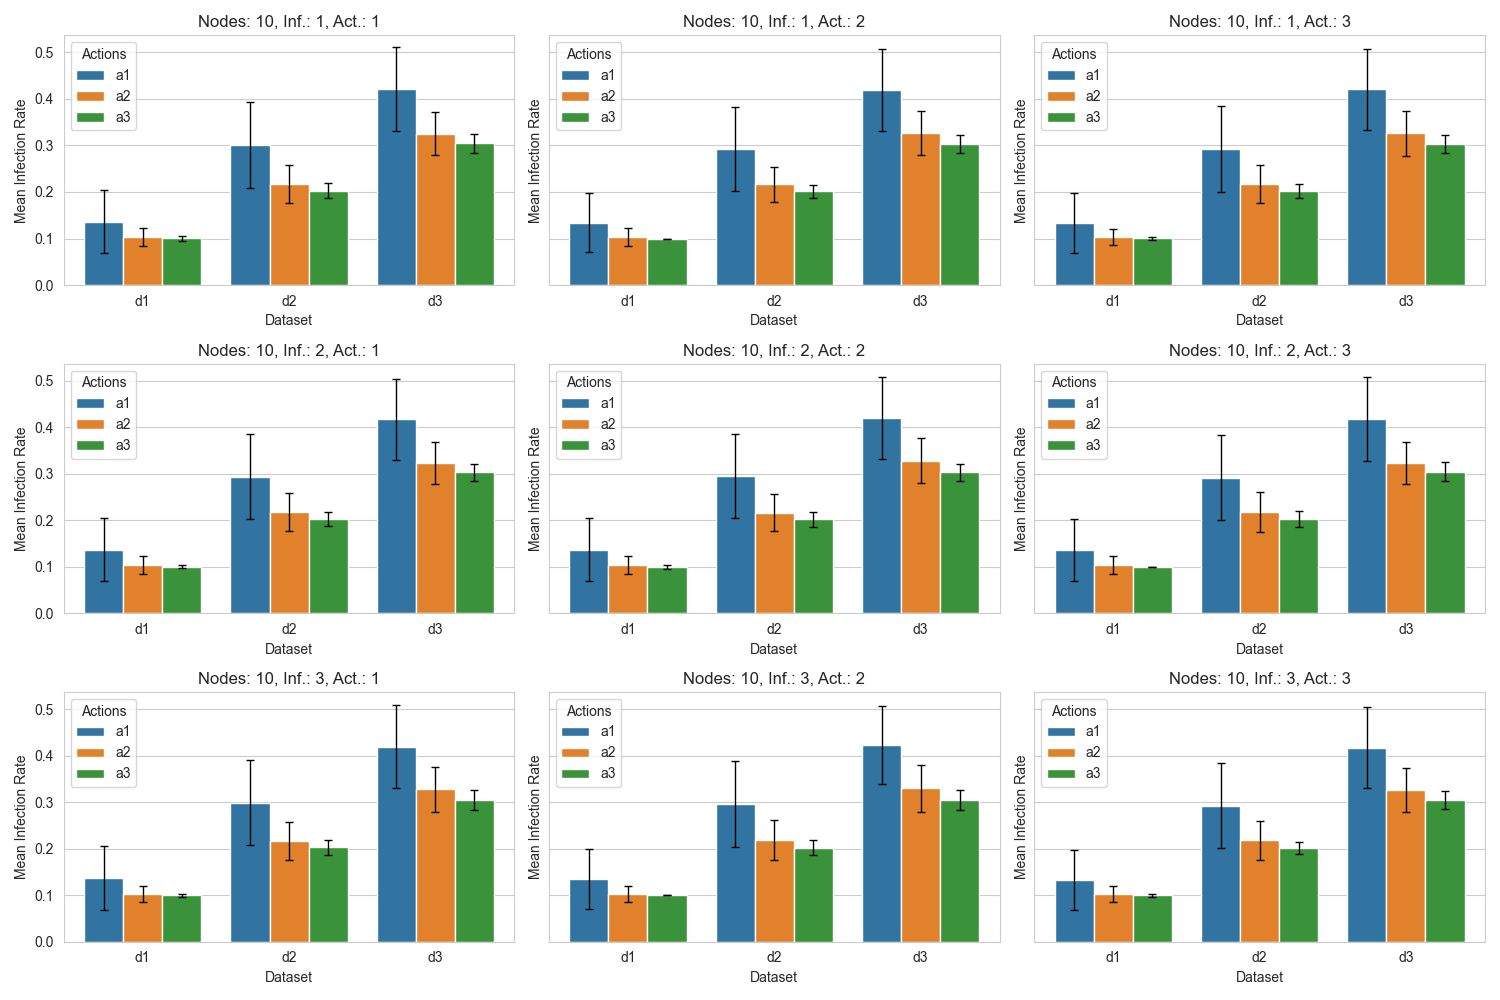}
    \caption{Case-3 v1 using R3: Performance comparison of the RL policies trained using ResNet model for a 10-node network. The barplot displays the mean infection rate for datasets d1, d2, and d3 of Dataset v1 type, differentiated by the number of initial misinformation sources (Inf.) and action budgets (Act.: a1, a2, a3). Each subplot illustrates the performance of a policy trained with the parameters indicated in its title. Lower infection rates indicate more effective policy learning and misinformation containment.}
    \label{fig:inf_resnet_c3v1r3_10}
\end{figure}

\begin{figure}
    \centering
    \includegraphics[scale=0.34]{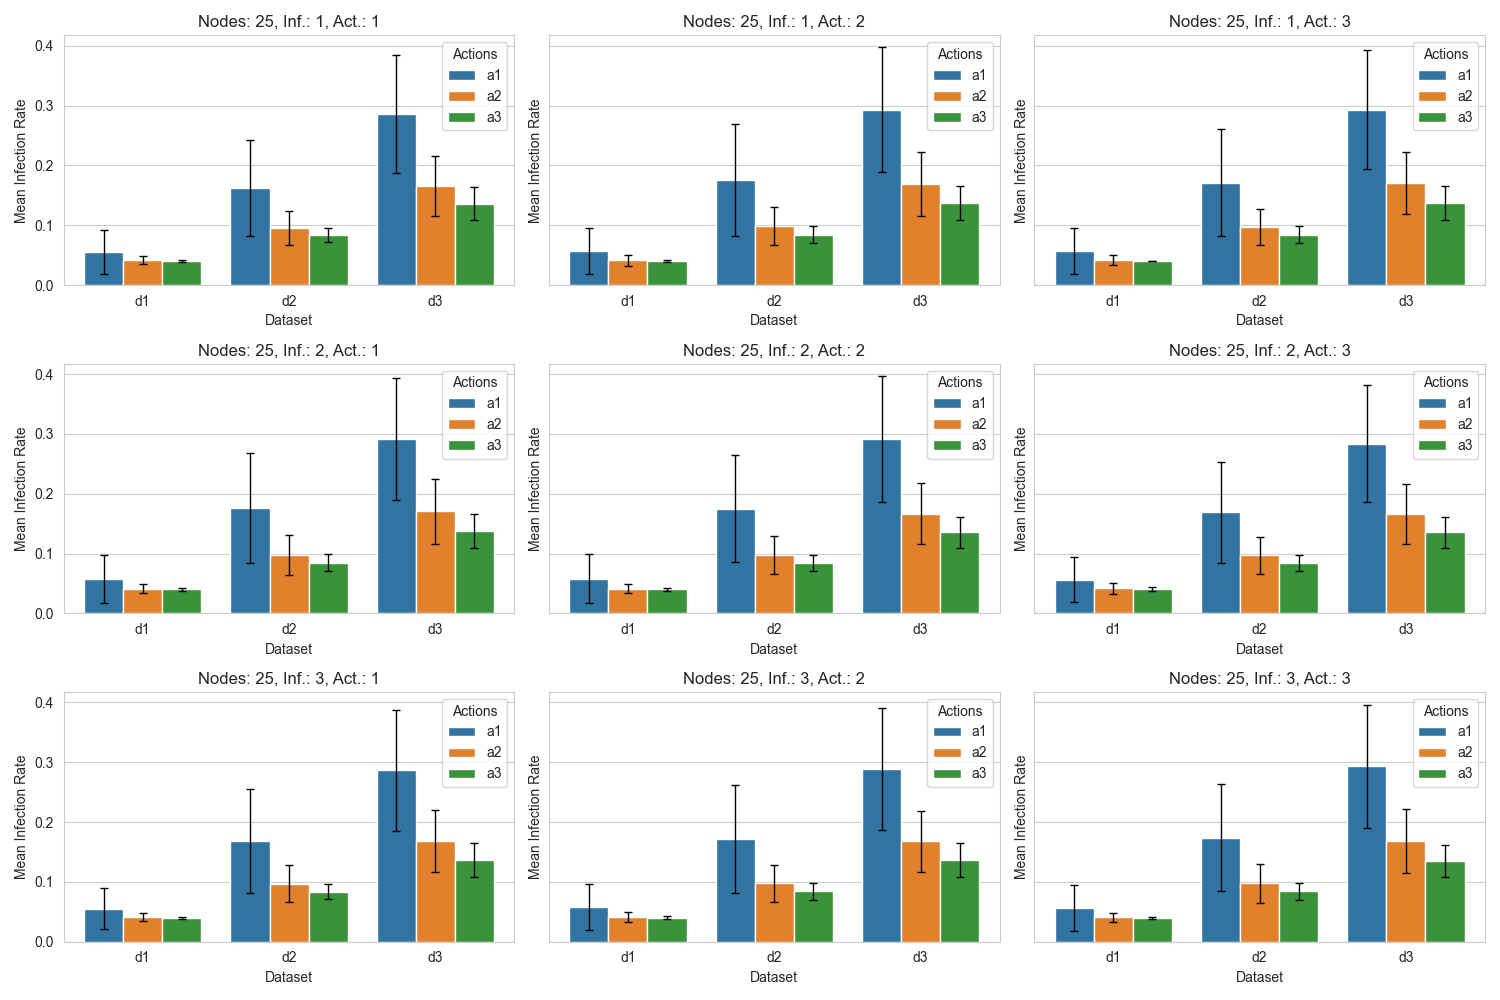}
    \caption{Case-3 v1 using R3: Performance comparison of the RL policies trained using ResNet model for a 25-node network. The barplot displays the mean infection rate for datasets d1, d2, and d3 of Dataset v1 type, differentiated by the number of initial misinformation sources (Inf.) and action budgets (Act.: a1, a2, a3). Each subplot illustrates the performance of a policy trained with the parameters indicated in its title. Lower infection rates indicate more effective policy learning and misinformation containment.}
    \label{fig:inf_resnet_c3v1r3_25}
\end{figure}

\begin{figure}
    \centering
    \includegraphics[scale=0.34]{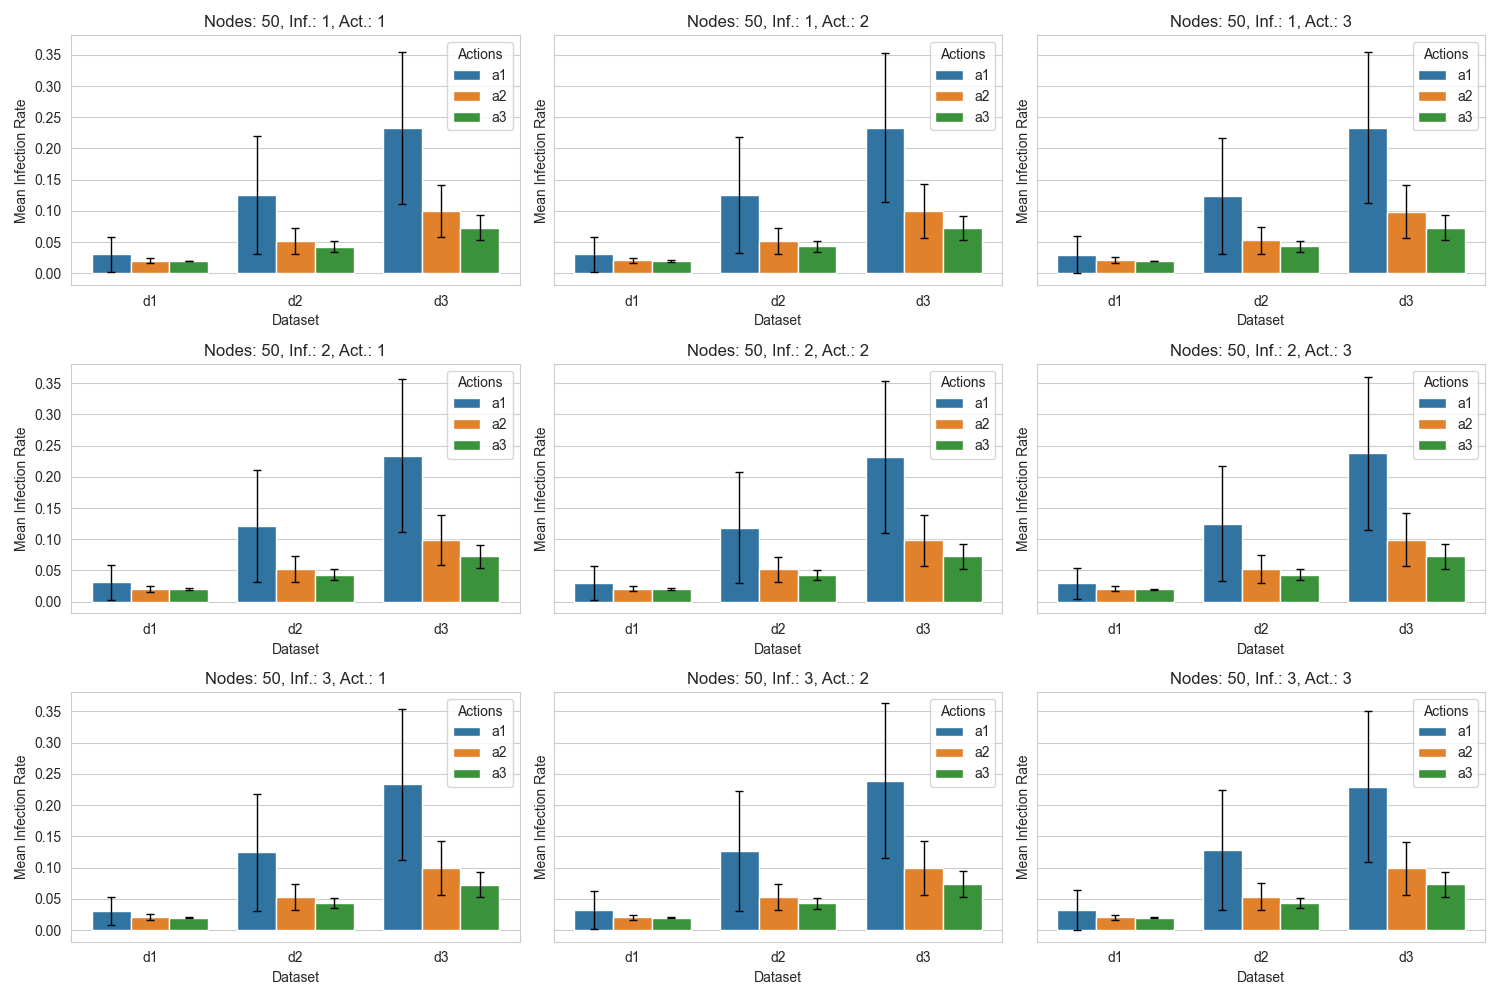}
    \caption{Case-3 v1 using R3: Performance comparison of the RL policies trained using ResNet model for a 50-node network. The barplot displays the mean infection rate for datasets d1, d2, and d3 of Dataset v1 type, differentiated by the number of initial misinformation sources (Inf.) and action budgets (Act.: a1, a2, a3). Each subplot illustrates the performance of a policy trained with the parameters indicated in its title. Lower infection rates indicate more effective policy learning and misinformation containment.}
    \label{fig:inf_resnet_c3v1r3_50}
\end{figure}

%%%%%% R4 %%%%%%%
\begin{figure}[!h]
    \centering
    \includegraphics[scale=0.34]{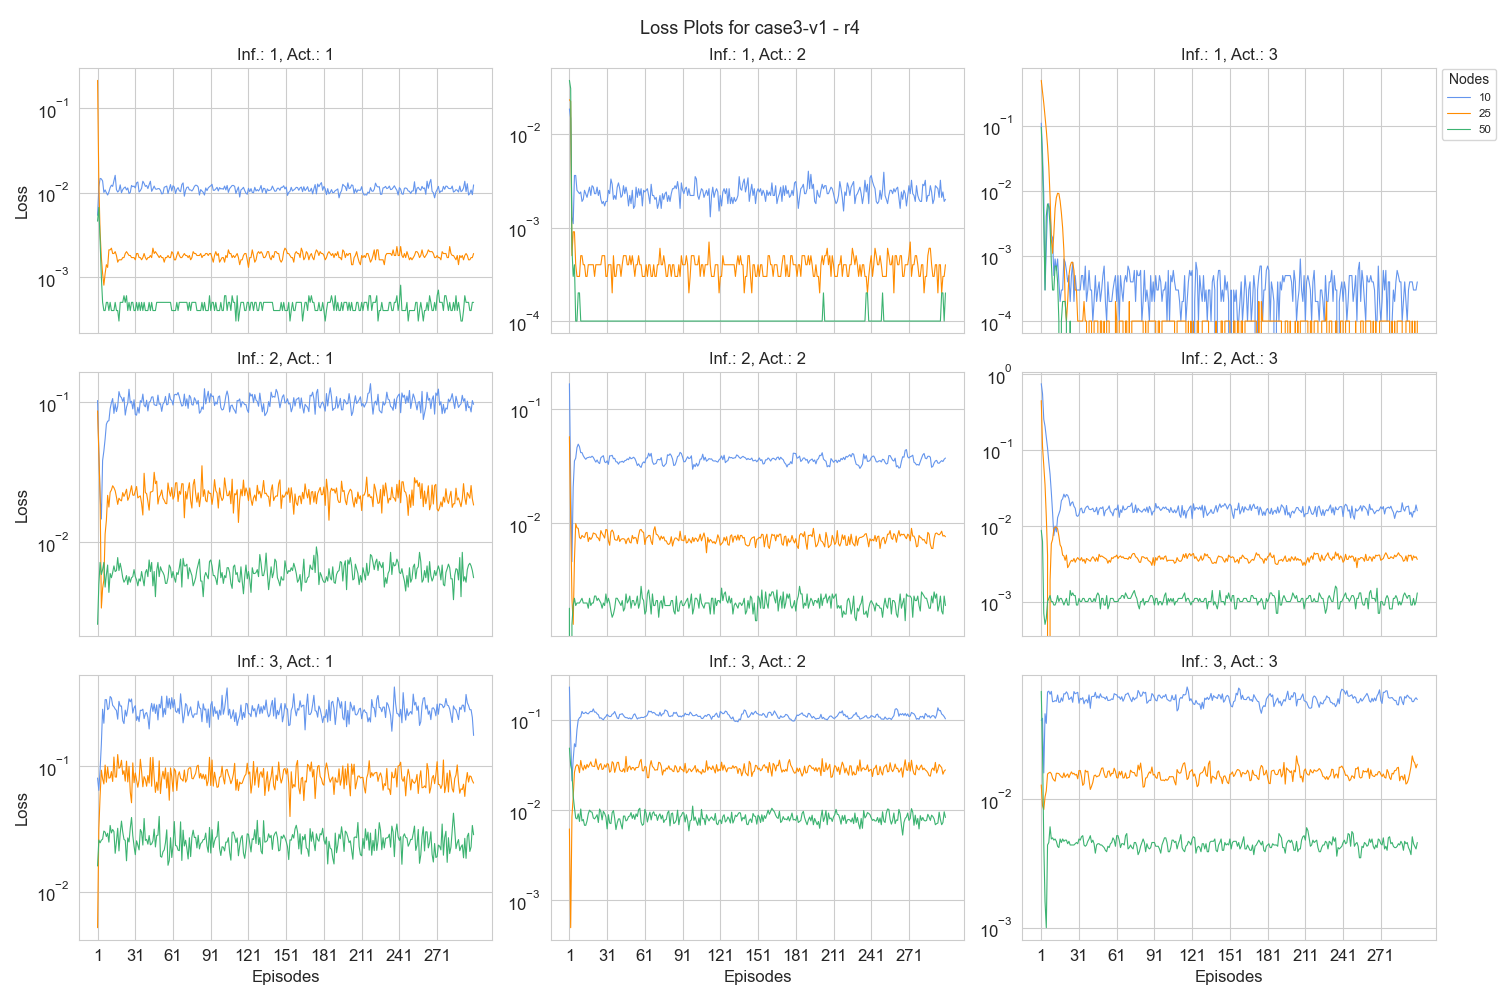}
    \caption{Case-3 v1 using R4: Training MSE loss evolution for RL policy using ResNet model across networks of 10 (blue), 25 (orange), and 50 (green) nodes, for varying initial misinformation sources (Inf.) and action budgets (Act.). Plotted on a logarithmic scale, the loss decreases over episodes, indicating improved policy performance and adaptation across network sizes.}
    \label{fig:resnet_c3v1r4_loss}
\end{figure}

\begin{figure}
    \centering
    \includegraphics[scale=0.34]{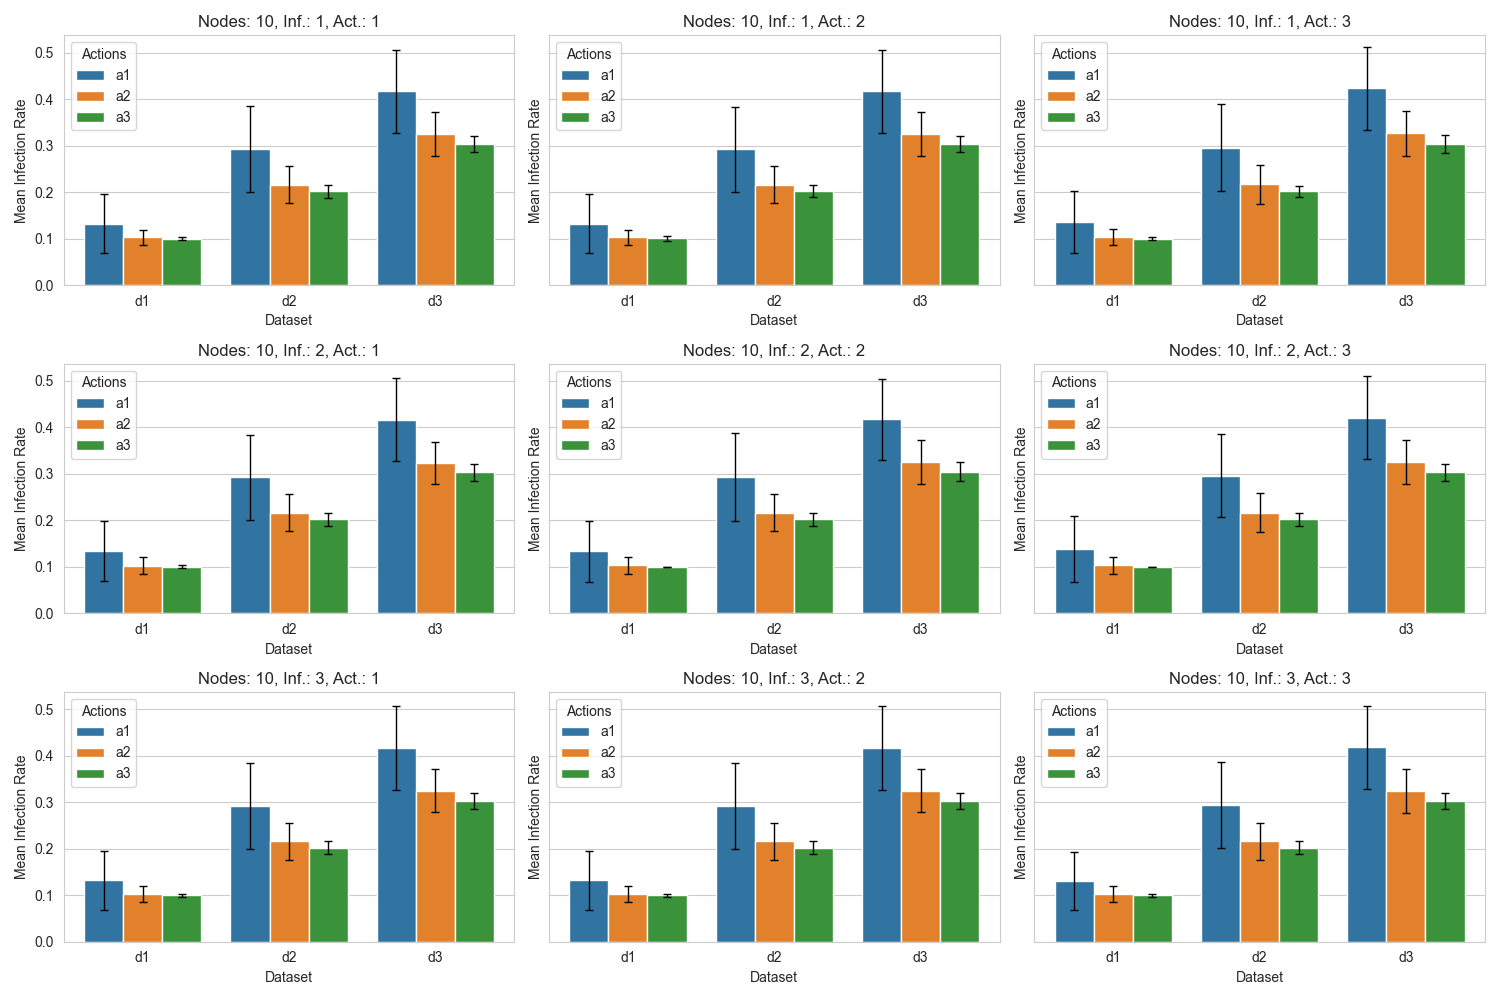}
    \caption{Case-3 v1 using R4: Performance comparison of the RL policies trained using ResNet model for a 10-node network. The barplot displays the mean infection rate for datasets d1, d2, and d3 of Dataset v1 type, differentiated by the number of initial misinformation sources (Inf.) and action budgets (Act.: a1, a2, a3). Each subplot illustrates the performance of a policy trained with the parameters indicated in its title. Lower infection rates indicate more effective policy learning and misinformation containment.}
    \label{fig:inf_resnet_c3v1r4_10}
\end{figure}

\begin{figure}
    \centering
    \includegraphics[scale=0.34]{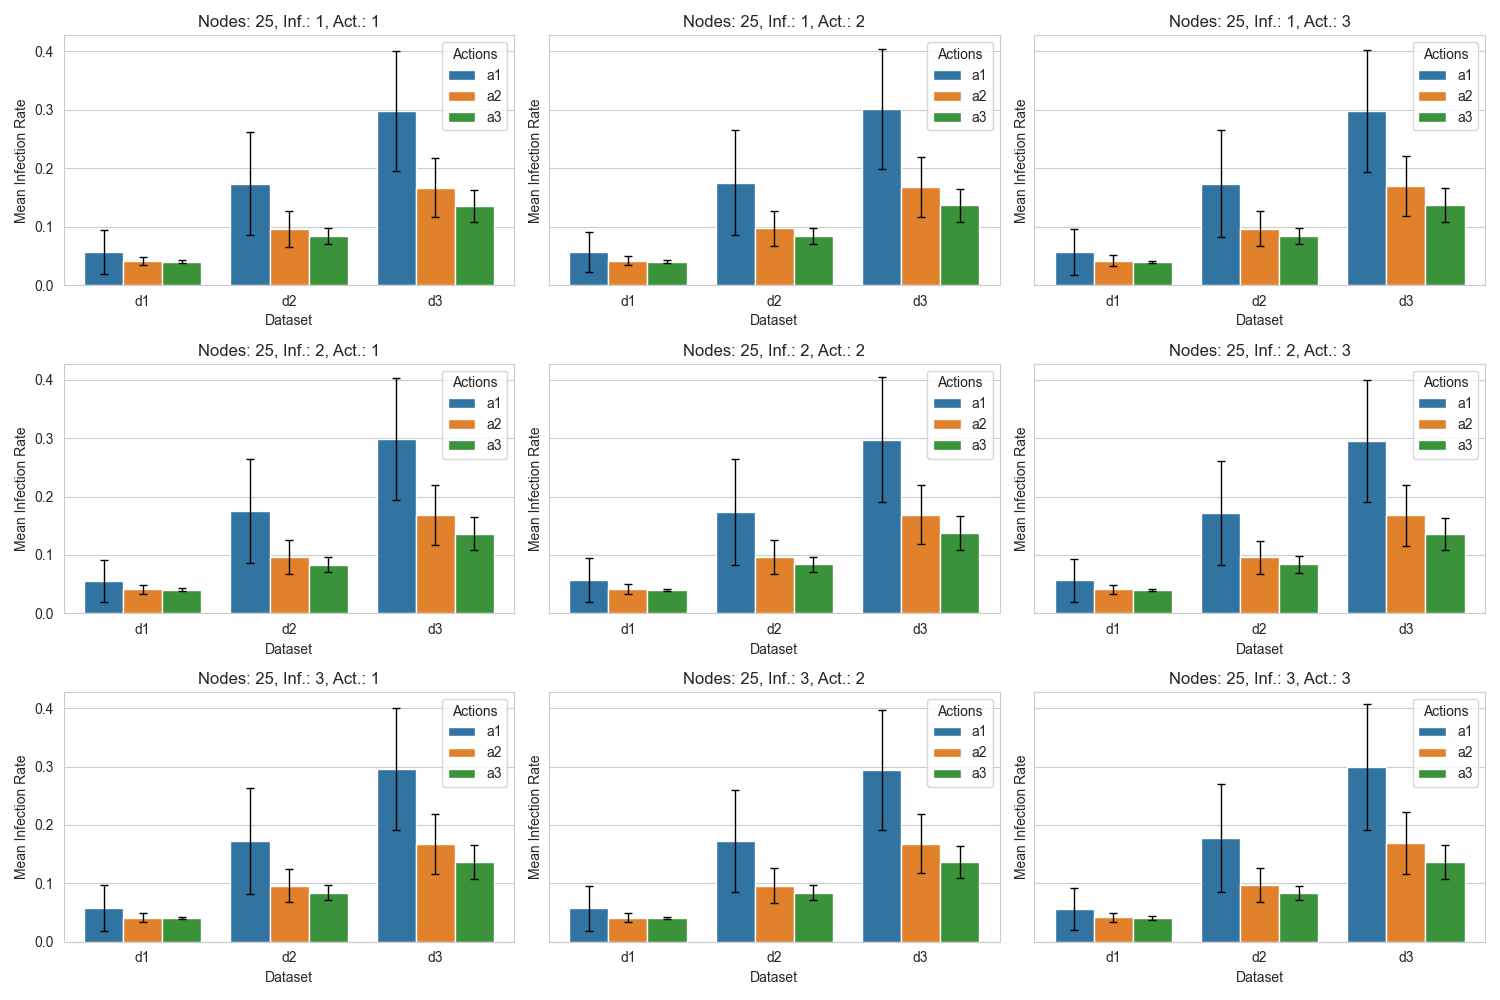}
    \caption{Case-3 v1 using R4: Performance comparison of the RL policies trained using ResNet model for a 25-node network. The barplot displays the mean infection rate for datasets d1, d2, and d3 of Dataset v1 type, differentiated by the number of initial misinformation sources (Inf.) and action budgets (Act.: a1, a2, a3). Each subplot illustrates the performance of a policy trained with the parameters indicated in its title. Lower infection rates indicate more effective policy learning and misinformation containment.}
    \label{fig:inf_resnet_c3v1r4_25}
\end{figure}

\begin{figure}
    \centering
    \includegraphics[scale=0.34]{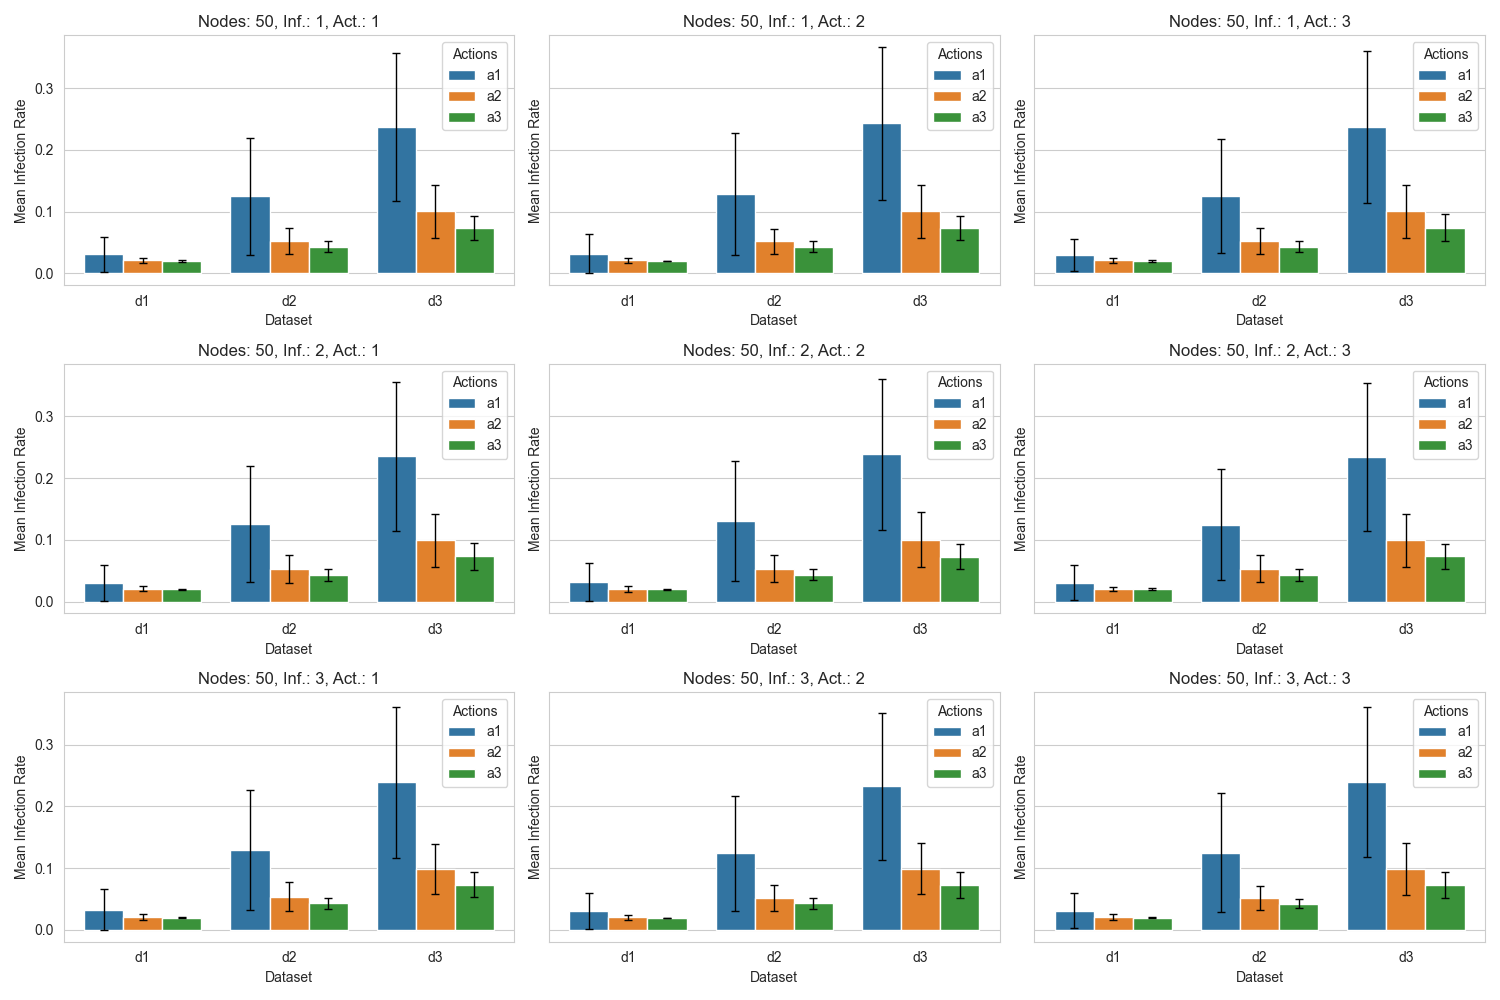}
    \caption{Case-3 v1 using R4: Performance comparison of the RL policies trained using ResNet model for a 50-node network. The barplot displays the mean infection rate for datasets d1, d2, and d3 of Dataset v1 type, differentiated by the number of initial misinformation sources (Inf.) and action budgets (Act.: a1, a2, a3). Each subplot illustrates the performance of a policy trained with the parameters indicated in its title. Lower infection rates indicate more effective policy learning and misinformation containment.}
    \label{fig:inf_resnet_c3v1r4_50}
\end{figure}

% #############################################

% ##################### GCN Figures ######################

%###### Case 1 GCN Figures #######
\begin{figure}[!h]
    \centering
    \includegraphics[scale=0.34]{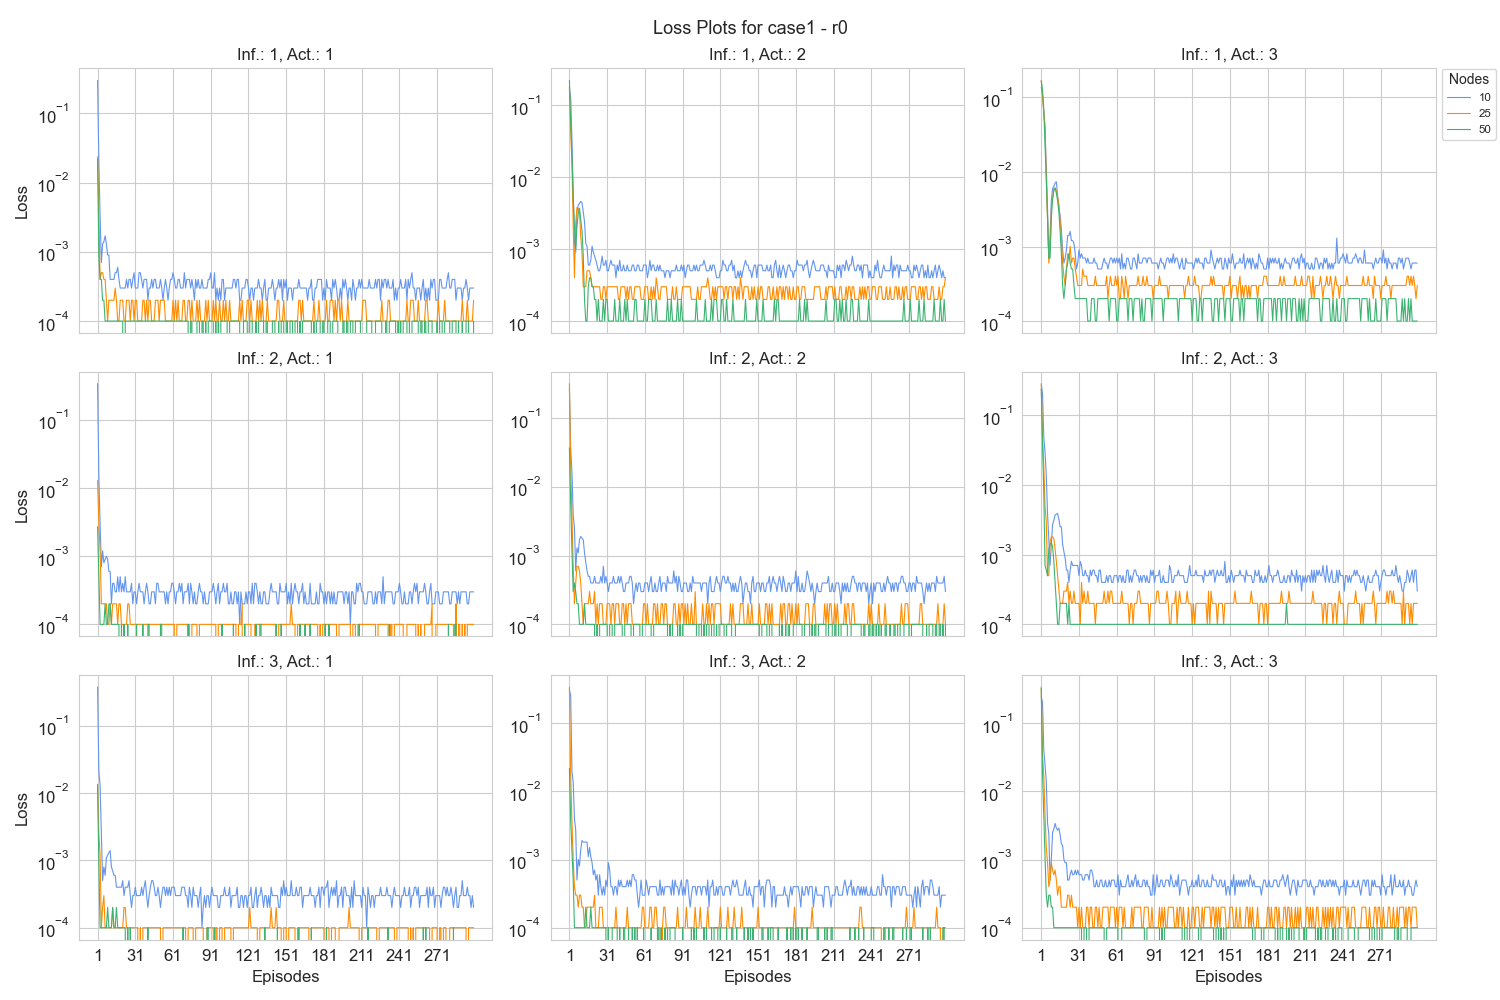}
    \caption{Case-1 using R0: Training MSE loss evolution for RL policy using GCN model across networks of 10 (blue), 25 (orange), and 50 (green) nodes, for varying initial misinformation sources (Inf.) and action budgets (Act.). Plotted on a logarithmic scale, the loss decreases over episodes, indicating improved policy performance and adaptation across network sizes.}
    \label{fig:gcn_c1r0_loss}
\end{figure}

\begin{figure}[!h]
    \centering
    \includegraphics[scale=0.34]{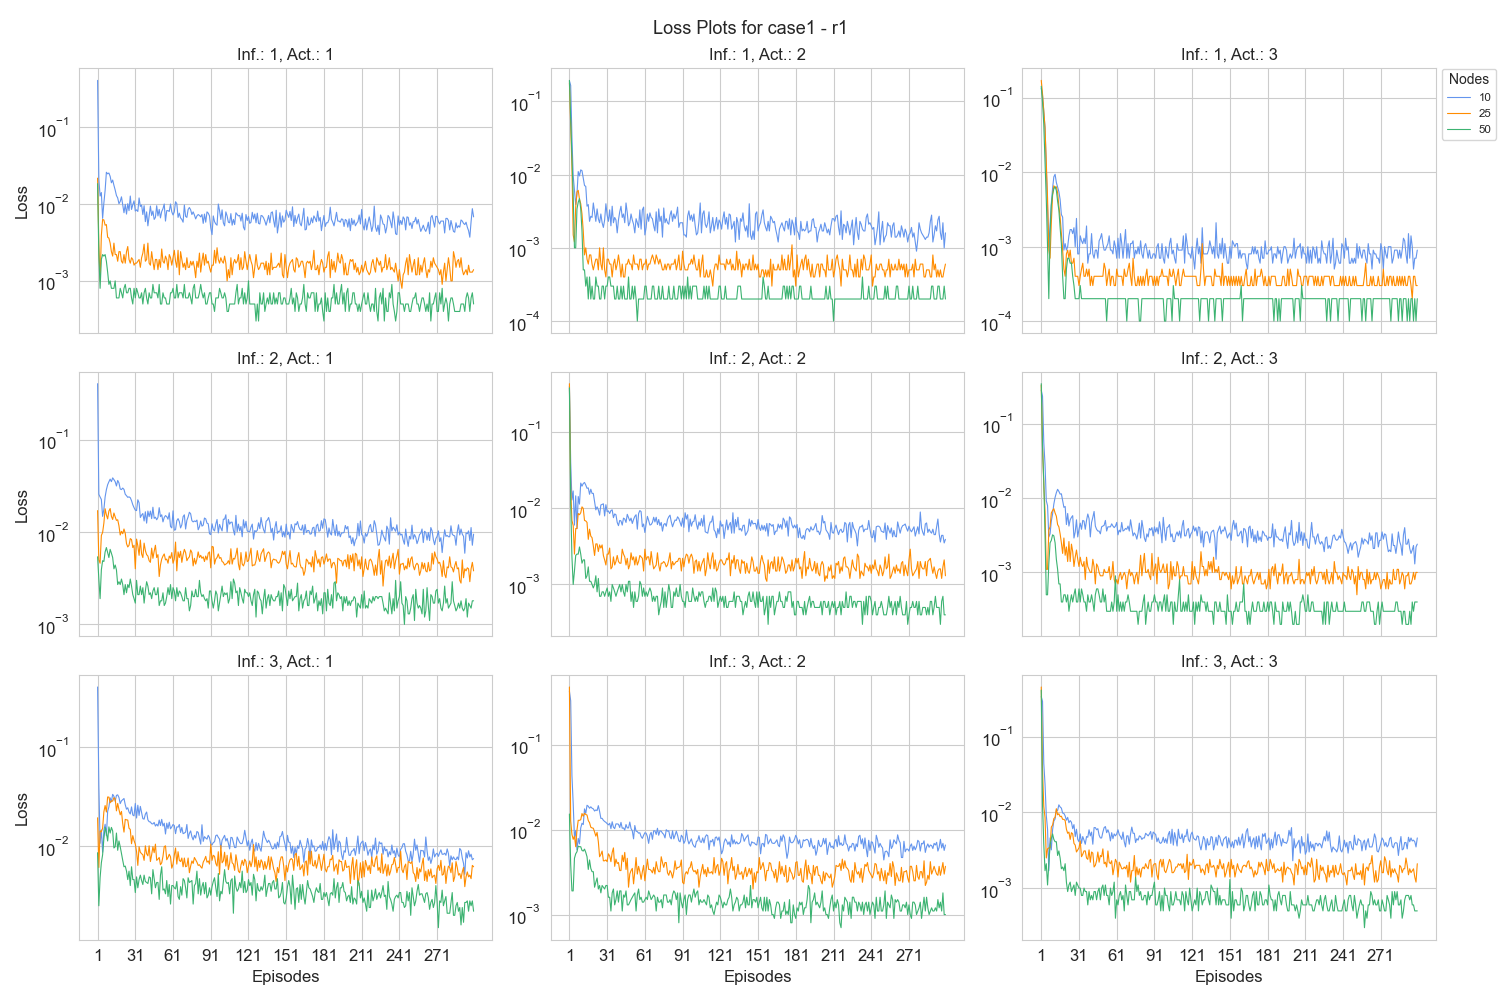}
    \caption{Case-1 using R1: Training MSE loss evolution for RL policy using GCN model across networks of 10 (blue), 25 (orange), and 50 (green) nodes, for varying initial misinformation sources (Inf.) and action budgets (Act.). Plotted on a logarithmic scale, the loss decreases over episodes, indicating improved policy performance and adaptation across network sizes.}
    \label{fig:gcn_c1r1_loss}
\end{figure}

\begin{figure}[!h]
    \centering
    \includegraphics[scale=0.34]{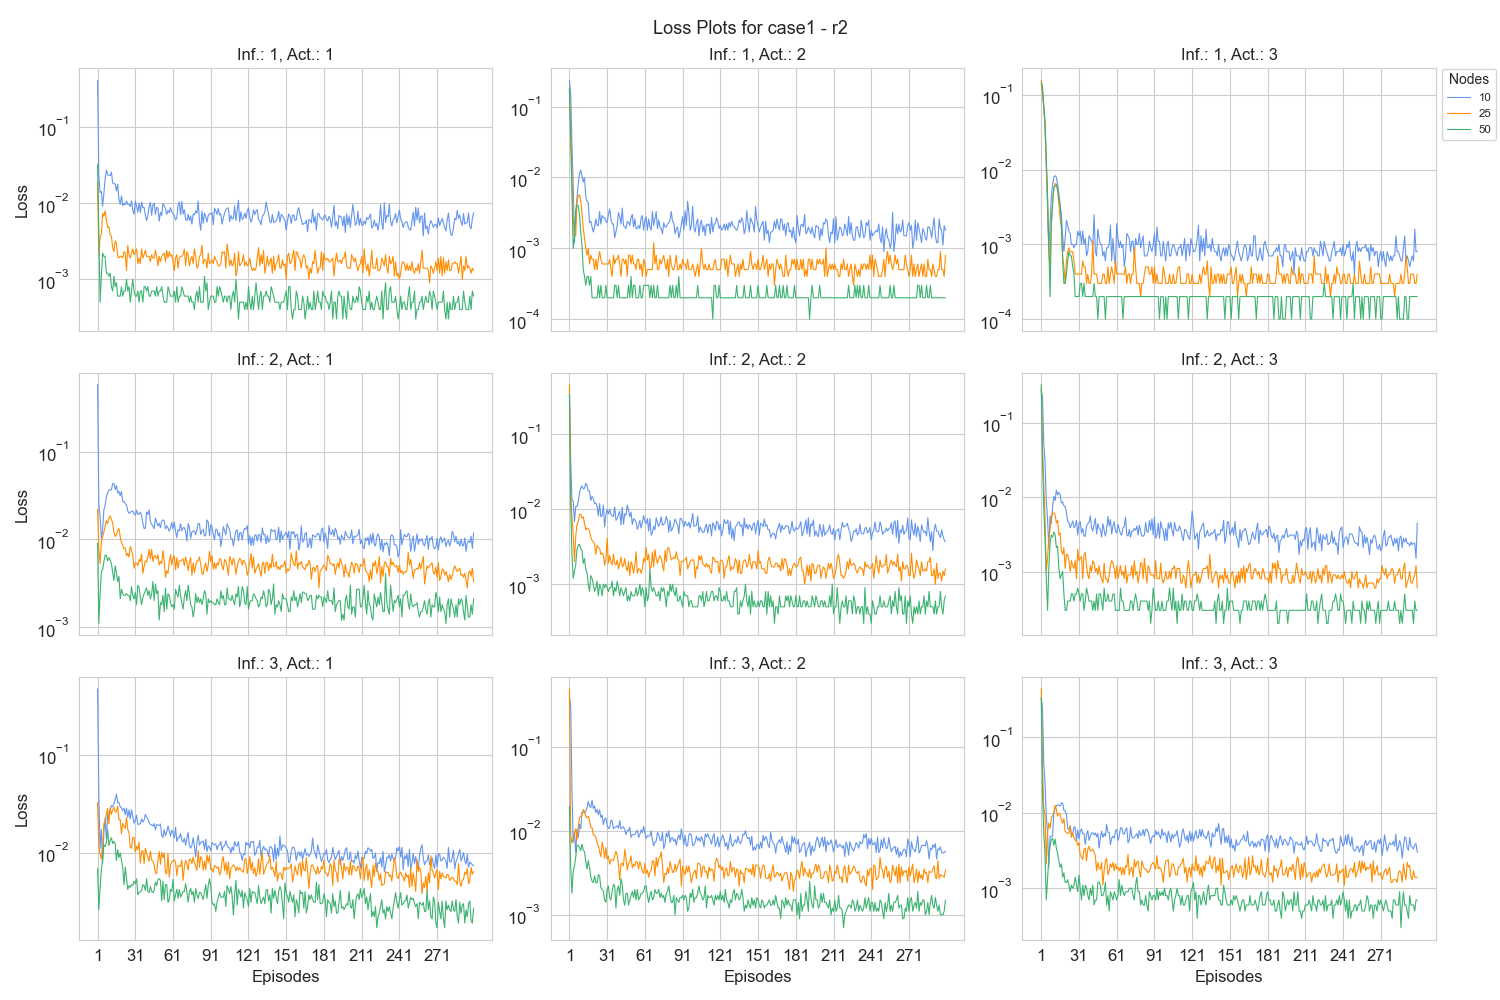}
    \caption{Case-1 using R2: Training MSE loss evolution for RL policy using GCN model across networks of 10 (blue), 25 (orange), and 50 (green) nodes, for varying initial misinformation sources (Inf.) and action budgets (Act.). Plotted on a logarithmic scale, the loss decreases over episodes, indicating improved policy performance and adaptation across network sizes.}
    \label{fig:gcn_c1r2_loss}
\end{figure}

\begin{figure}[!h]
    \centering
    \includegraphics[scale=0.34]{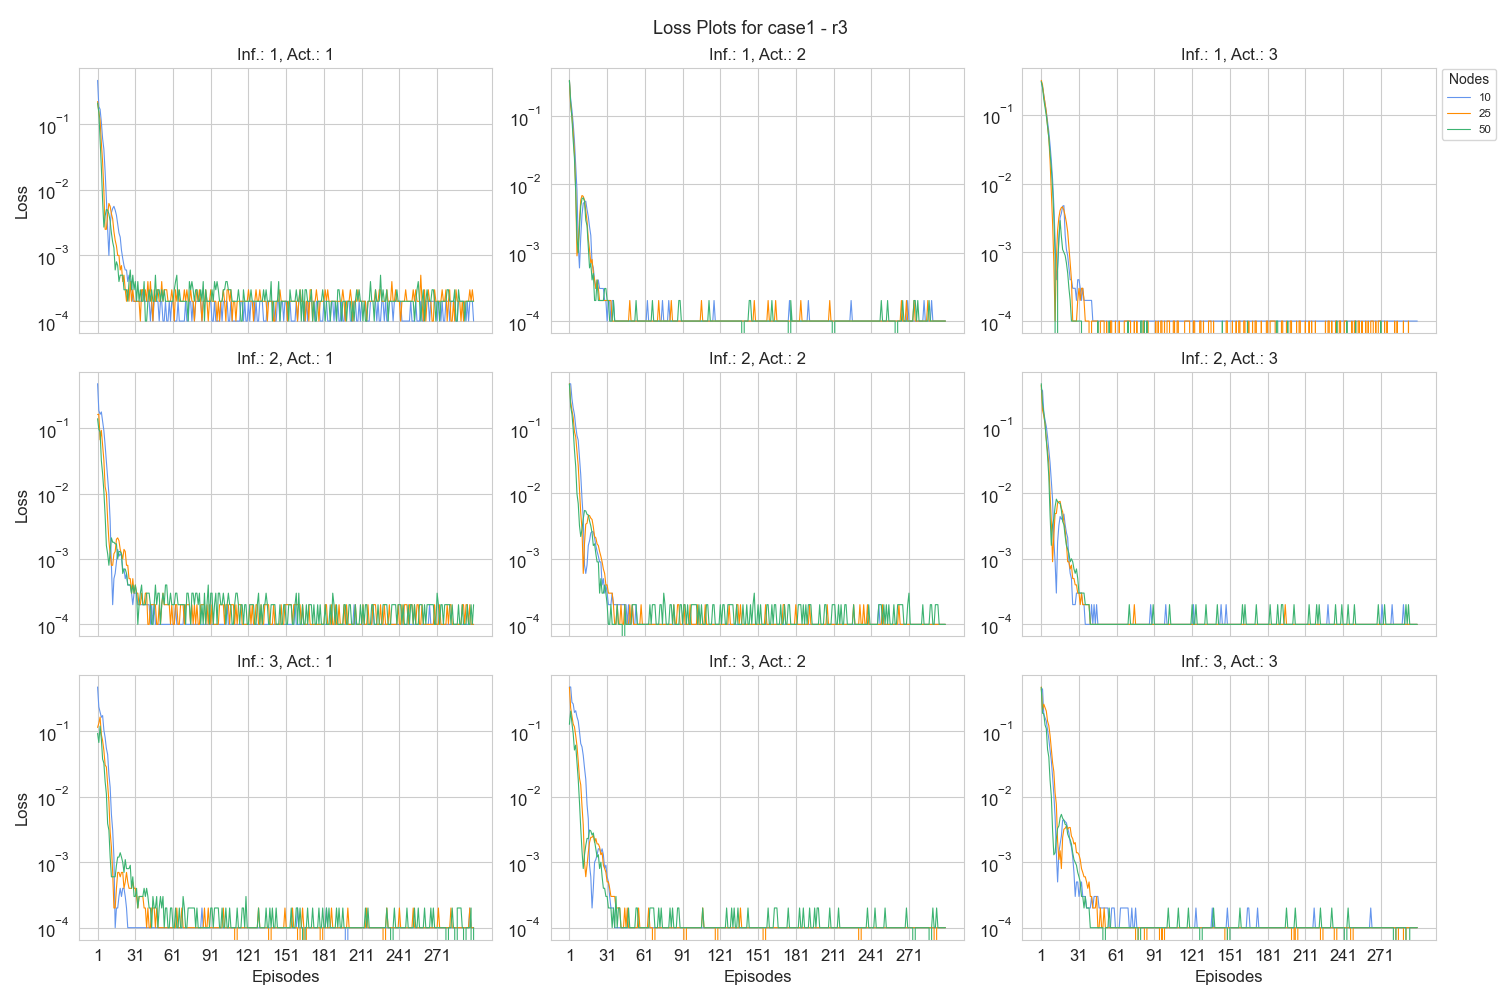}
    \caption{Case-1 using R3: Training MSE loss evolution for RL policy using GCN model across networks of 10 (blue), 25 (orange), and 50 (green) nodes, for varying initial misinformation sources (Inf.) and action budgets (Act.). Plotted on a logarithmic scale, the loss decreases over episodes, indicating improved policy performance and adaptation across network sizes.}
    \label{fig:gcn_c1r3_loss}
\end{figure}

\begin{figure}[!h]
    \centering
    \includegraphics[scale=0.34]{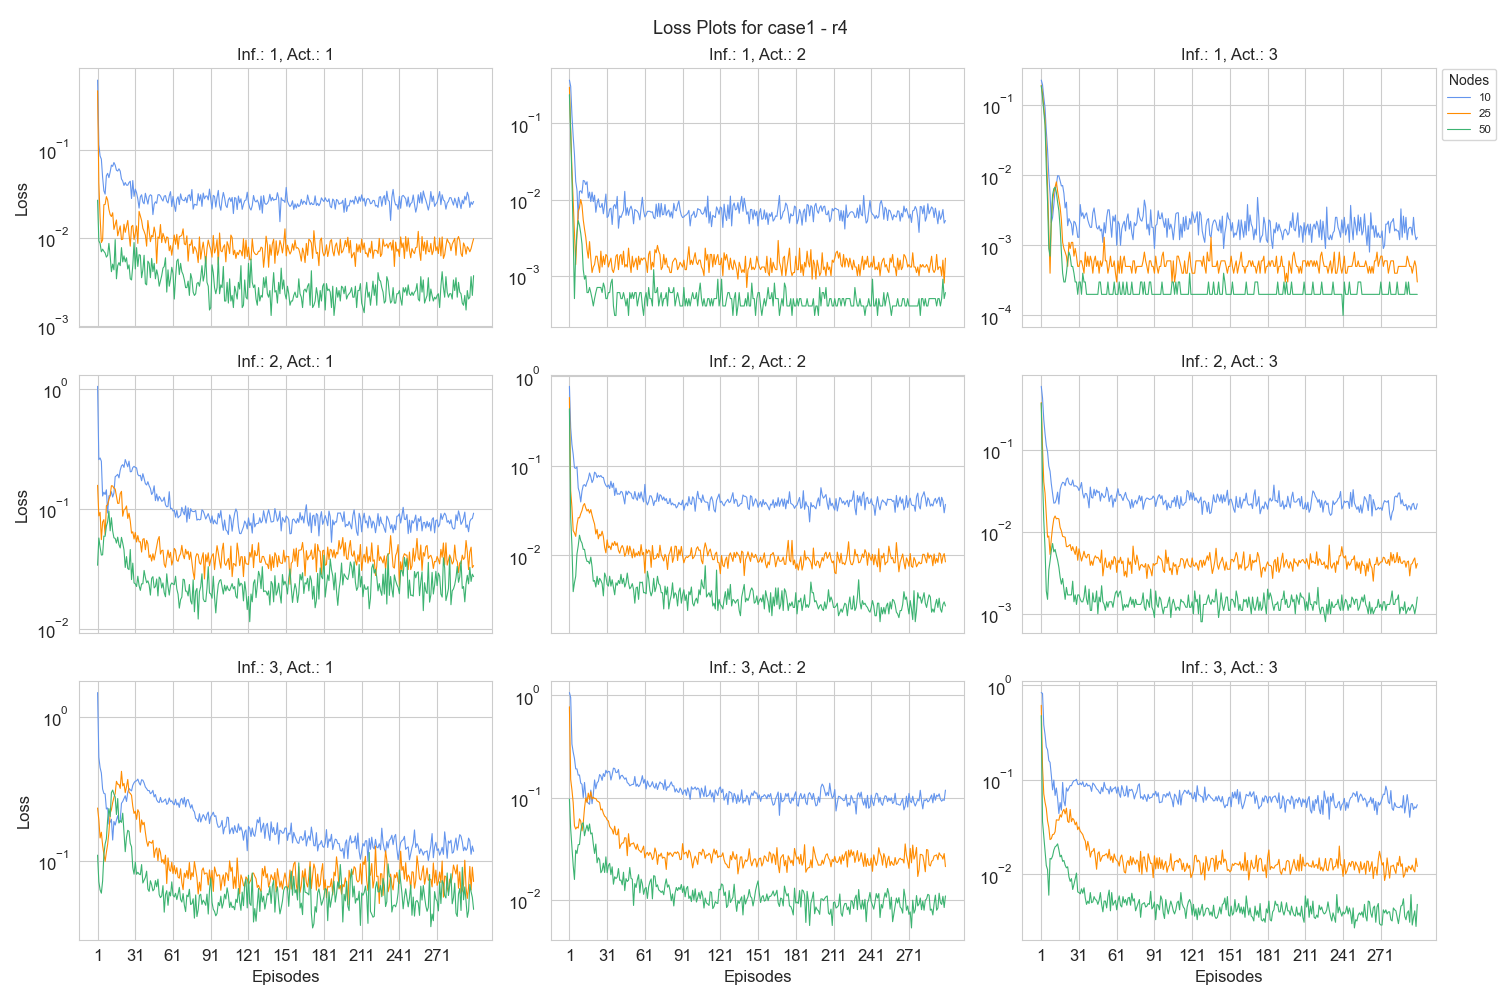}
    \caption{Case-1 using R4: Training MSE loss evolution for RL policy using GCN model across networks of 10 (blue), 25 (orange), and 50 (green) nodes, for varying initial misinformation sources (Inf.) and action budgets (Act.). Plotted on a logarithmic scale, the loss decreases over episodes, indicating improved policy performance and adaptation across network sizes.}
    \label{fig:gcn_c1r4_loss}
\end{figure}

%###########################

%###### Case 2 GCN Figures #######
\begin{figure}[!h]
    \centering
    \includegraphics[scale=0.34]{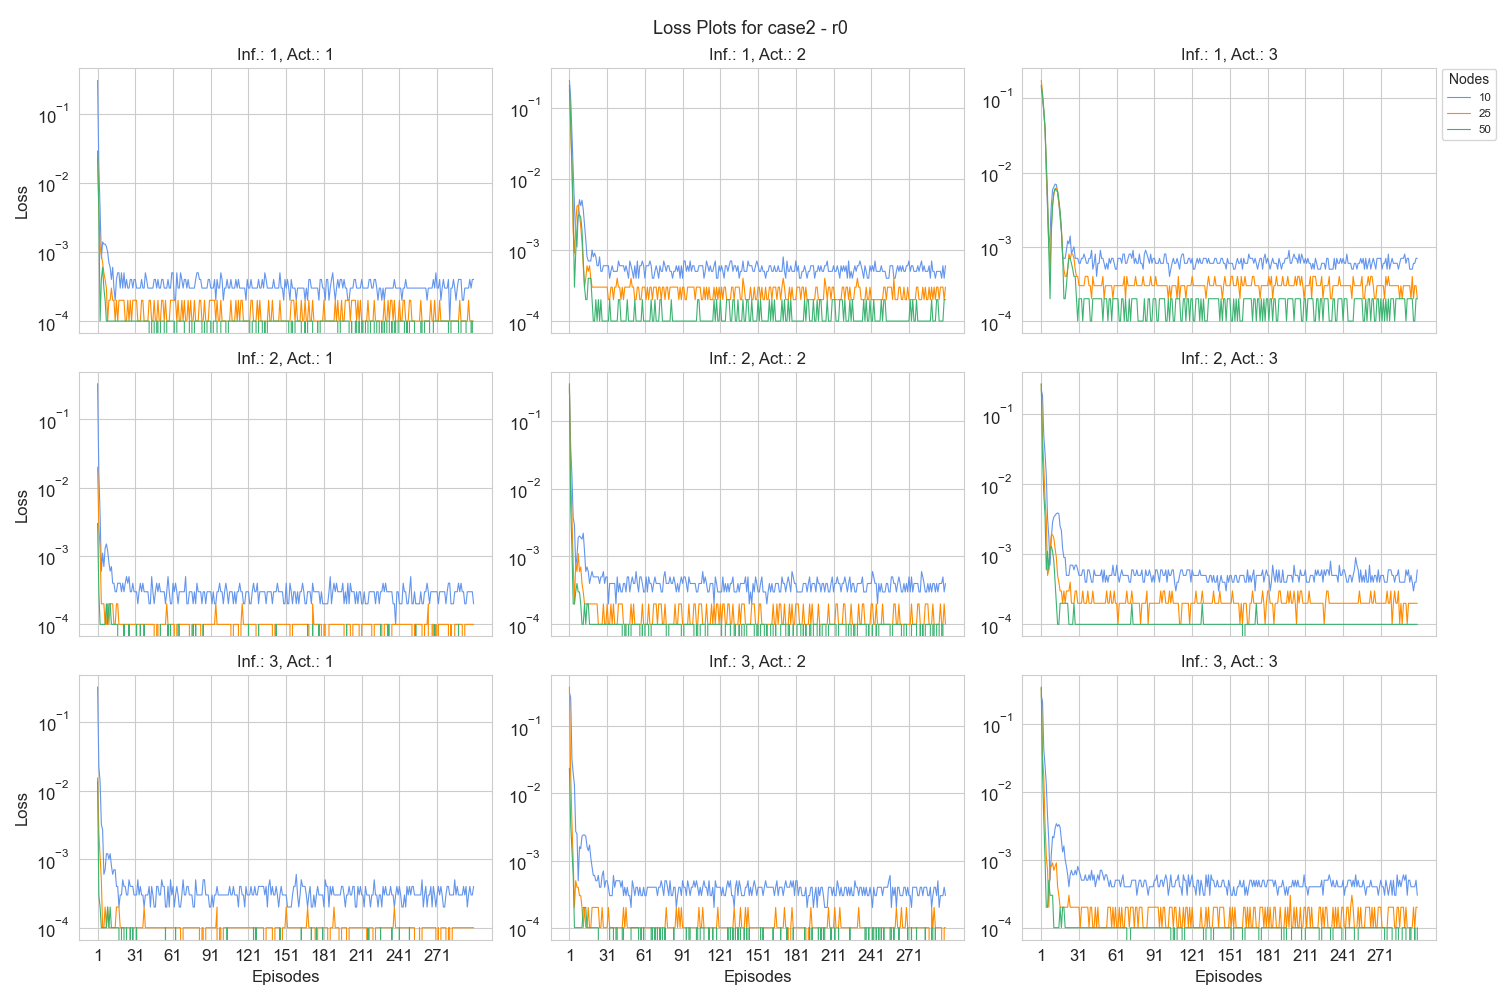}
    \caption{Case-2 using R0: Training MSE loss evolution for RL policy using GCN model across networks of 10 (blue), 25 (orange), and 50 (green) nodes, for varying initial misinformation sources (Inf.) and action budgets (Act.). Plotted on a logarithmic scale, the loss decreases over episodes, indicating improved policy performance and adaptation across network sizes.}
    \label{fig:gcn_c2r0_loss}
\end{figure}

\begin{figure}[!h]
    \centering
    \includegraphics[scale=0.34]{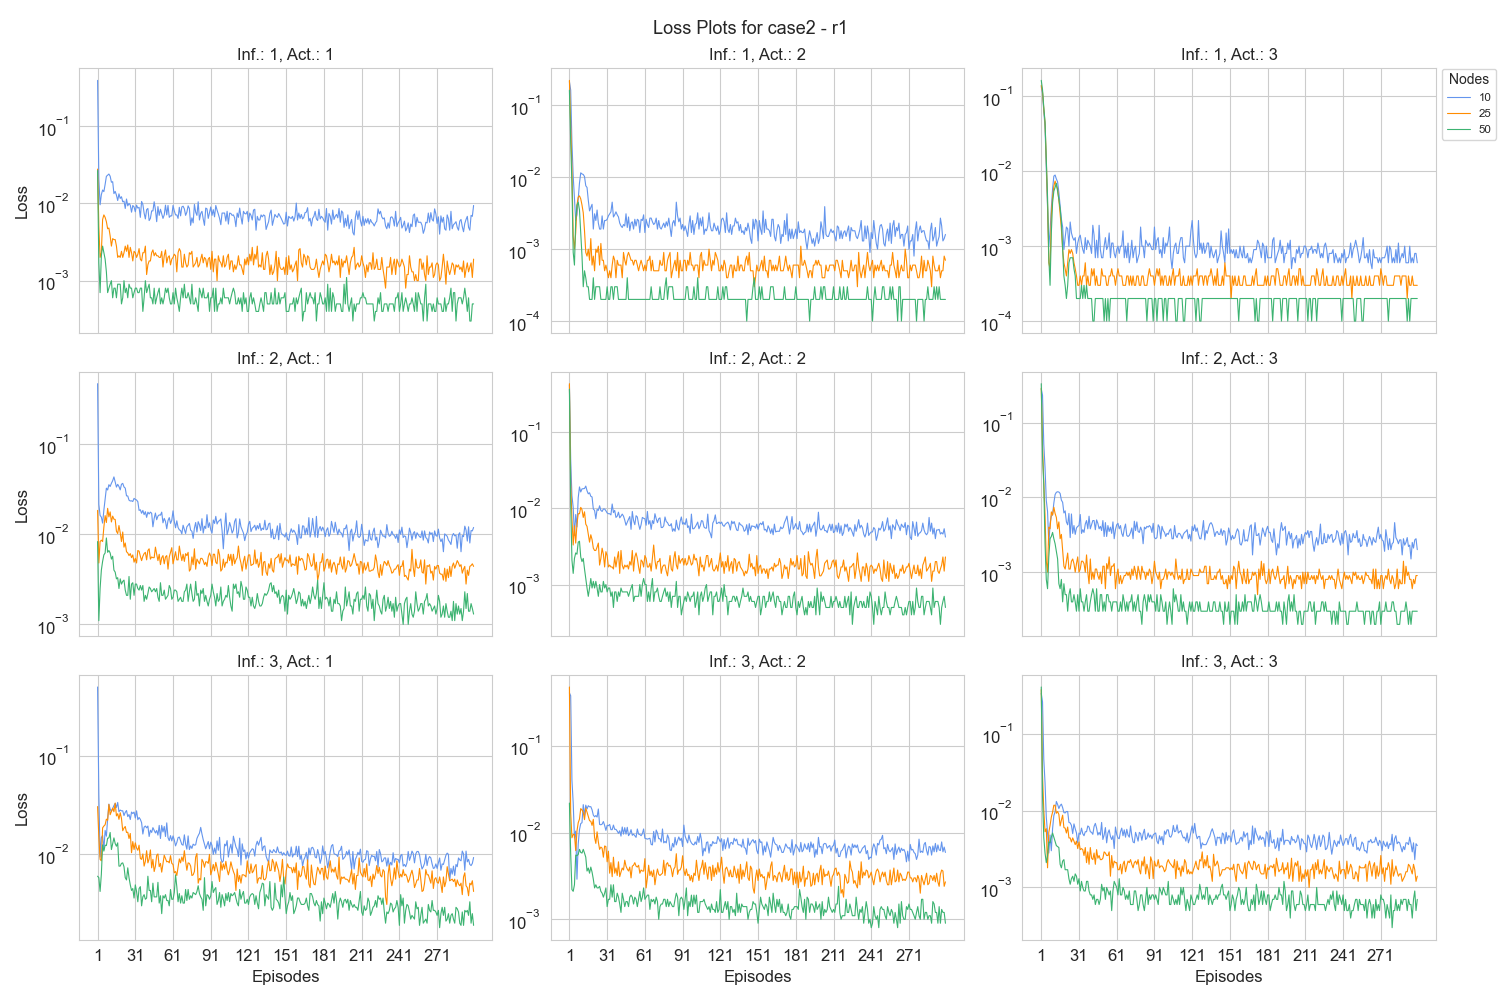}
    \caption{Case-2 using R1: Training MSE loss evolution for RL policy using GCN model across networks of 10 (blue), 25 (orange), and 50 (green) nodes, for varying initial misinformation sources (Inf.) and action budgets (Act.). Plotted on a logarithmic scale, the loss decreases over episodes, indicating improved policy performance and adaptation across network sizes.}
    \label{fig:gcn_c2r1_loss}
\end{figure}

\begin{figure}[!h]
    \centering
    \includegraphics[scale=0.34]{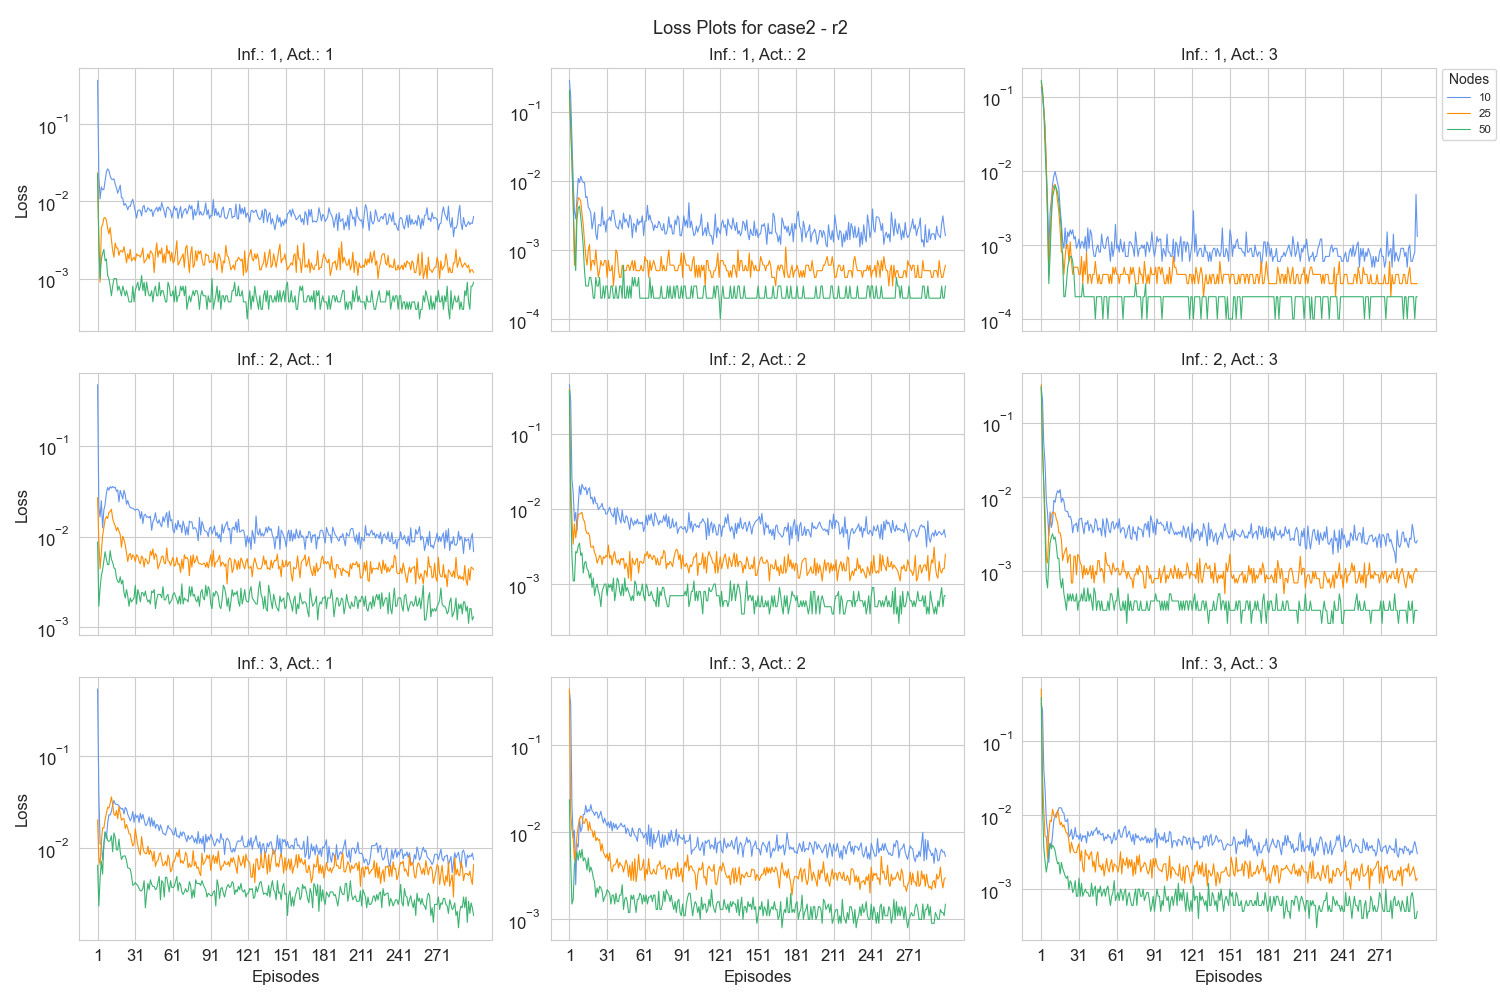}
    \caption{Case-2 using R2: Training MSE loss evolution for RL policy using GCN model across networks of 10 (blue), 25 (orange), and 50 (green) nodes, for varying initial misinformation sources (Inf.) and action budgets (Act.). Plotted on a logarithmic scale, the loss decreases over episodes, indicating improved policy performance and adaptation across network sizes.}
    \label{fig:gcn_c2r2_loss}
\end{figure}

\begin{figure}[!h]
    \centering
    \includegraphics[scale=0.34]{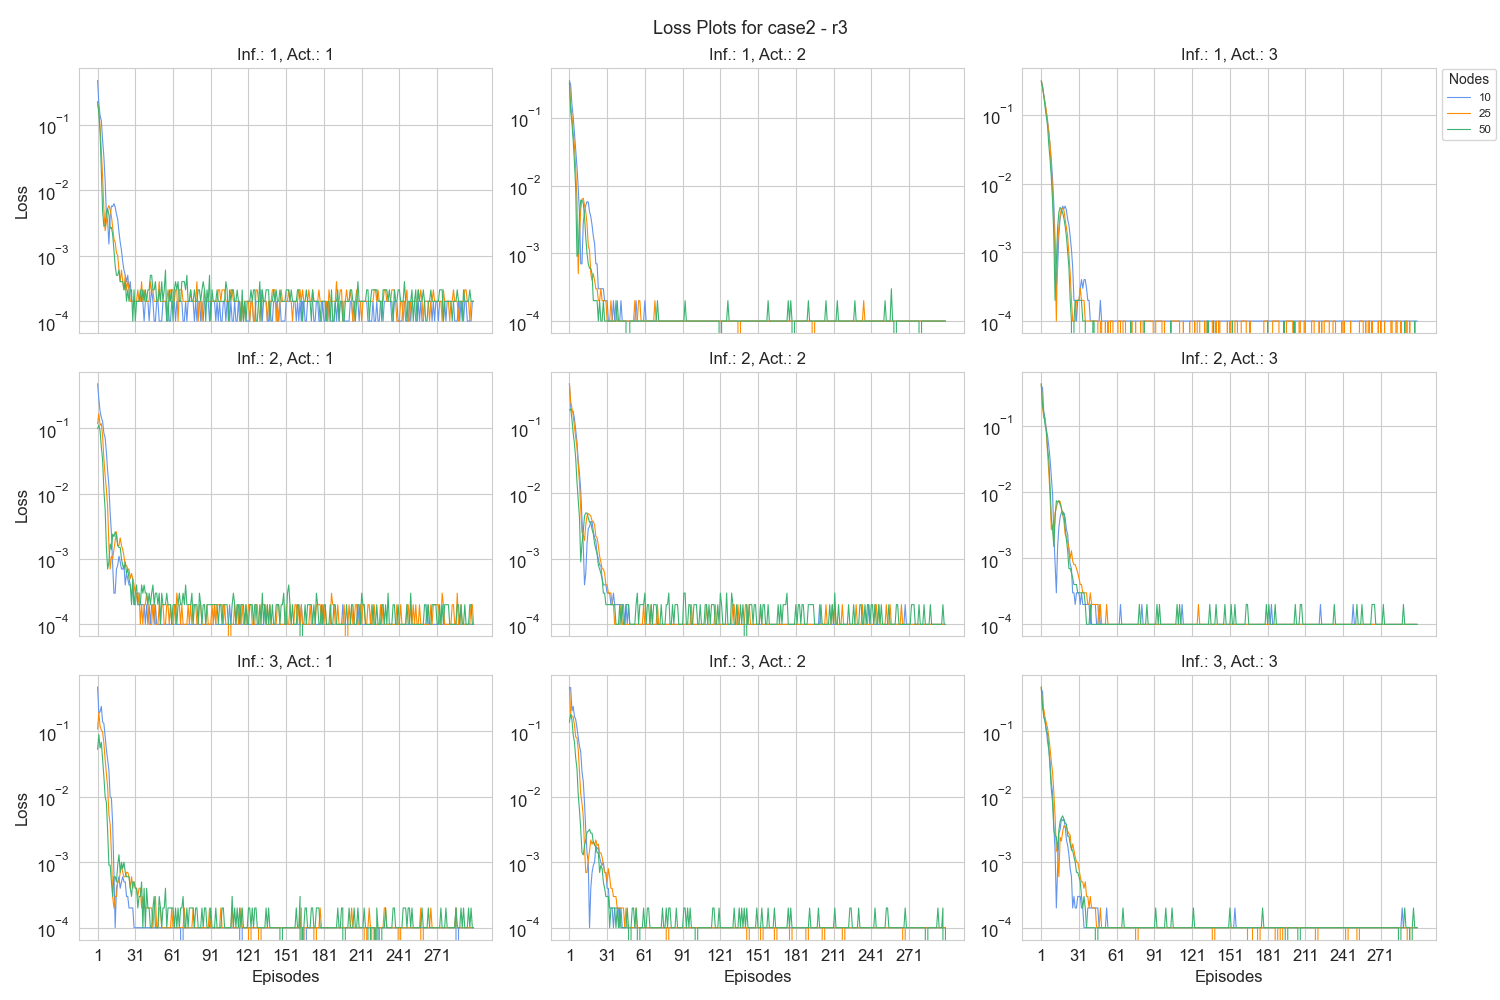}
    \caption{Case-2 using R3: Training MSE loss evolution for RL policy using GCN model across networks of 10 (blue), 25 (orange), and 50 (green) nodes, for varying initial misinformation sources (Inf.) and action budgets (Act.). Plotted on a logarithmic scale, the loss decreases over episodes, indicating improved policy performance and adaptation across network sizes.}
    \label{fig:gcn_c2r3_loss}
\end{figure}

\begin{figure}[!h]
    \centering
    \includegraphics[scale=0.34]{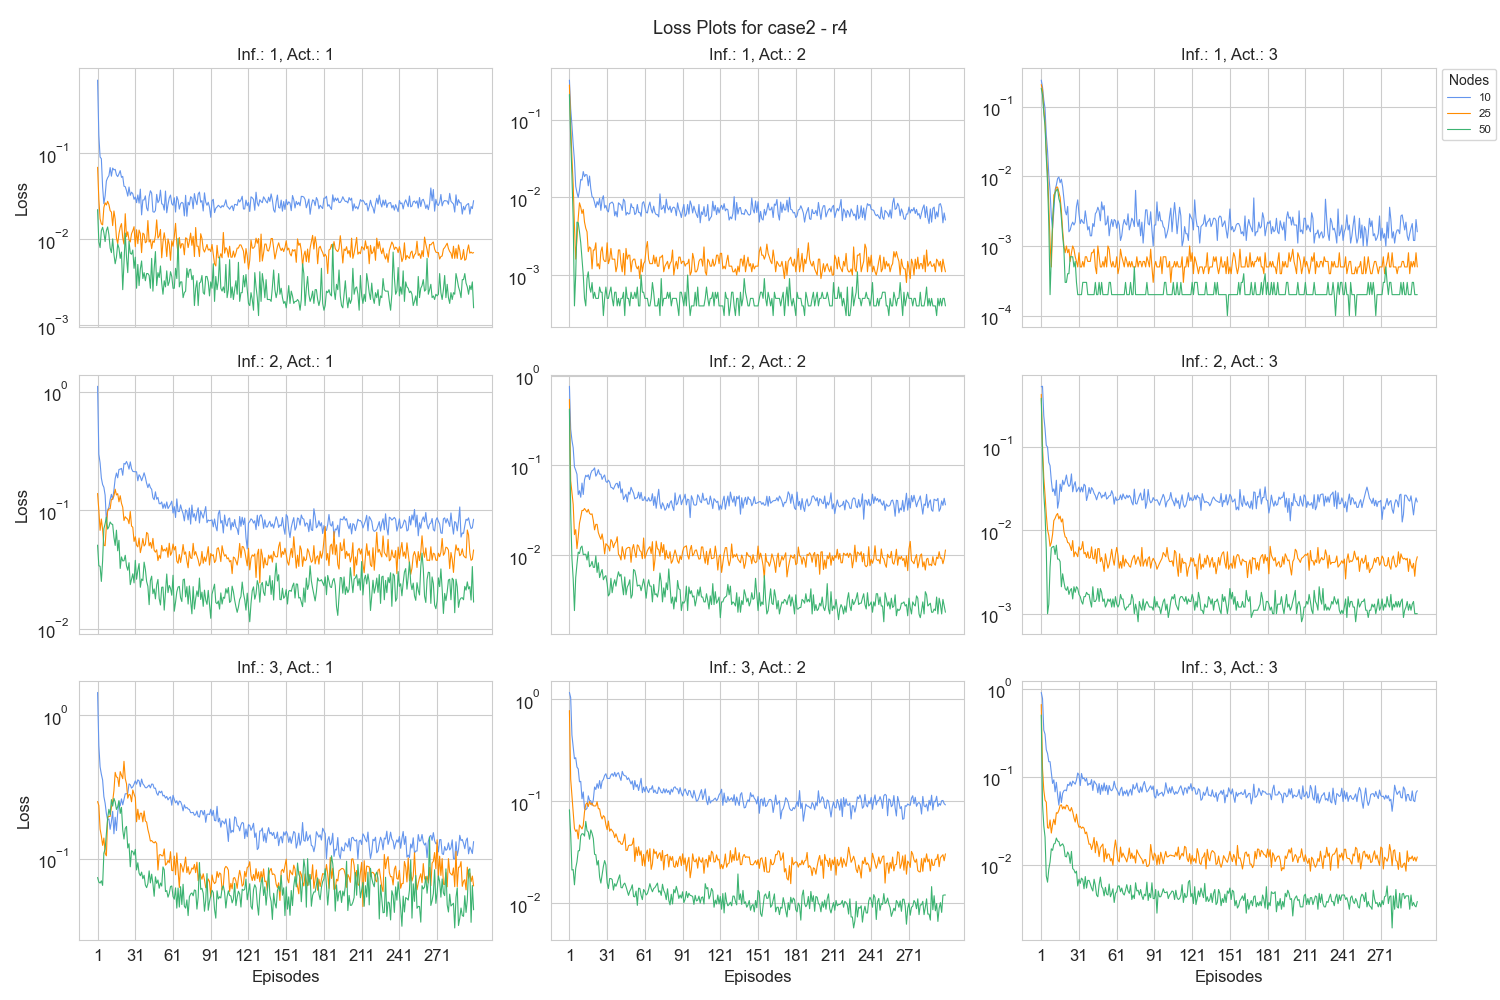}
    \caption{Case-2 using R4: Training MSE loss evolution for RL policy using GCN model across networks of 10 (blue), 25 (orange), and 50 (green) nodes, for varying initial misinformation sources (Inf.) and action budgets (Act.). Plotted on a logarithmic scale, the loss decreases over episodes, indicating improved policy performance and adaptation across network sizes.}
    \label{fig:gcn_c2r4_loss}
\end{figure}
%####################################
